# Supplementary material for: Bayesian Emulation of Grey-Box Multi-Model Ensembles Exploiting Known Interior Structure
Source: arXiv:2406.08367 source file (2025-05-02)
Supplement: Supplementary file 1 [file Structured-Emulation-with-Two-Sided-Truncation.tex]

\section{Structured Emulation with Two-Sided Truncation} \label{sec:Structured-Emulation-with-Two-Sided-Truncation}

In this appendix we present an alternative variant of structured emulation exploiting the known simulator behaviour from \cref{subsec:Emulators-Exploiting-Known-Simulator-Behaviour-for-NPV-Constituents} which uses a two-sided truncation, as presented in \cite[Sec.~3.3.2]{2022:Owen:PhD-Thesis}. It is unnecessary for the application to the \TNOChallengeWC{} in \cref{sec:Results}, but is utilised in another application described in \cite[Sec.~5.4.1 \& 5.8.1]{2022:Owen:PhD-Thesis}. In addition, we detail the truncated normal distribution equations used in both methodologies.

Estimation of the change points and extrapolation cut-offs remains as described in \cref{subsubsec:Structured-Emulation-Change-Points,subsubsec:Structured-Emulation-Extrapolation-Cut-Offs} respectively, as does the physical maximum constraint discussed in \ref{subsubsec:Structured-Emulation-Methodology}. A lower truncation, denoted by $a_i$, may also be imposed, for example, to represent the constraint that the WOPT and WWIT NPV constituents within a control interval must be non-negative ($a_i = 0$). Both constraints are utilised alongside the preliminary Bayes linear emulator in a modified classification step:
\begin{enumerate*}
	\item \textbf{Slope Region:} If $\dcp < \extrapco{jk}{t_i}$ \textbf{or} for the preliminary emulator \lword{$\E_{\boldFi^\prime}[\fid] - 3 \sqrt{\Var_{\boldFi^\prime}[\fid]} > \dcp \cdot \Delta t_i$}, then collapse the emulator such that for the structured emulator $\E_{\boldFi^\prime}[\fid] = \dcp \cdot \Delta t_i$ with fixed maximum absolute errors of size $\delta_i$.% This corresponds to when the output is strongly believed to be in the slope region.
	
%	\item \textbf{Uncertain Region around Change Point:} As for the upper truncation version above, if for the preliminary emulator $\E_{\boldFi^\prime}[\fid] - 3 \sqrt{\Var_{\boldFi^\prime}[\fid]} \leq \dcp \cdot \Delta t_i < \E_{\boldFi^\prime}[\fid] + 3 \sqrt{\Var_{\boldFi^\prime}[\fid]}$, \textbf{or} if the additional criterion of $\E_{\boldFi^\prime}[\fid] - 3 \sqrt{\Var_{\boldFi^\prime}[\fid]} <  a_i$ \textbf{whilst} $\E_{\boldFi^\prime}[\fid] + 3 \sqrt{\Var_{\boldFi^\prime}[\fid]} \leq \dcp \cdot \Delta t_i$, a truncated GP emulator is evaluated. The mean and variance are determined by \cref{eq:Truncated-normal-distribution-mean,eq:Truncated-normal-distribution-variance} respectively and are computed as for the upper truncation version above noting the change in the lower truncation bound $a_i$ and hence $\alpha_i$. This form of emulation is used in the uncertain region around the true location of the change point.
	\item \textbf{Intermediate Region:} As for the upper truncation version, if the preliminary emulator satisfies $\E_{\boldFi^\prime}[\fid] - 3 \sqrt{\Var_{\boldFi^\prime}[\fid]} \leq \dcp \cdot \Delta t_i < \E_{\boldFi^\prime}[\fid] + 3 \sqrt{\Var_{\boldFi^\prime}[\fid]}$, \textbf{or} if the additional criterion of $\E_{\boldFi^\prime}[\fid] - 3 \sqrt{\Var_{\boldFi^\prime}[\fid]} <  a_i$ \textbf{whilst} $\E_{\boldFi^\prime}[\fid] + 3 \sqrt{\Var_{\boldFi^\prime}[\fid]} \leq \dcp \cdot \Delta t_i$, a truncated GP emulator is evaluated. The mean and variance are determined by \cref{eq:Truncated-normal-distribution-mean,eq:Truncated-normal-distribution-variance} respectively.% This form of emulation is used in the uncertain region around the true location of the change point.
	
	\item \textbf{Plateau Region:} In all other cases where $\E_{\boldFi^\prime}[\fid] - 3 \sqrt{\Var_{\boldFi^\prime}[\fid]} \geq a_i$ \textbf{and} $\E_{\boldFi^\prime}[\fid] + 3 \sqrt{\Var_{\boldFi^\prime}[\fid]} \leq \dcp \cdot \Delta t_i$, use the preliminary emulator .% This corresponds to when the output is strongly believed to be in the plateau region.
\end{enumerate*}

The structured emulation methodology utilises a truncated Gaussian process (truncated GP) emulator for which the mean and variance are determined by \cref{eq:Truncated-normal-distribution-mean,eq:Truncated-normal-distribution-variance} respectively \cite{1994:Johnson:Continuous-Univariate-Distributions-Vol-1}, where $\phi(\cdot)$ and $\Phi(\cdot)$ represent the probability density and cumulative distribution functions respectively of a standard normal distribution. These are computed assuming a preliminary Gaussian process emulator with posterior mean and variance, abbreviated to $\mu_i$ and $\sigma_i^2$ respectively, equal to the computed adjusted expectation and variance, and truncation bounds $a_i$ and $b_i = \dcp \cdot \Delta t_i$, with $\alpha_i = \frac{a_i - \mu_i}{\sigma_i}$, and $\beta_i = \frac{b_i - \mu_i}{\sigma_i}$. This form of emulation is used in the intermediate uncertain region around the change point true location.
\begin{align}
	\E_{\boldFi^\prime}[\fid \mid a_i < \fid < b_i] &{} = \mu_i + \sigma \dfrac{\phi(\alpha_i) - \phi(\beta_i)}{\Phi(\beta_i) - \Phi(\alpha_i)} \label{eq:Truncated-normal-distribution-mean} \\
	\Var_{\boldFi^\prime}[\fid \mid a_i < \fid < b_i] &{} = \sigma_i^2 \left[ 1 + \dfrac{\alpha_i \phi(\alpha_i) - \beta_i \phi(\beta_i)}{\Phi(\beta_i) - \Phi(\alpha_i)} - \left( \dfrac{\phi(\alpha_i) - \phi(\beta_i)}{\Phi(\beta_i) - \Phi(\alpha_i)} \right)^2 \right] \label{eq:Truncated-normal-distribution-variance}
\end{align}

%%% Notes %%%
%Add discussion of structured emulation with two-sided truncation. This builds on the methodology in \cref{subsec:Emulators-Exploiting-Known-Simulator-Behaviour-for-NPV-Constituents} and is an alternative to \cref{subsubsec:Structured-Emulation-Methodology}.
%
%Include the truncated normal distribution equations.
