# Supplementary material for: Bayesian Emulation of Grey-Box Multi-Model Ensembles Exploiting Known Interior Structure
Source: arXiv:2406.08367 source file (2025-05-02)

# FOPT for OLYMPUS\_1

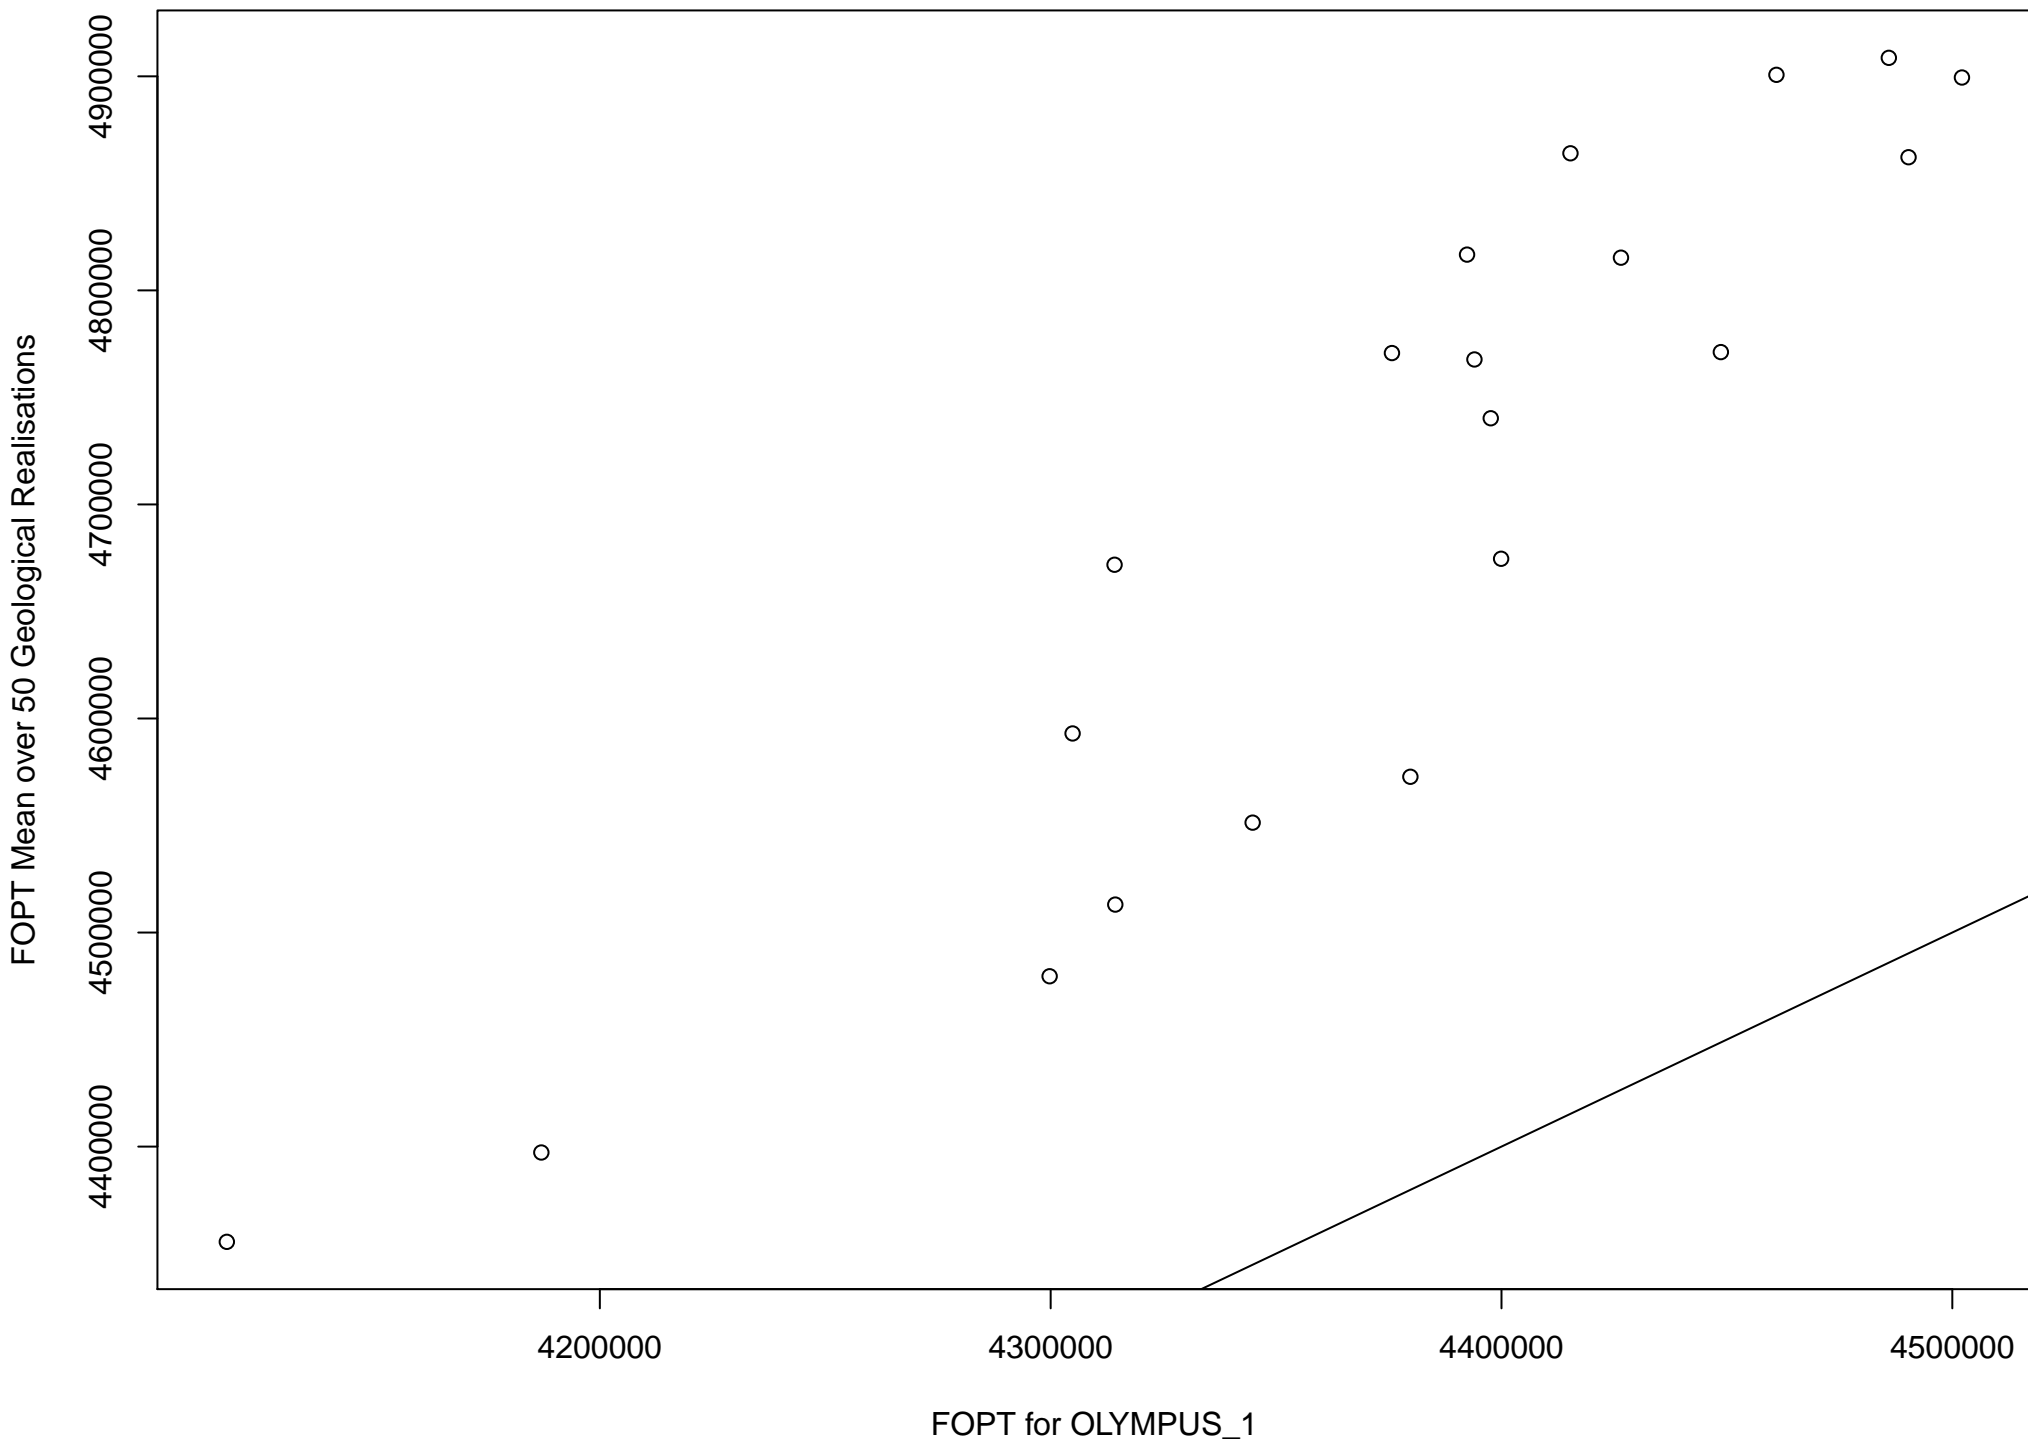

FOPT for OLYMPUS\_2

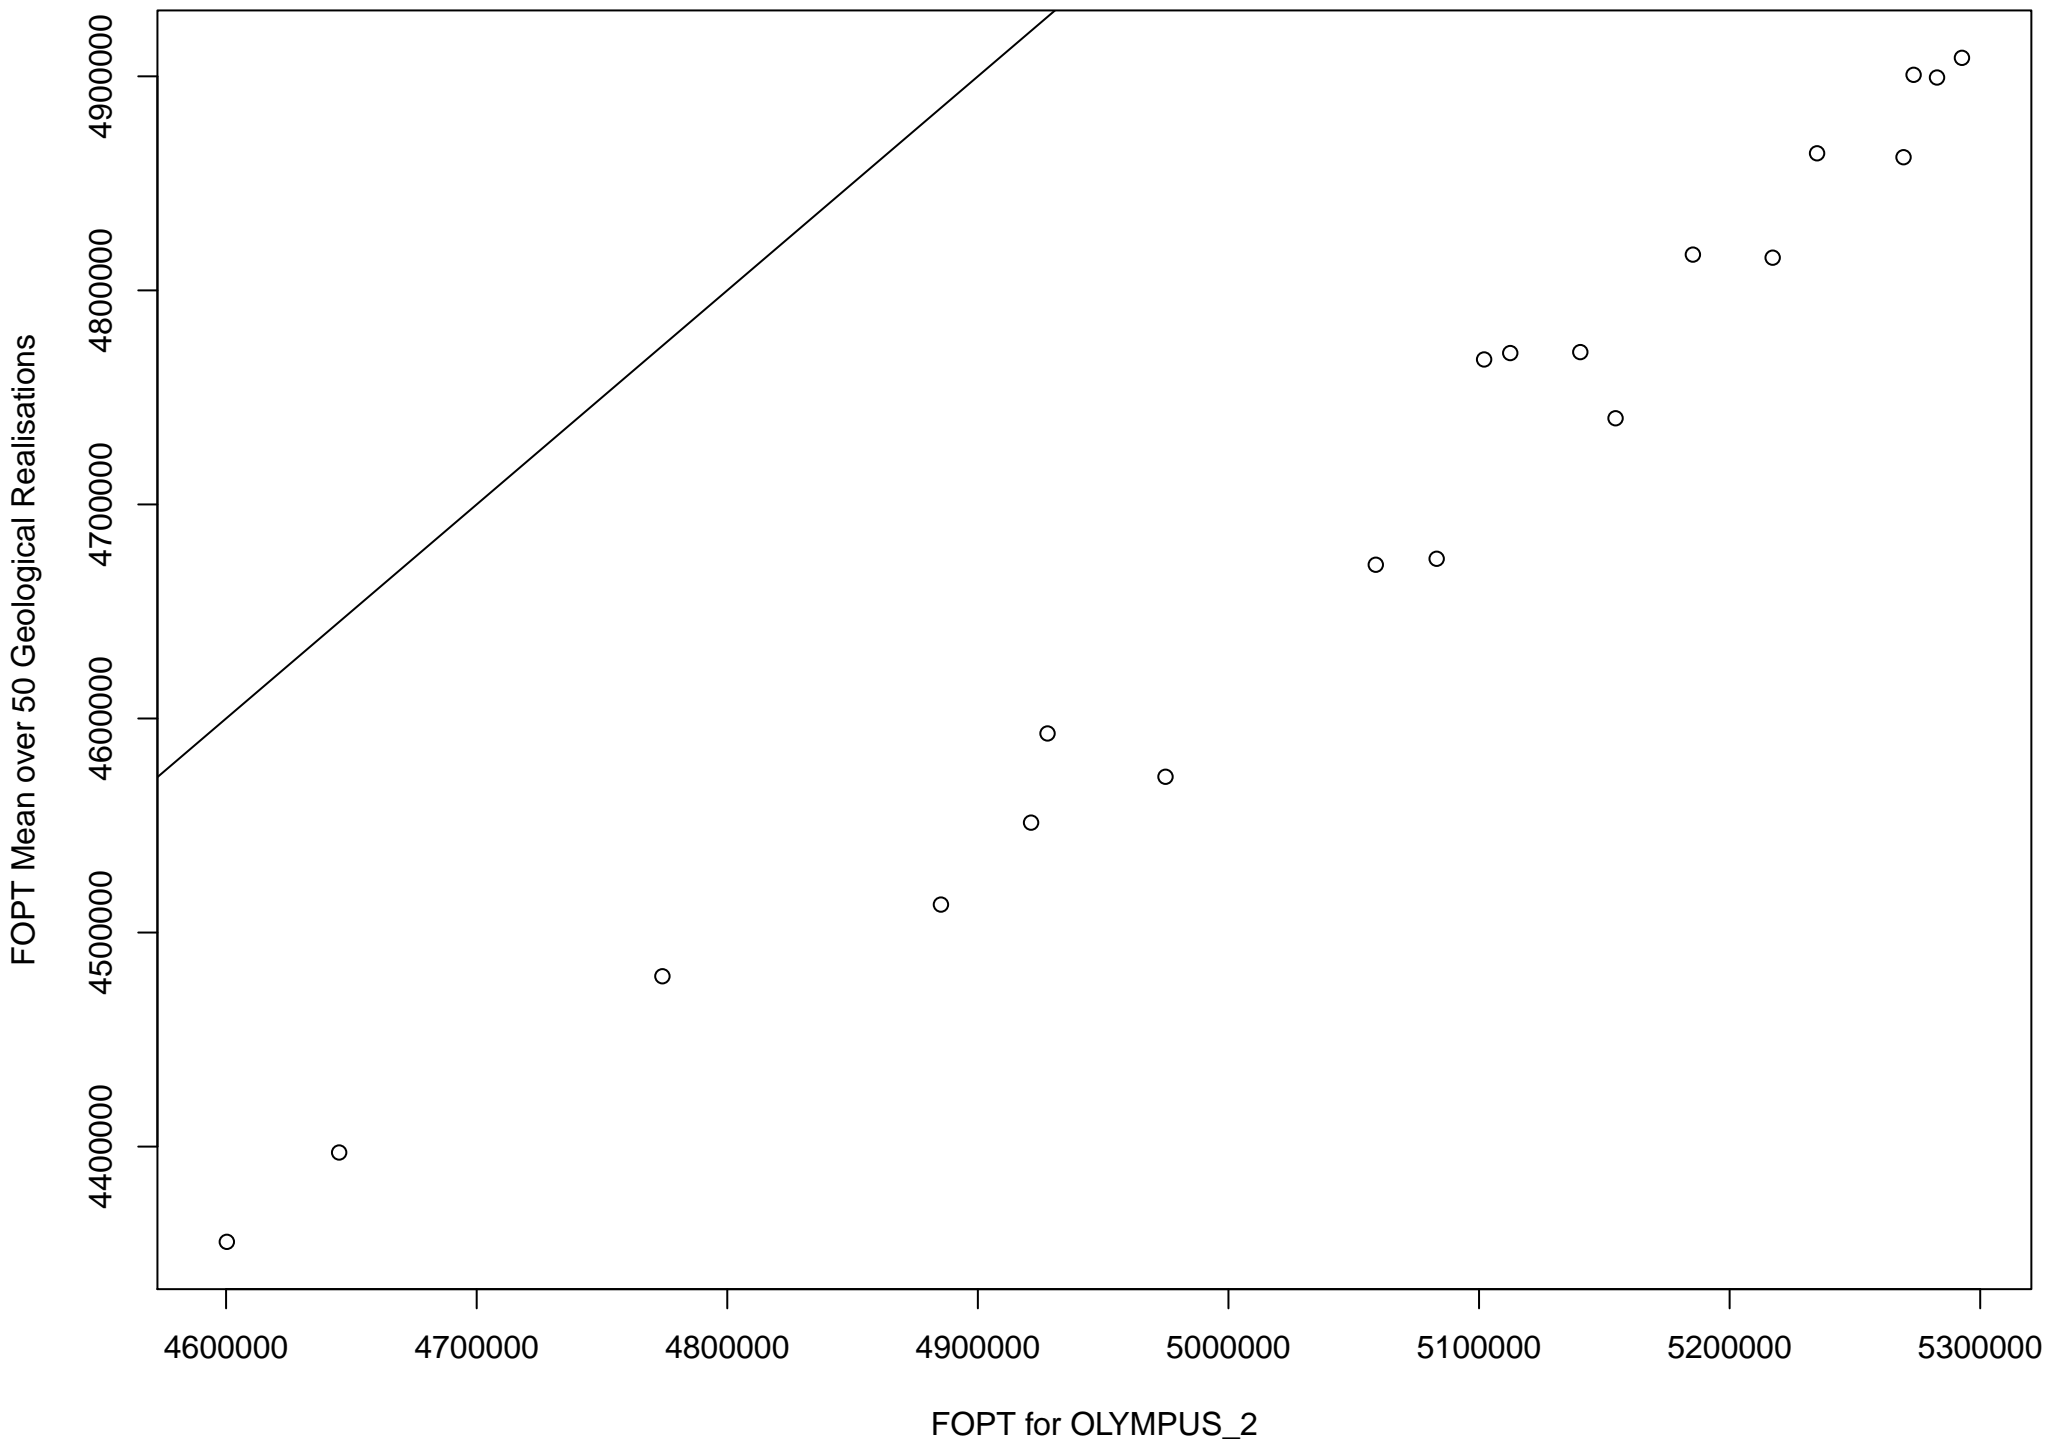

FOPT for OLYMPUS\_3

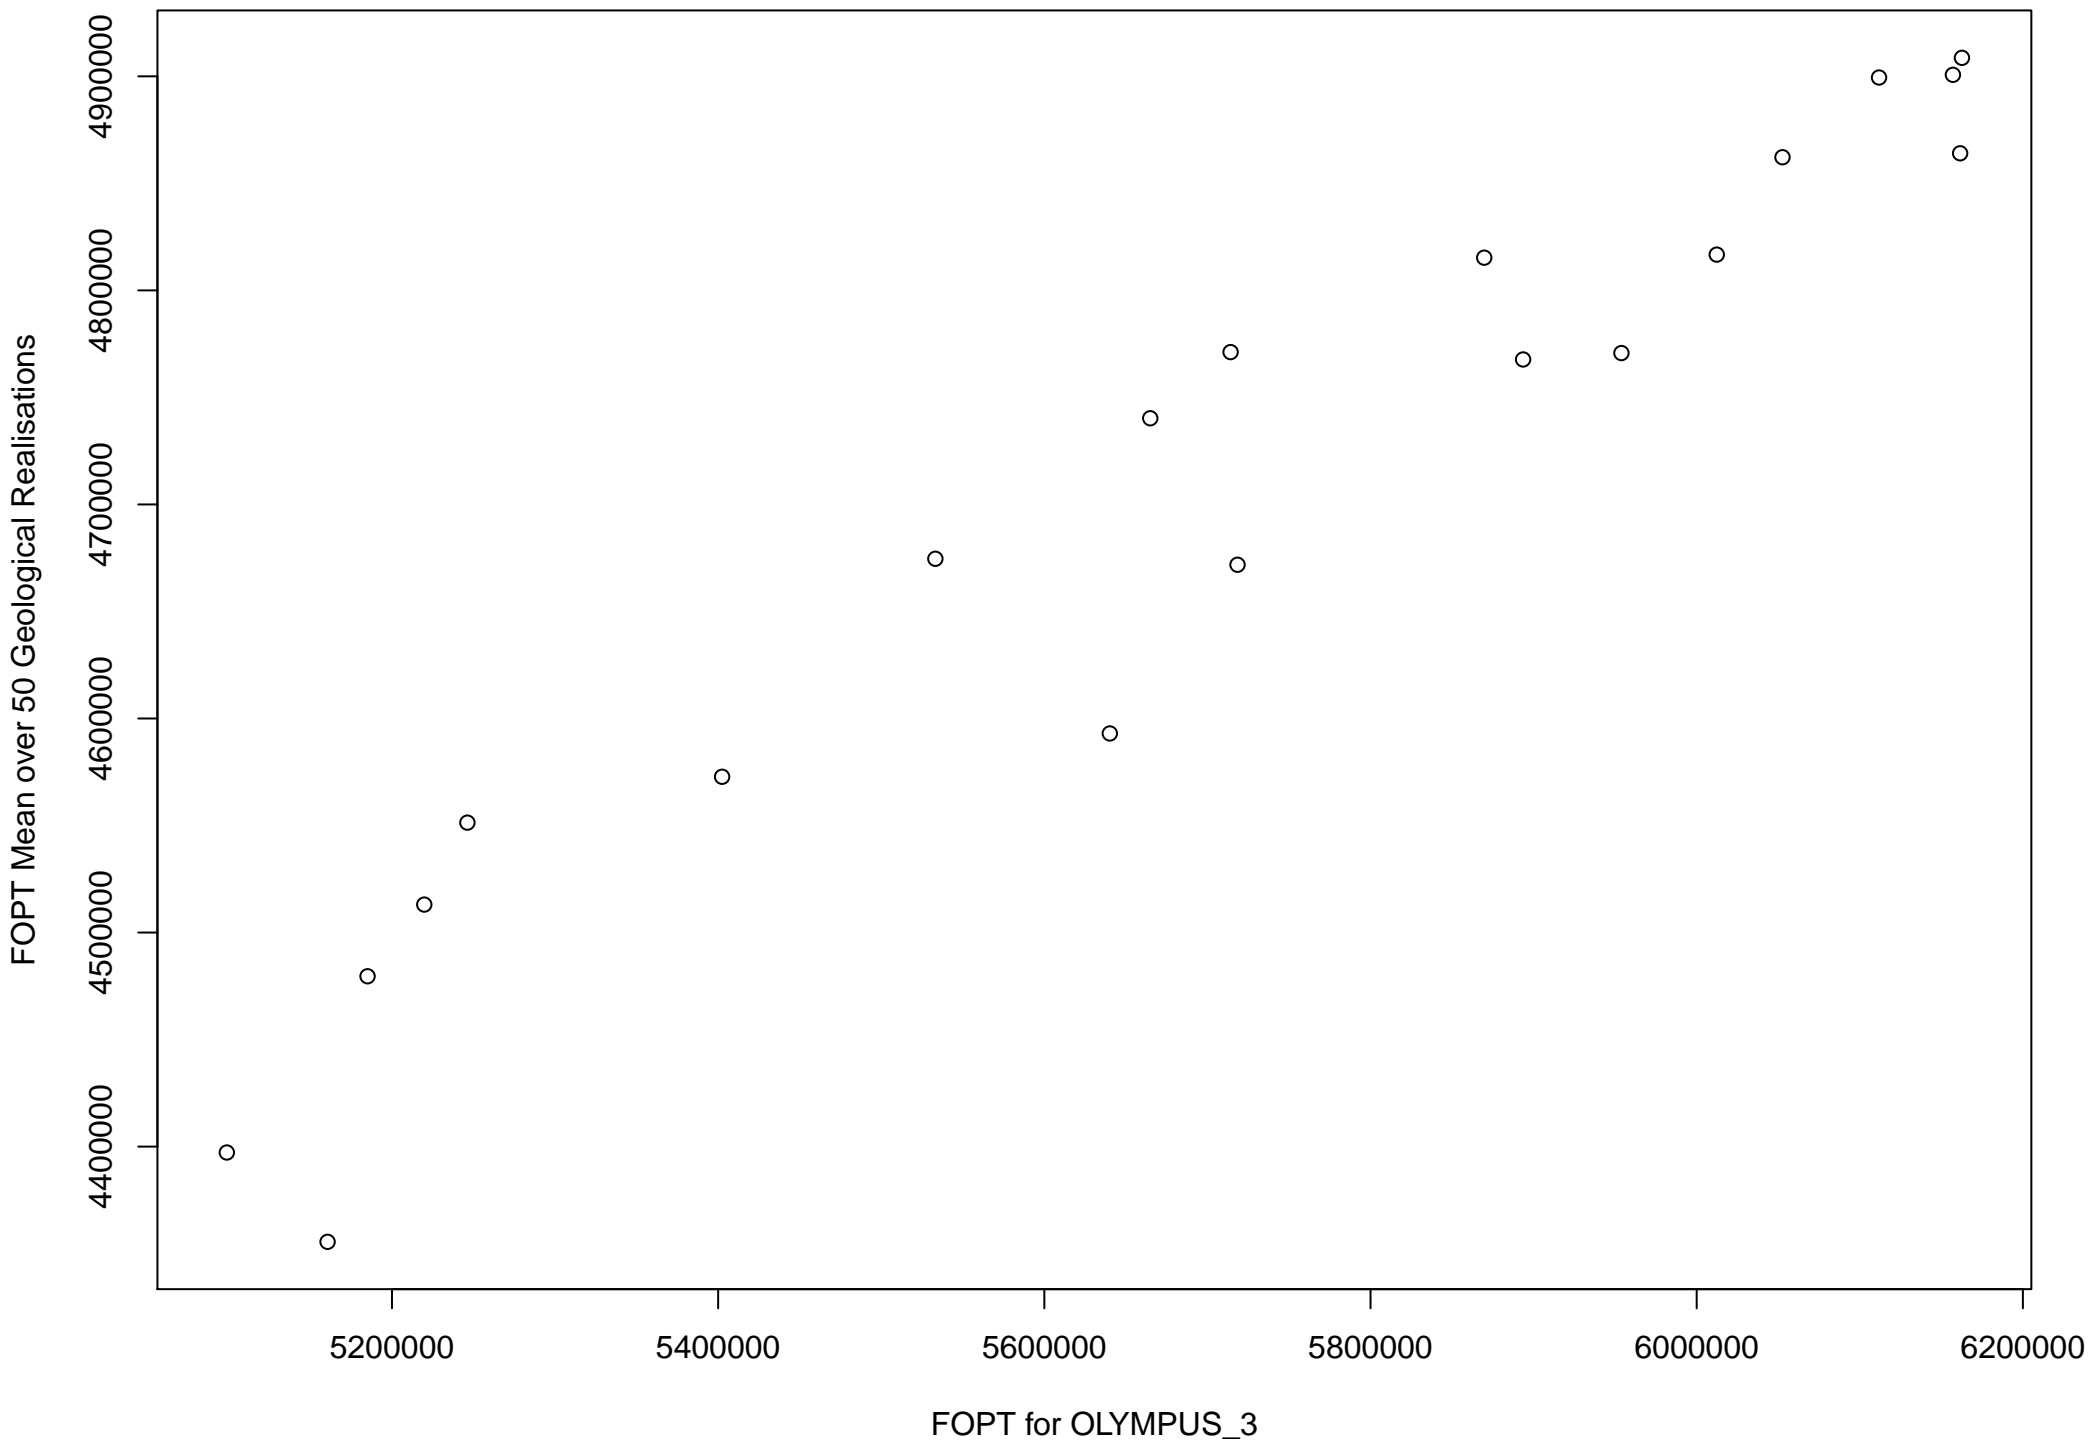

FOPT for OLYMPUS\_4

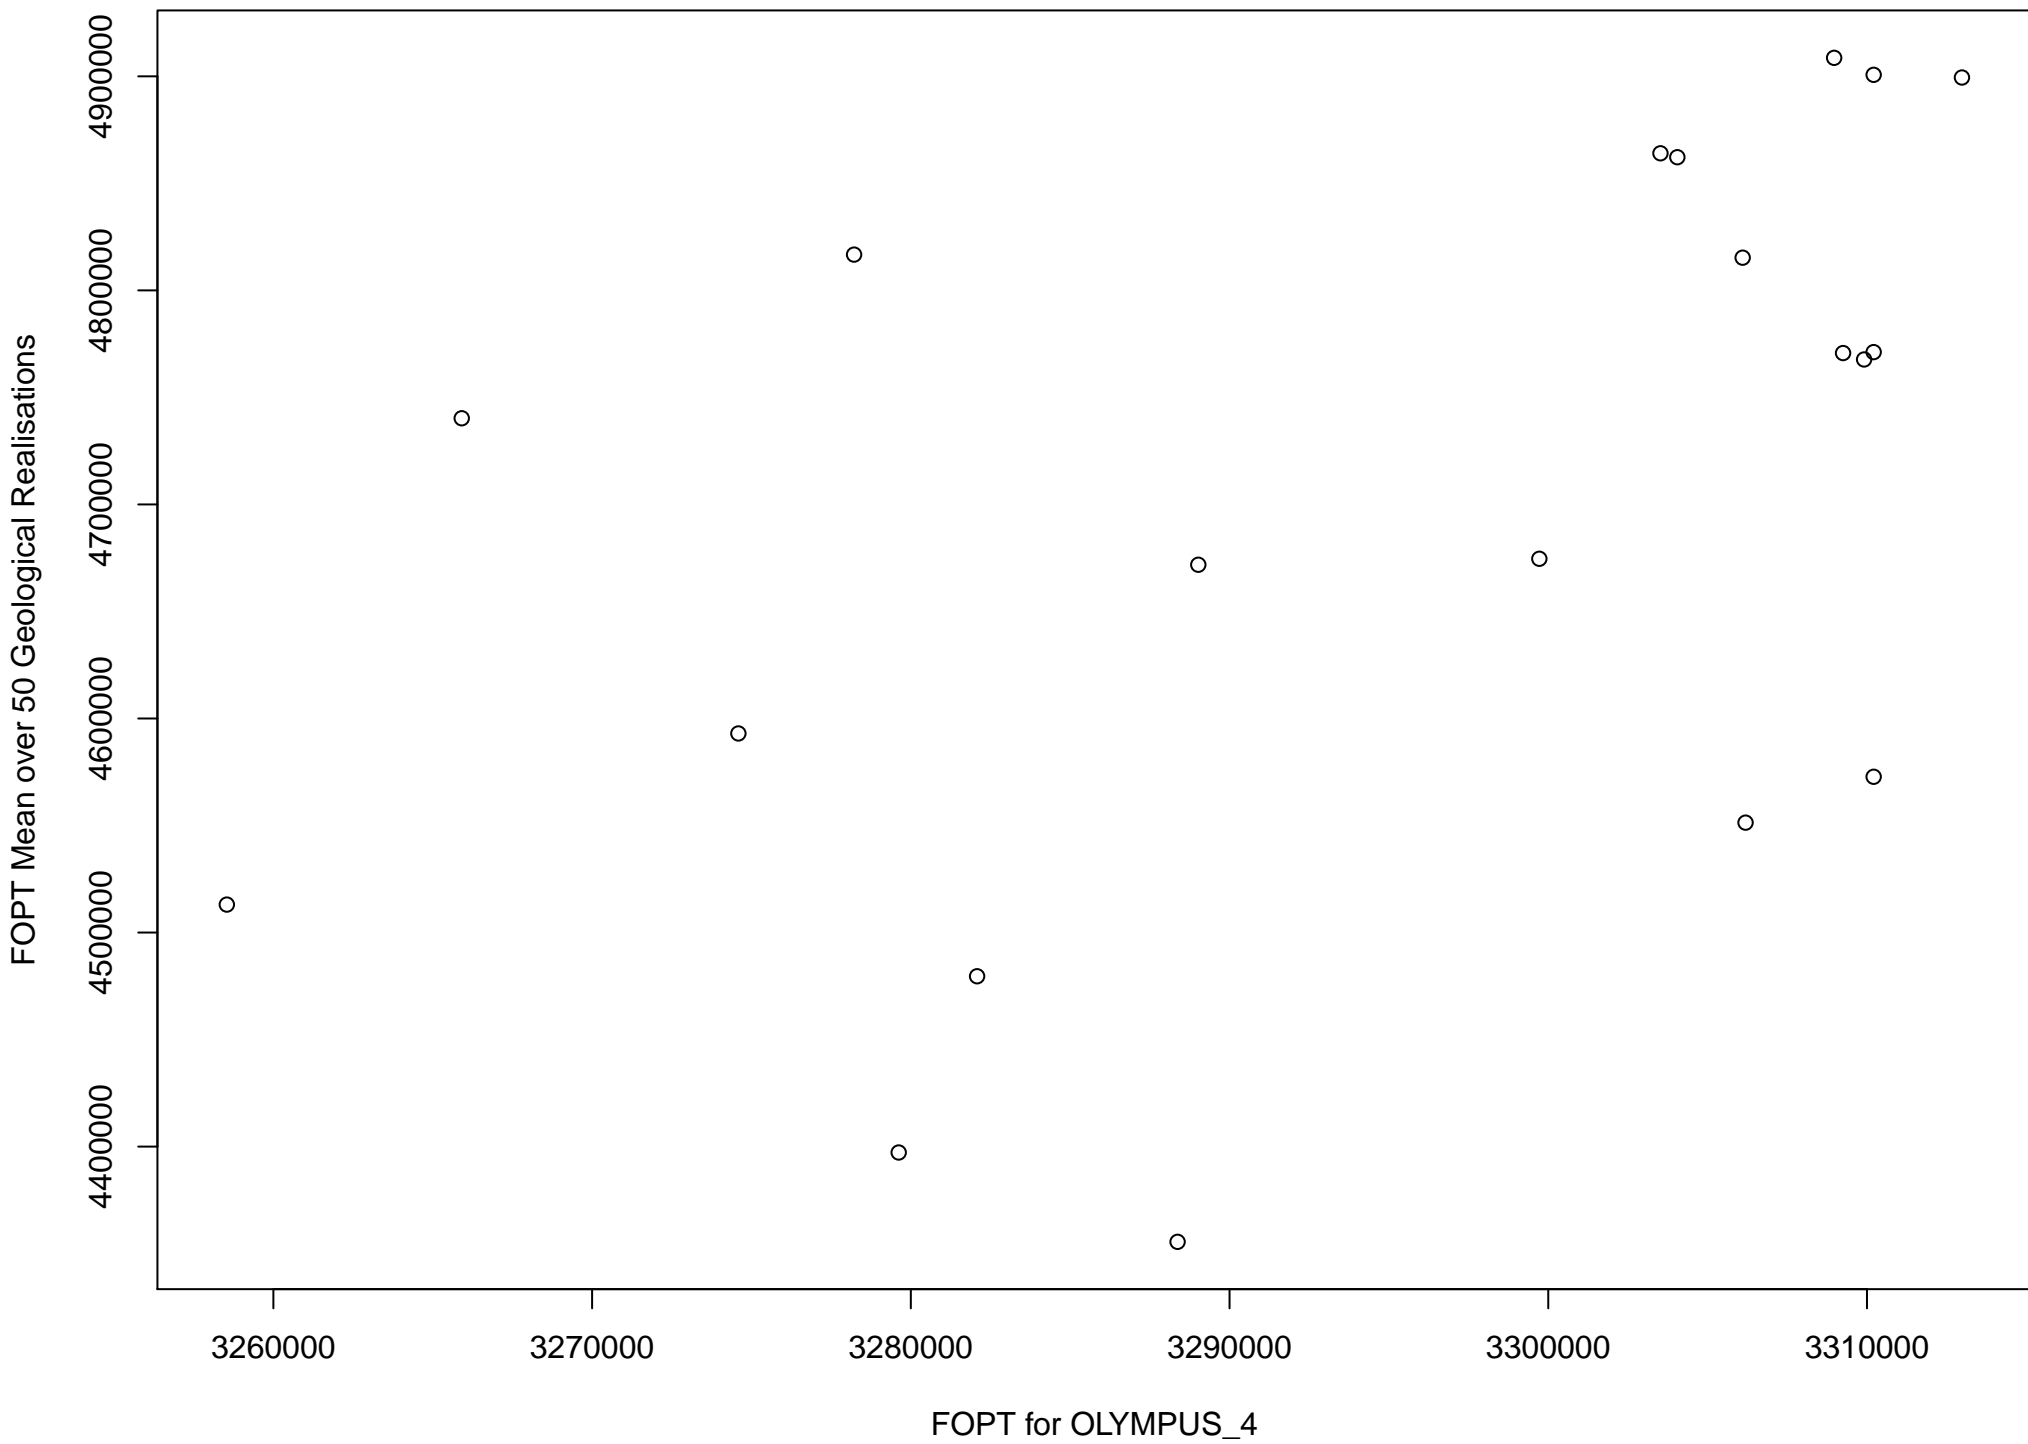

FOPT for OLYMPUS\_5

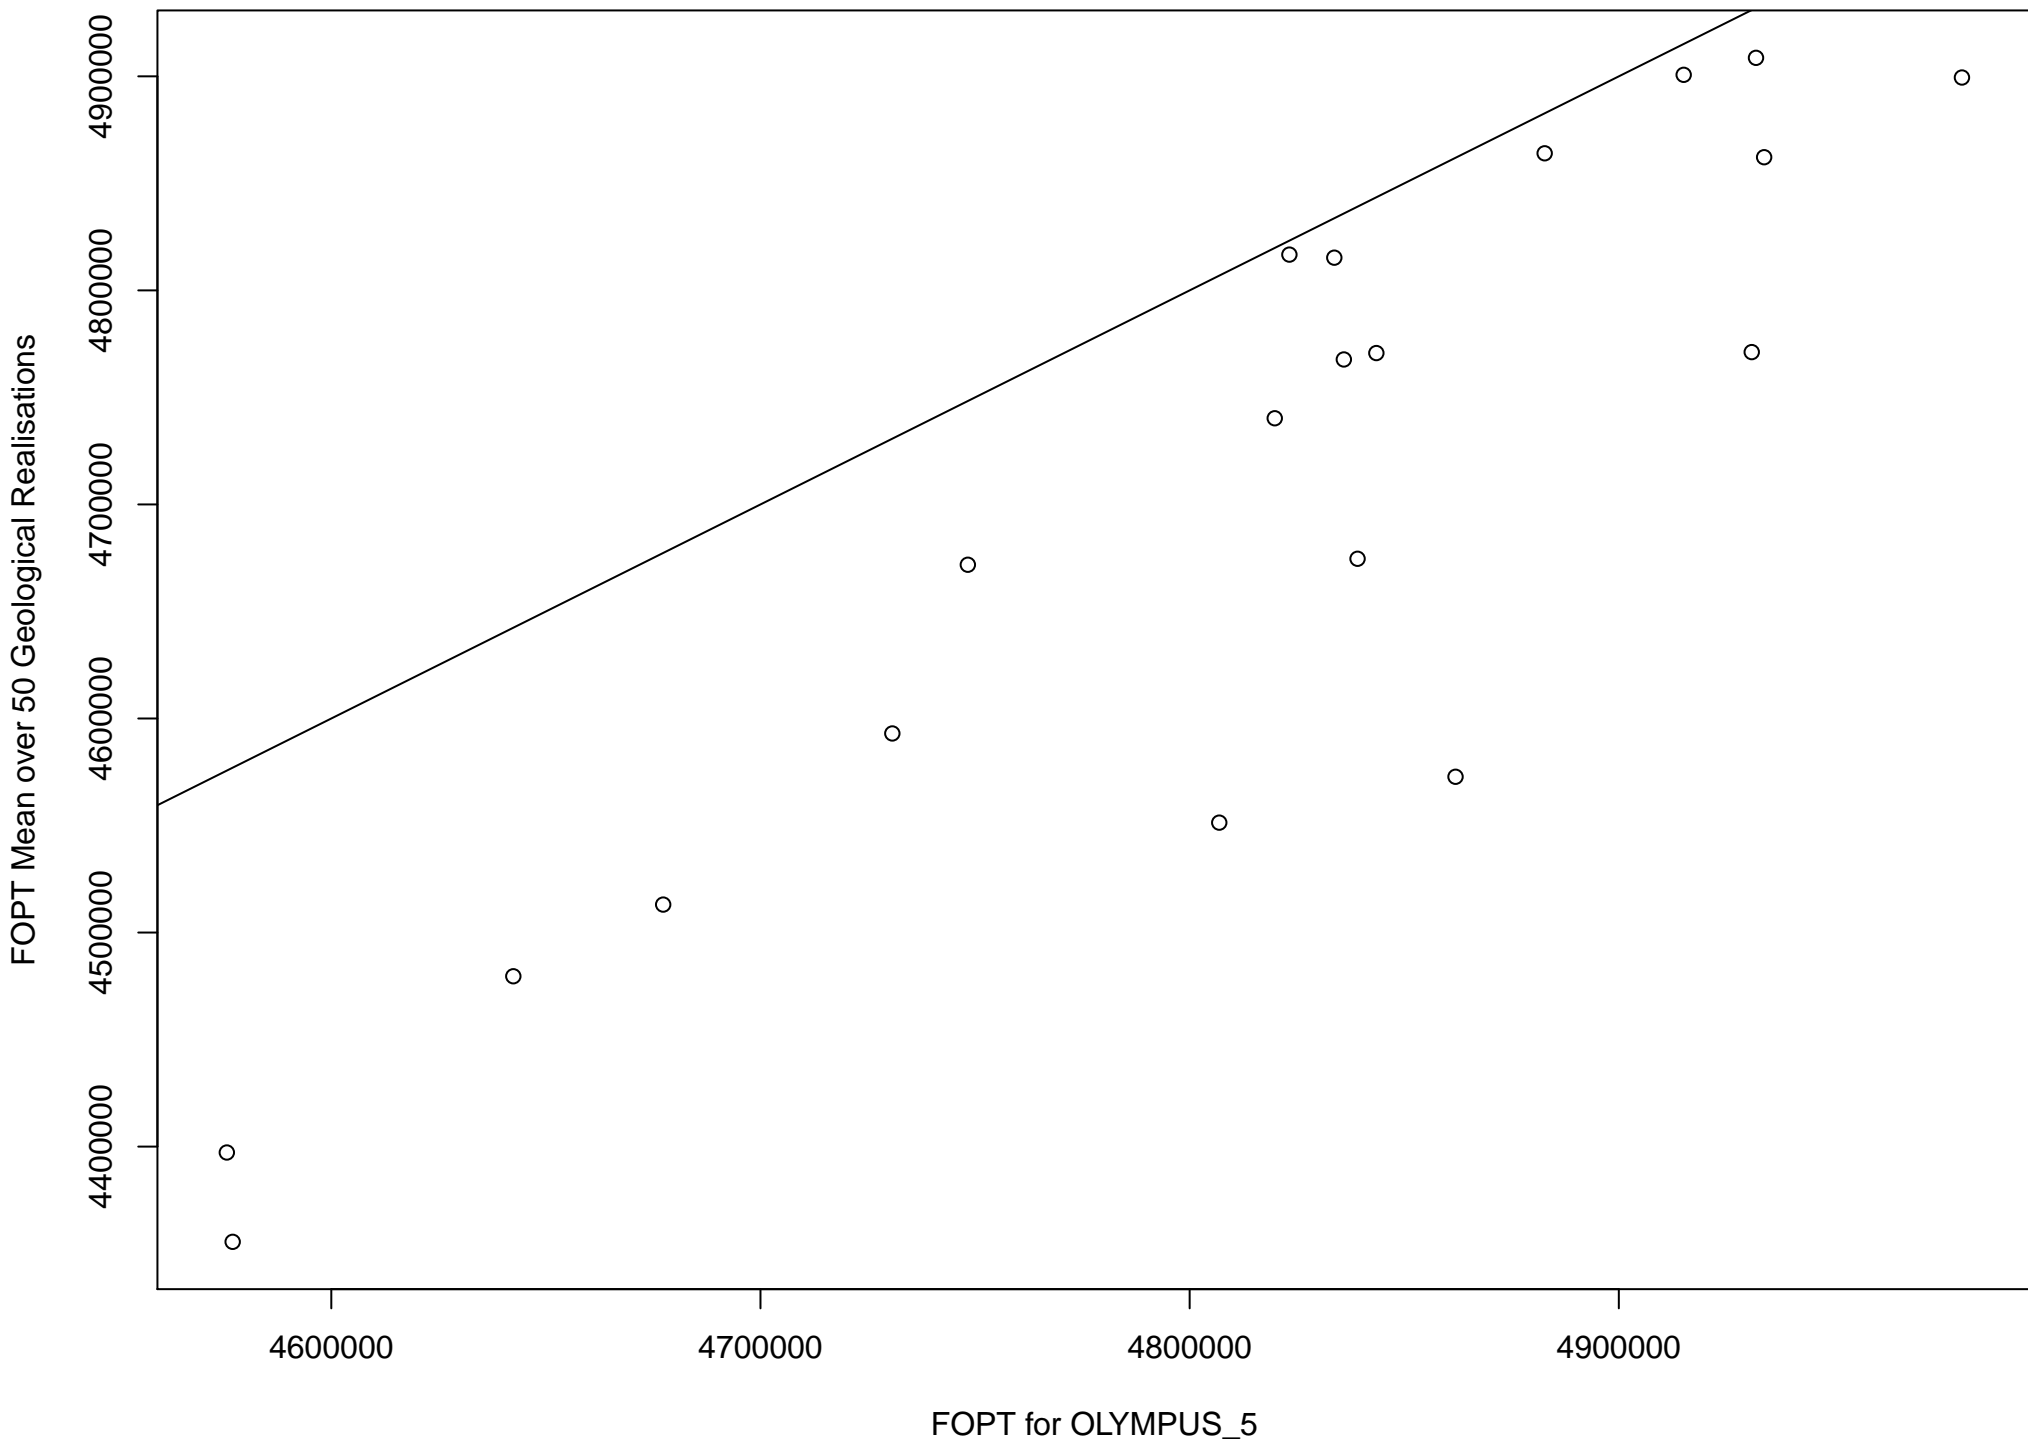

FOPT for OLYMPUS\_6

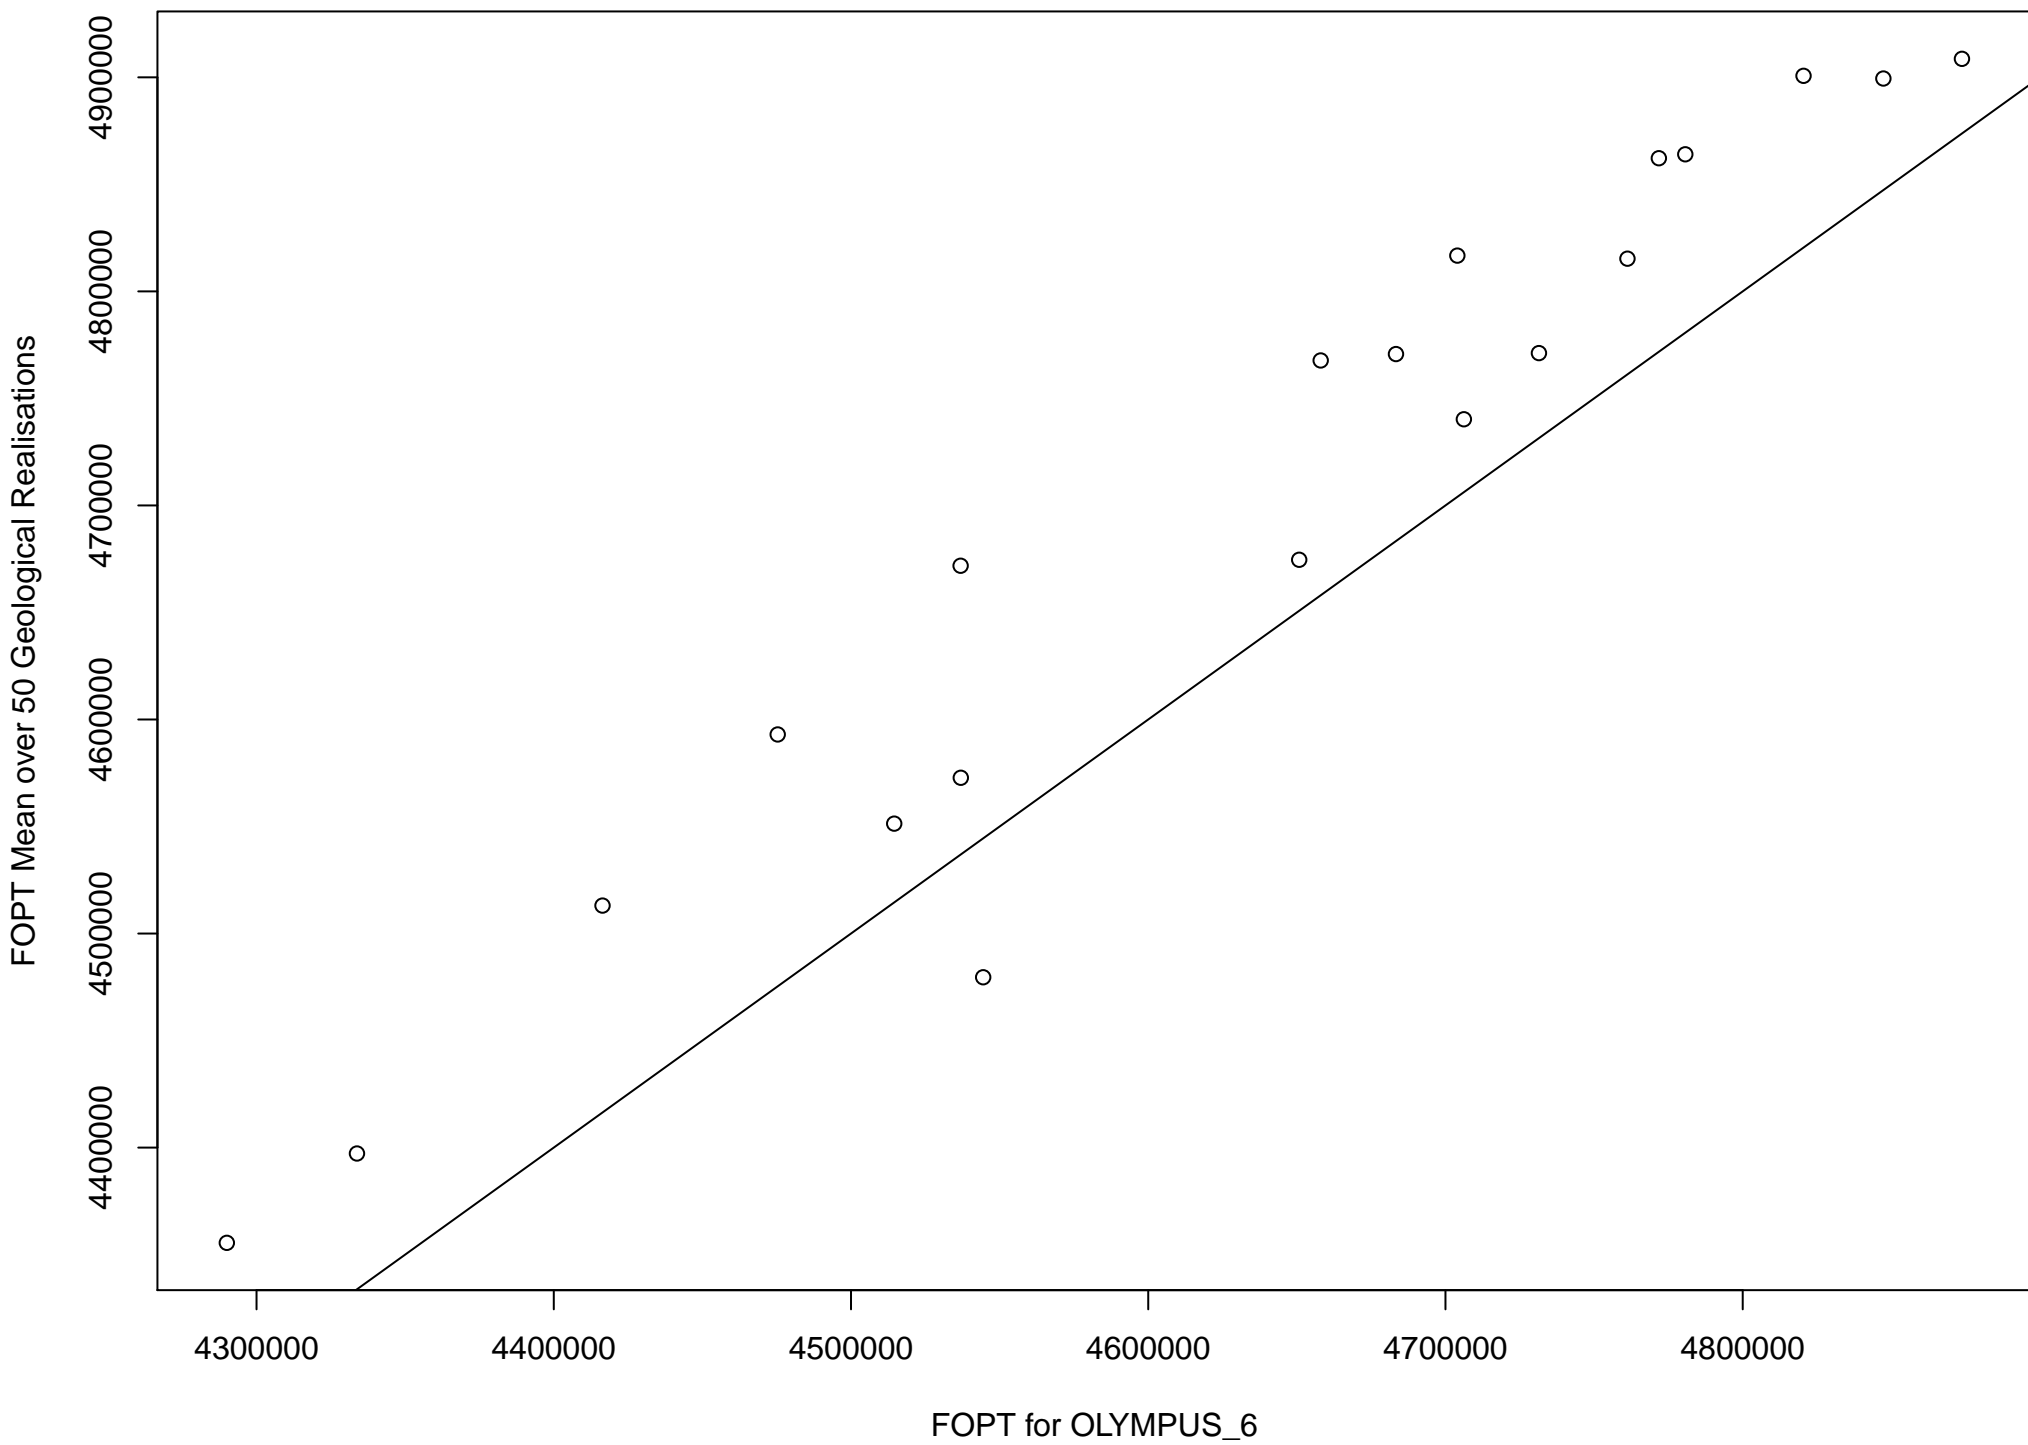

FOPT for OLYMPUS\_7

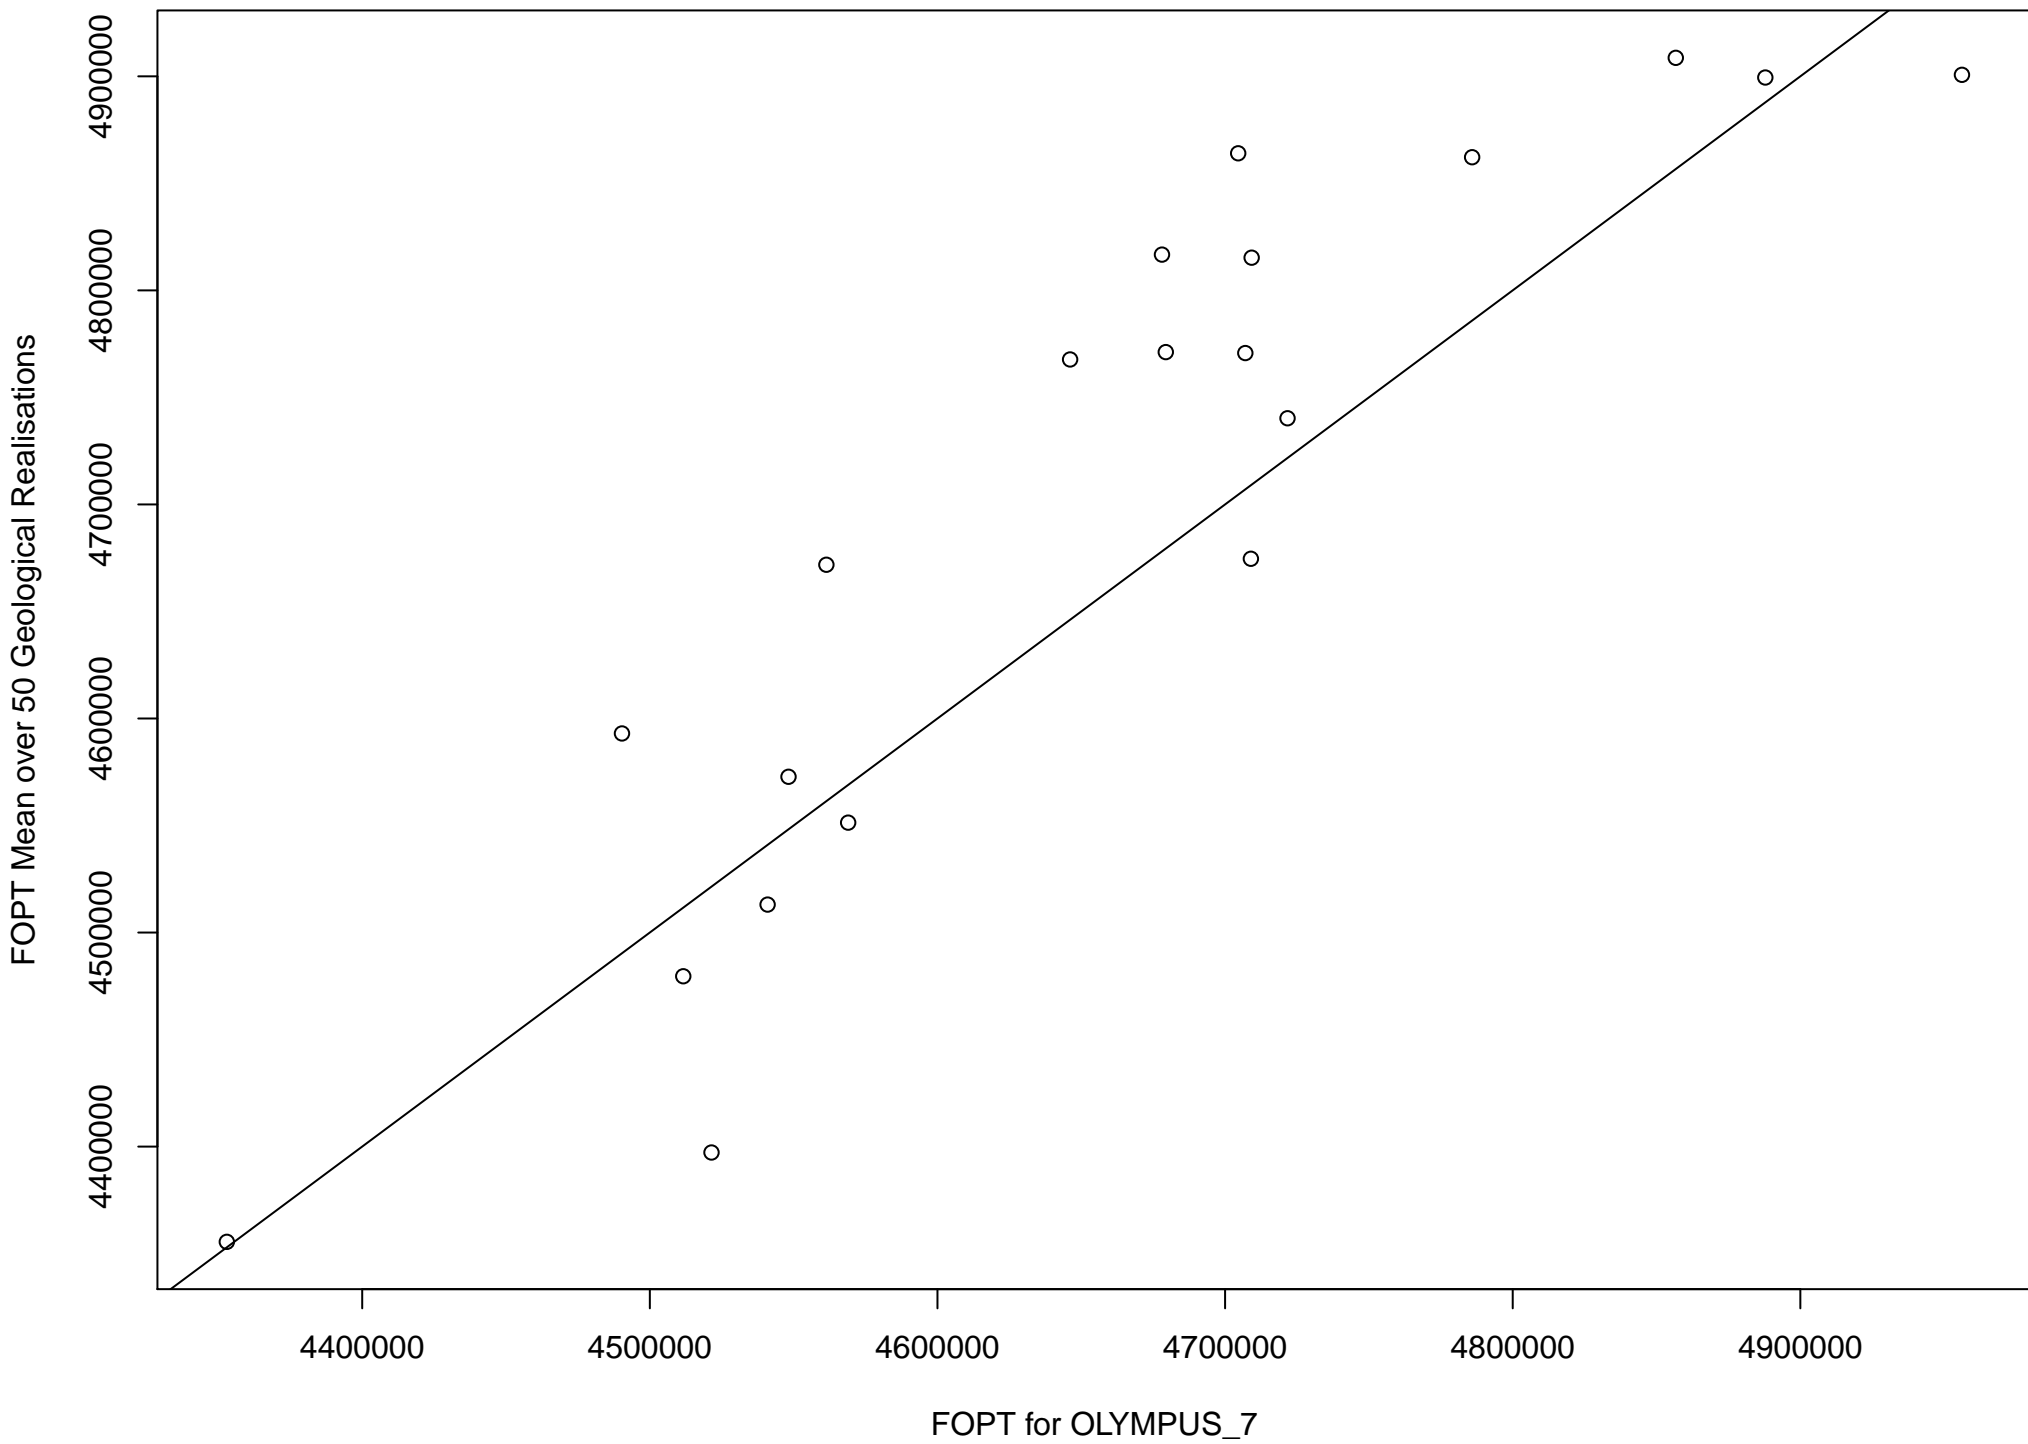

FOPT for OLYMPUS\_8

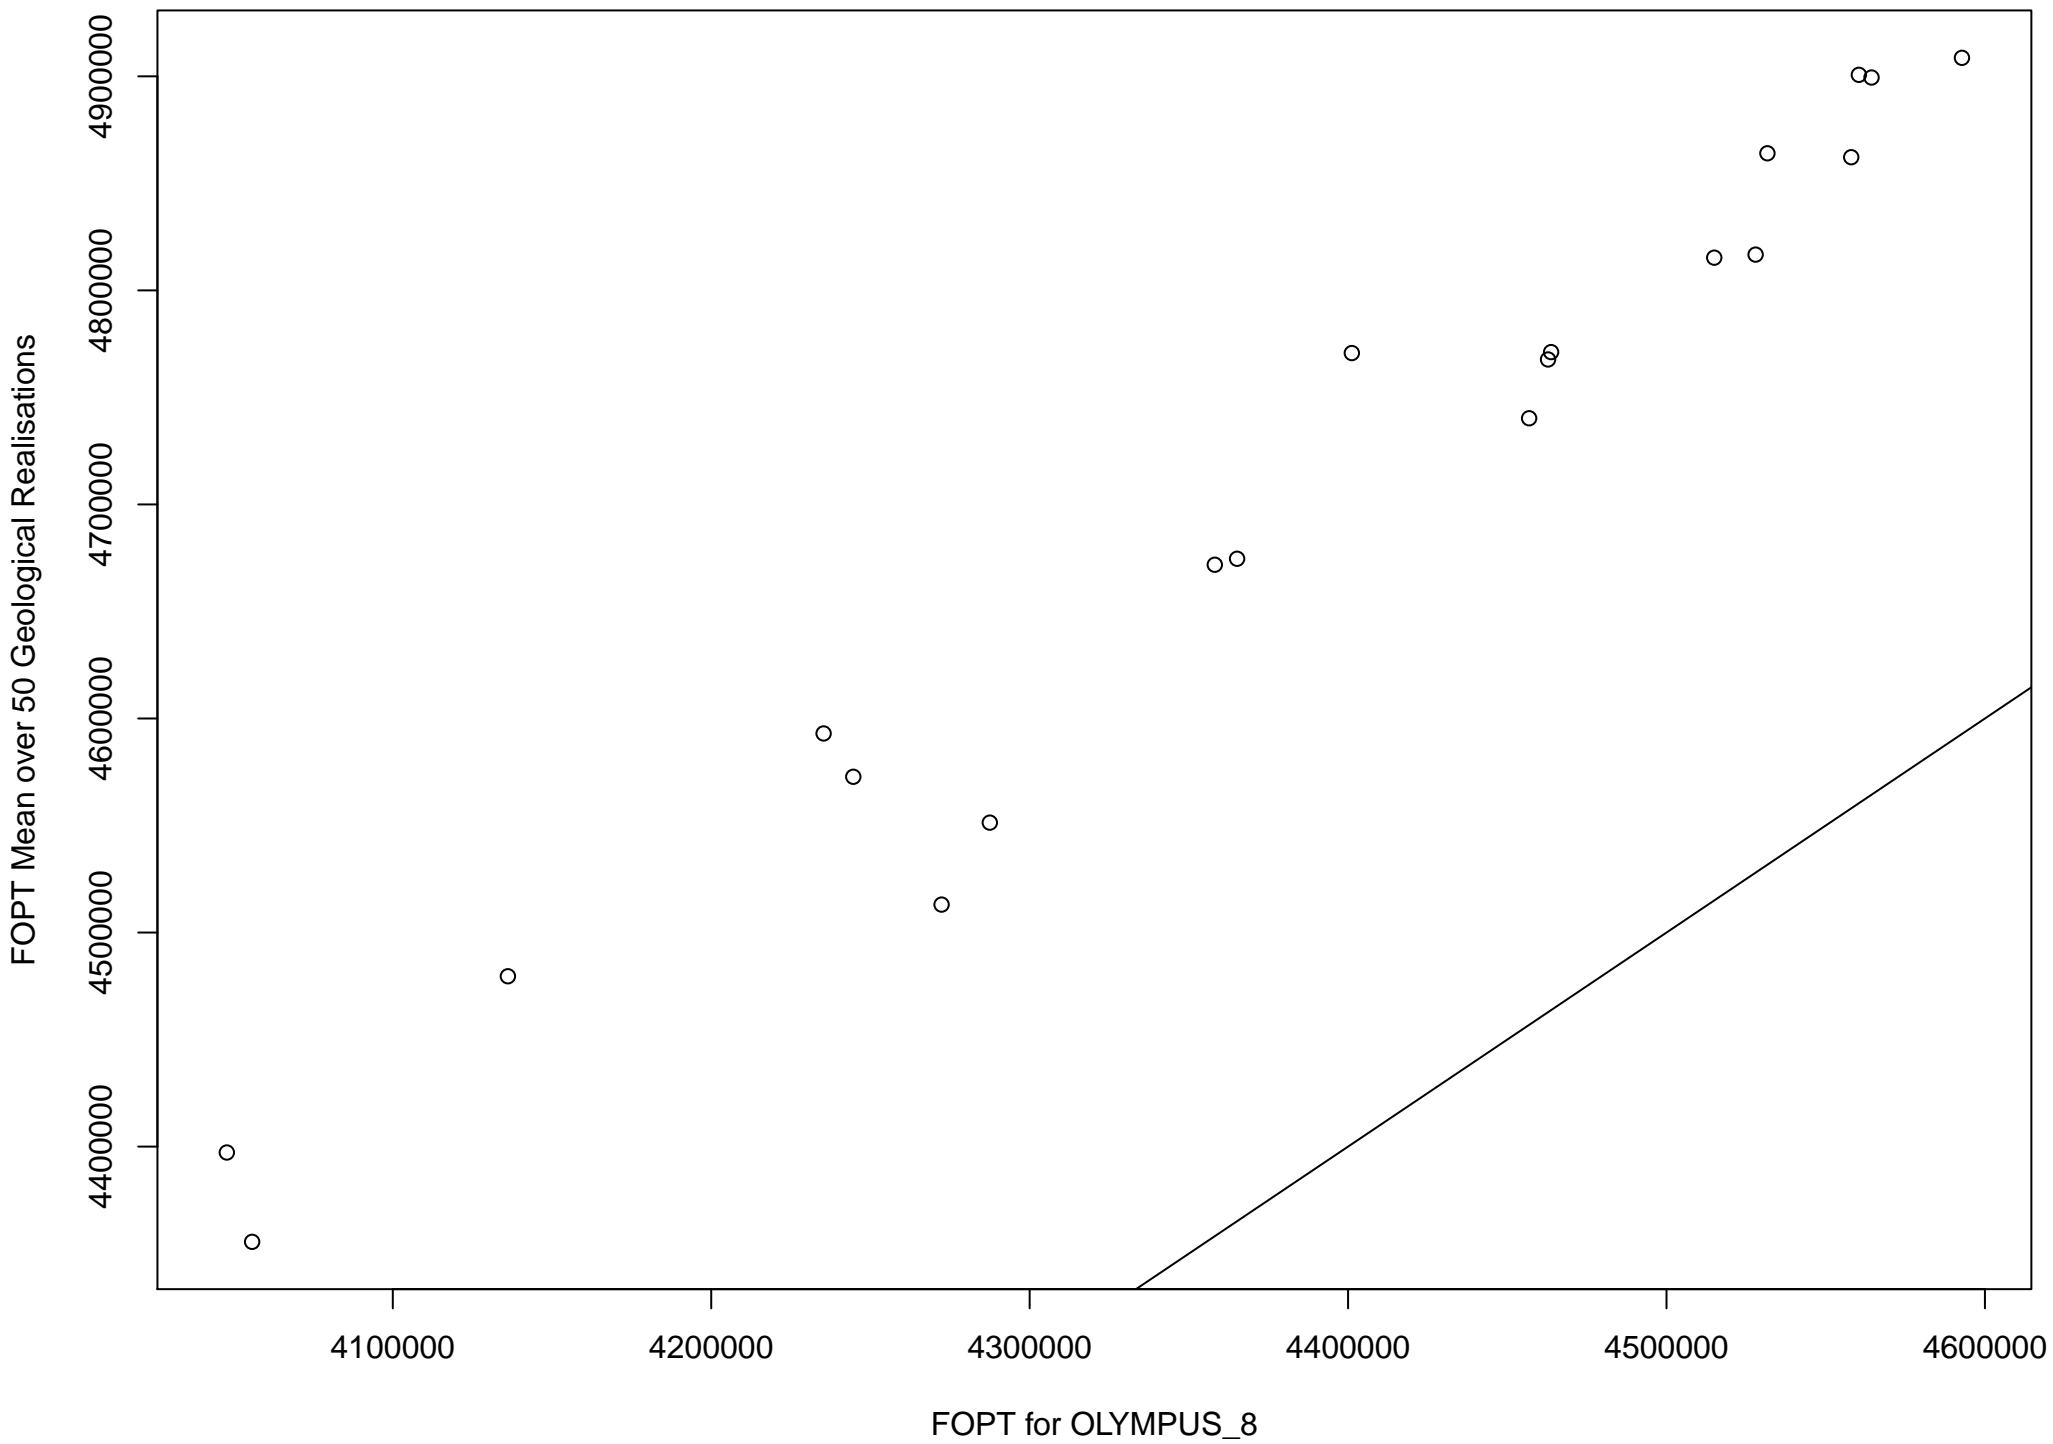



FOPT for OLYMPUS\_9

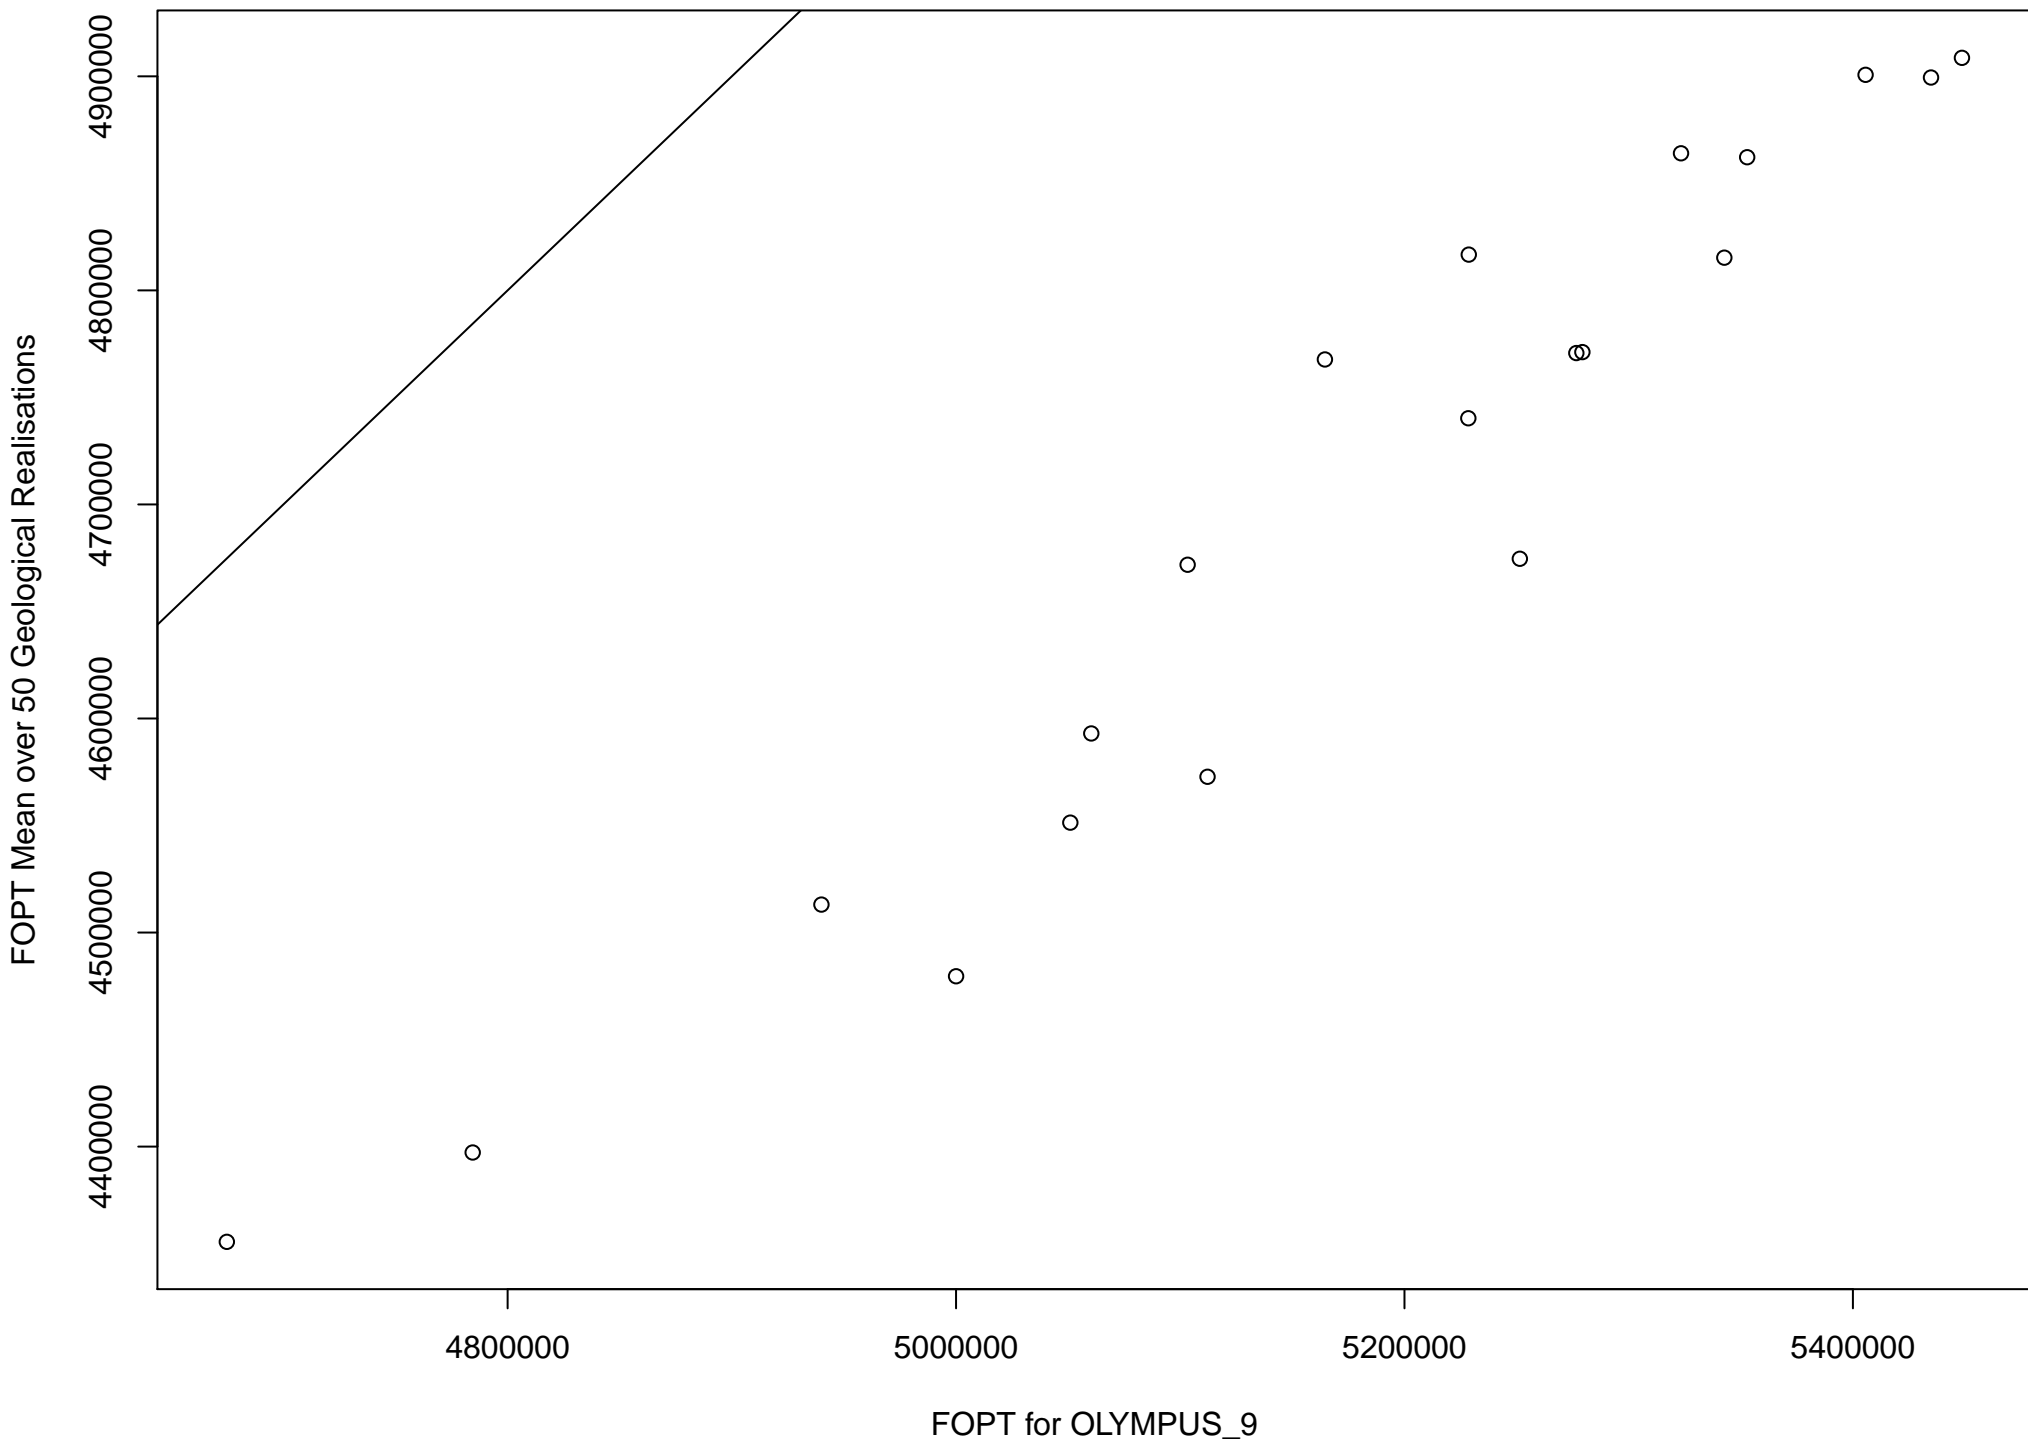

FOPT for OLYMPUS\_10

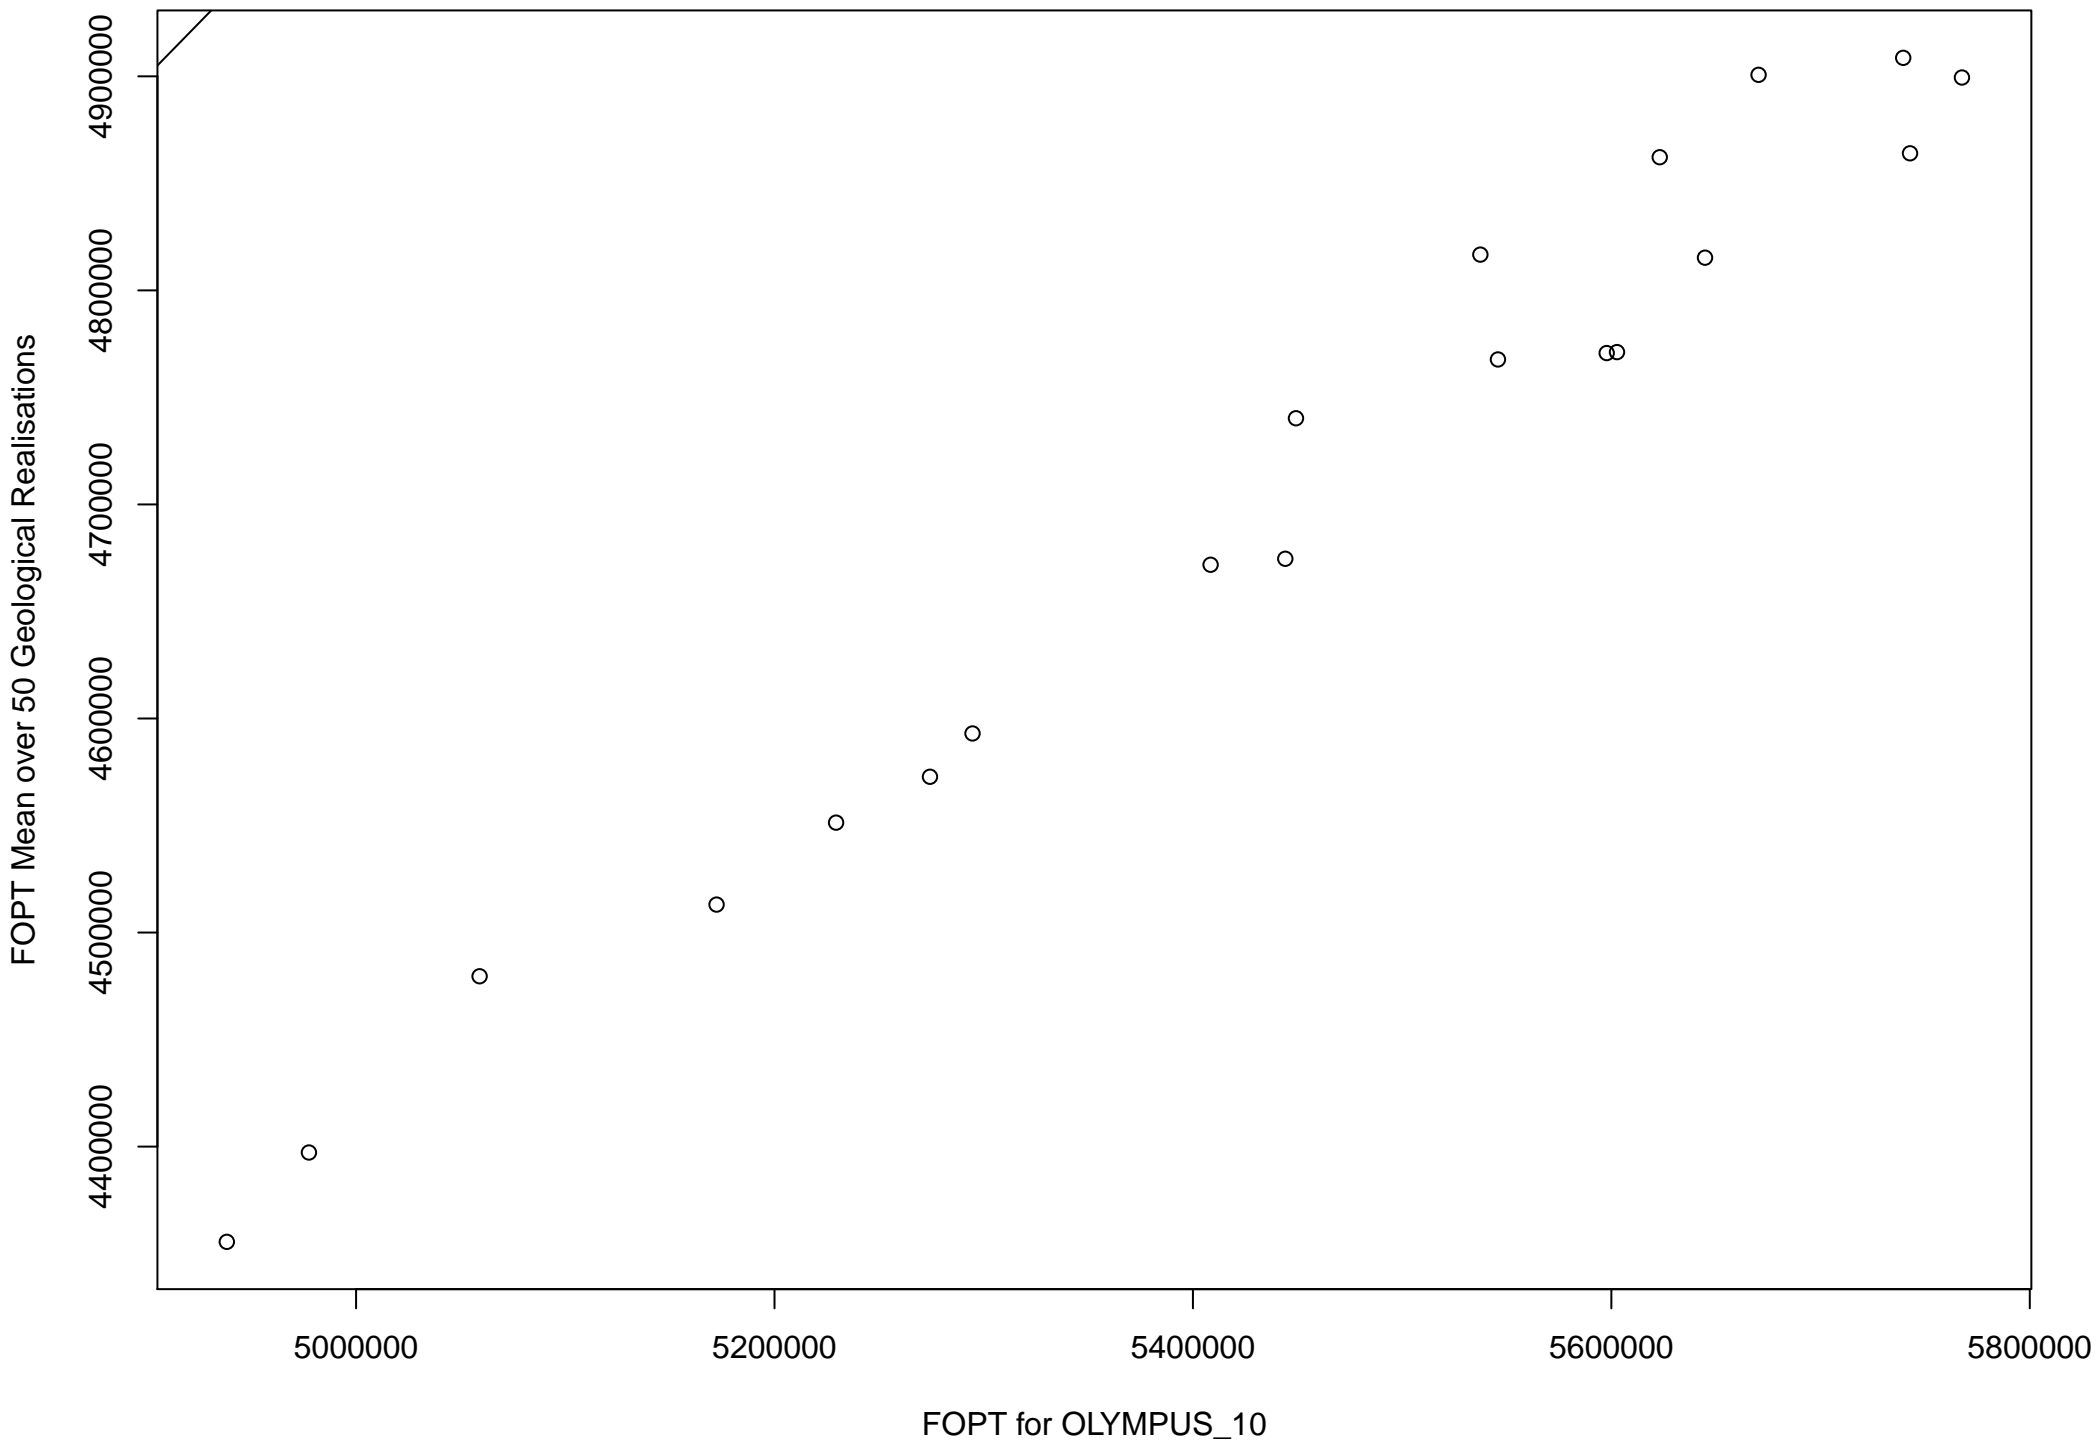

FOPT for OLYMPUS\_11

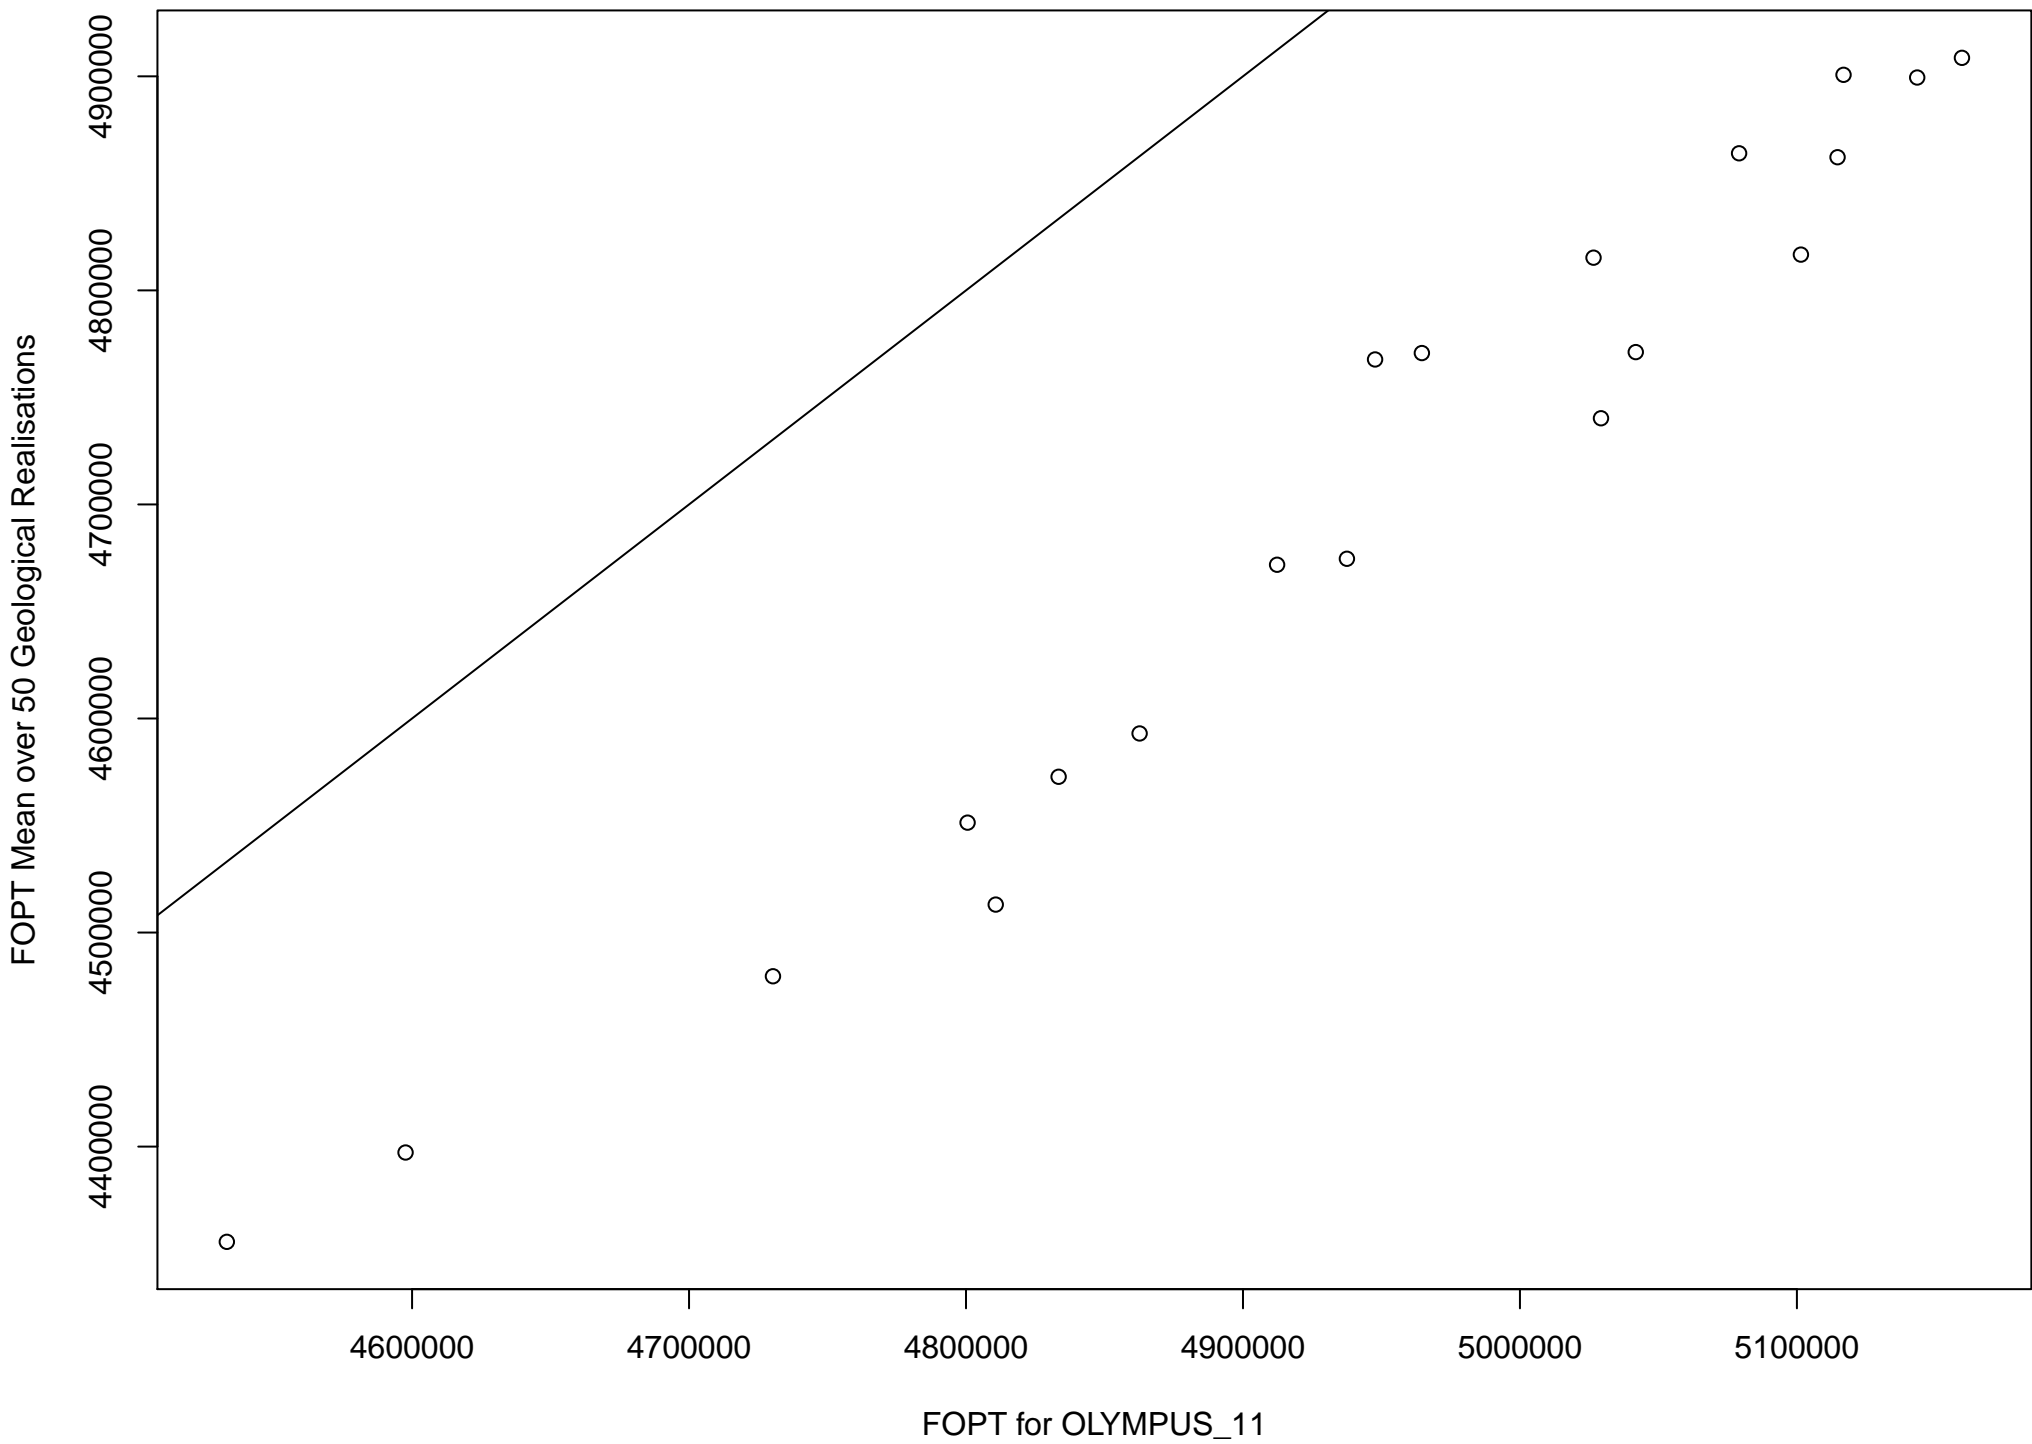

FOPT for OLYMPUS\_12

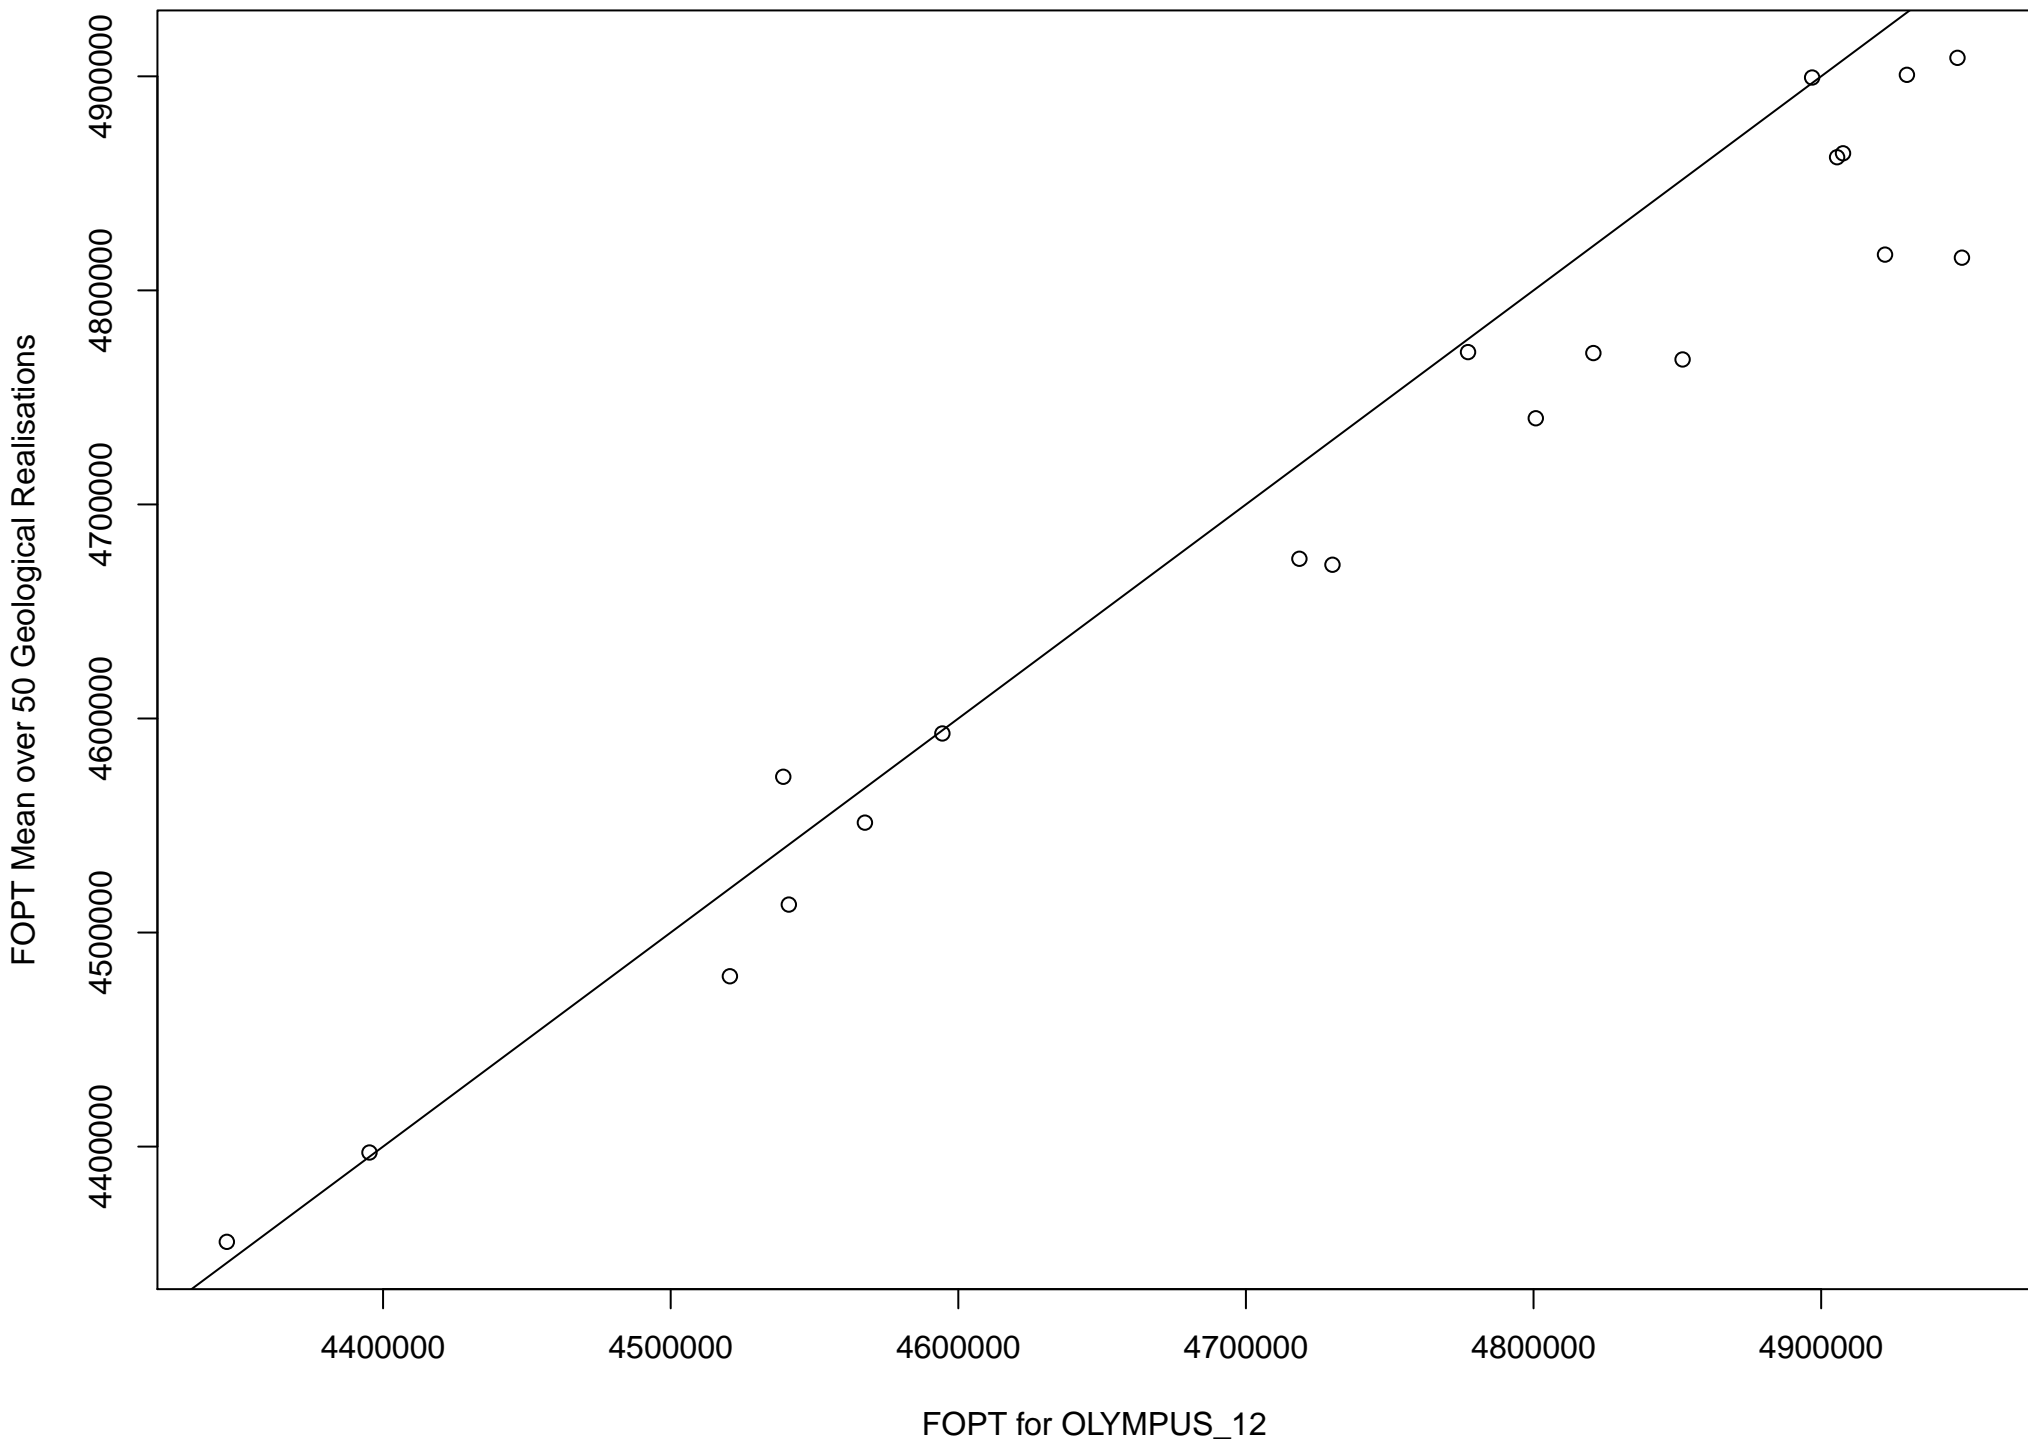

FOPT for OLYMPUS\_13

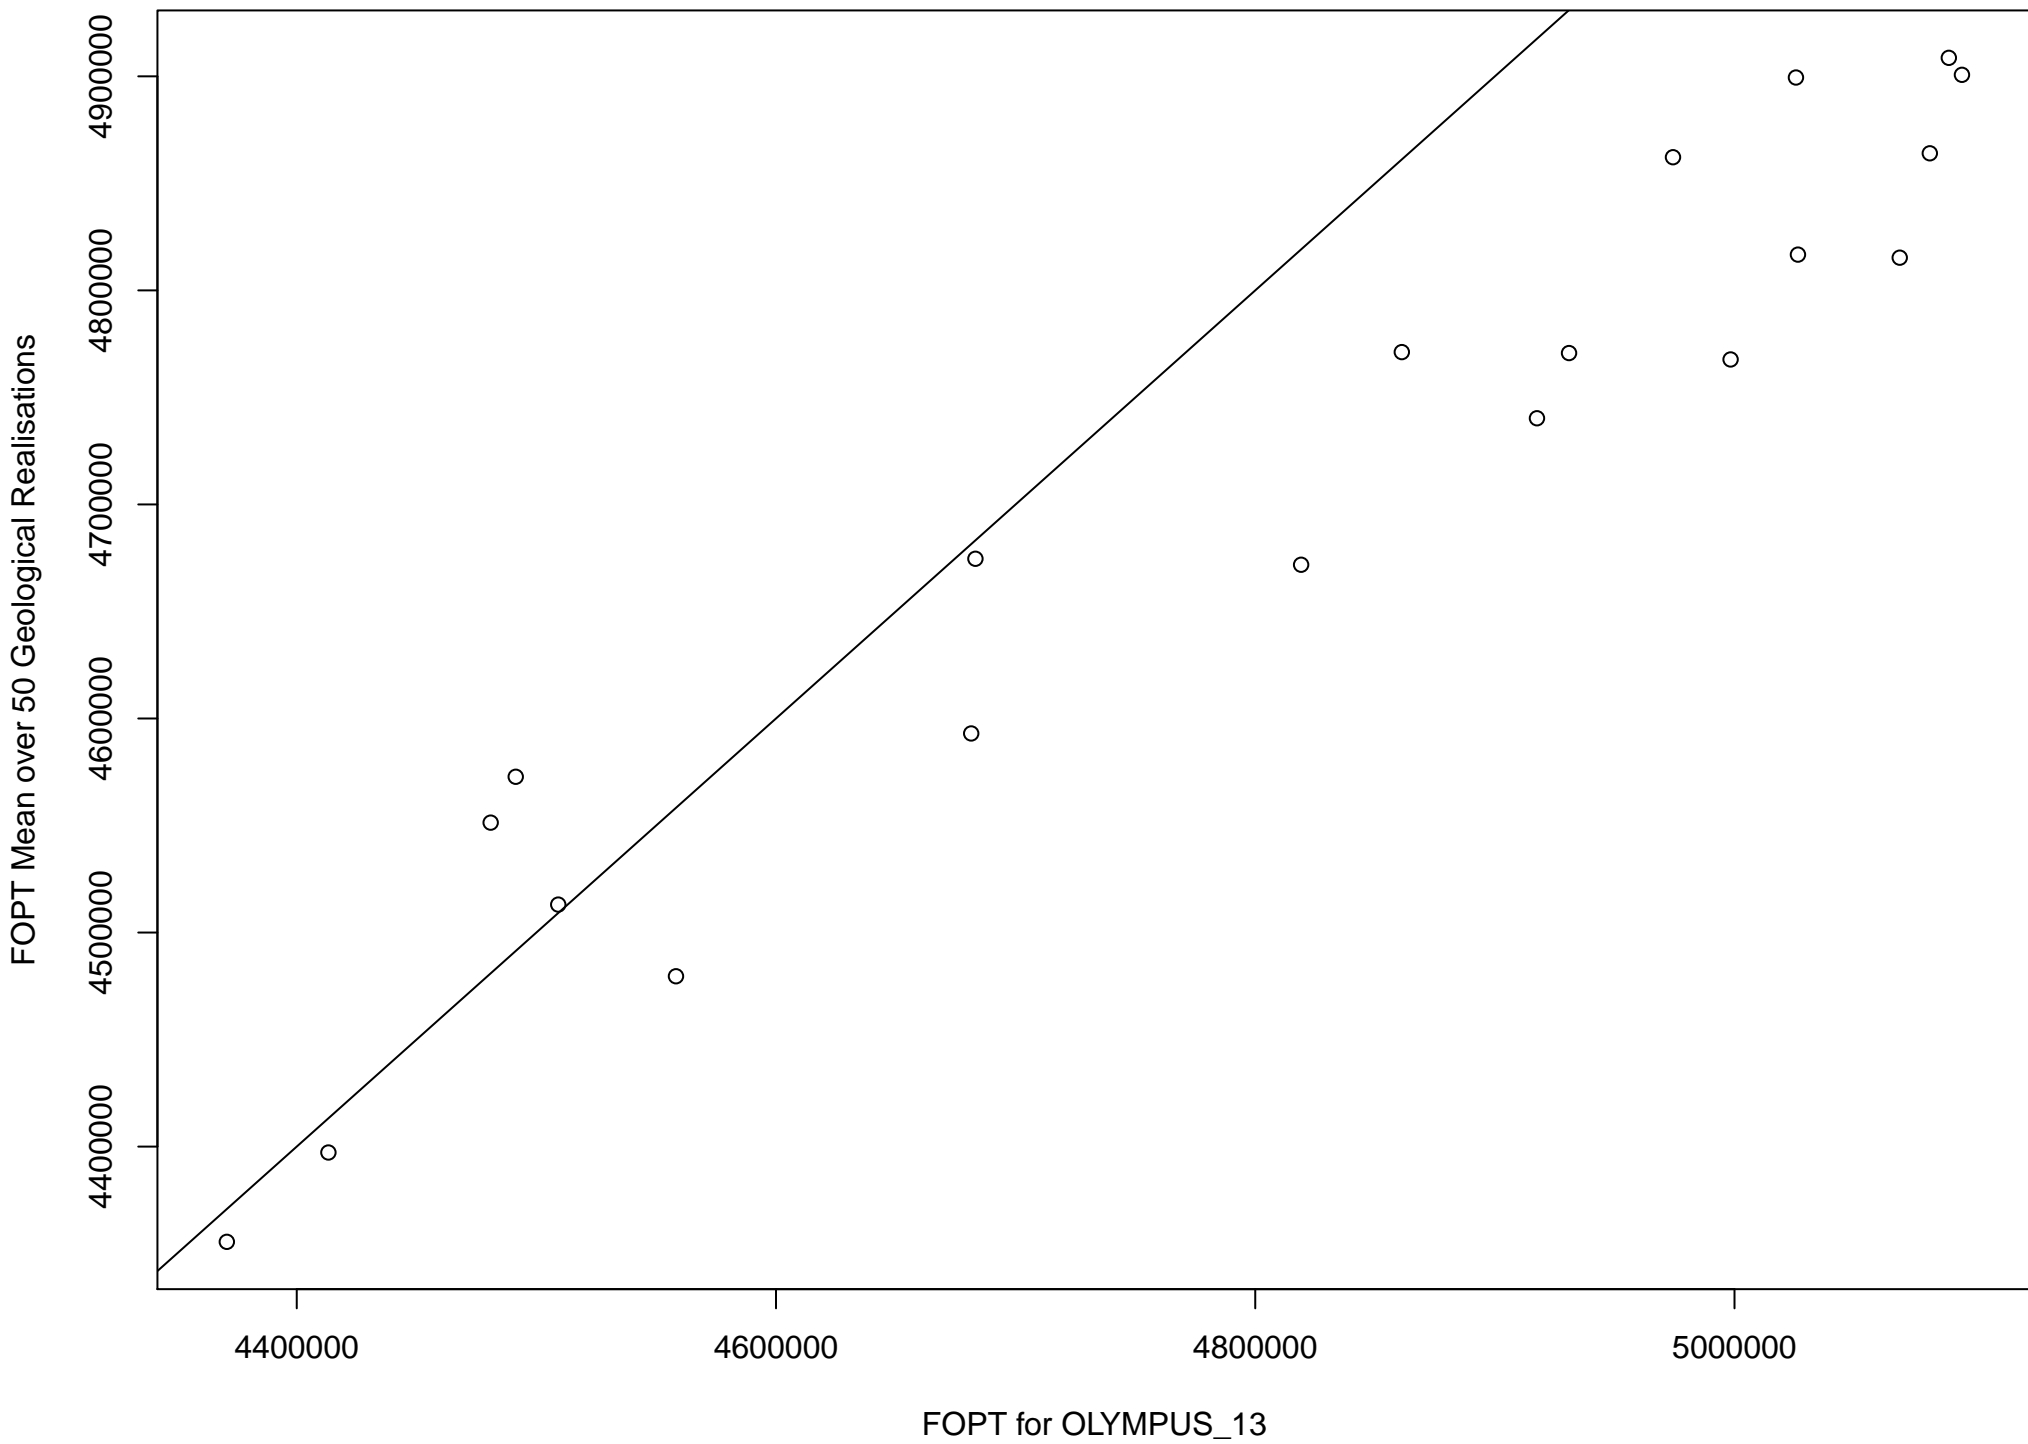

FOPT for OLYMPUS\_14

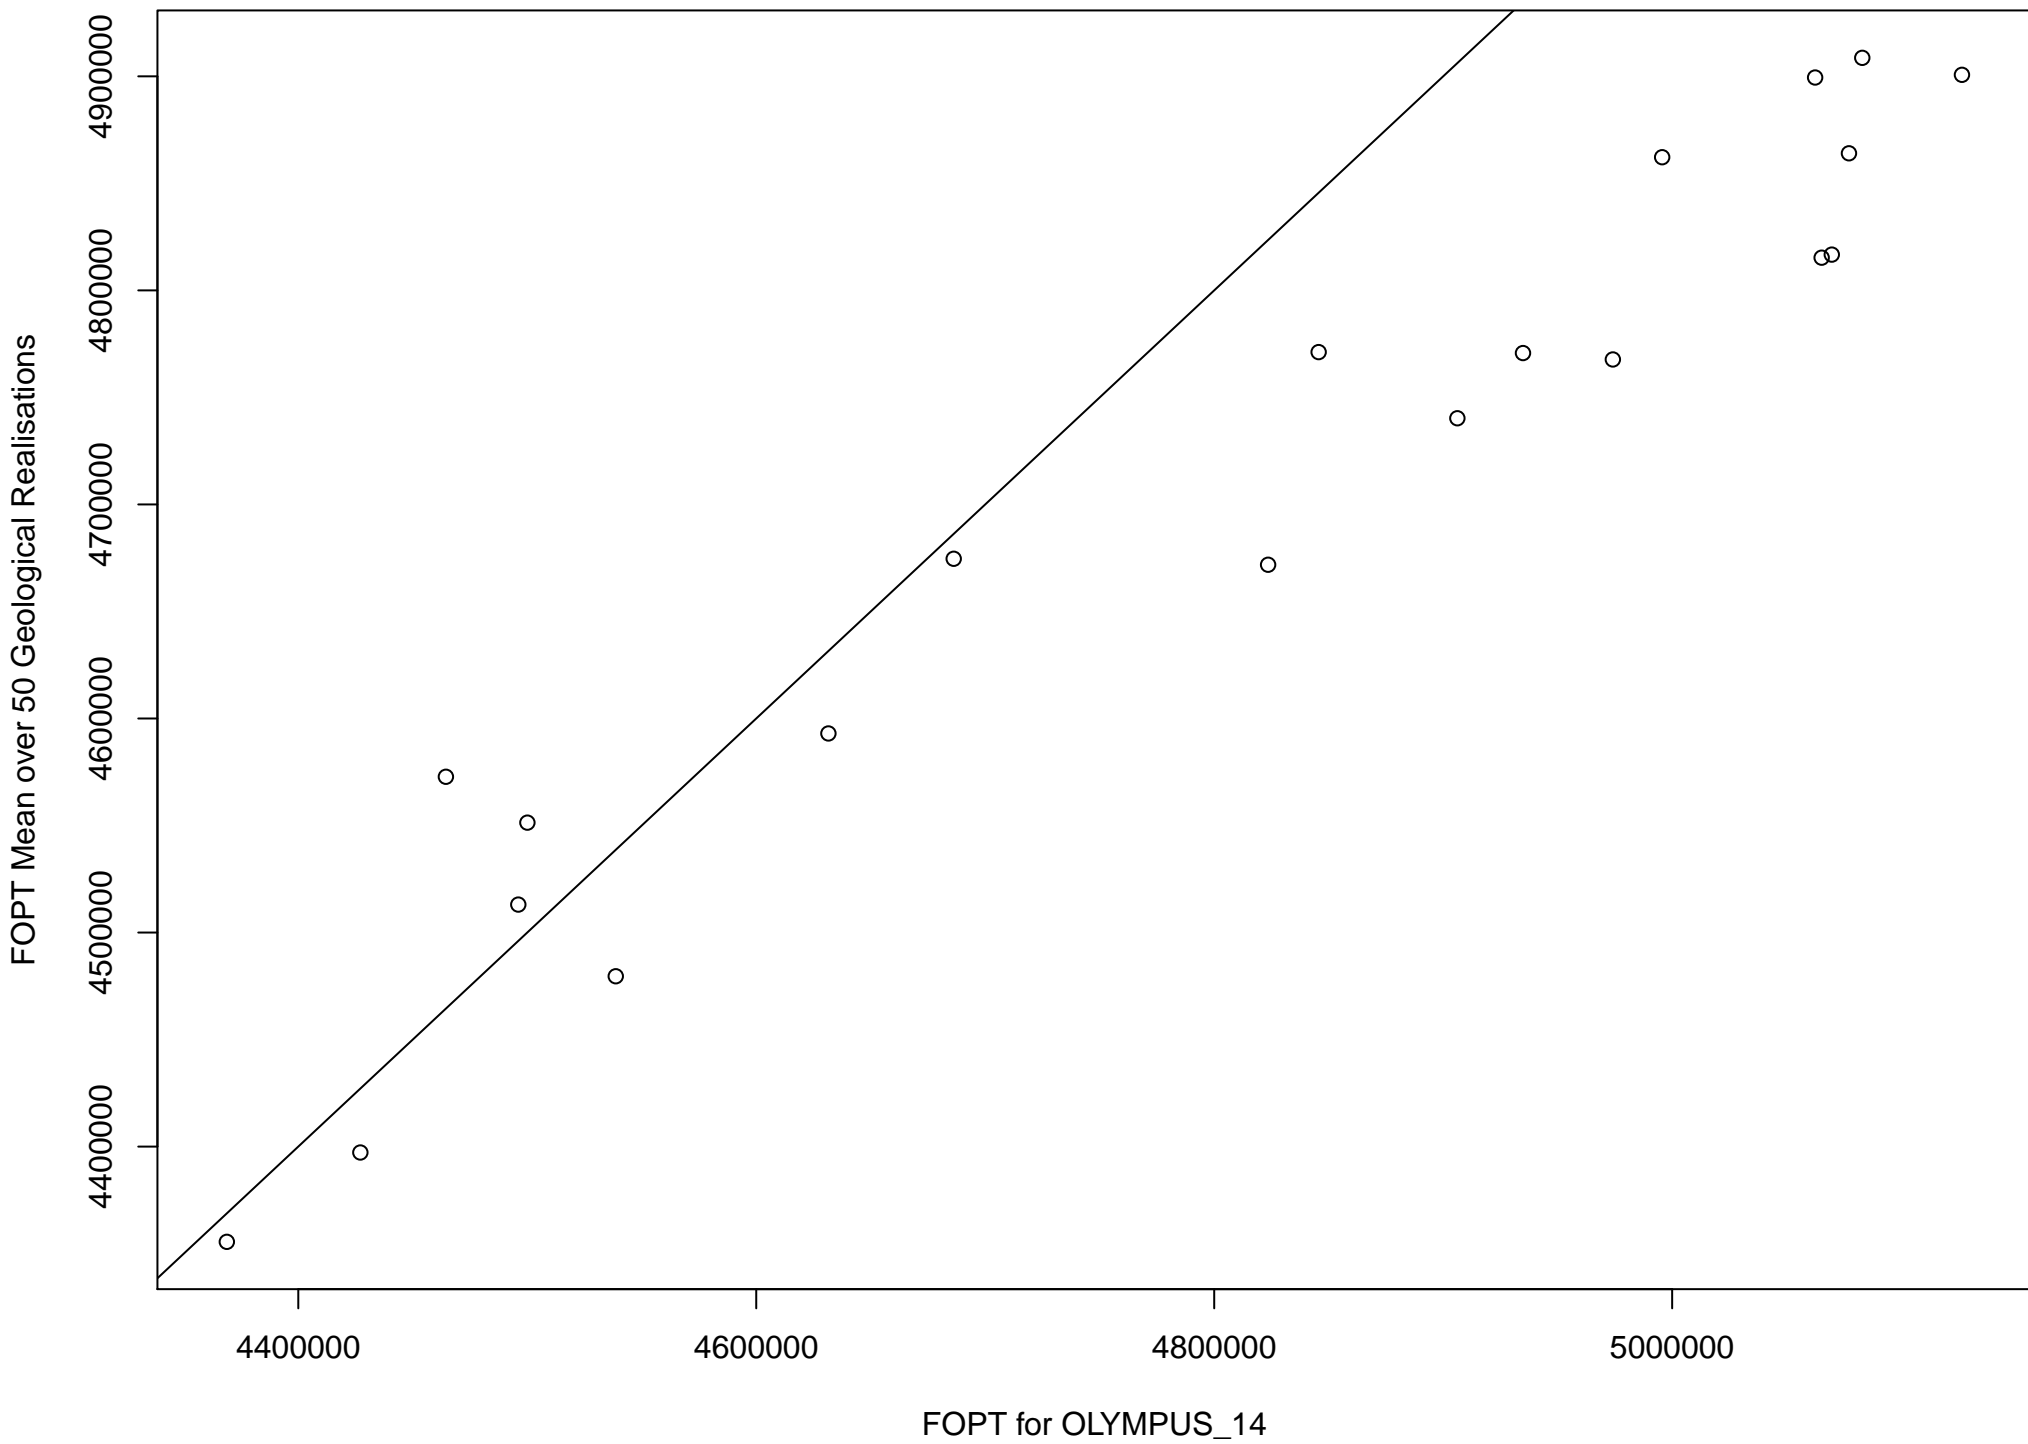

FOPT for OLYMPUS\_15

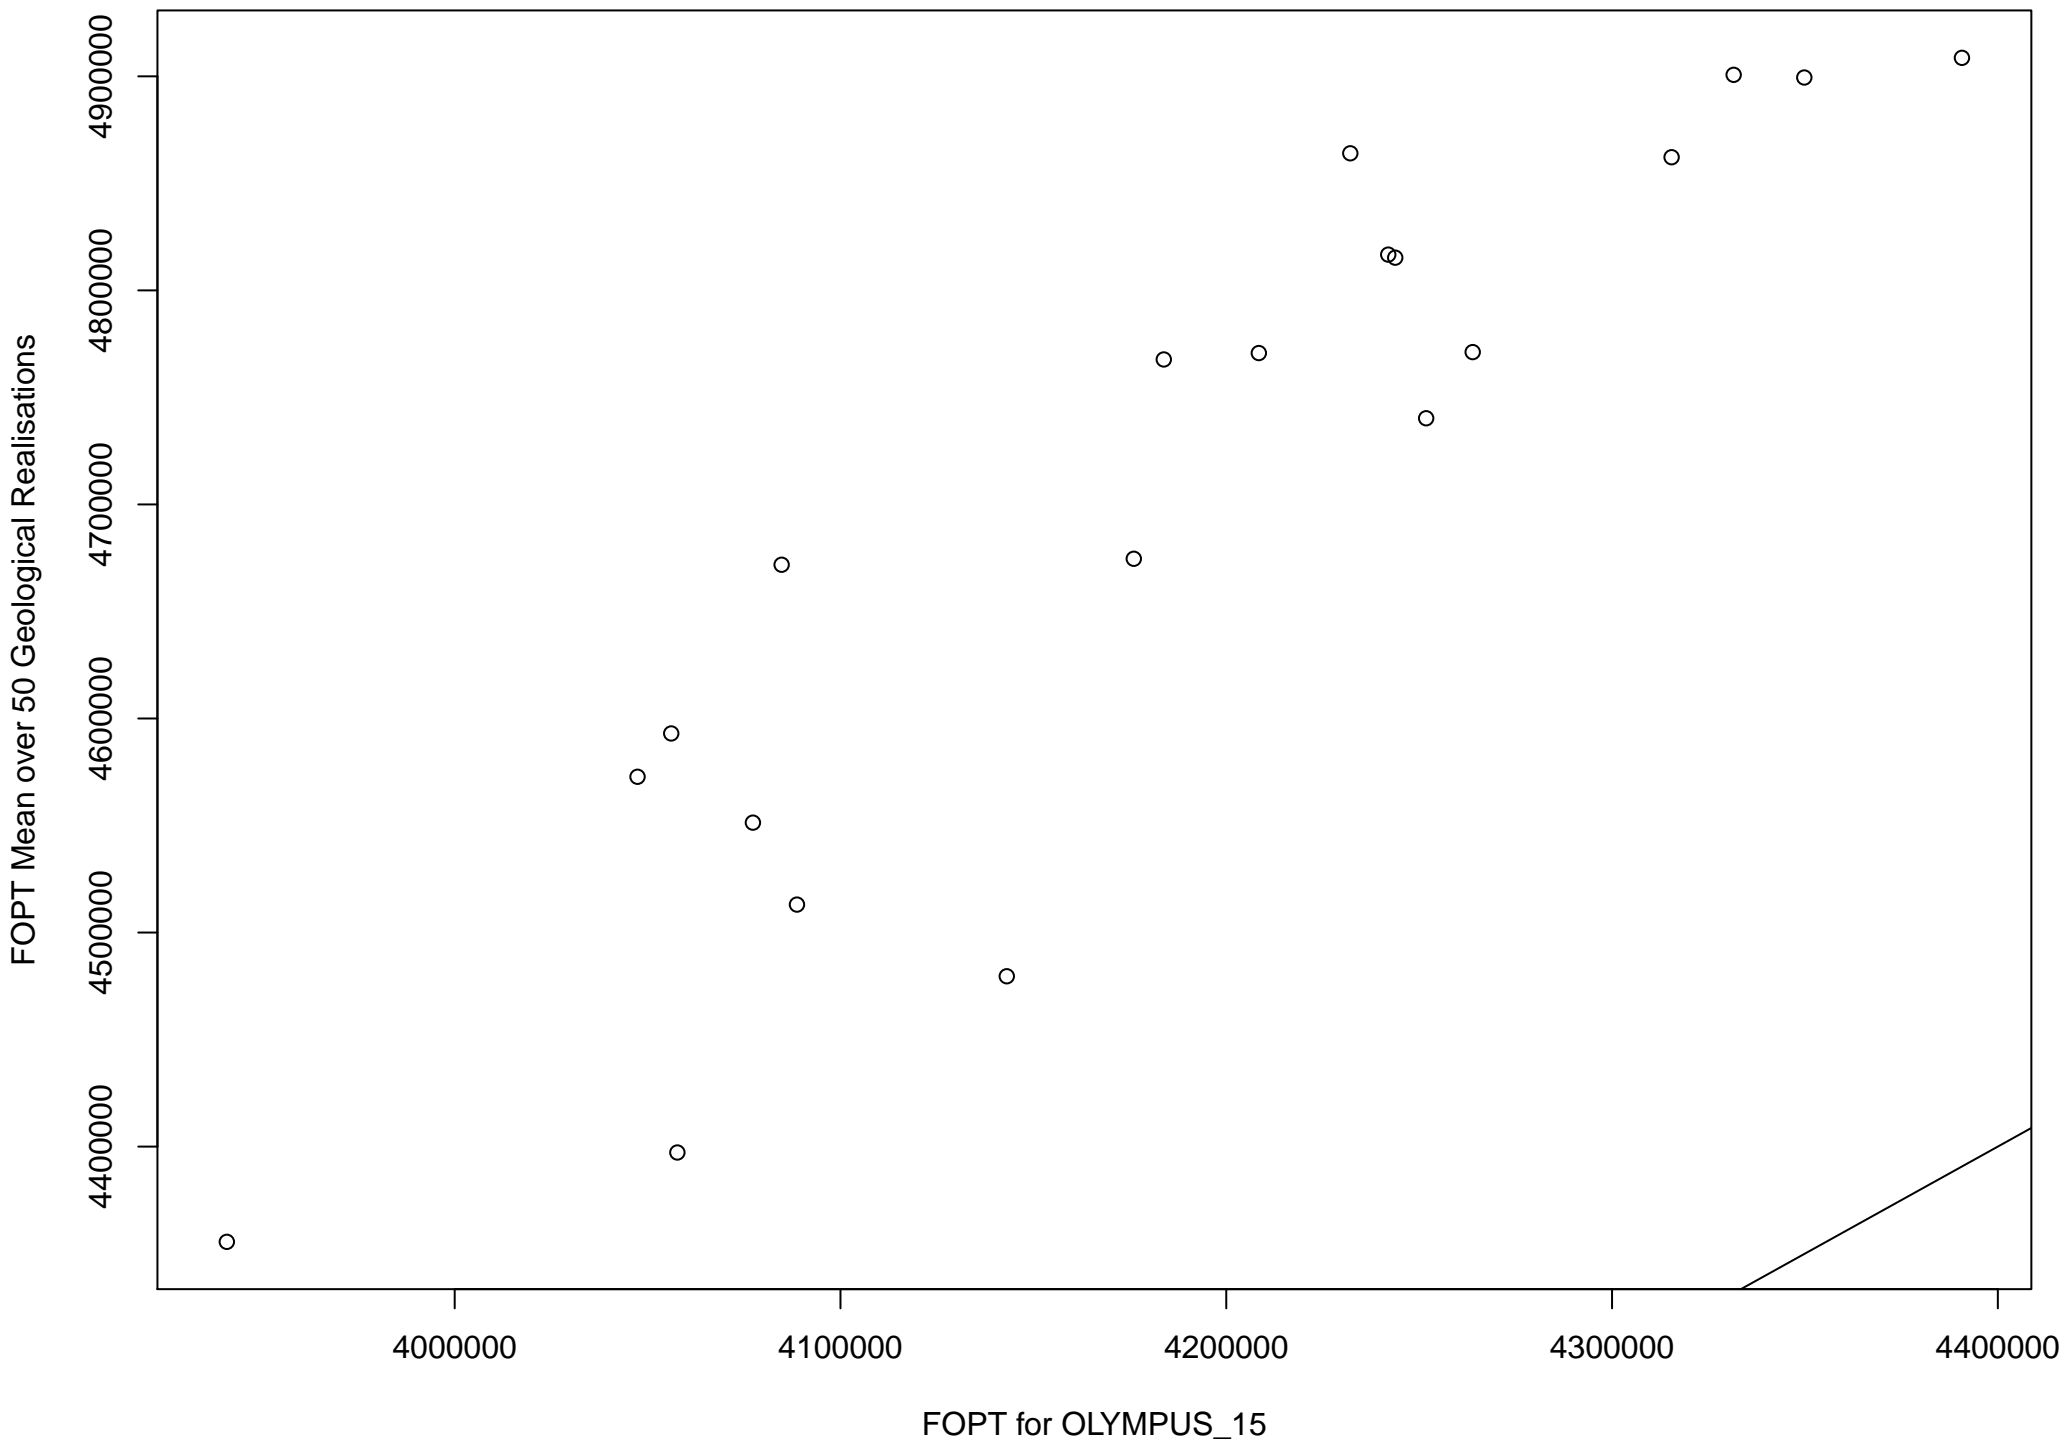

FOPT for OLYMPUS\_16

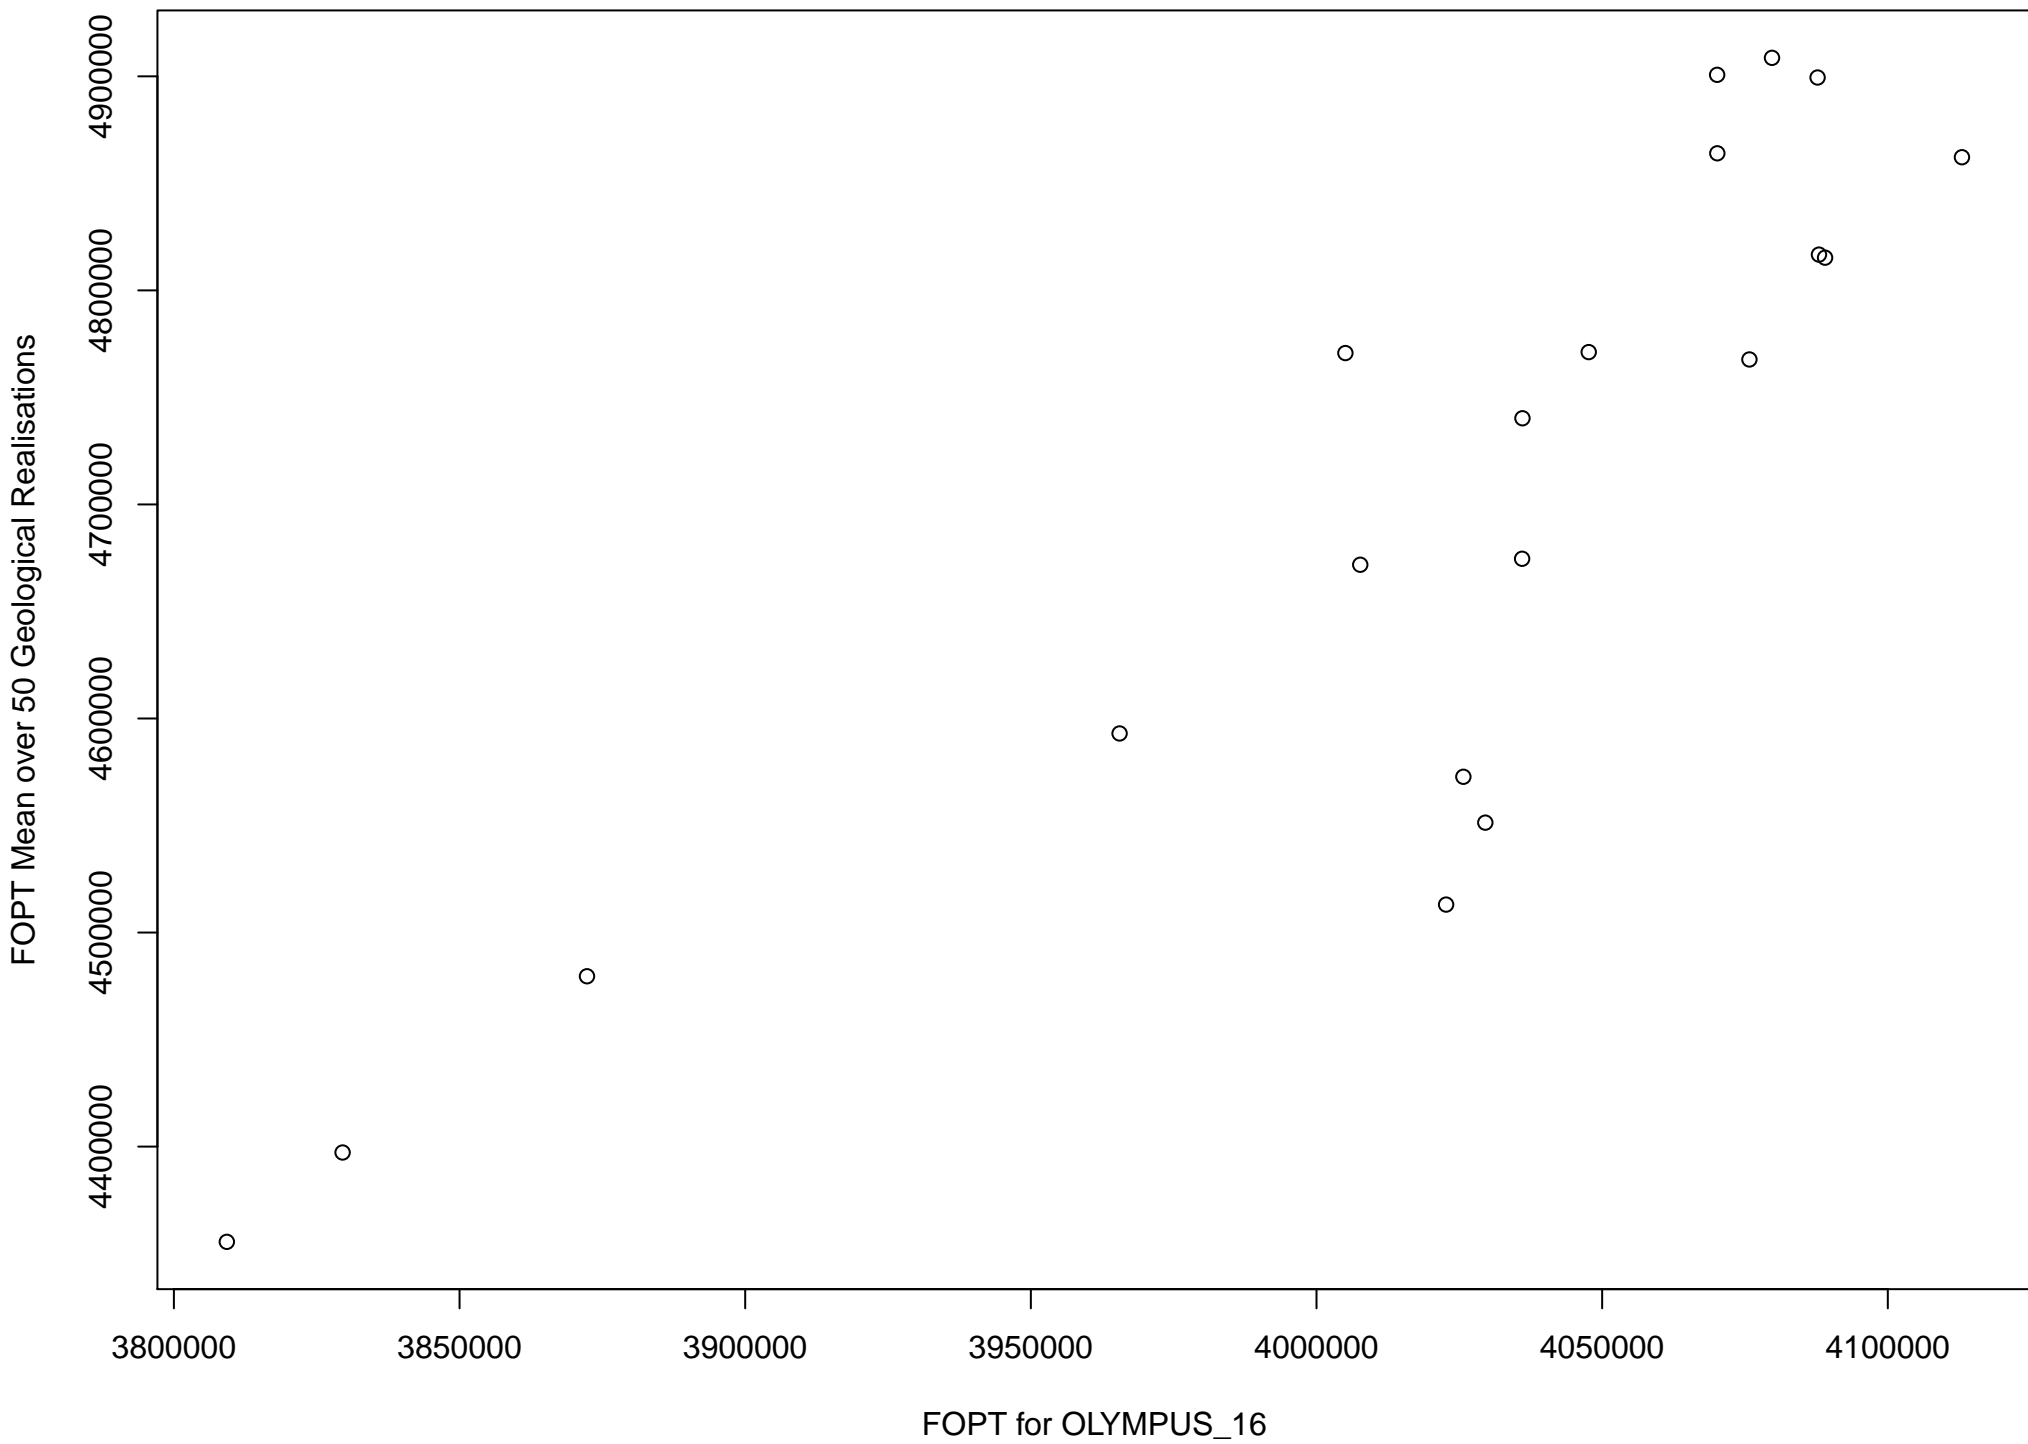



FOPT for OLYMPUS\_17

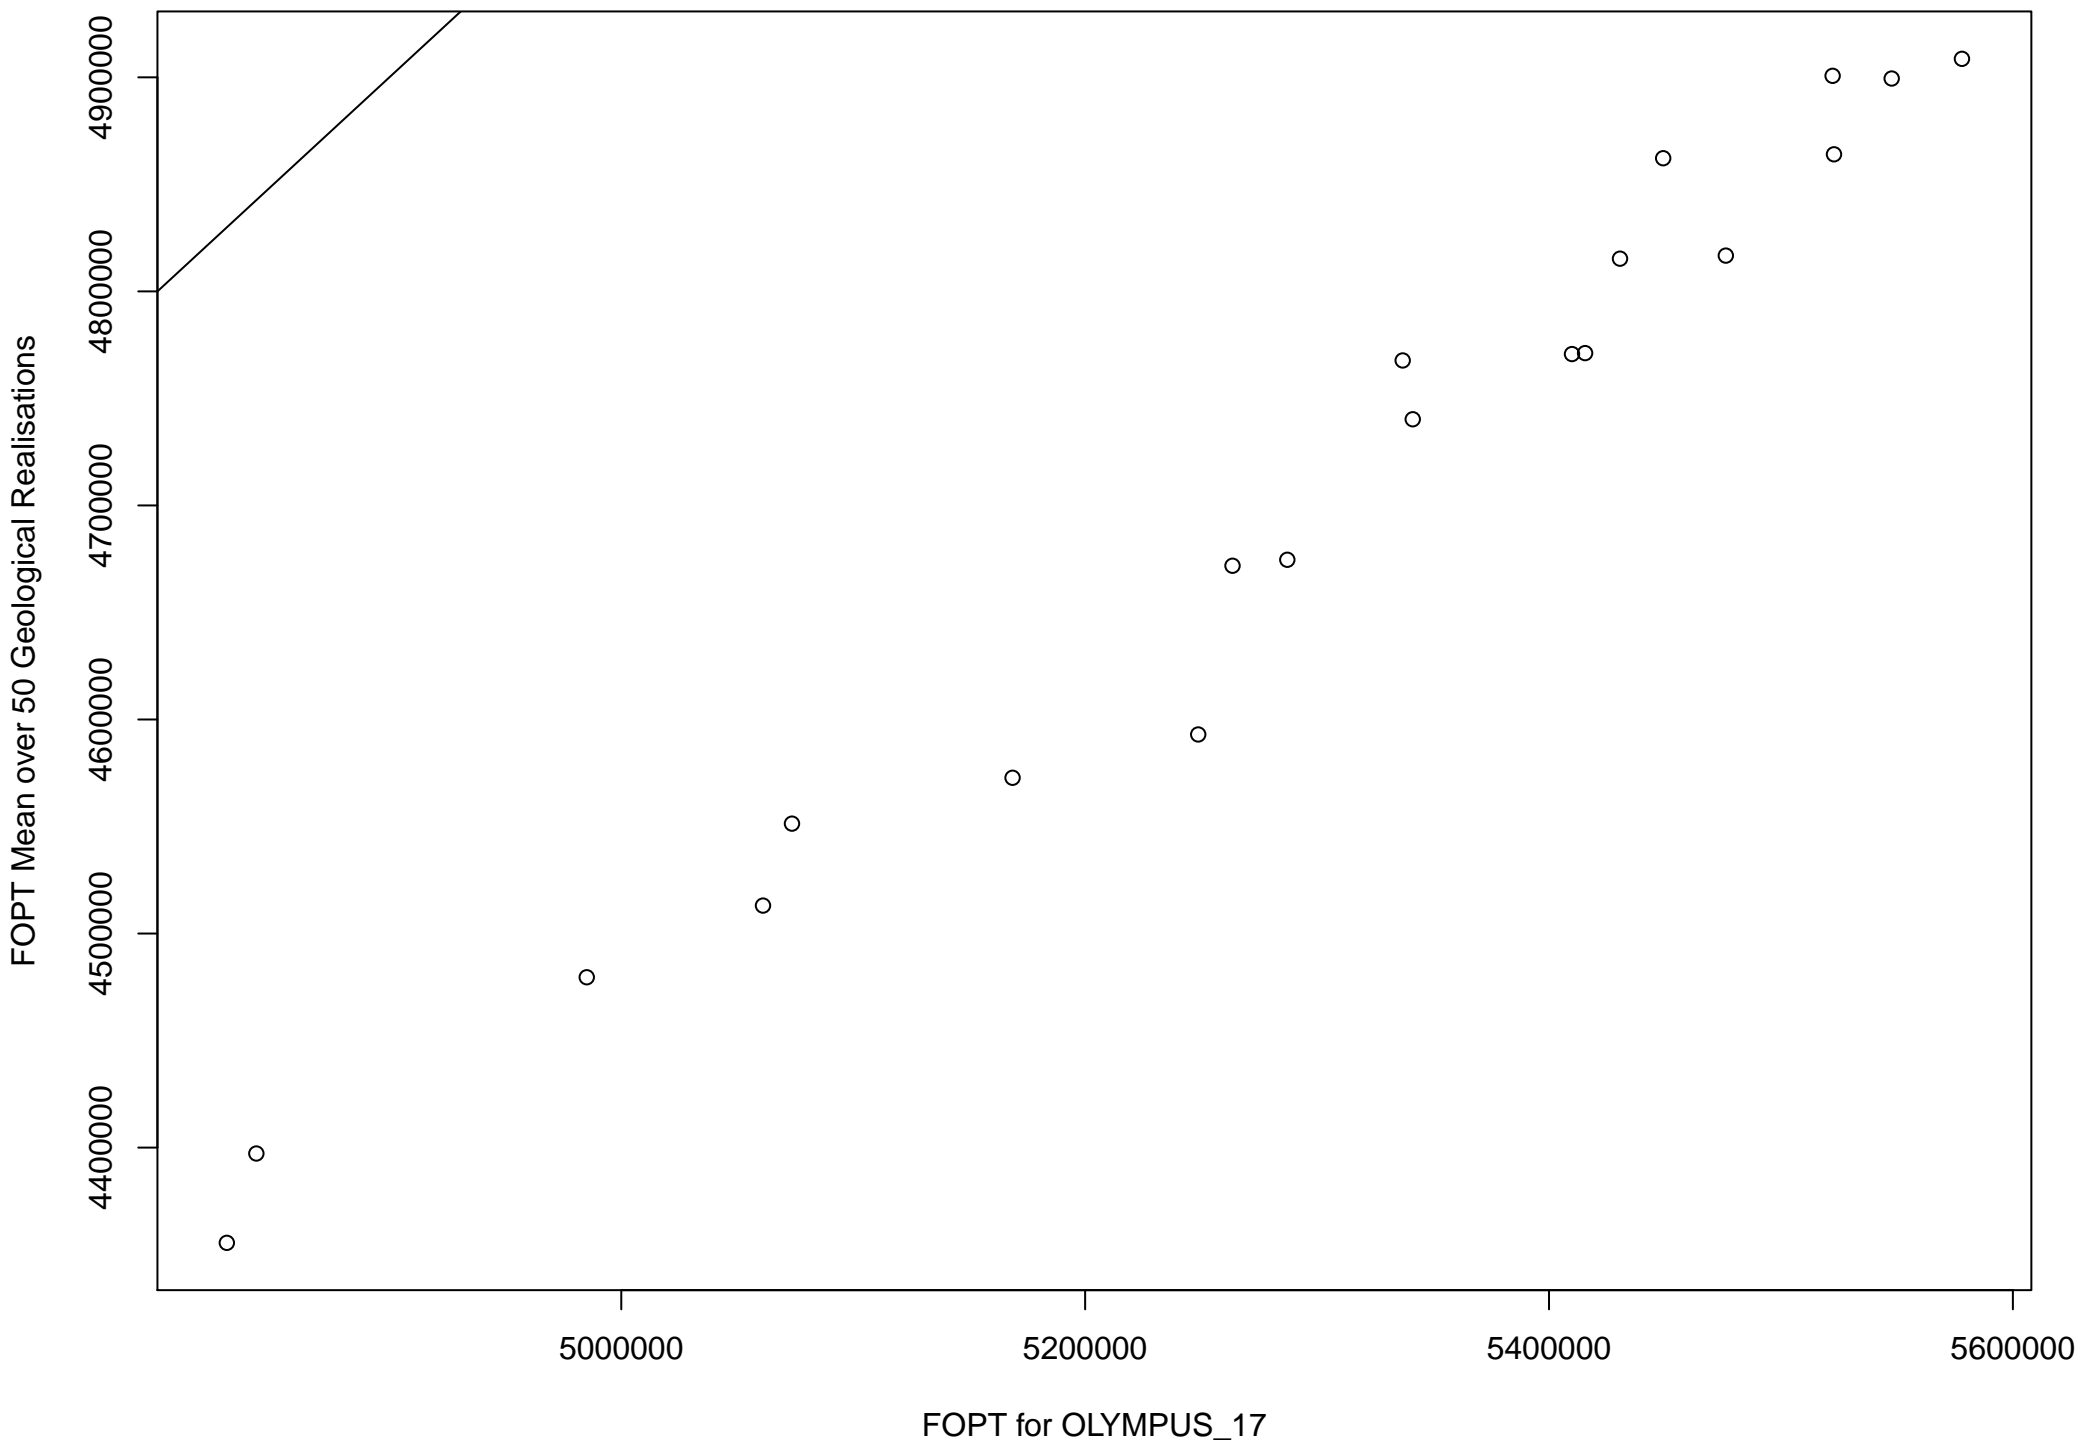

FOPT for OLYMPUS\_18

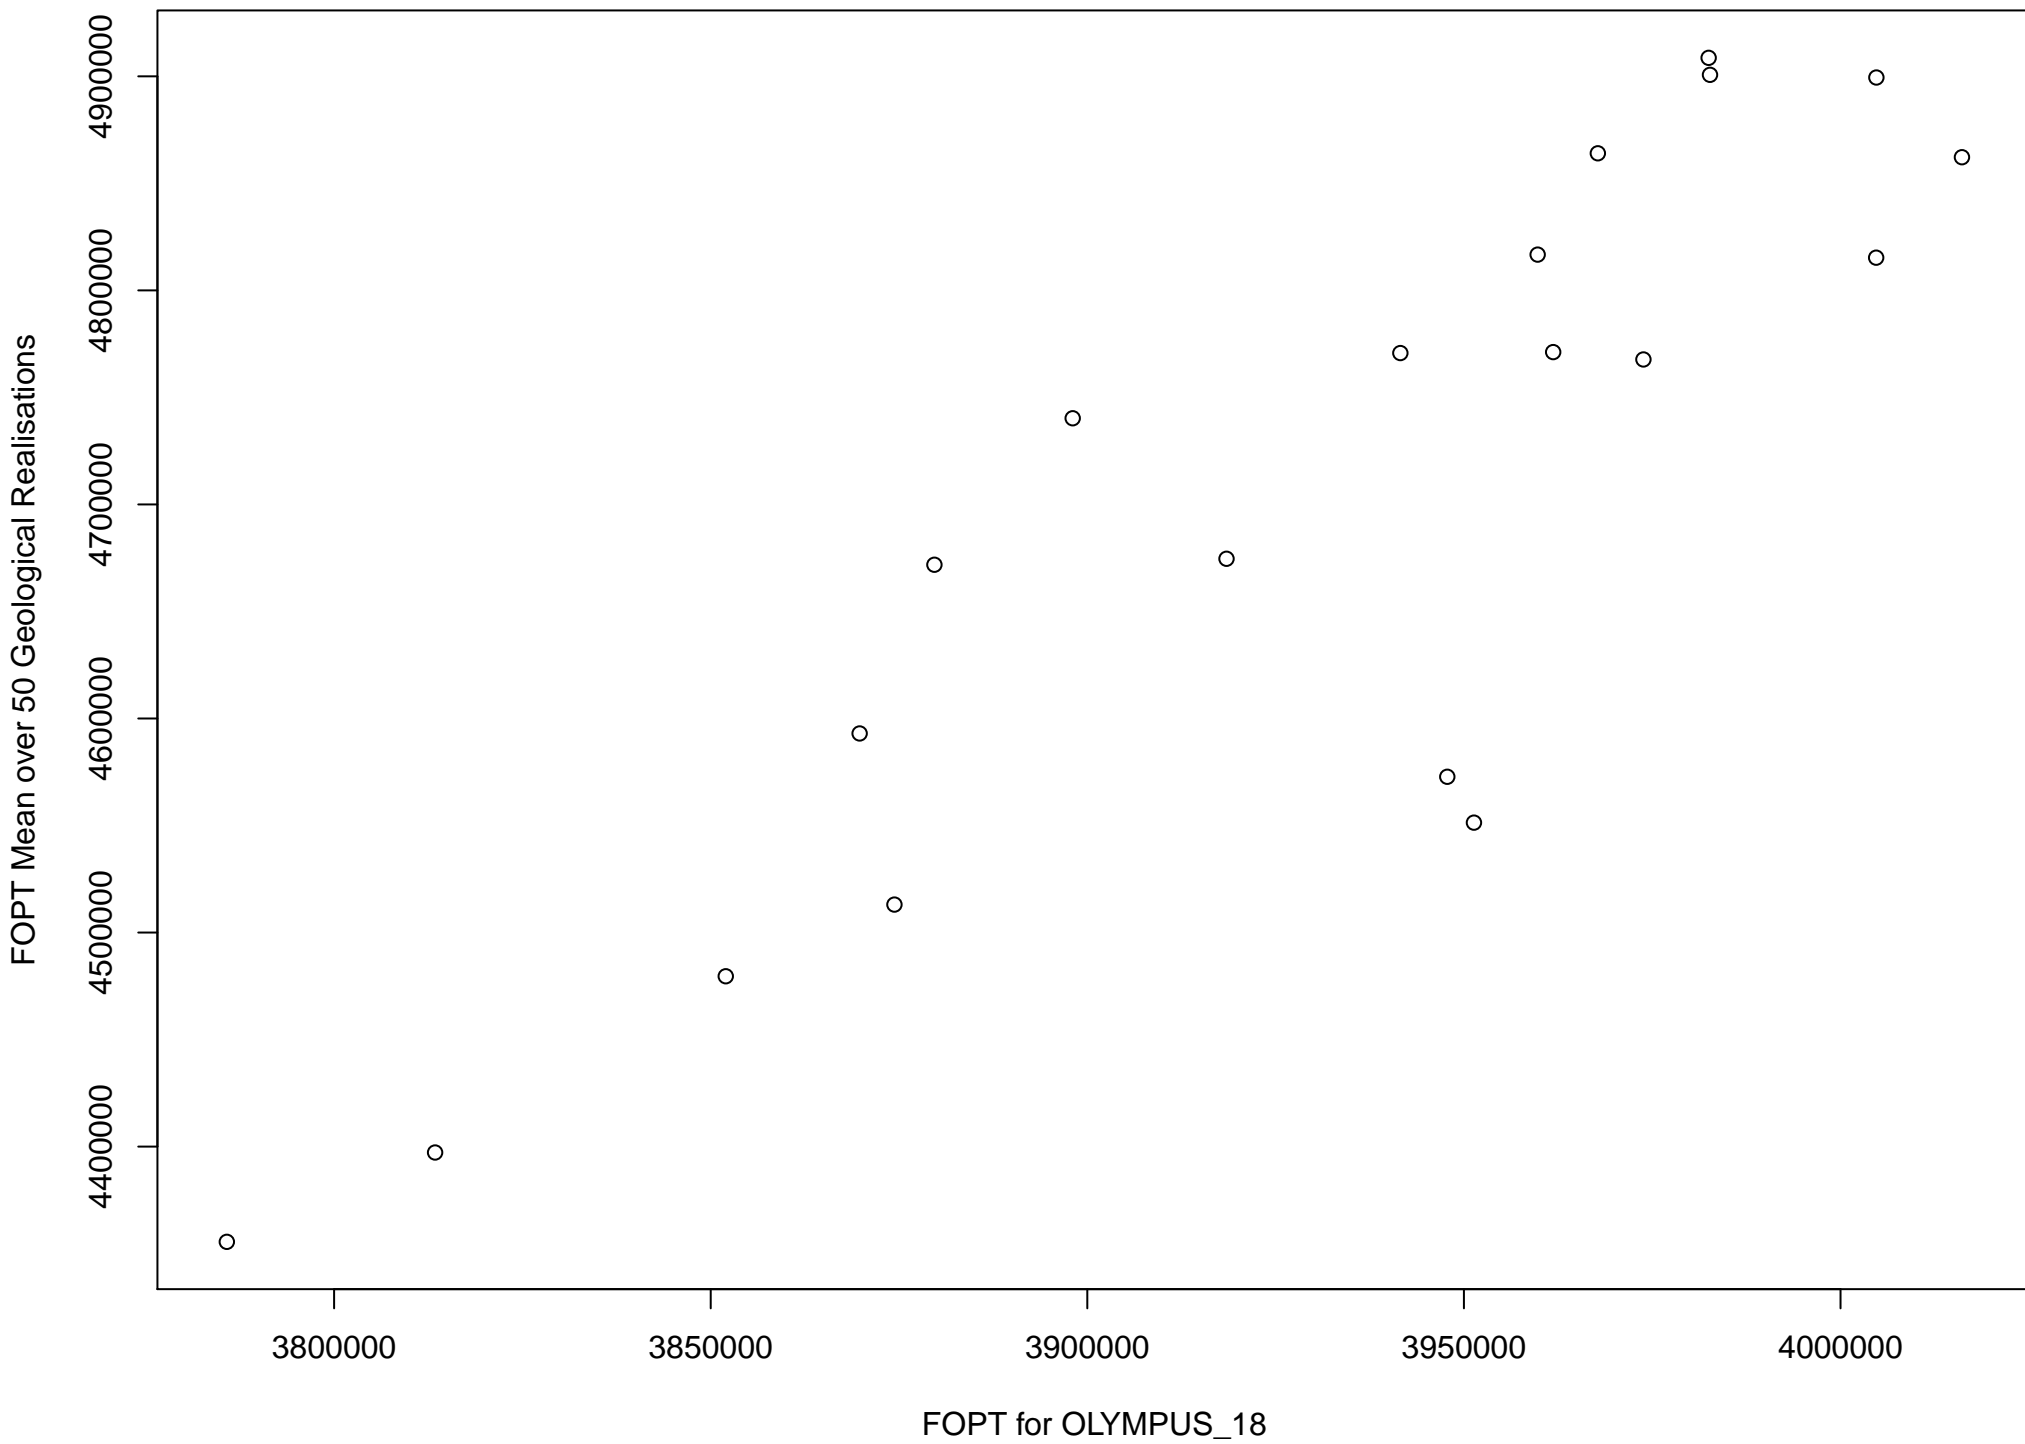

FOPT for OLYMPUS\_19

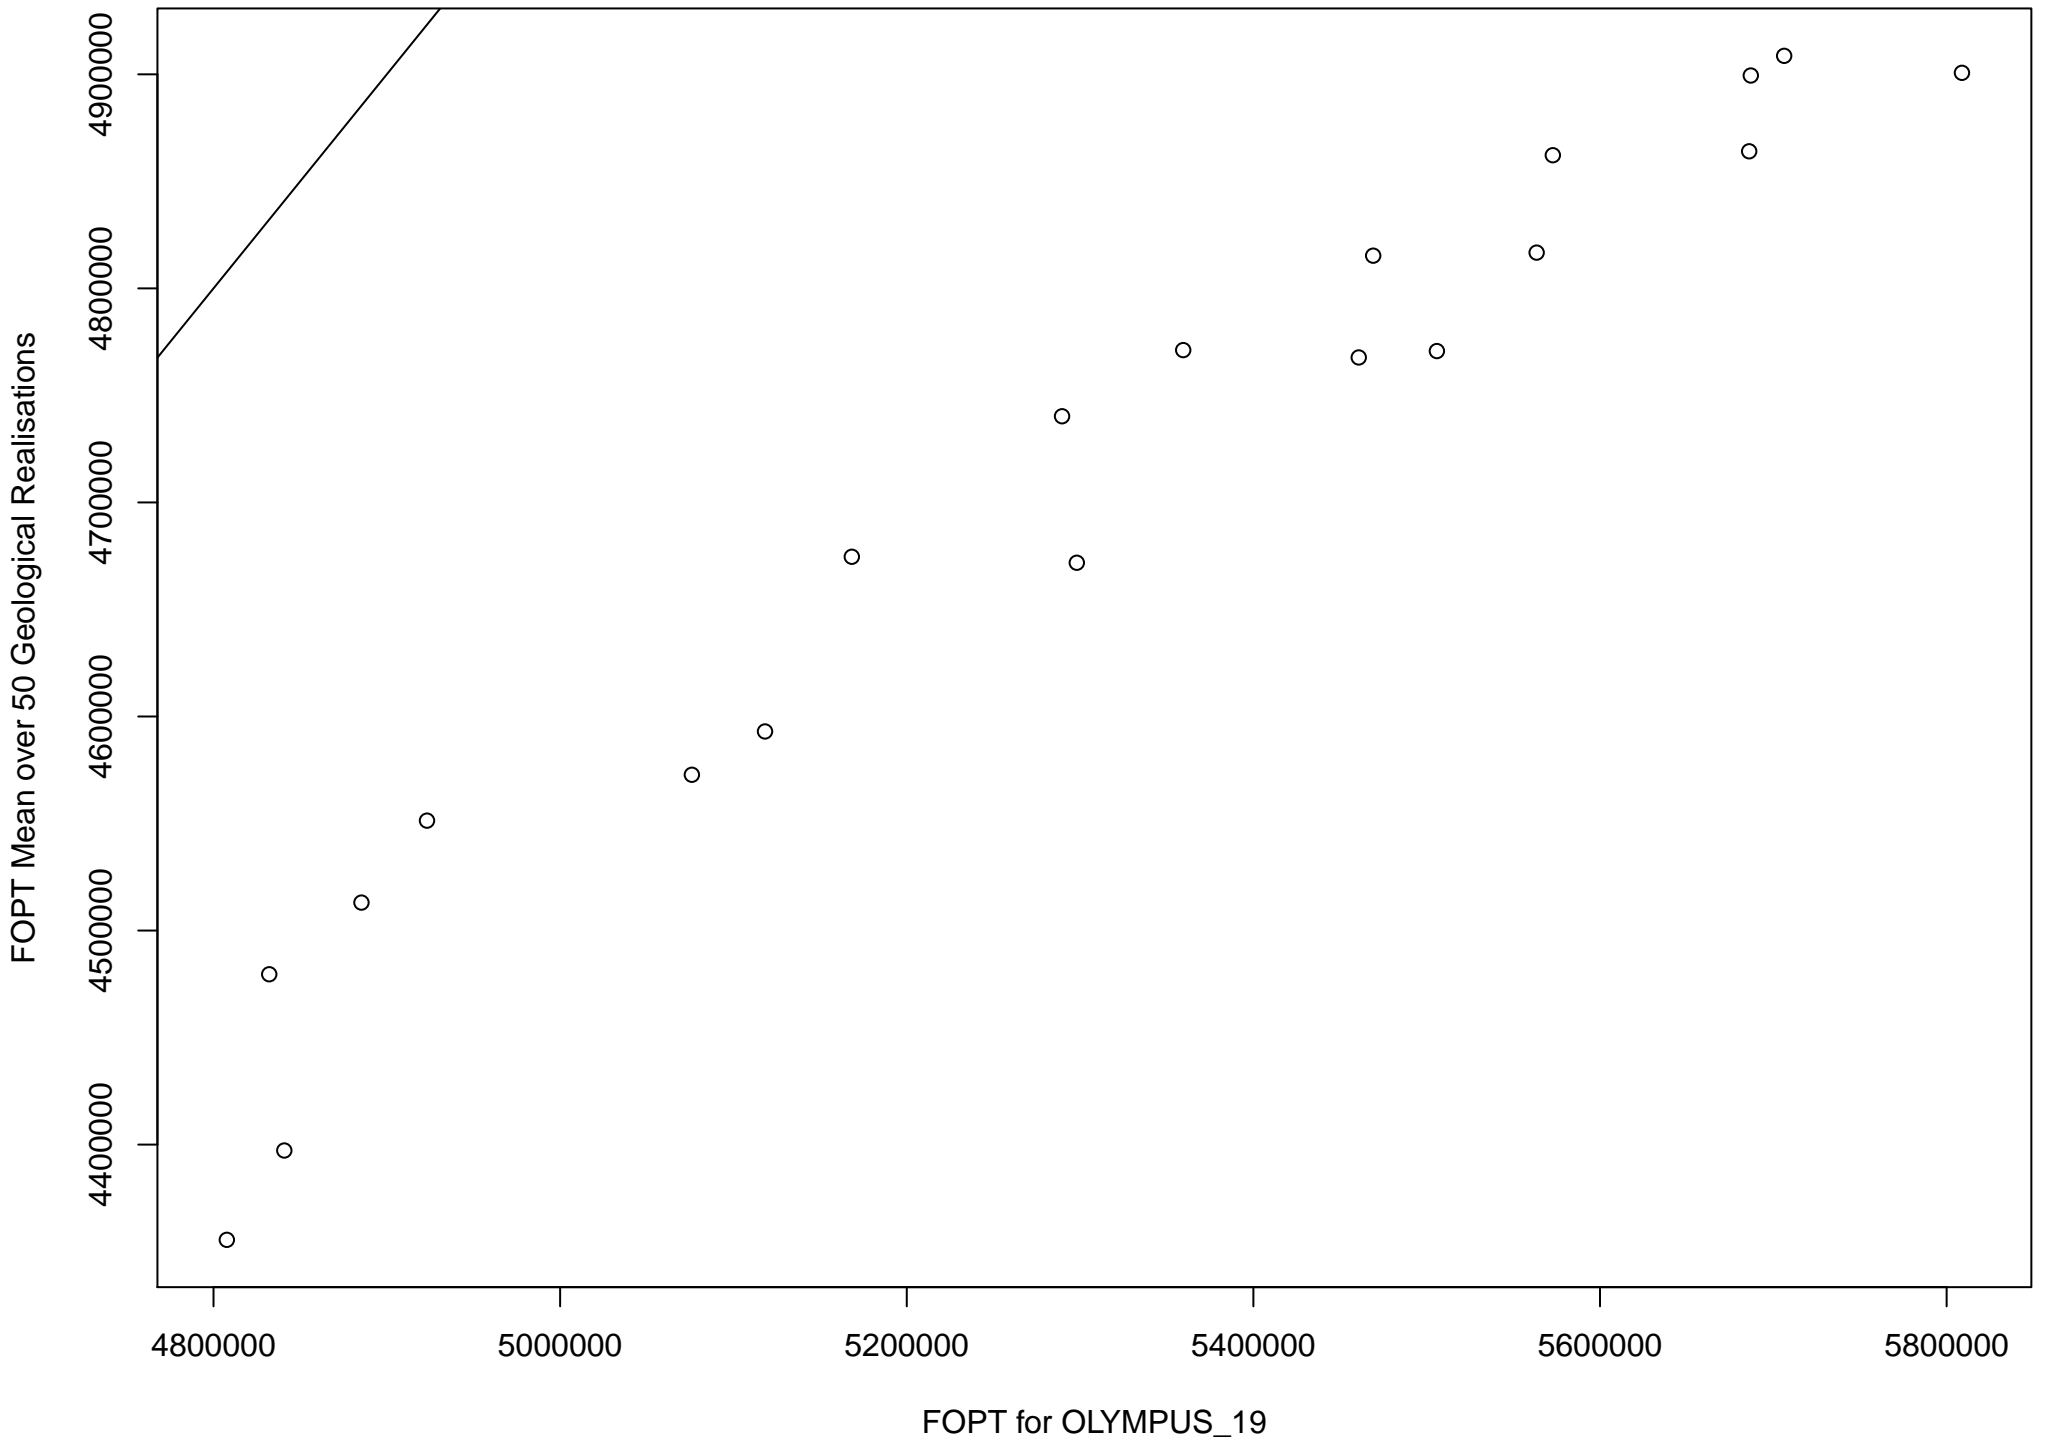

FOPT for OLYMPUS\_20

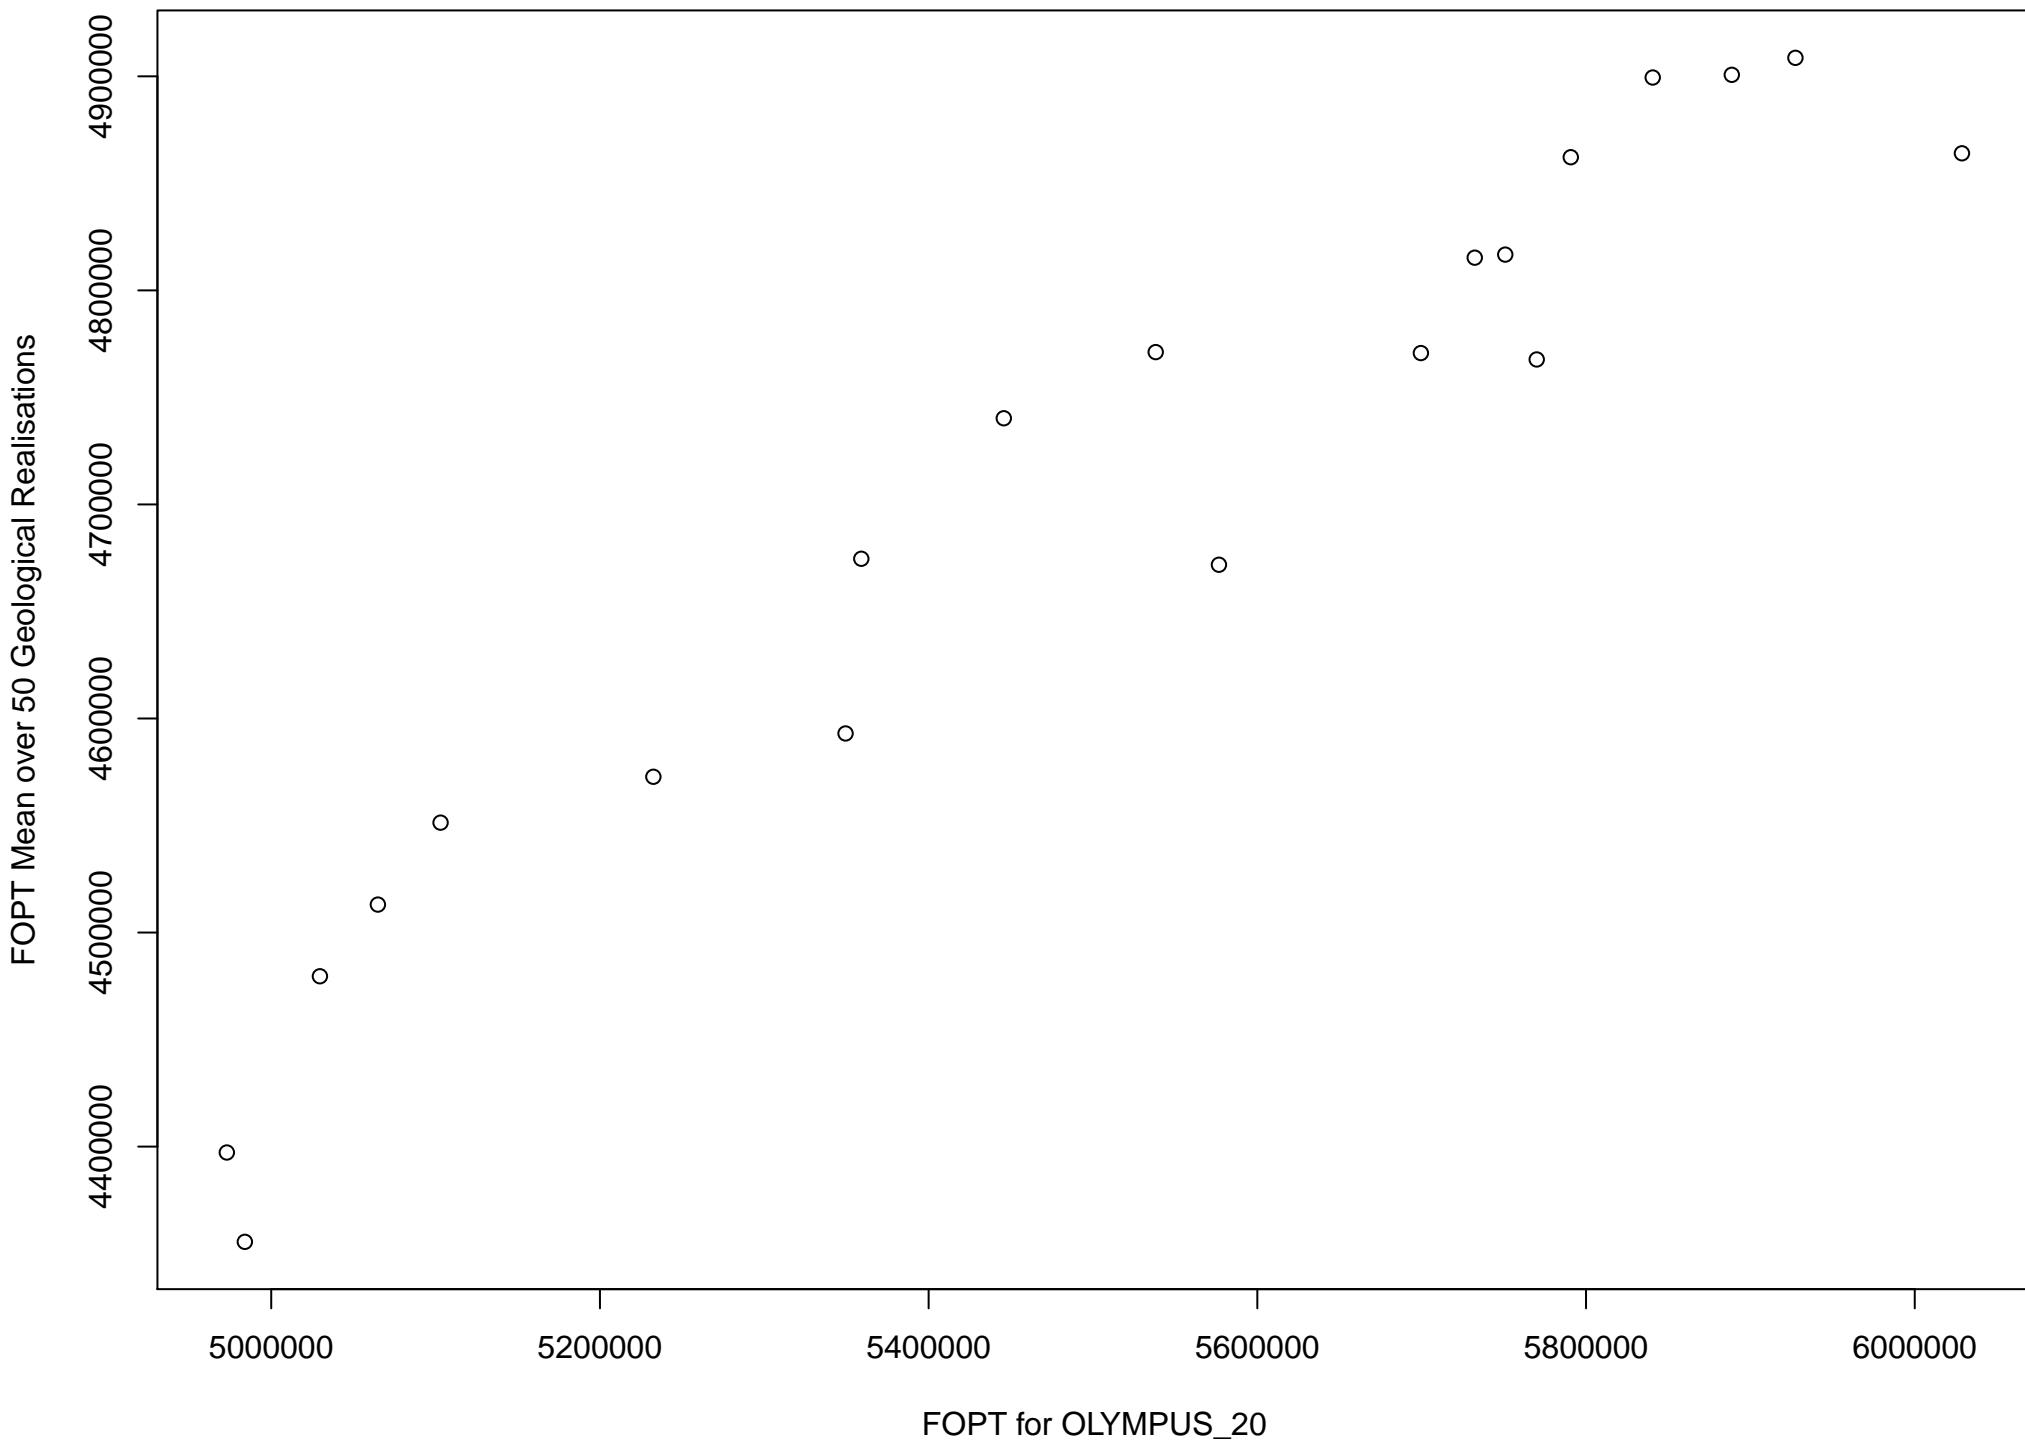

FOPT for OLYMPUS\_21

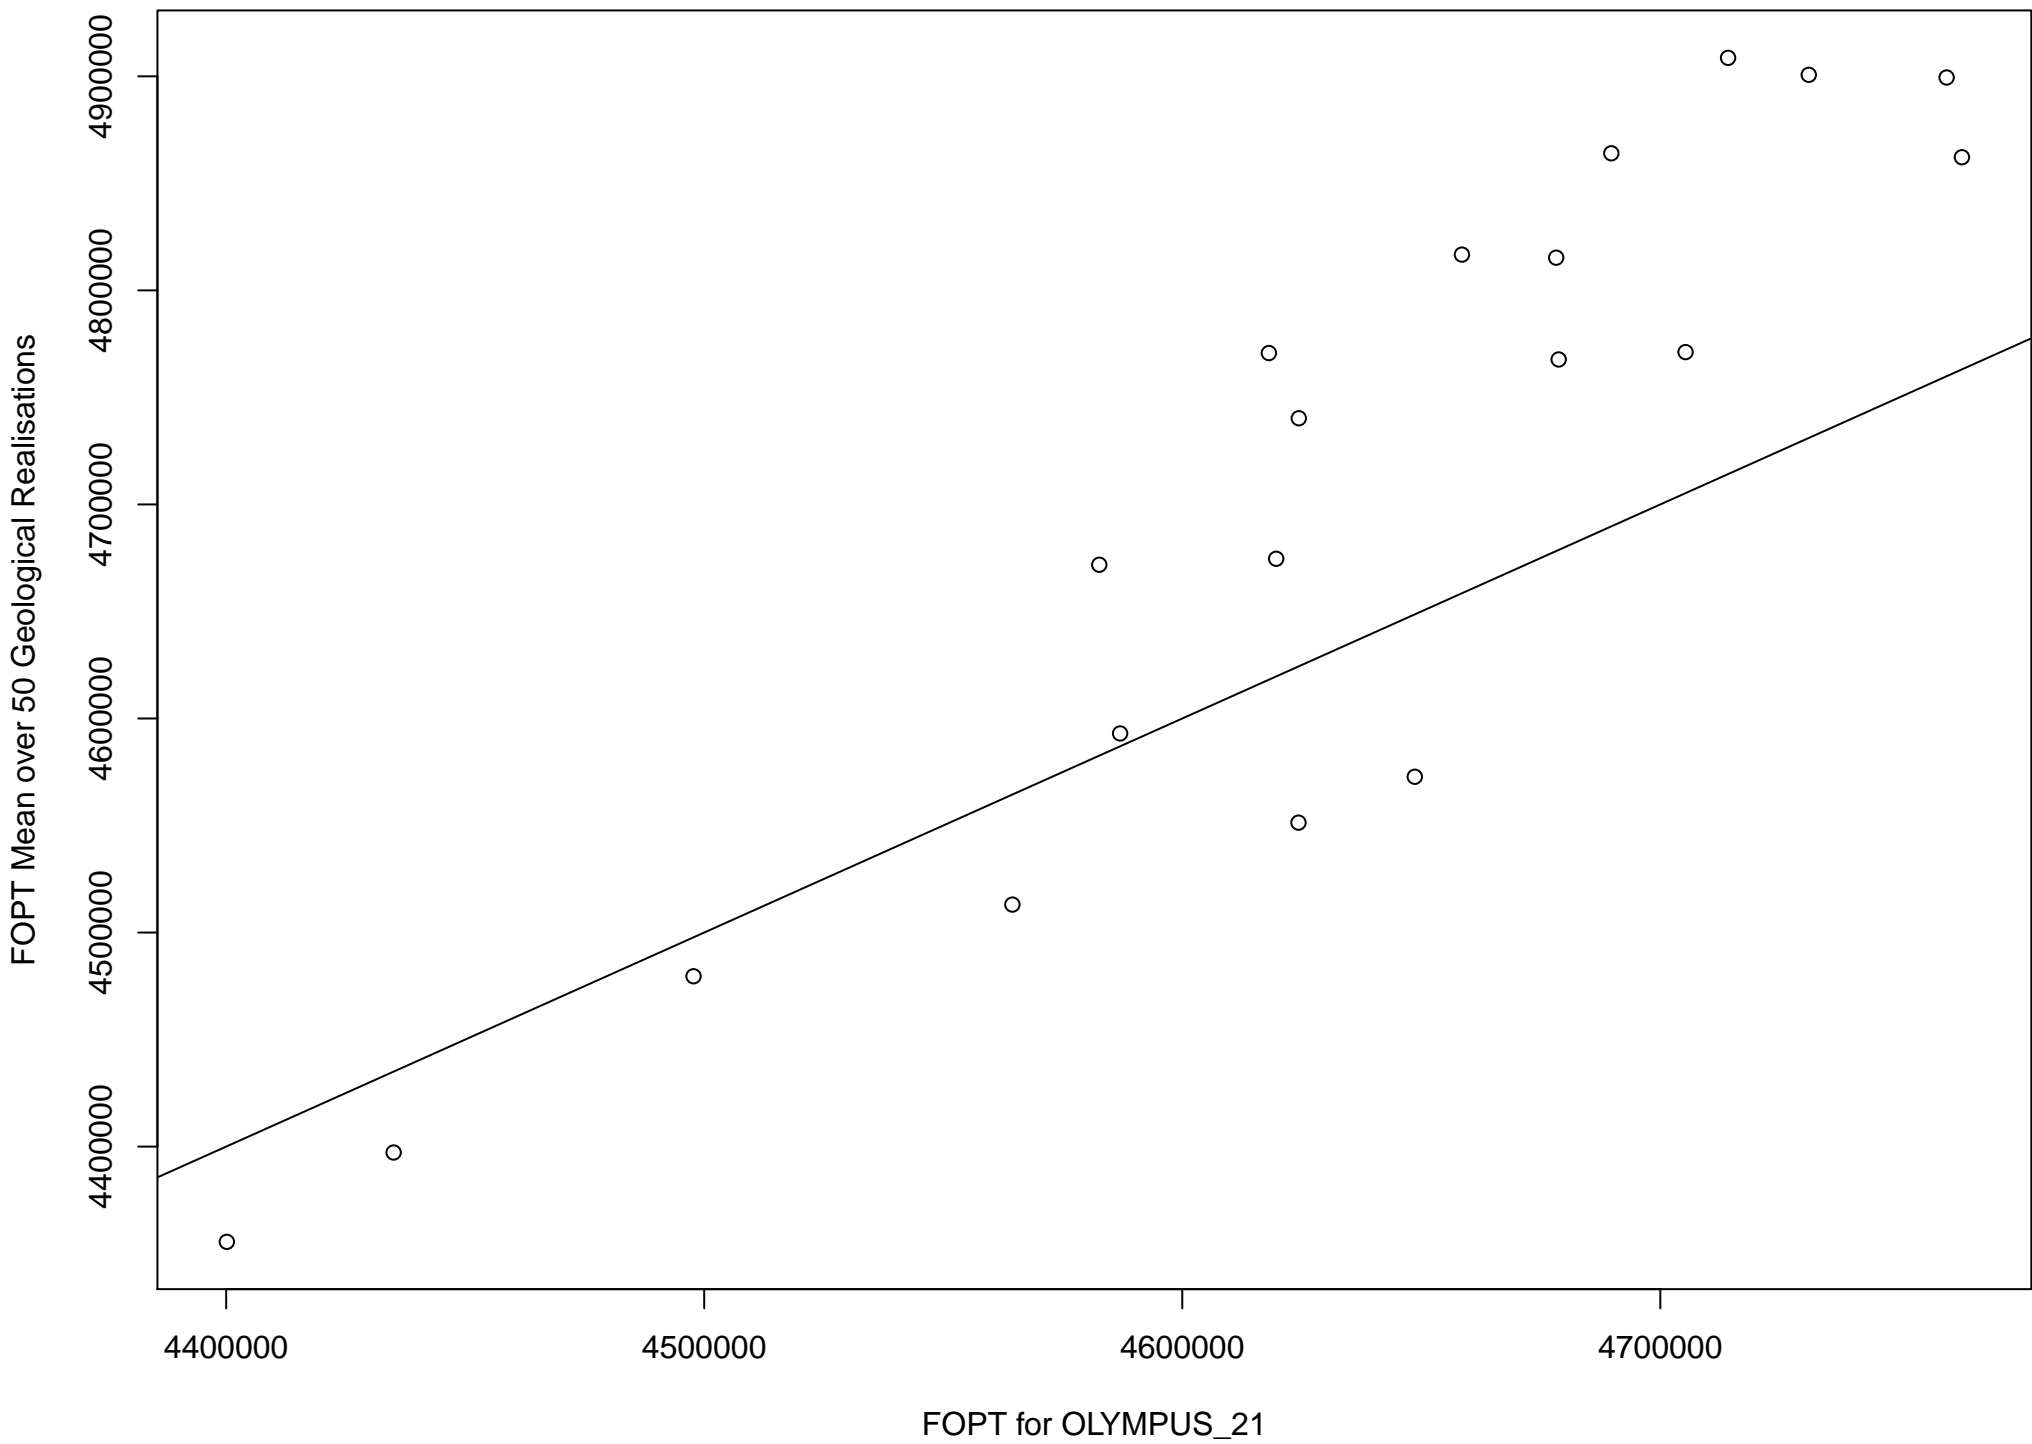

FOPT for OLYMPUS\_22

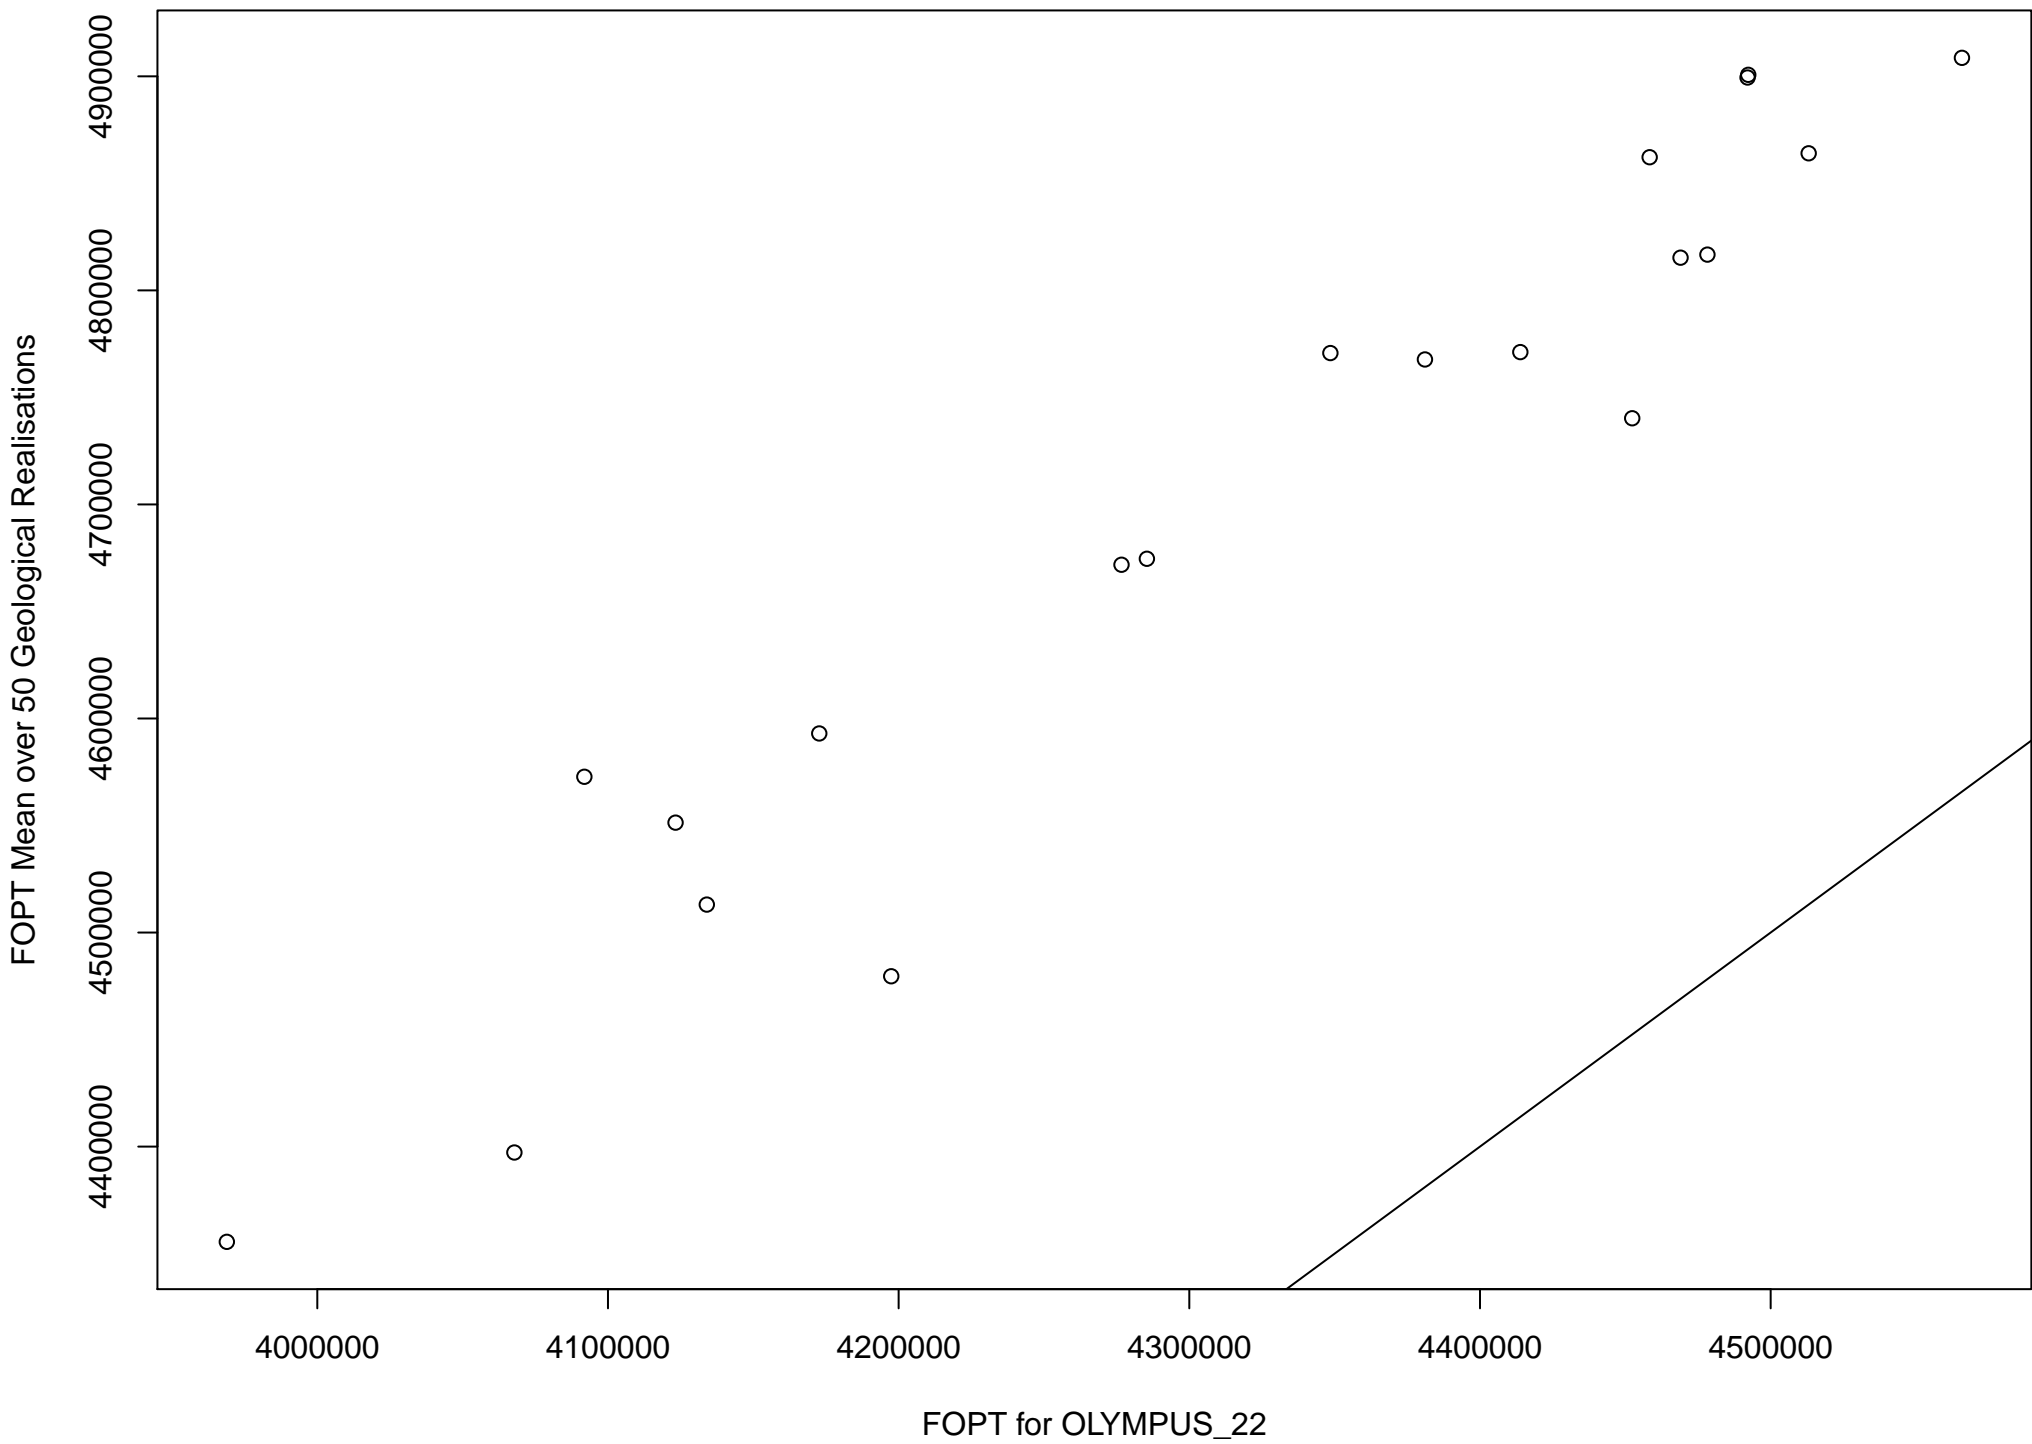

FOPT for OLYMPUS\_23

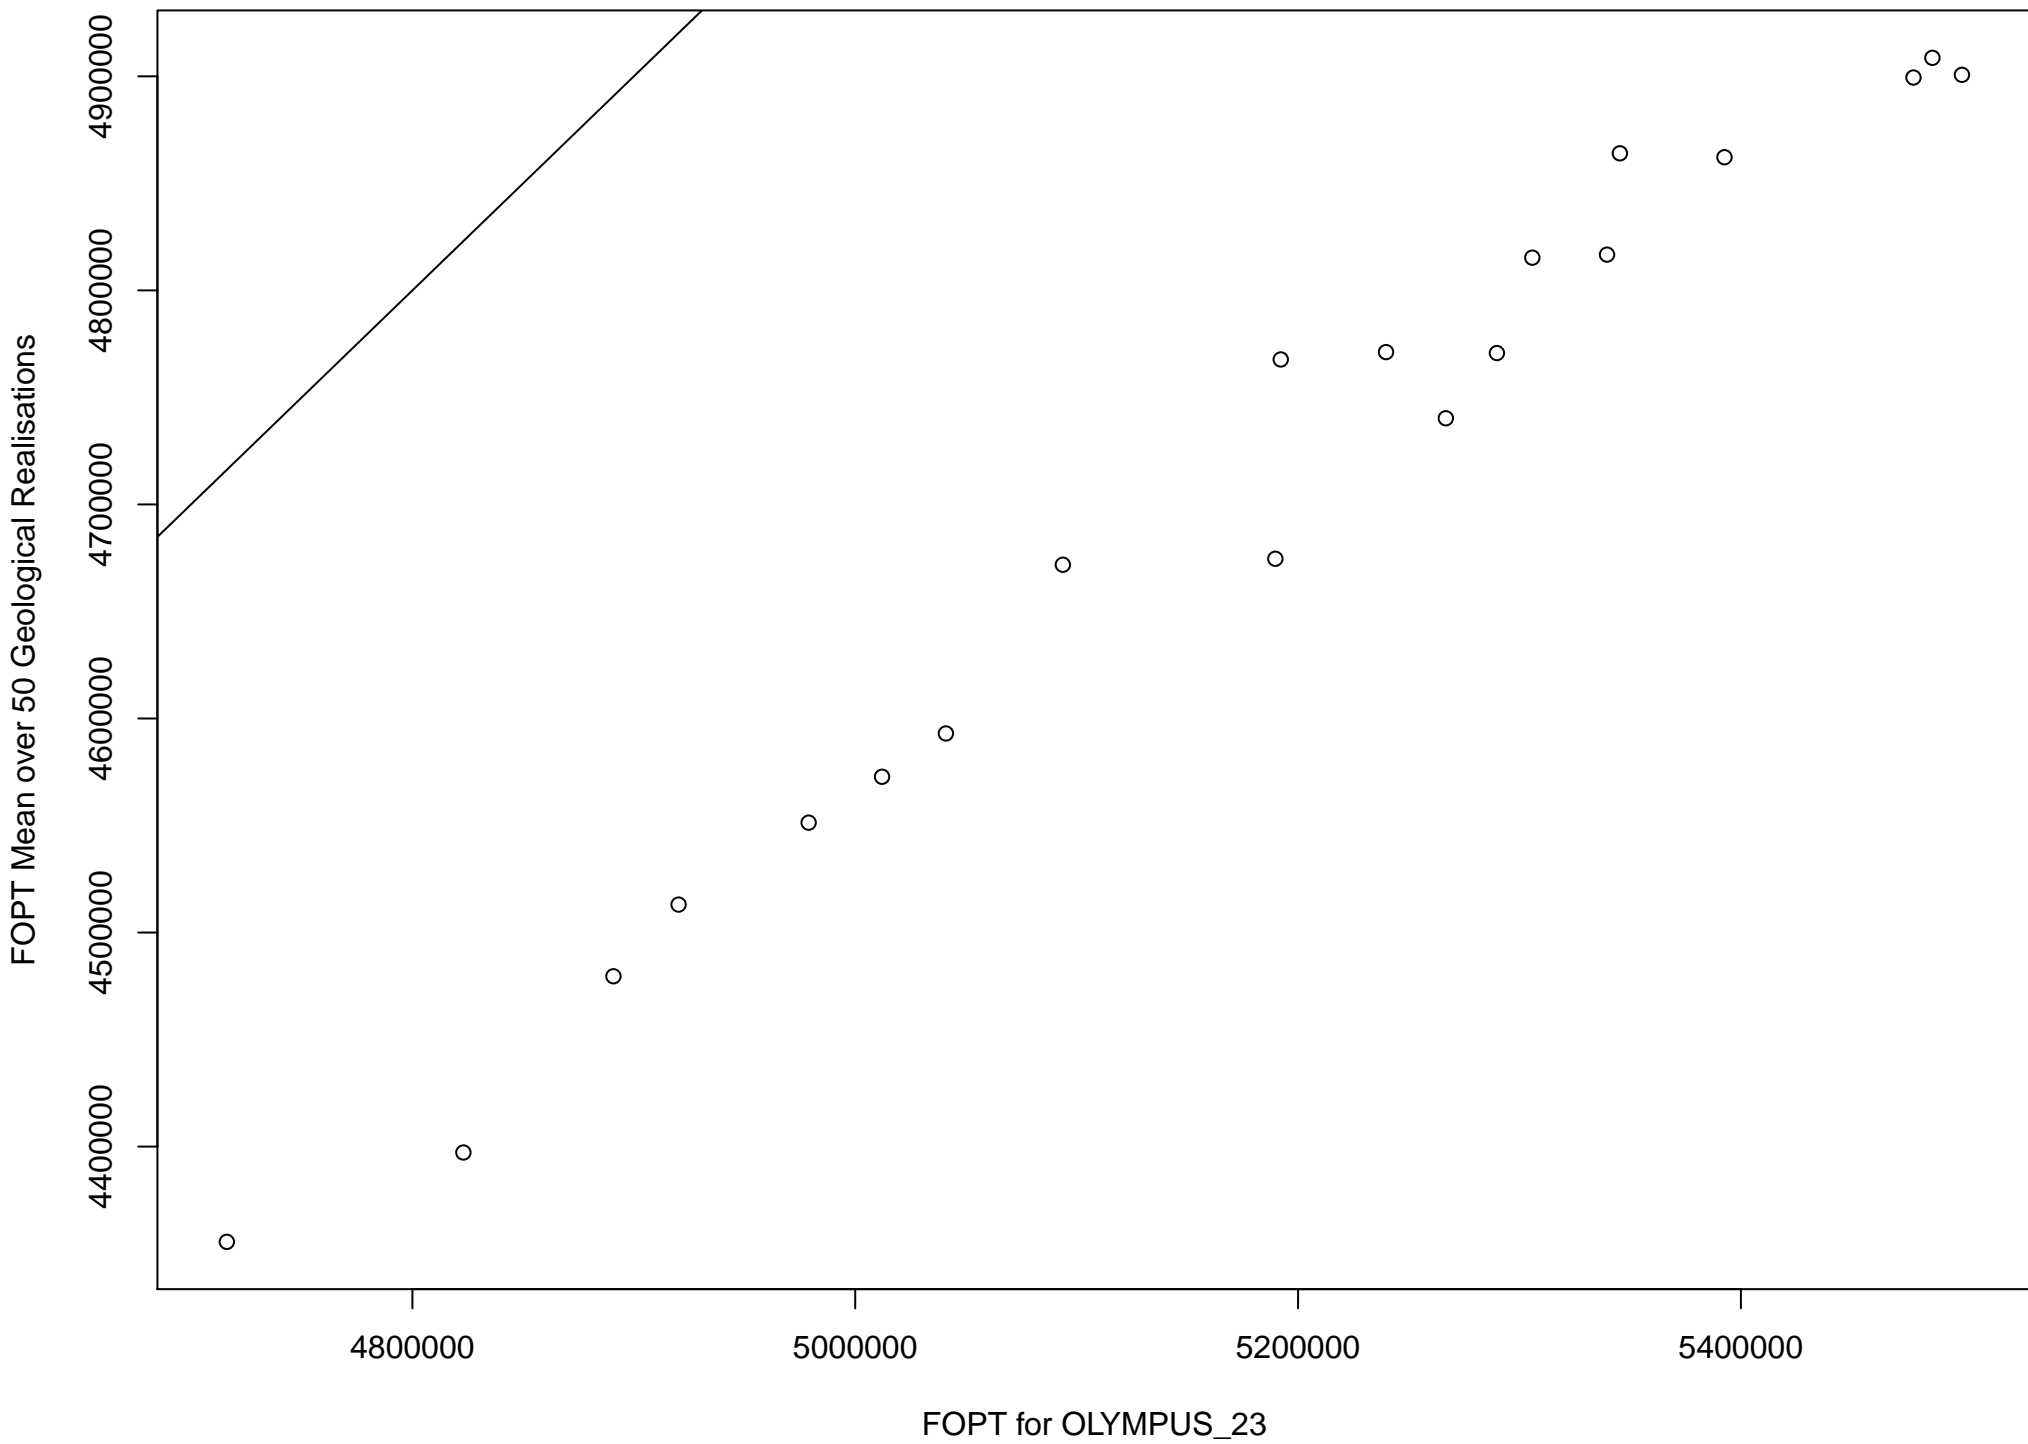

FOPT for OLYMPUS\_24

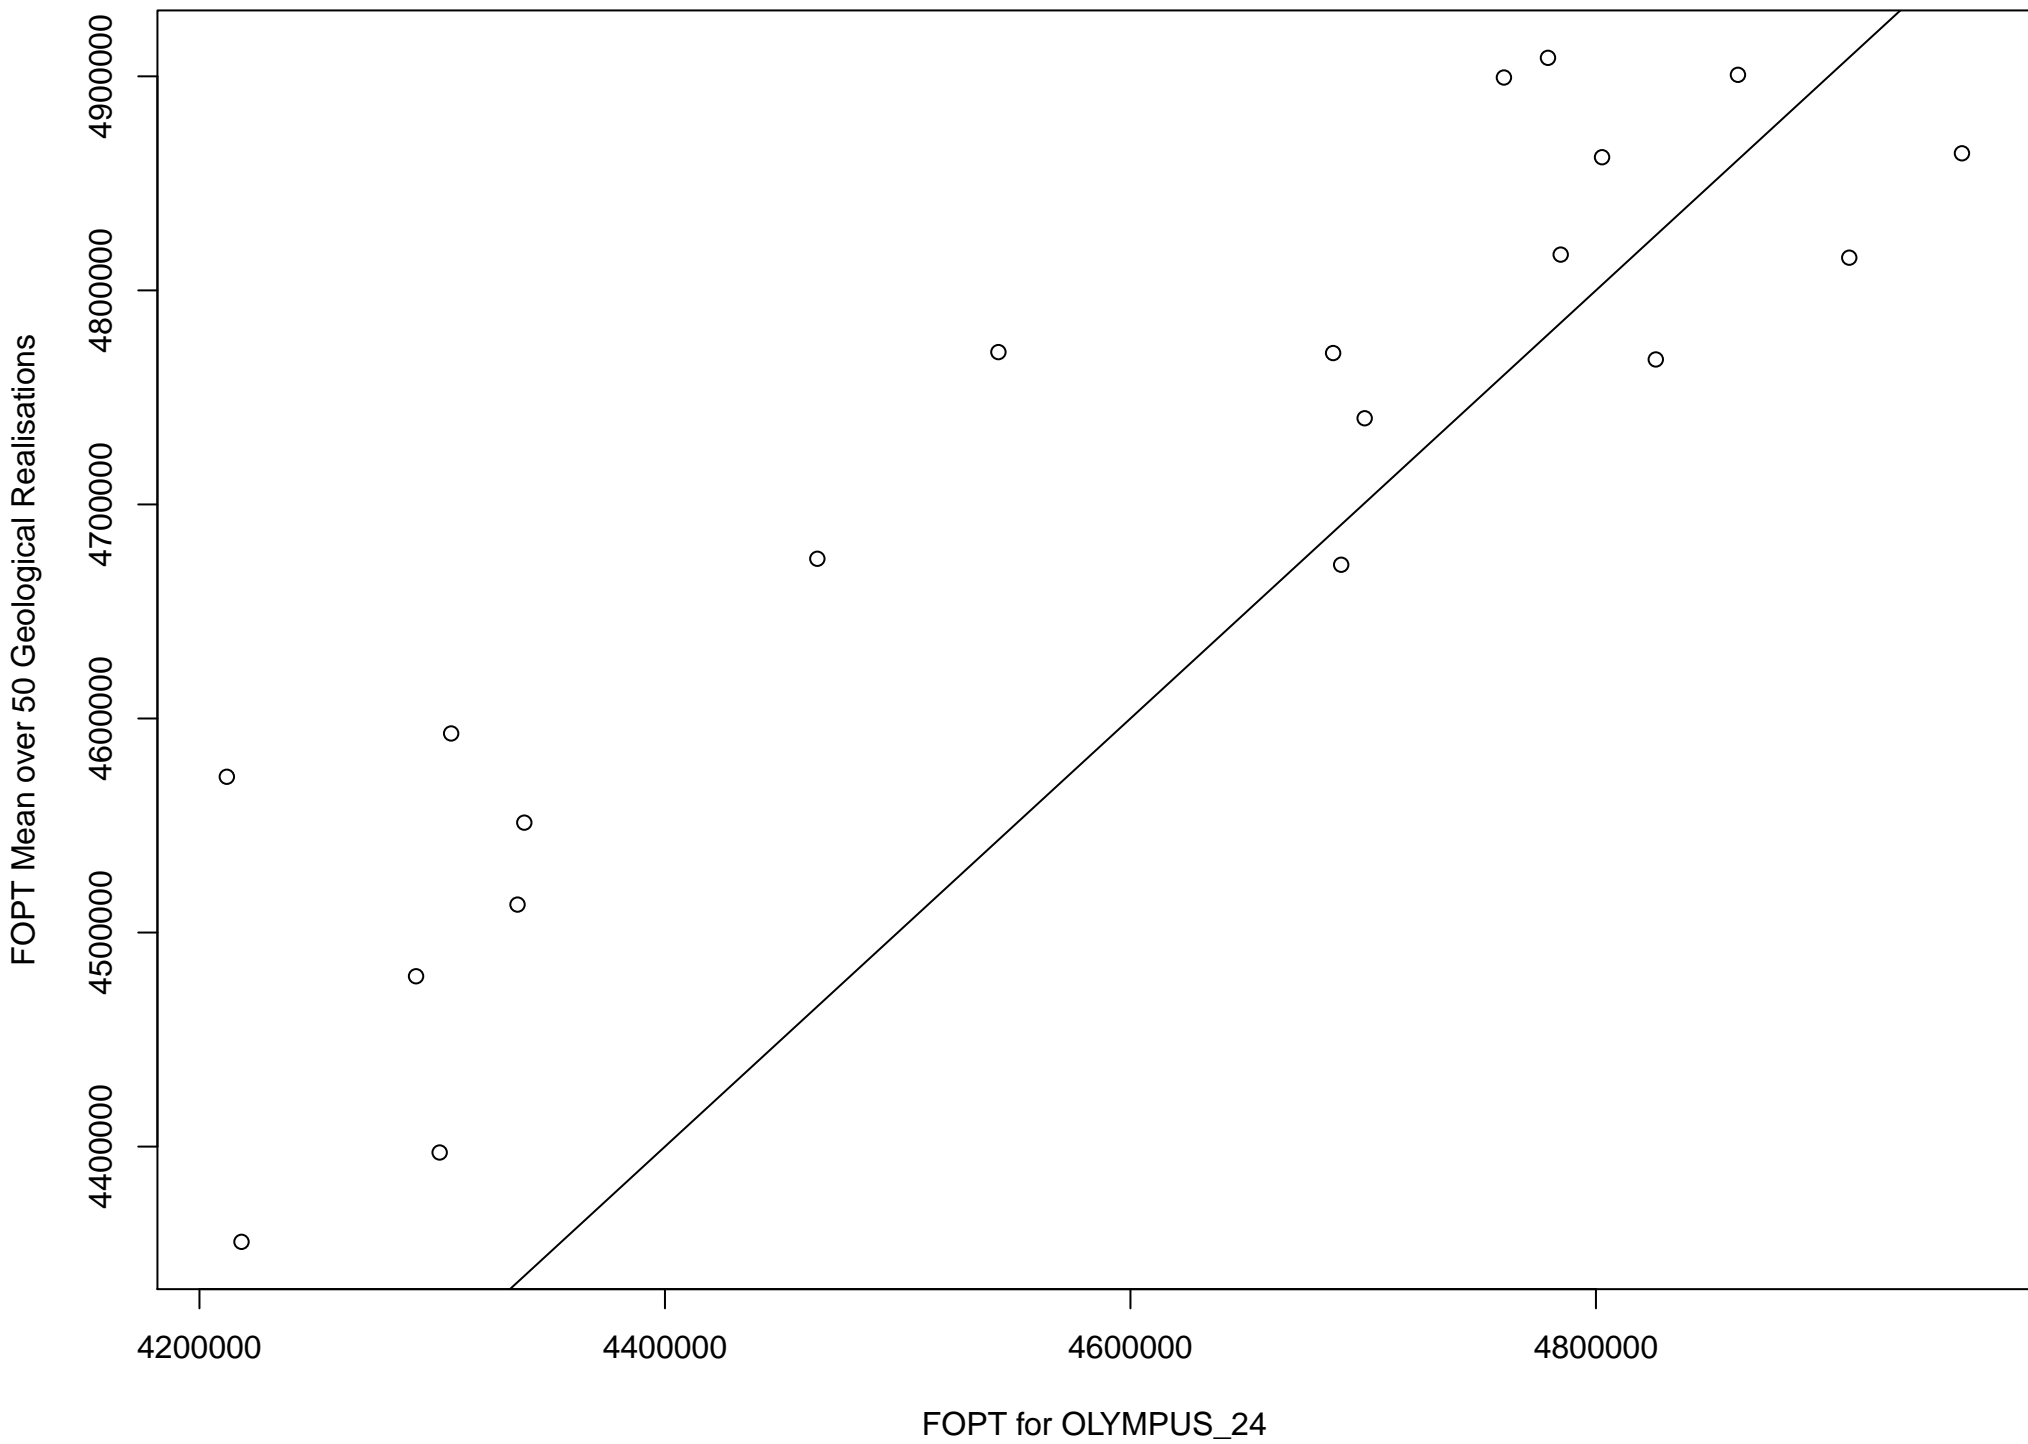



FOPT for OLYMPUS\_25

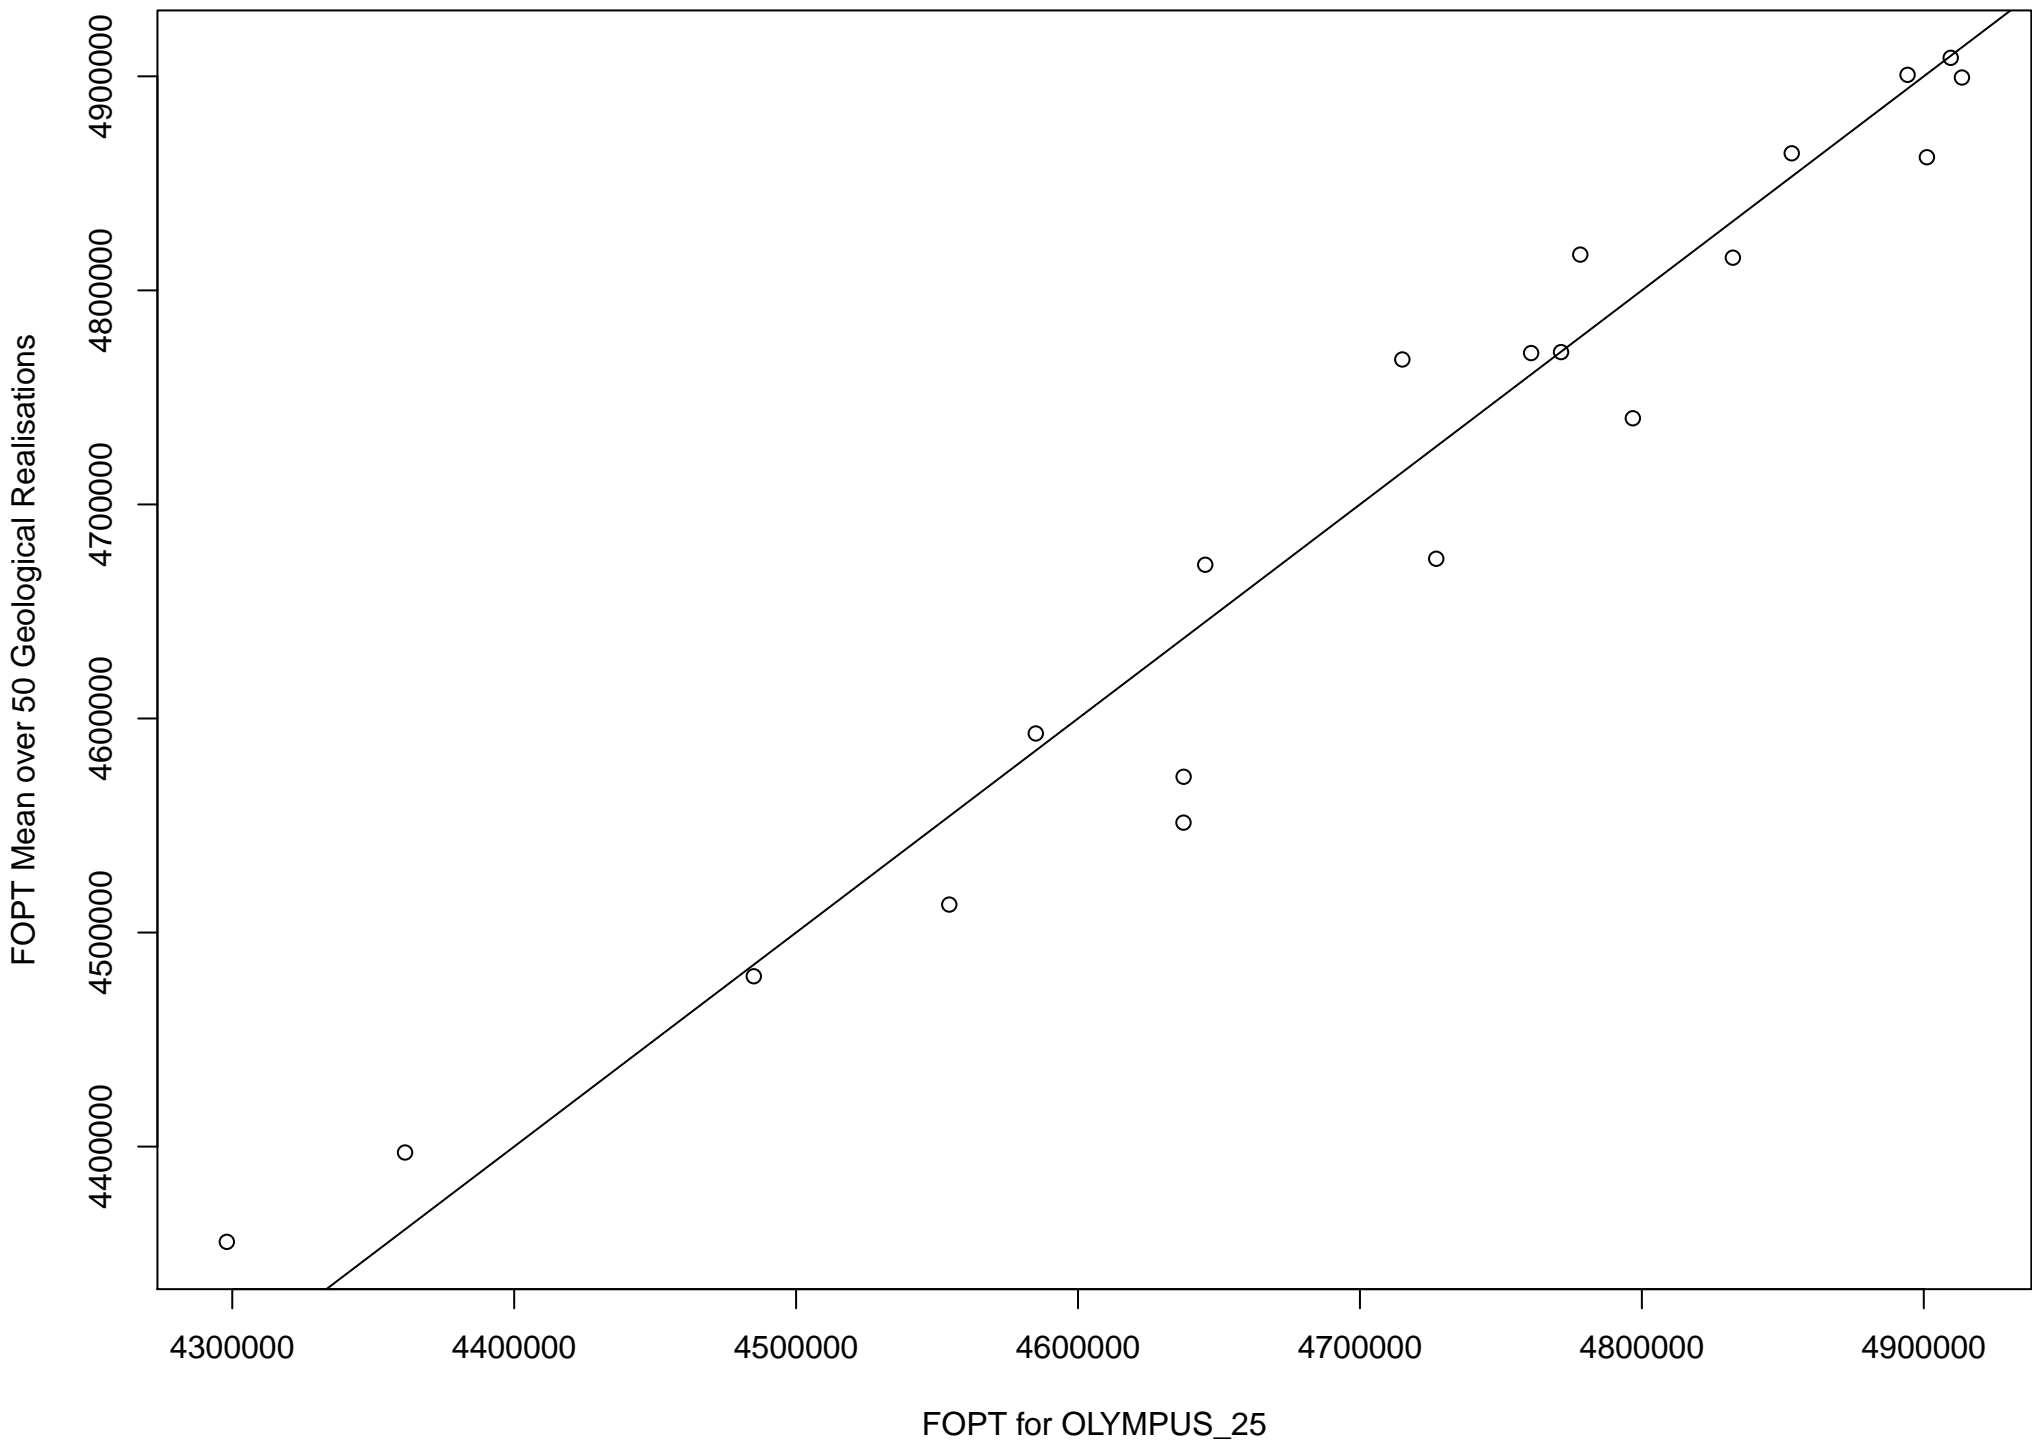

FOPT for OLYMPUS\_26

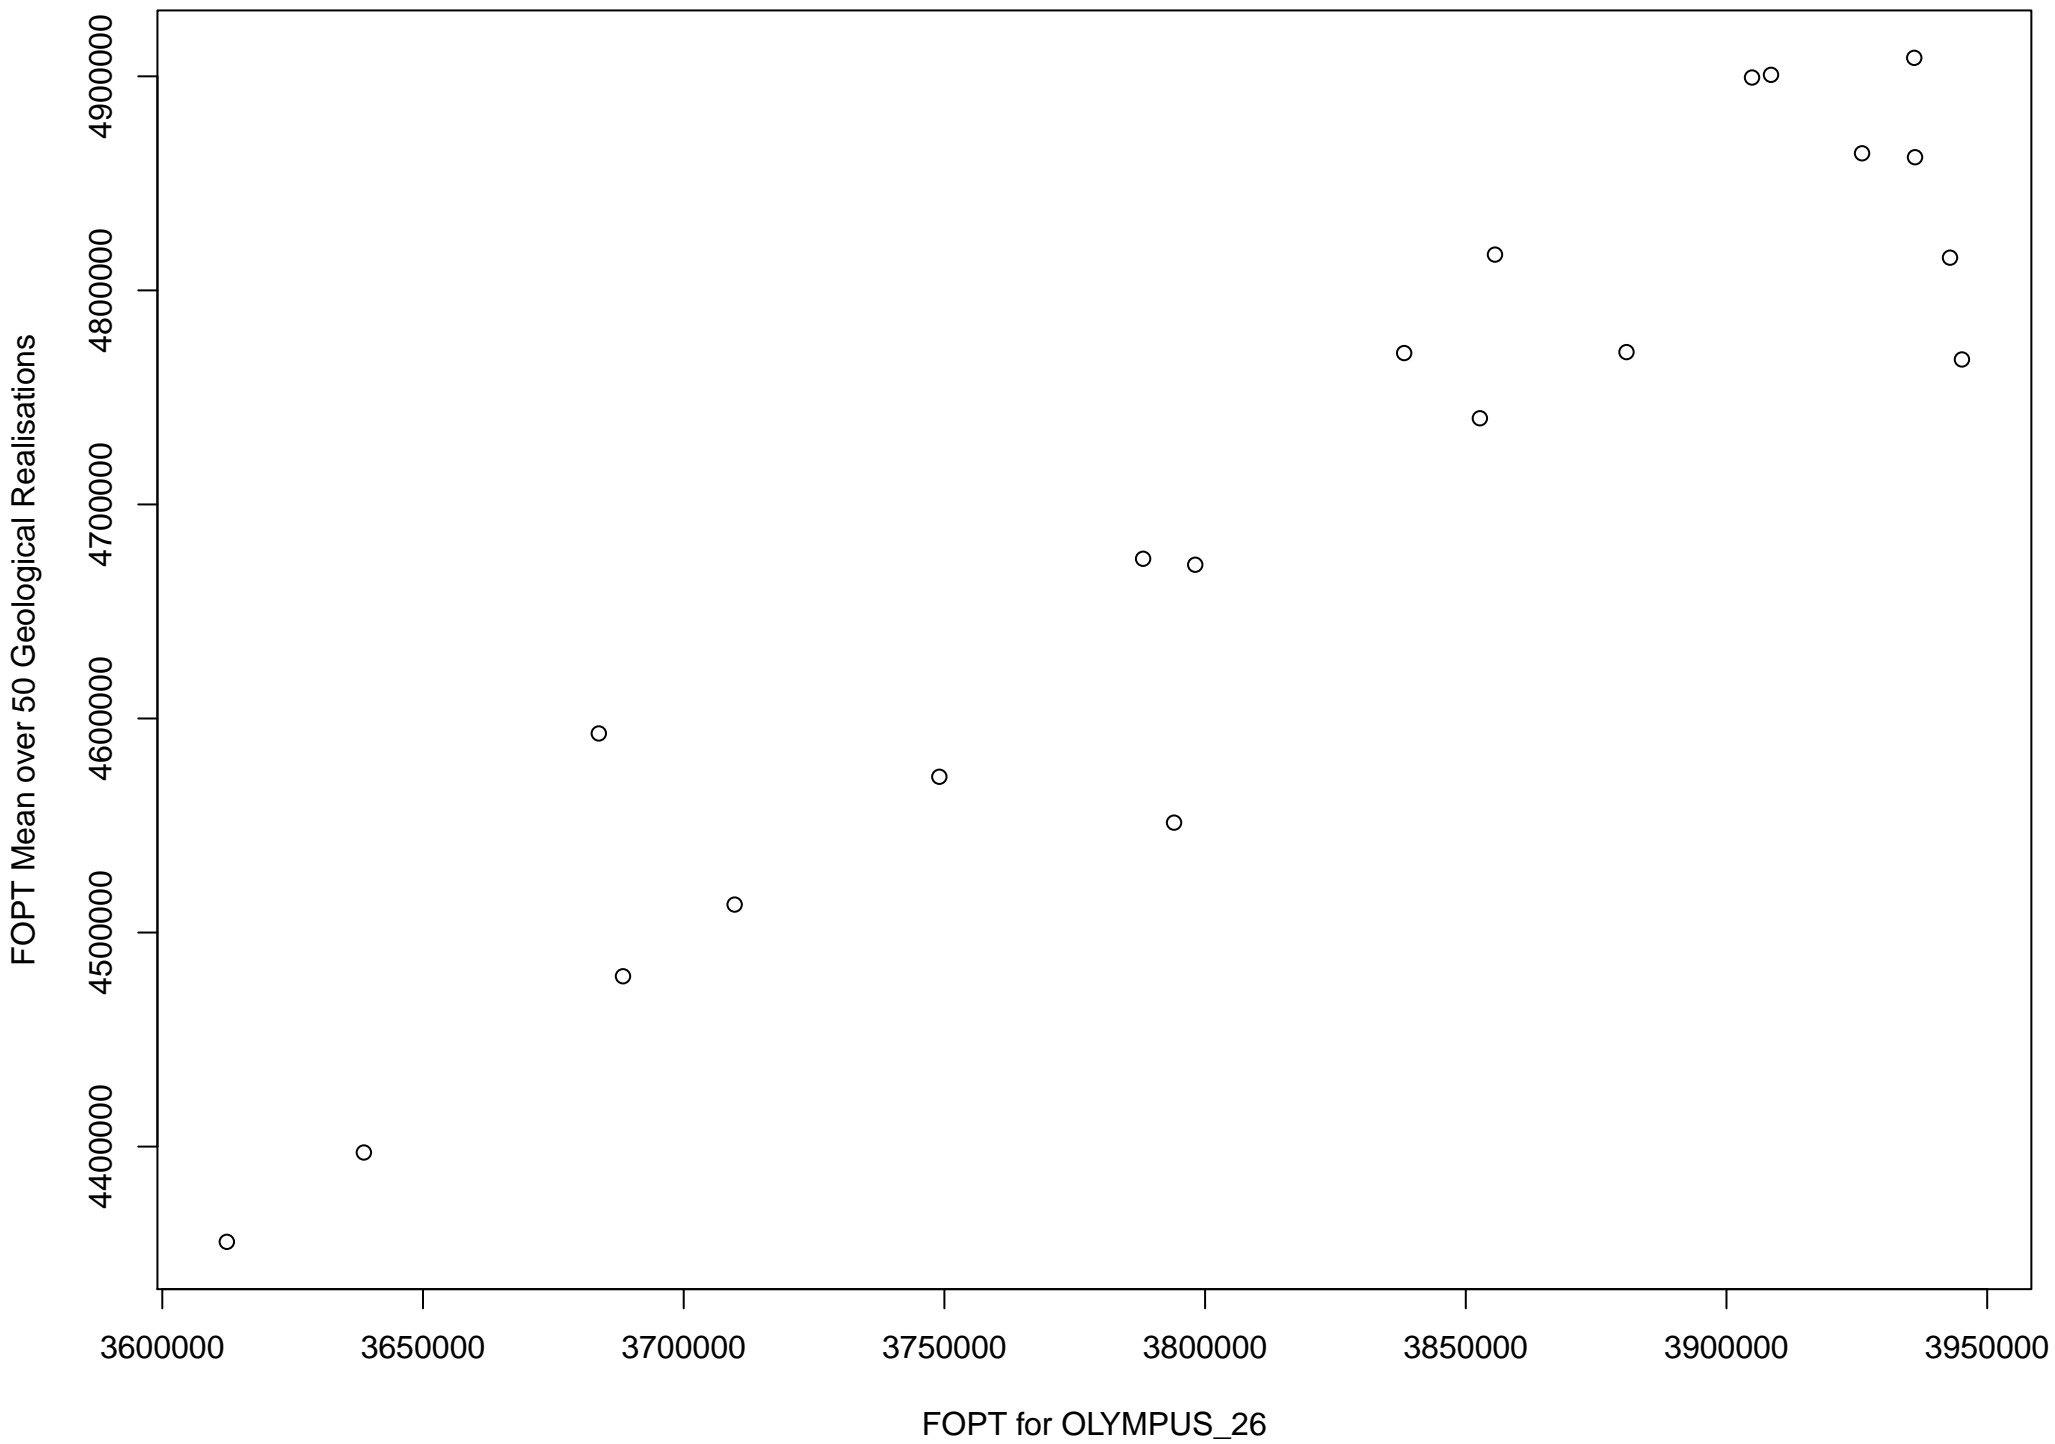

FOPT for OLYMPUS\_27

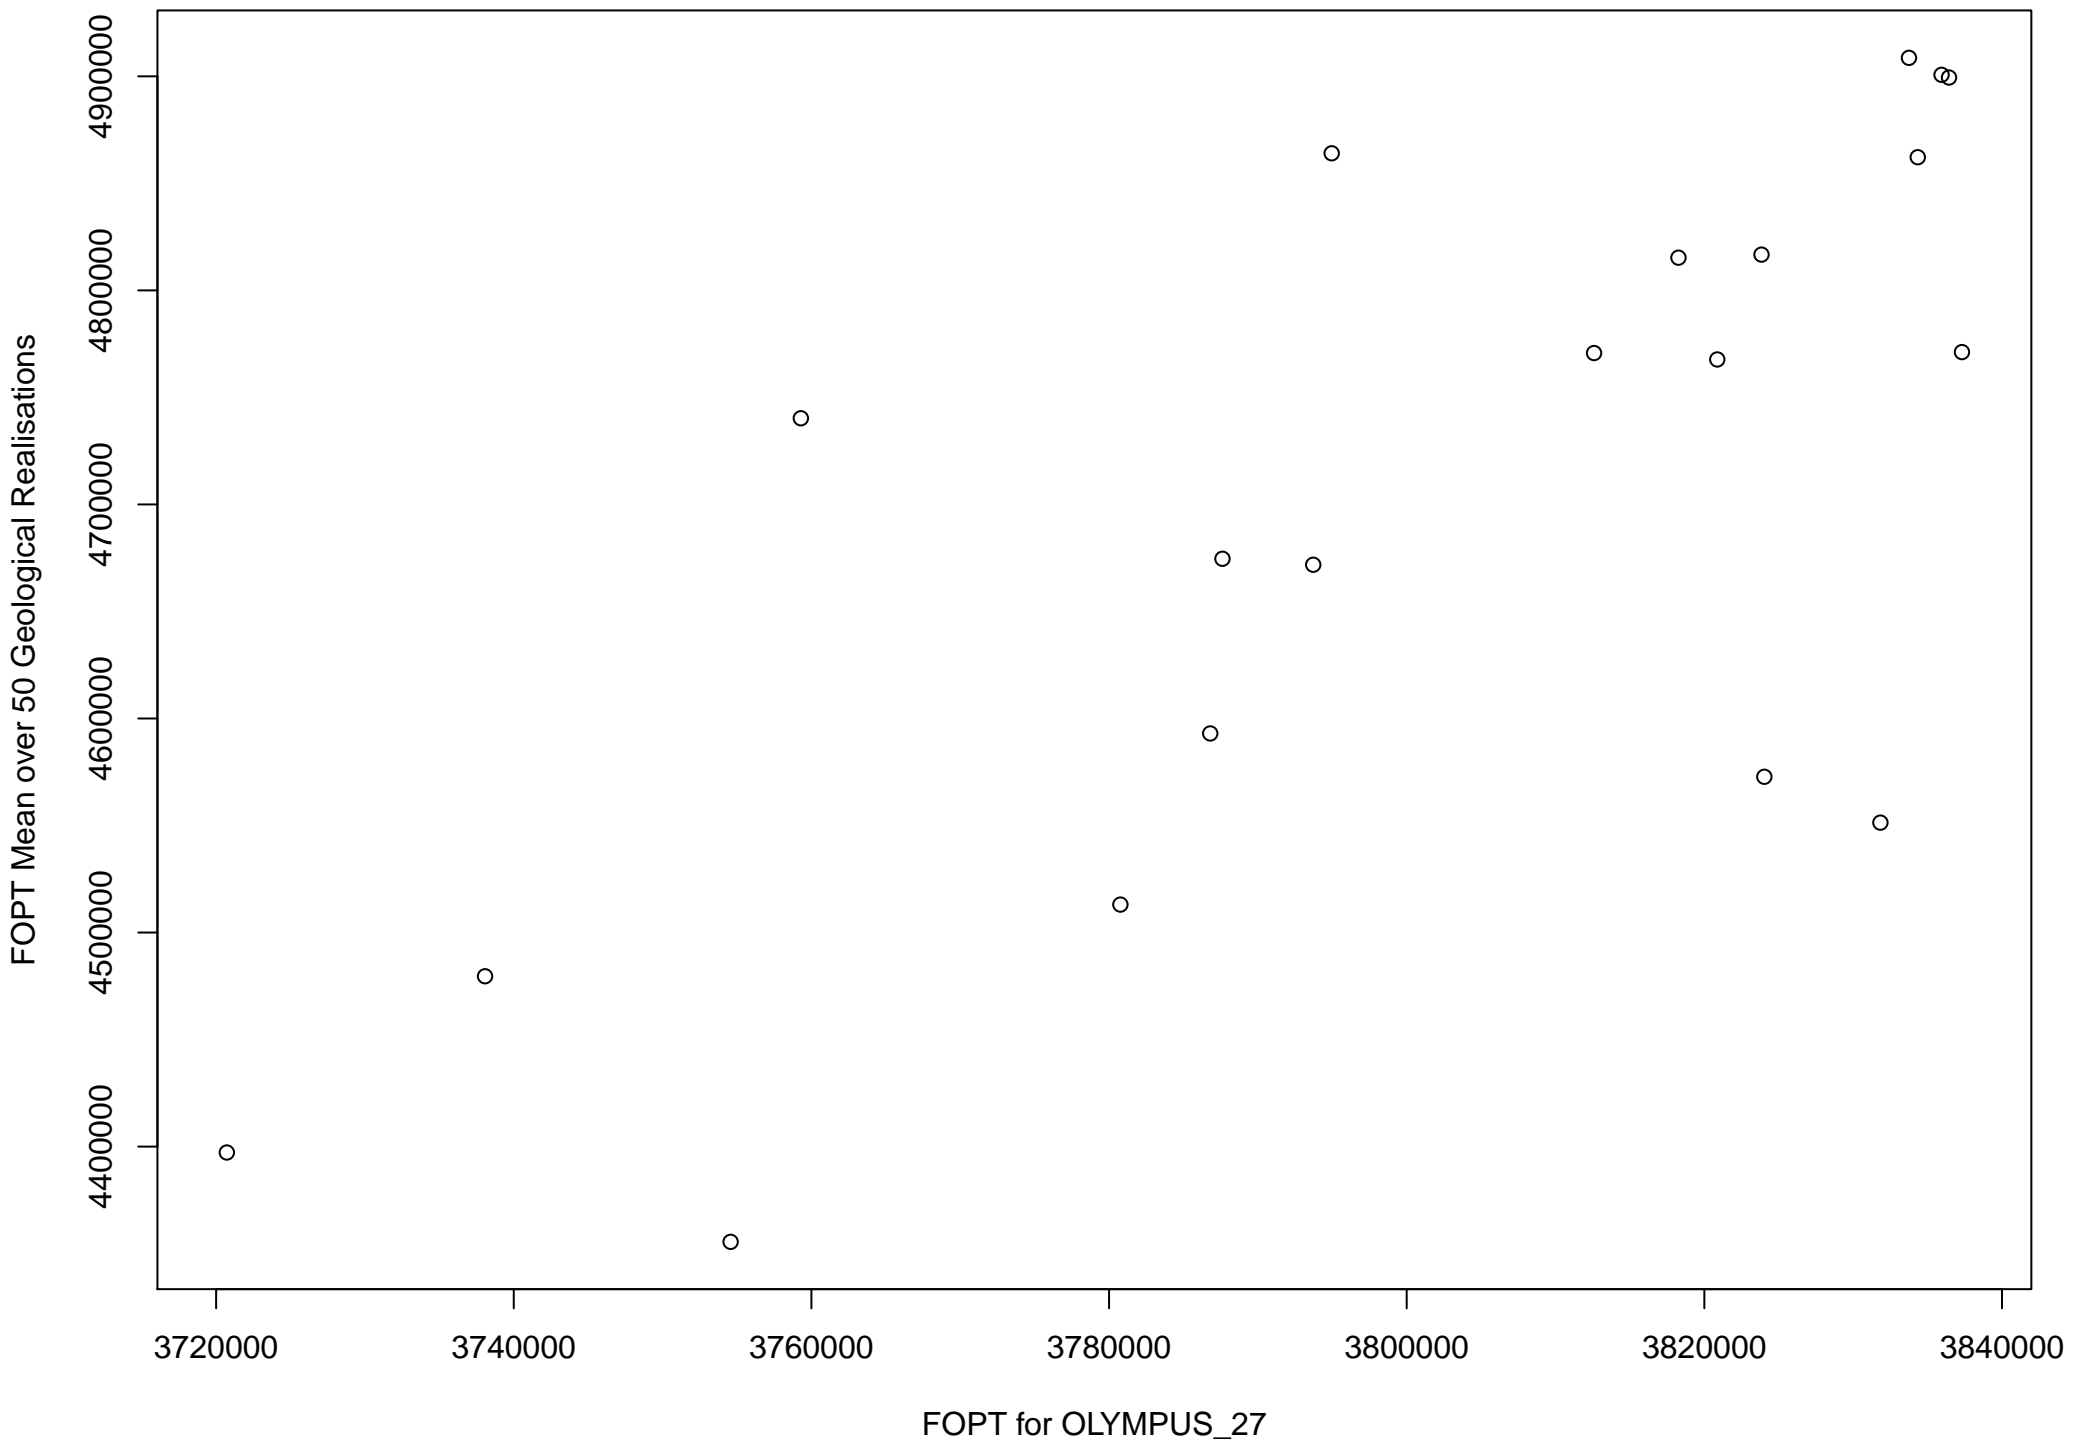

# FOPT for OLYMPUS\_28

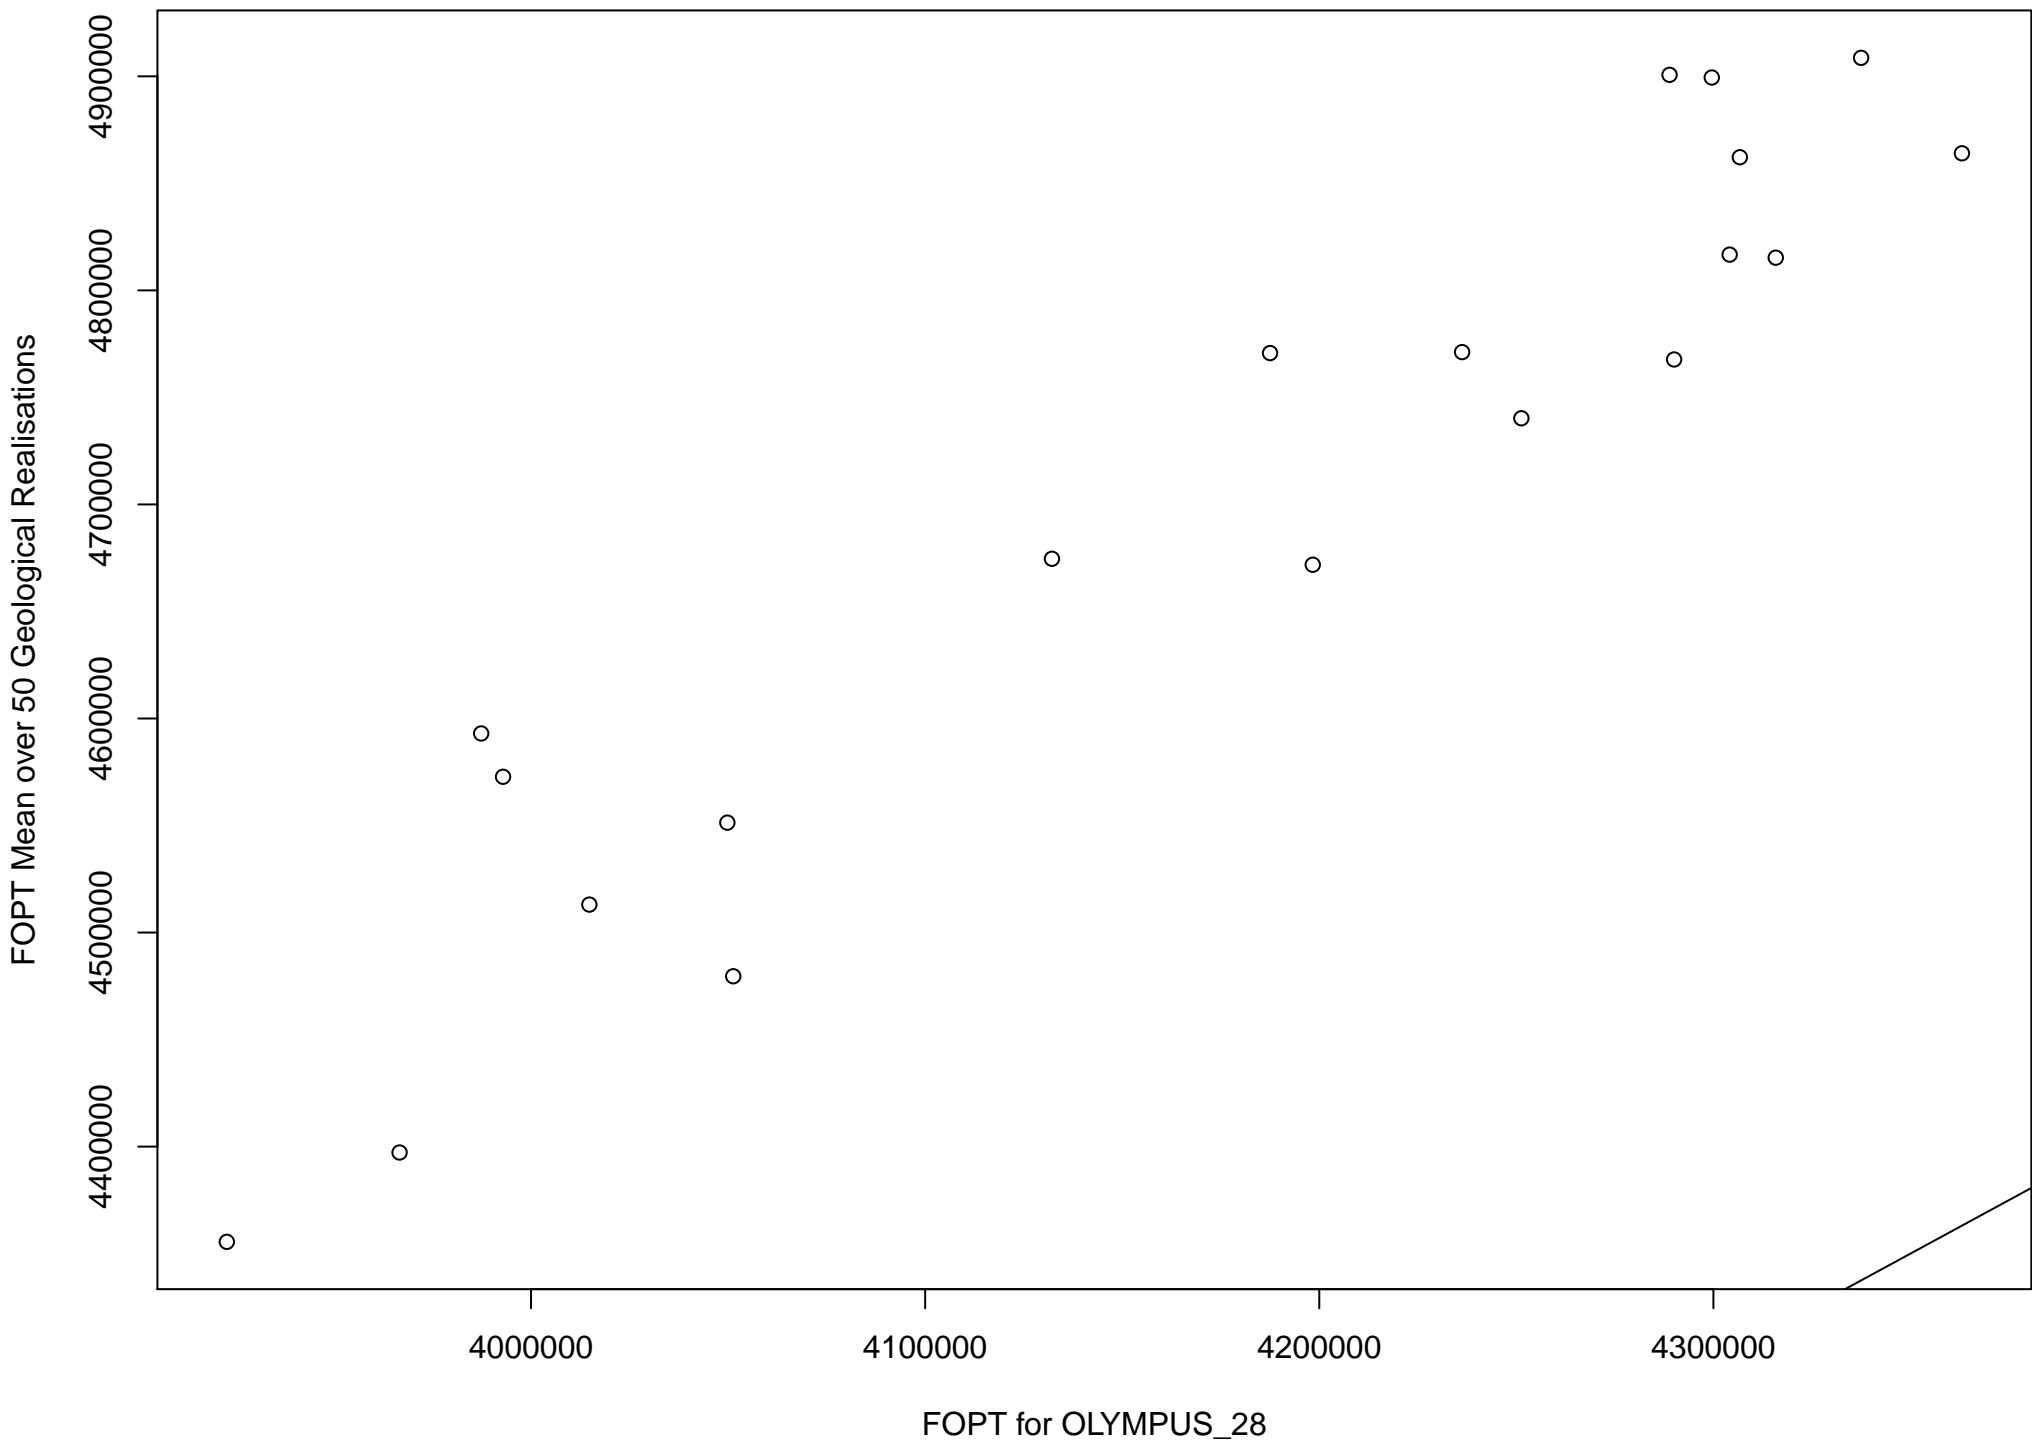

FOPT for OLYMPUS\_29

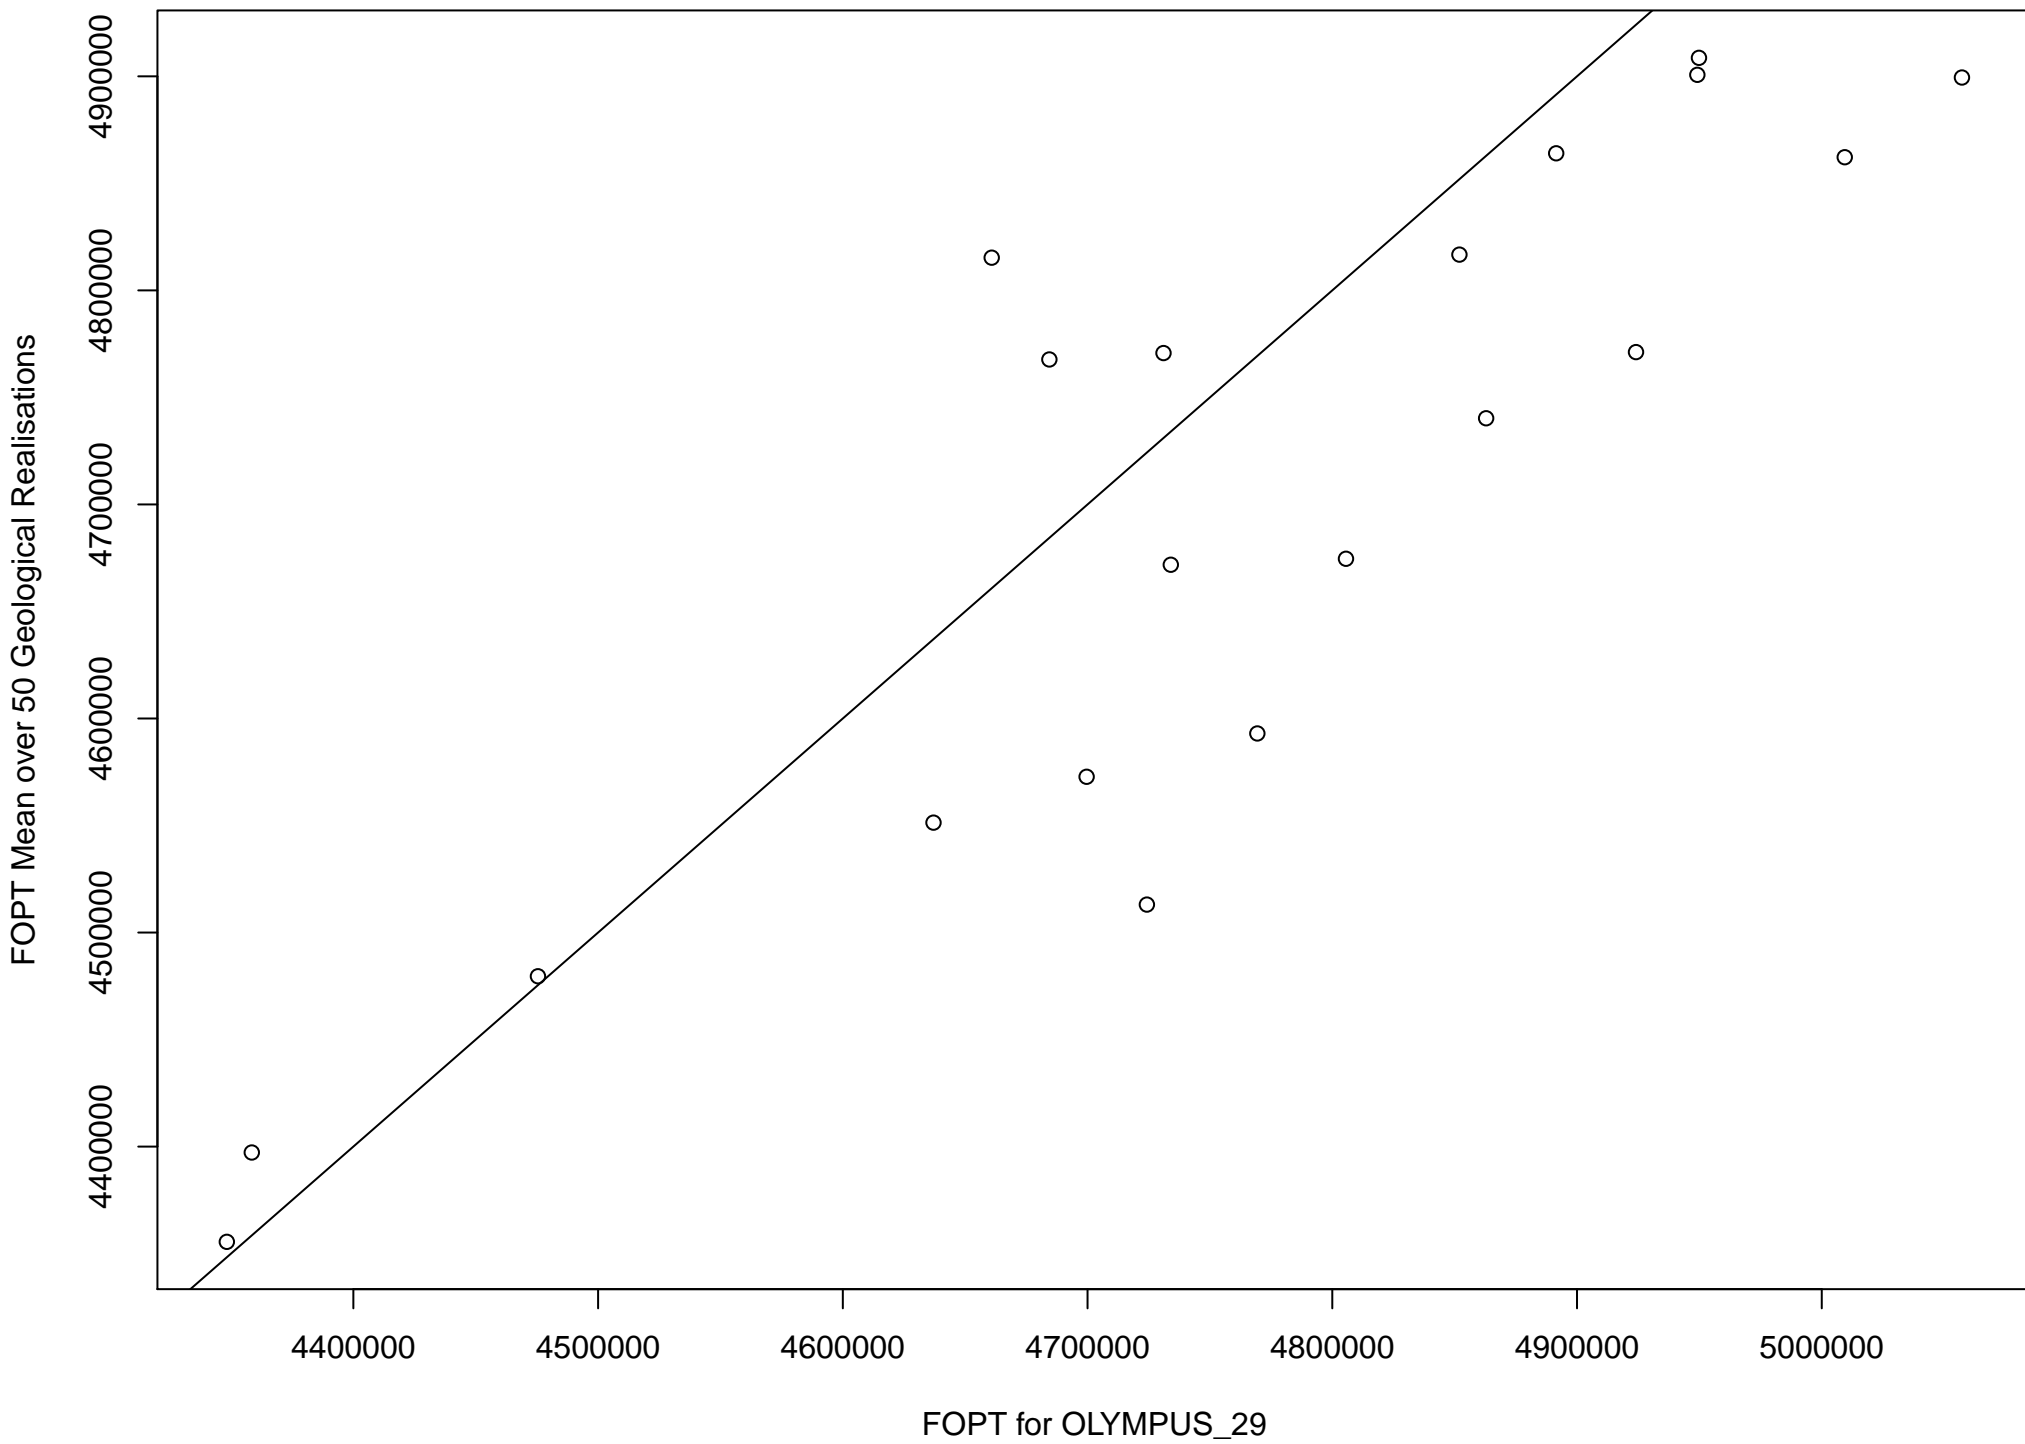

FOPT for OLYMPUS\_30

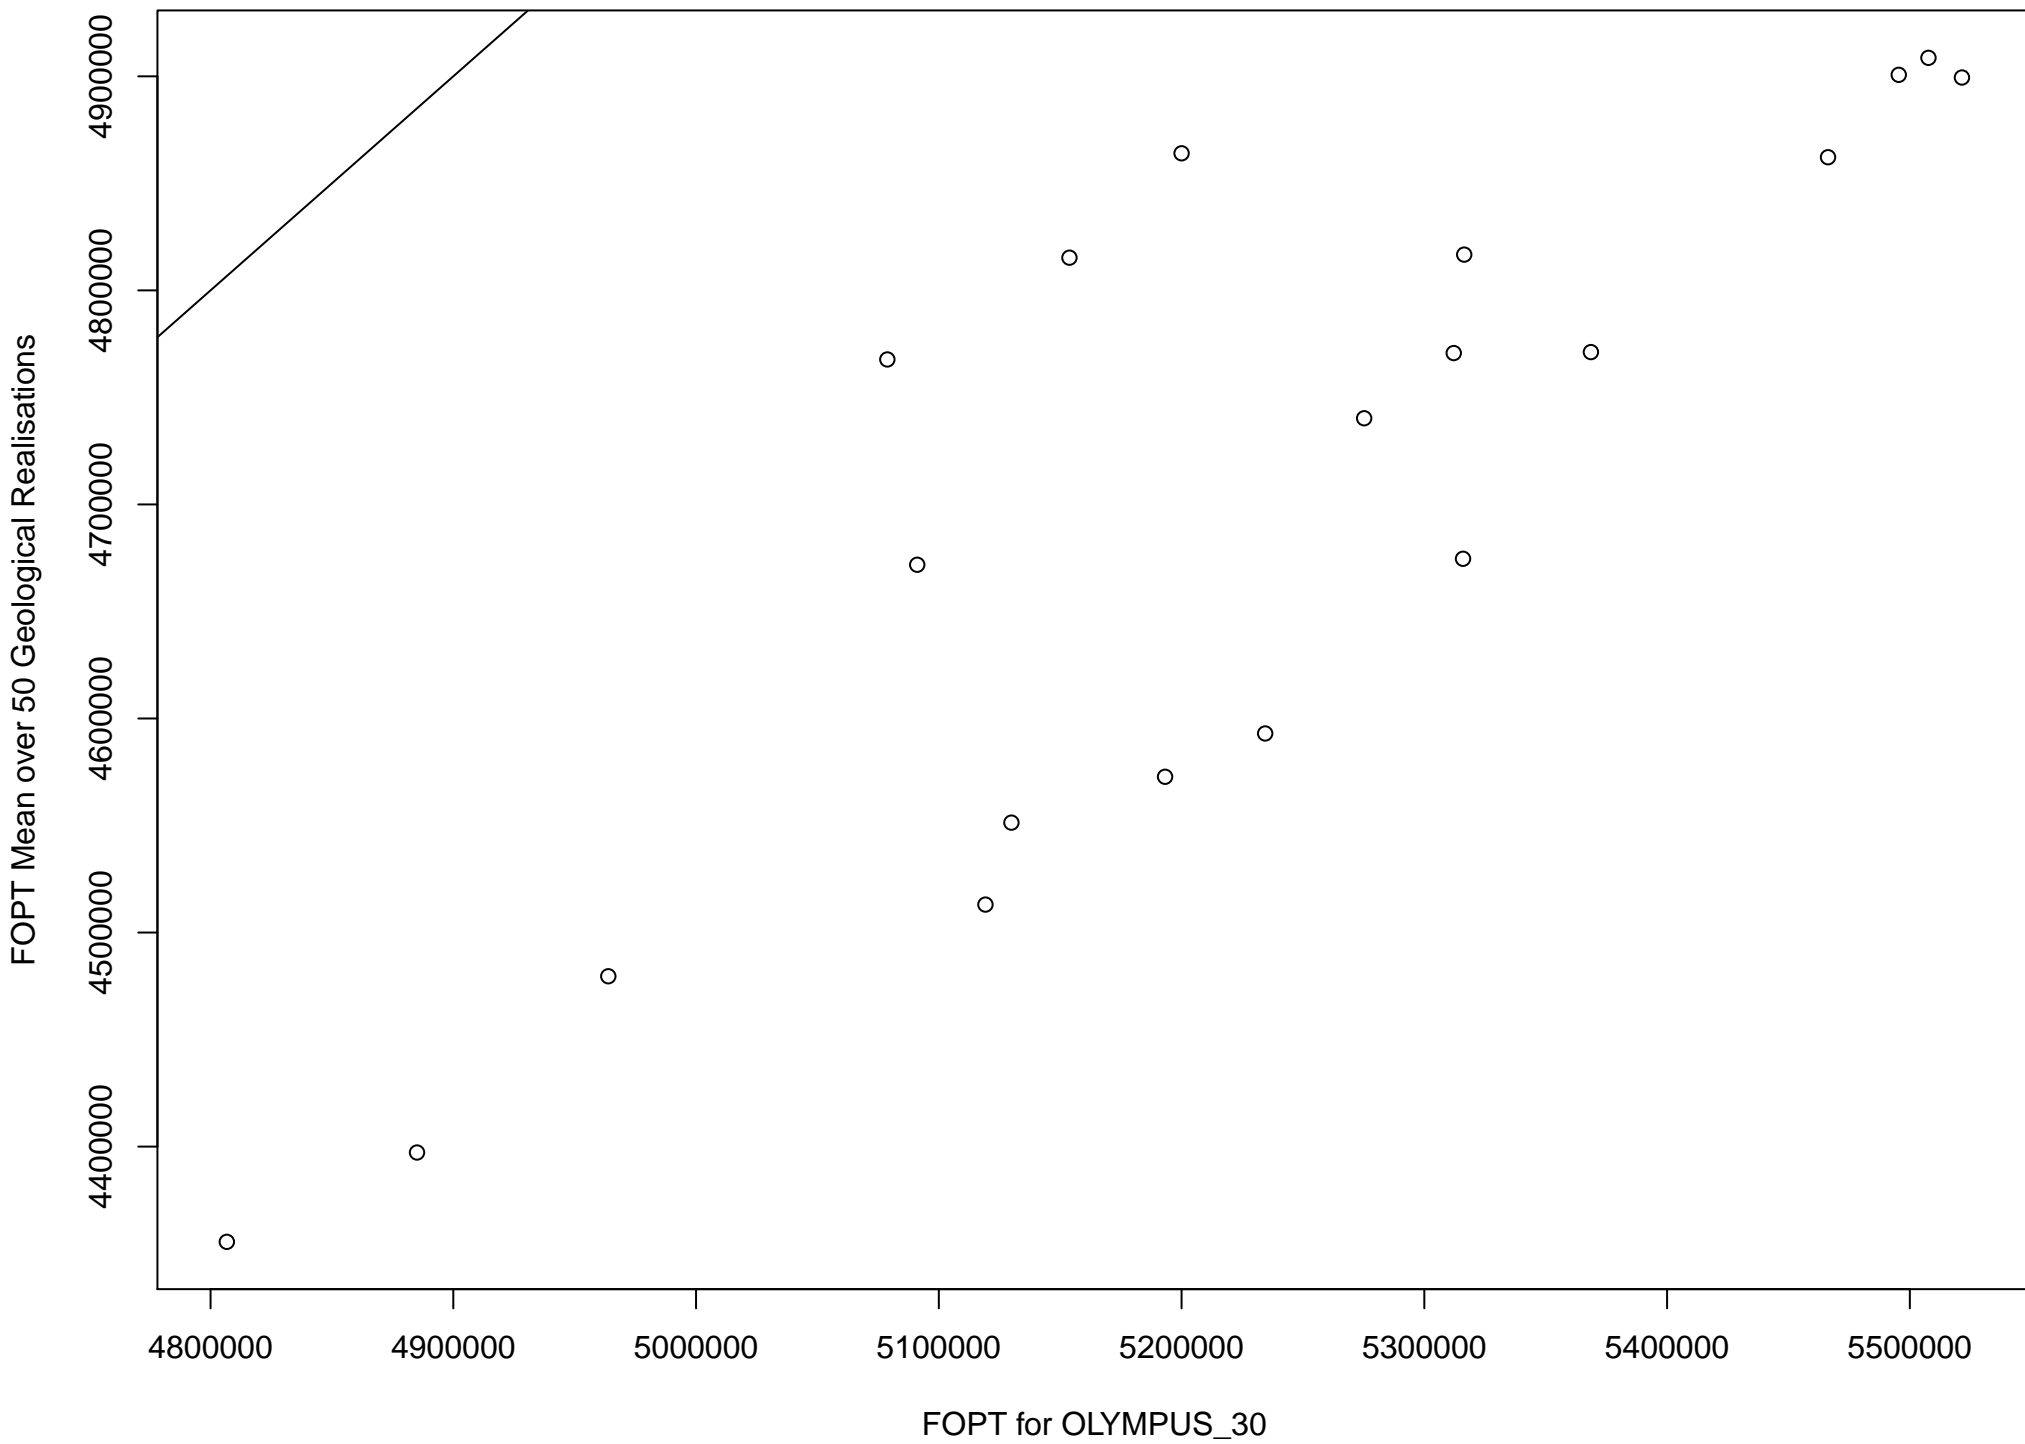

FOPT for OLYMPUS\_31

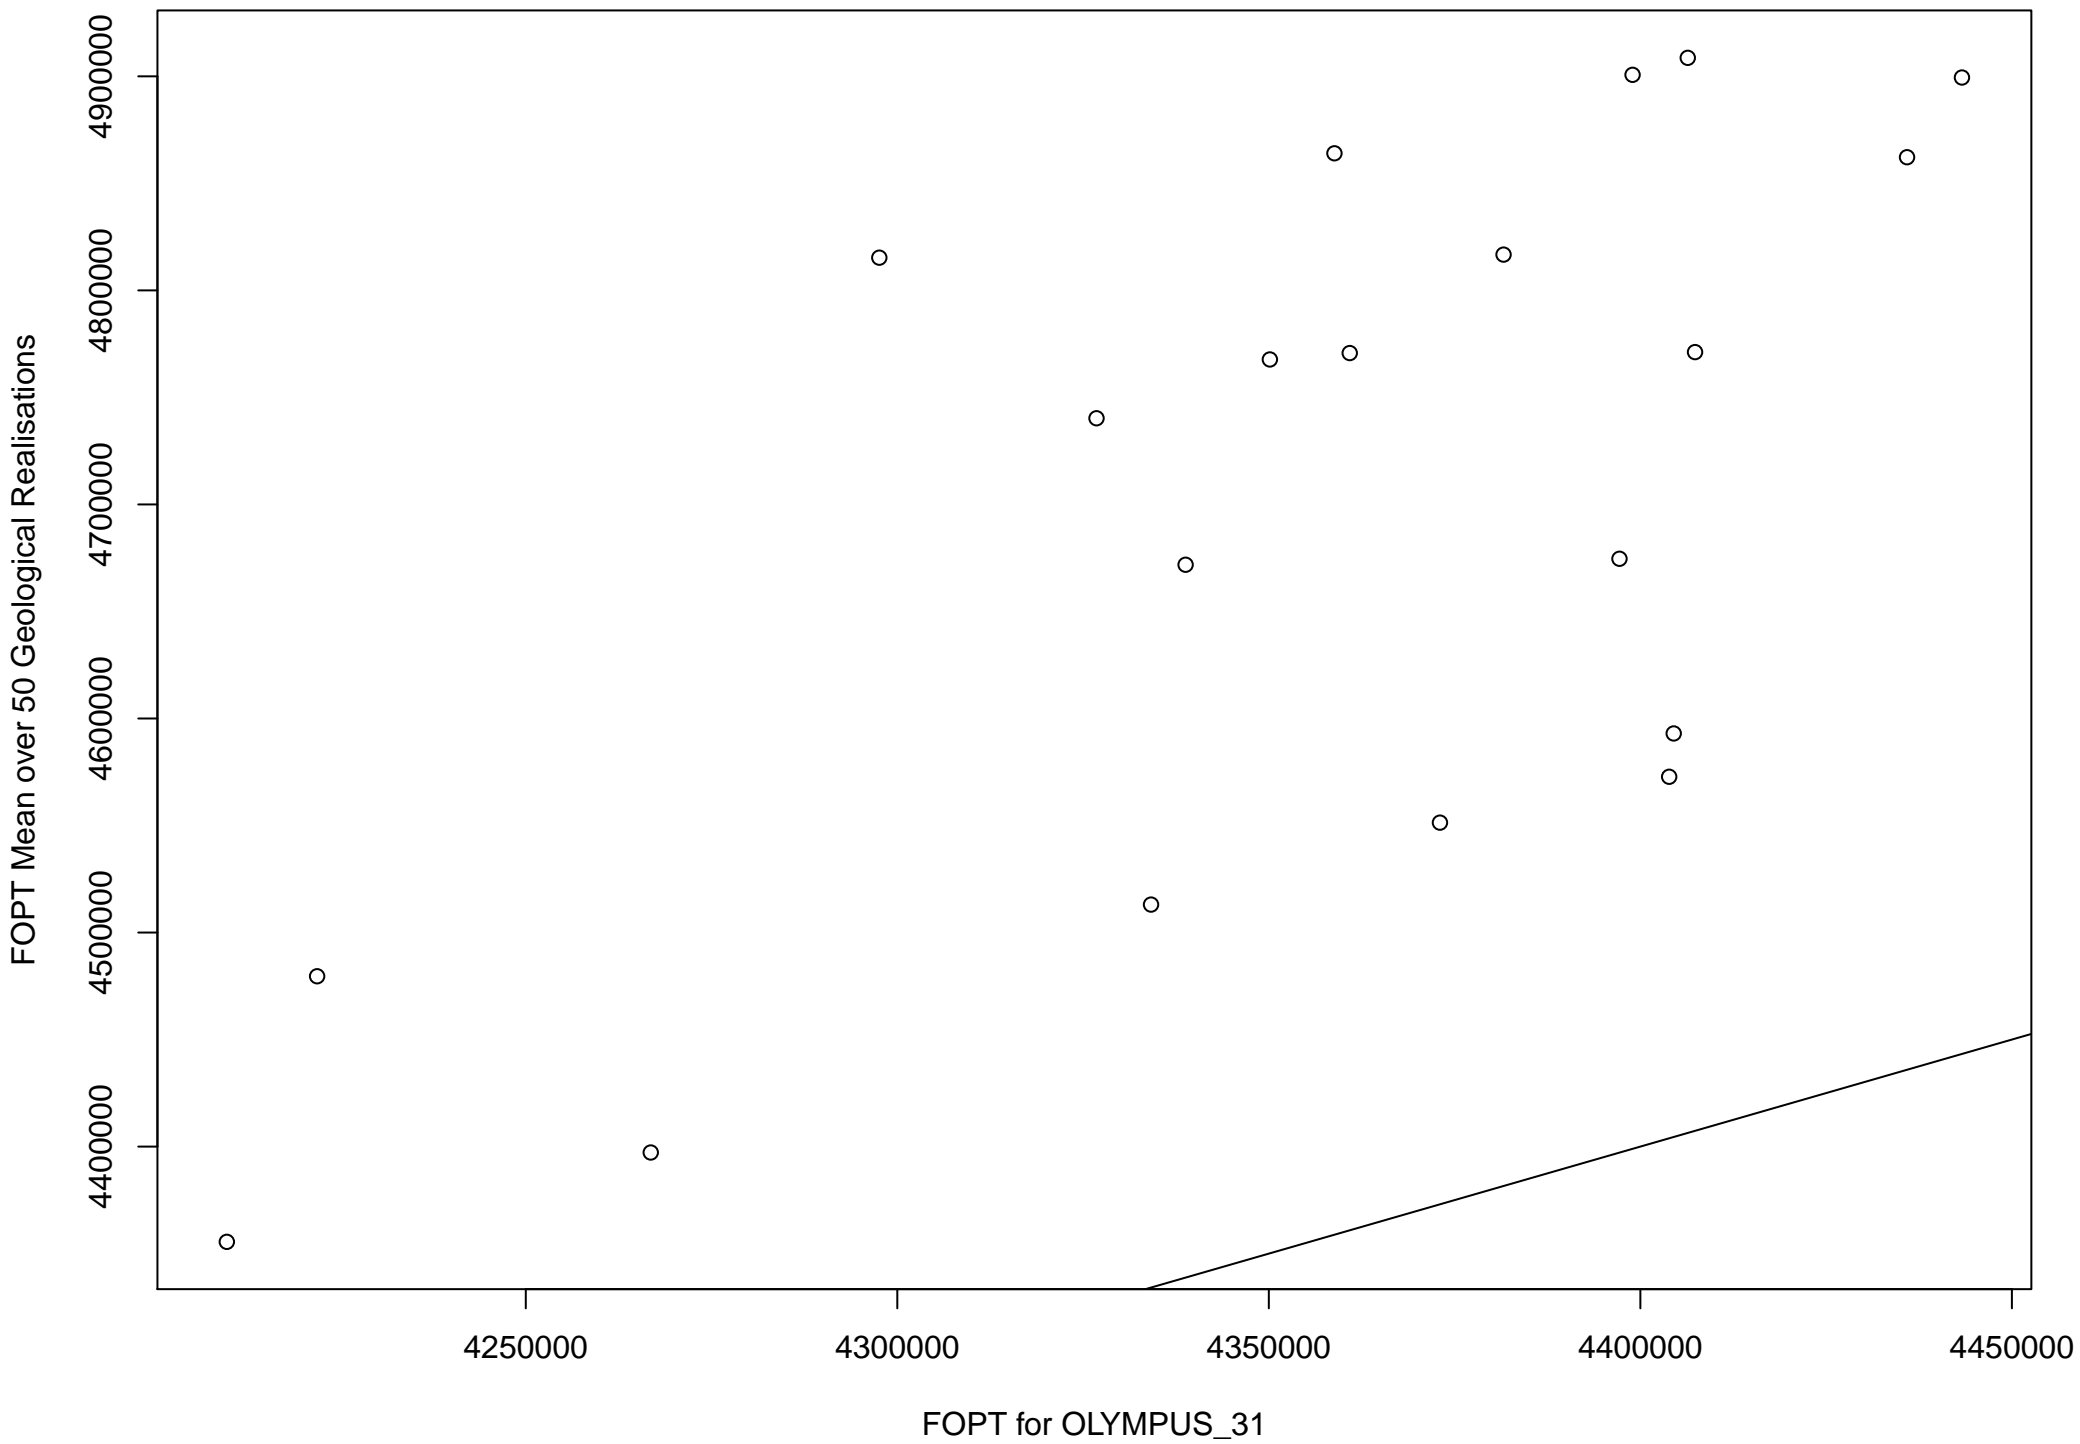

FOPT for OLYMPUS\_32

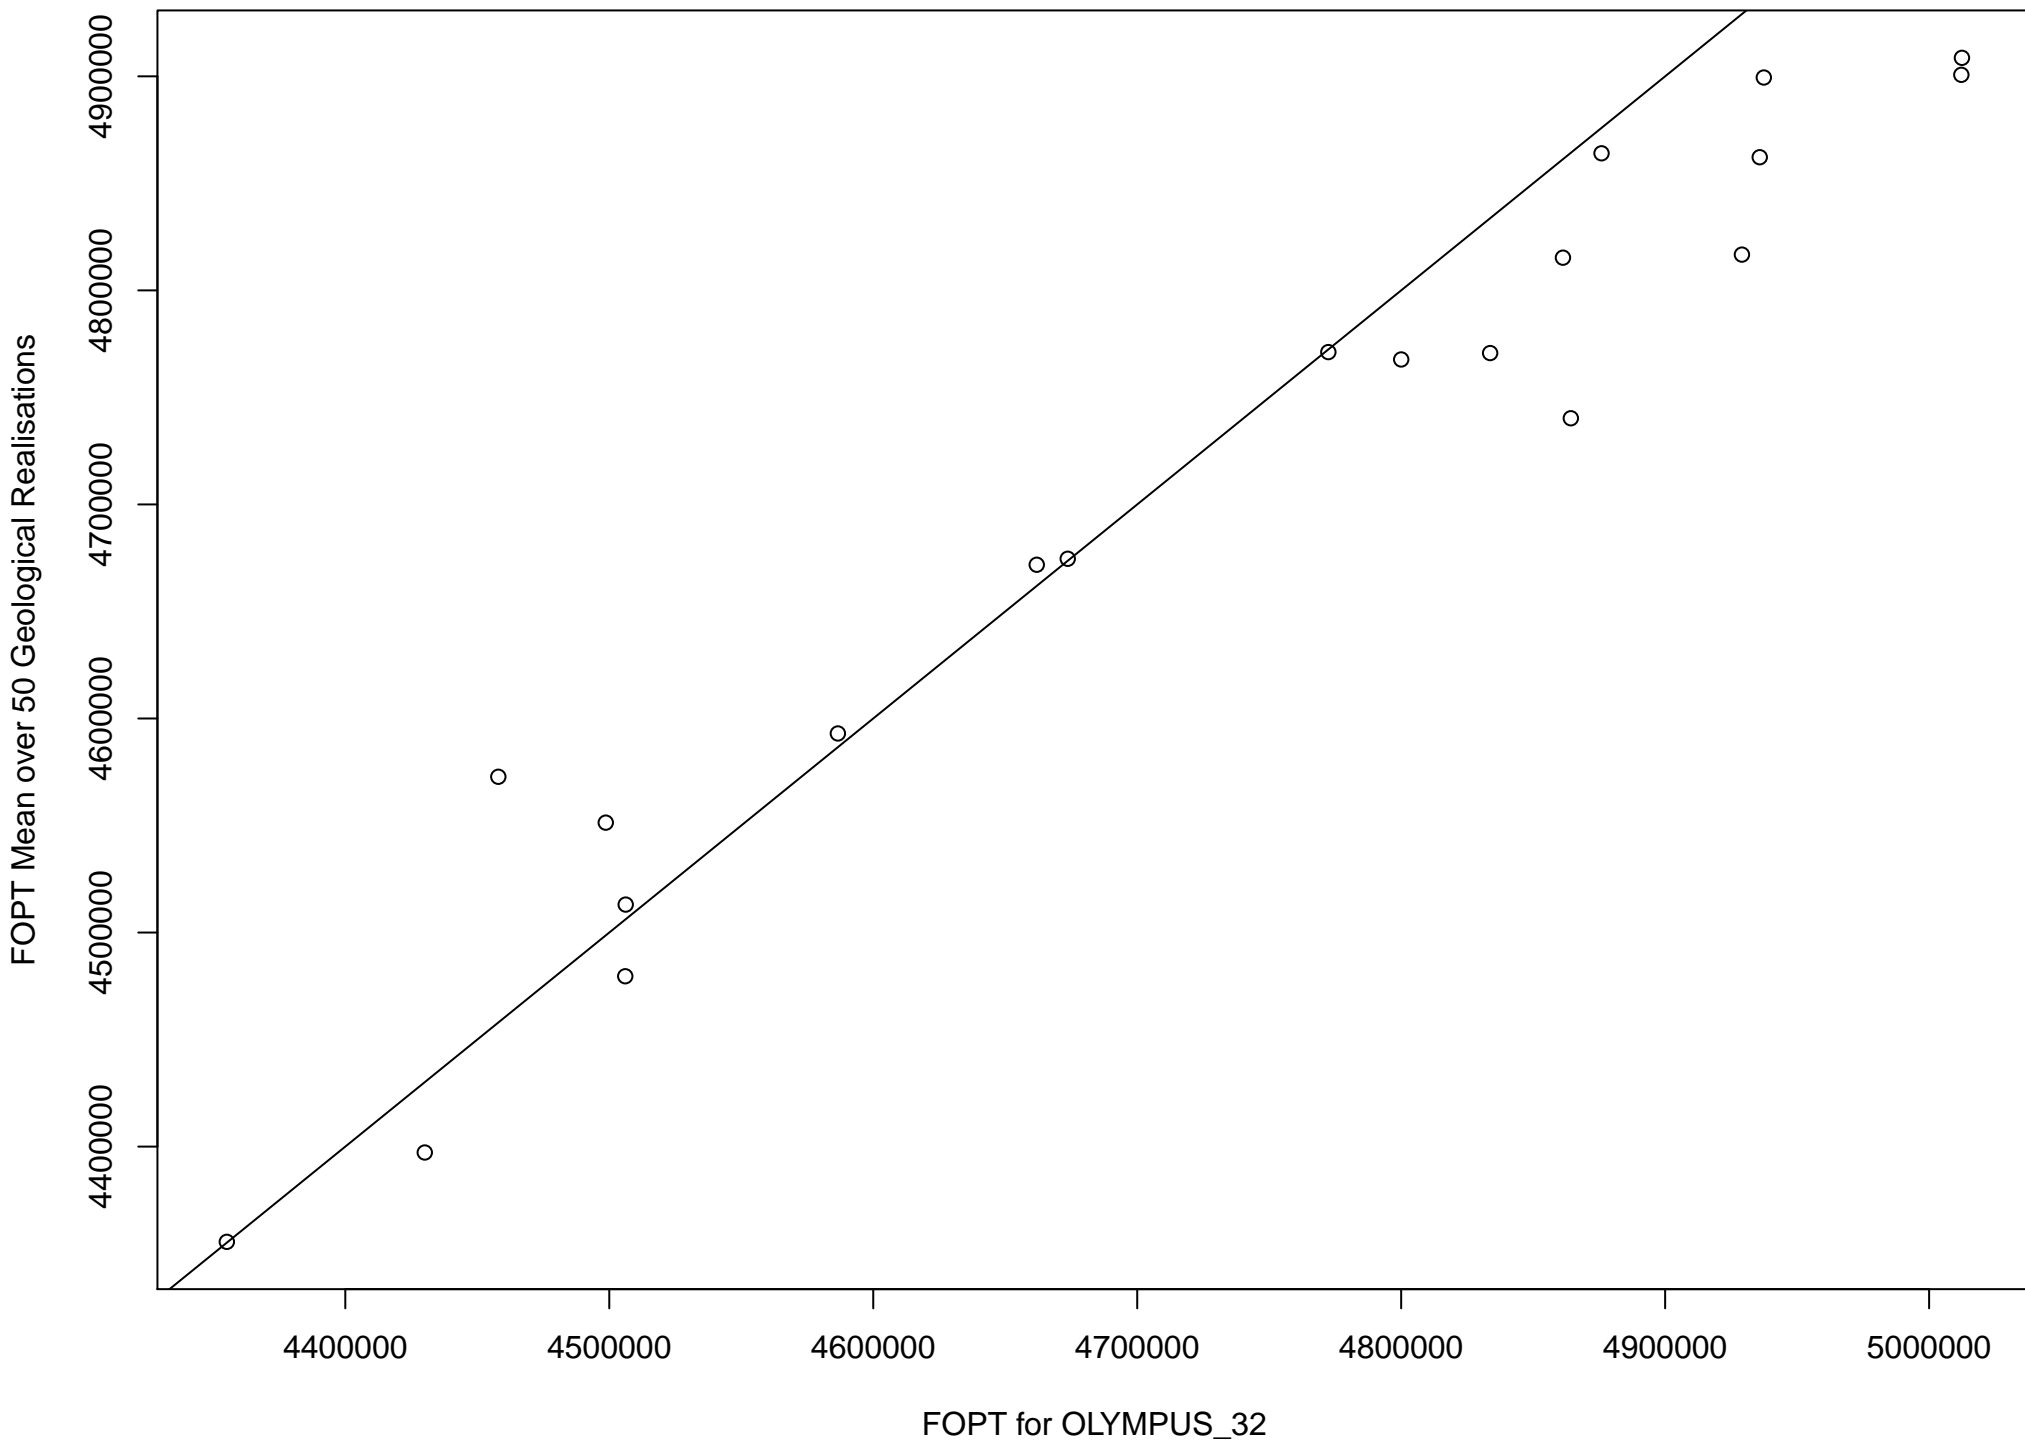



# FOPT for OLYMPUS\_33

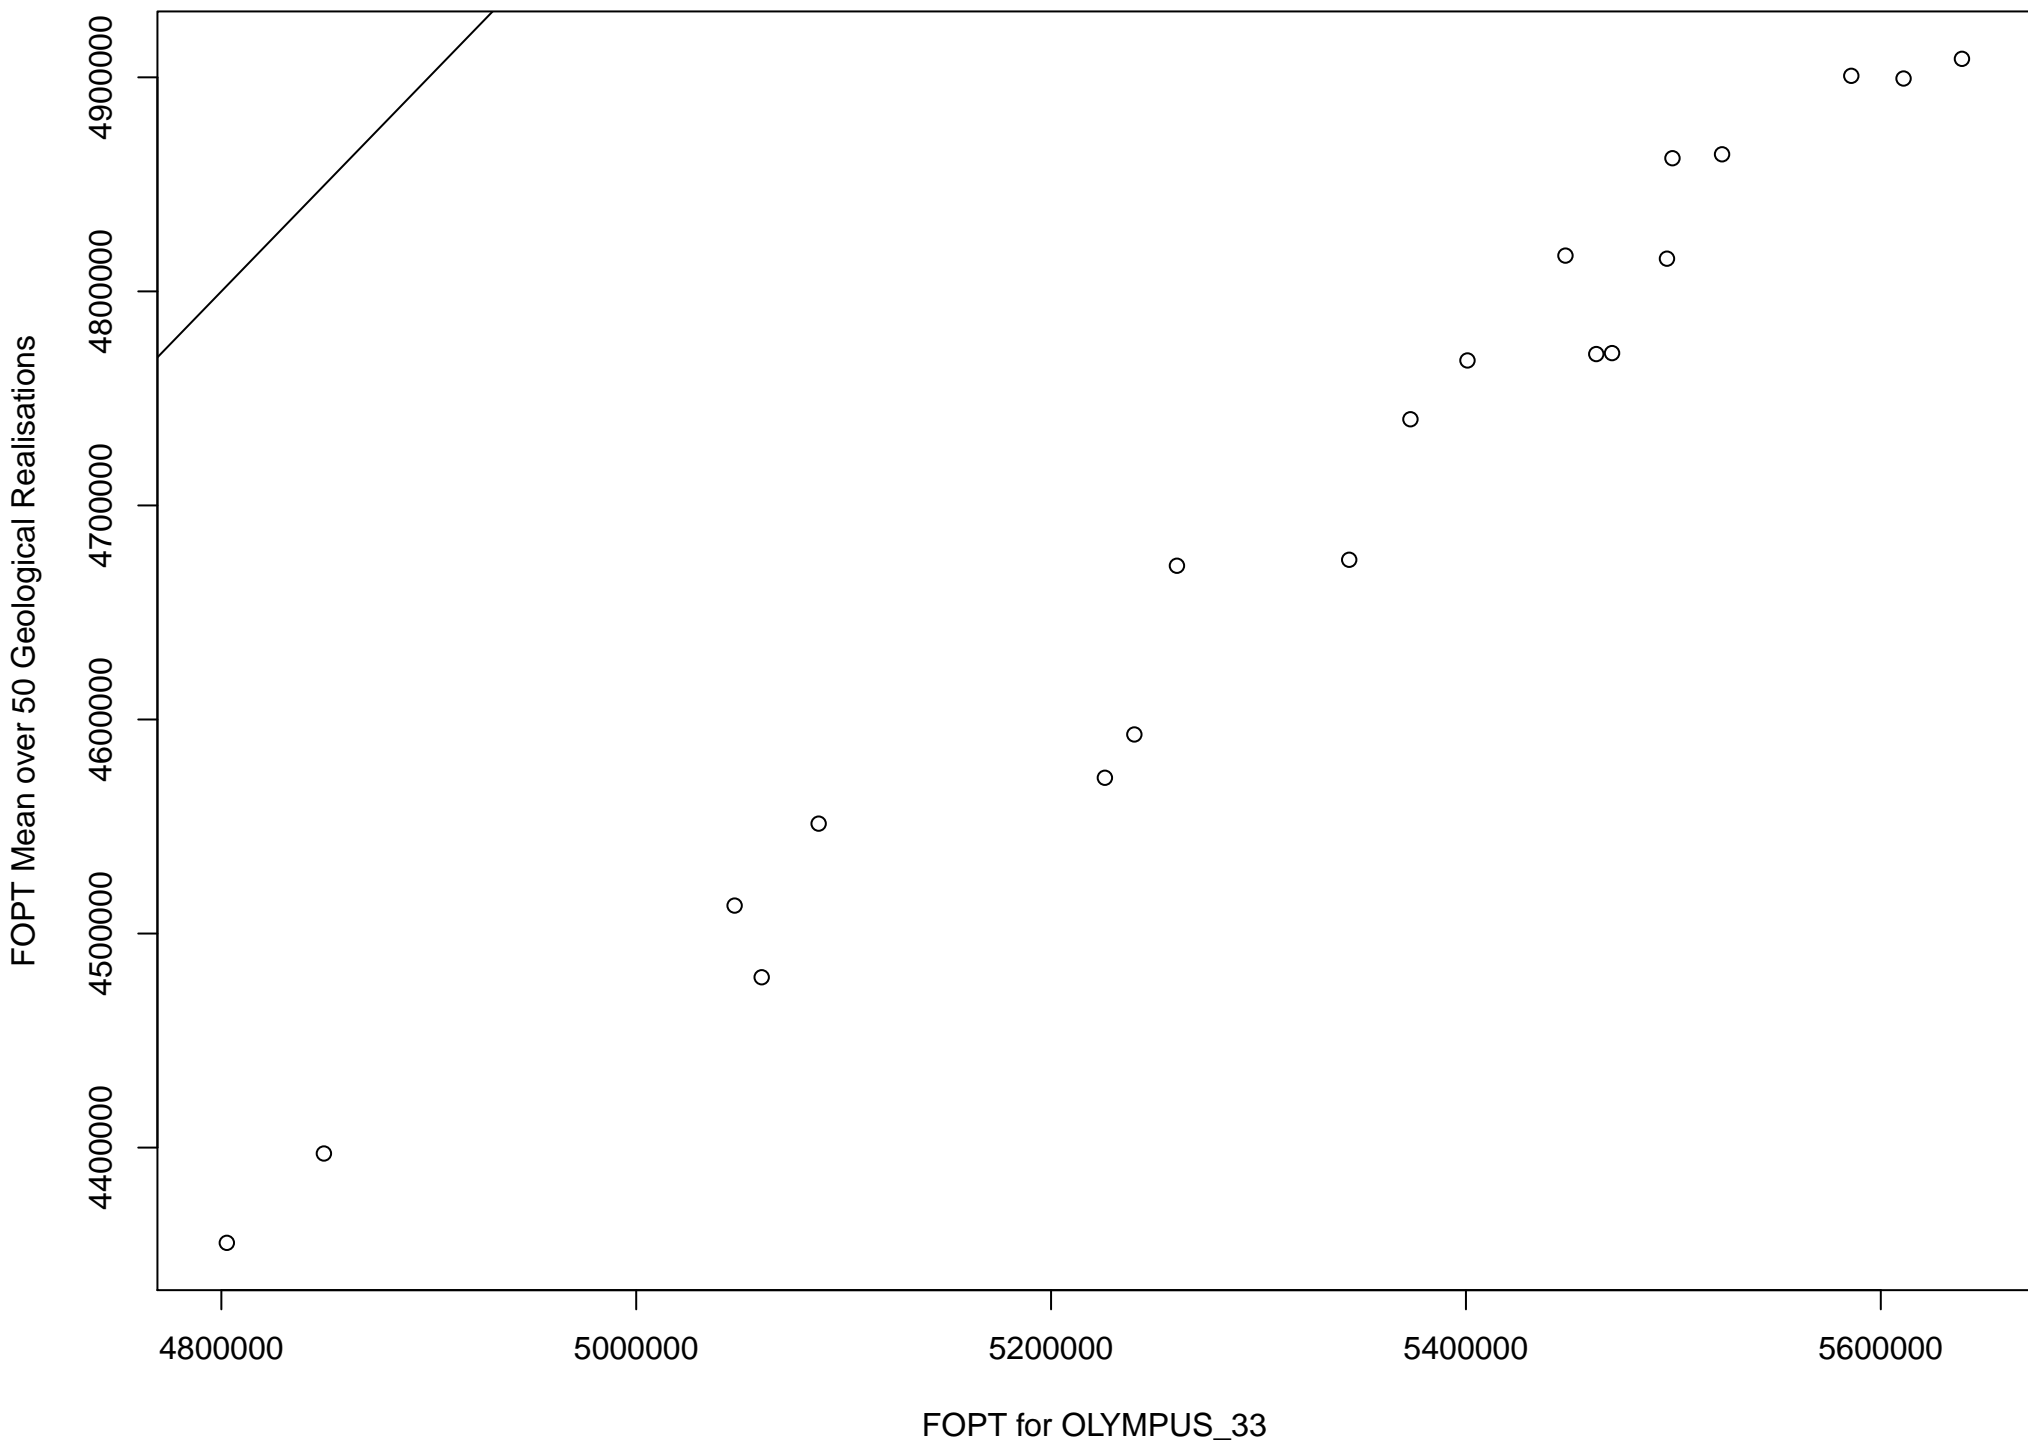

FOPT for OLYMPUS\_34

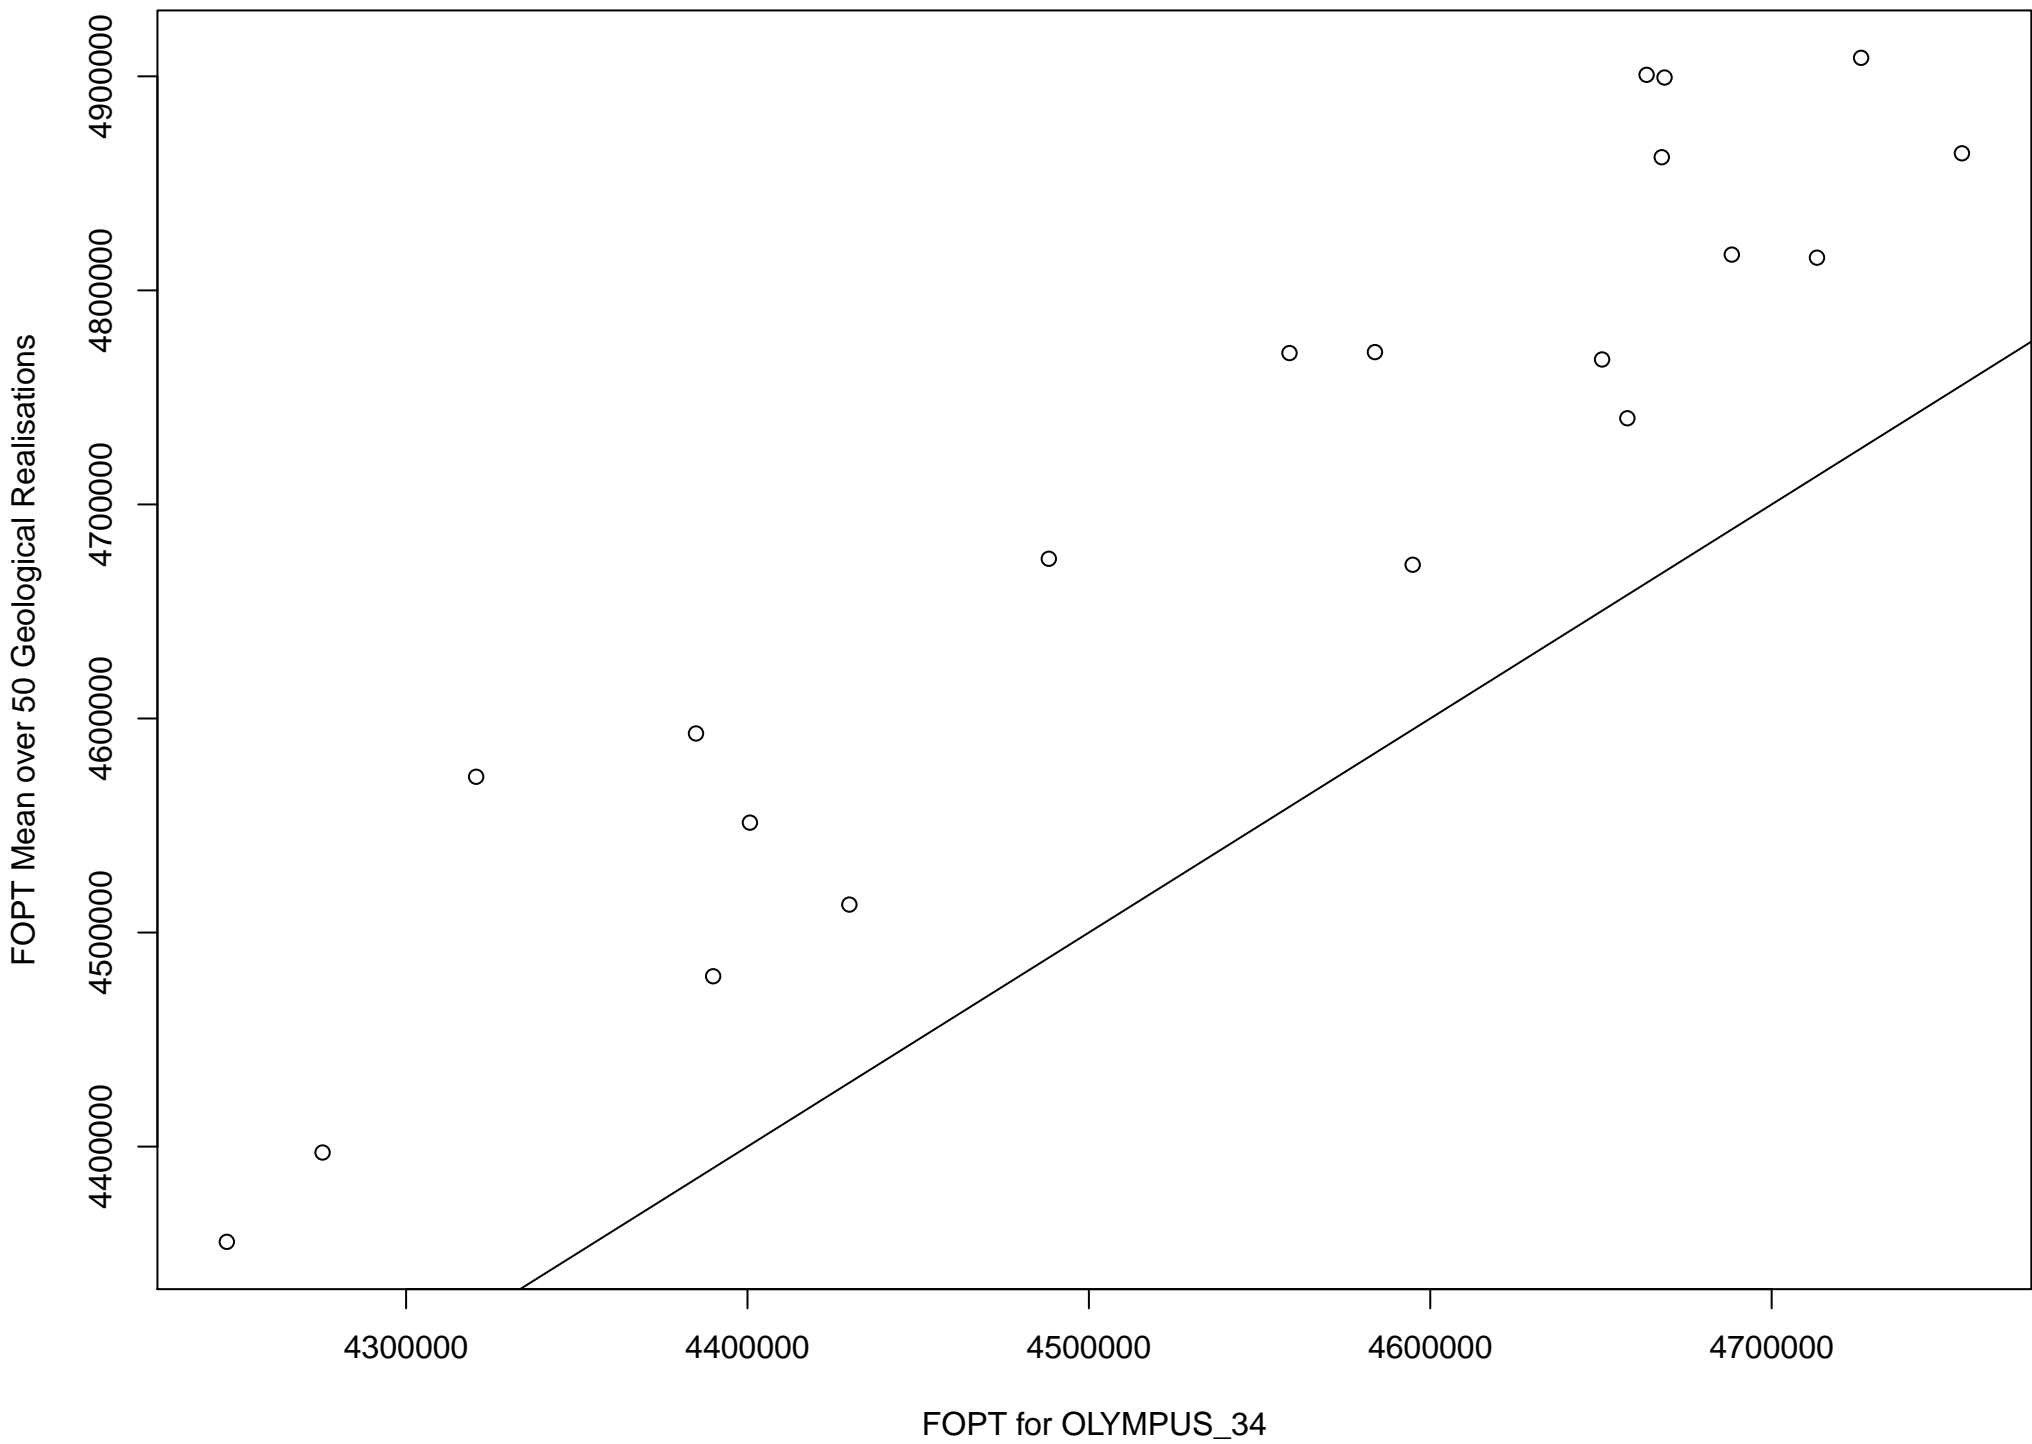

FOPT for OLYMPUS\_35

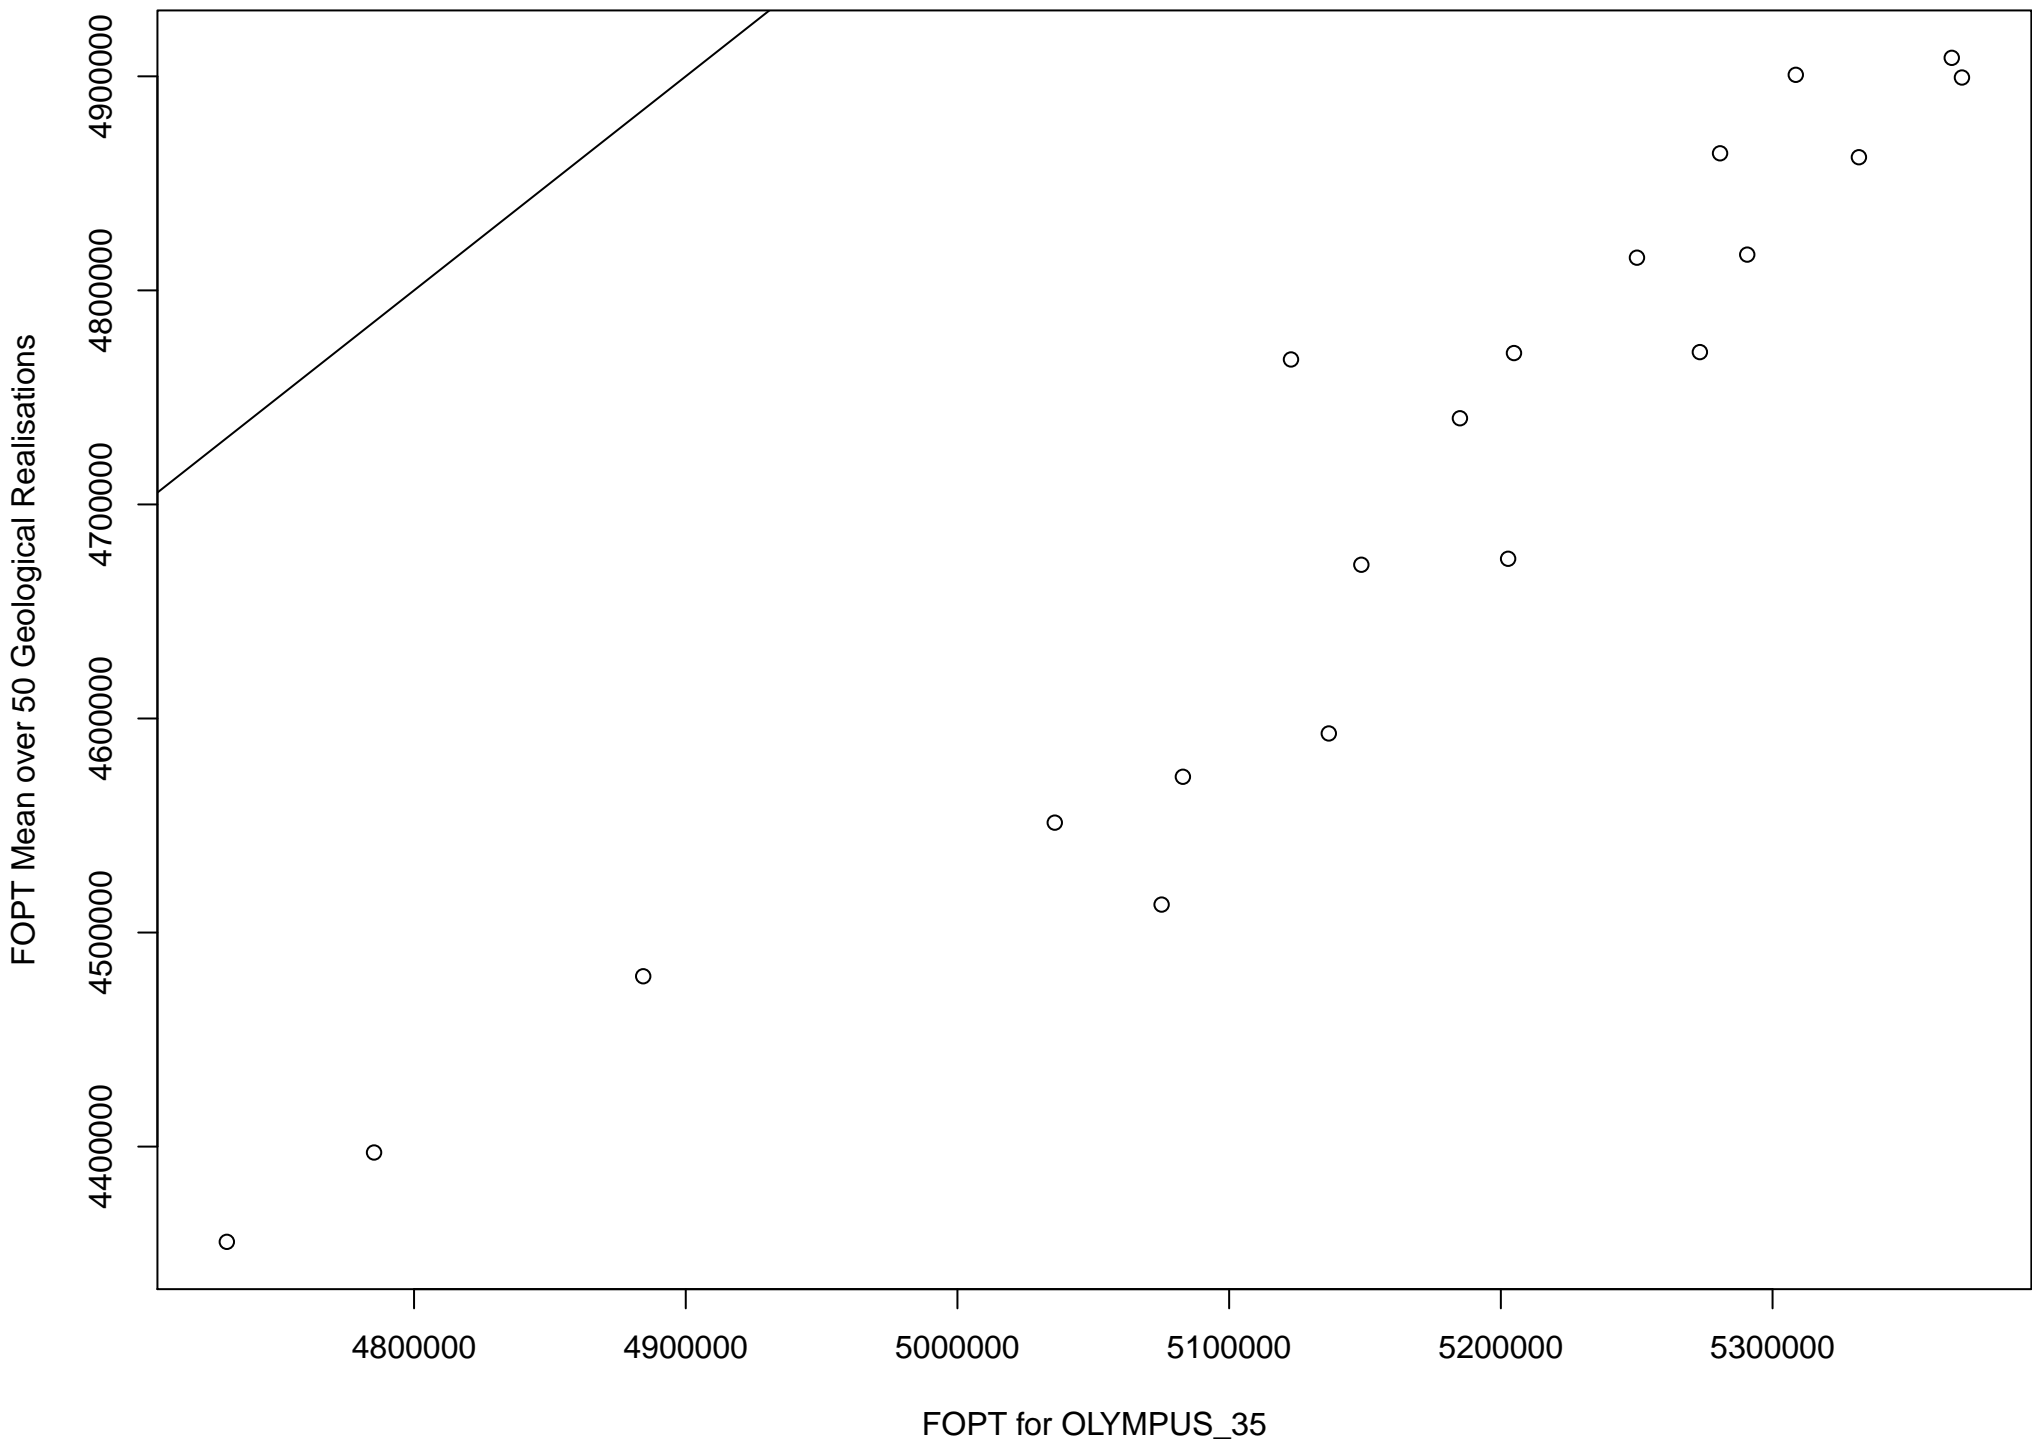

FOPT for OLYMPUS\_36

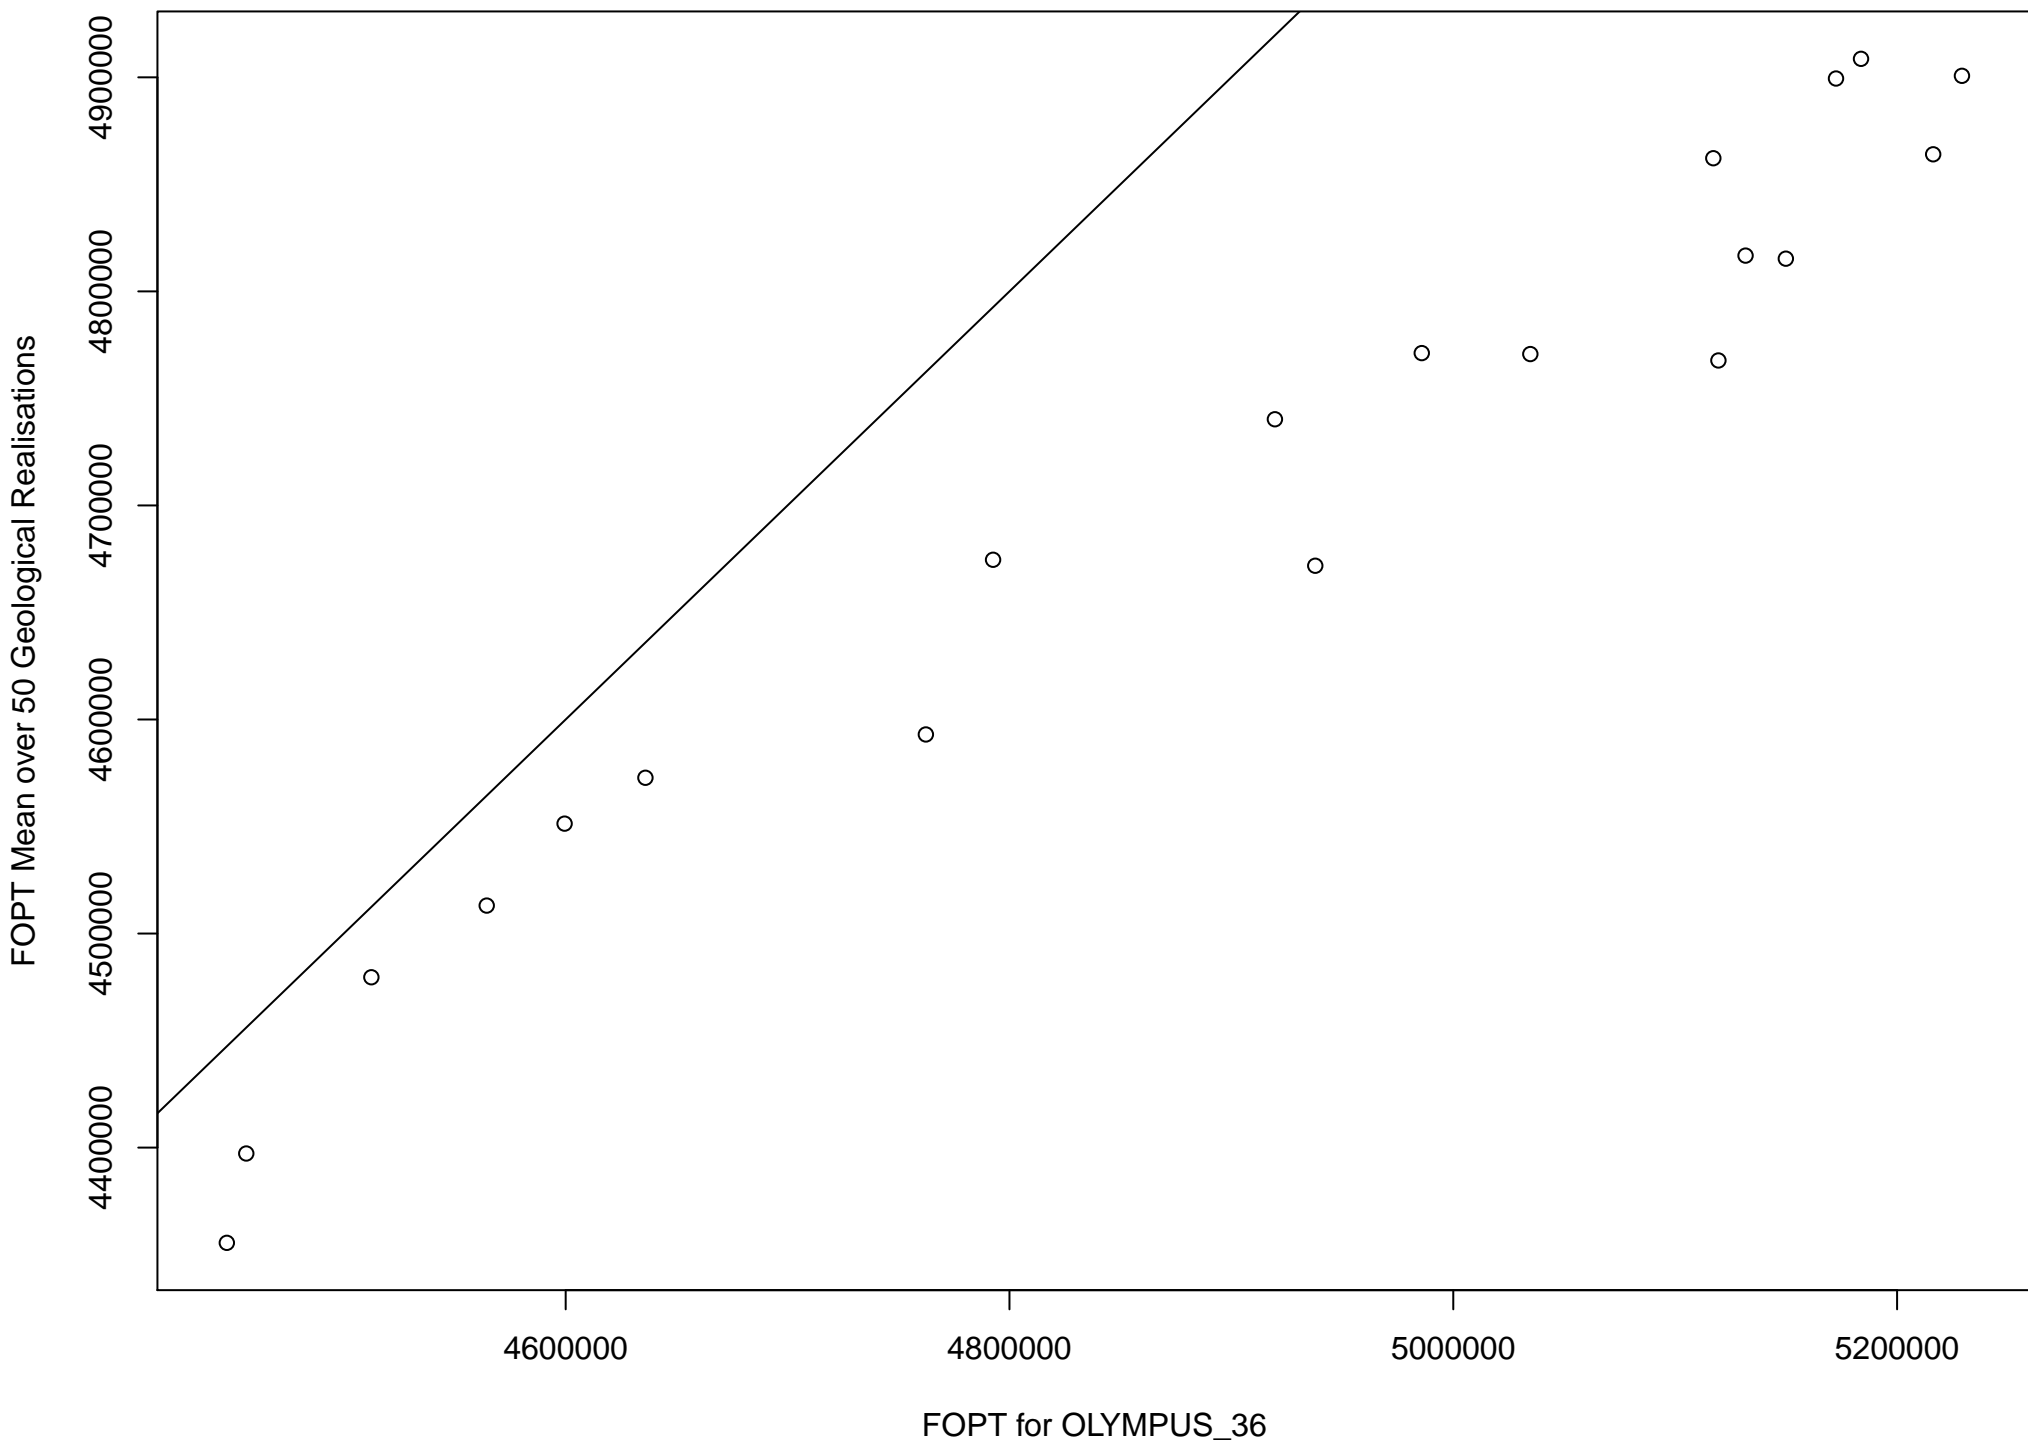

FOPT for OLYMPUS\_37

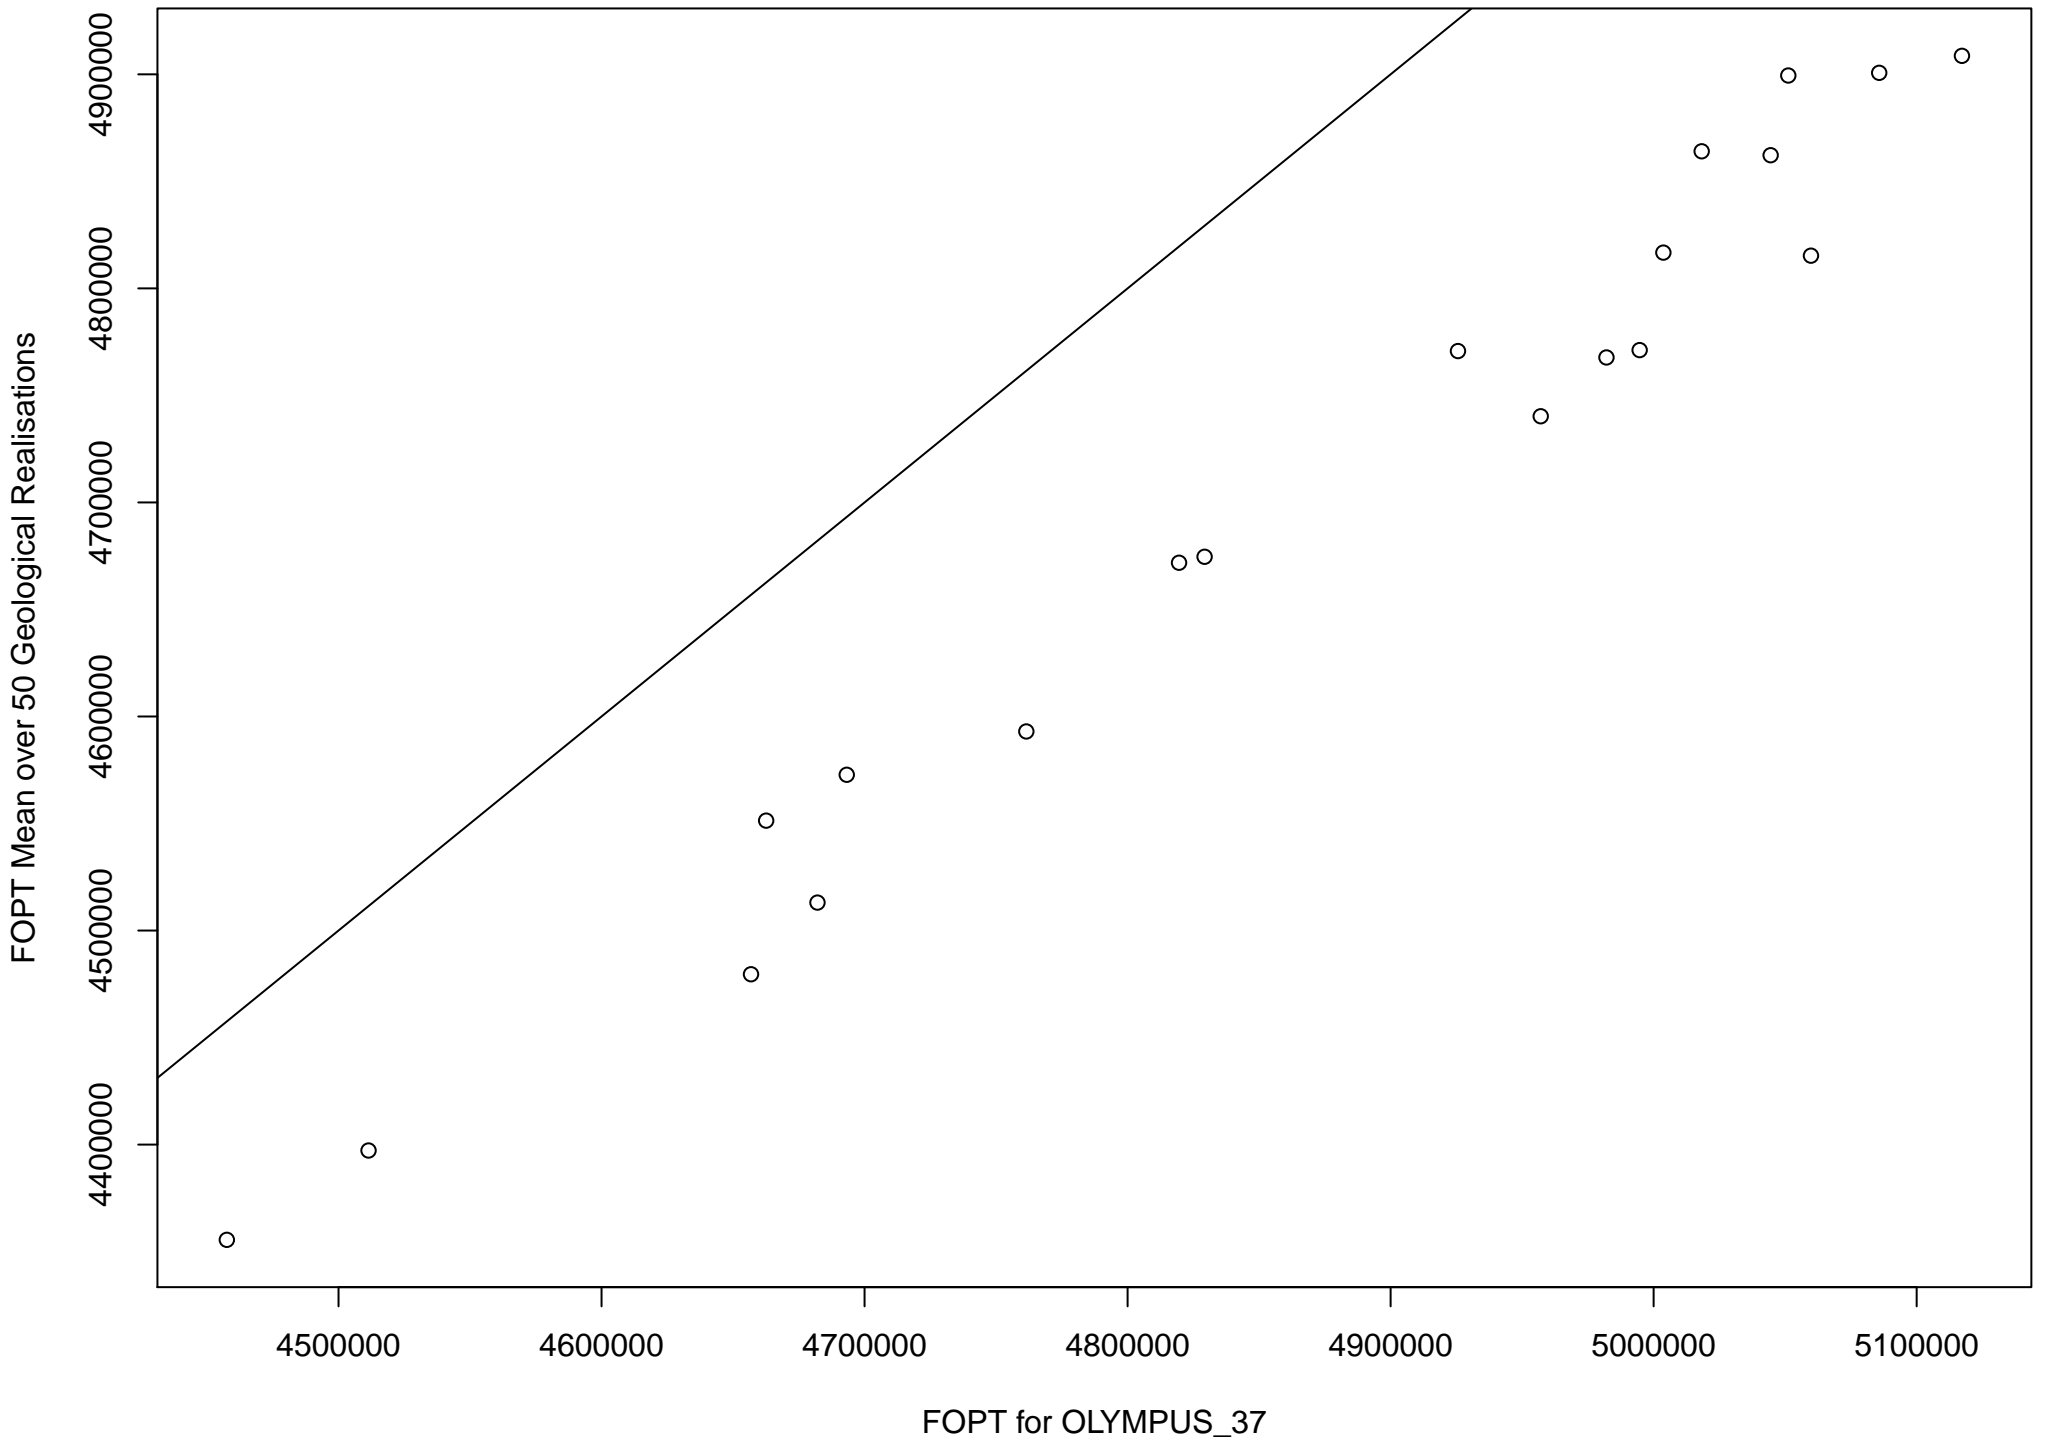

FOPT for OLYMPUS\_38

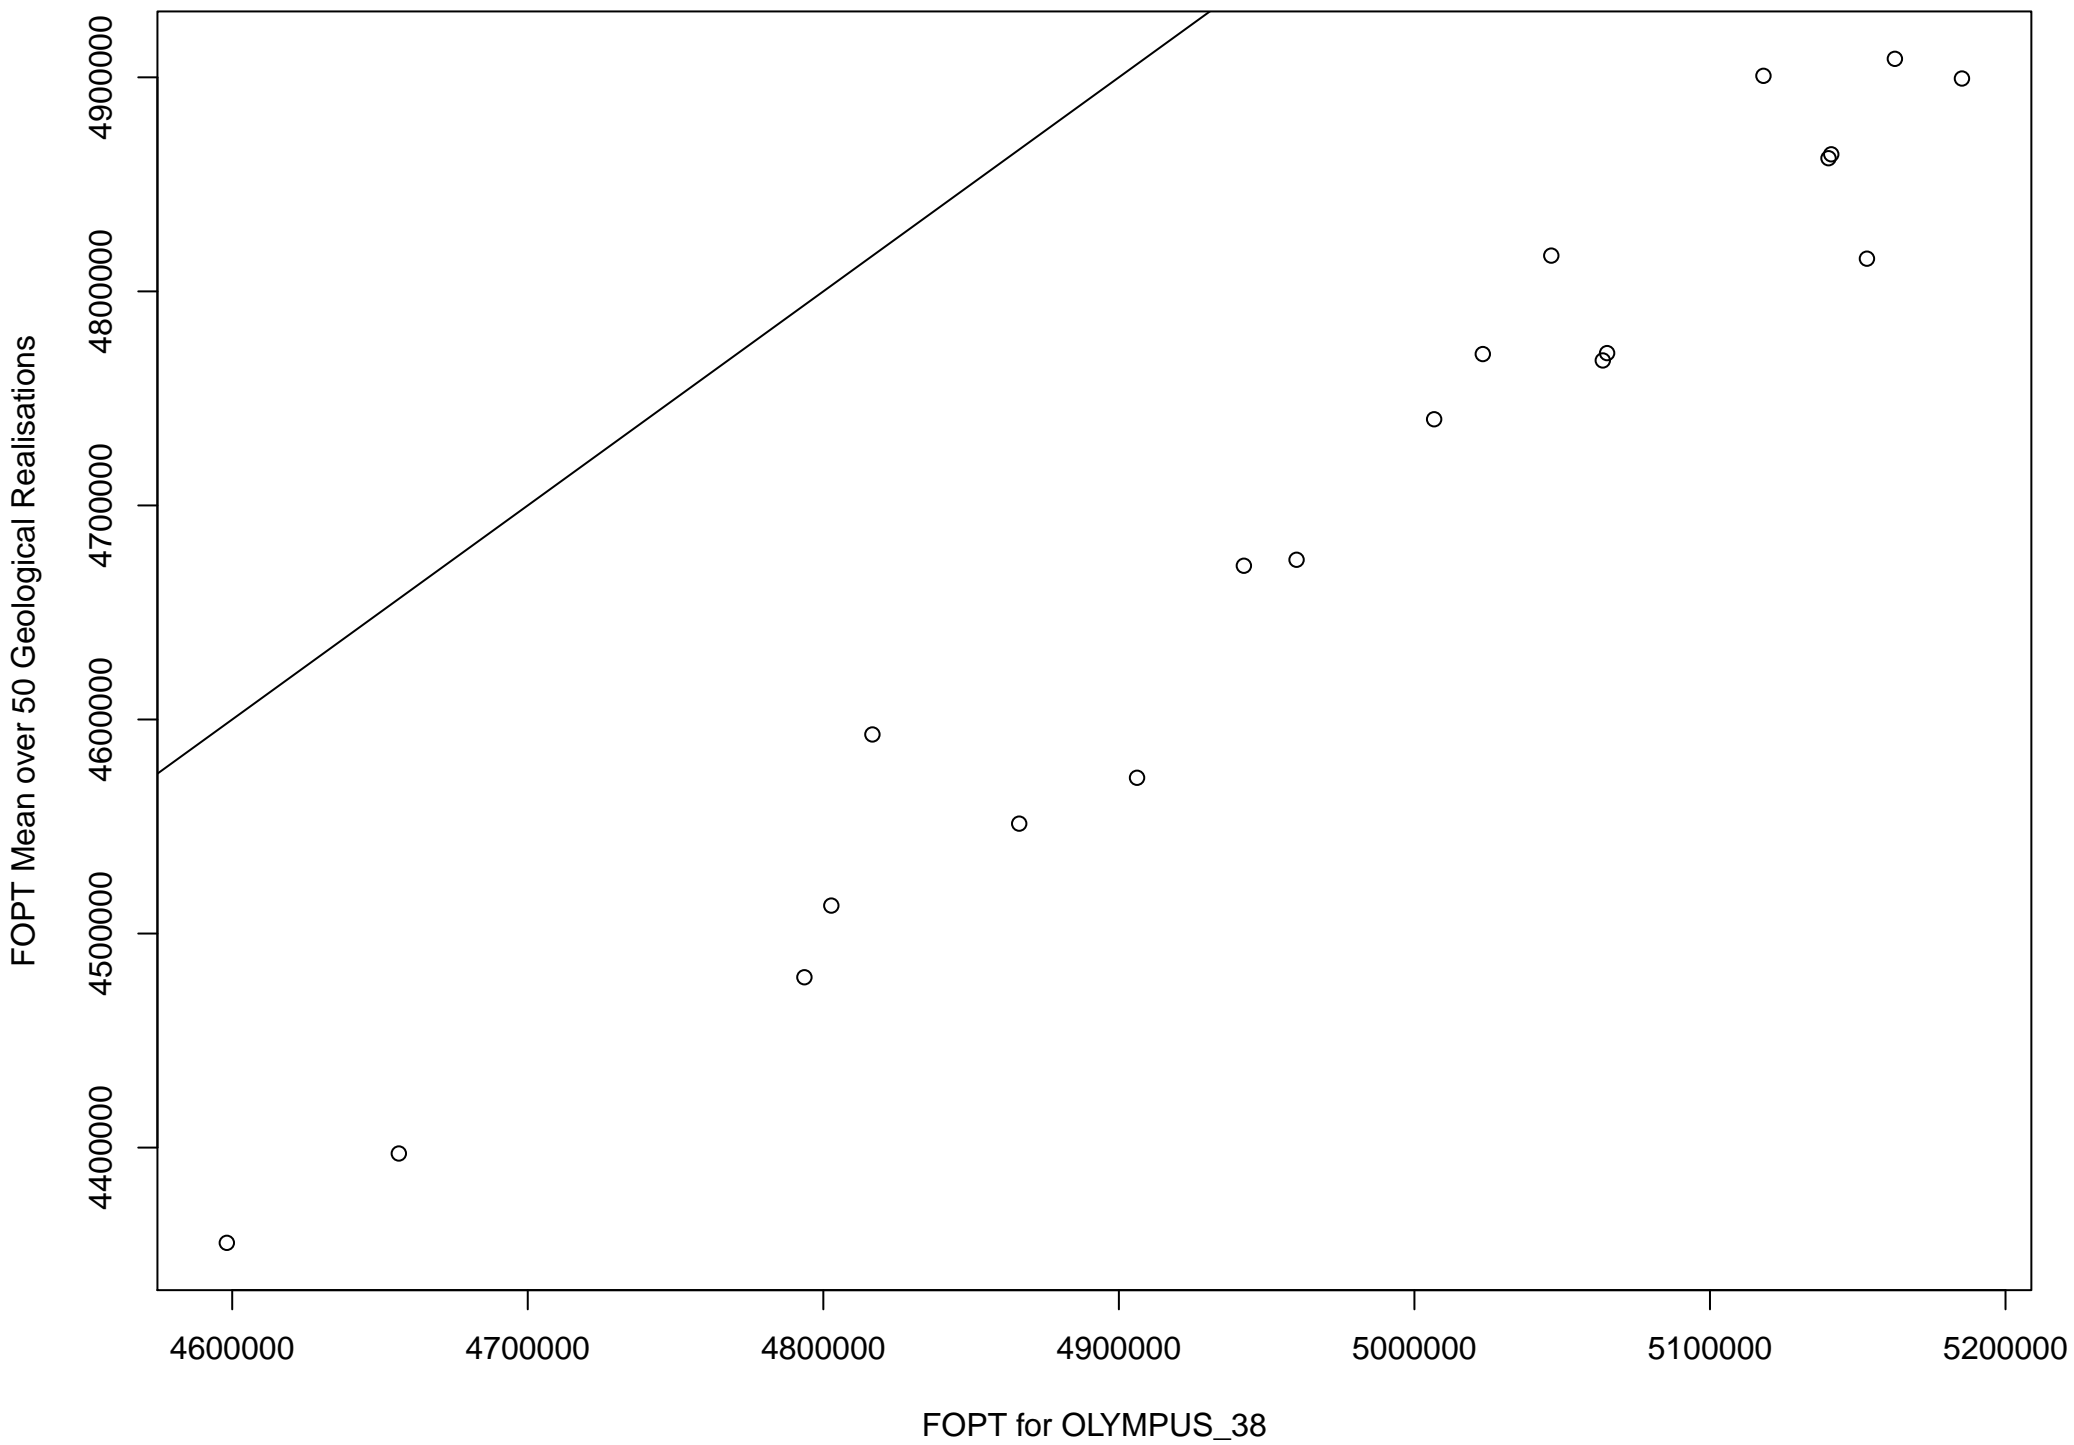

FOPT for OLYMPUS\_39

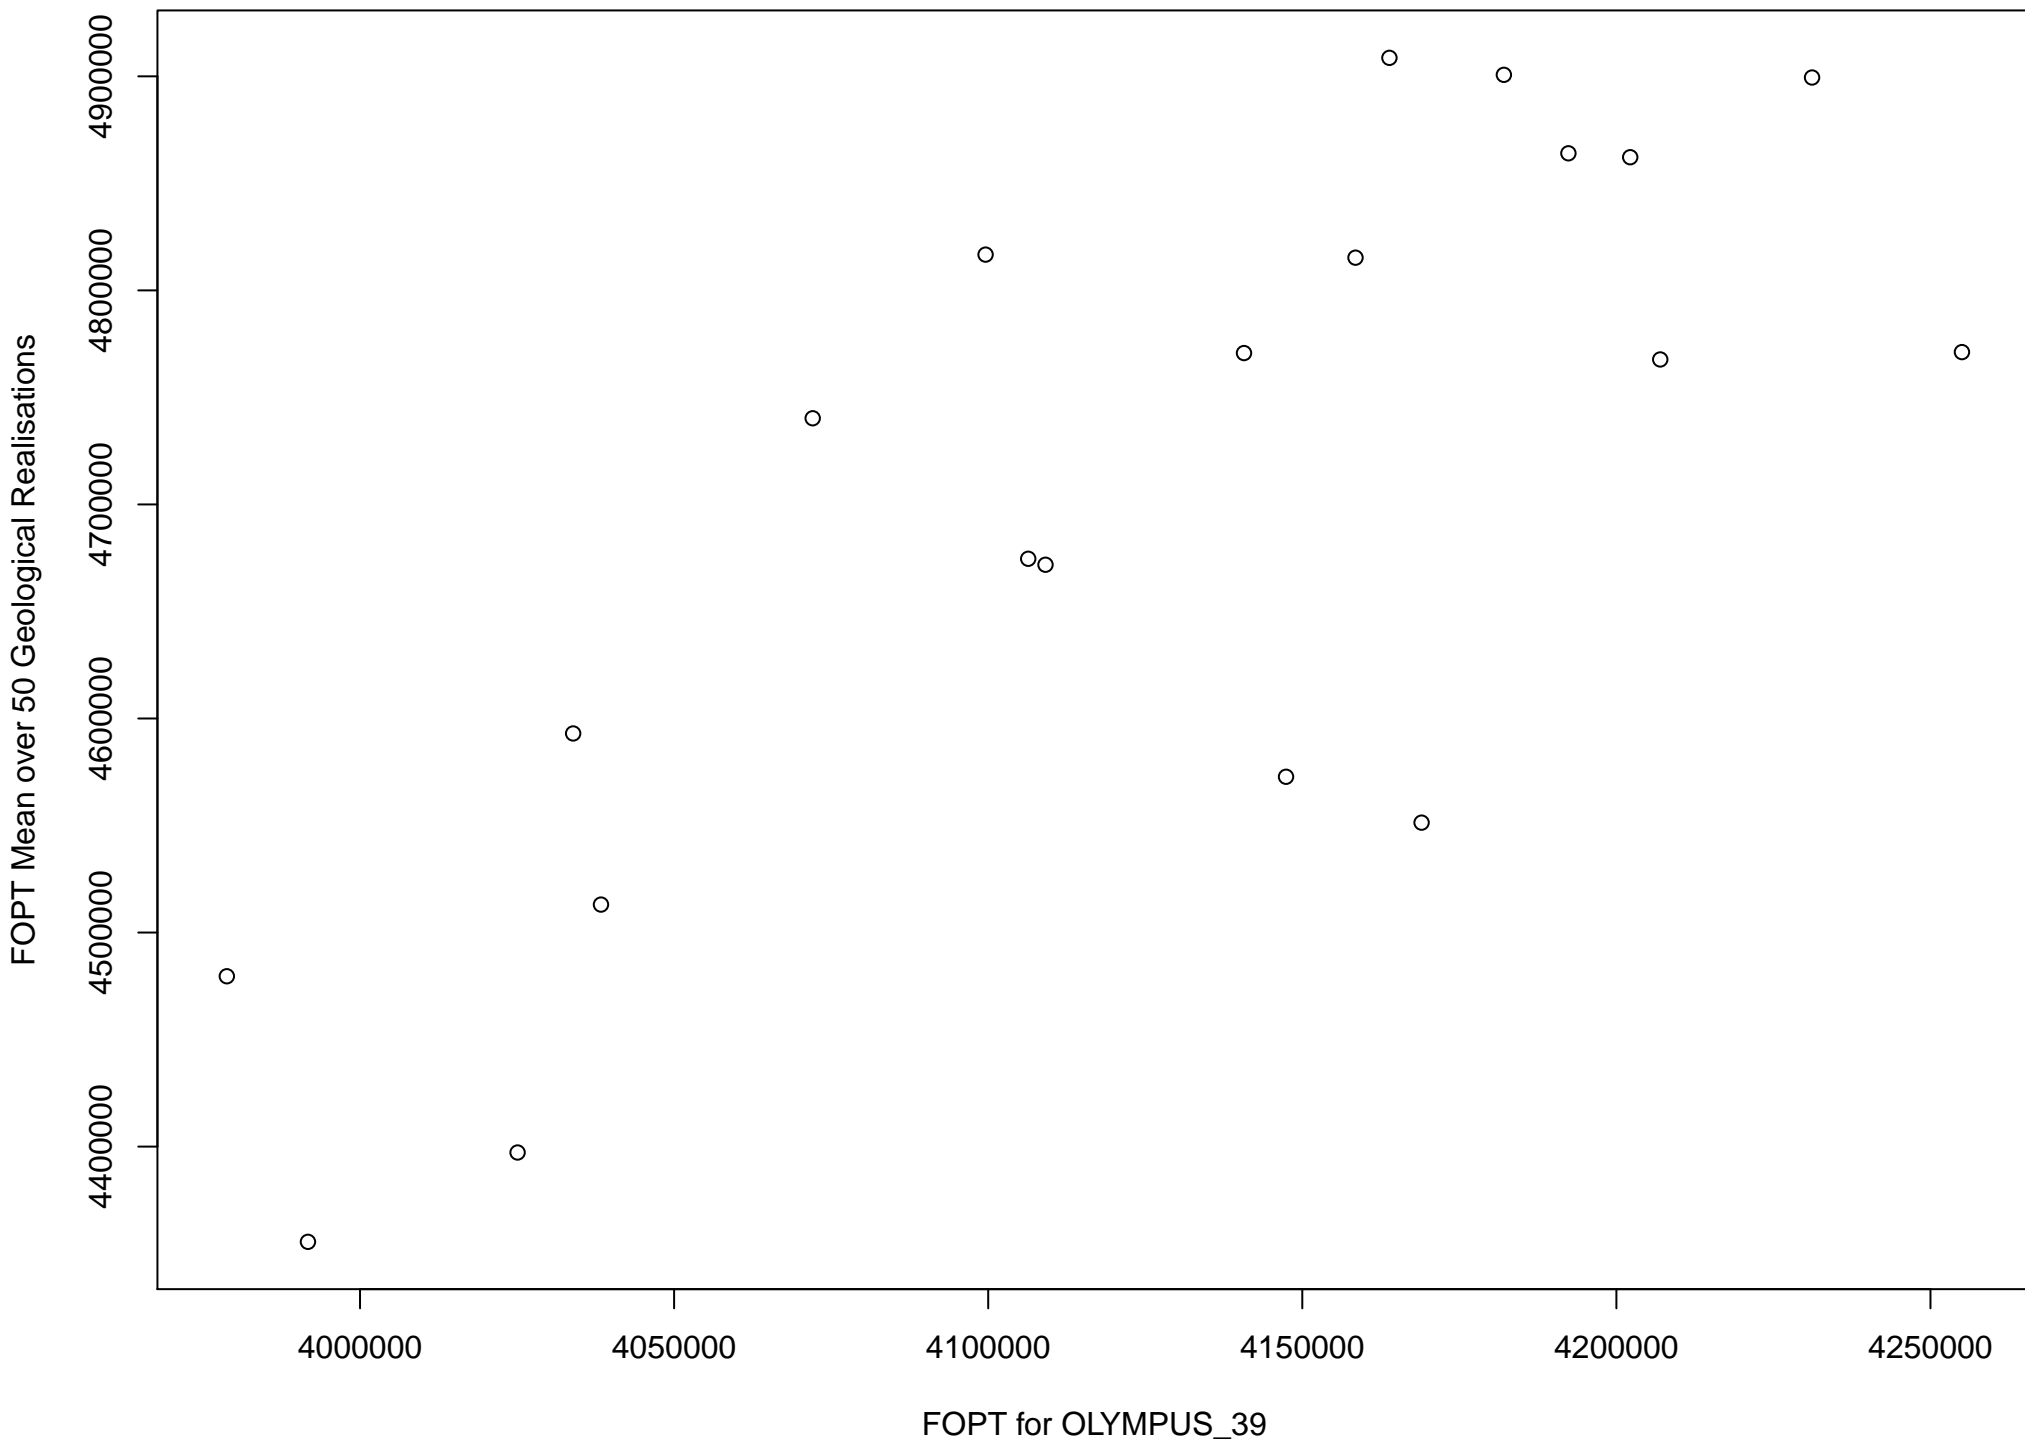

FOPT for OLYMPUS\_40

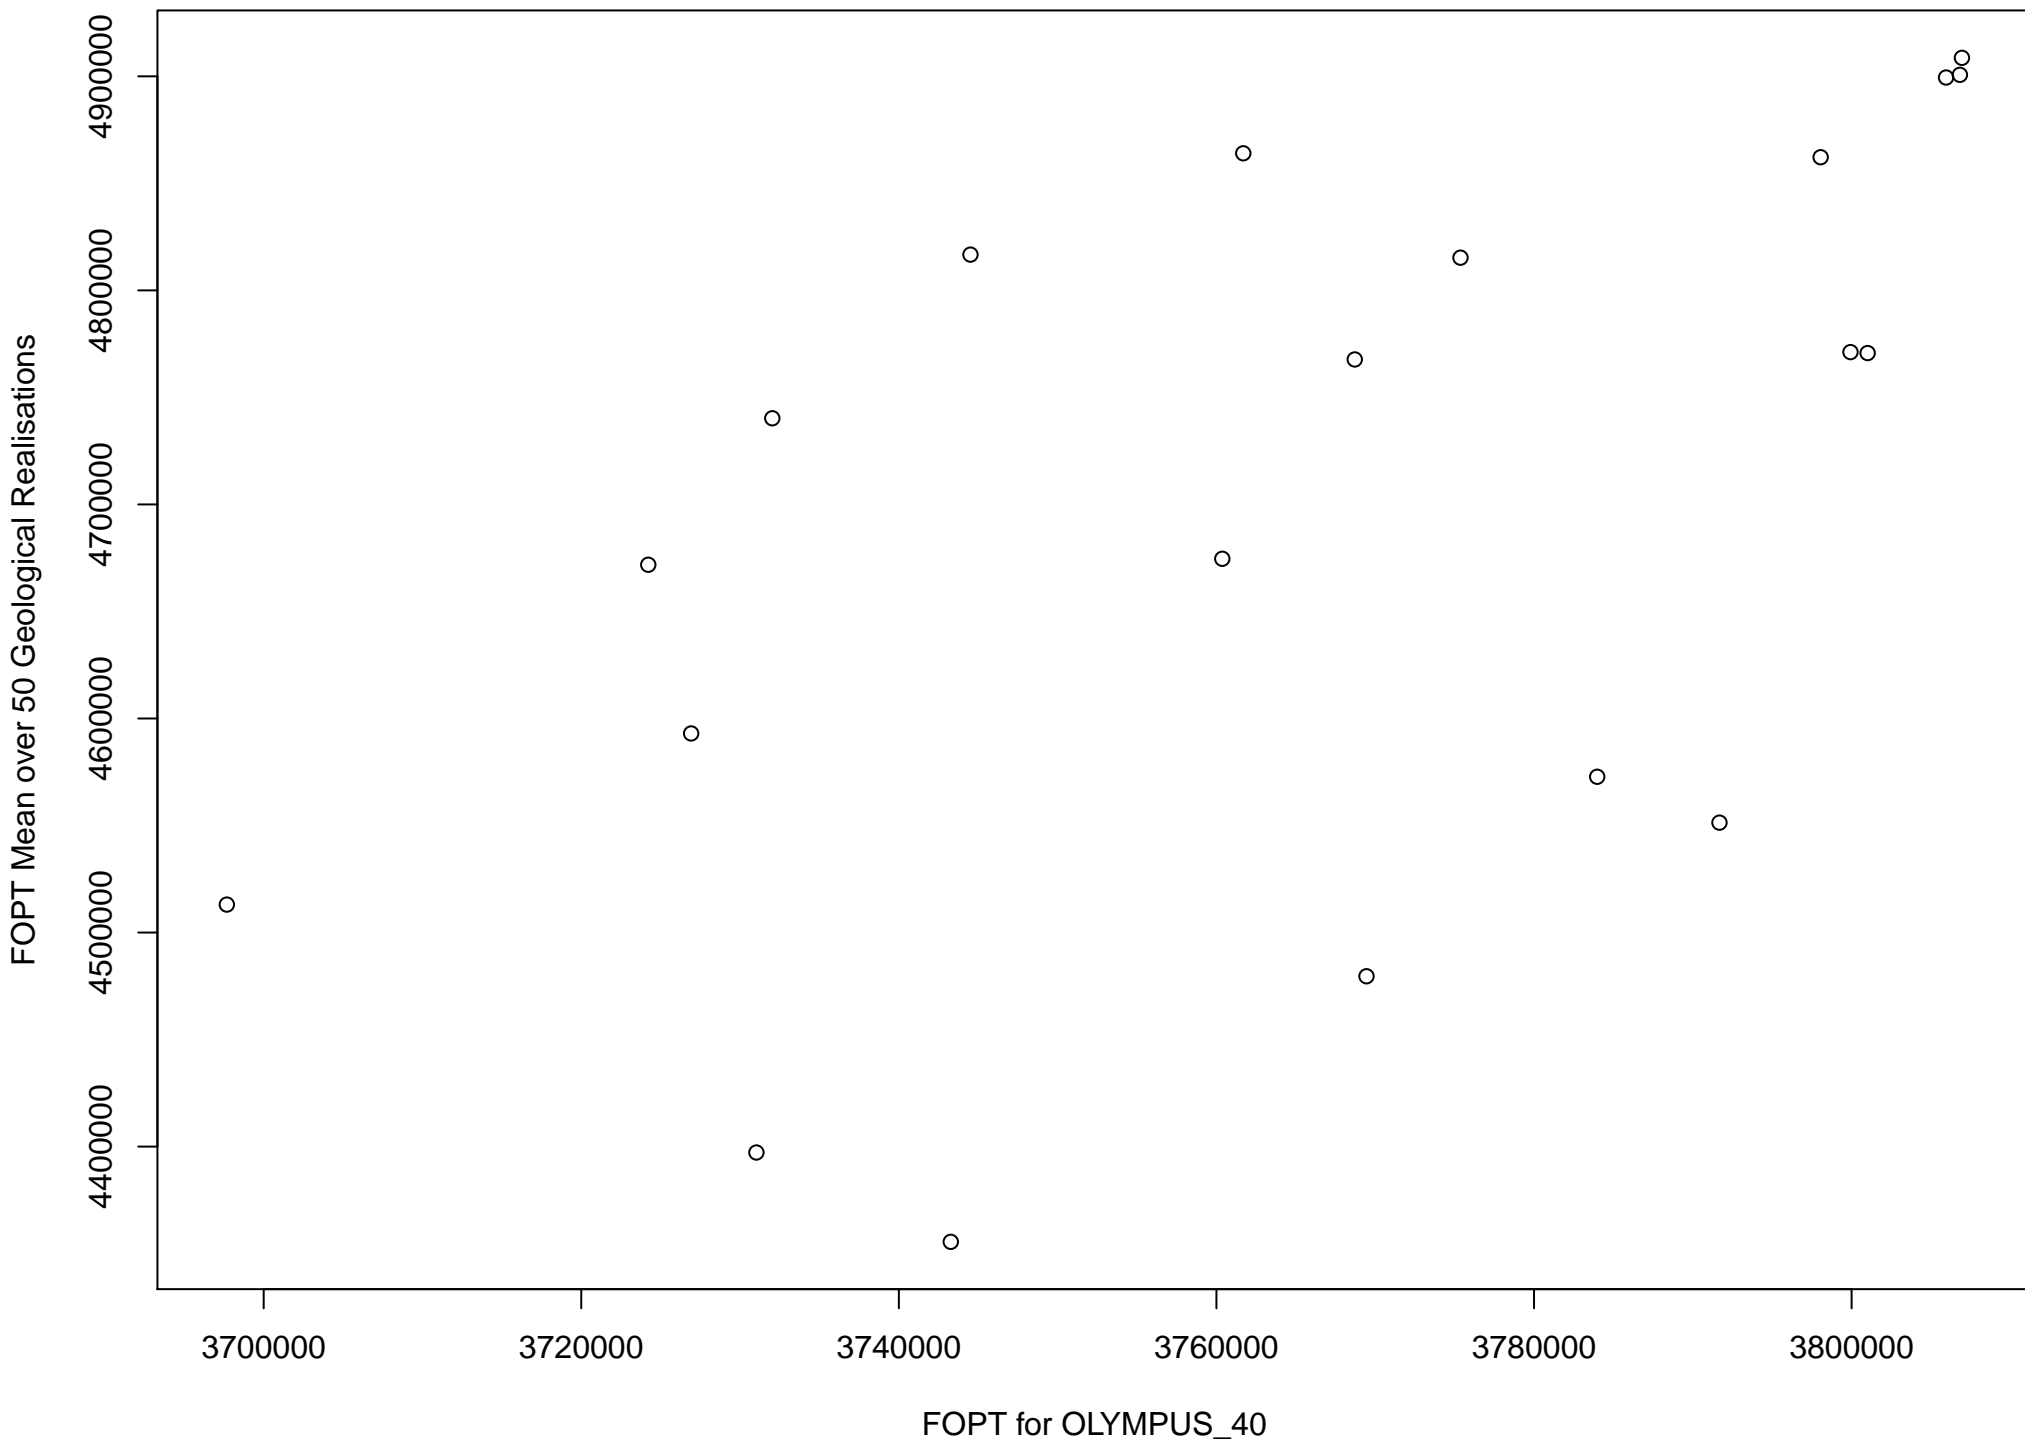



FOPT for OLYMPUS\_41

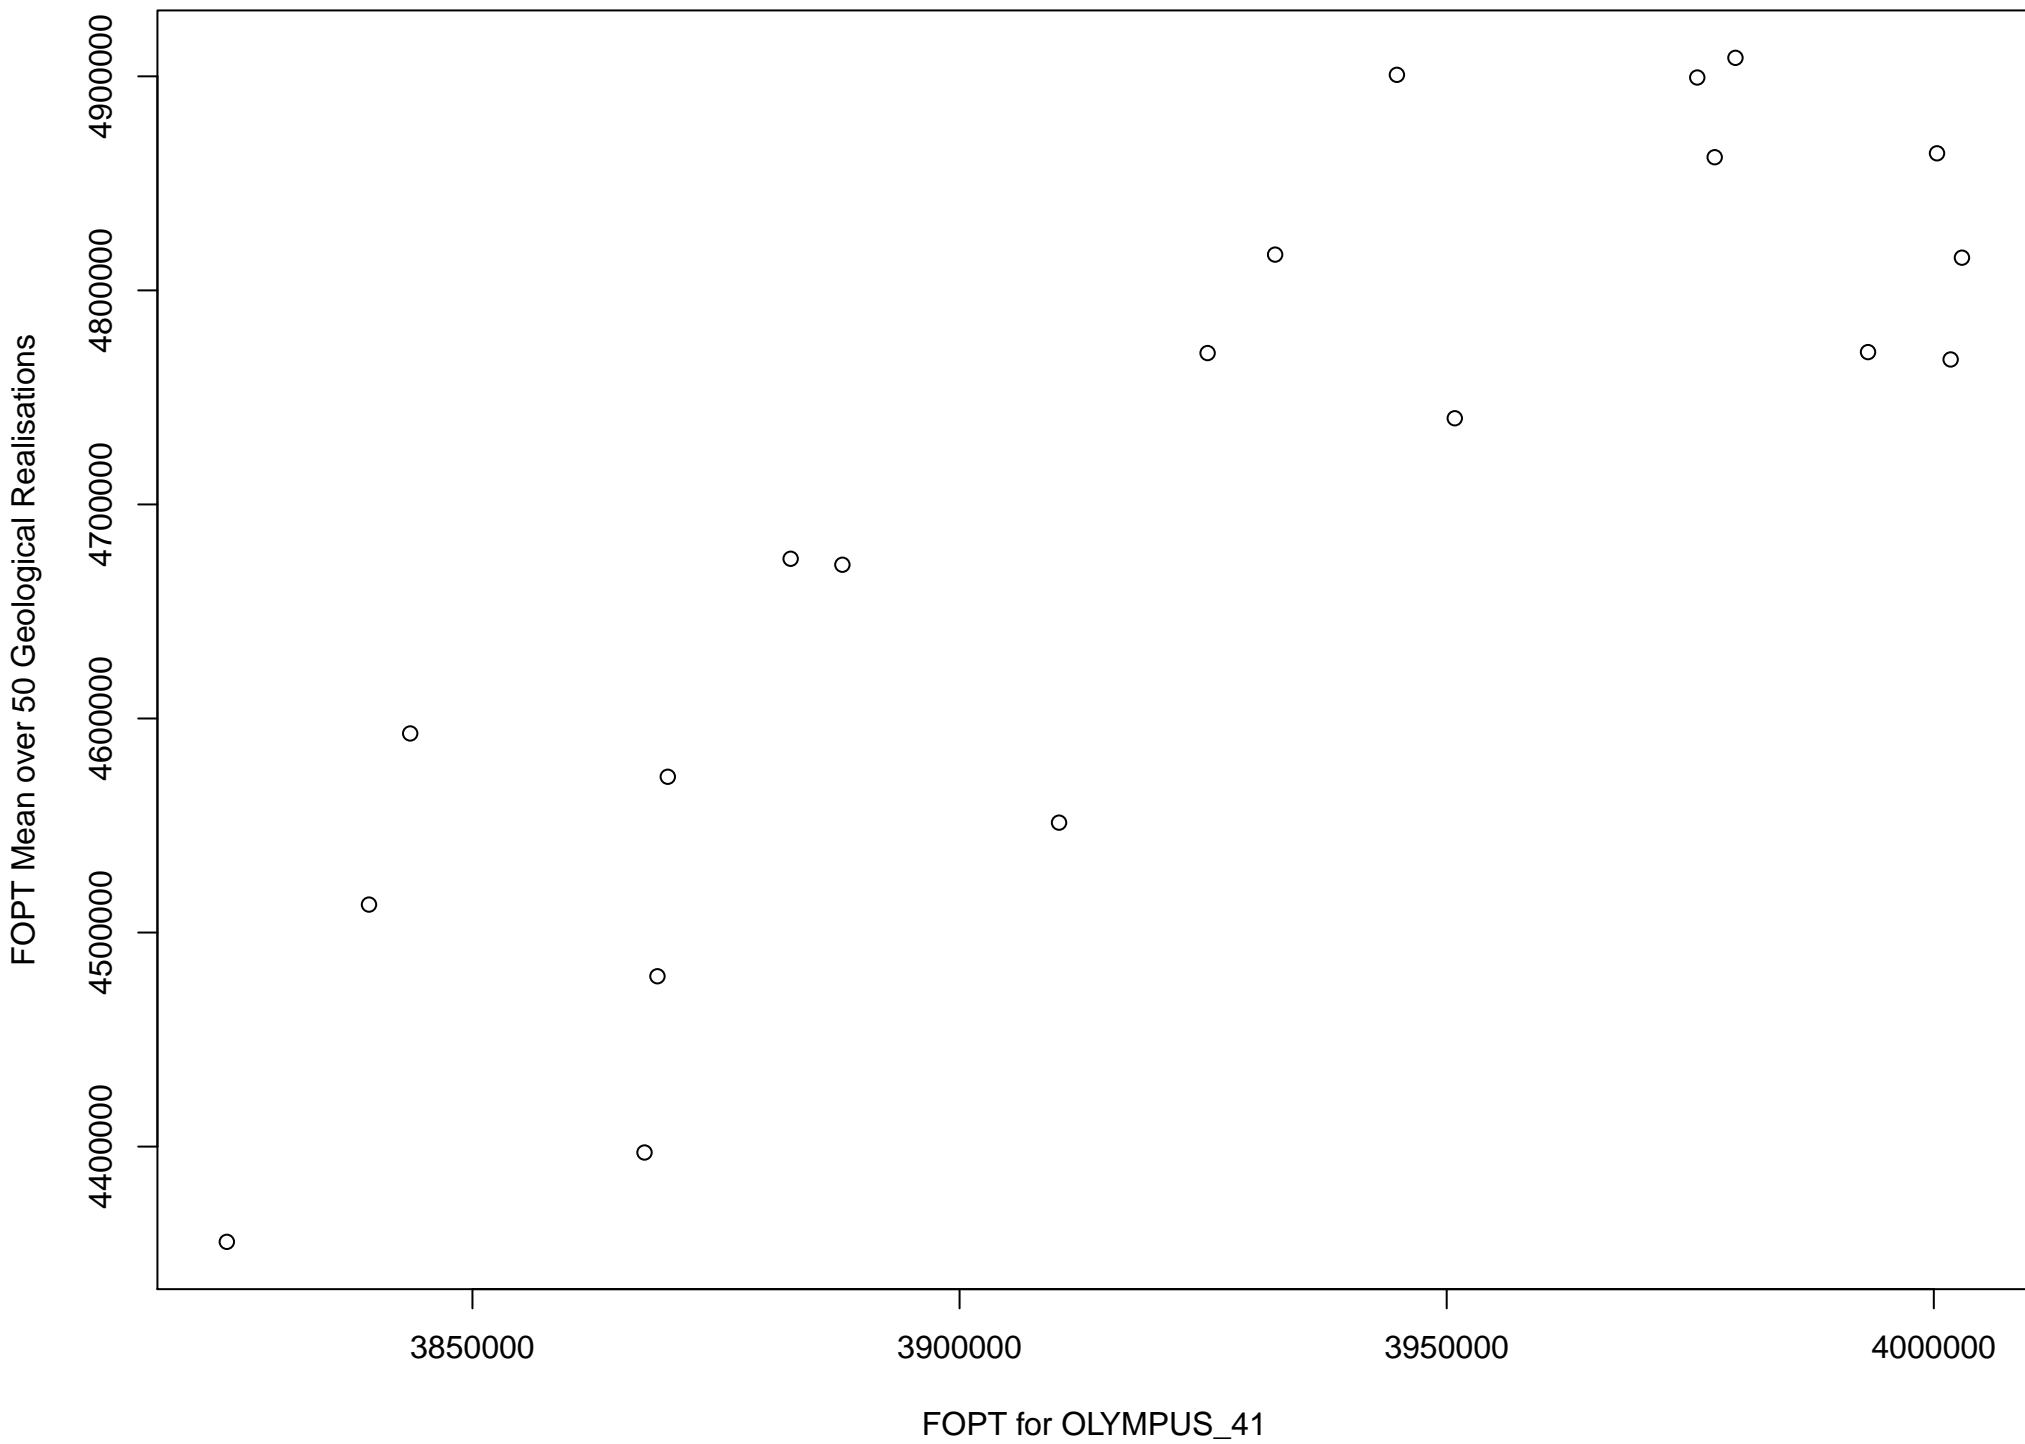

FOPT for OLYMPUS\_42

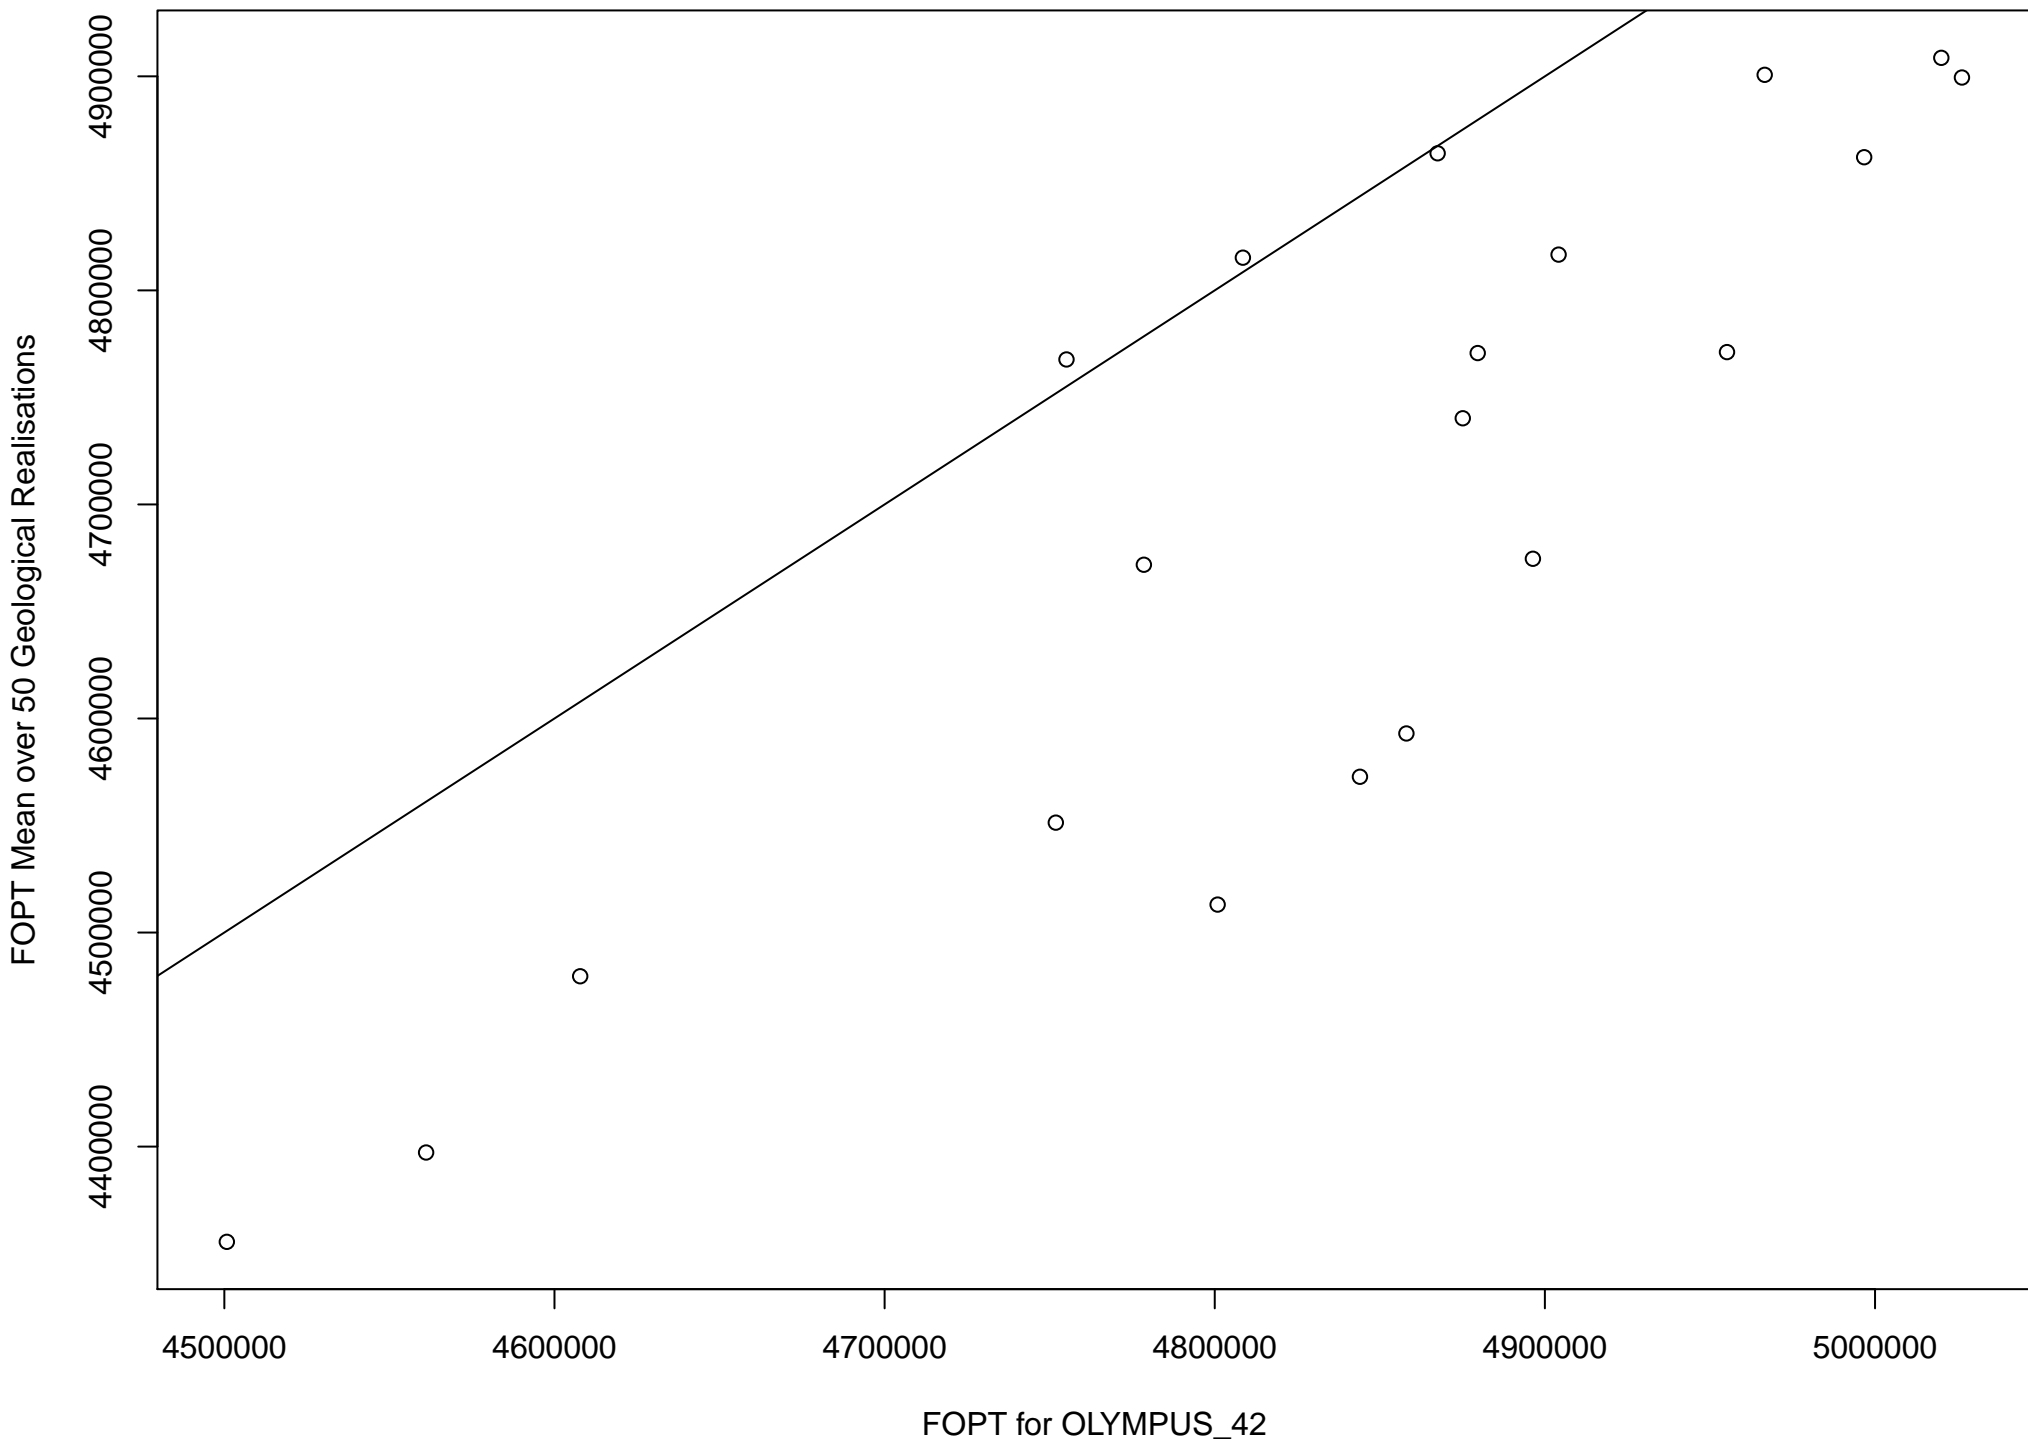

FOPT for OLYMPUS\_43

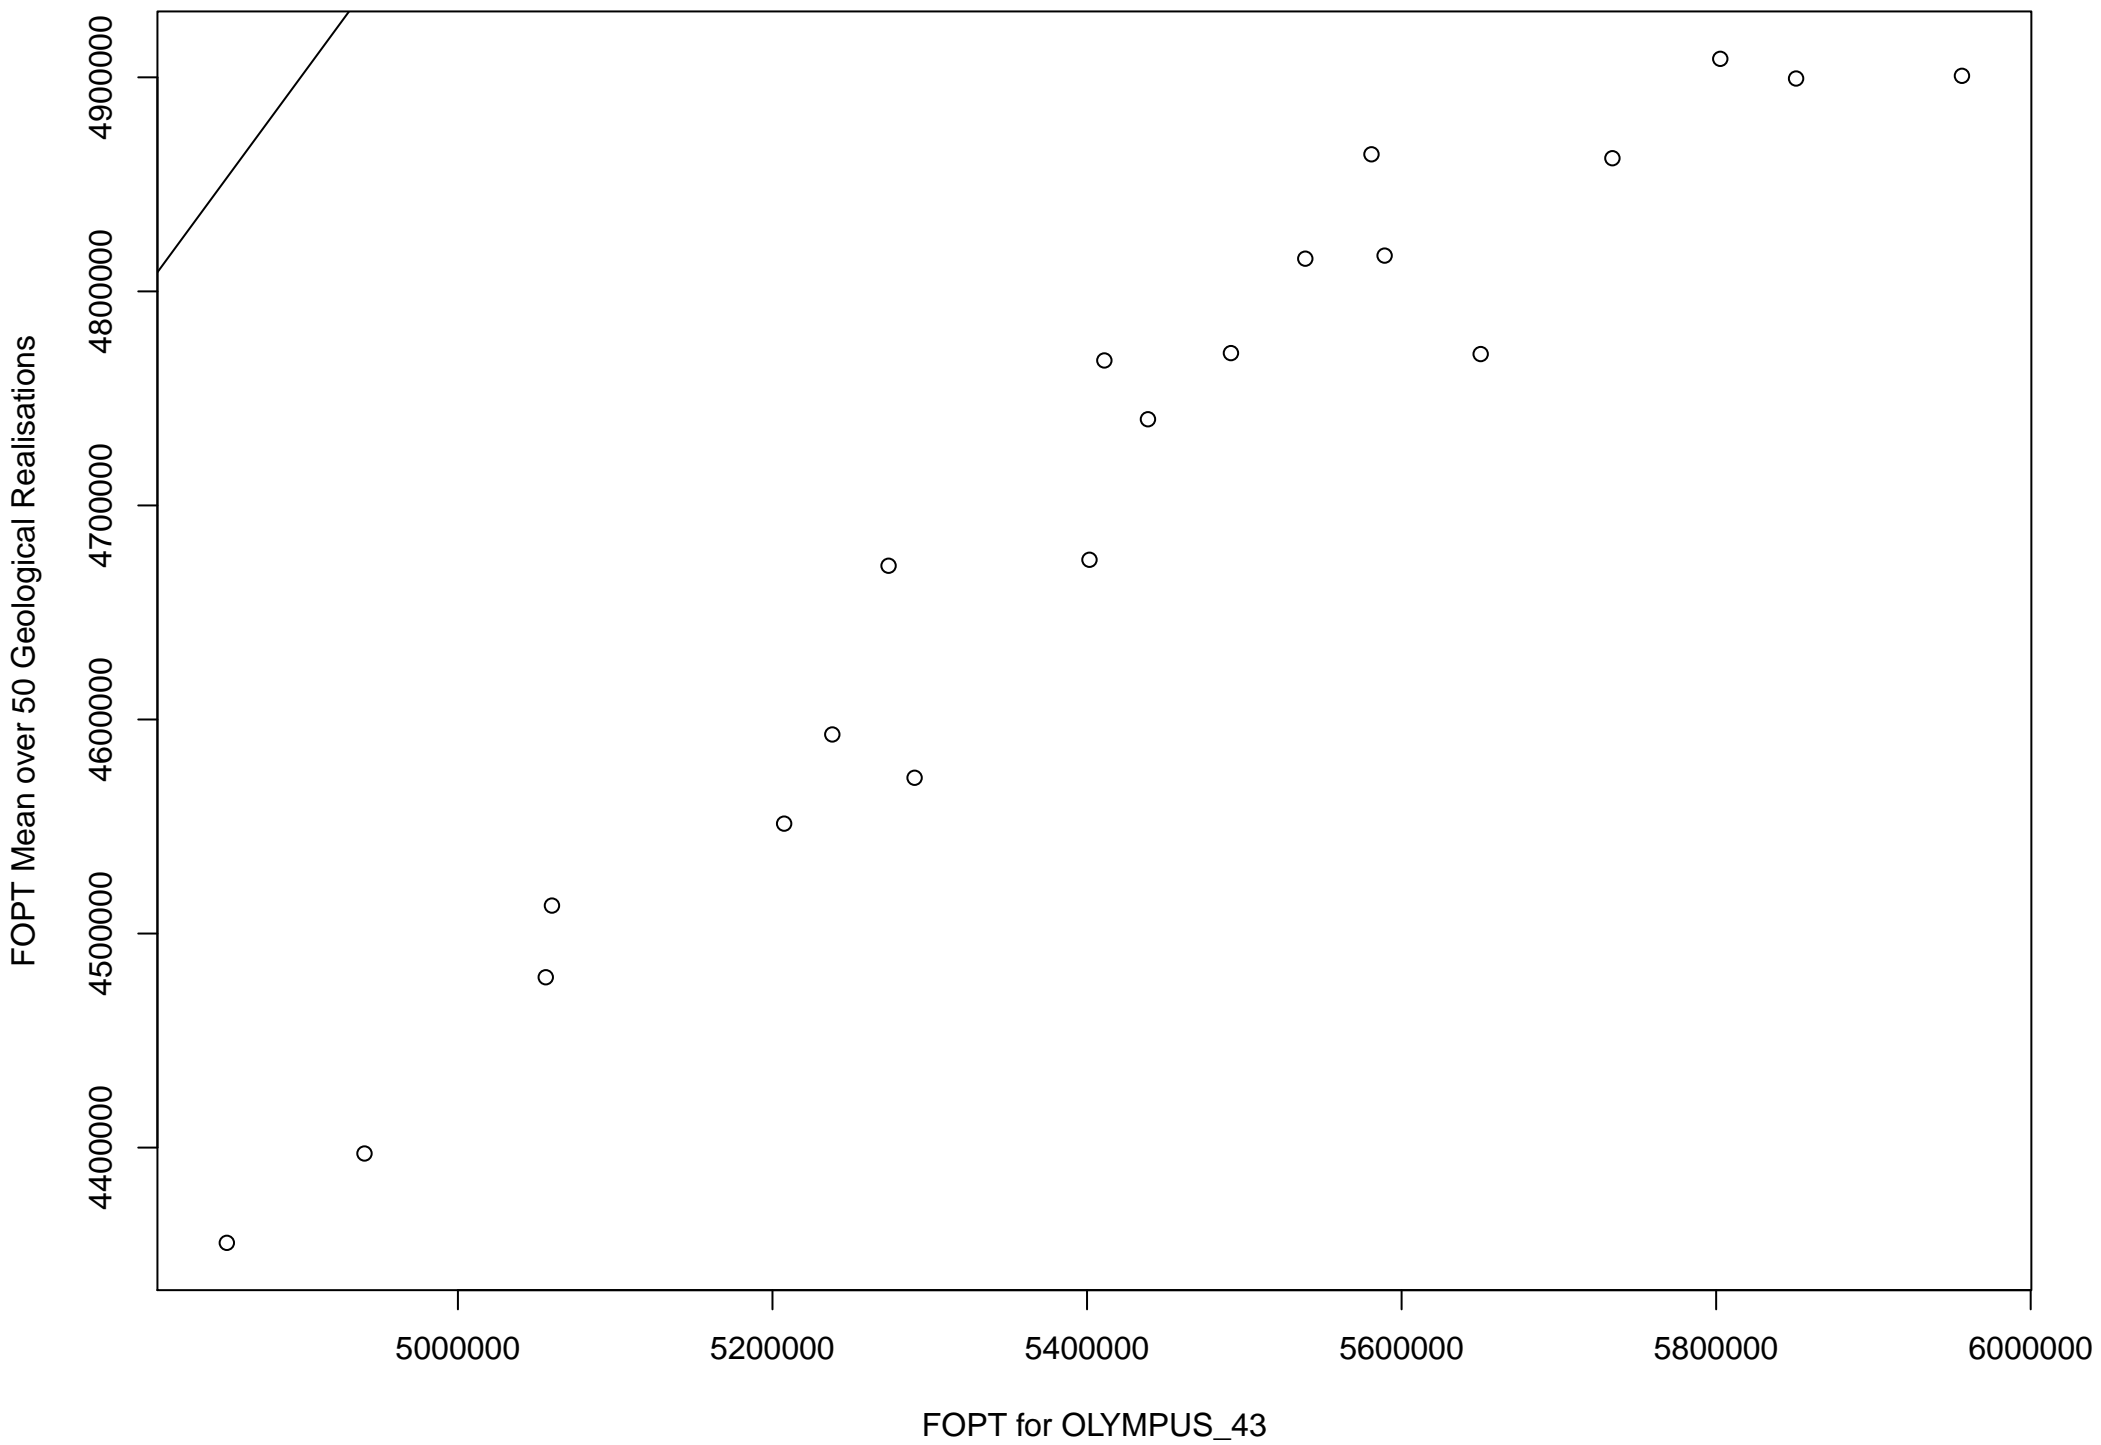

FOPT for OLYMPUS\_44

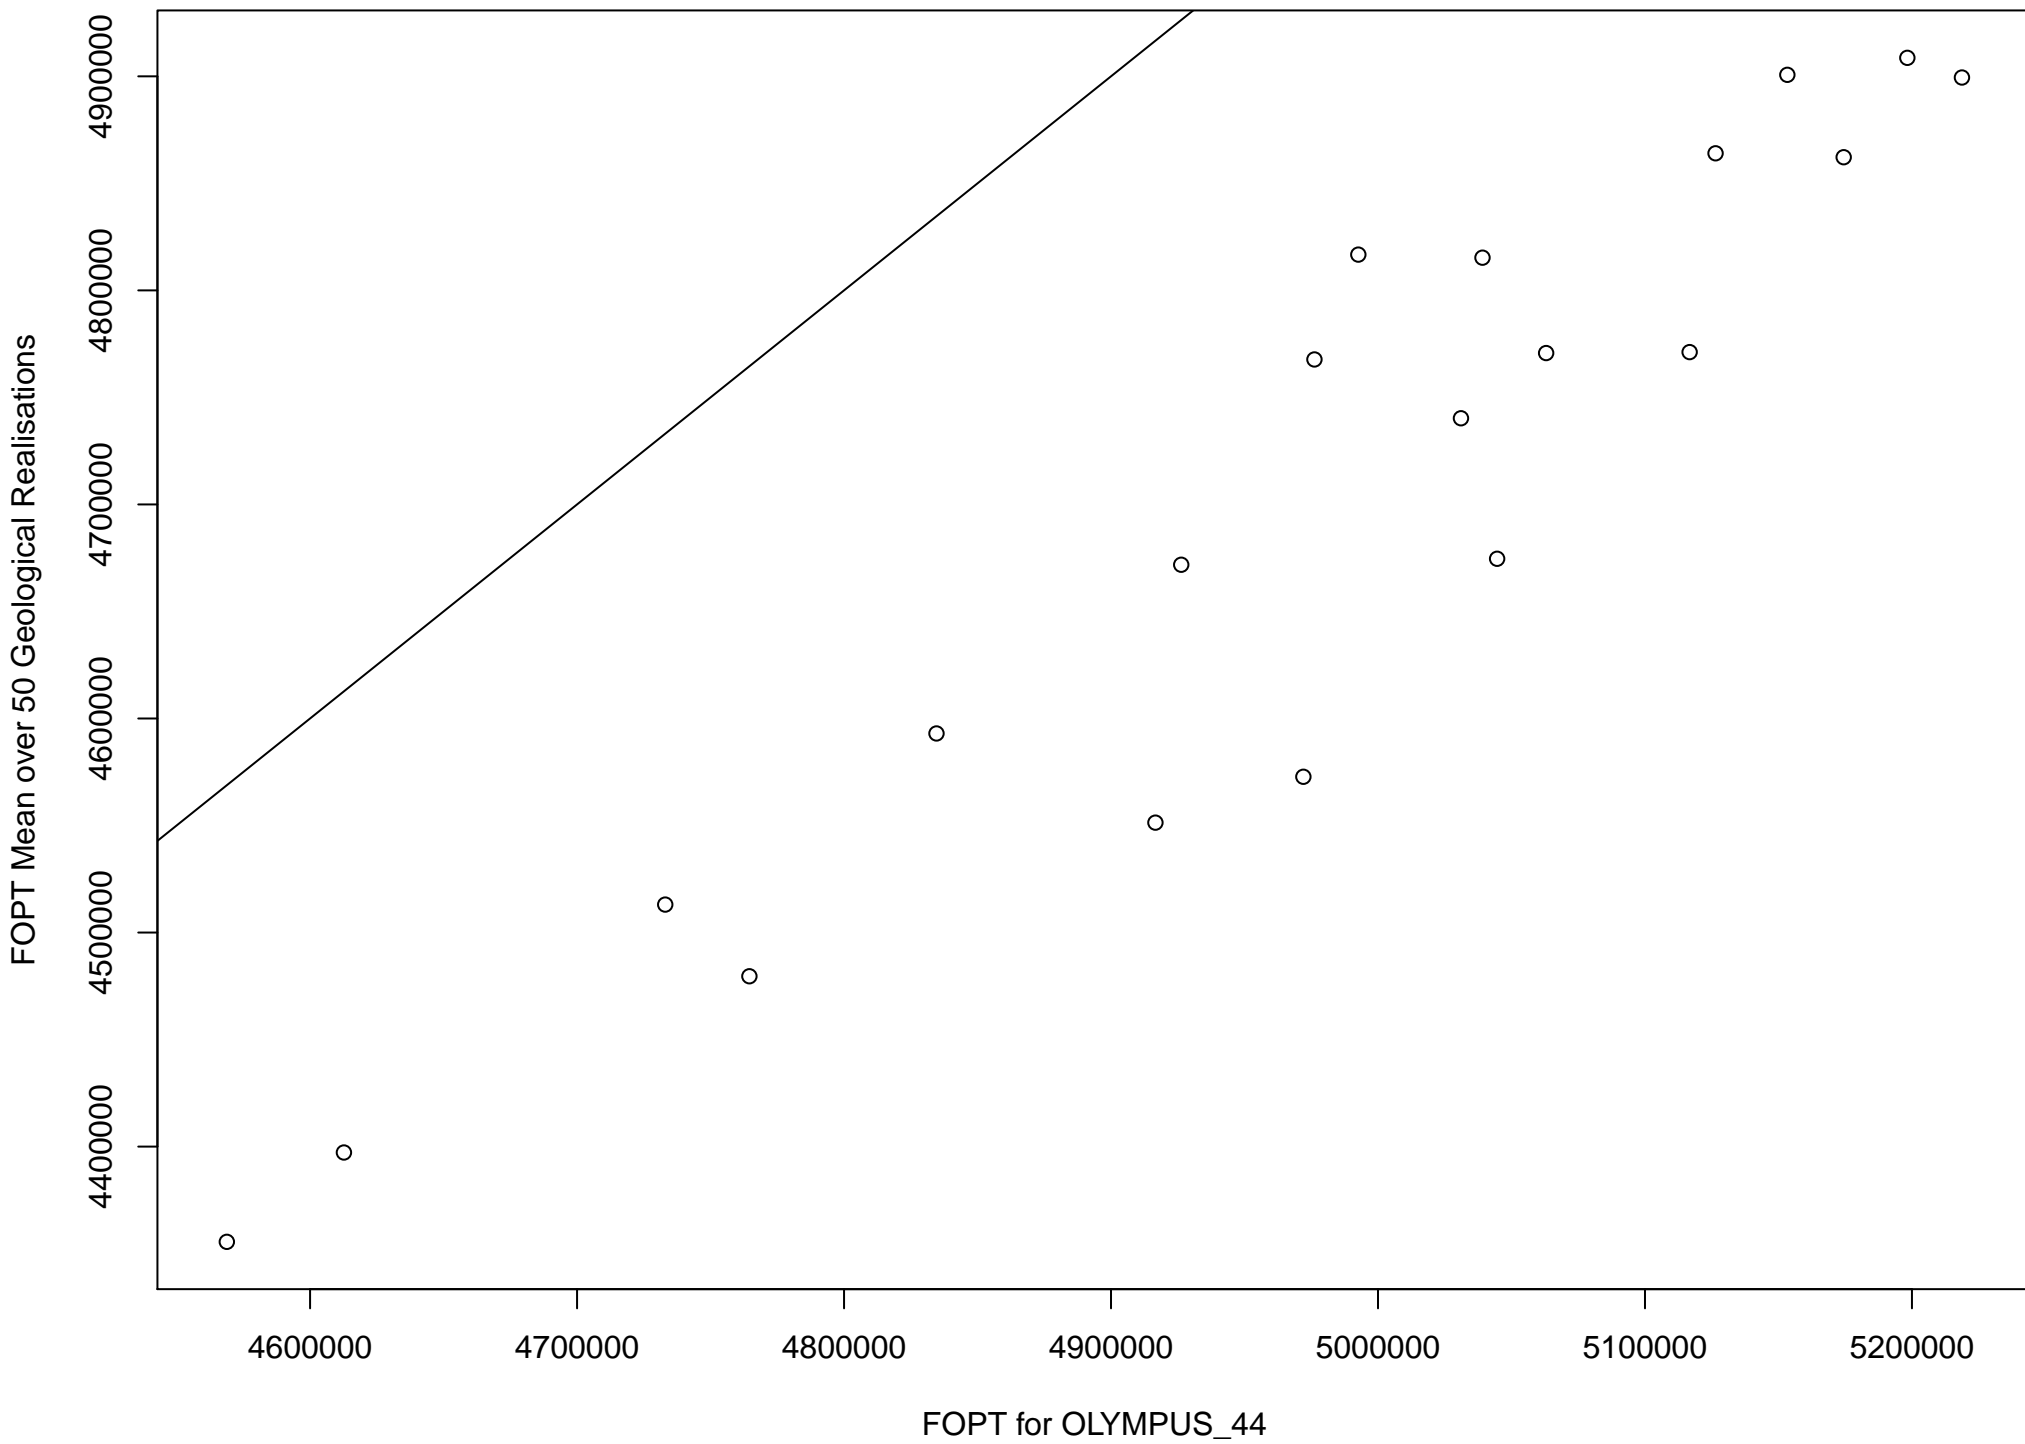

FOPT for OLYMPUS\_45

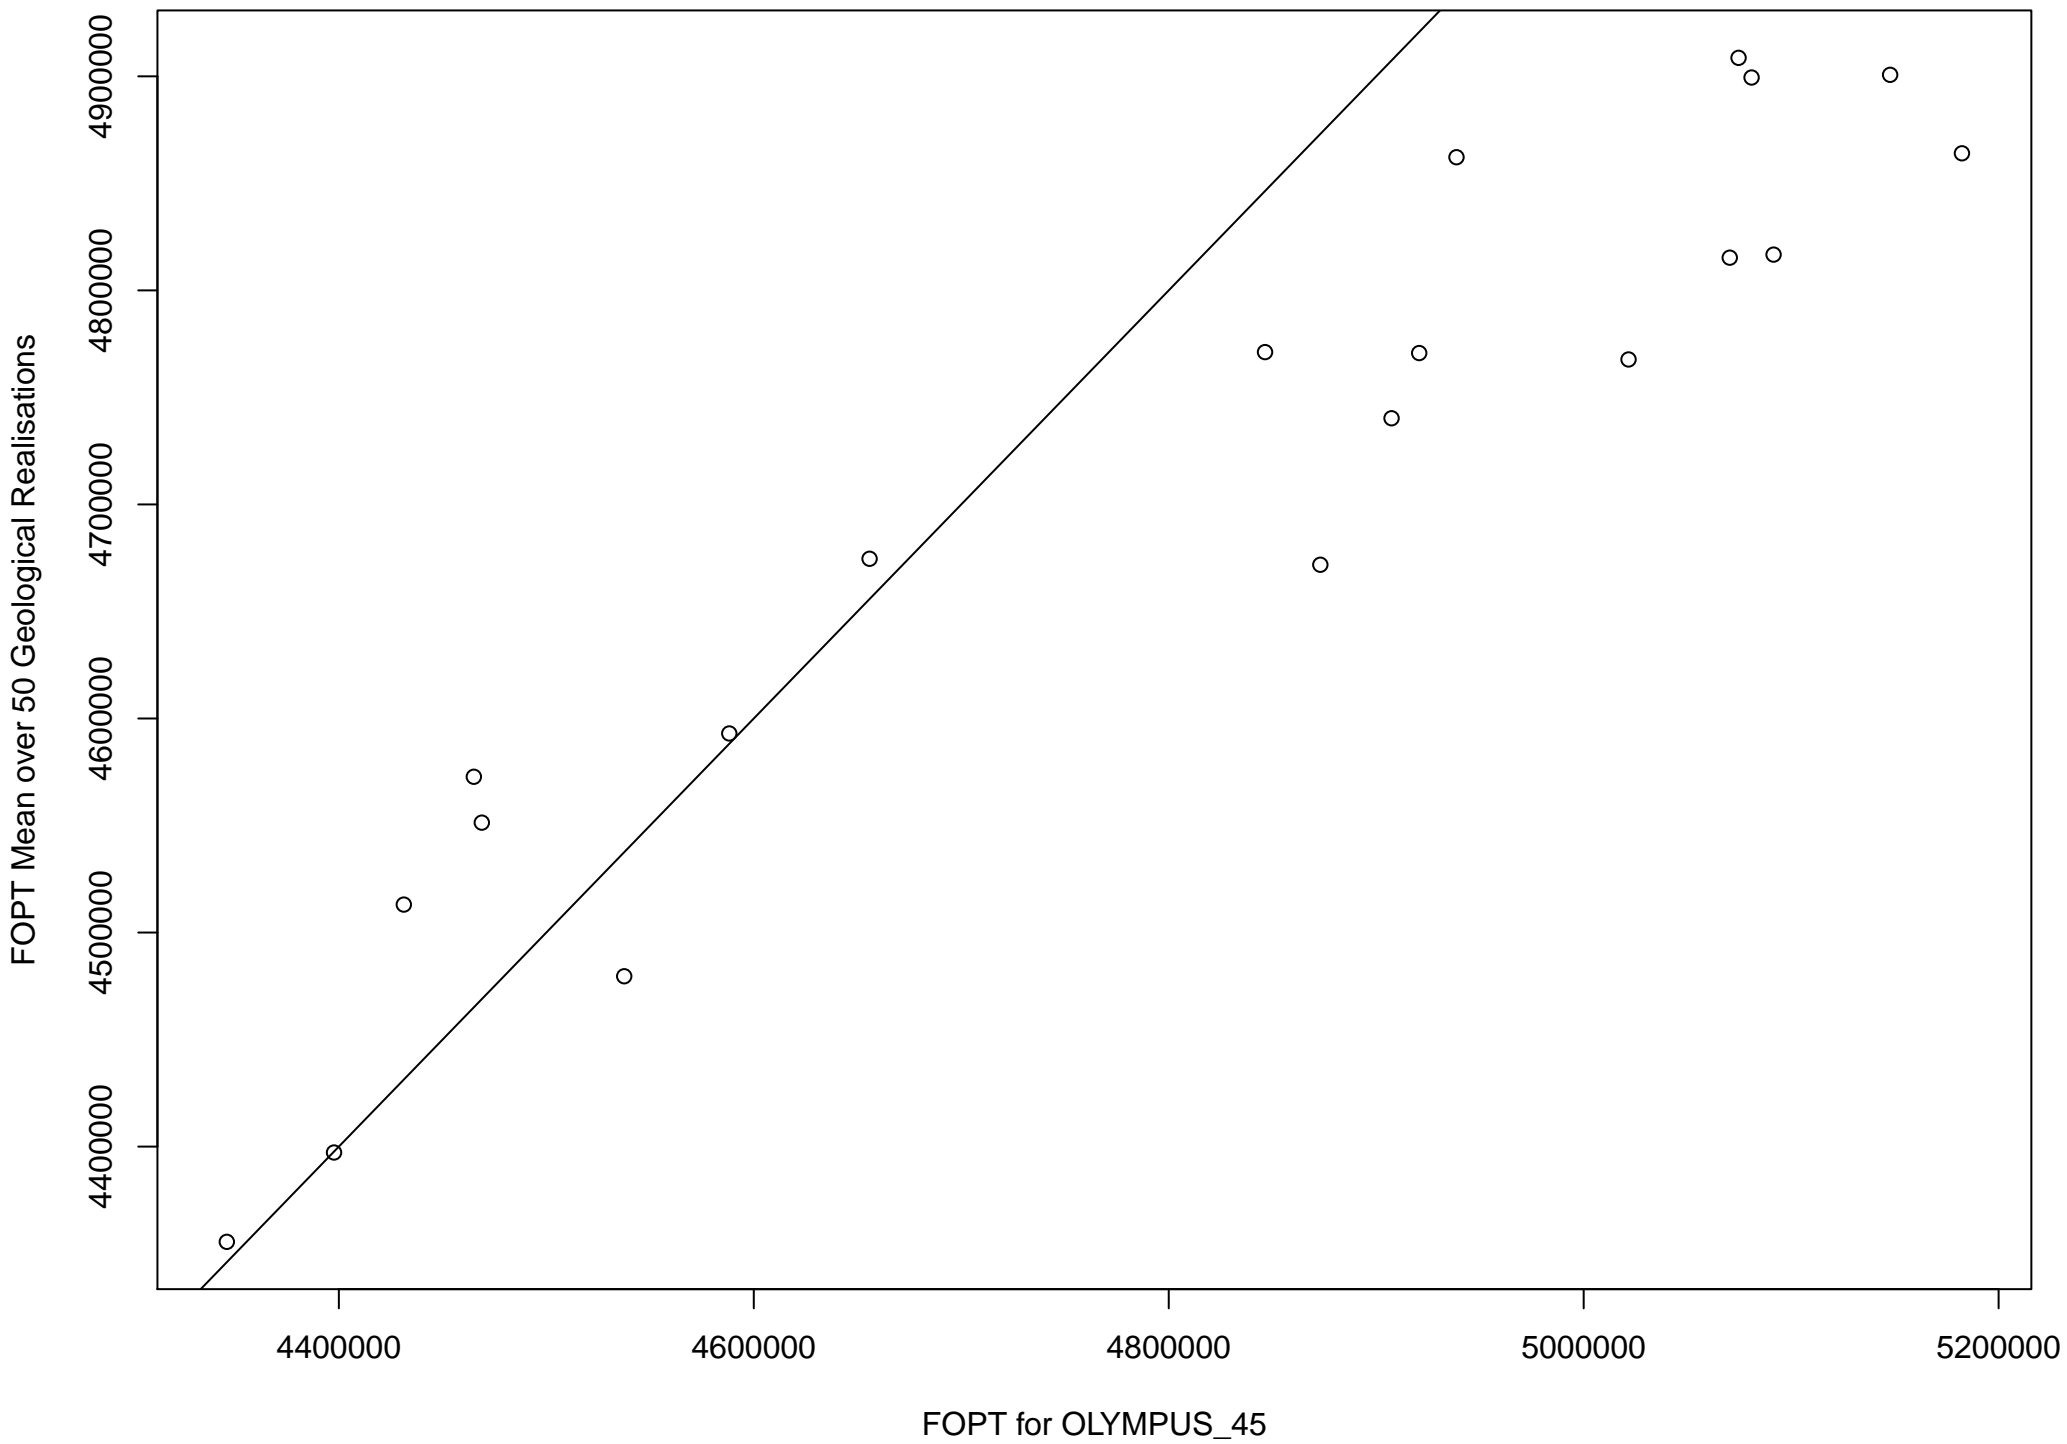

FOPT for OLYMPUS\_46

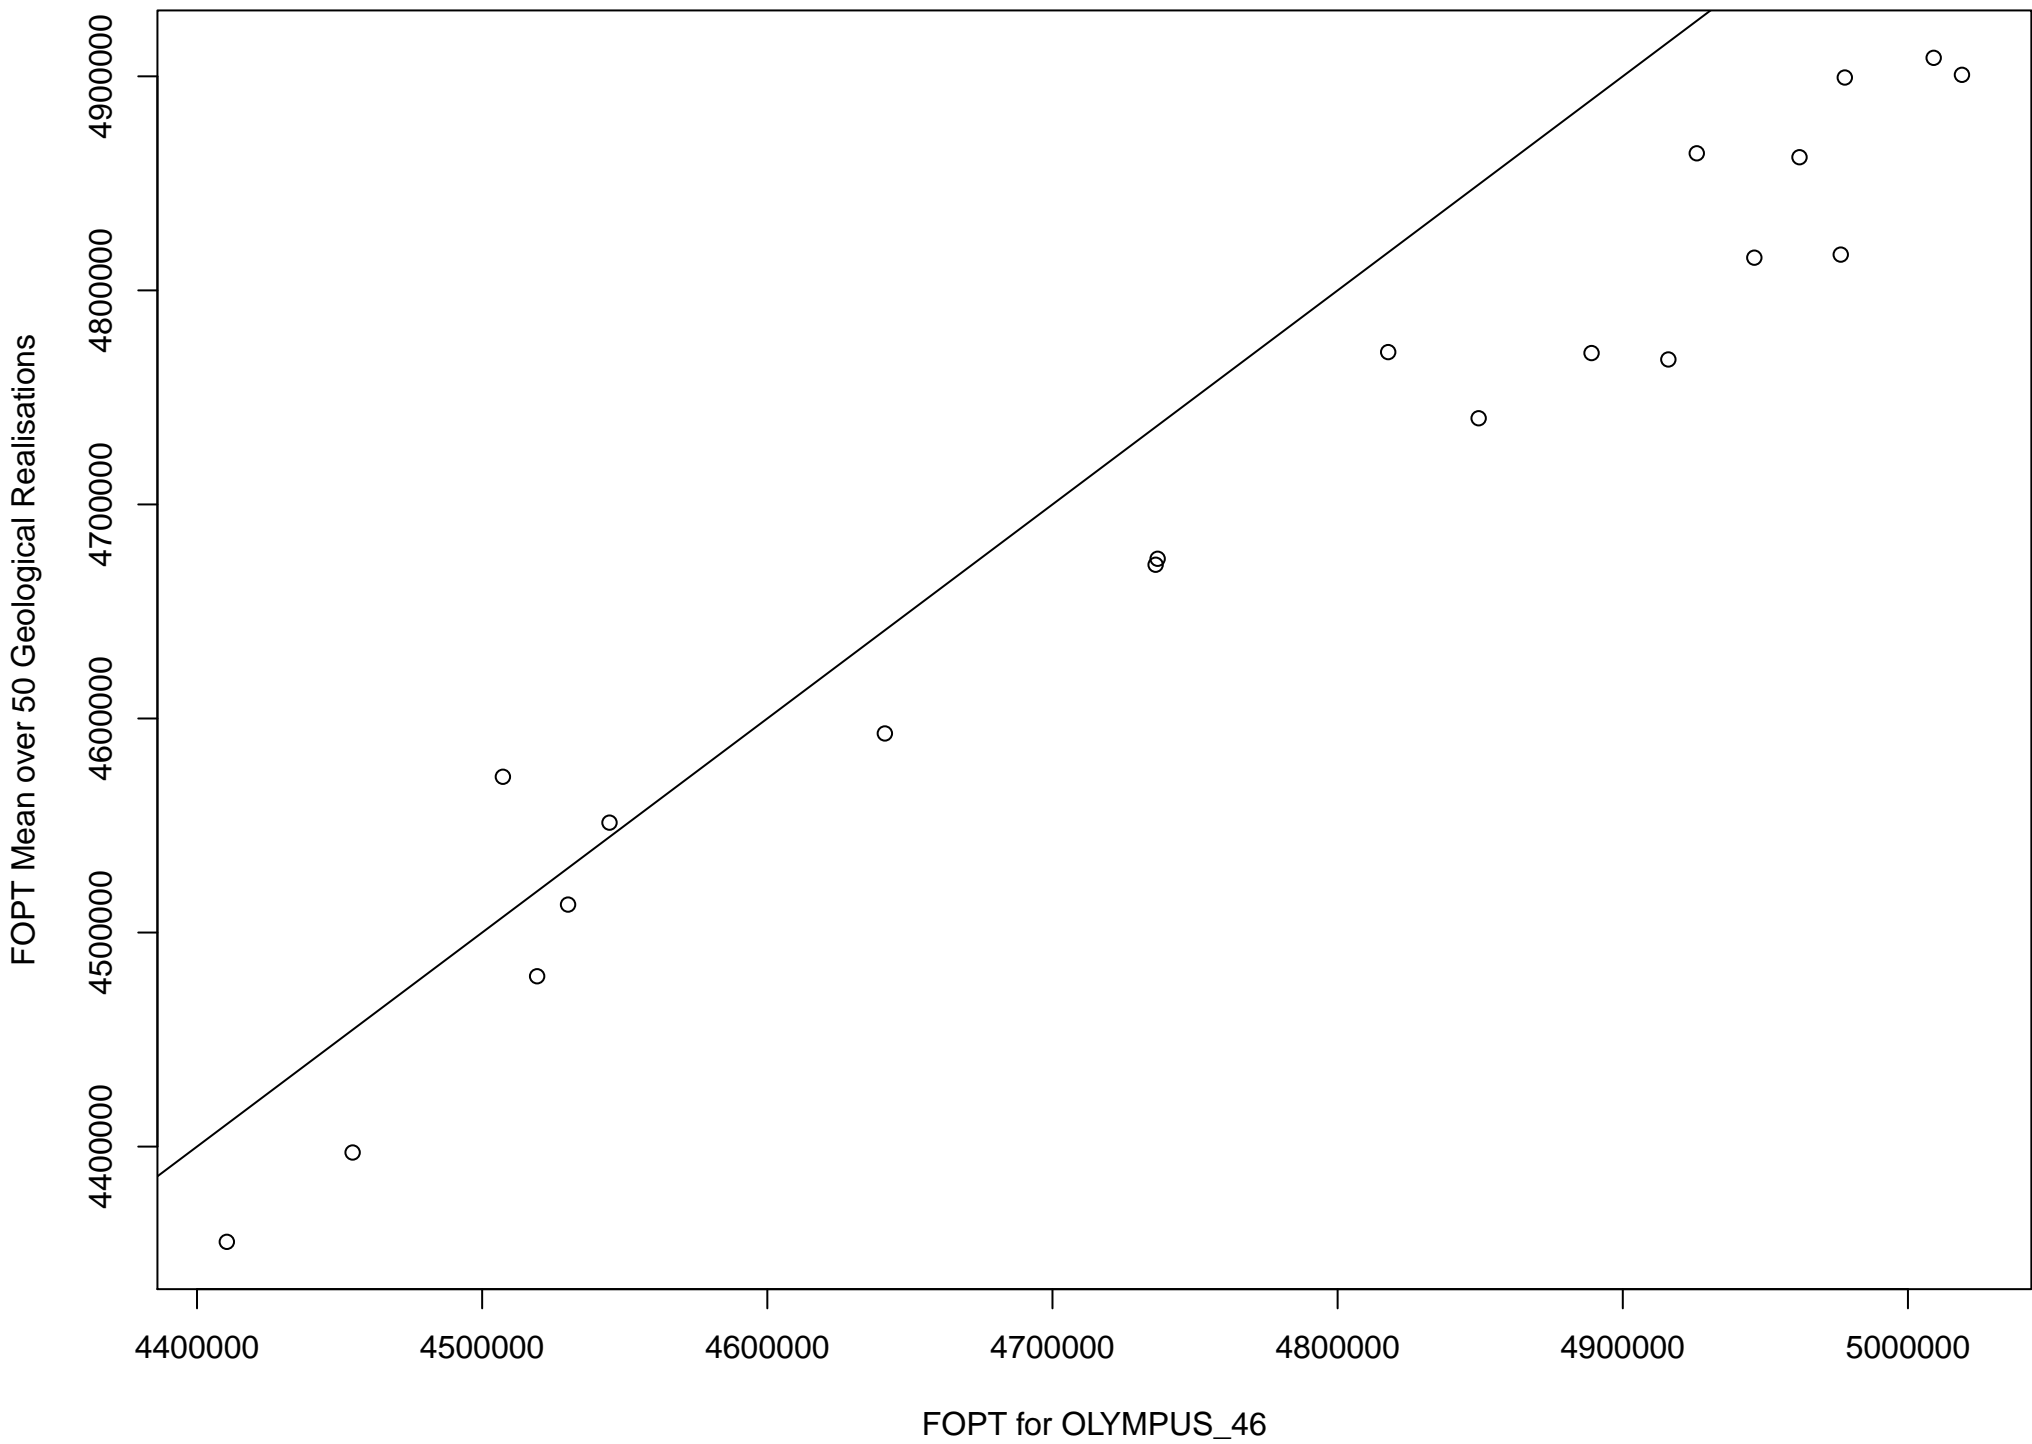

FOPT for OLYMPUS\_47

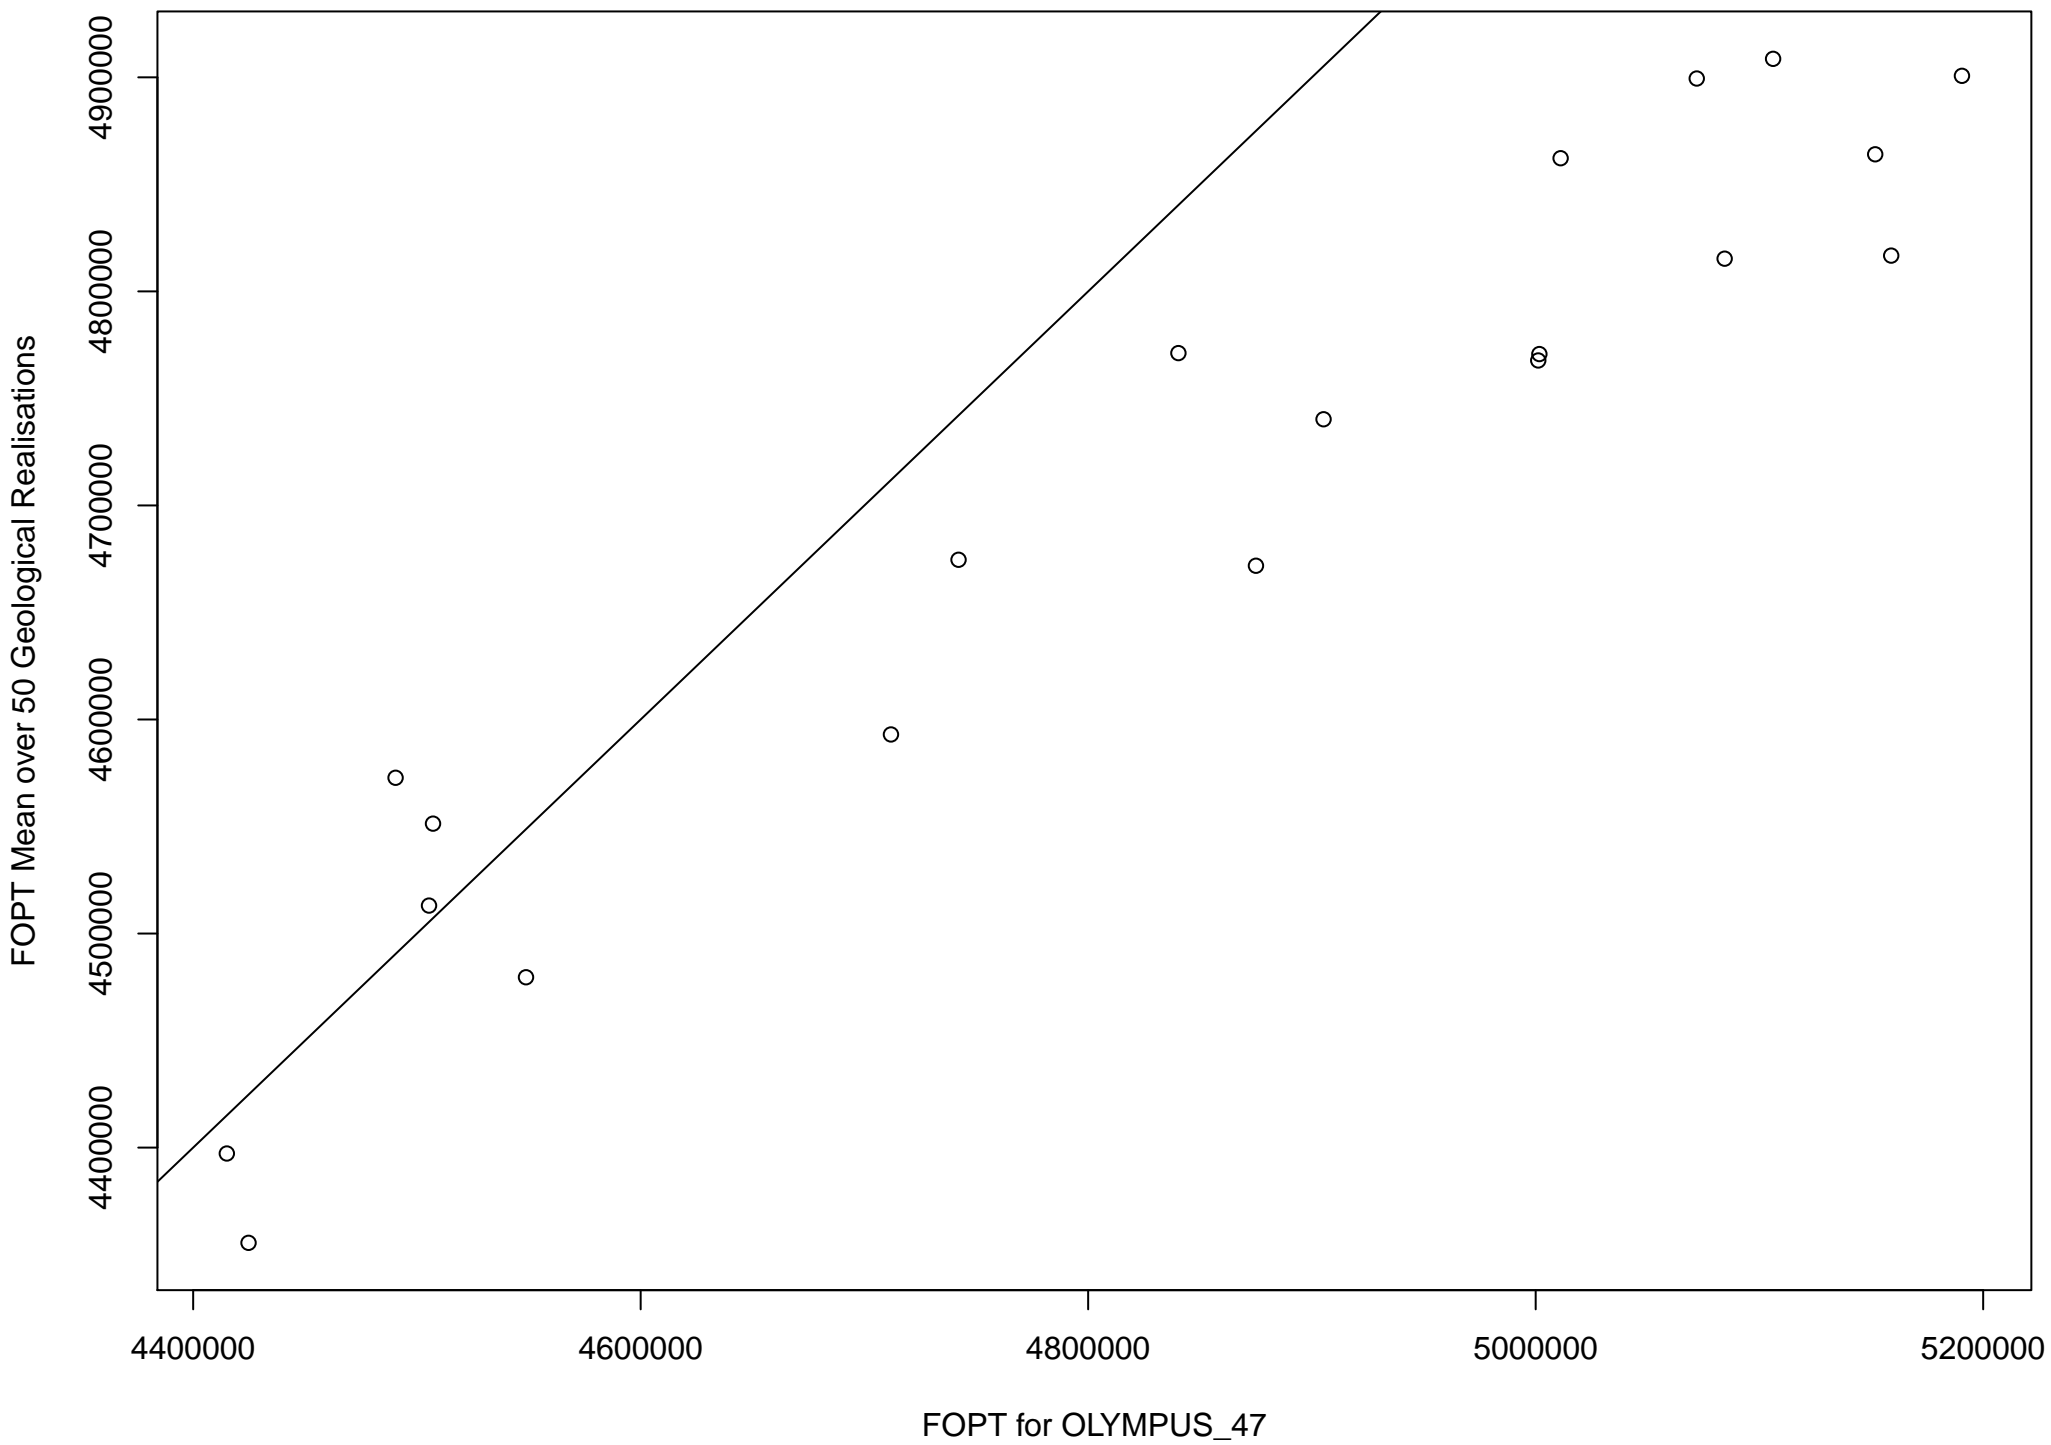

FOPT for OLYMPUS\_48

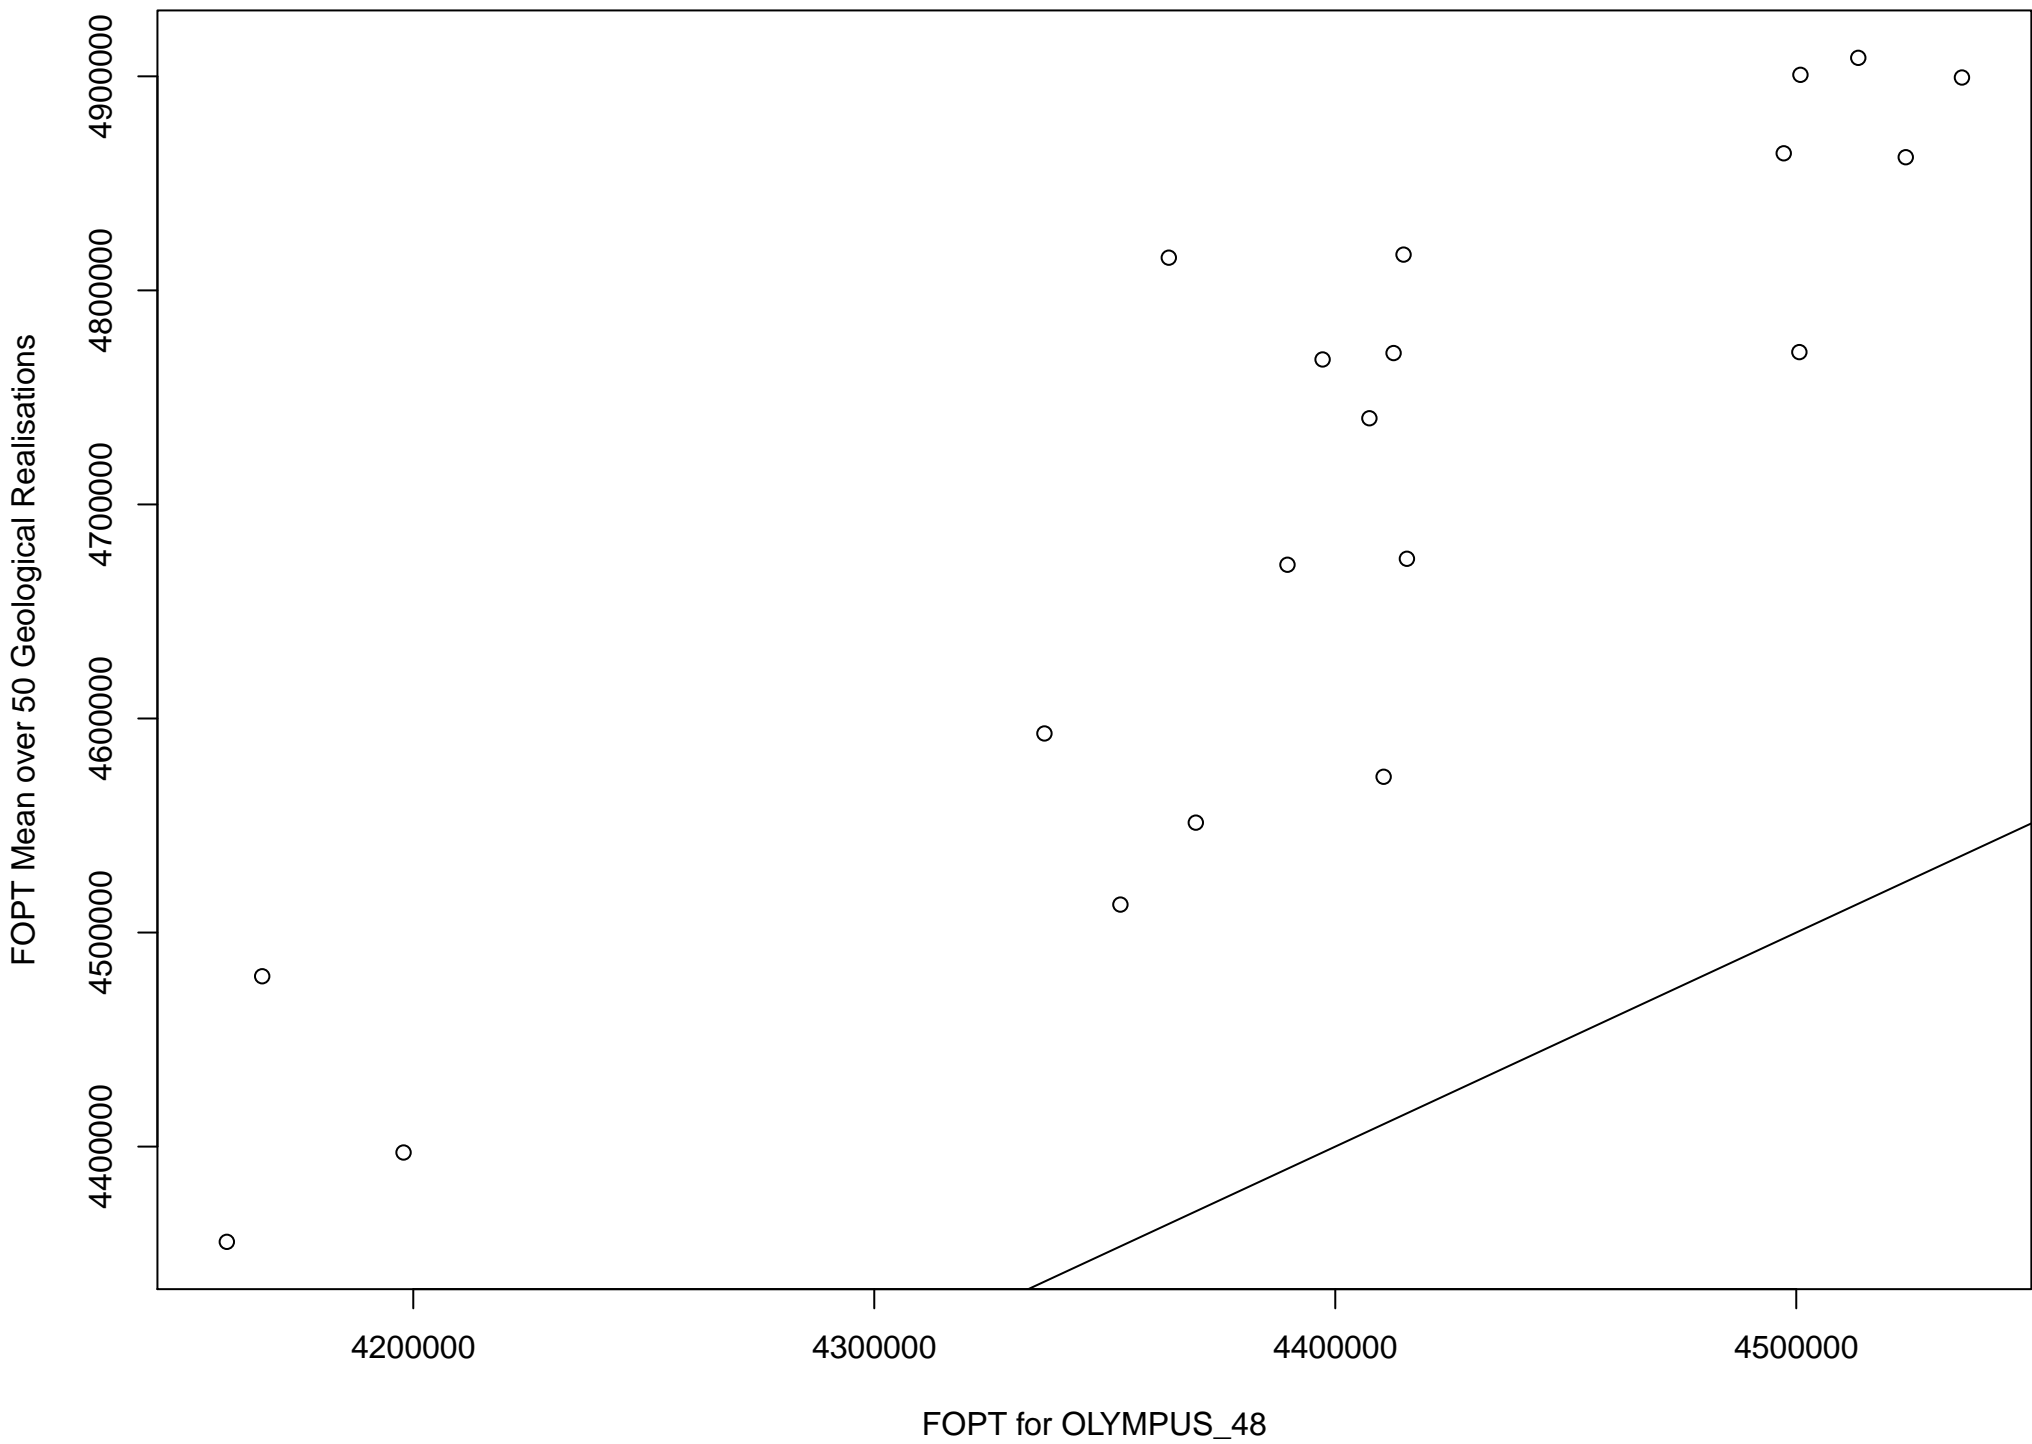



FOPT for OLYMPUS\_49

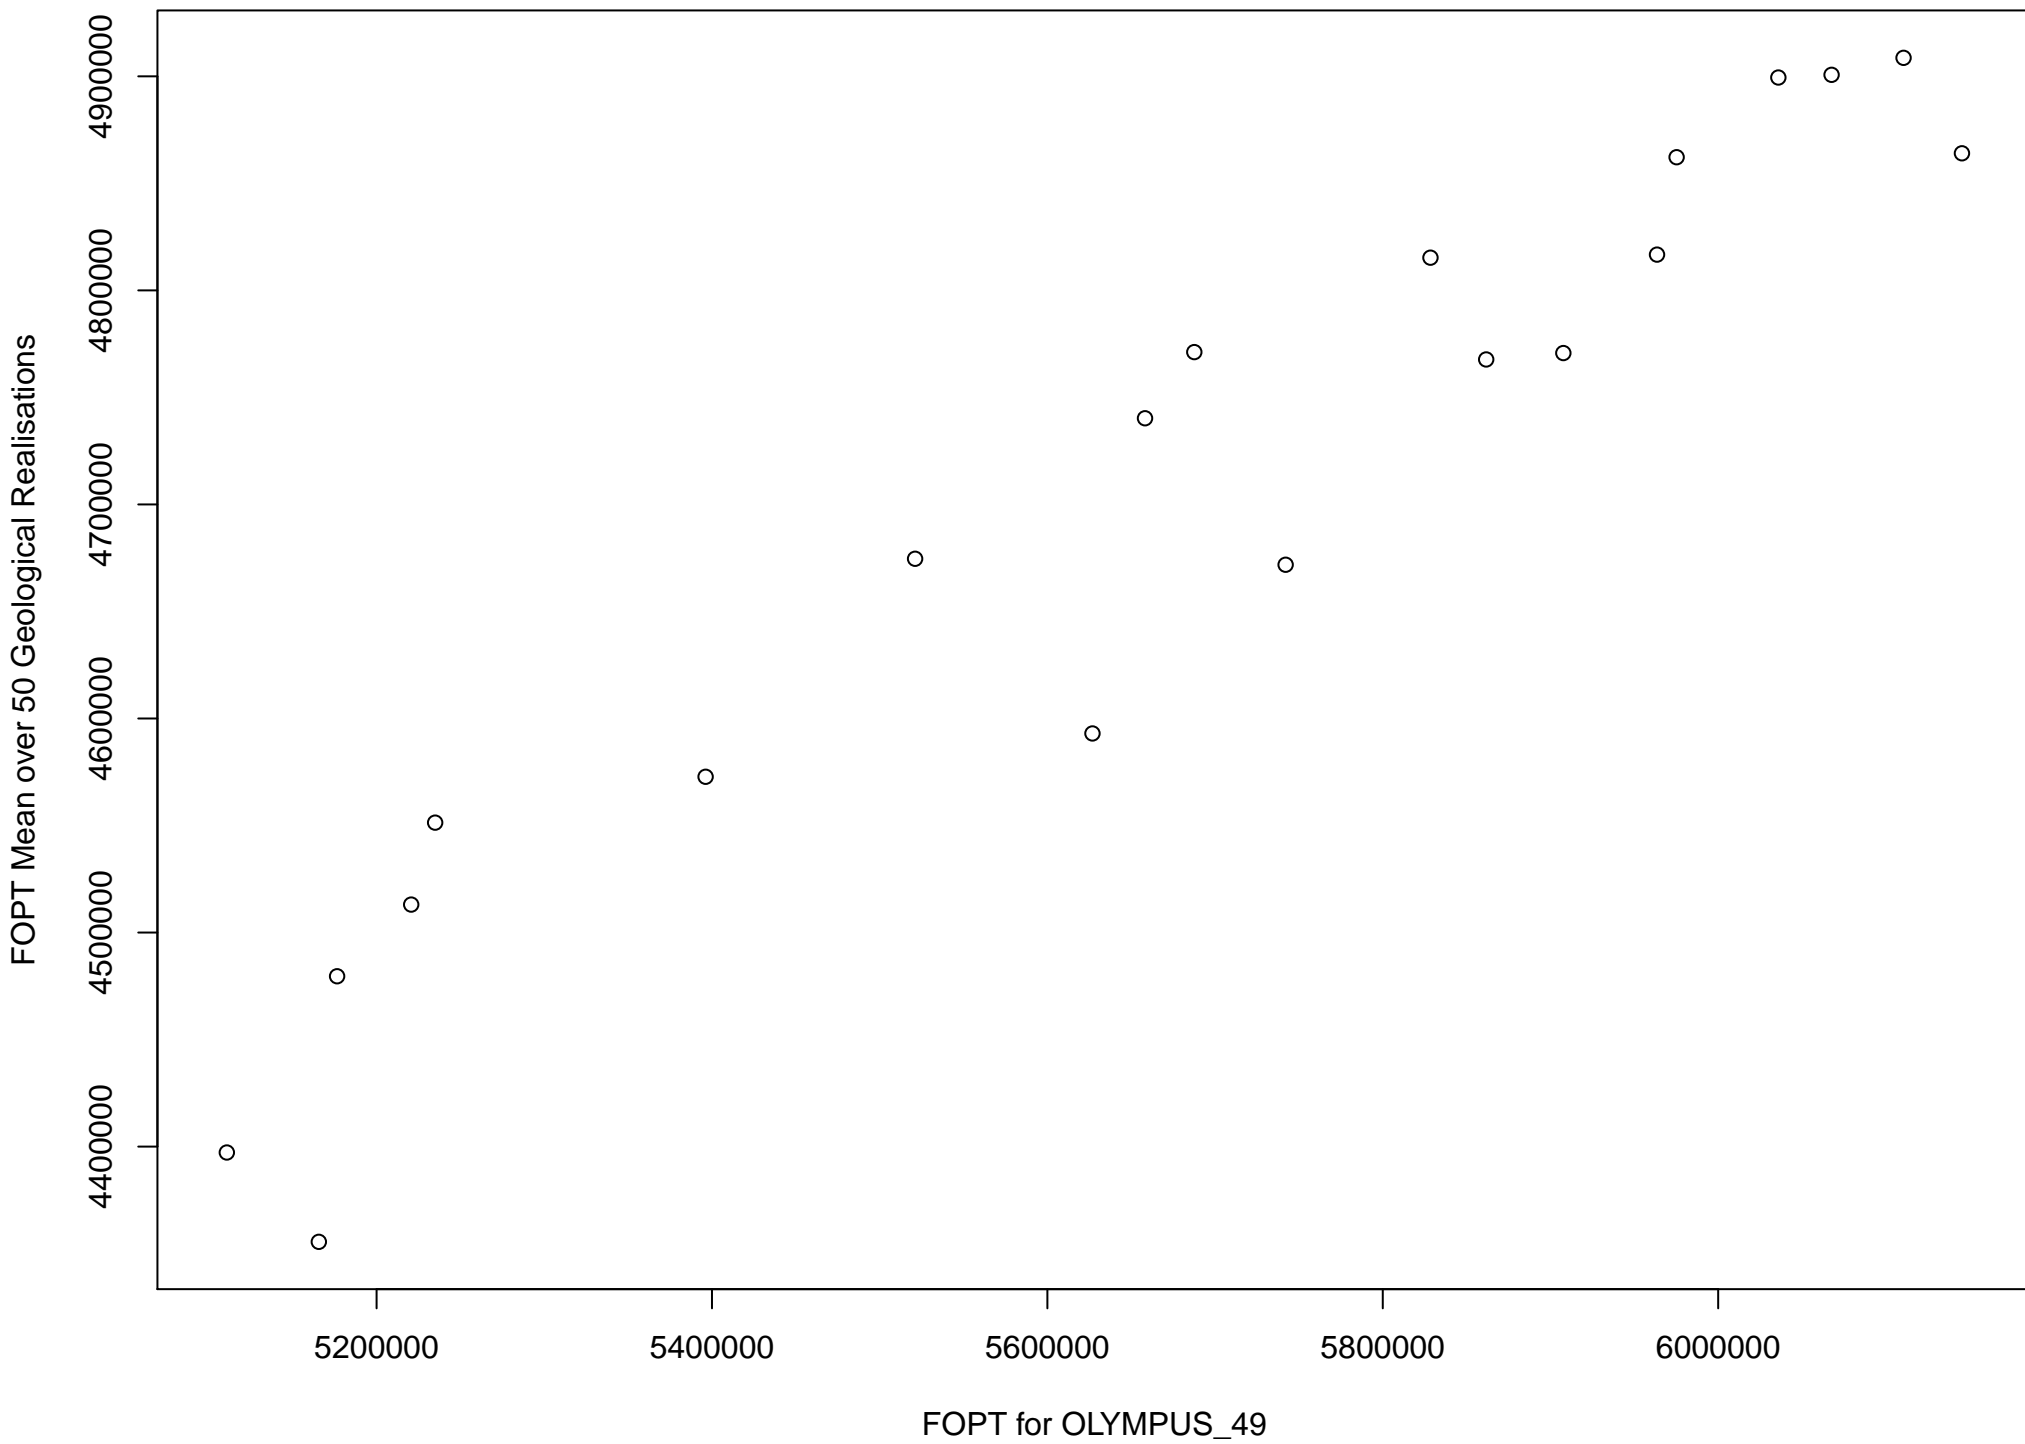

FOPT for OLYMPUS\_50

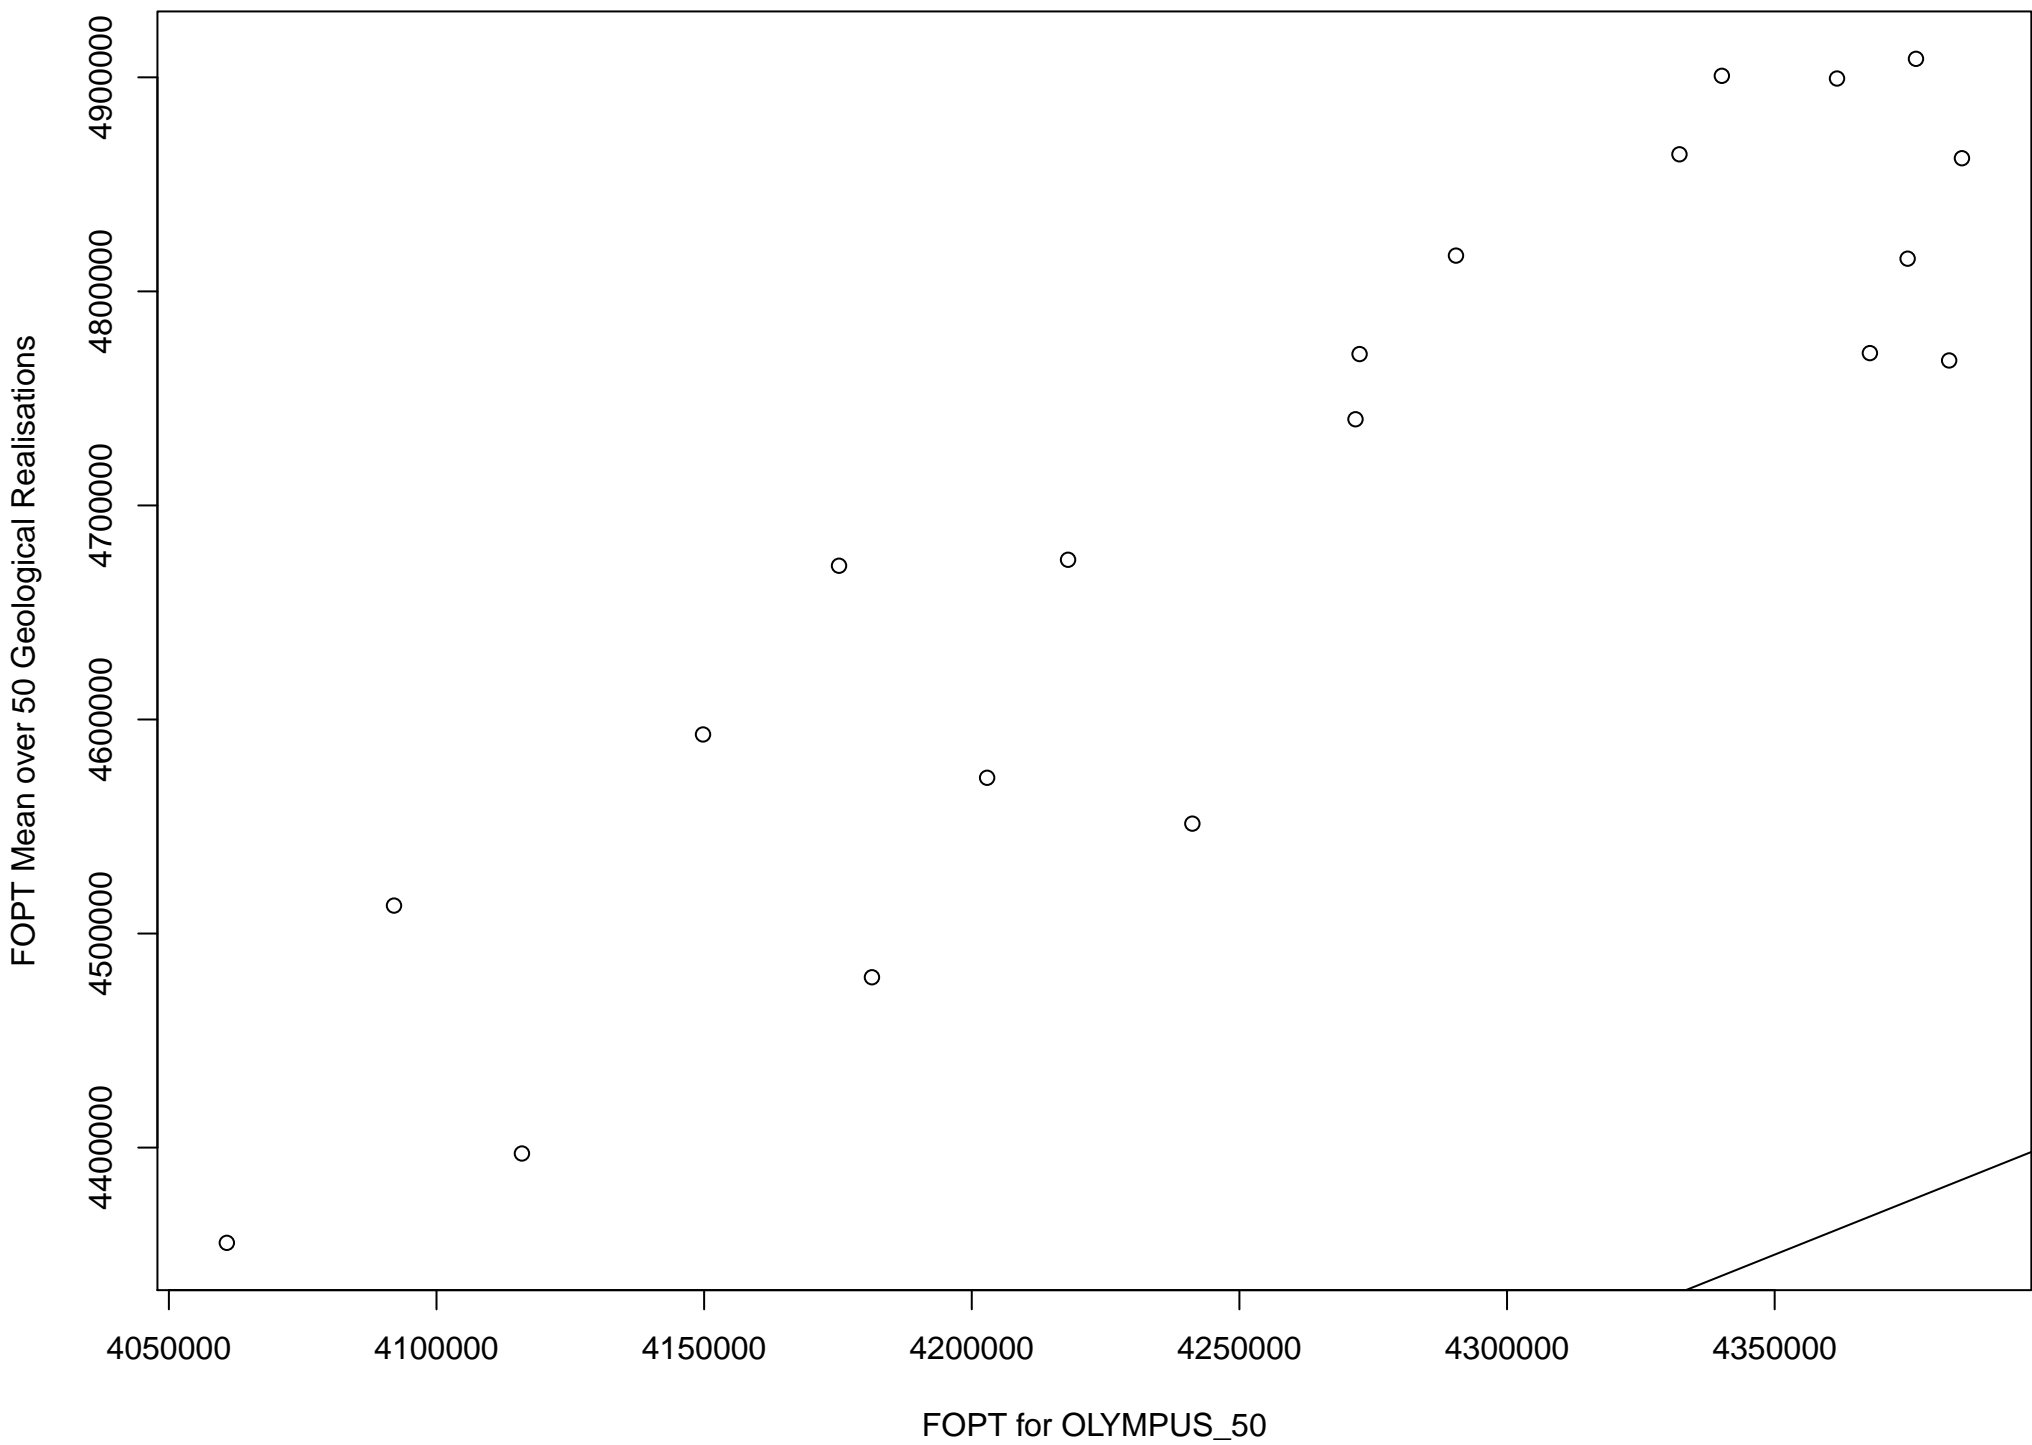

Supplement: Supplementary file 3 [file FOPT-Mean-vs-Model-Output-all-Models.pdf]
