# Supplementary material for: Bayesian Emulation of Grey-Box Multi-Model Ensembles Exploiting Known Interior Structure
Source: arXiv:2406.08367 source file (2025-05-02)

FWIT for OLYMPUS\_1

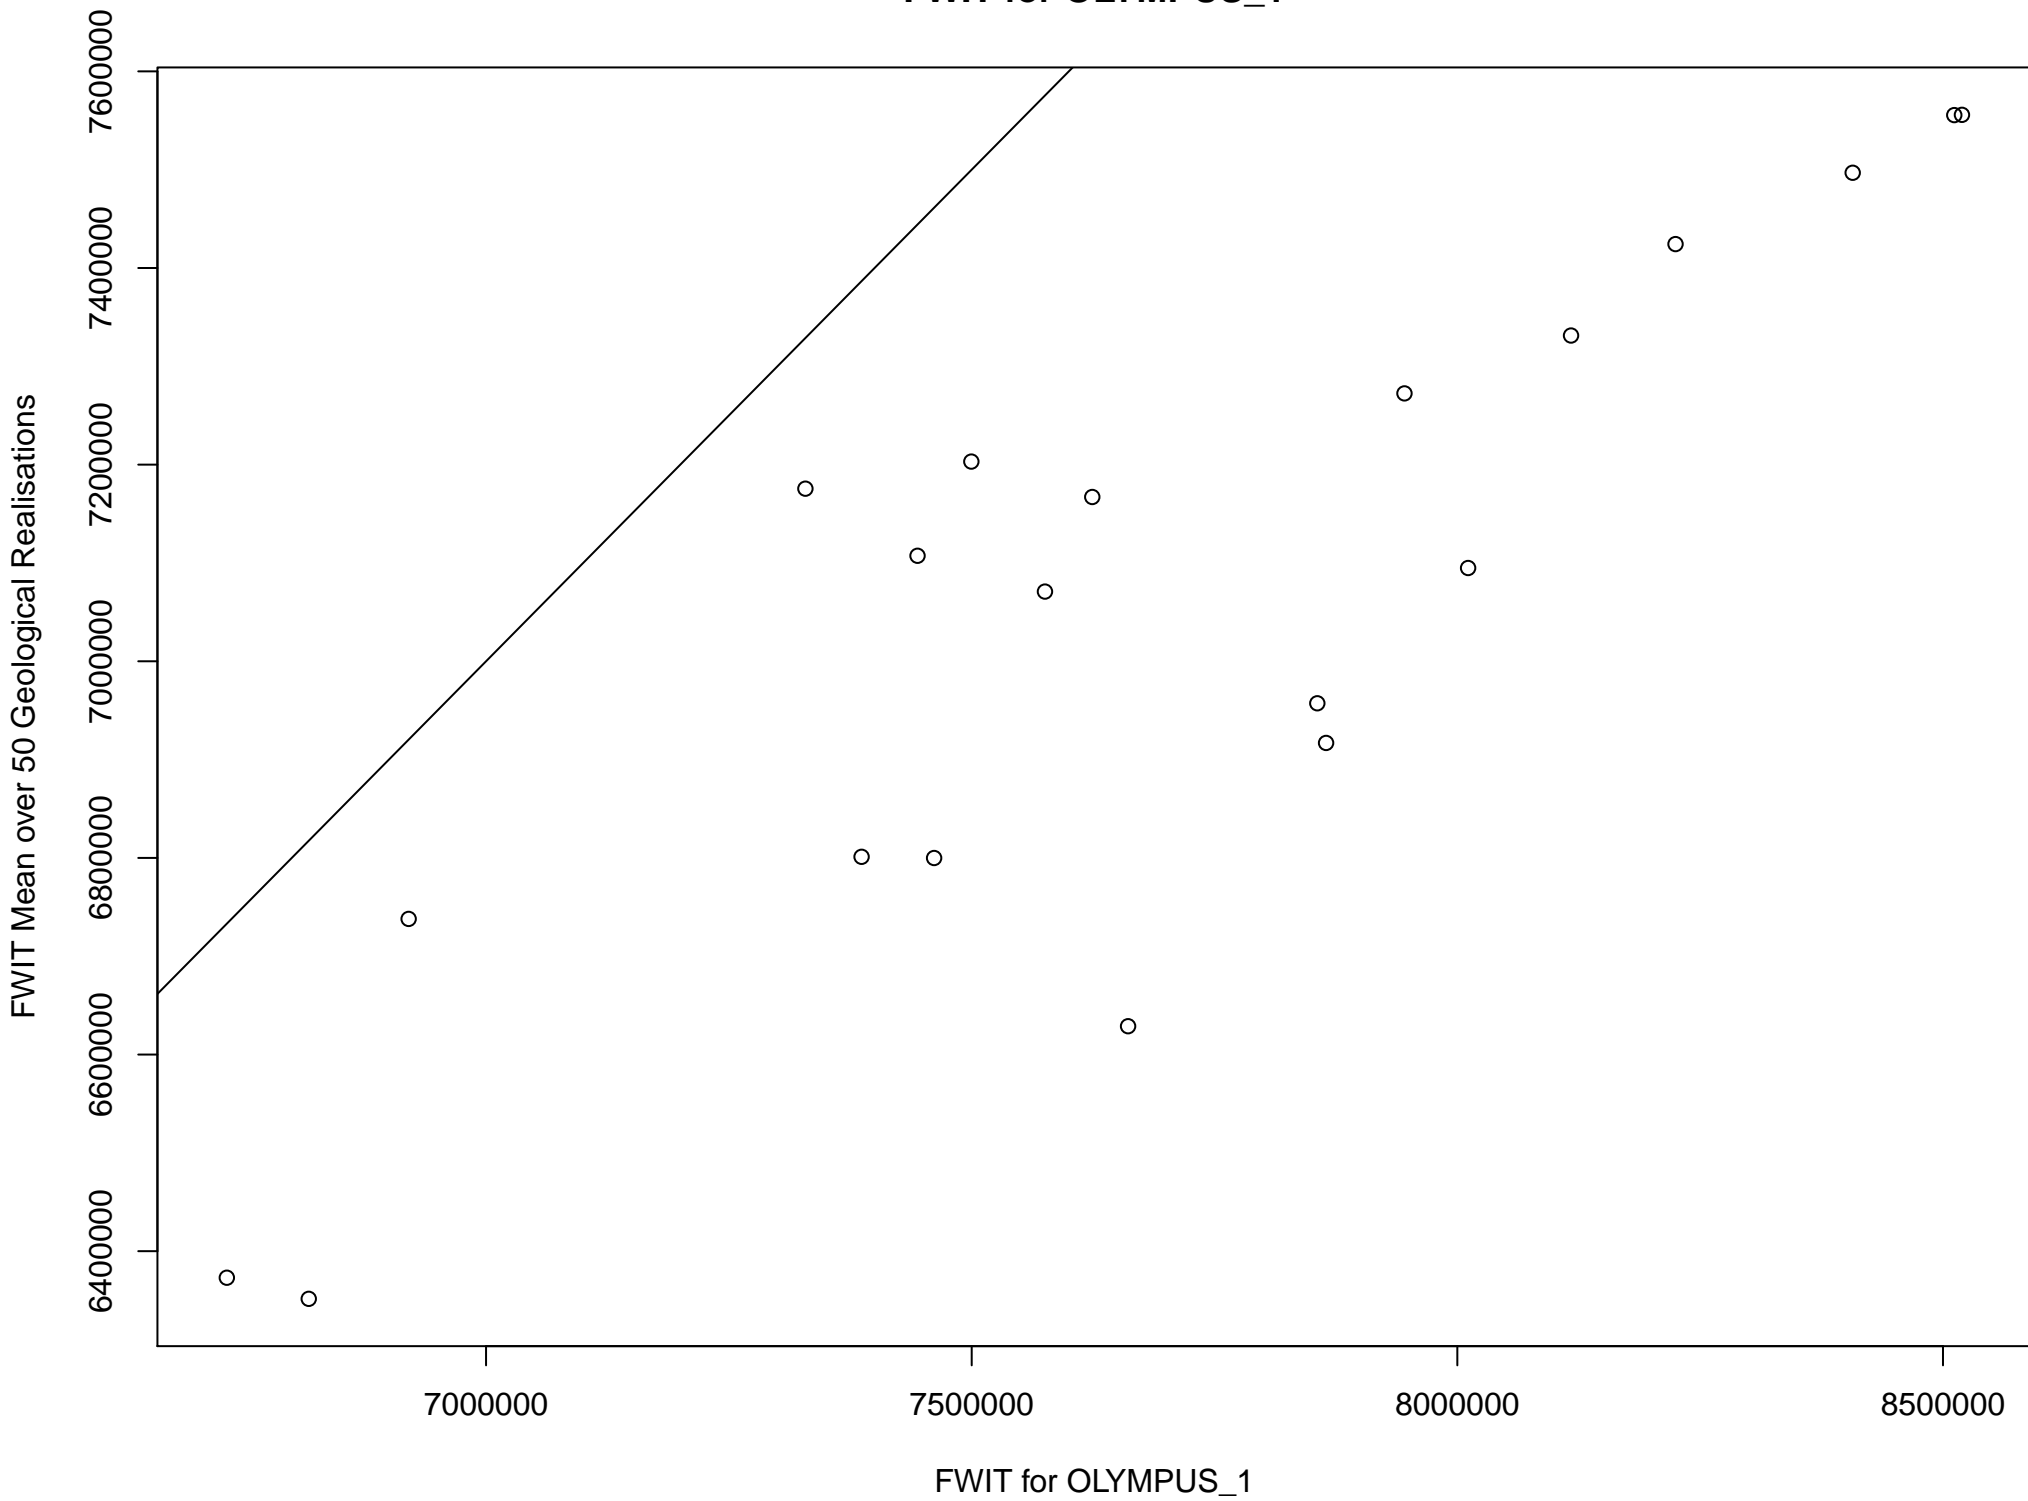

FWIT for OLYMPUS\_2

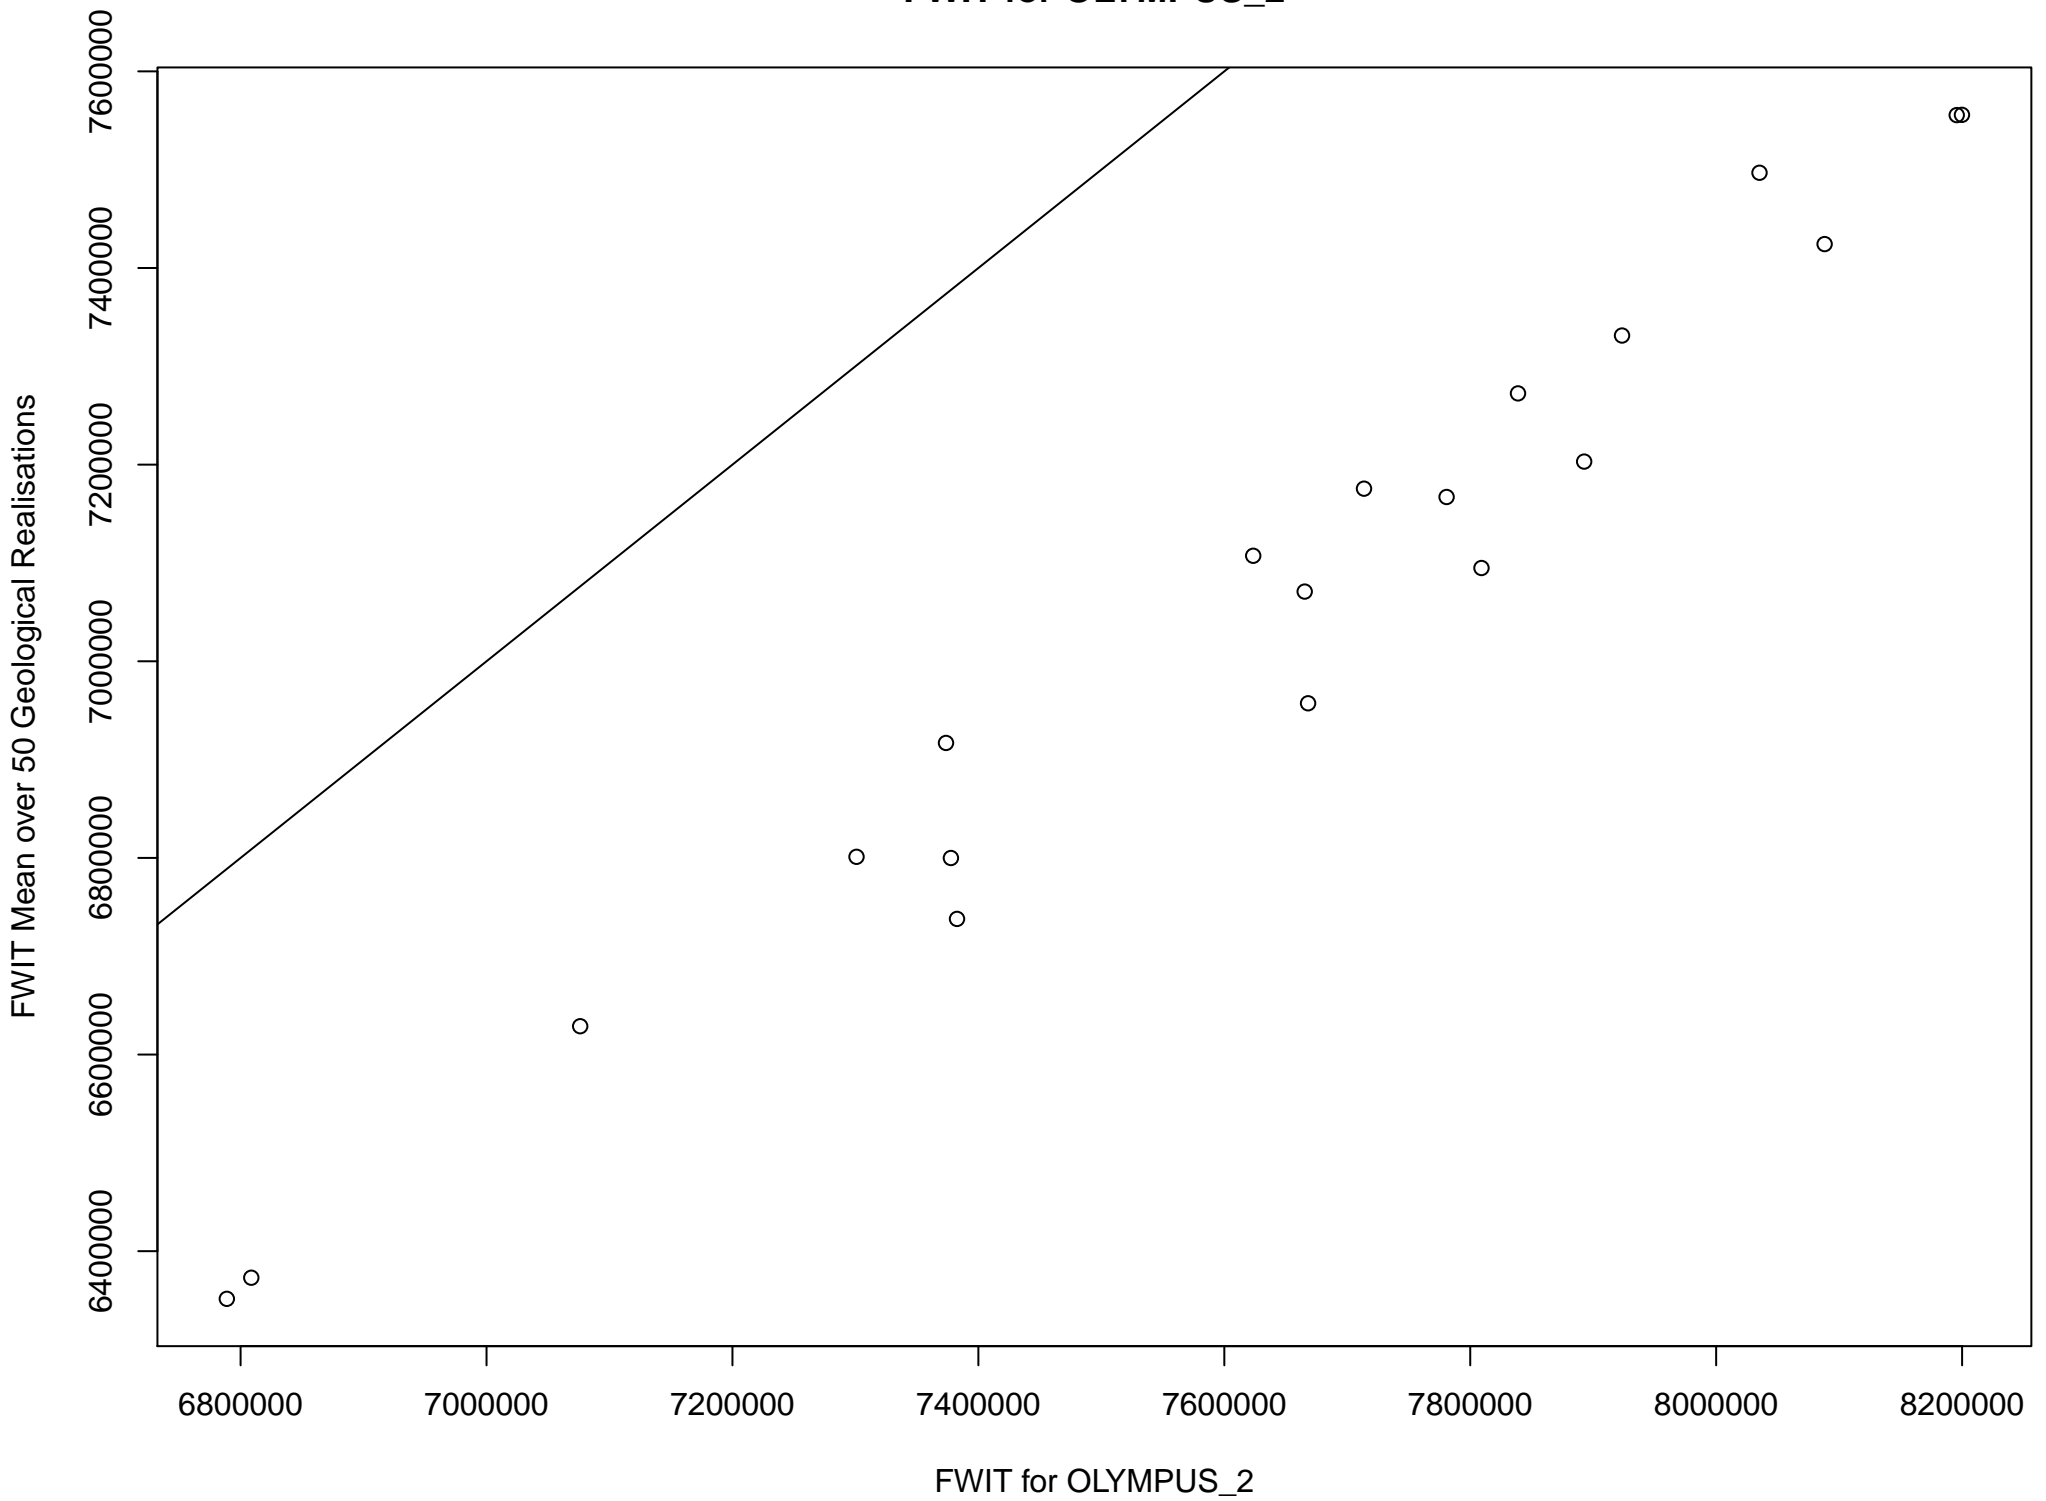

FWIT for OLYMPUS\_3

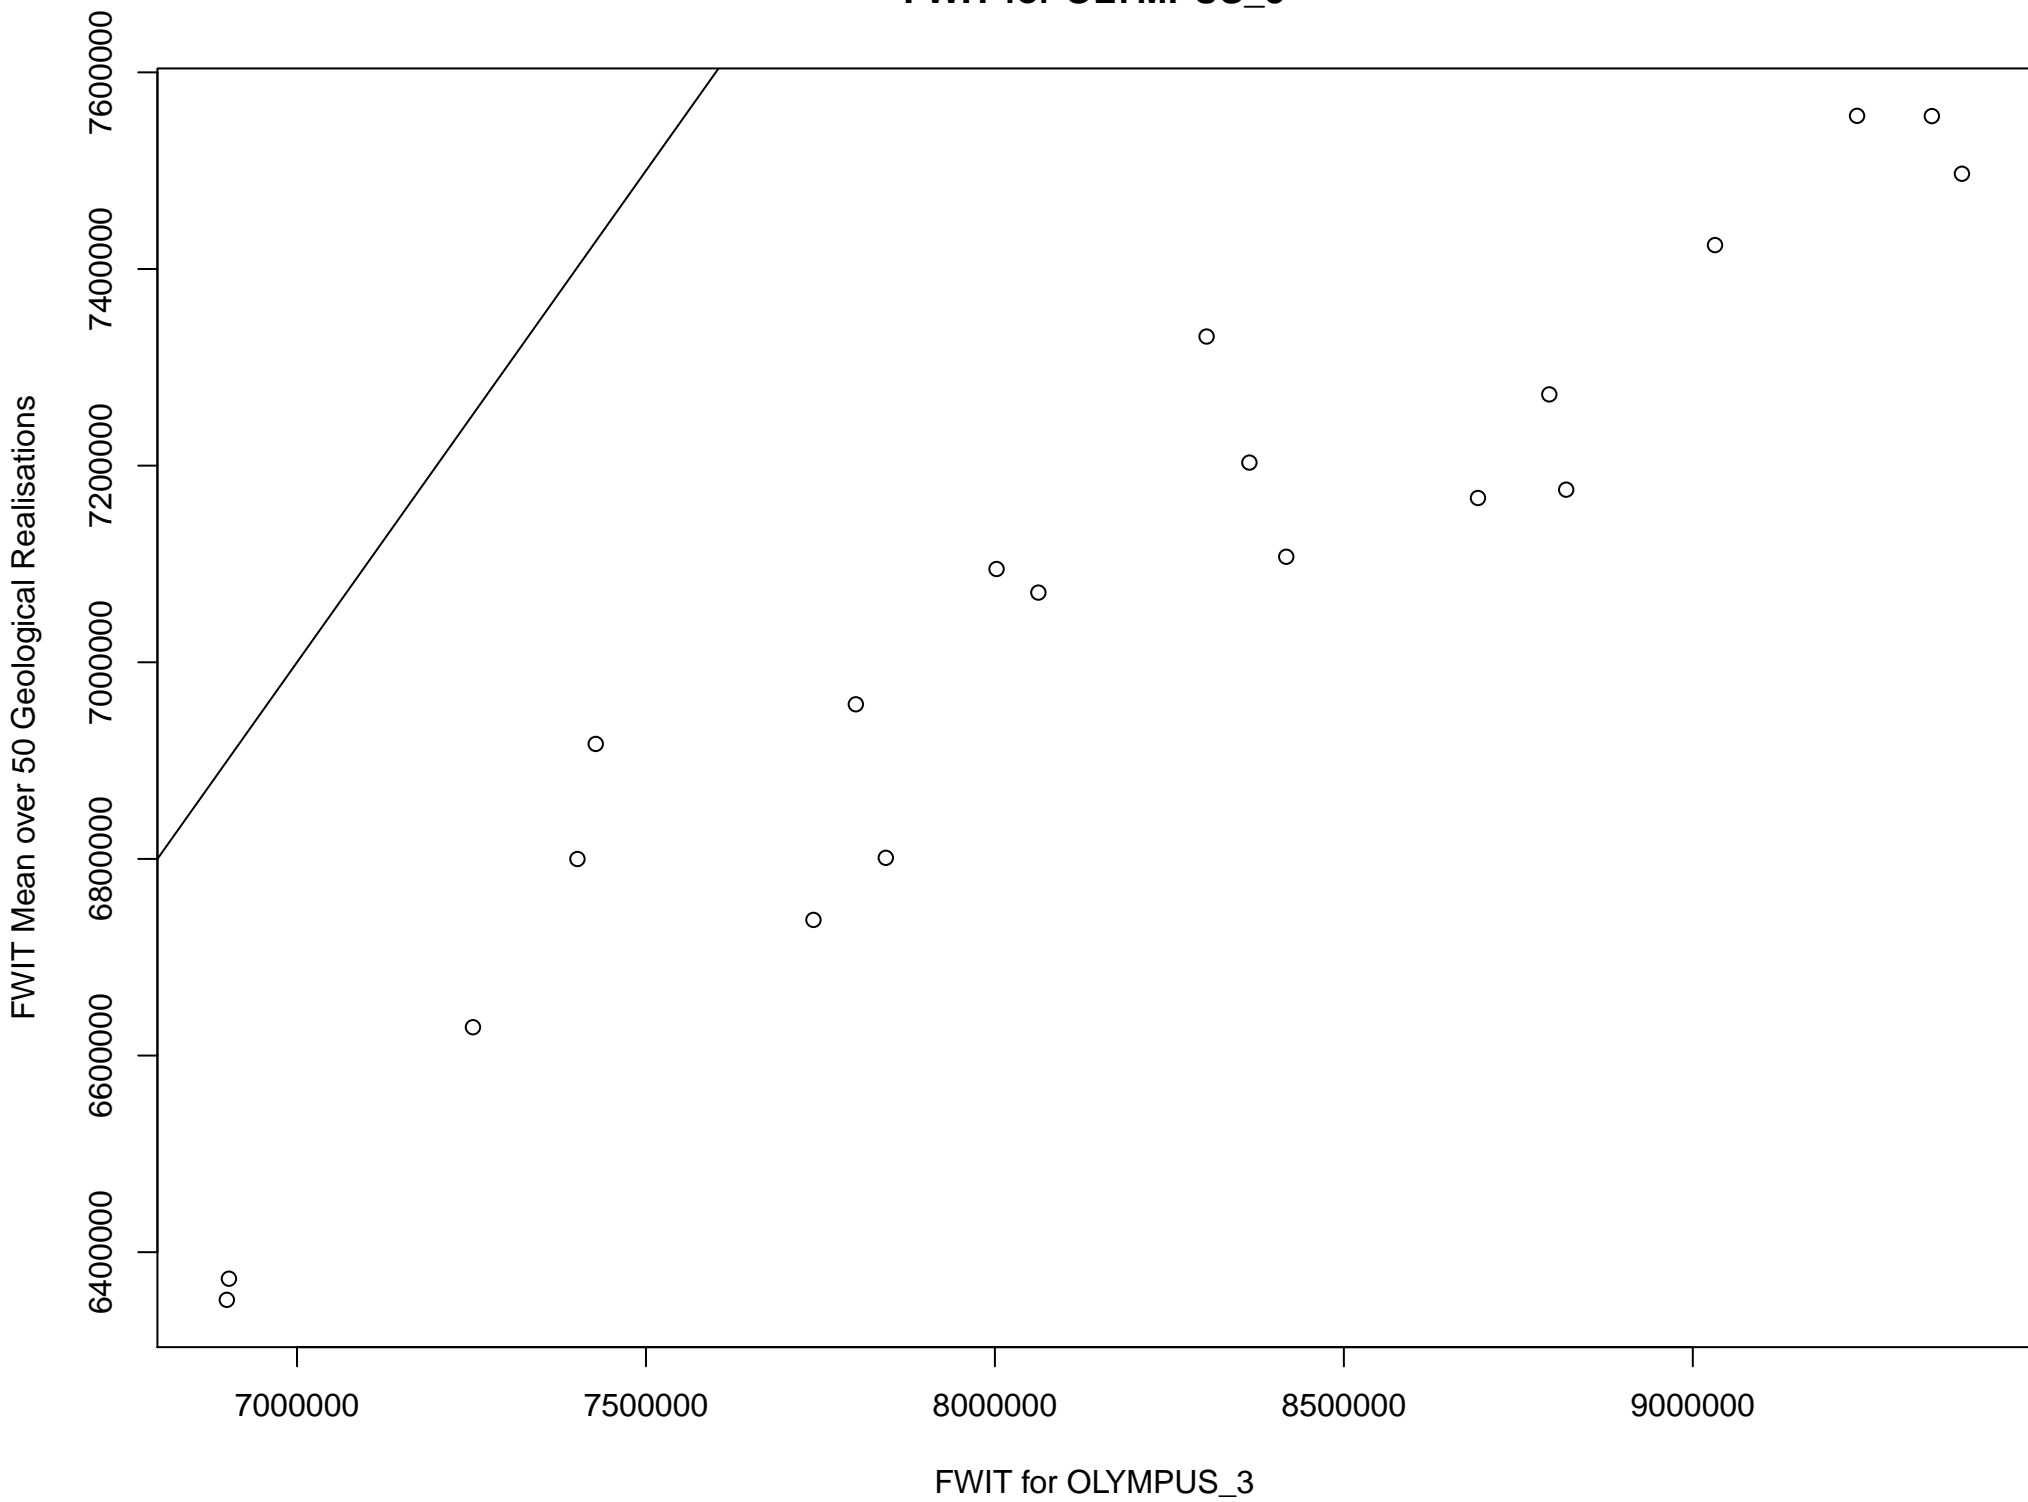

FWIT for OLYMPUS\_4

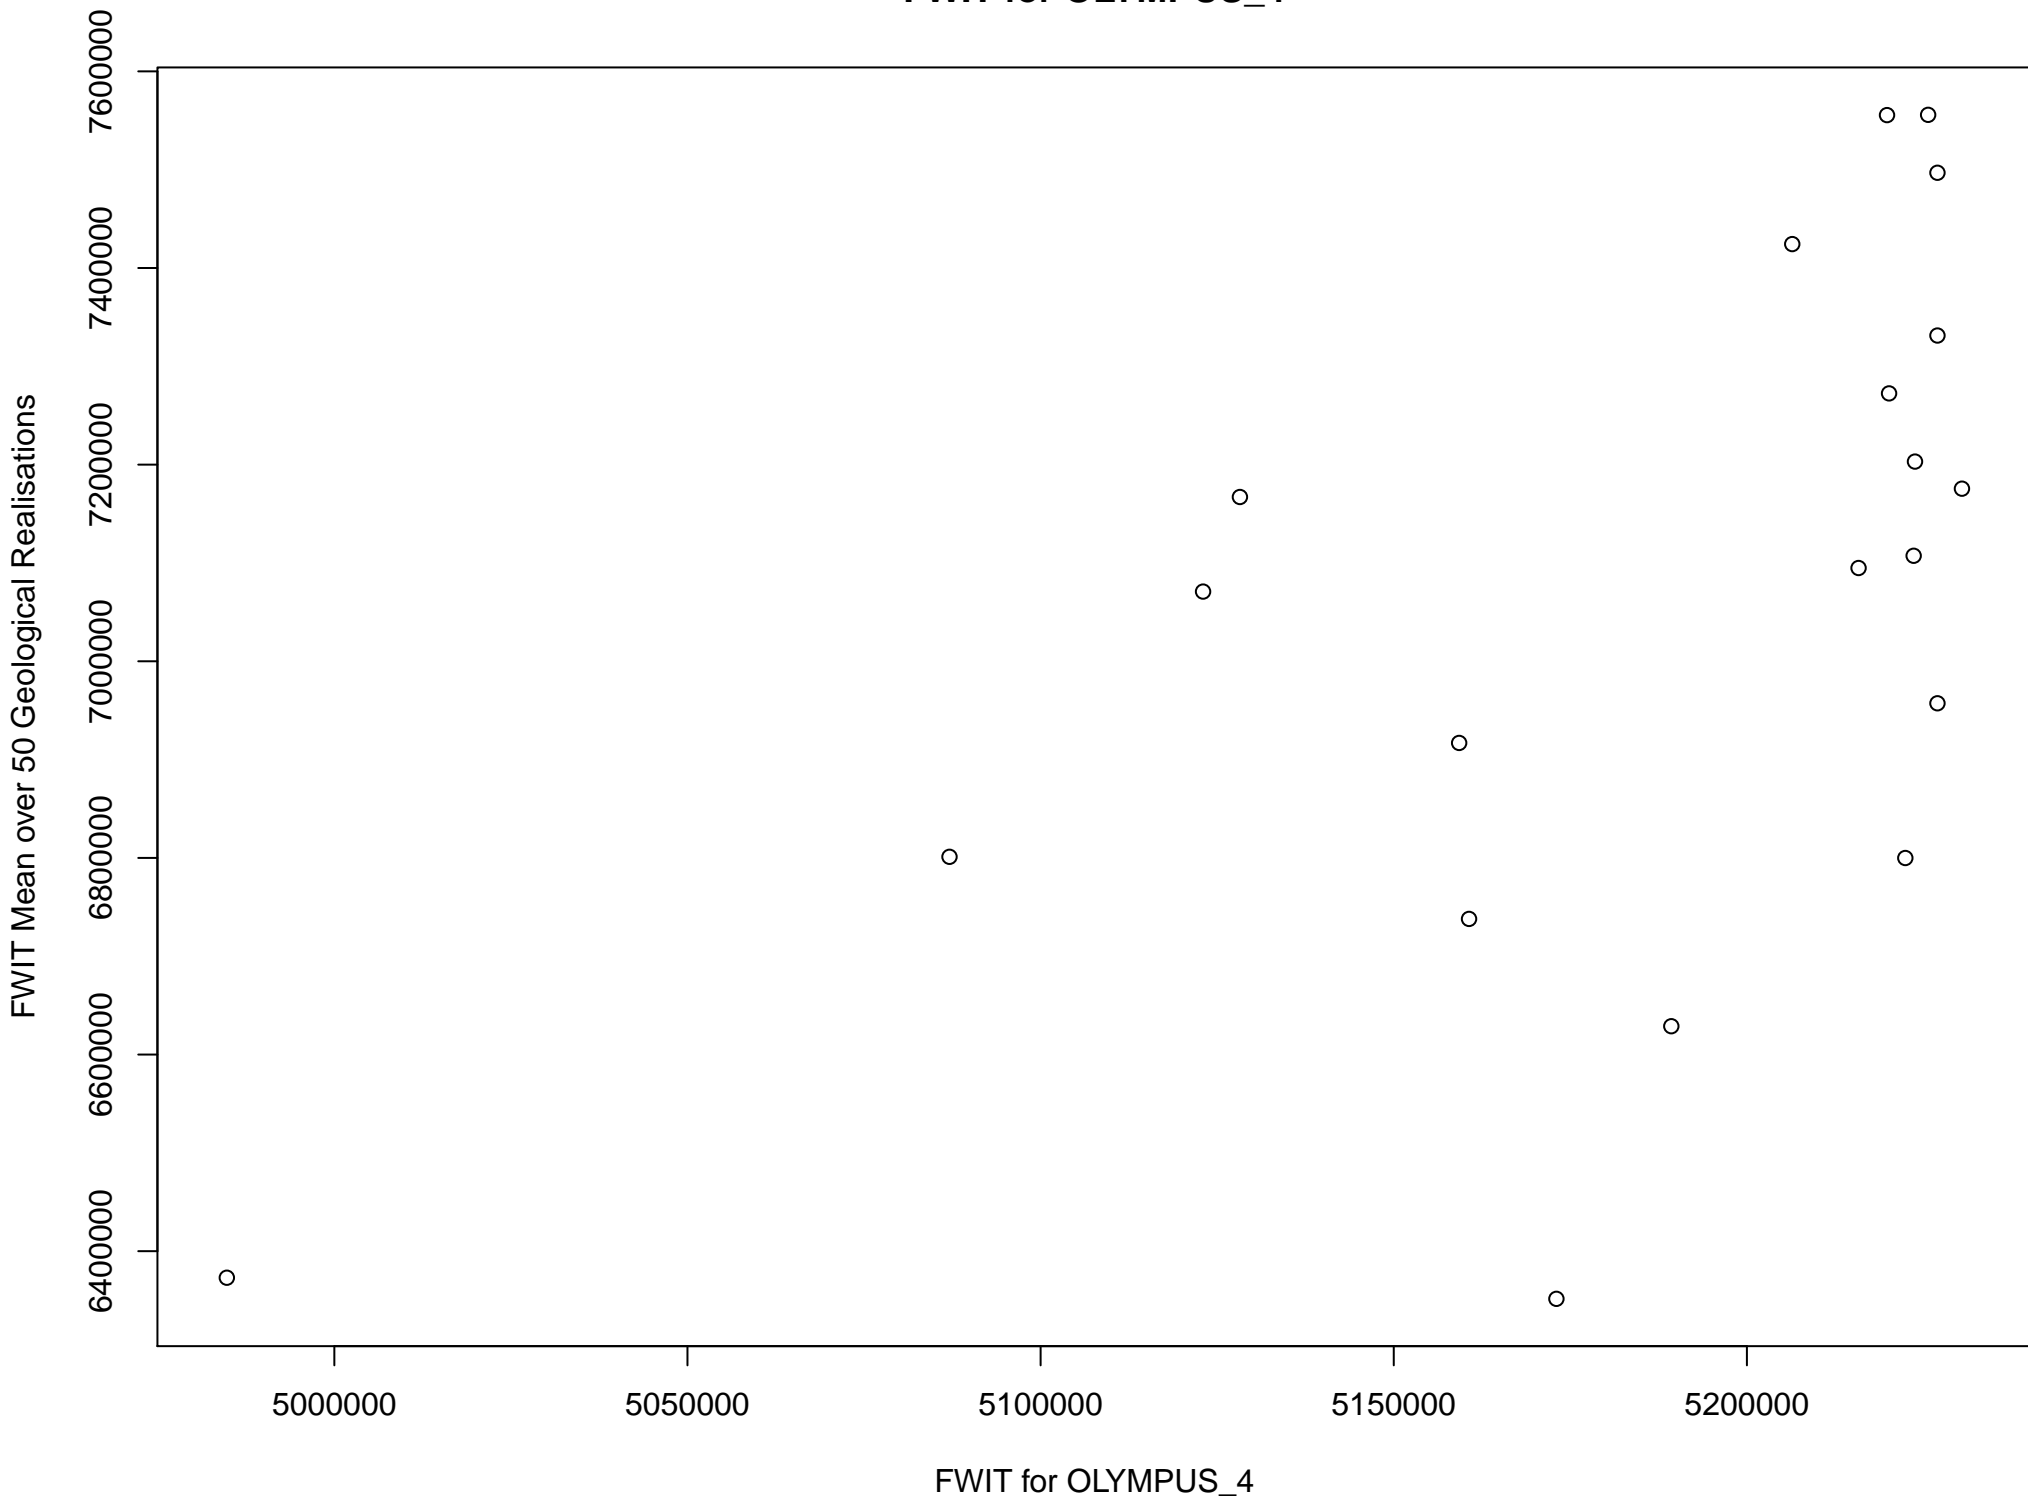

FWIT for OLYMPUS\_5

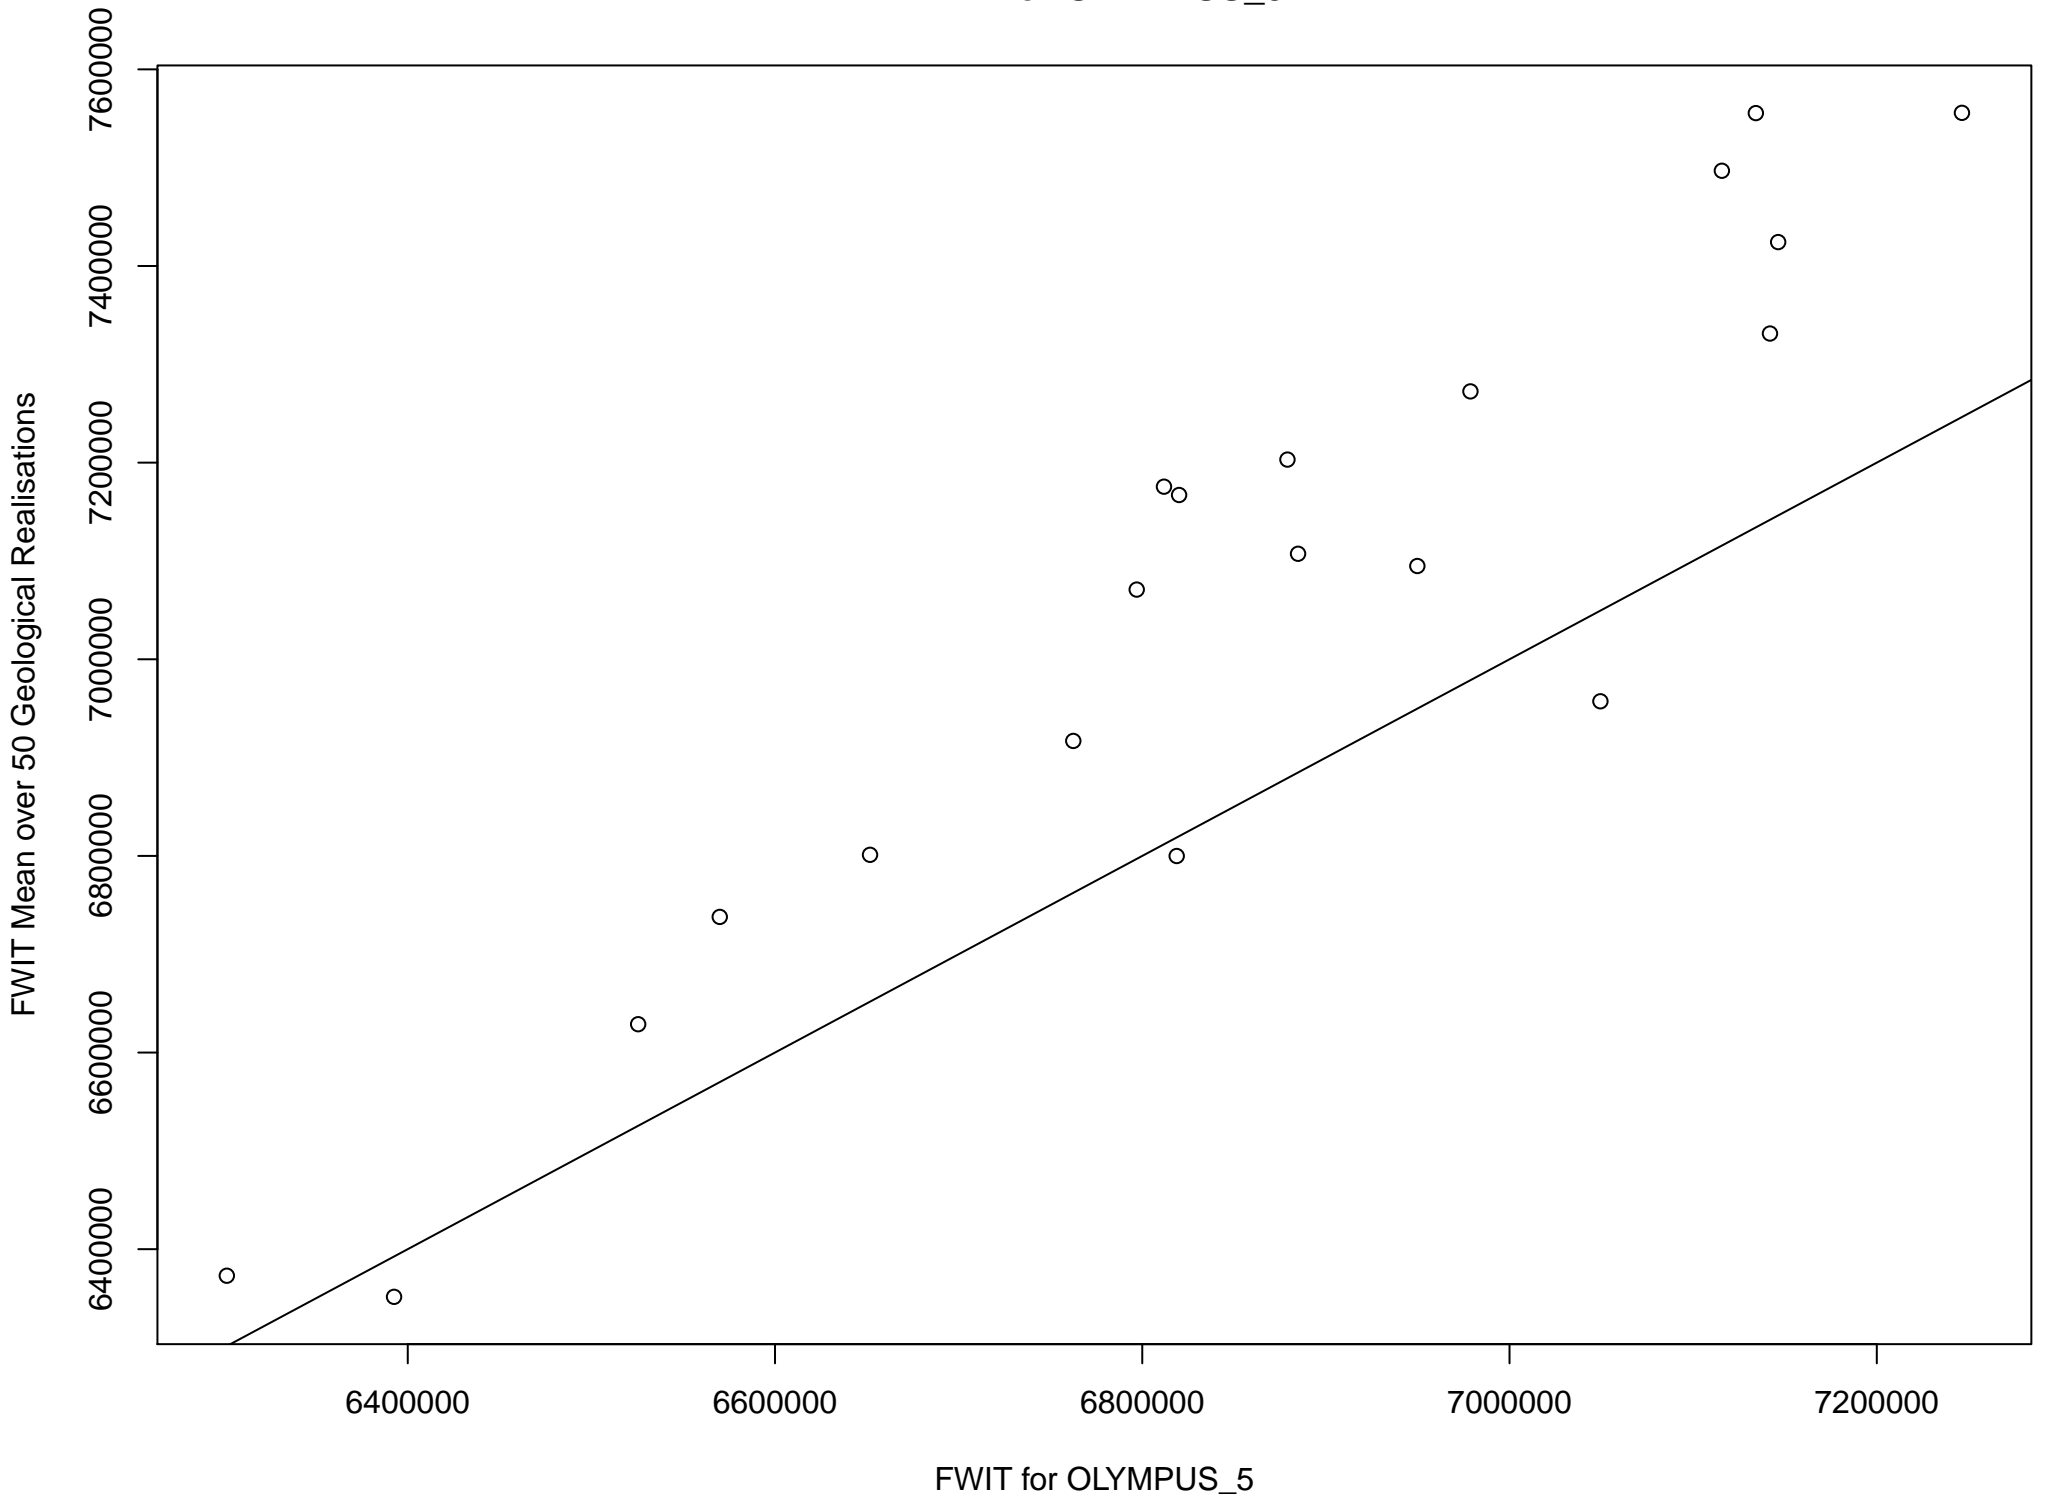

FWIT for OLYMPUS\_6

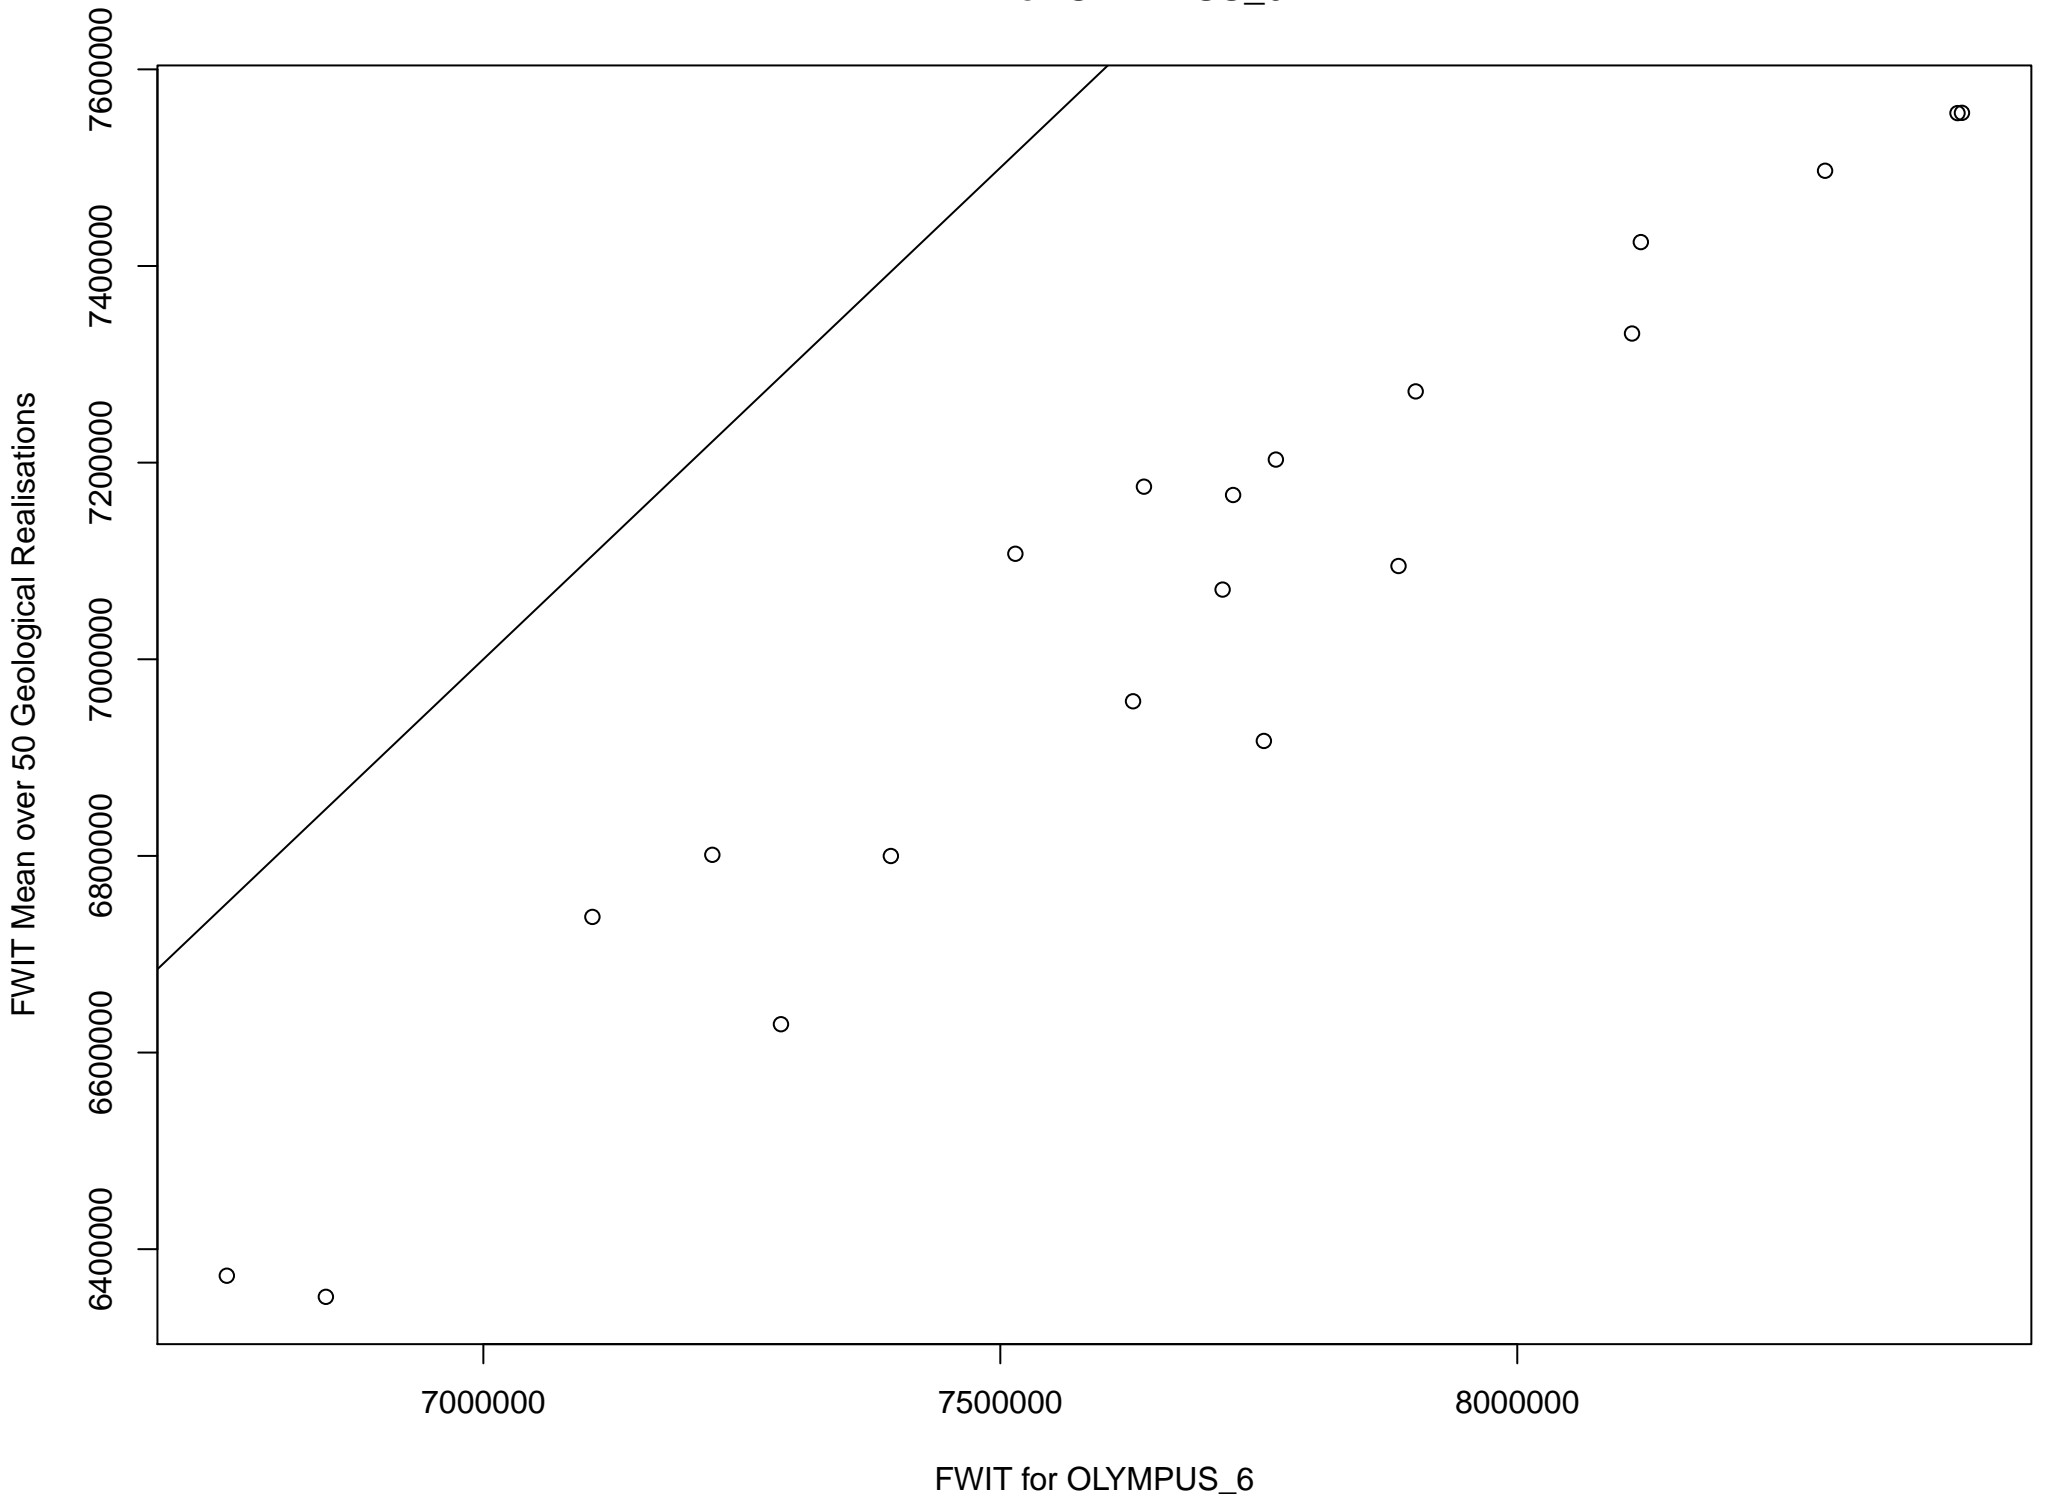

FWIT for OLYMPUS\_7

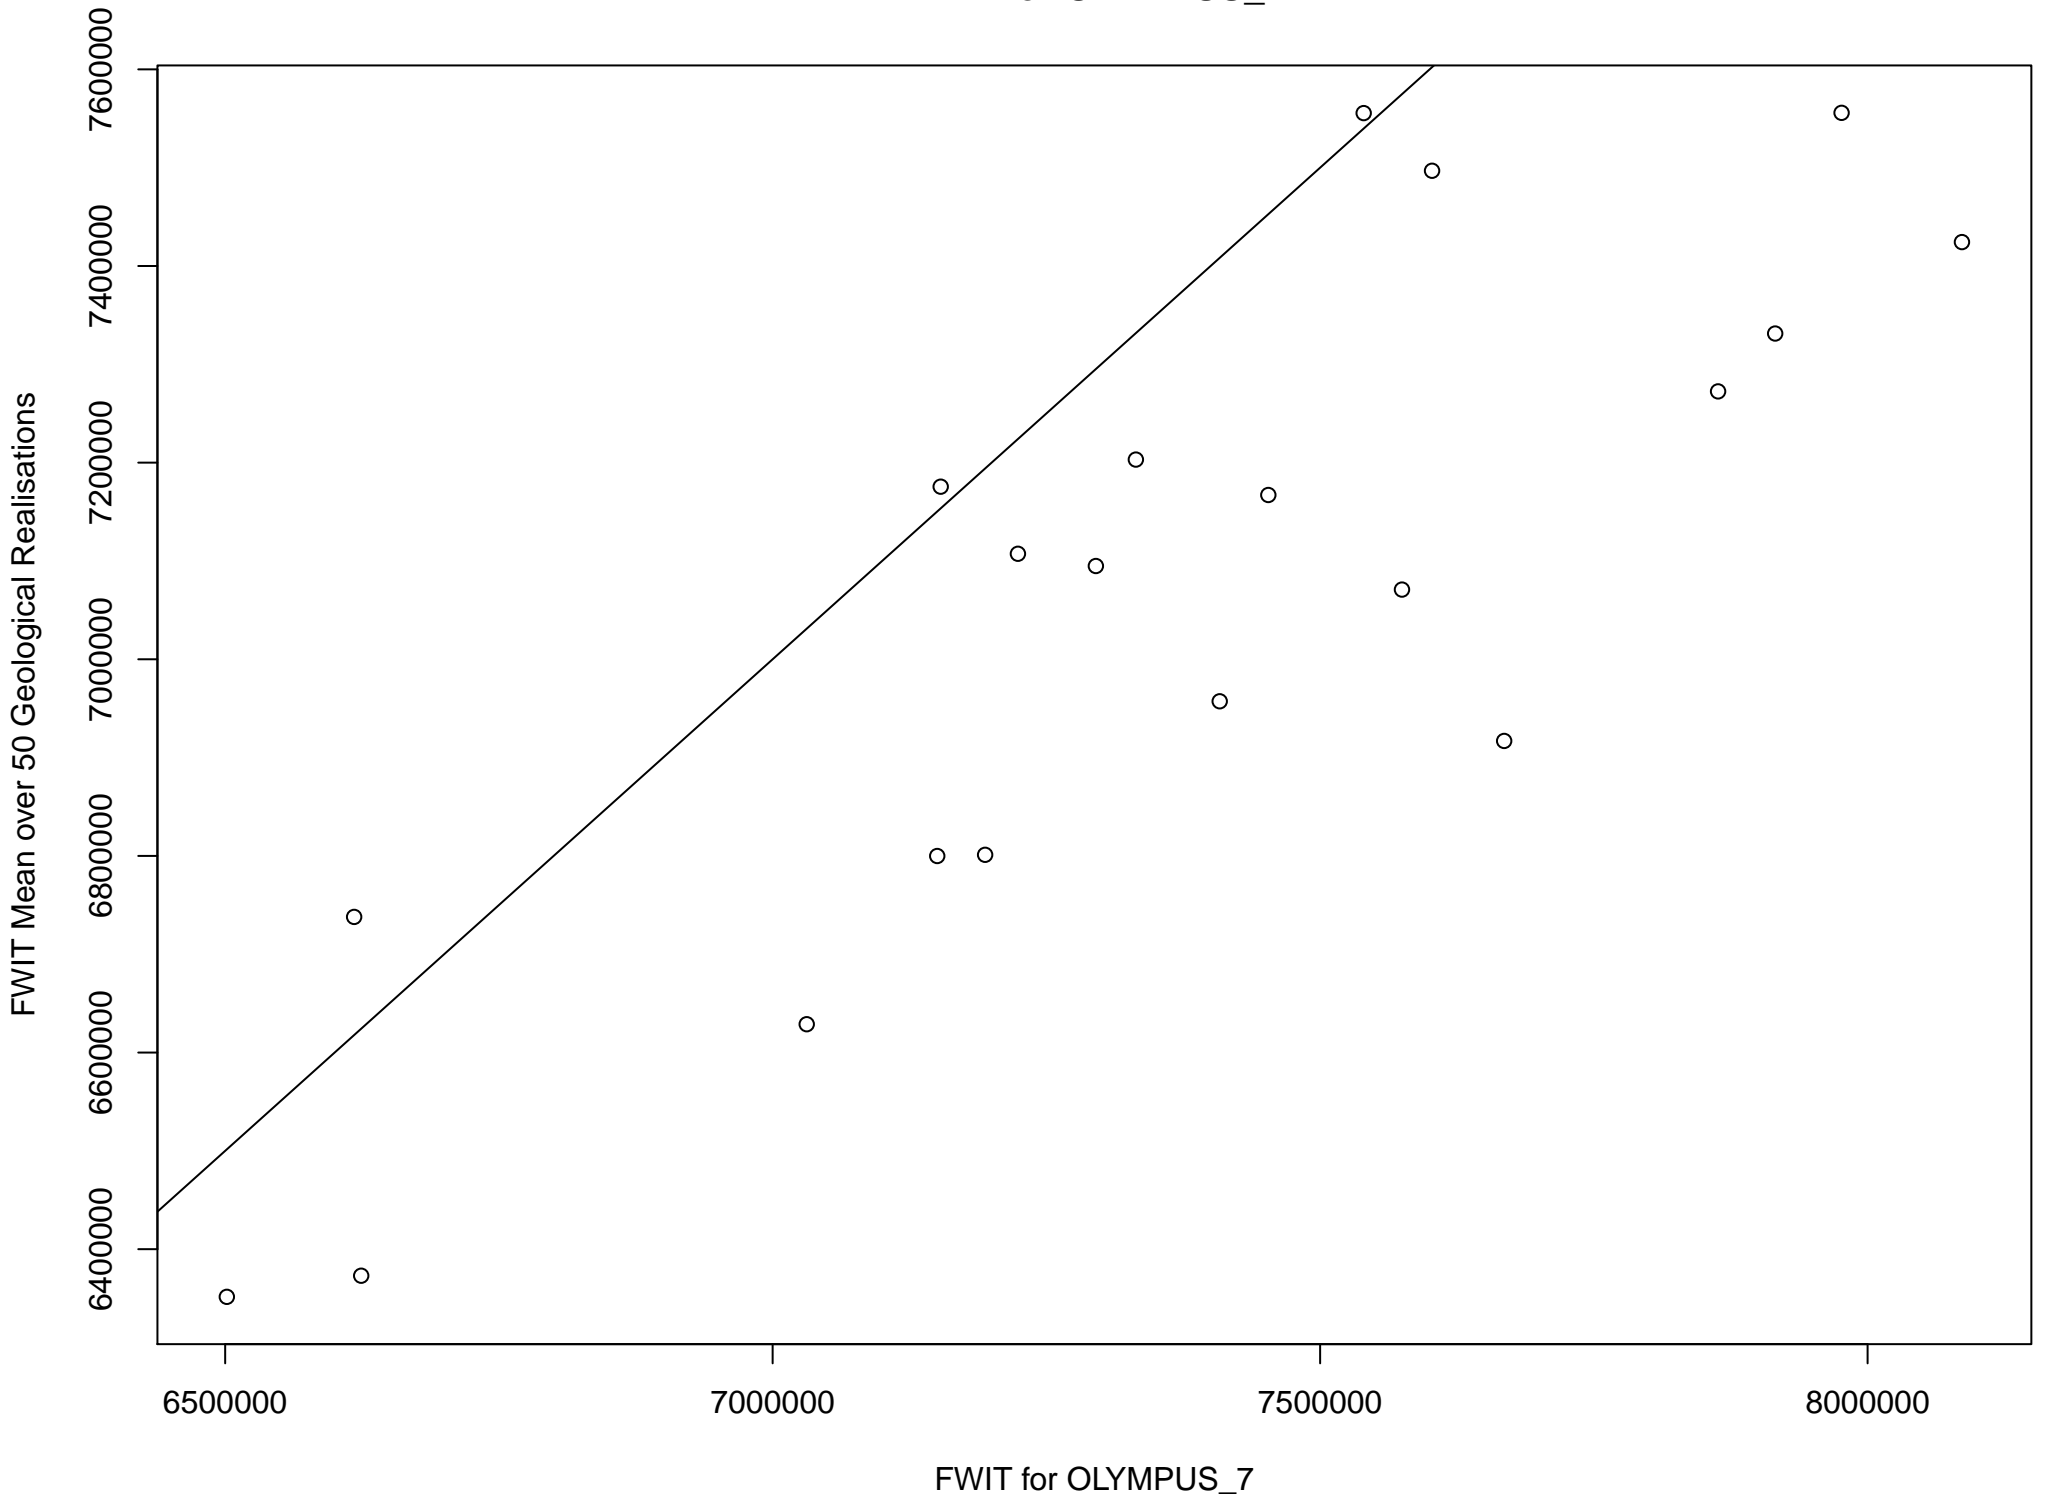

FWIT for OLYMPUS\_8

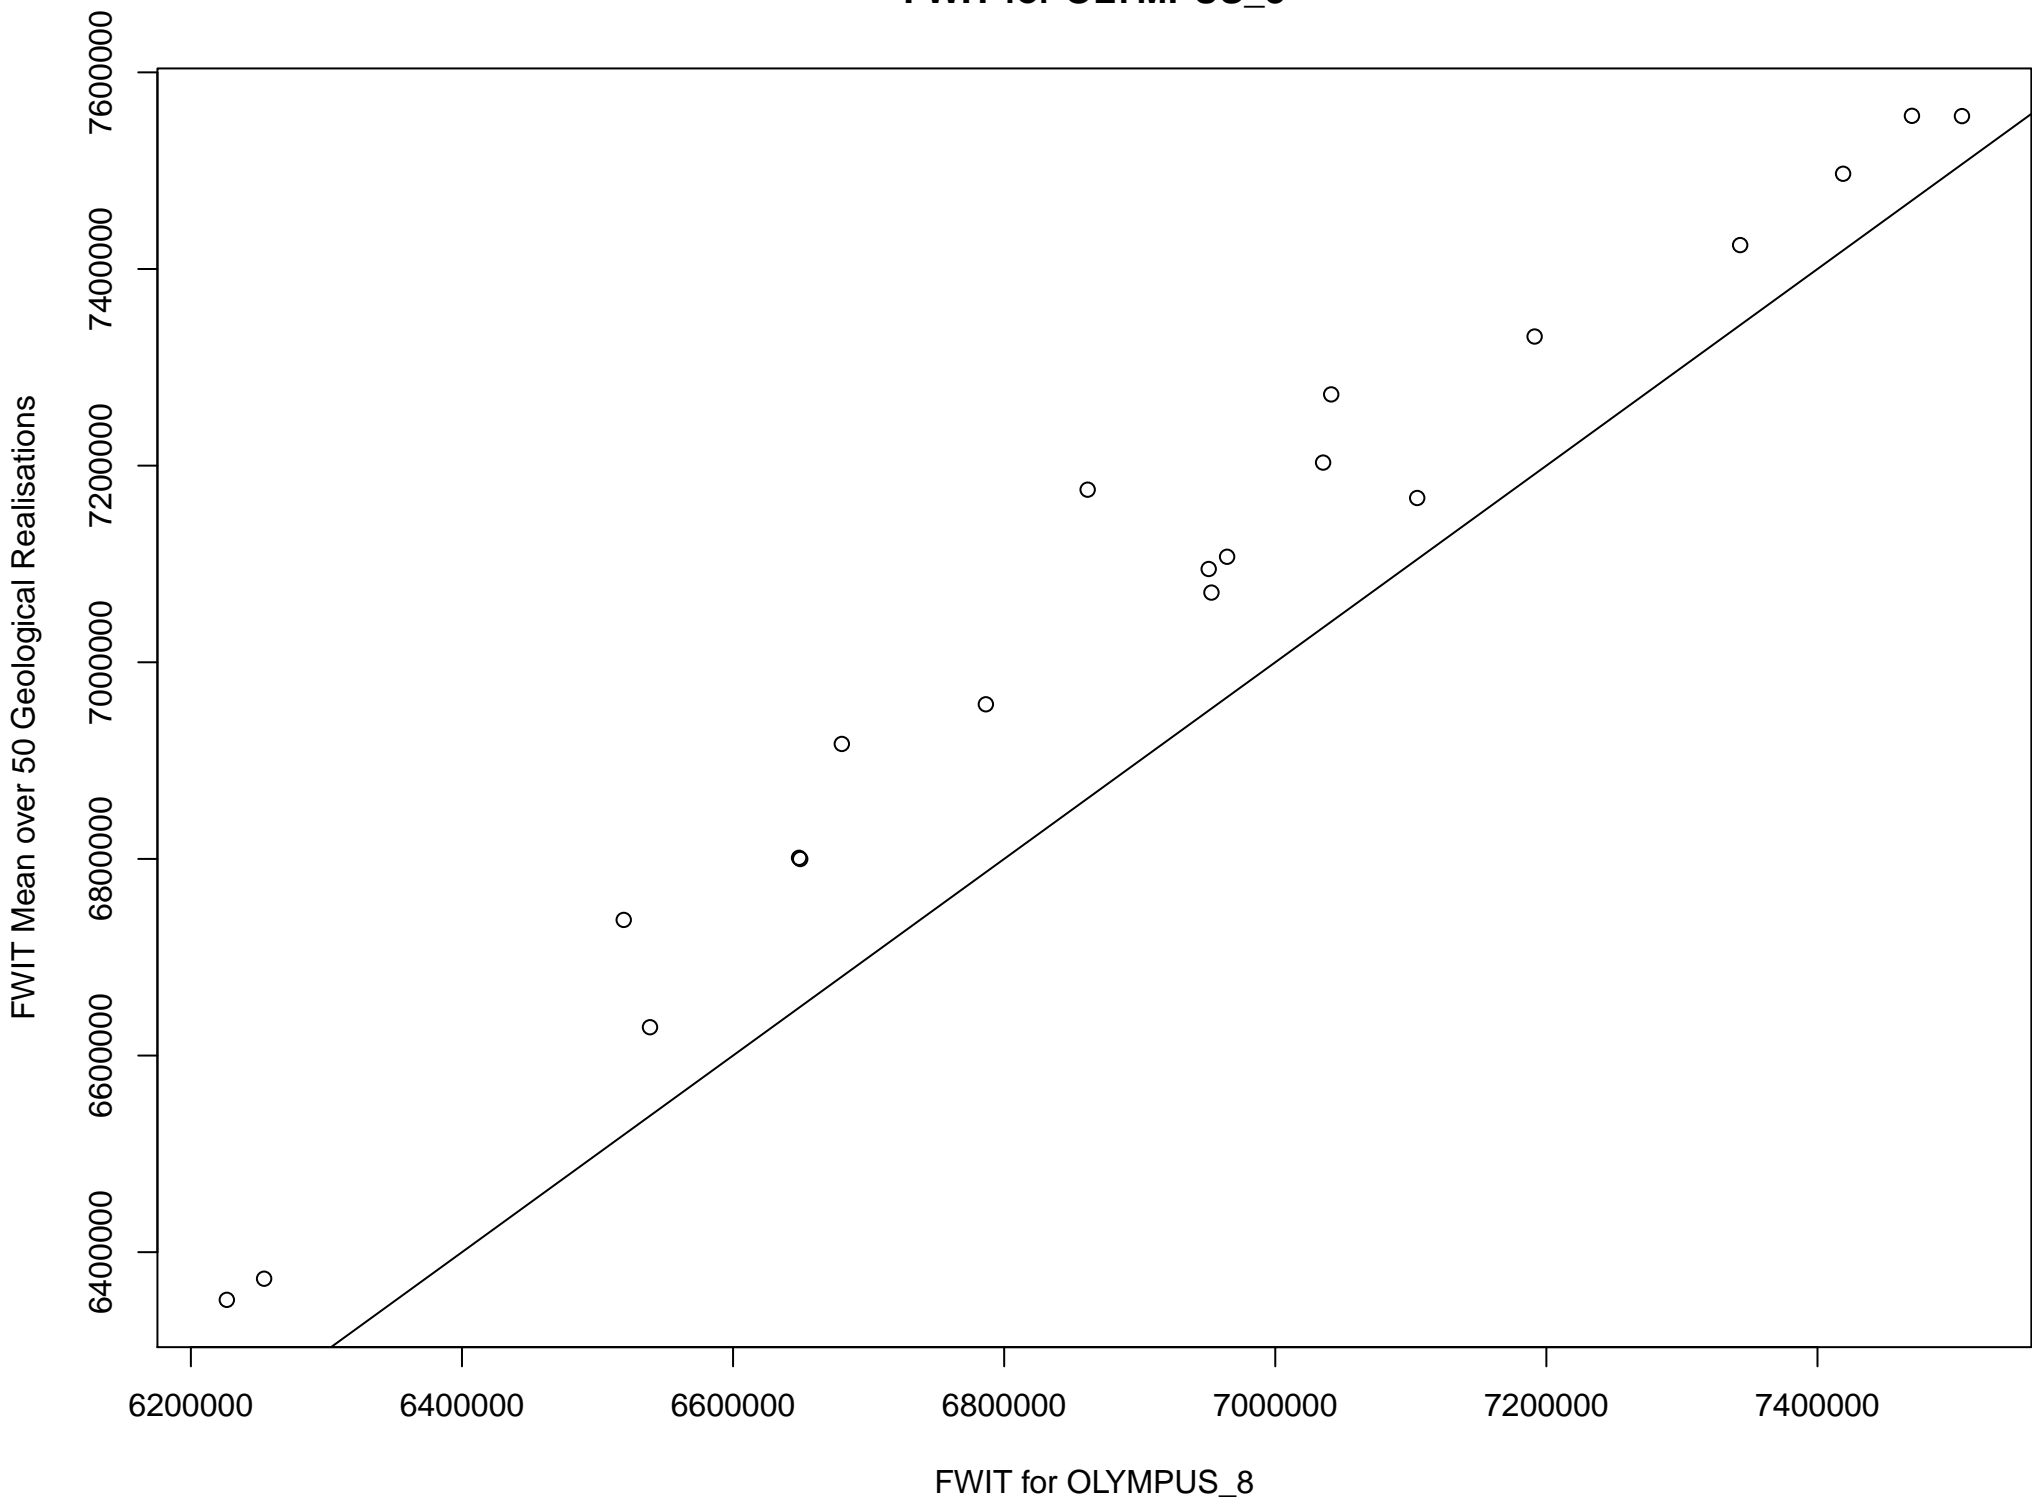



FWIT for OLYMPUS\_9

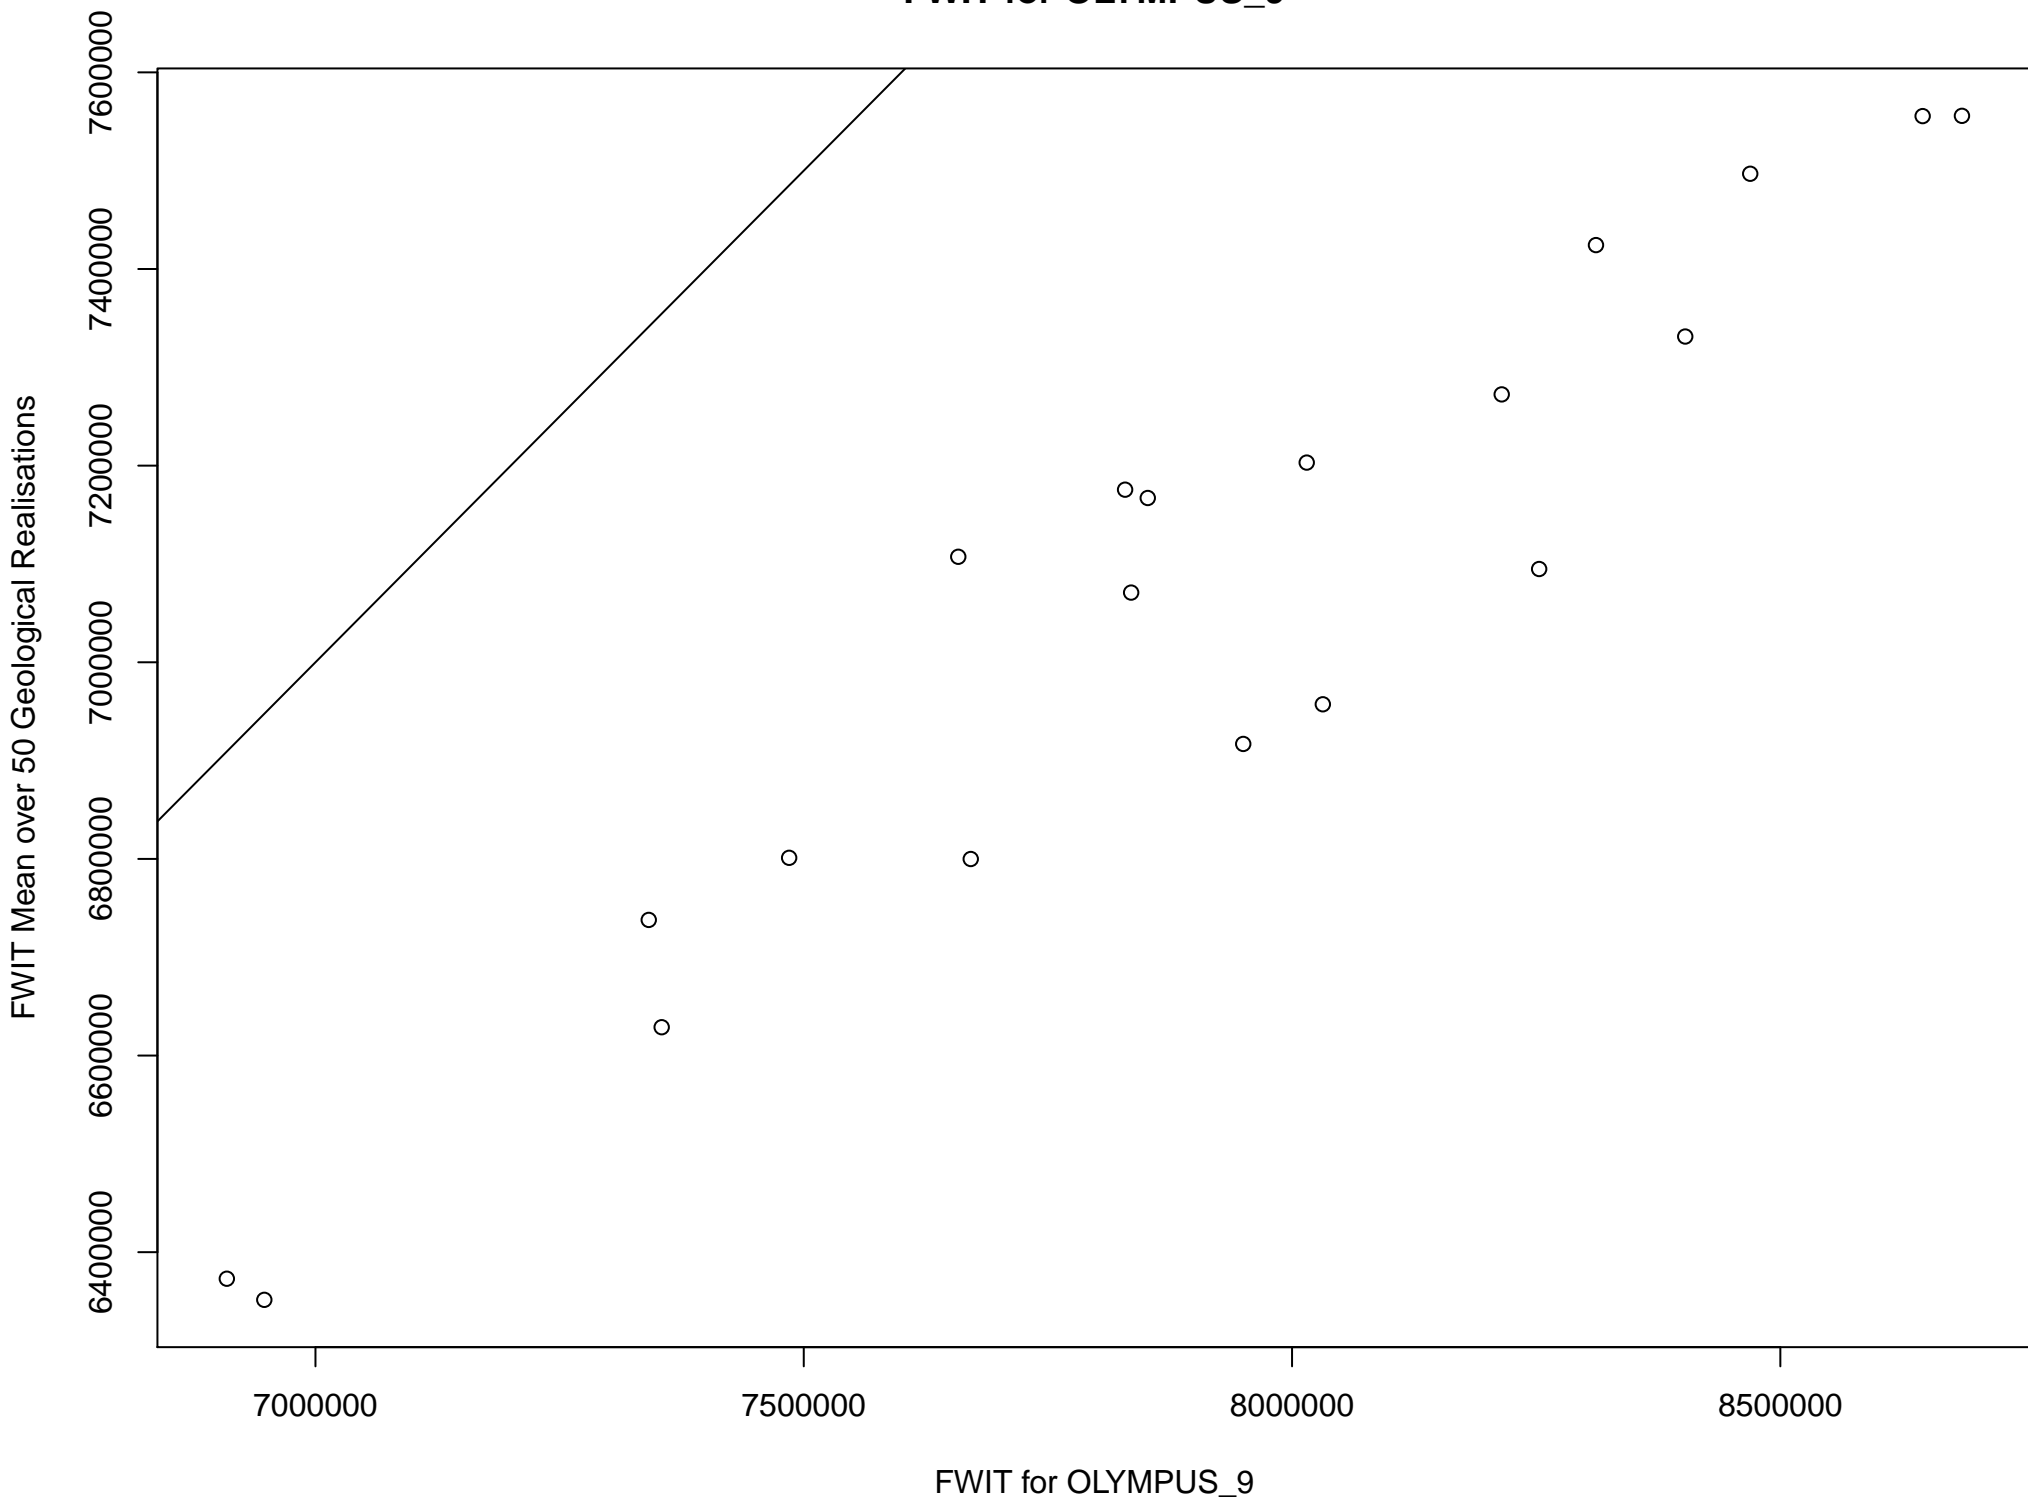

FWIT for OLYMPUS\_10

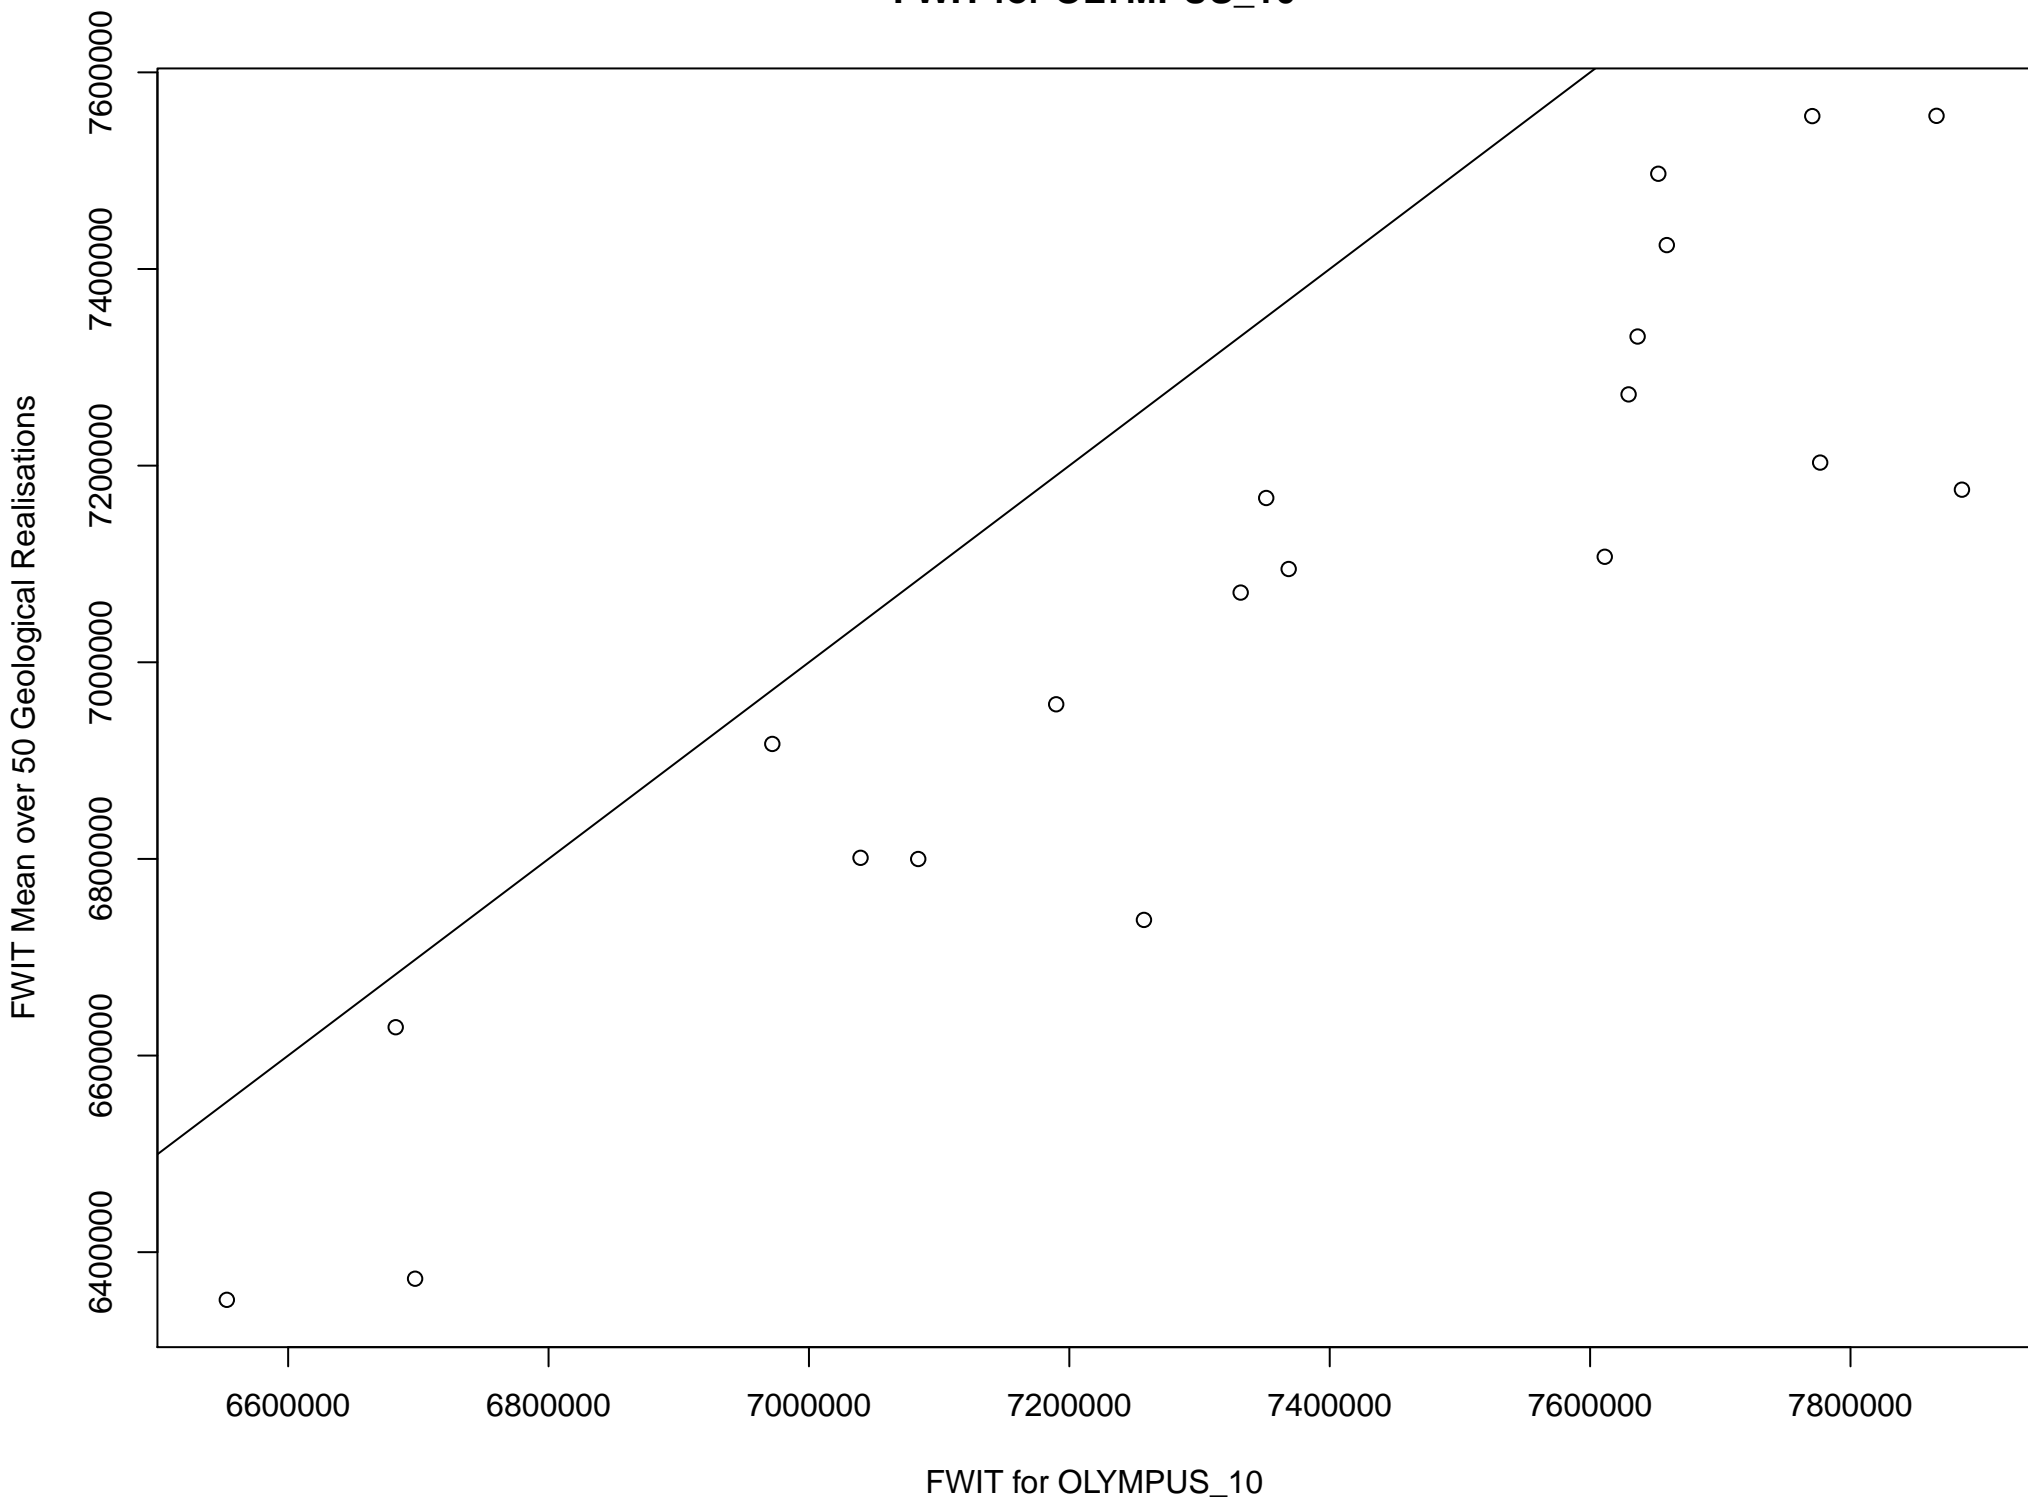

FWIT for OLYMPUS\_11

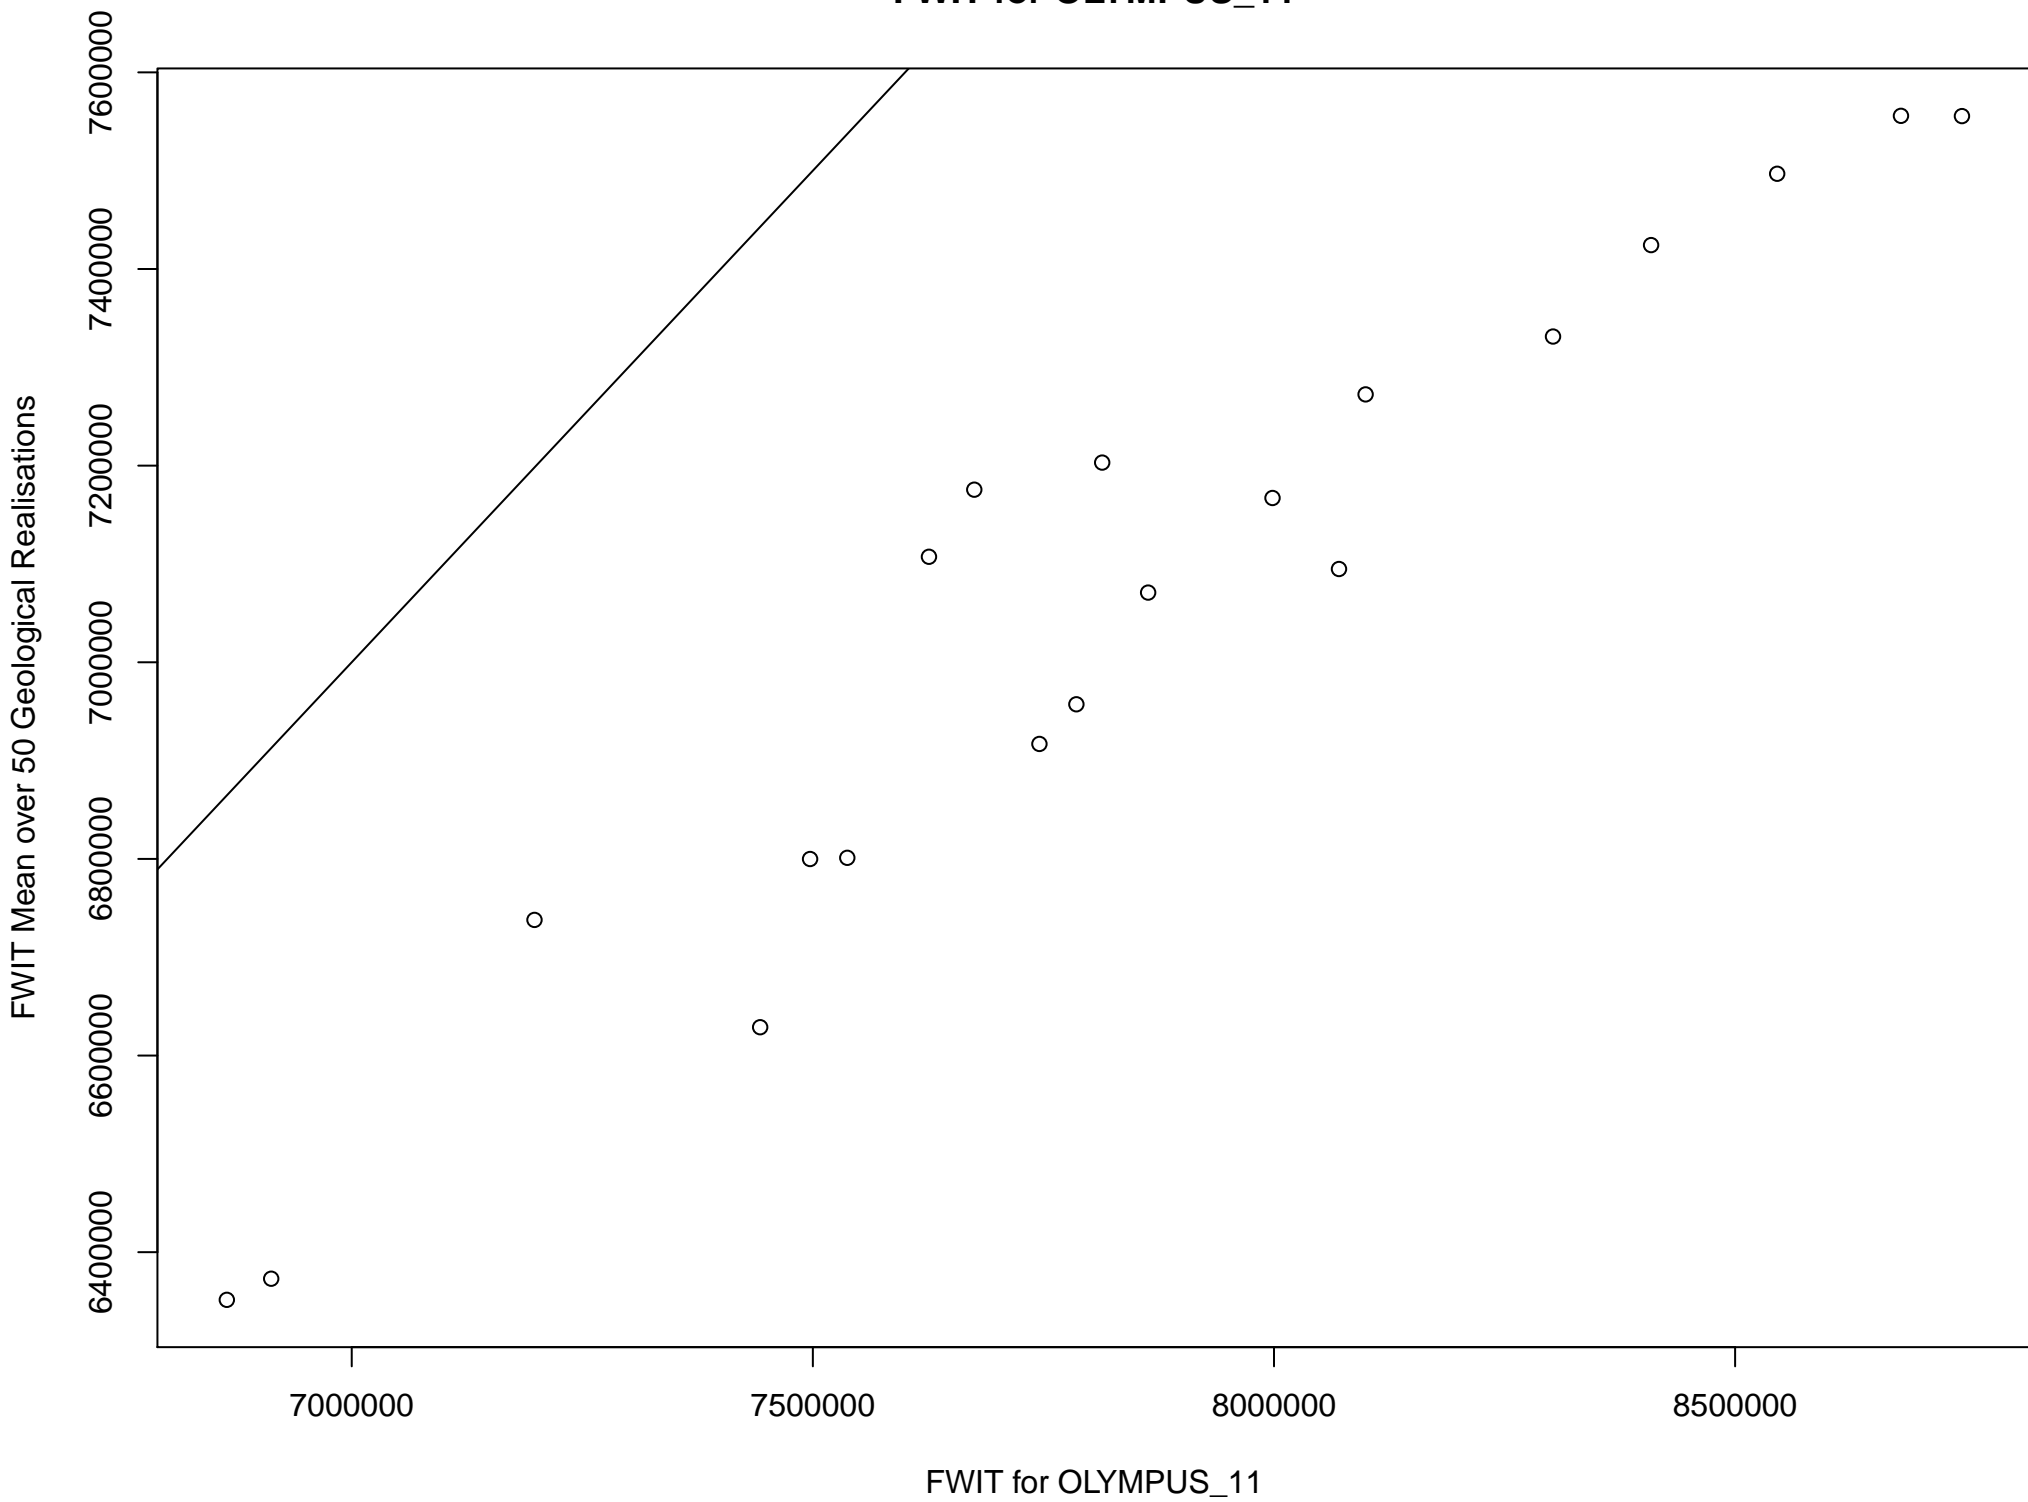

FWIT for OLYMPUS\_12

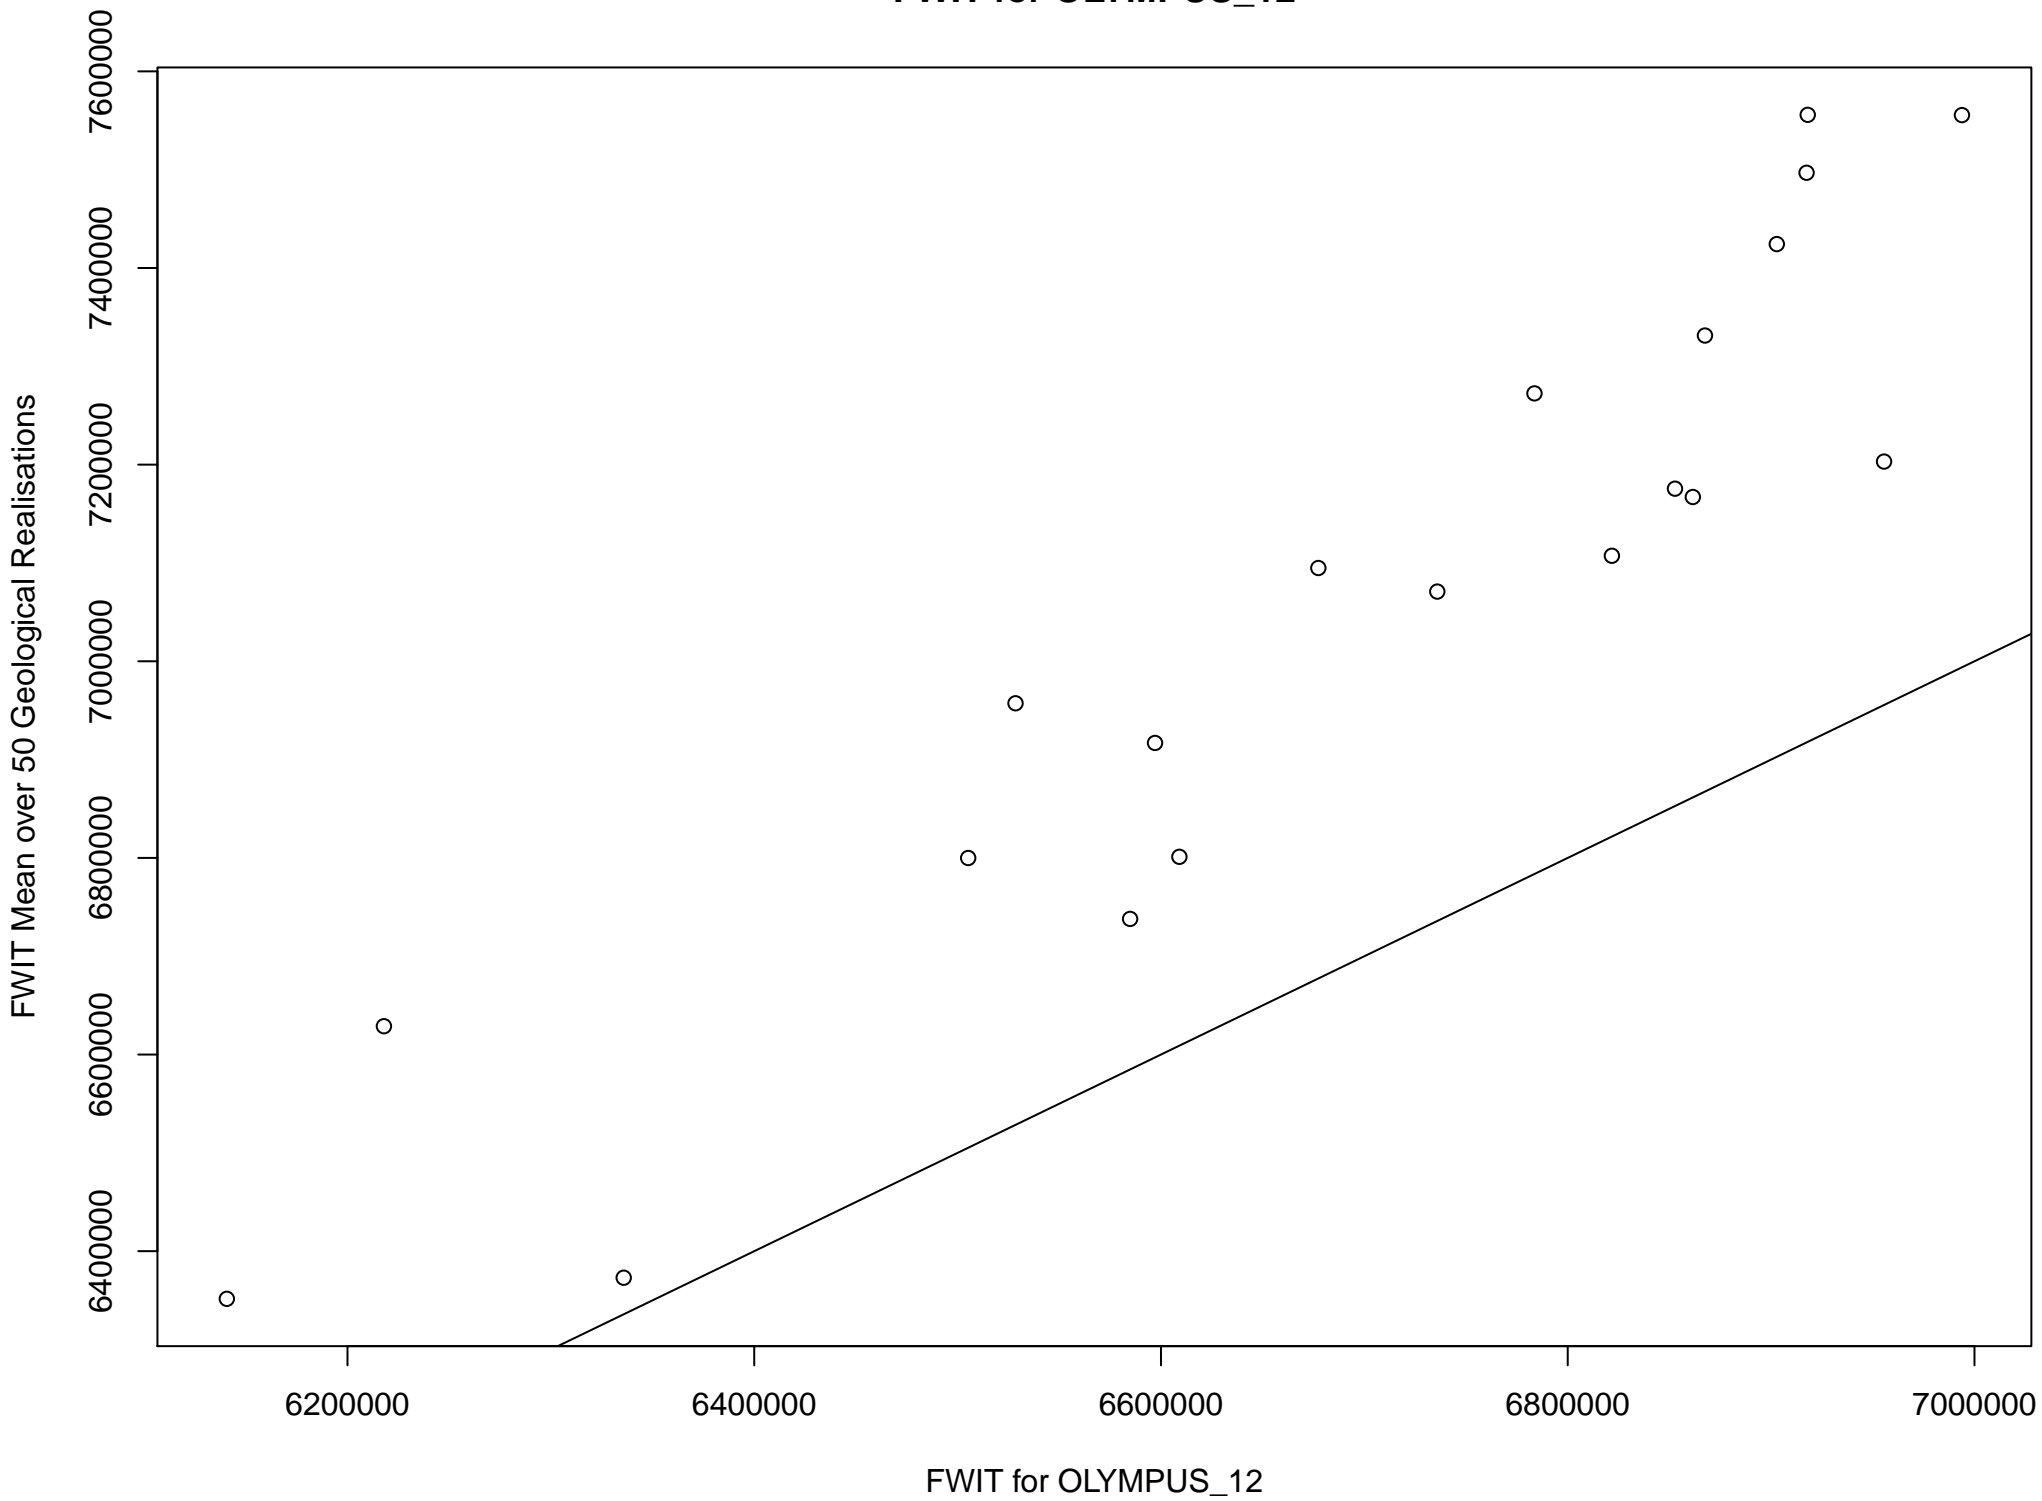

FWIT for OLYMPUS\_13

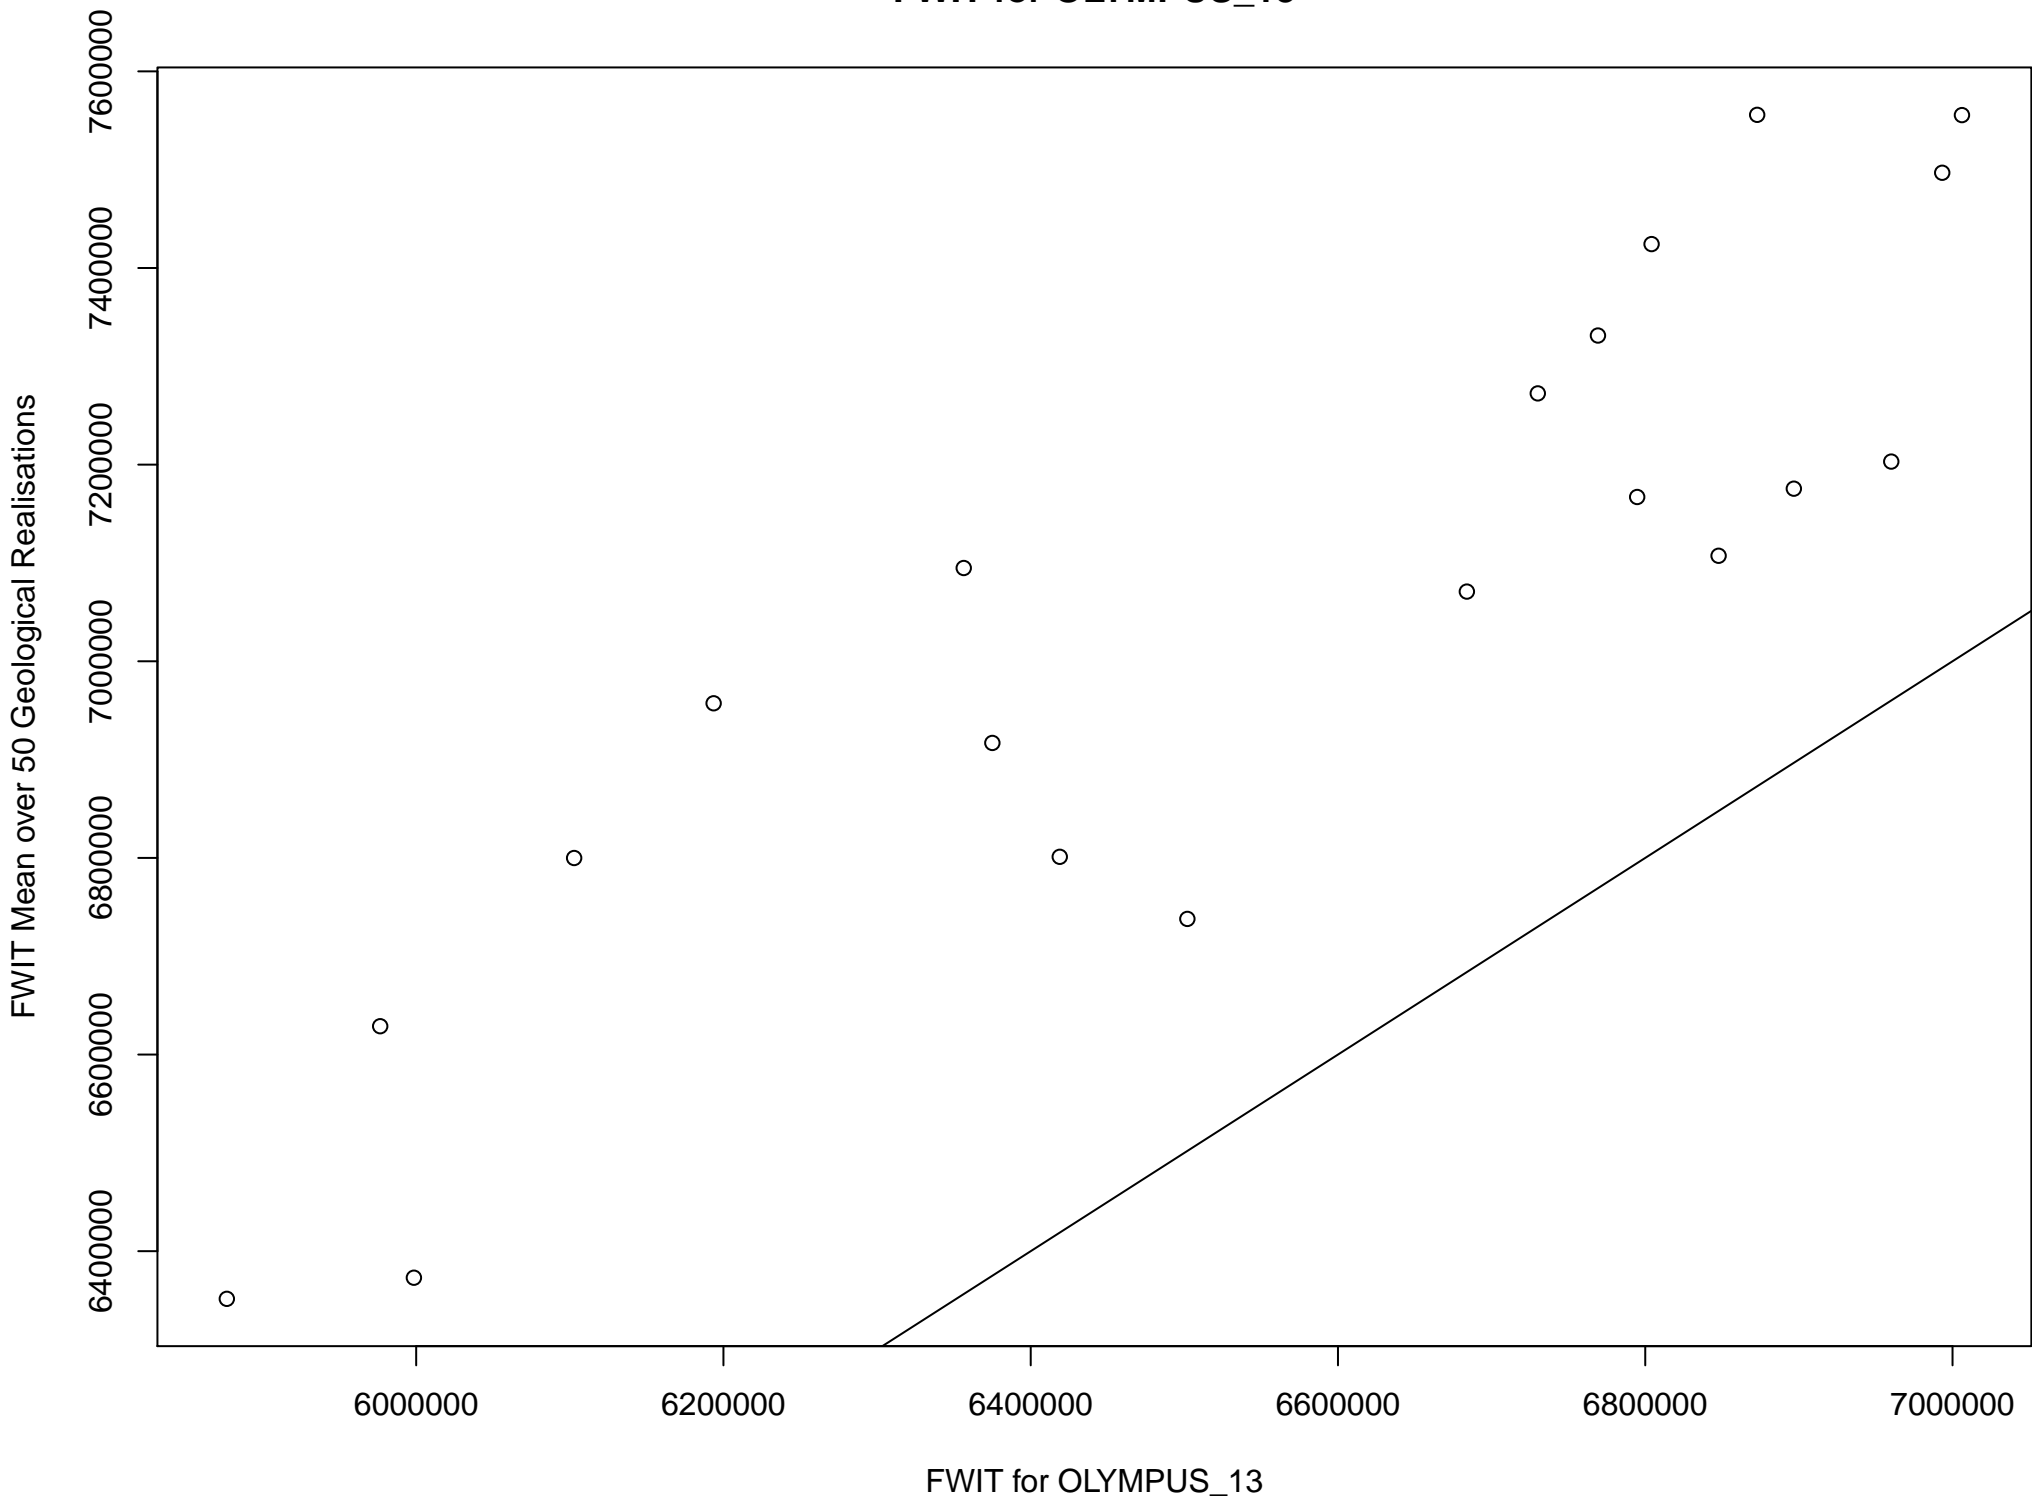

FWIT for OLYMPUS\_14

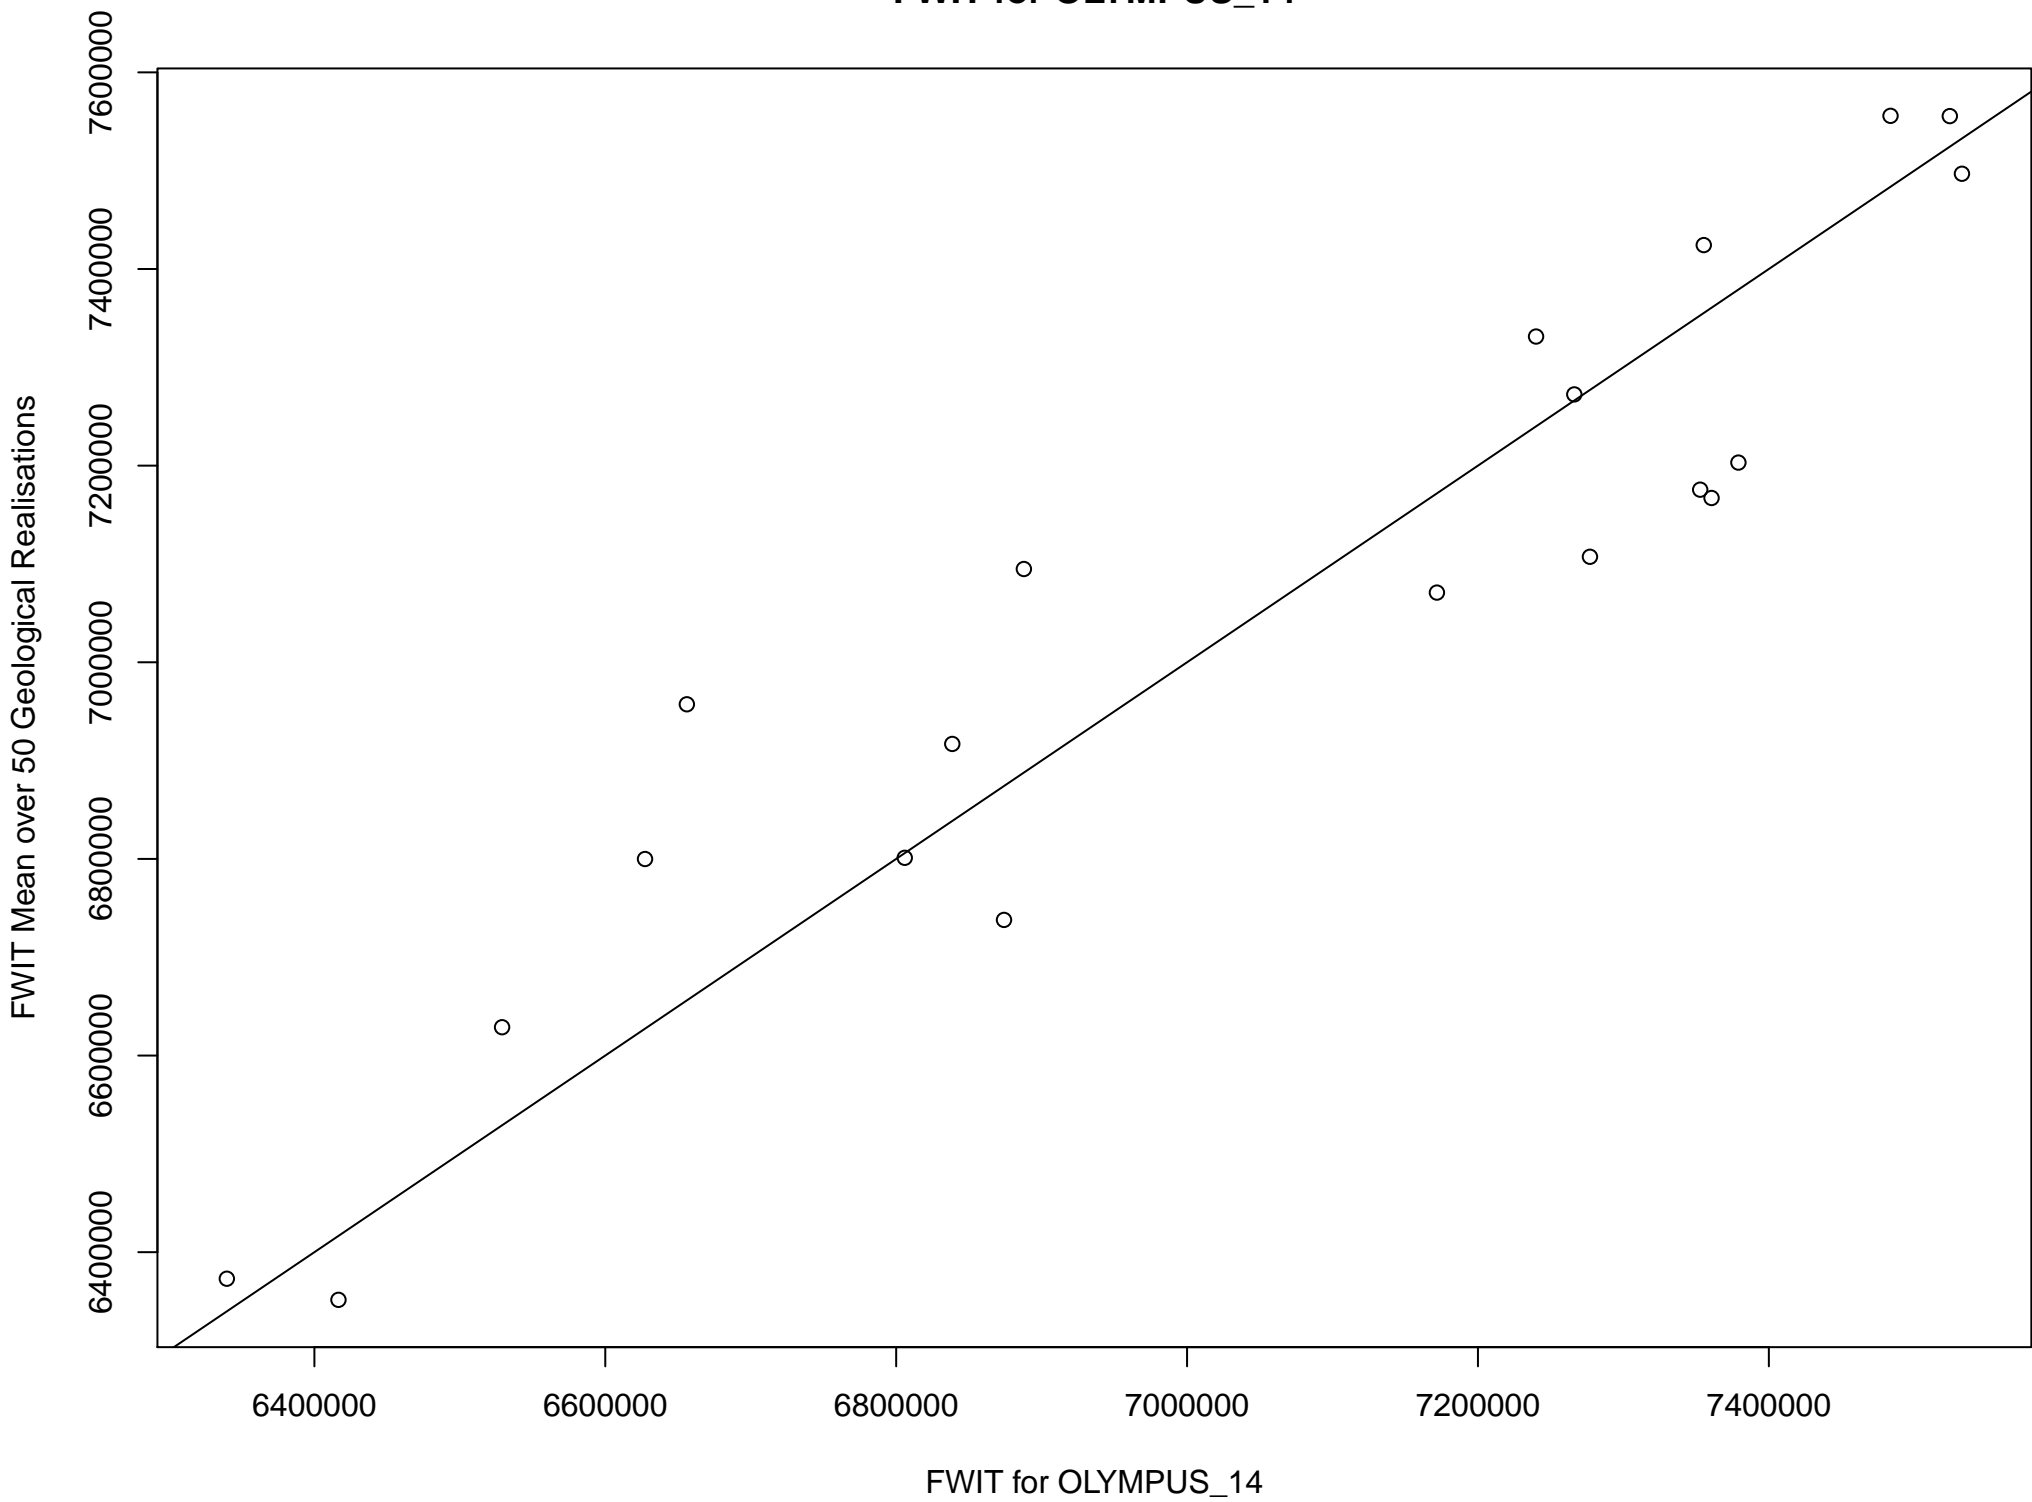

FWIT for OLYMPUS\_15

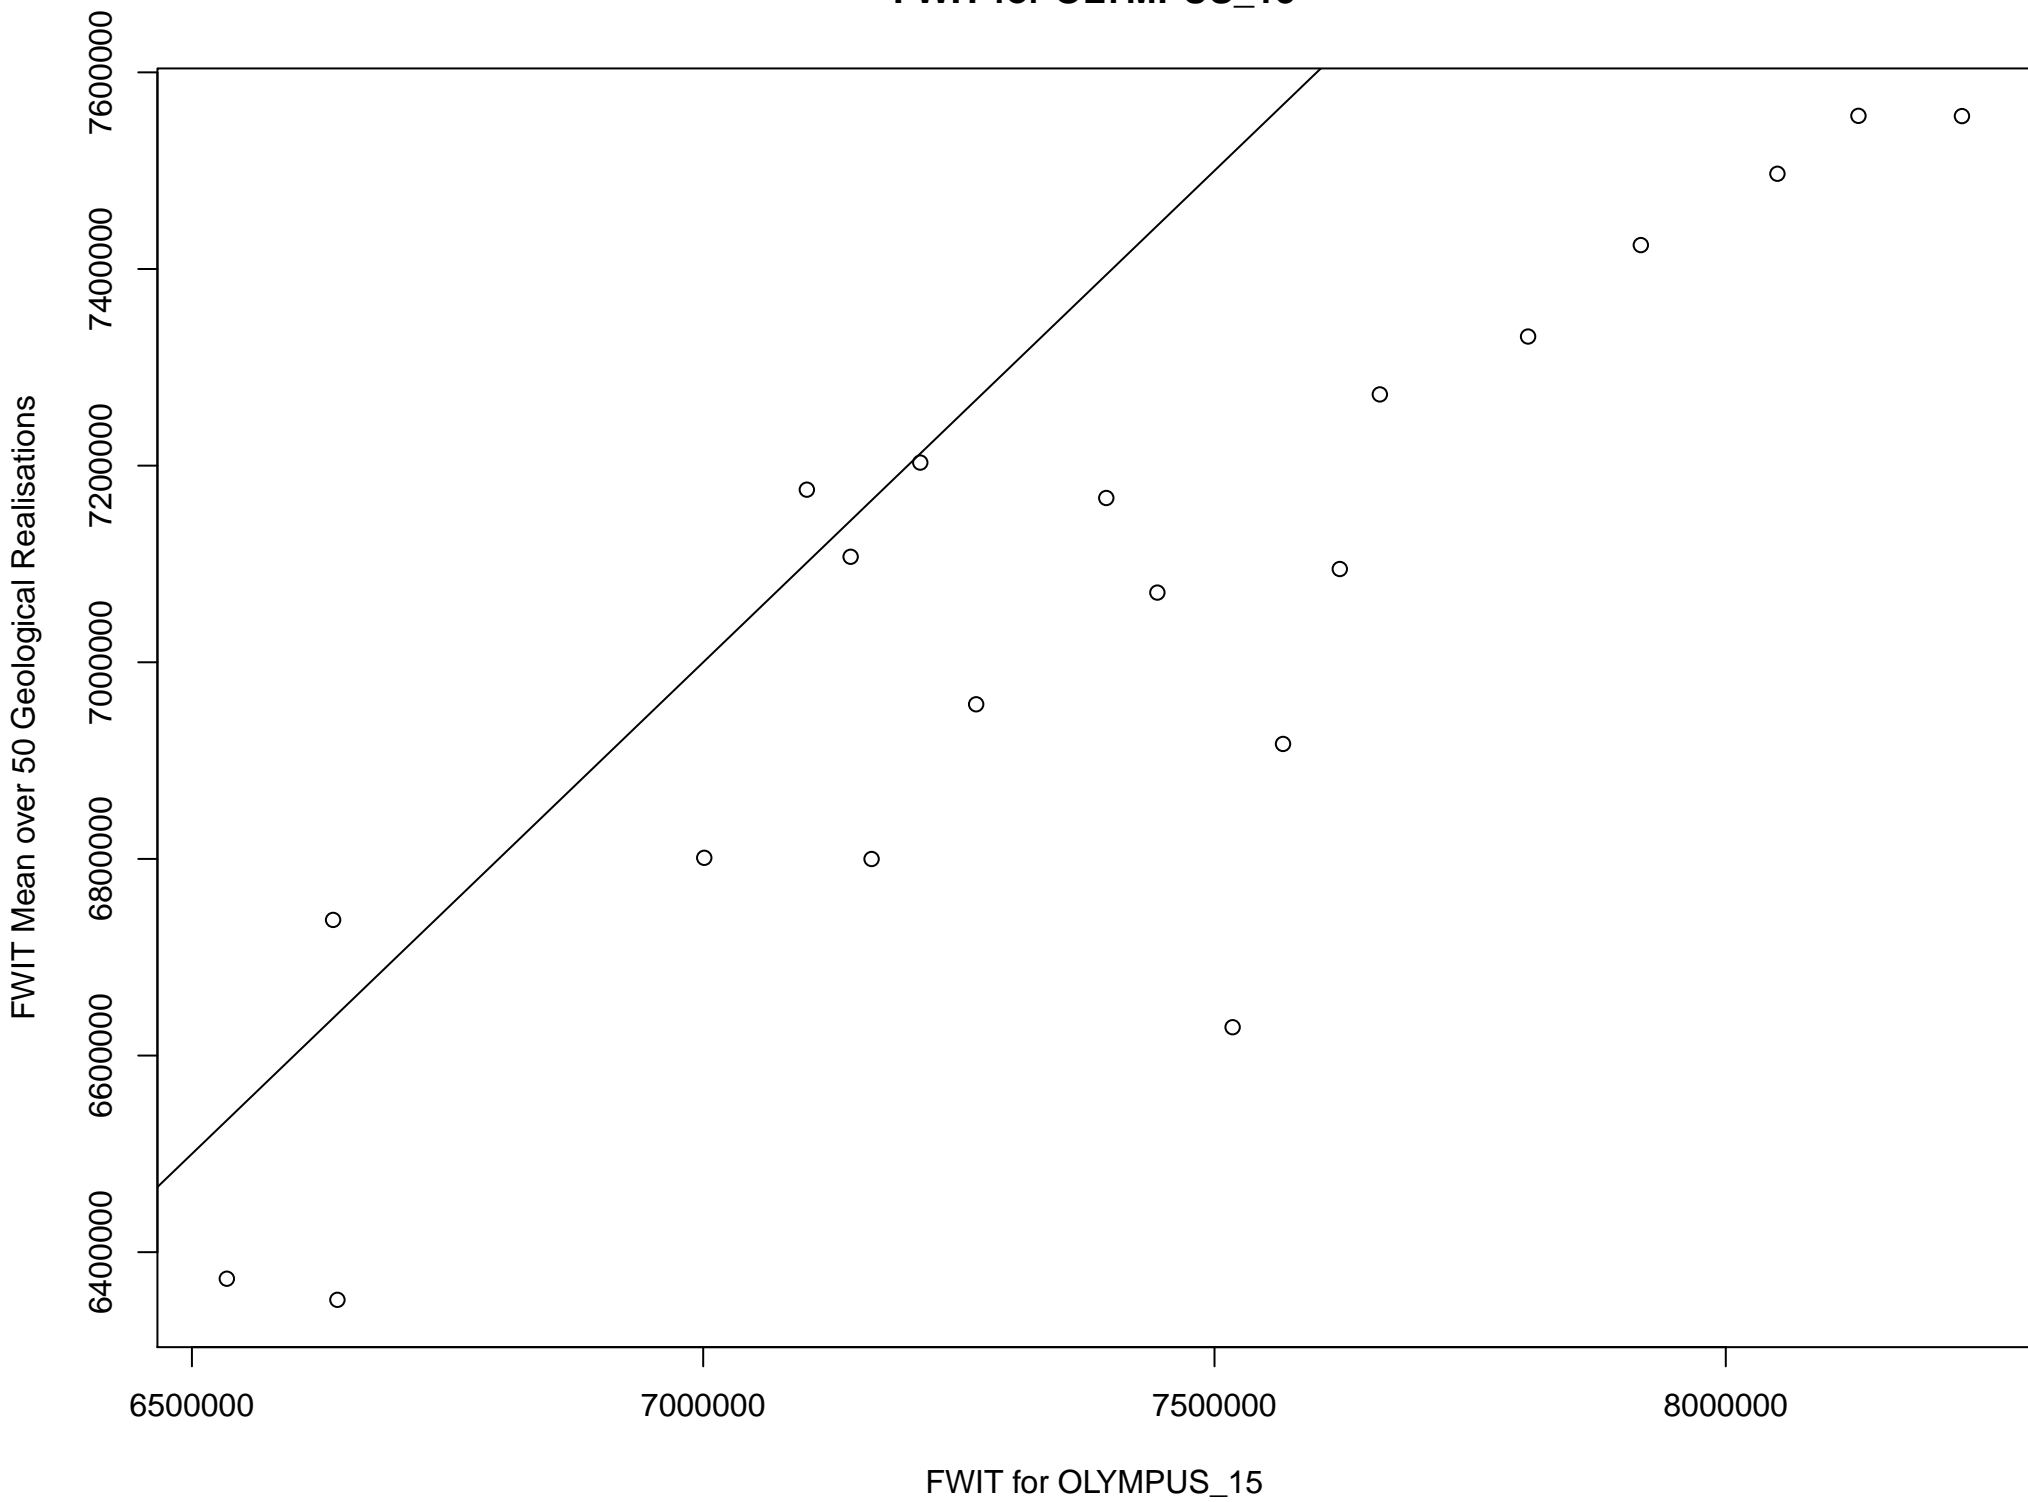

FWIT for OLYMPUS\_16

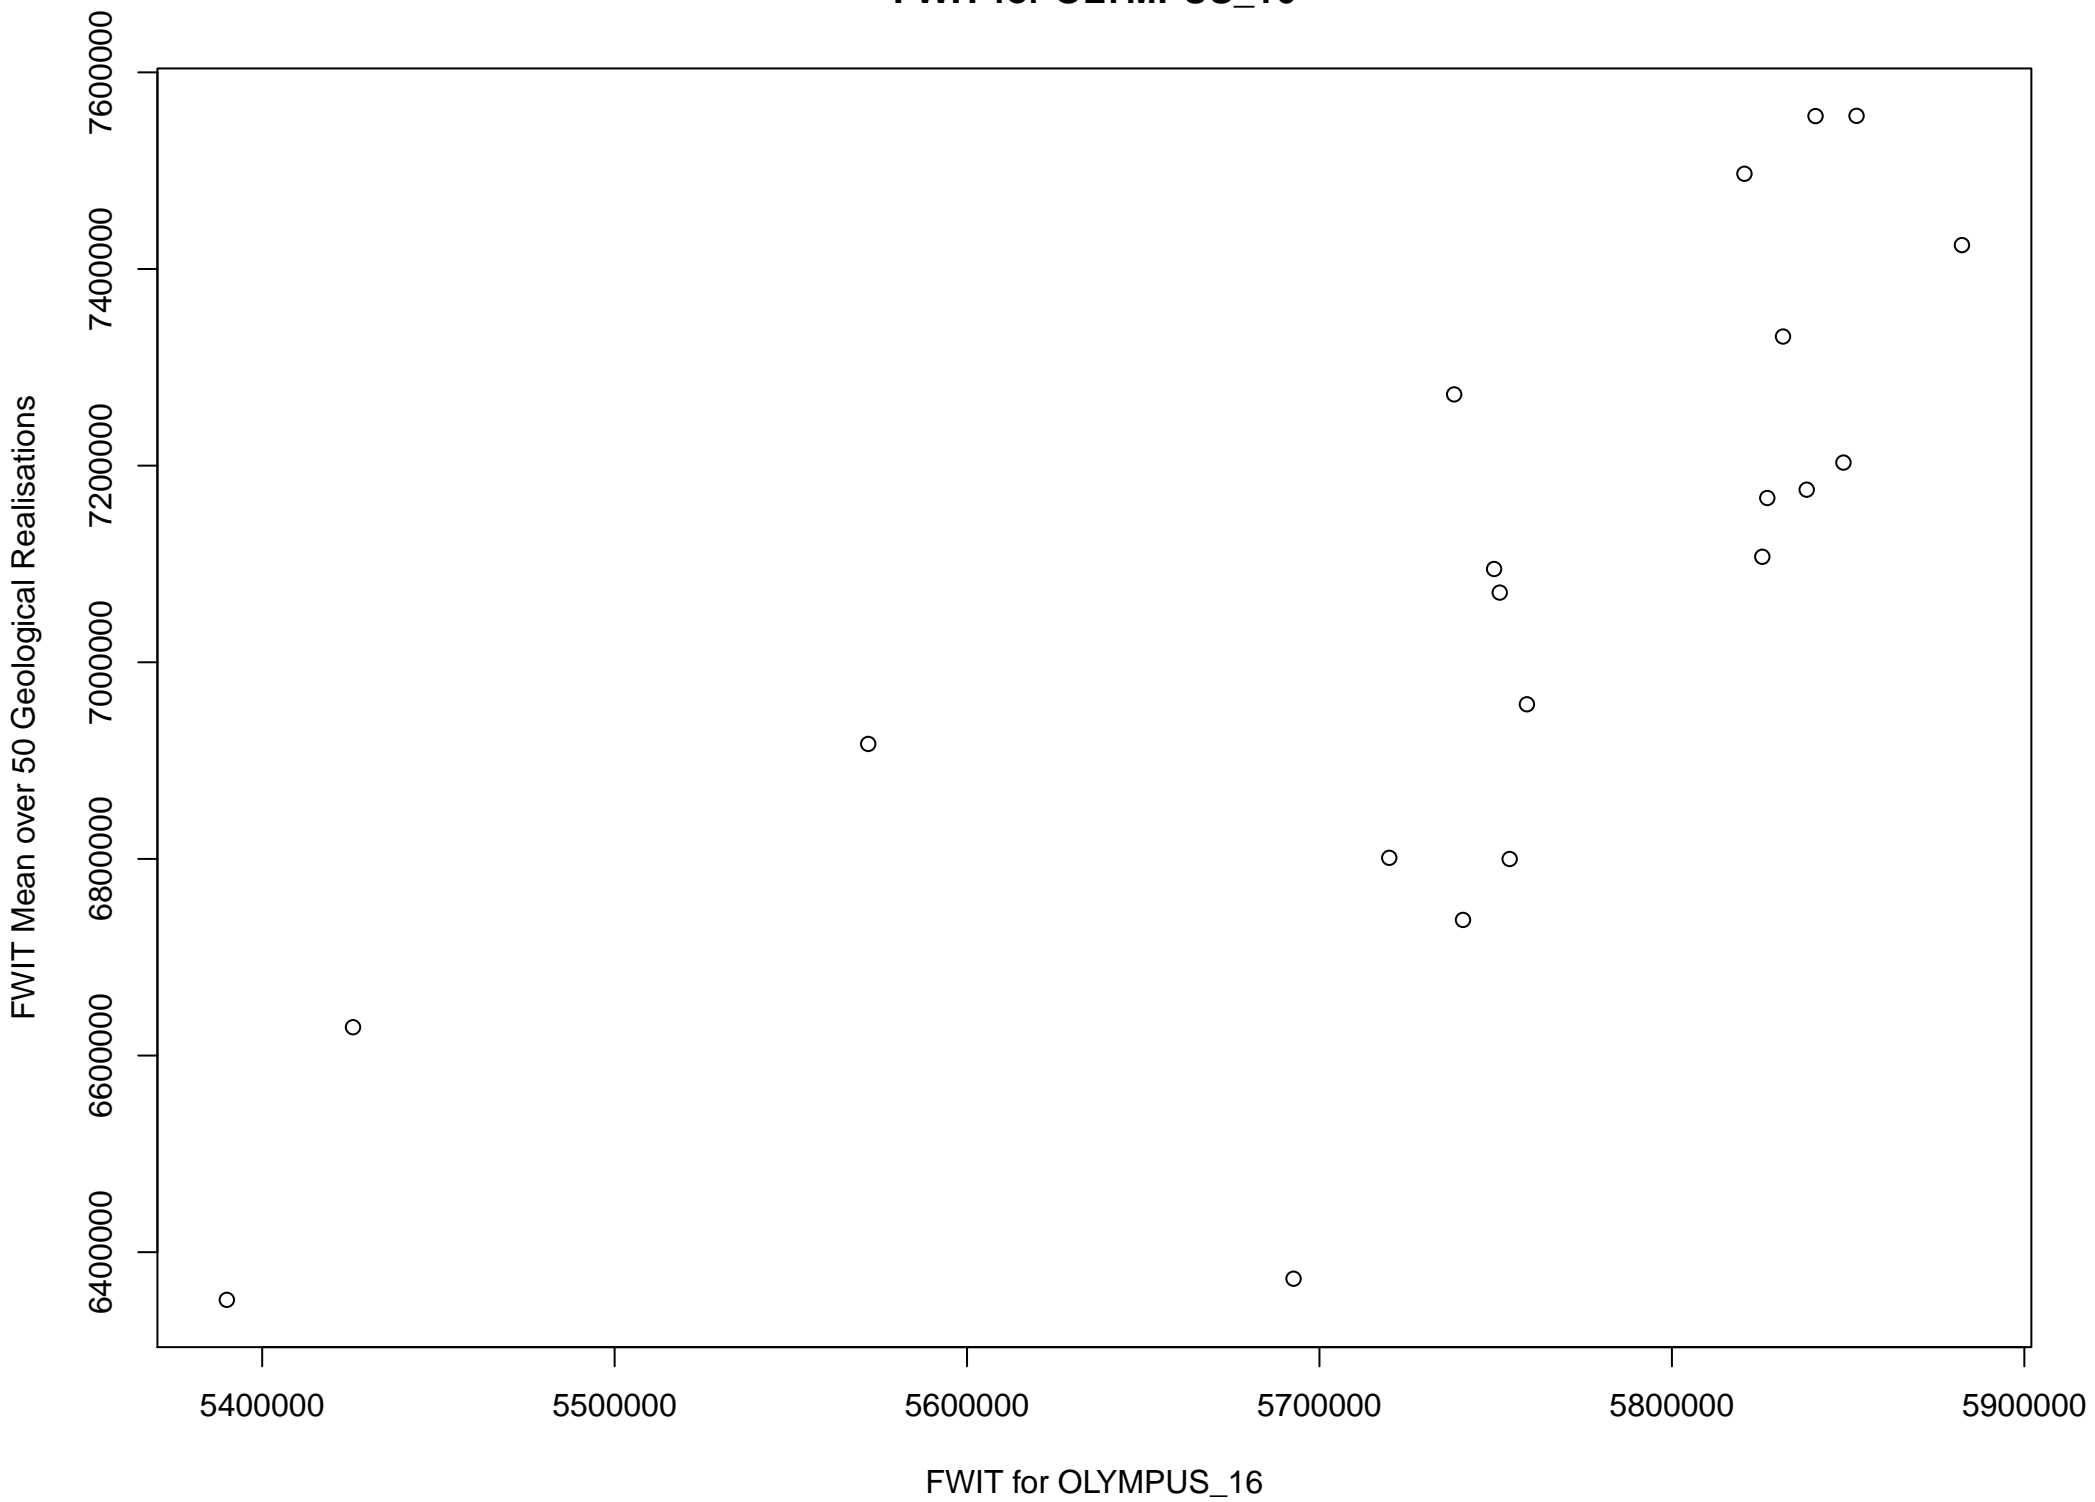



FWIT for OLYMPUS\_17

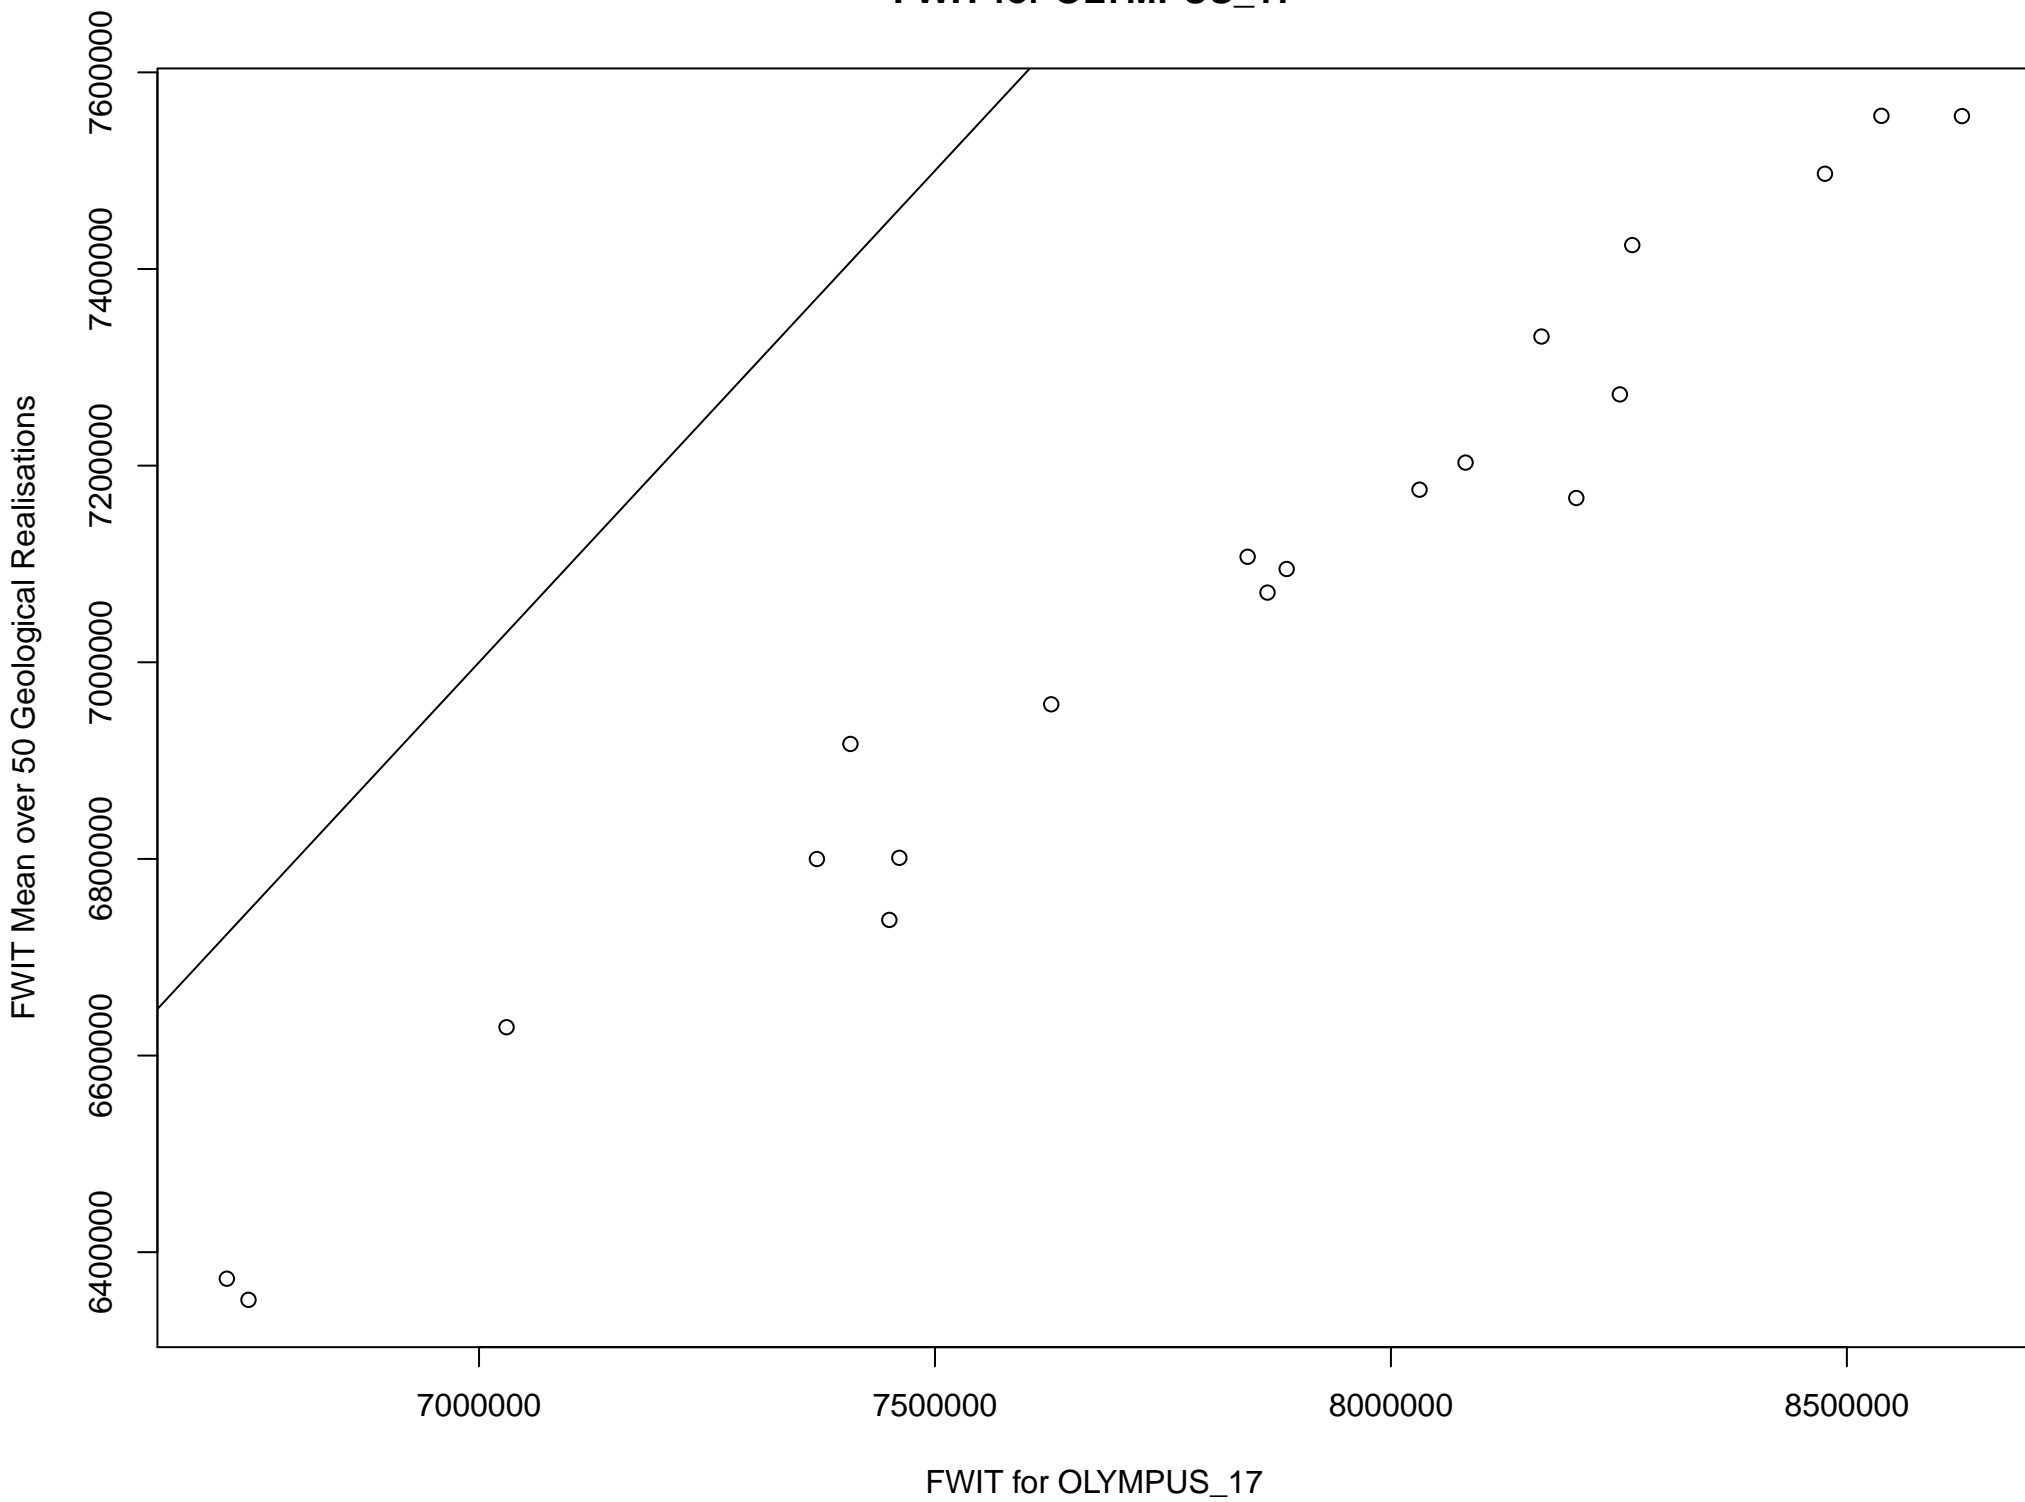

FWIT for OLYMPUS\_18

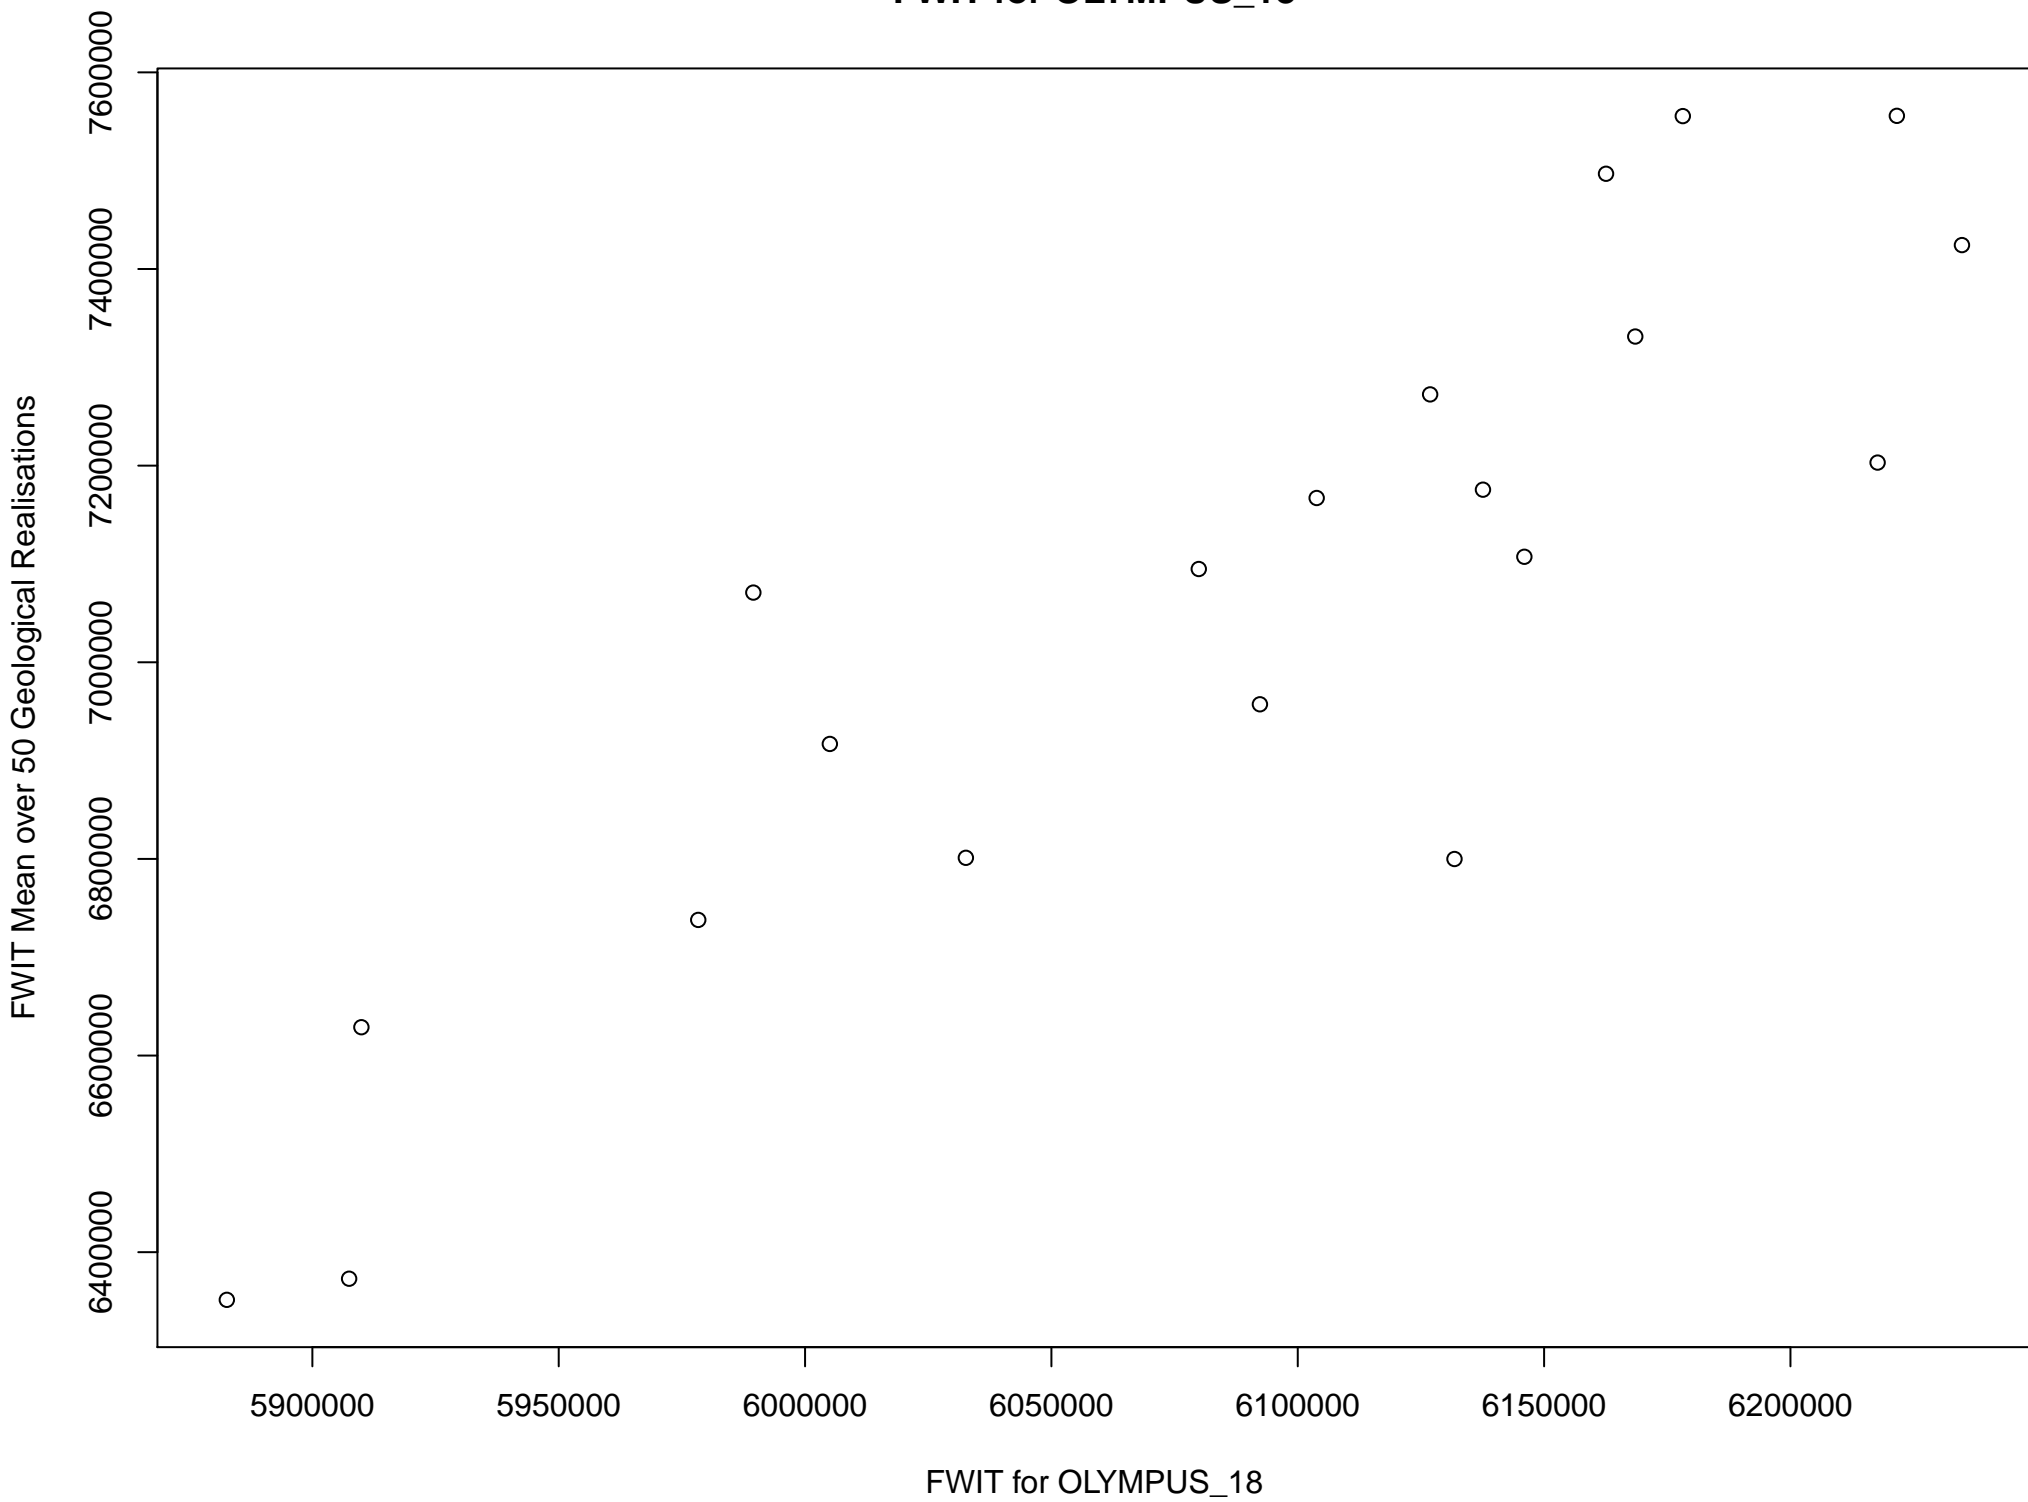

FWIT for OLYMPUS\_19

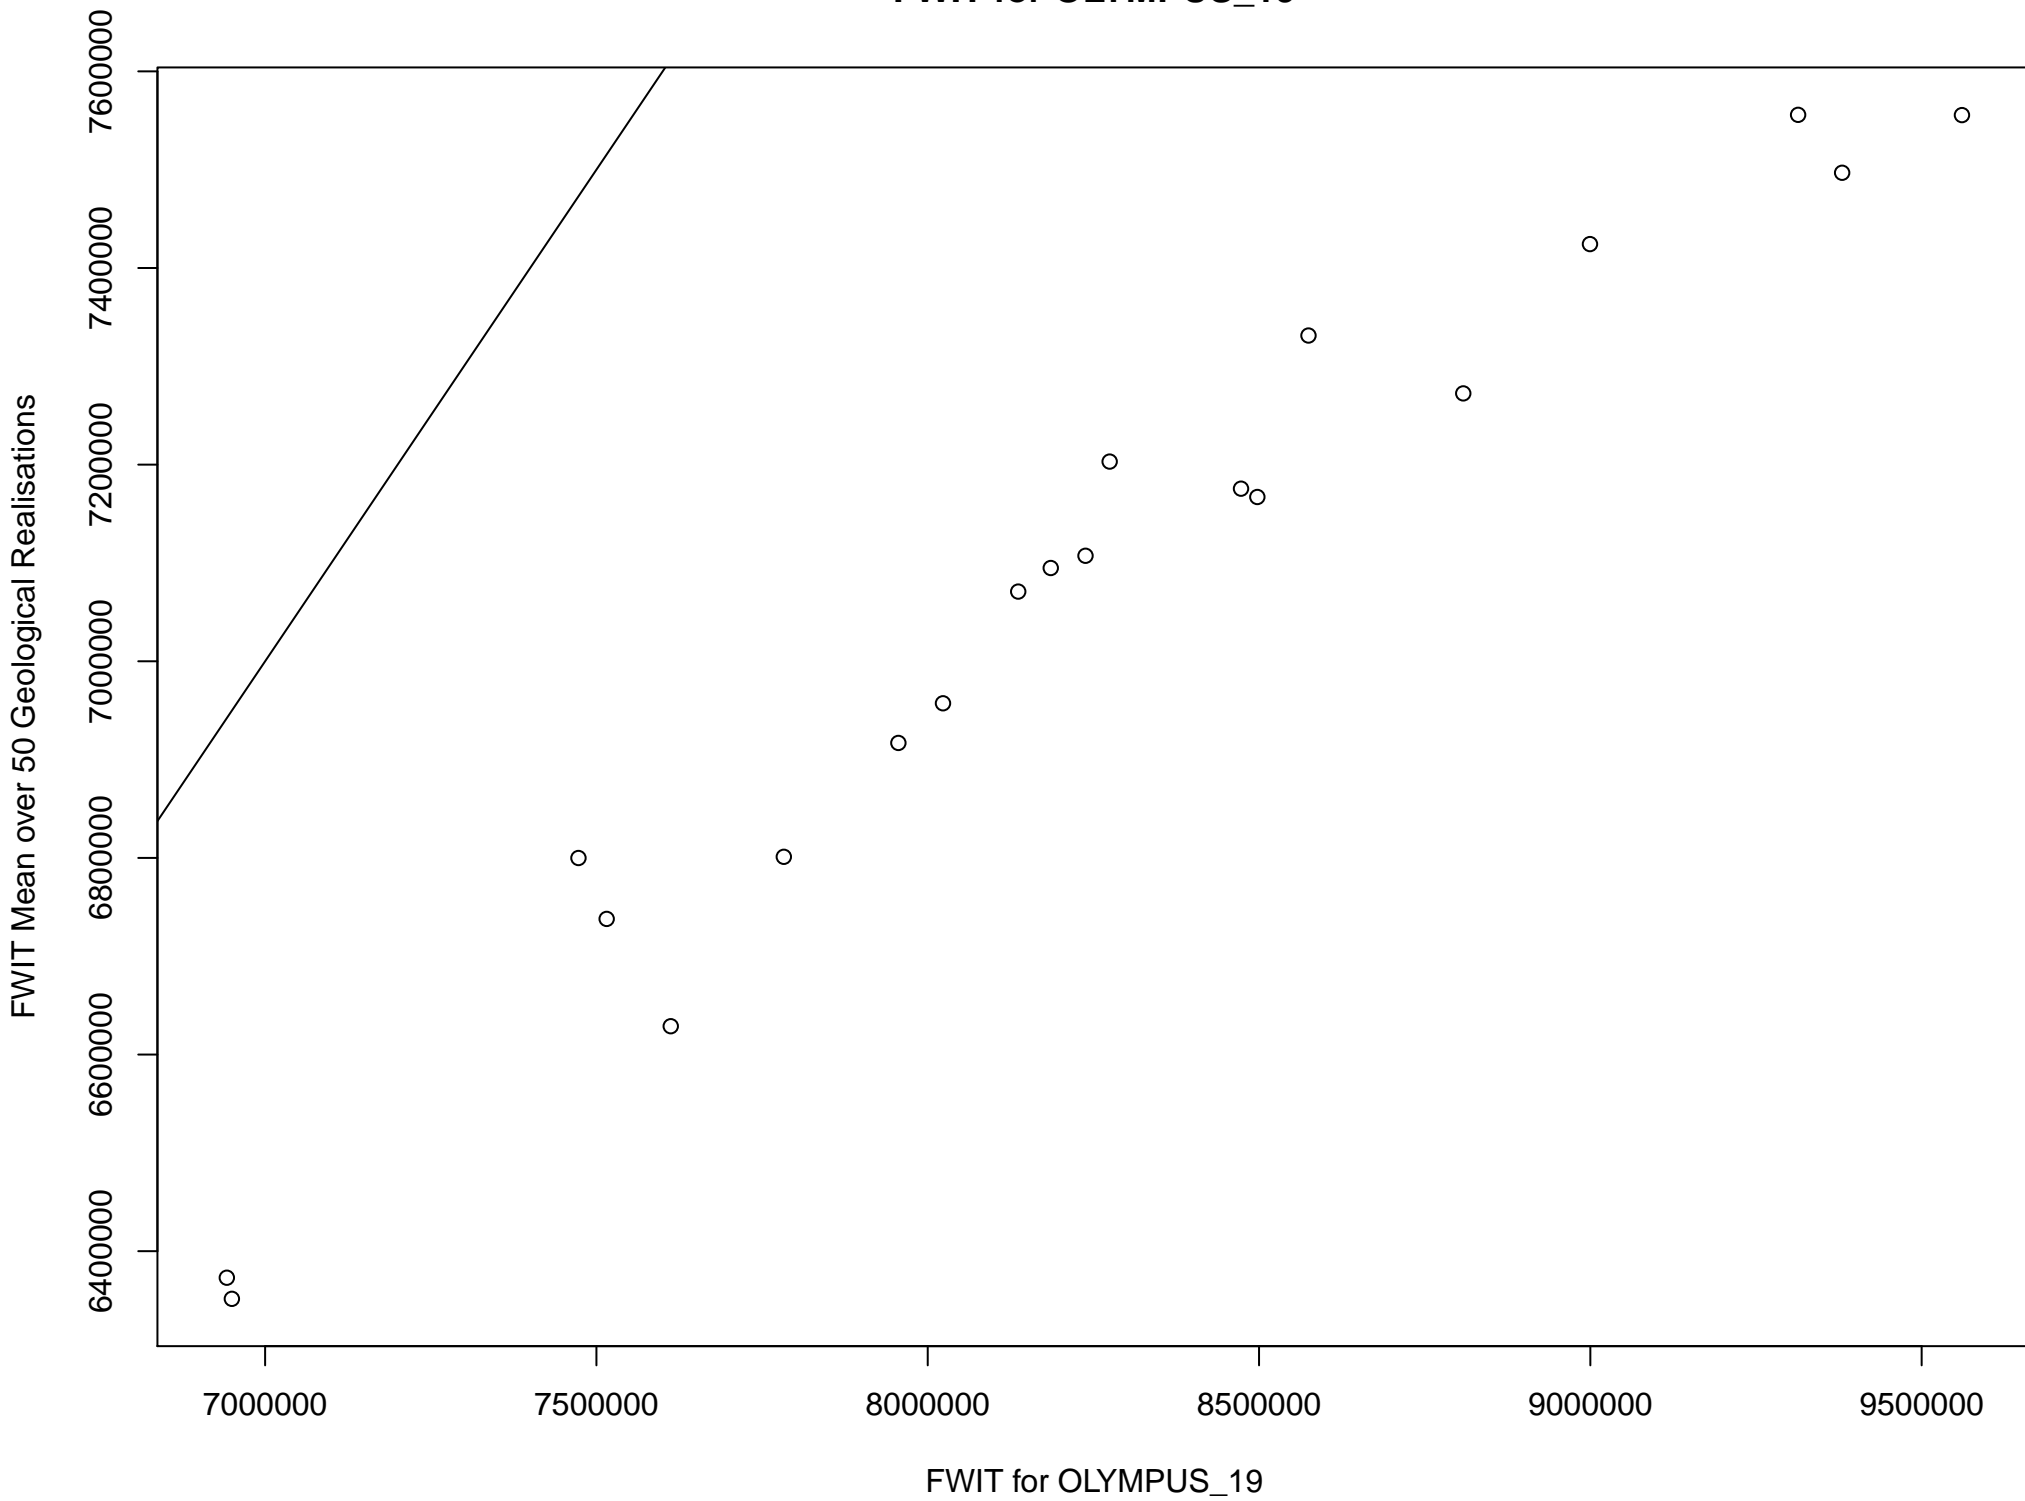

FWIT for OLYMPUS\_20

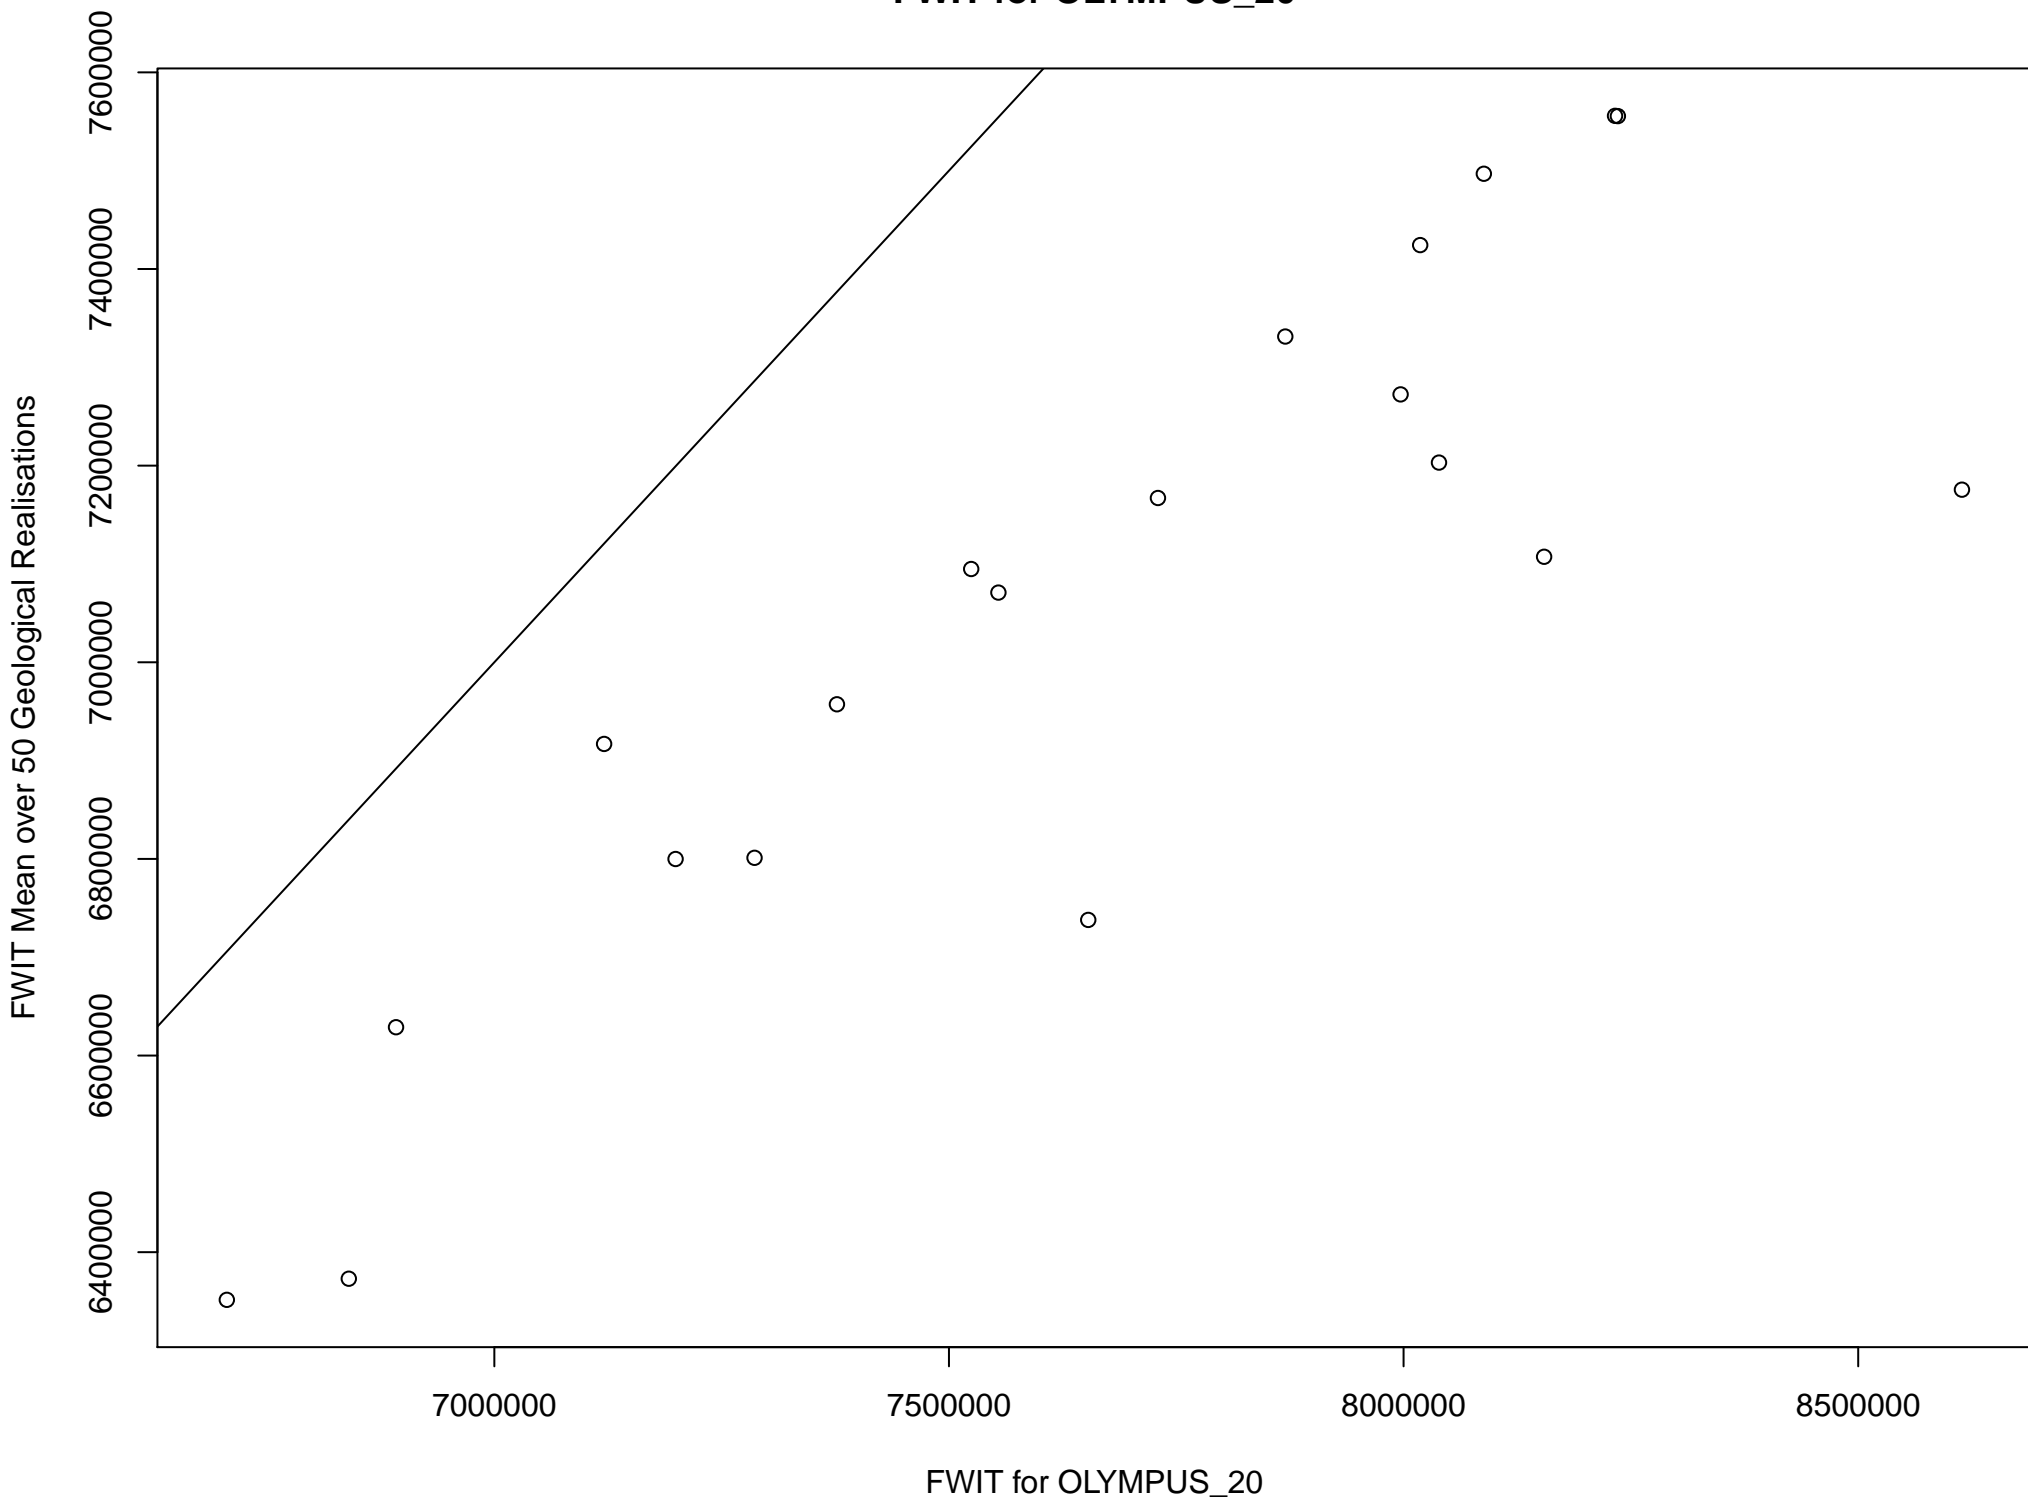

FWIT for OLYMPUS\_21

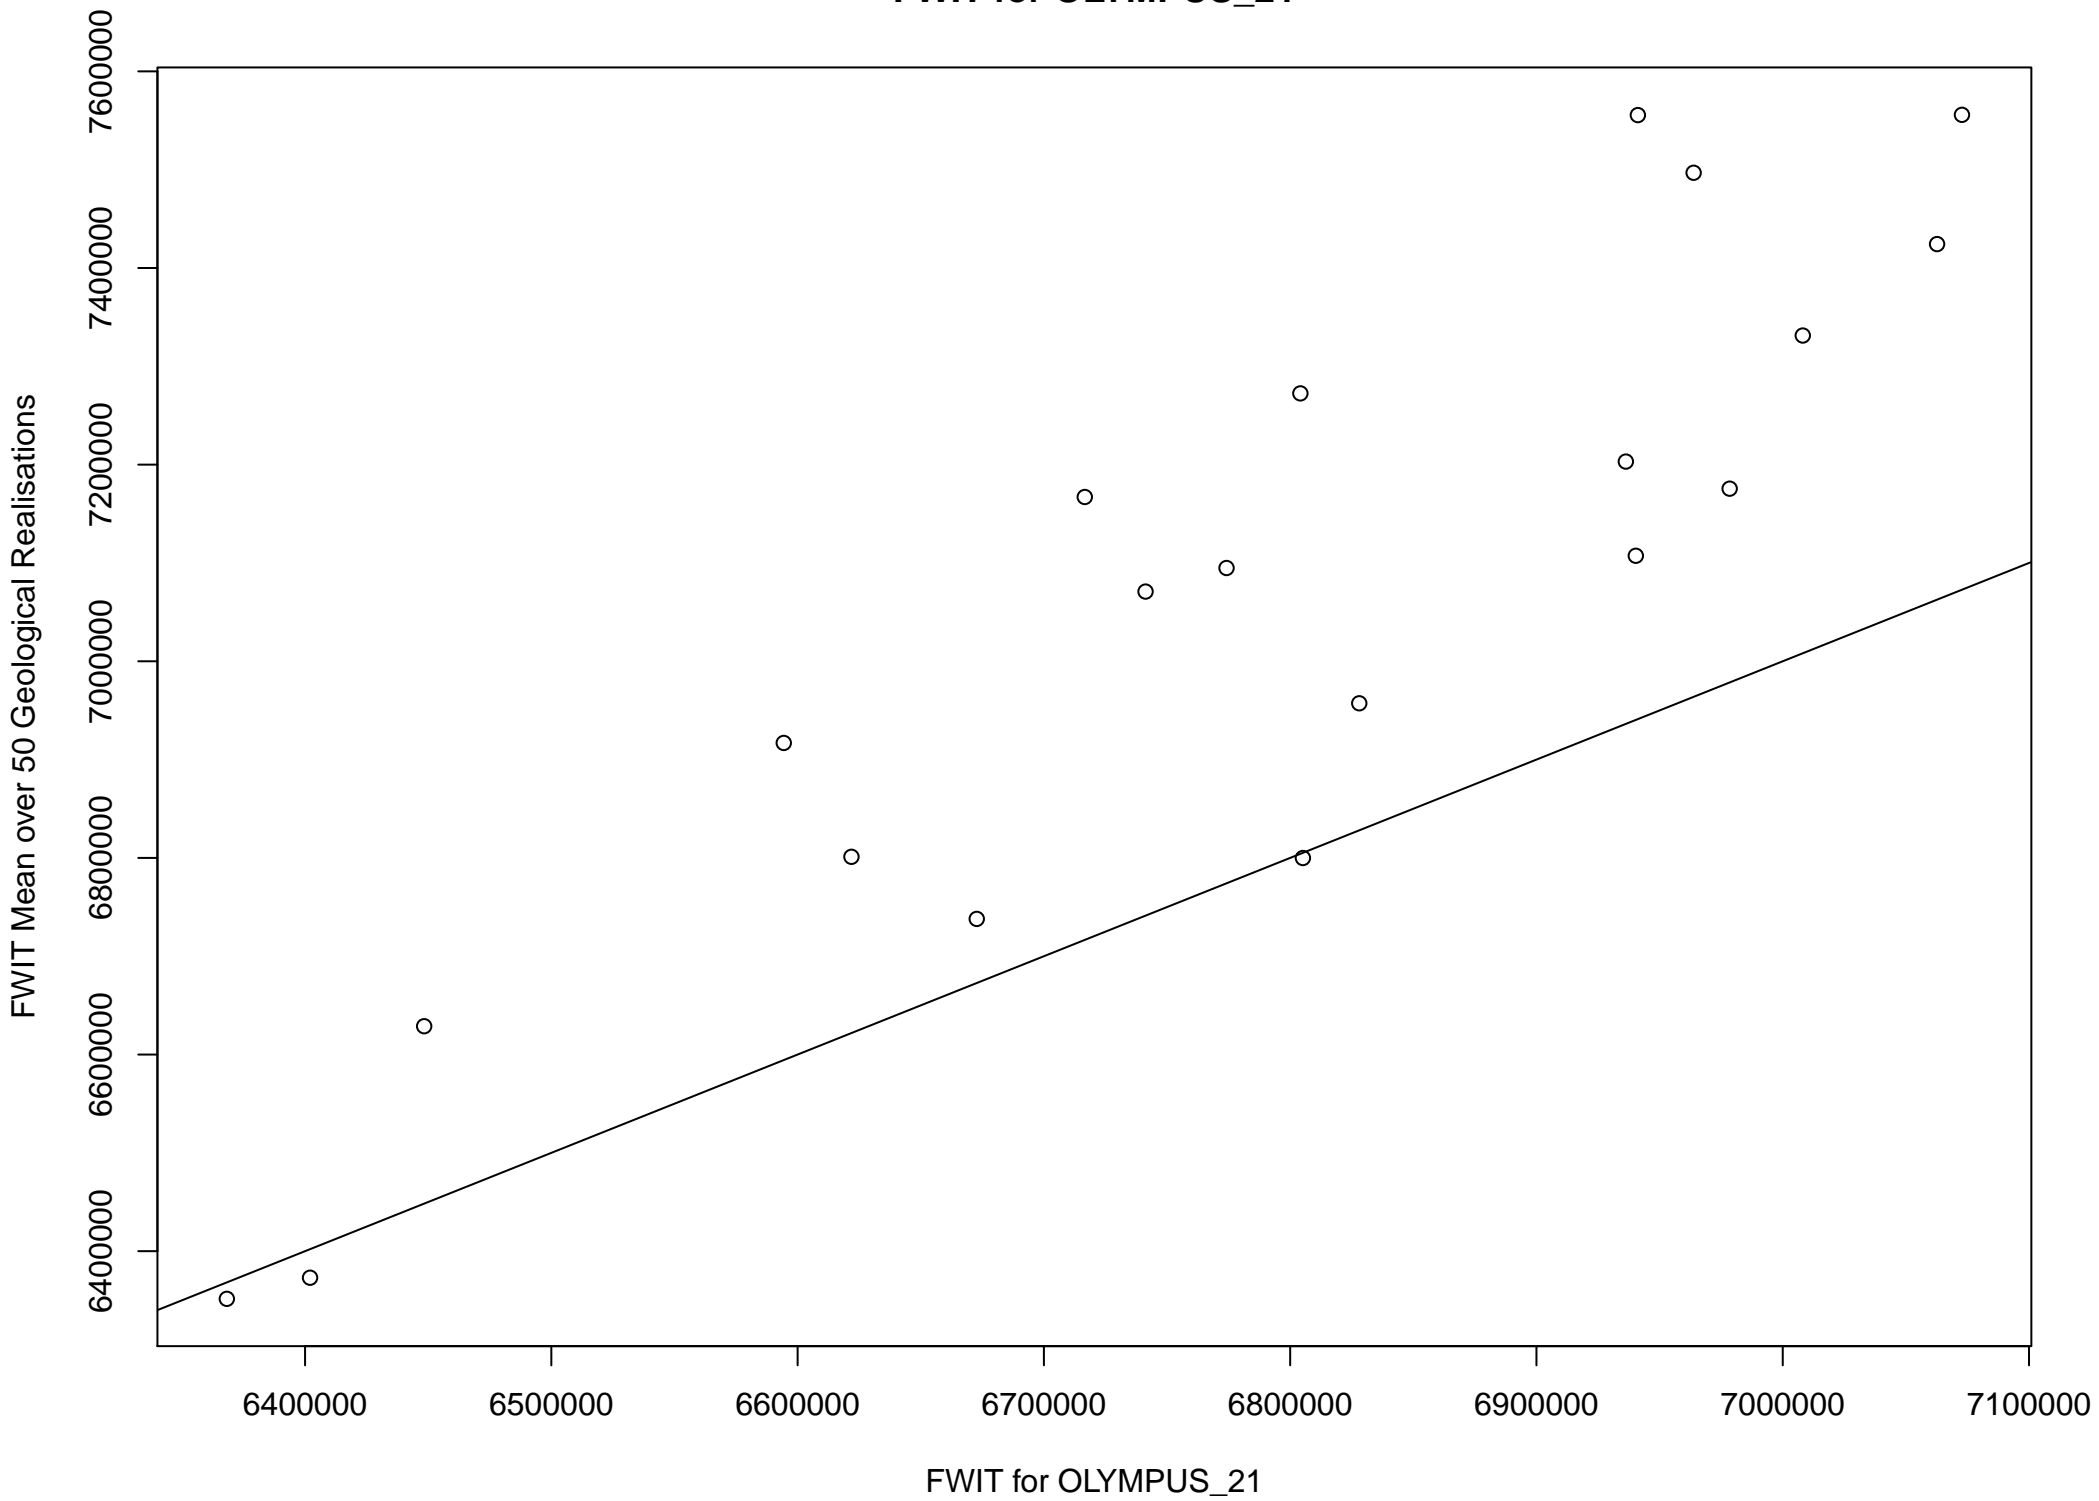

FWIT for OLYMPUS\_22

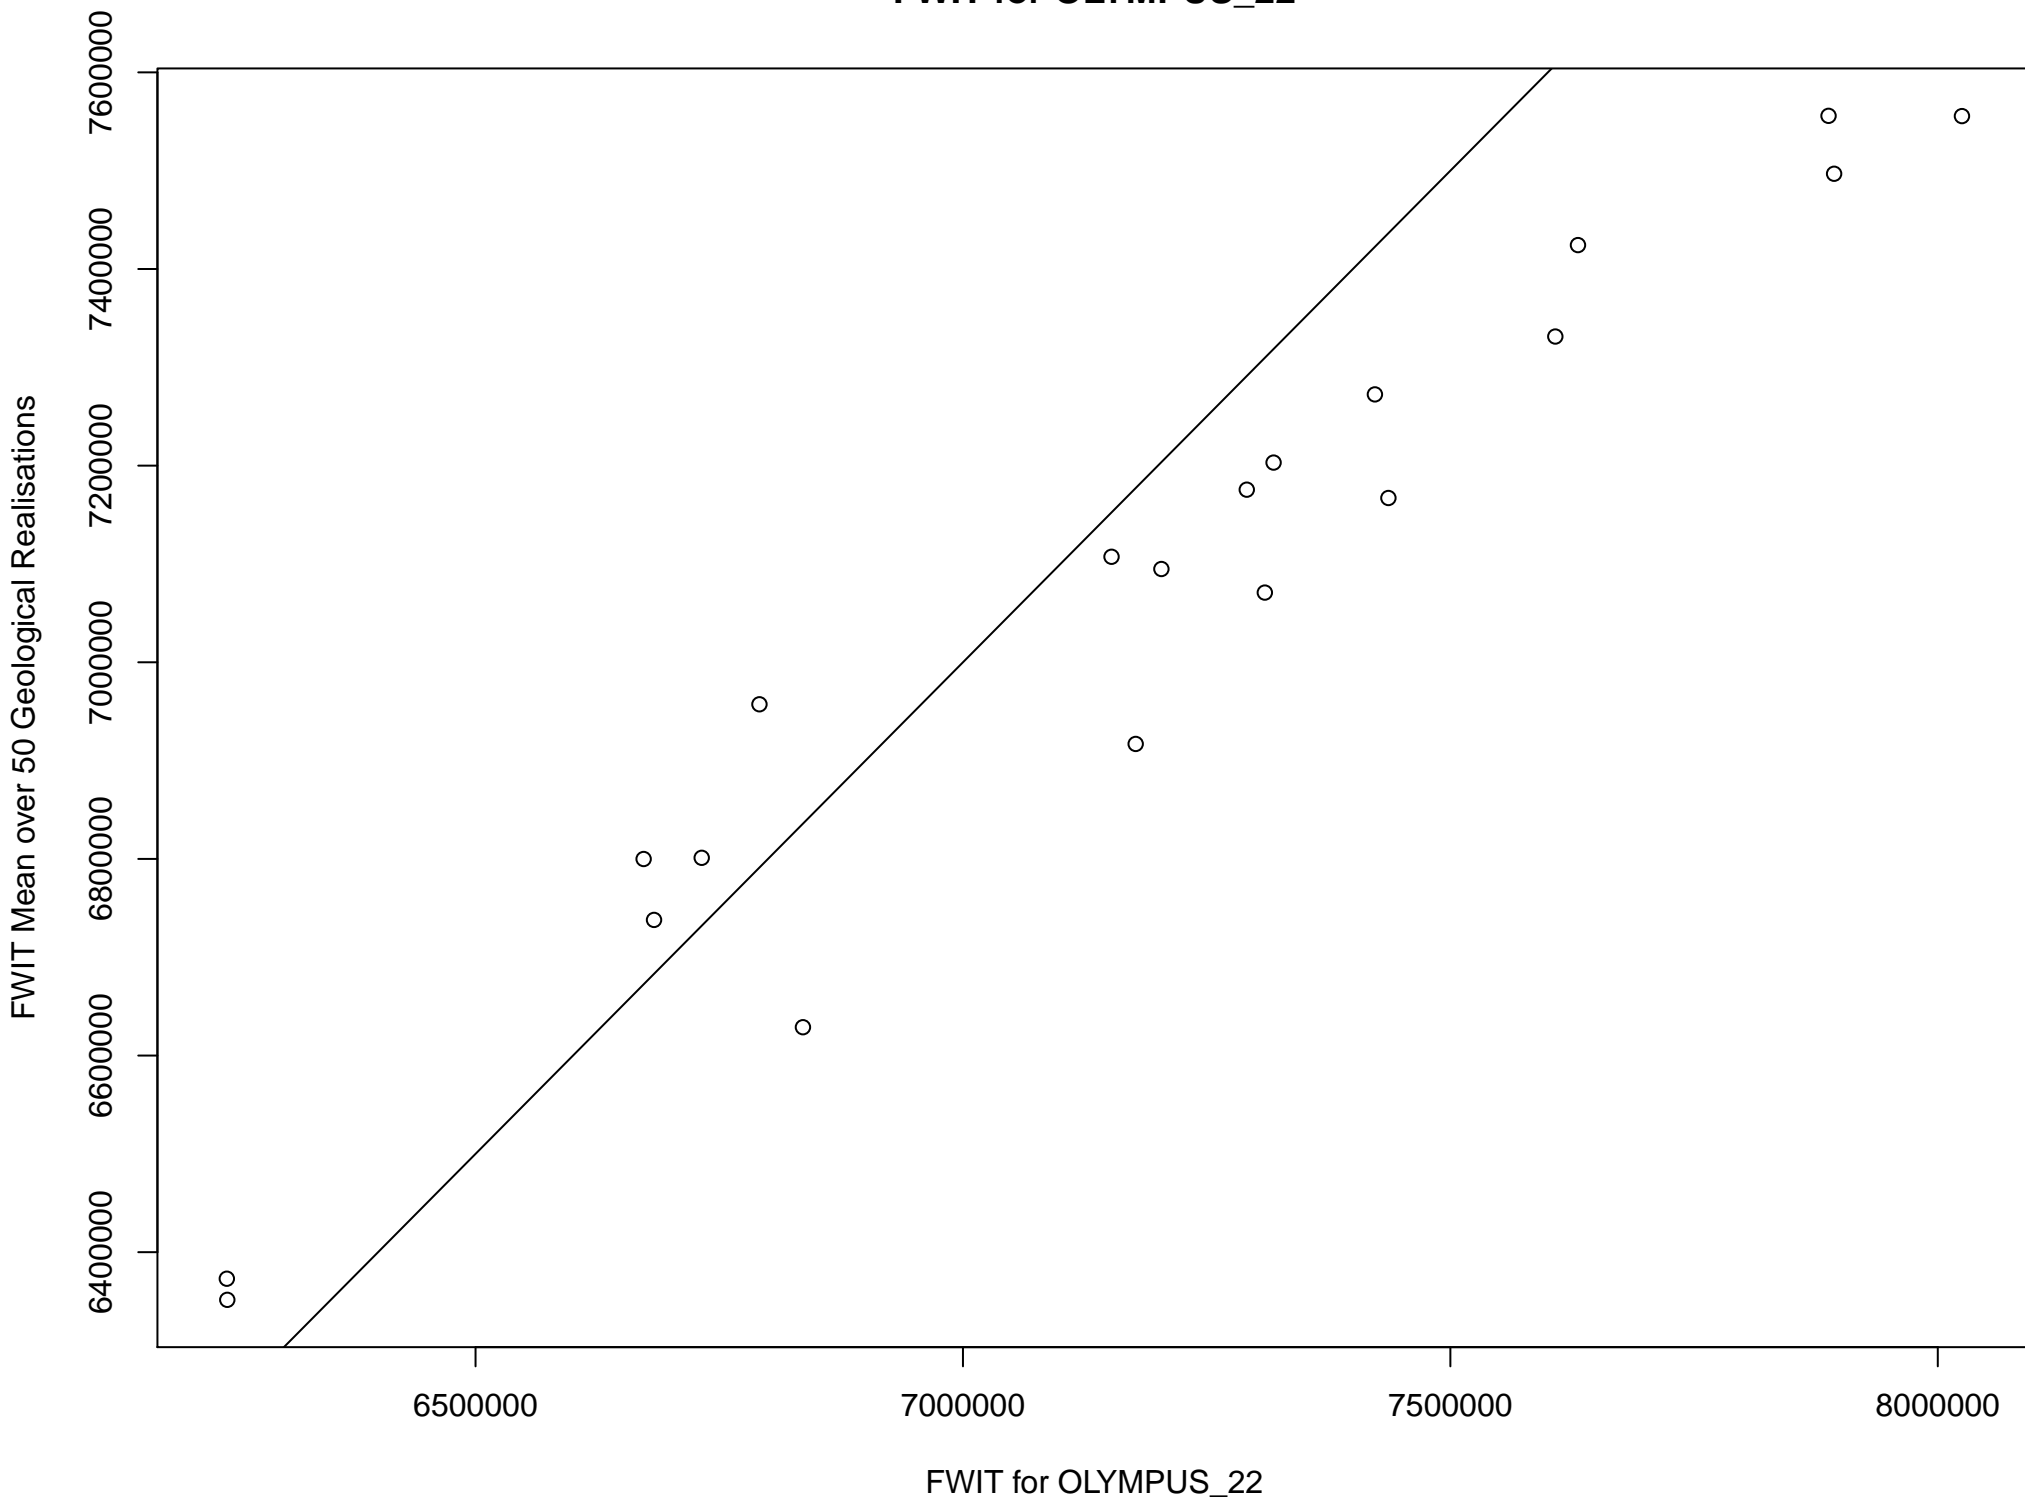

FWIT for OLYMPUS\_23

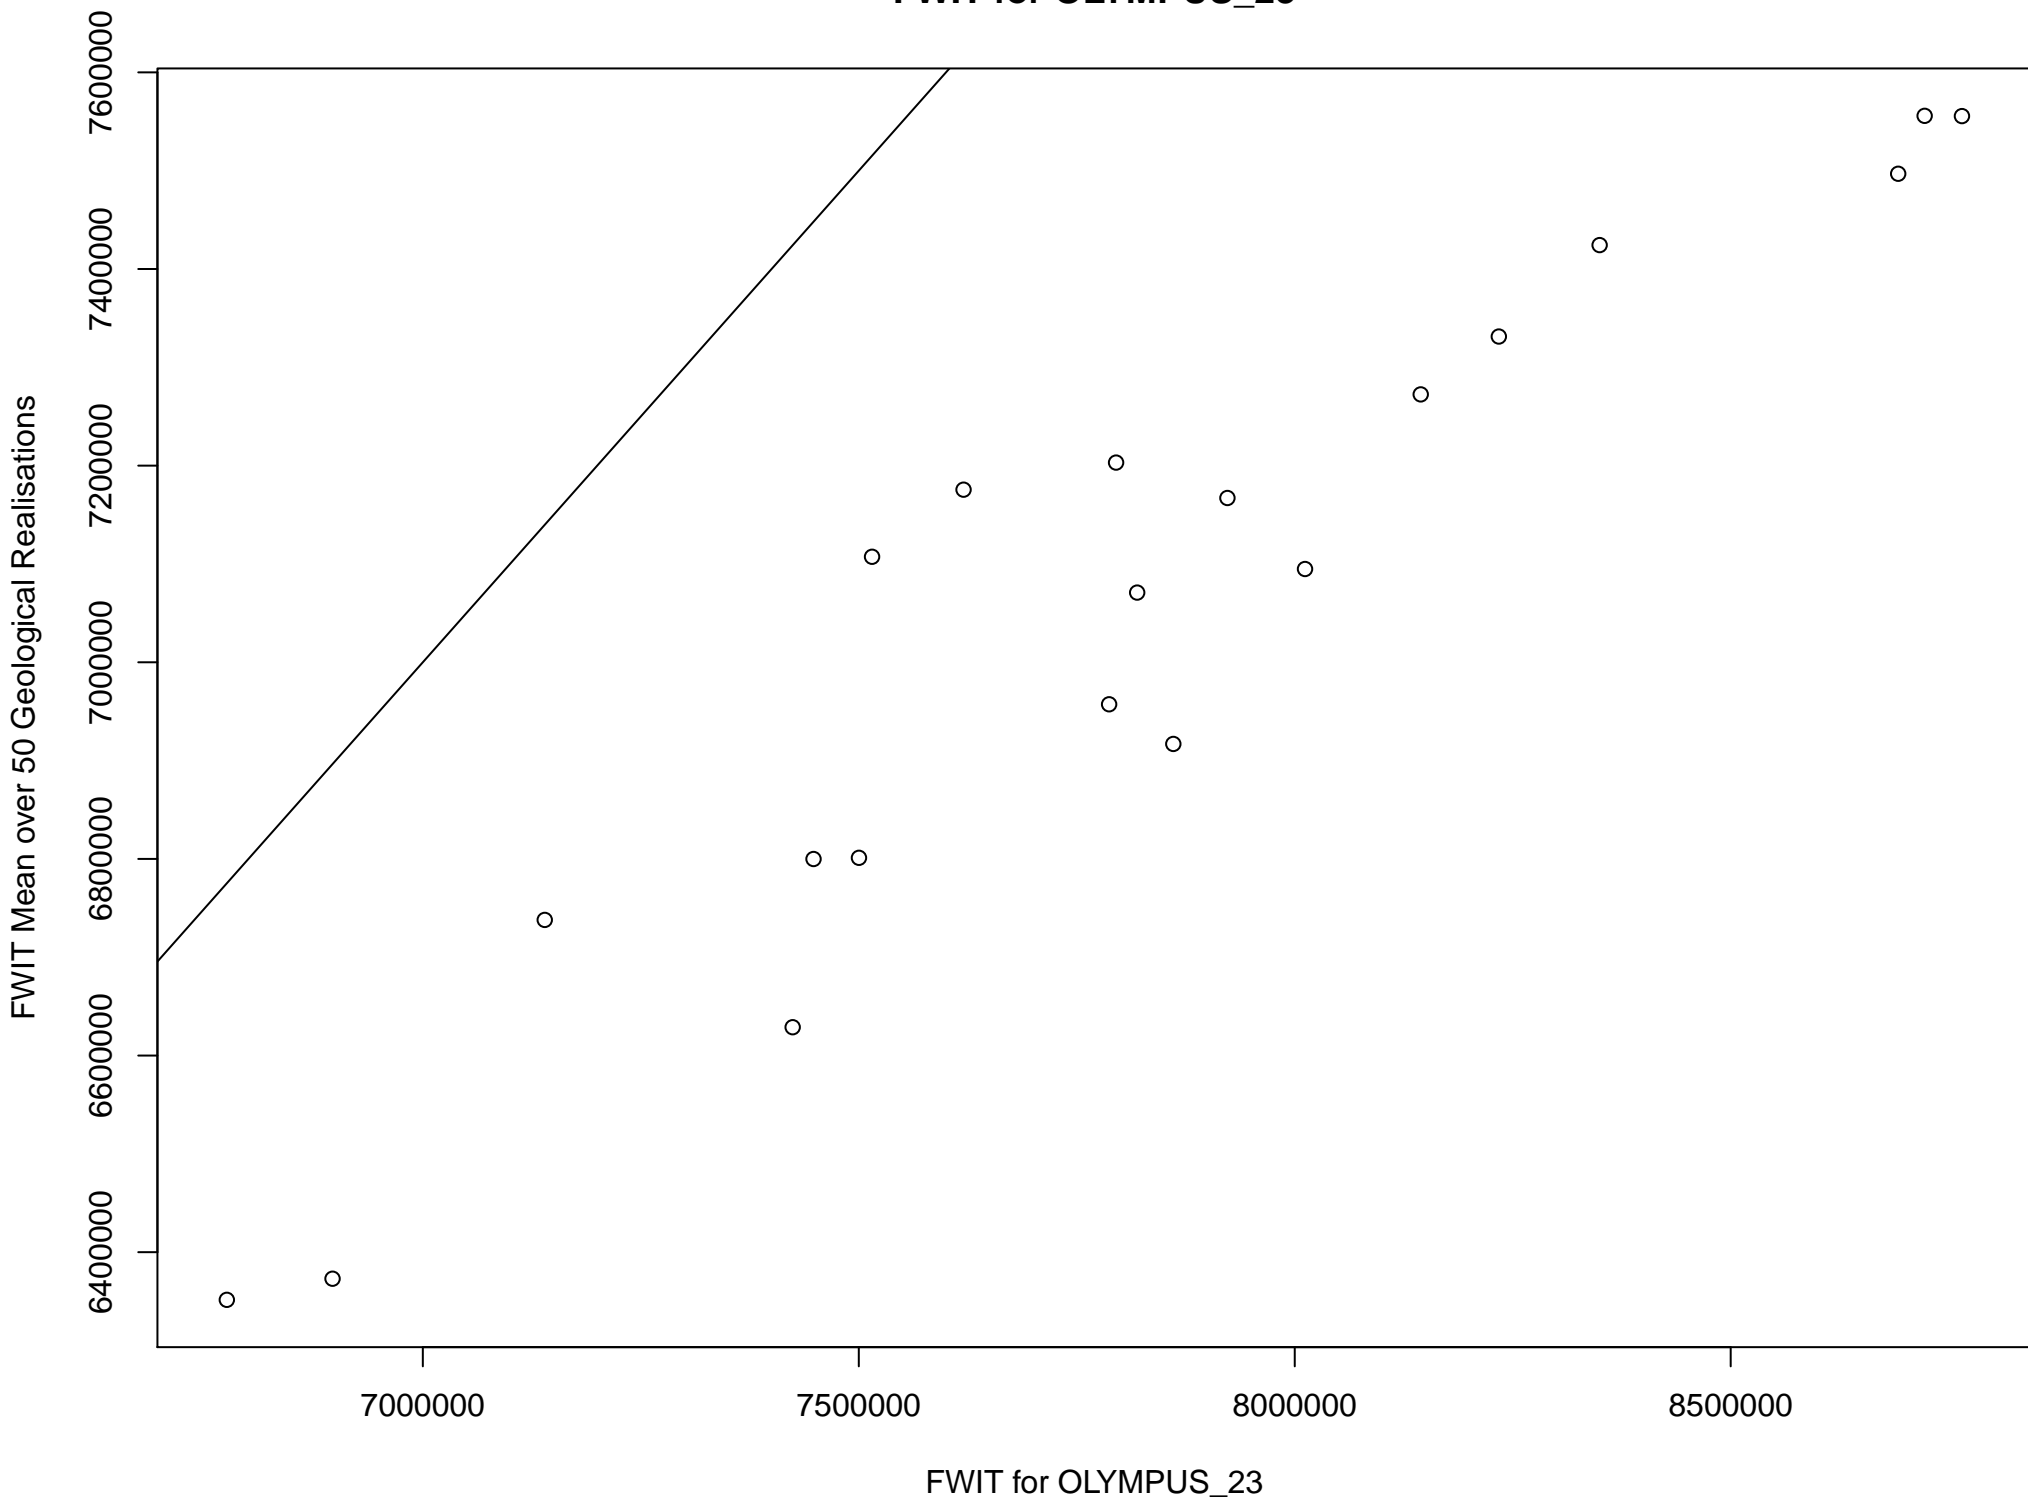

FWIT for OLYMPUS\_24

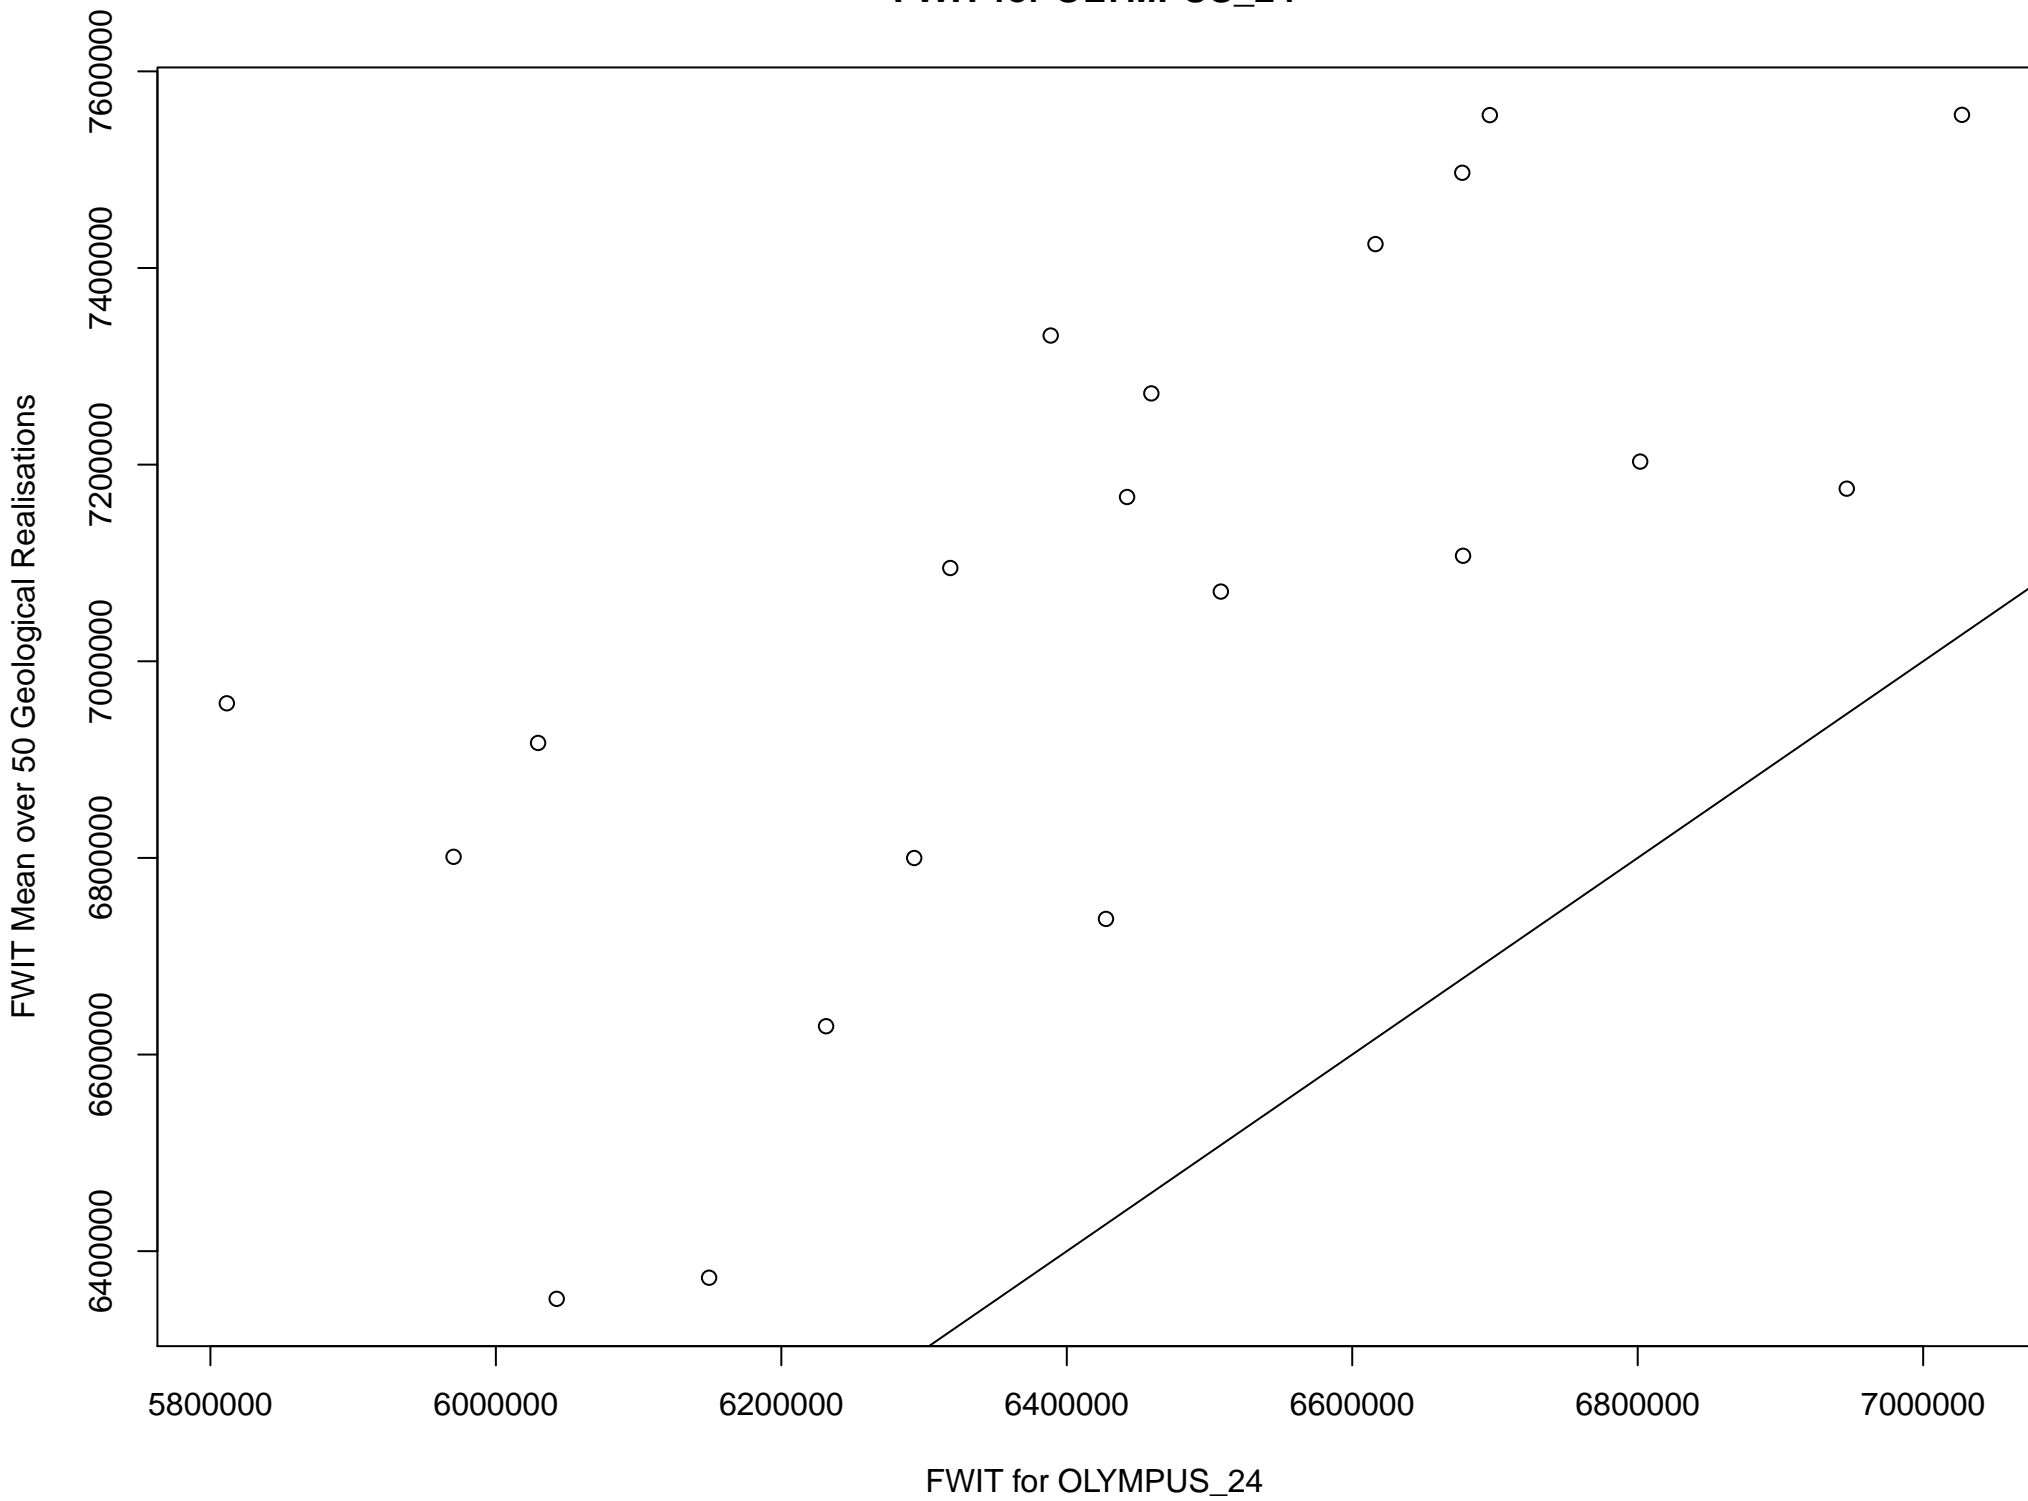



FWIT for OLYMPUS\_25

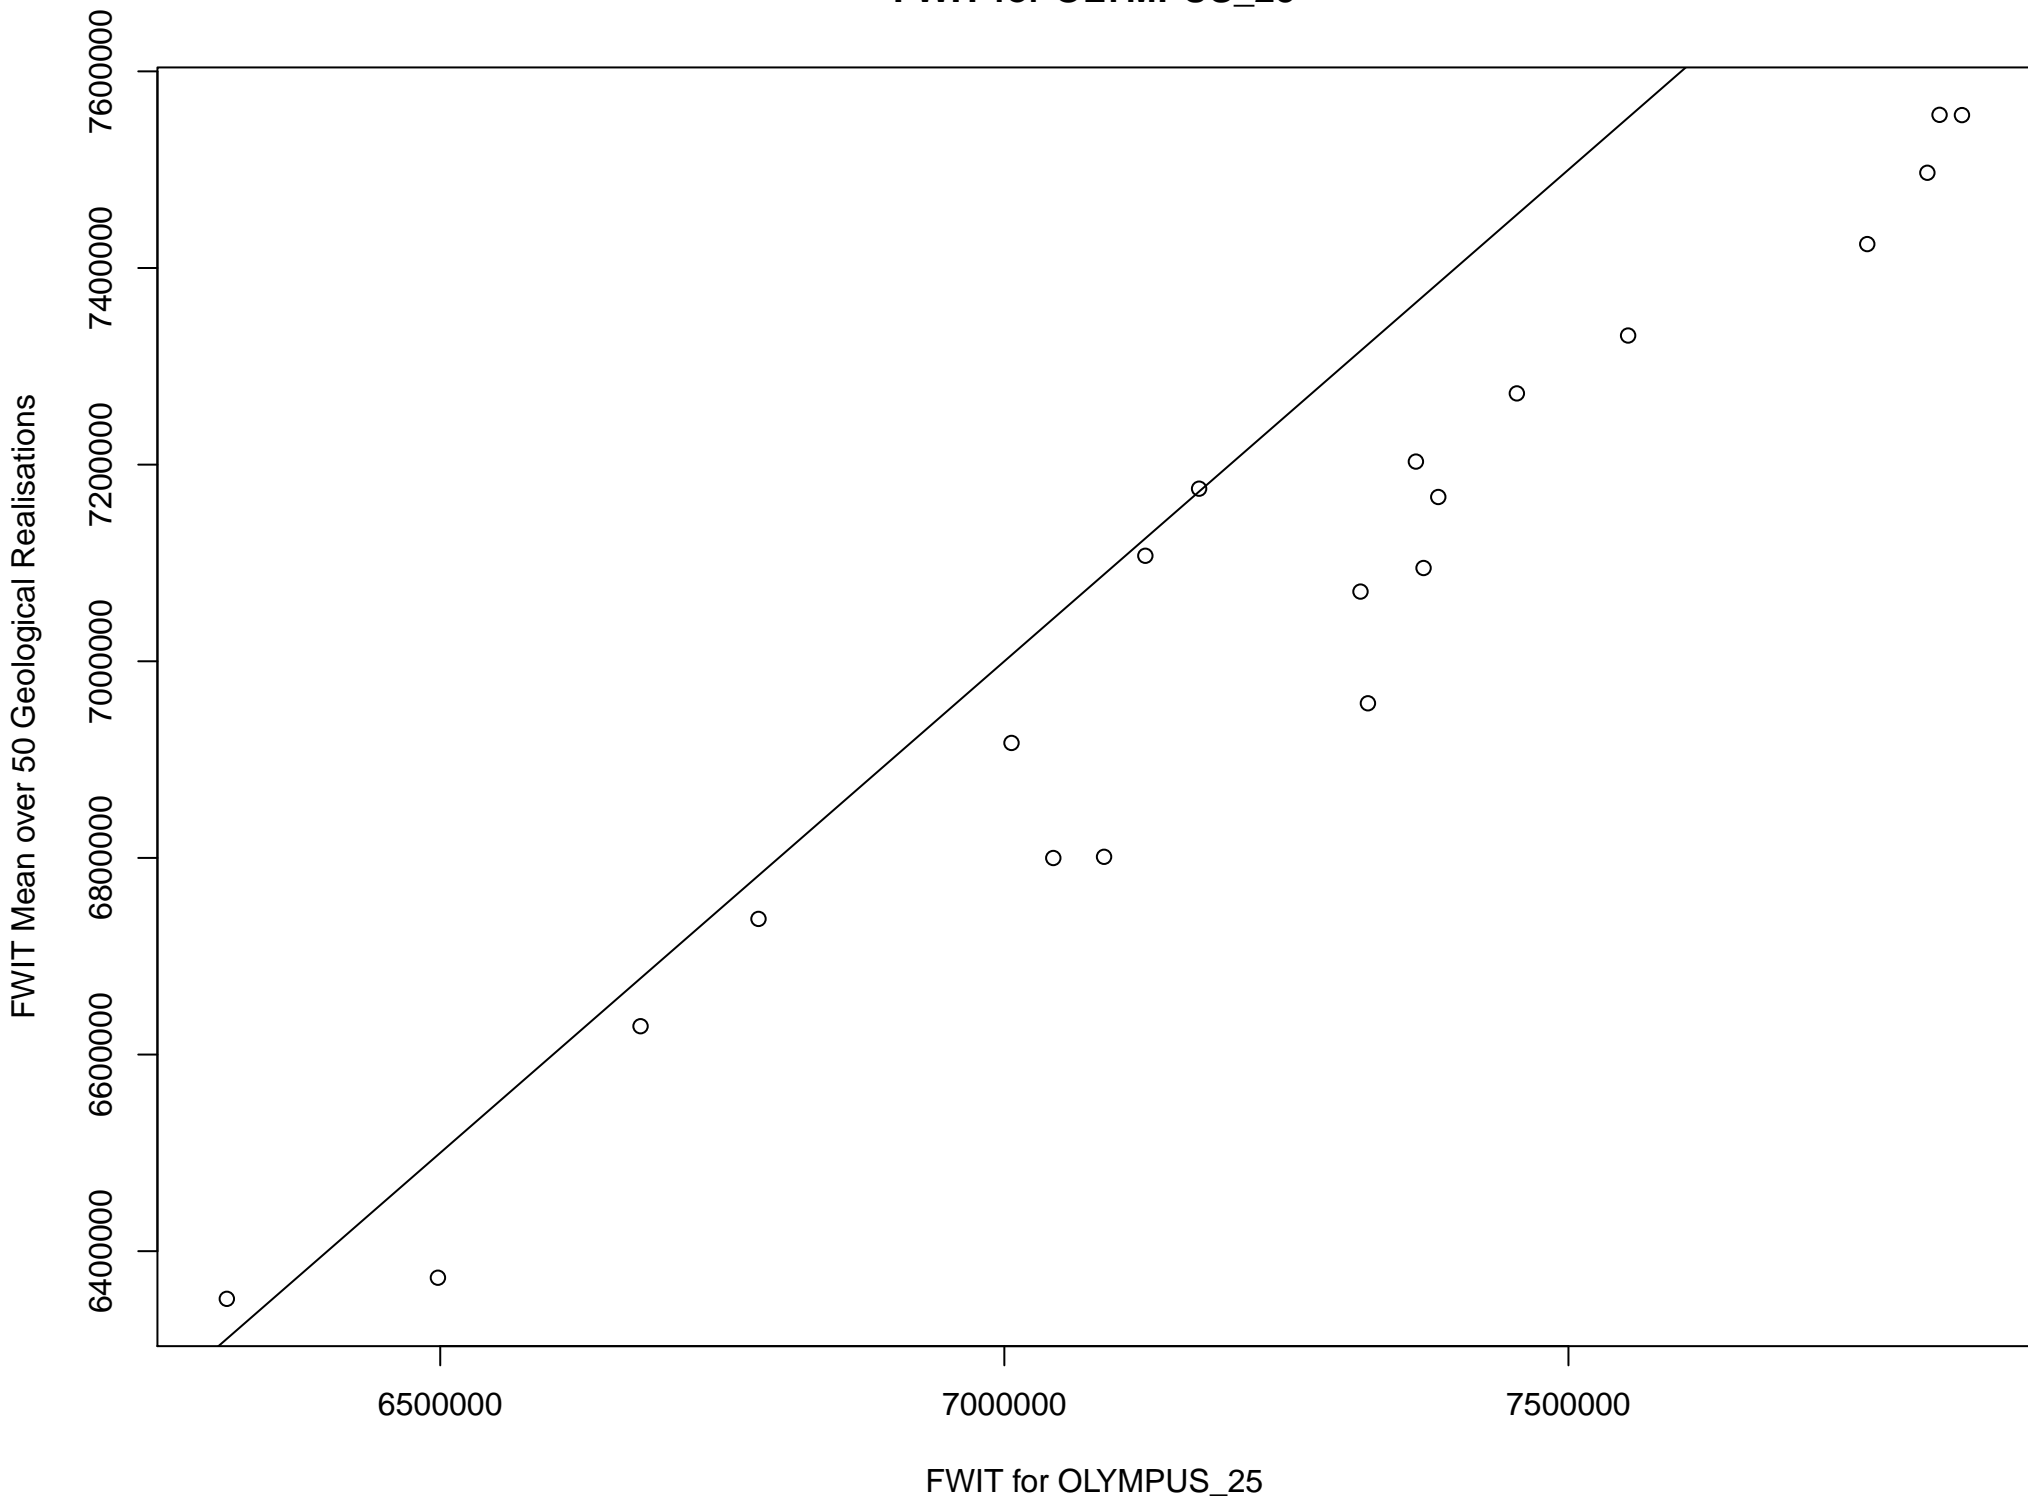

FWIT for OLYMPUS\_26

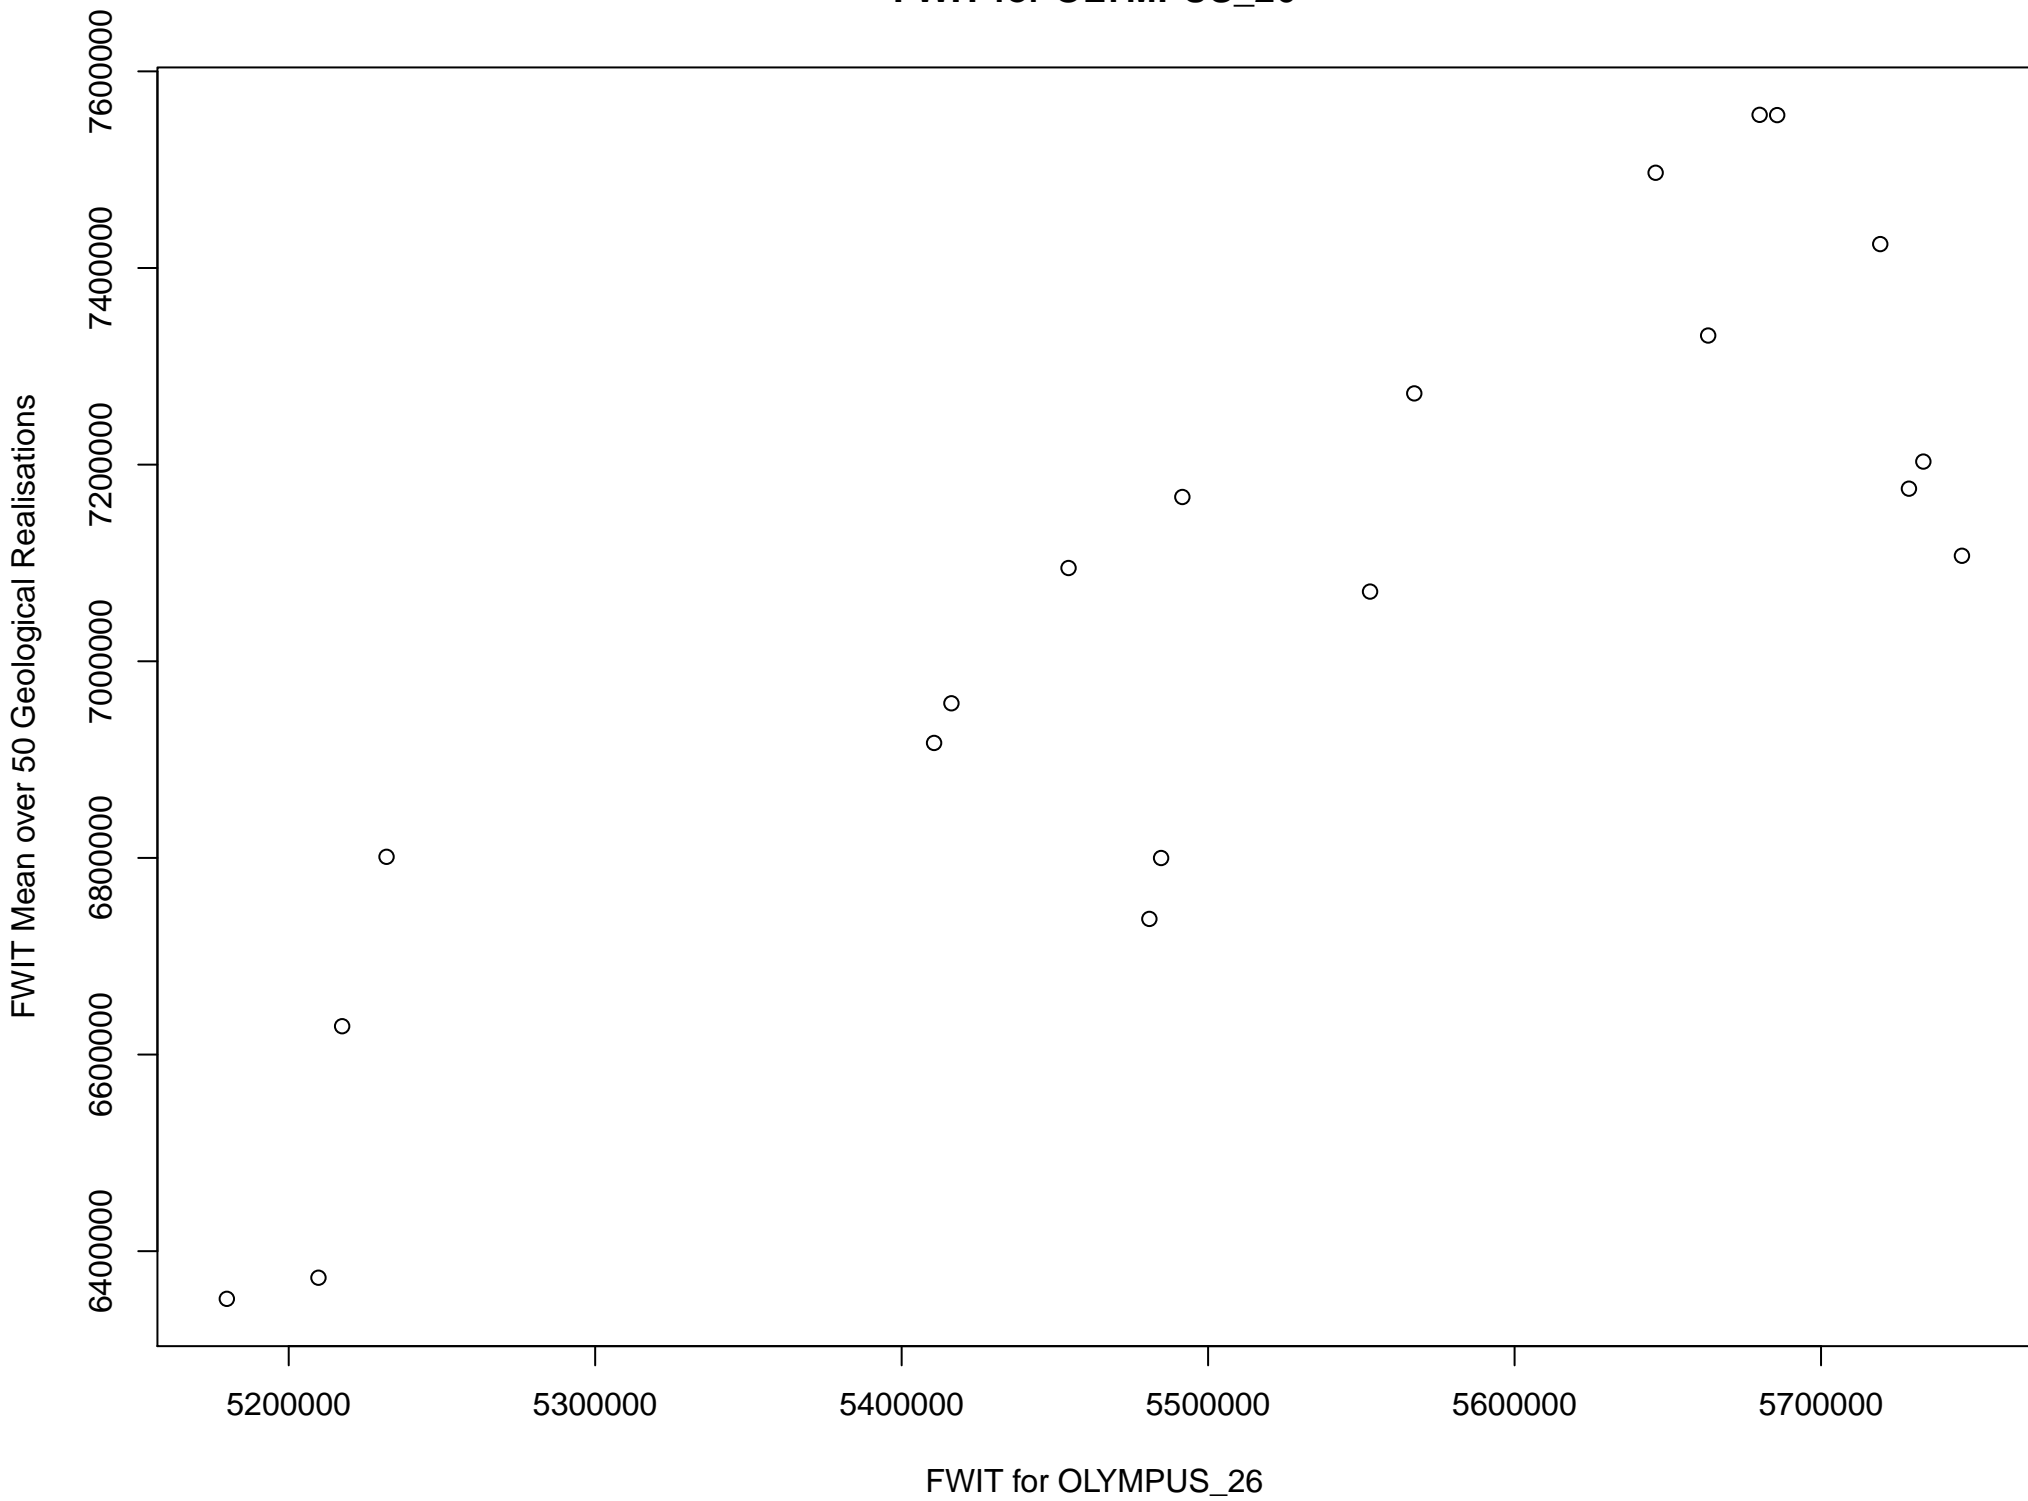

FWIT for OLYMPUS\_27

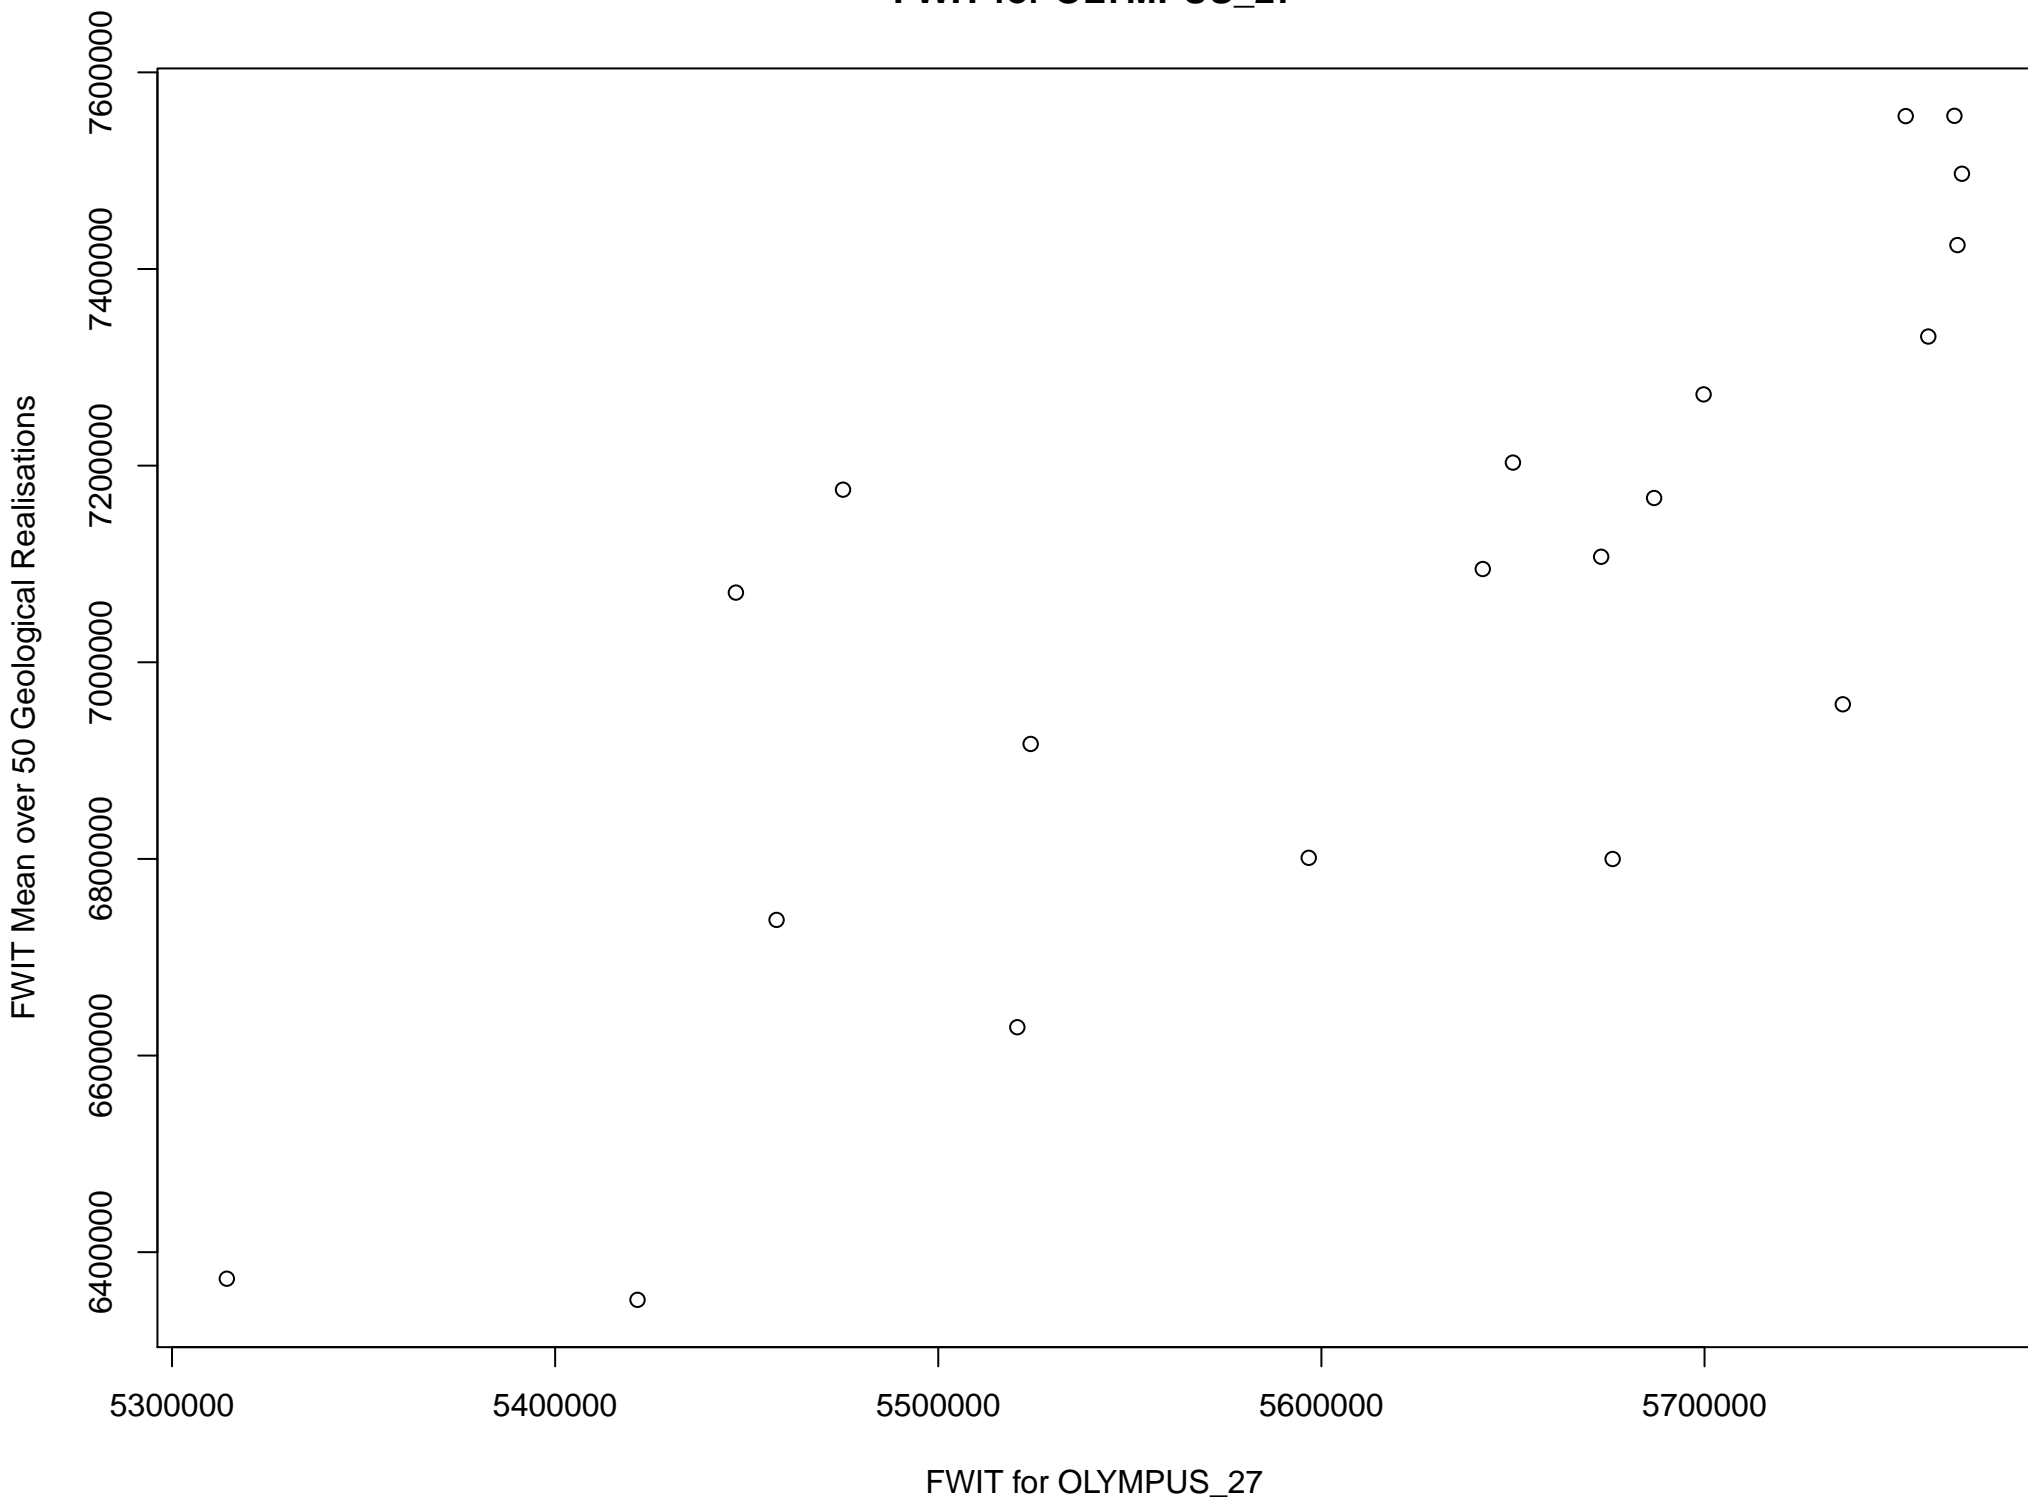

FWIT for OLYMPUS\_28

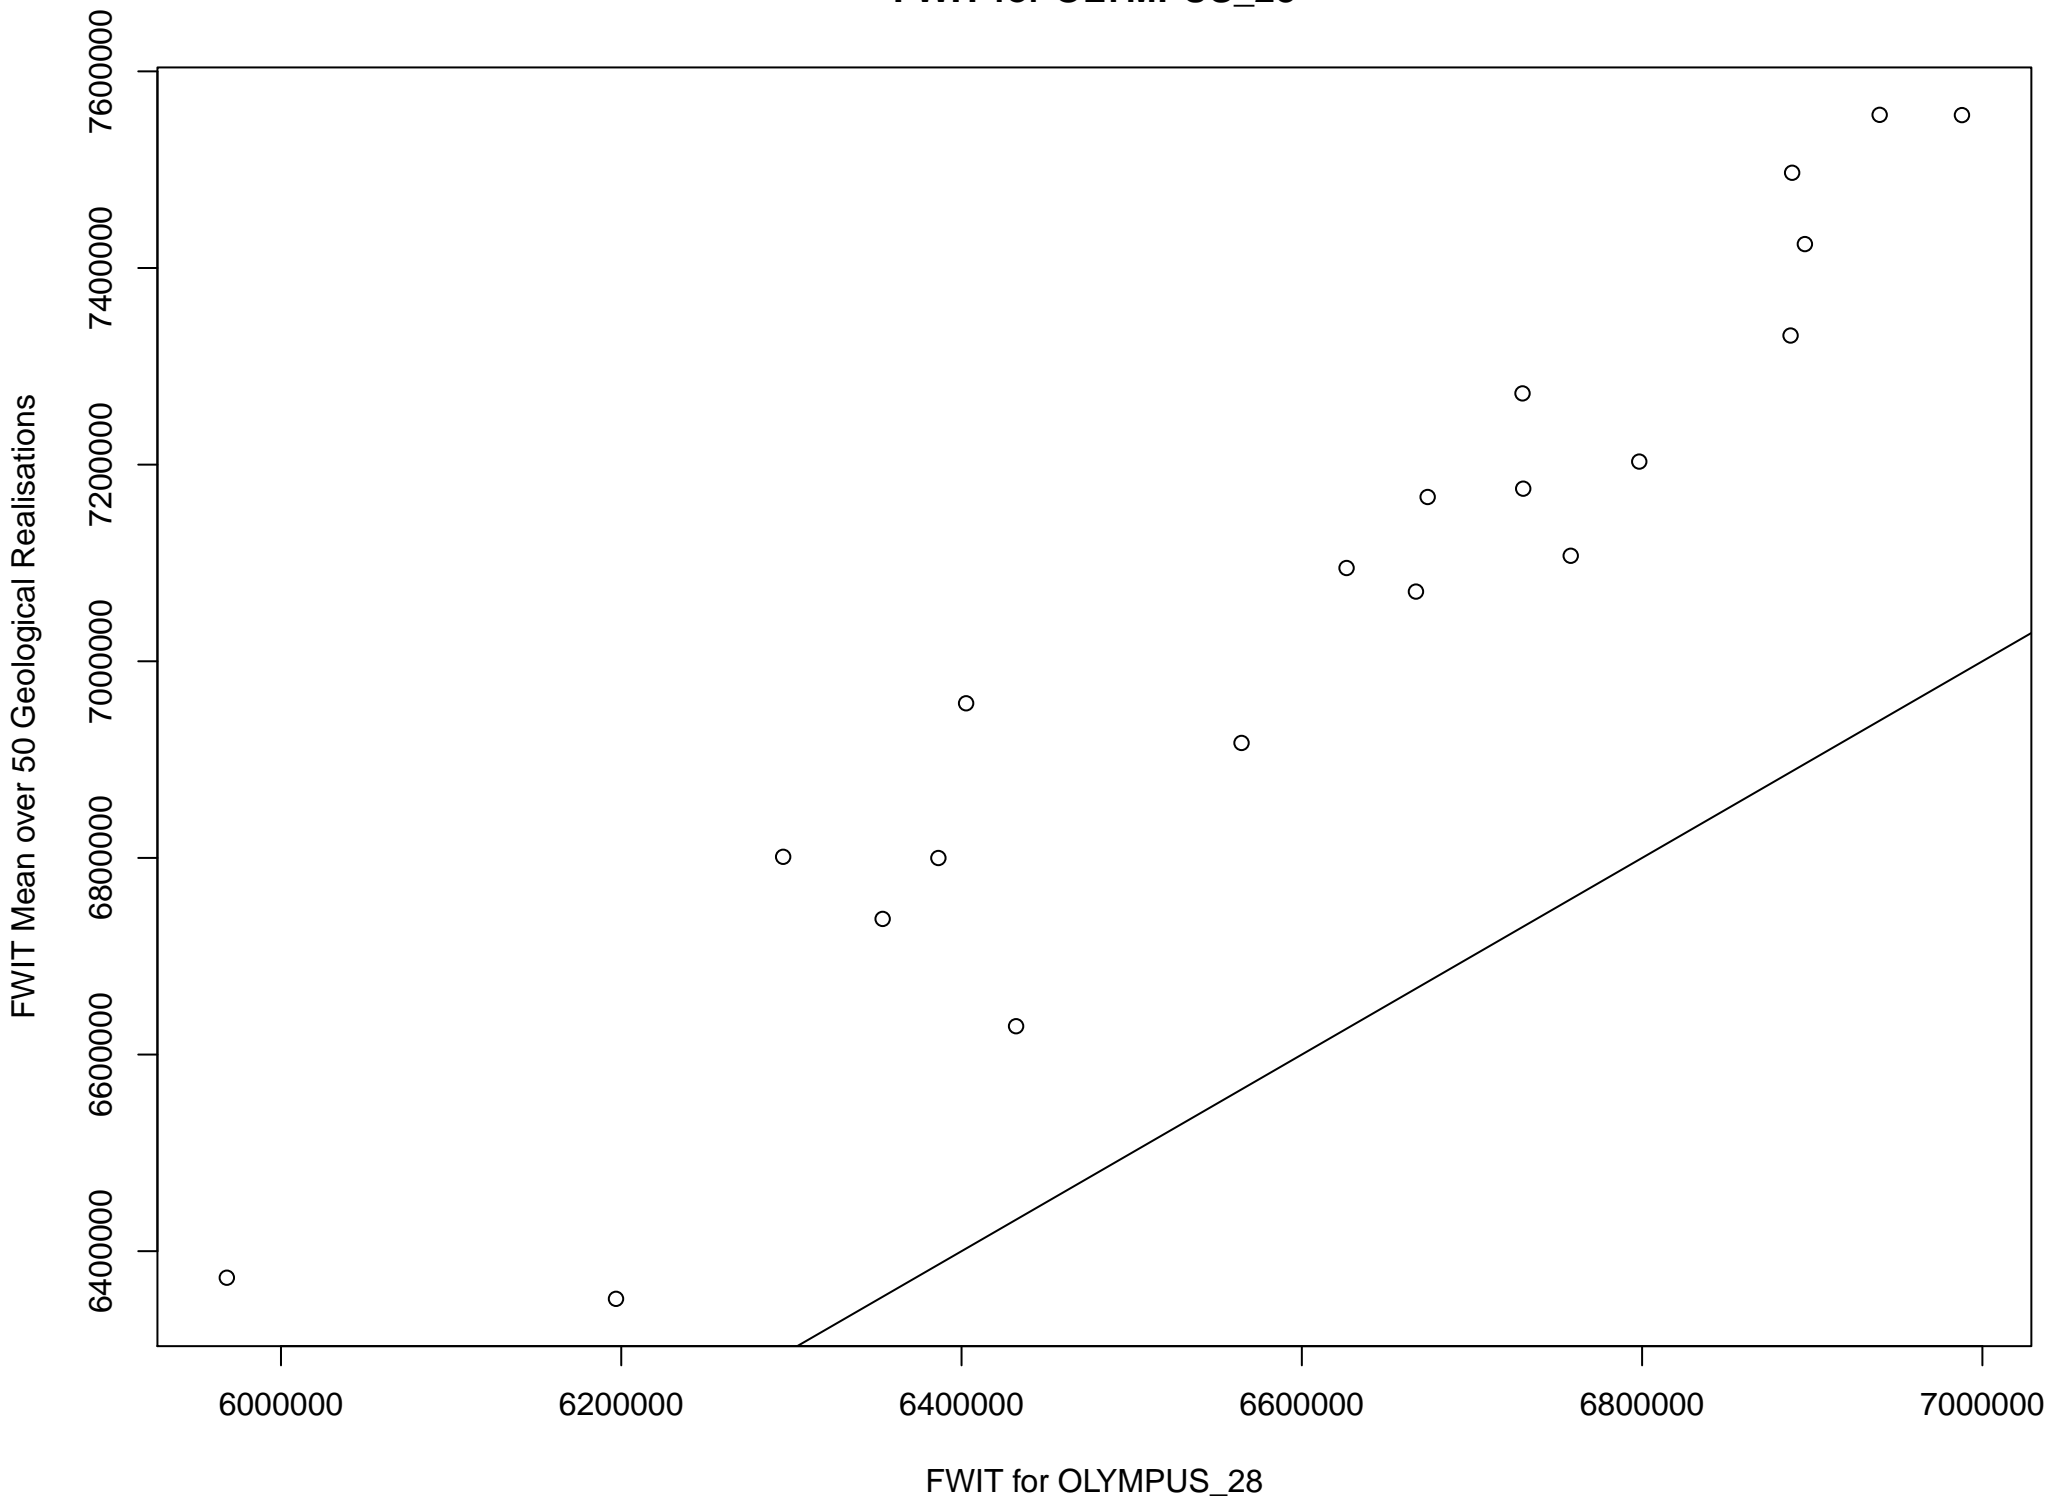

FWIT for OLYMPUS\_29

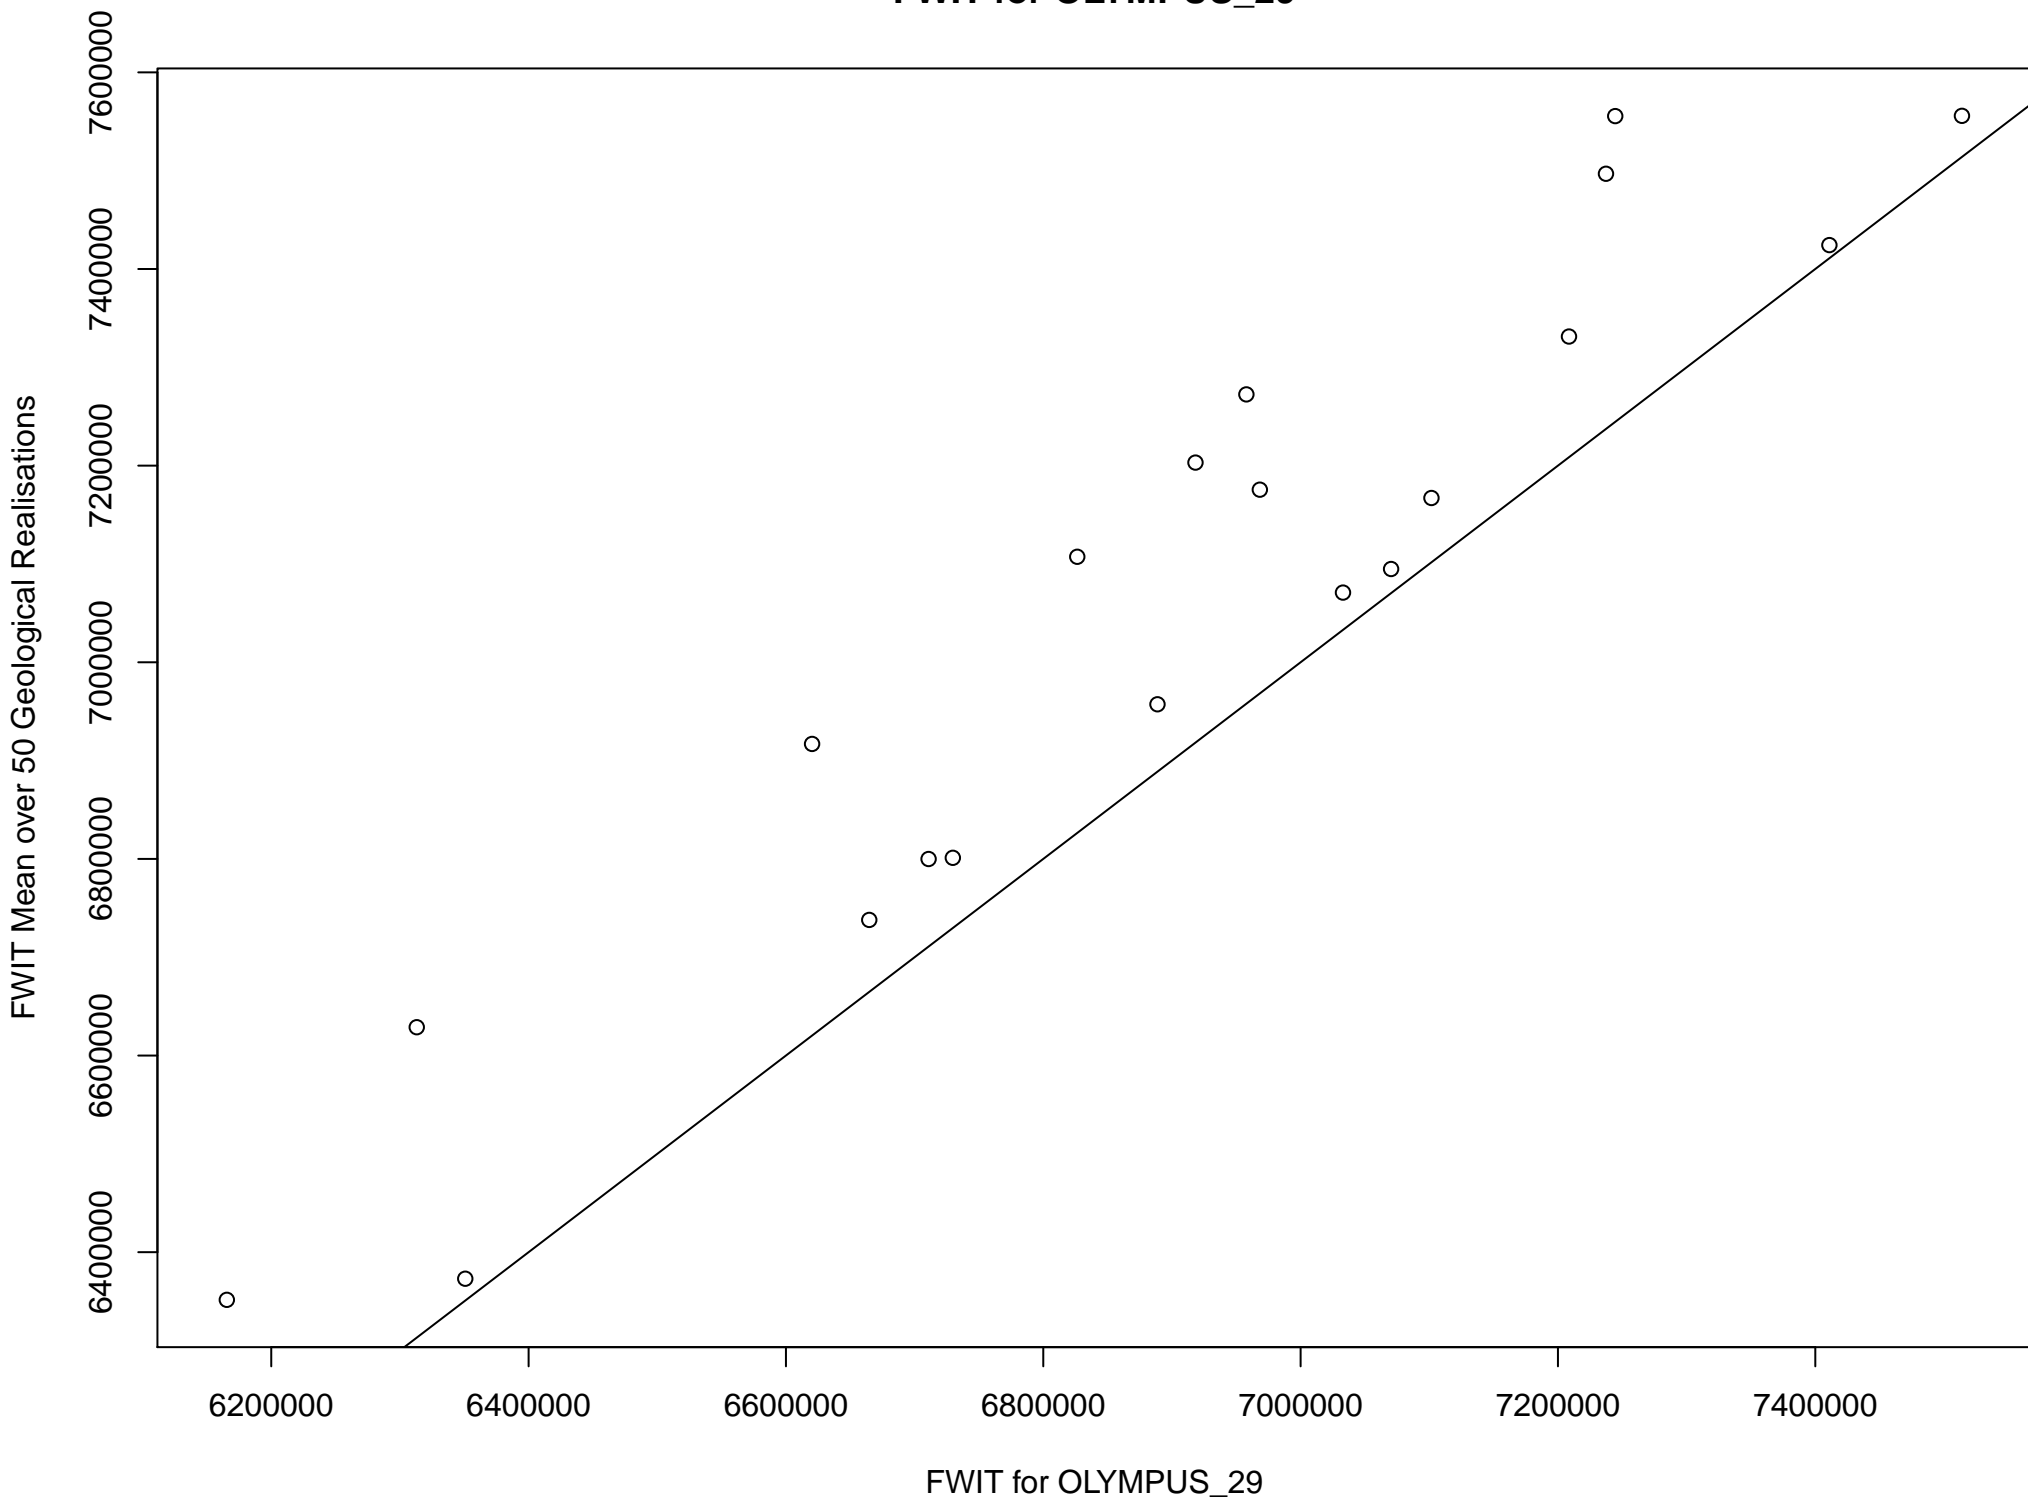

FWIT for OLYMPUS\_30

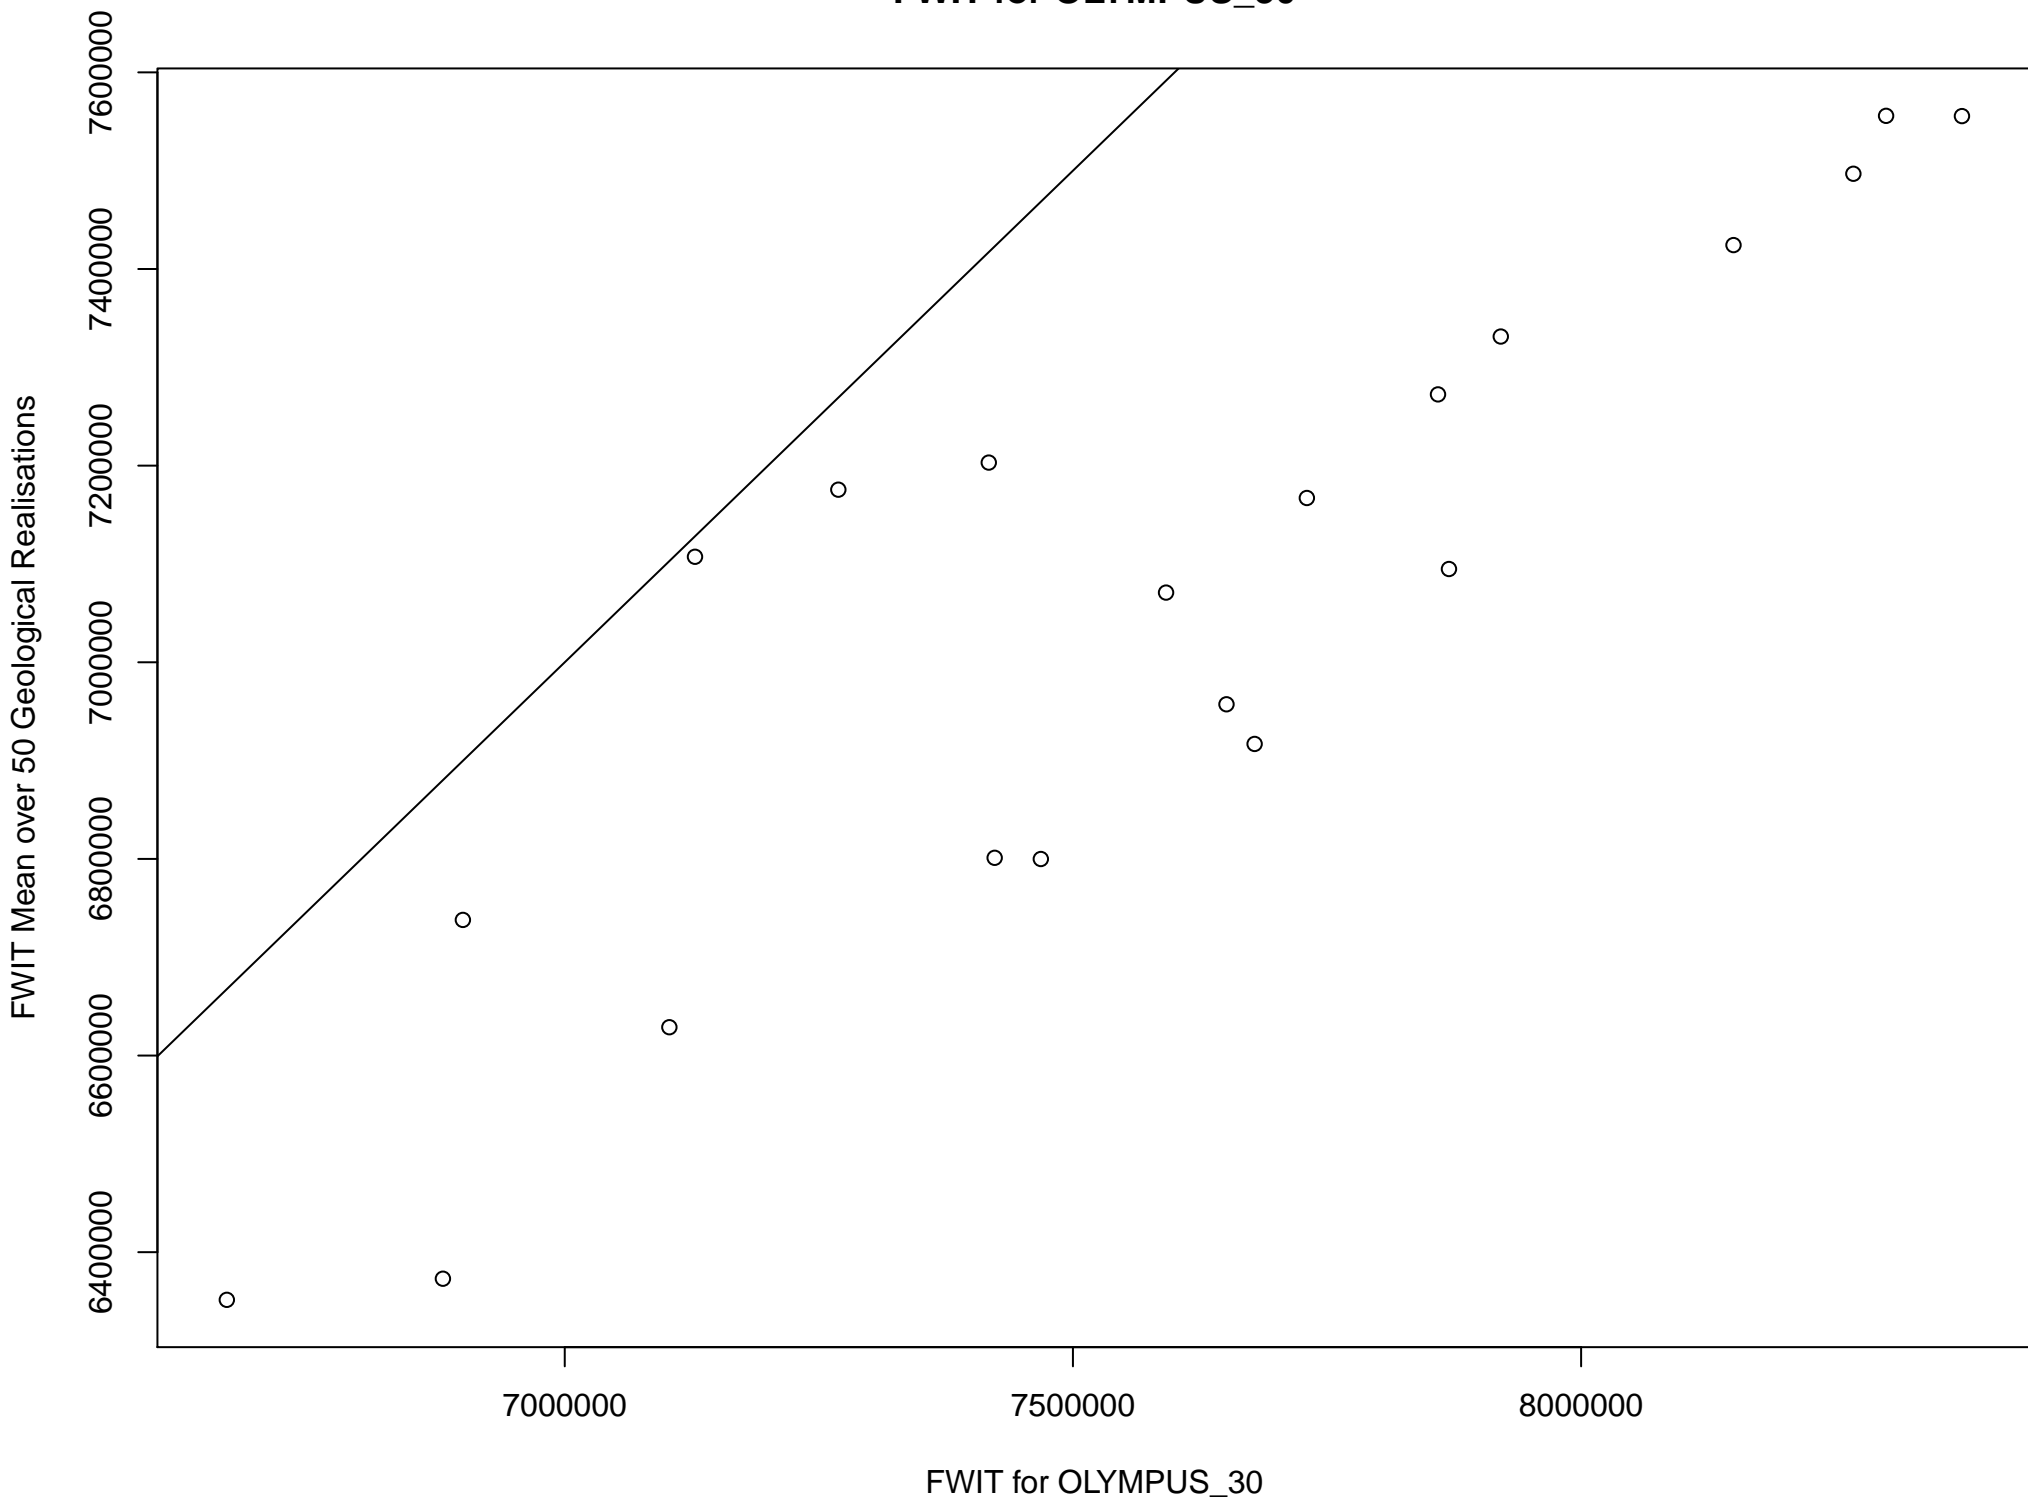

FWIT for OLYMPUS\_31

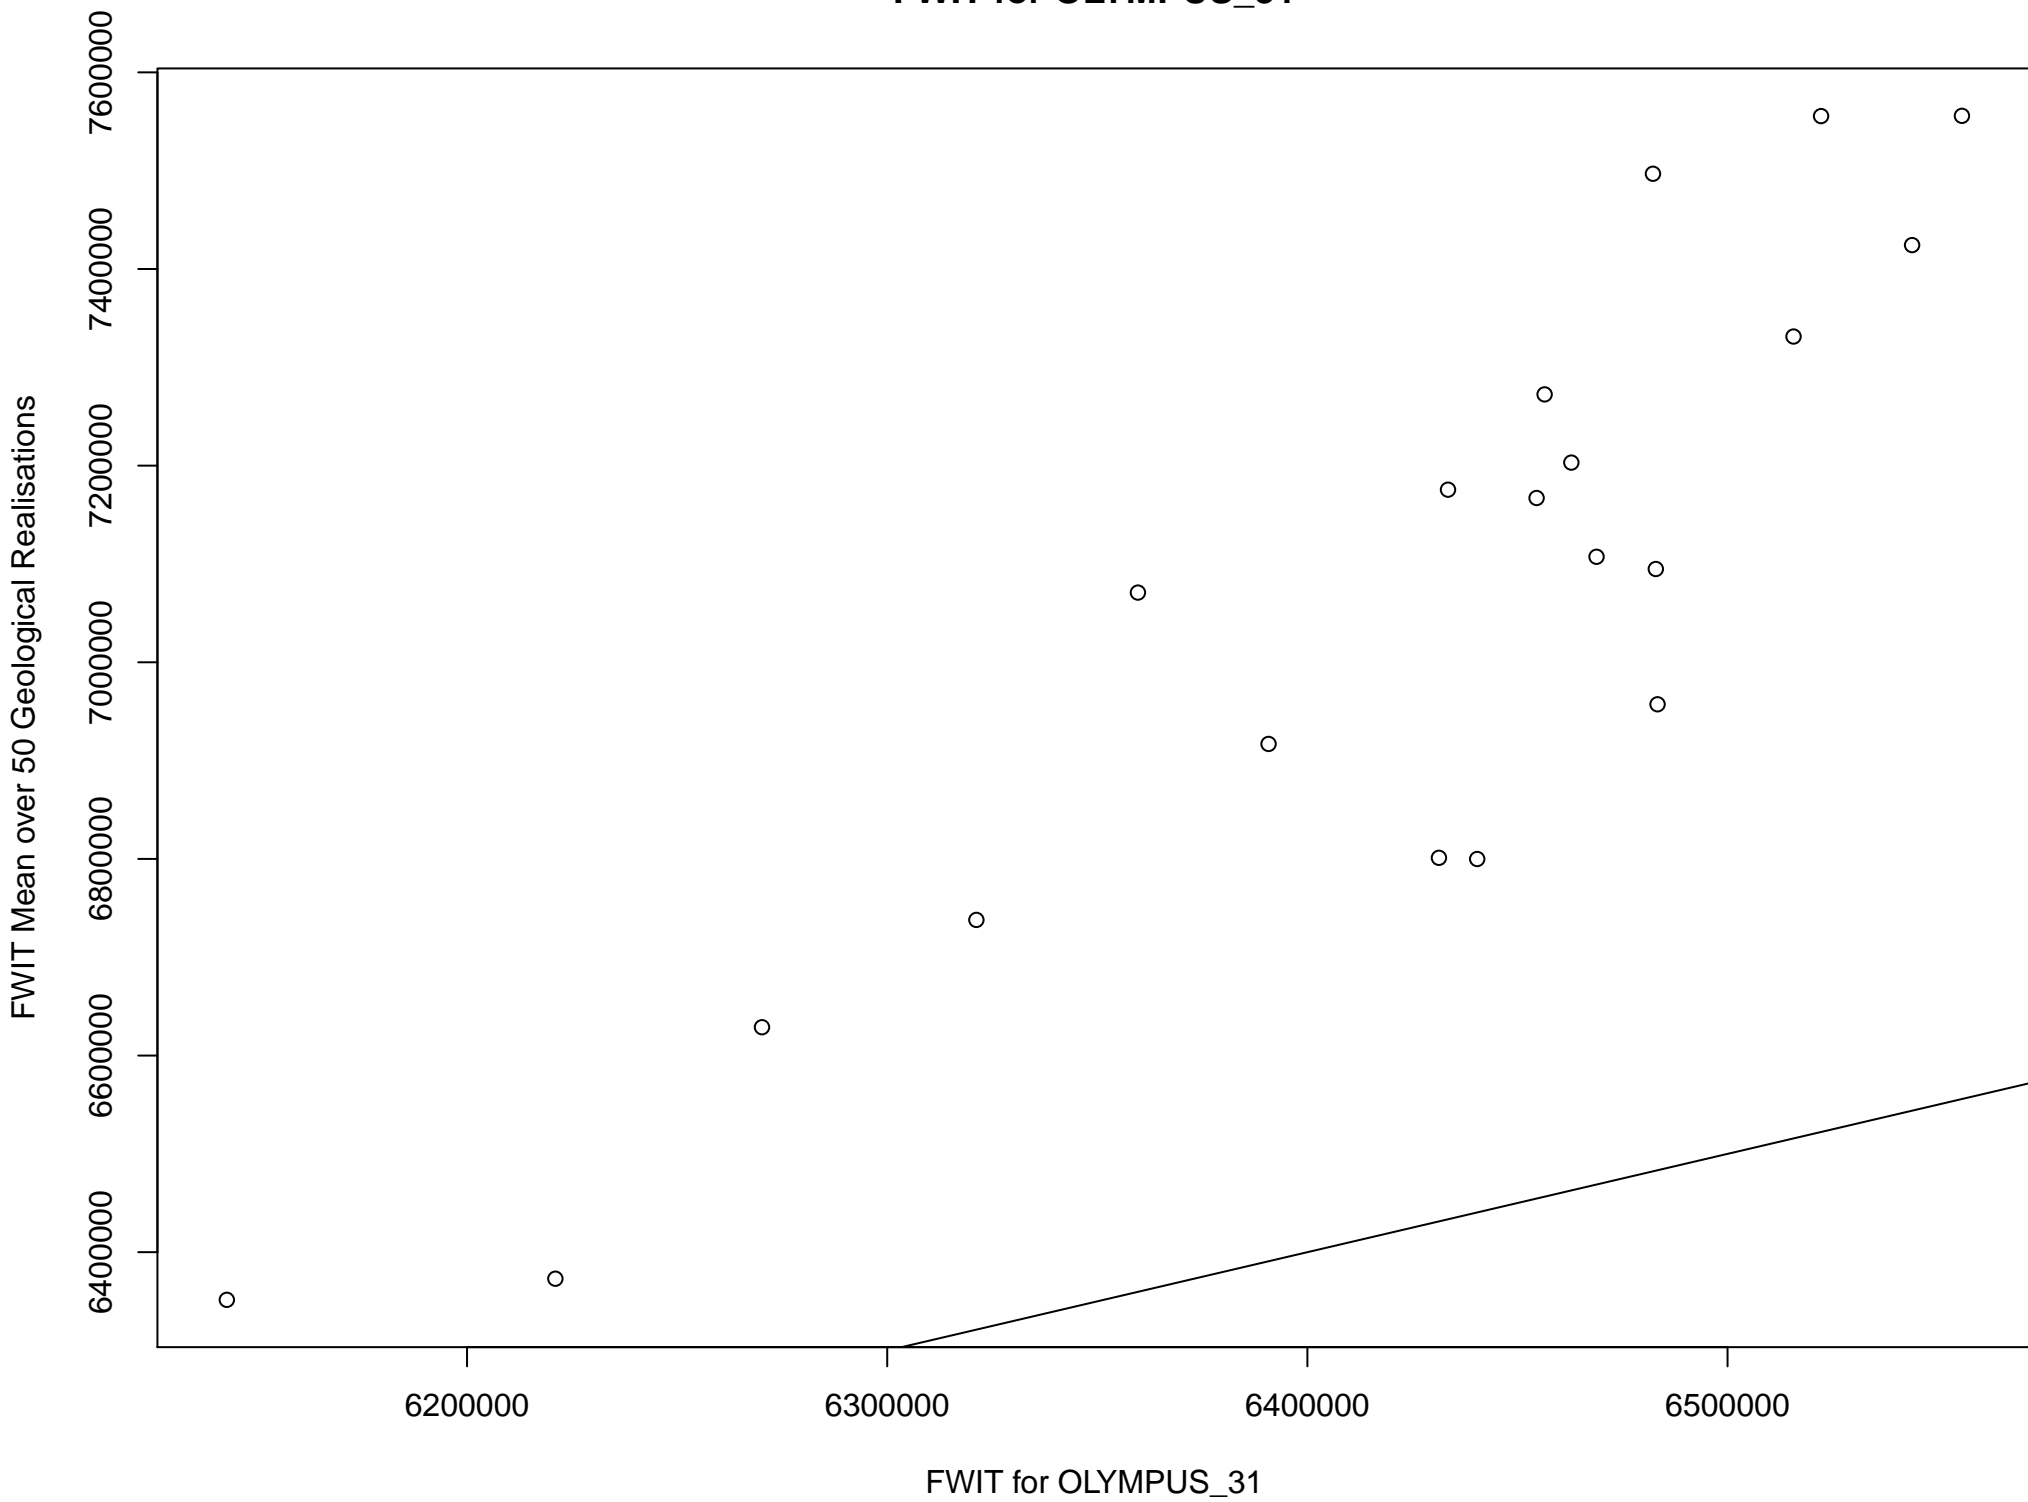

FWIT for OLYMPUS\_32

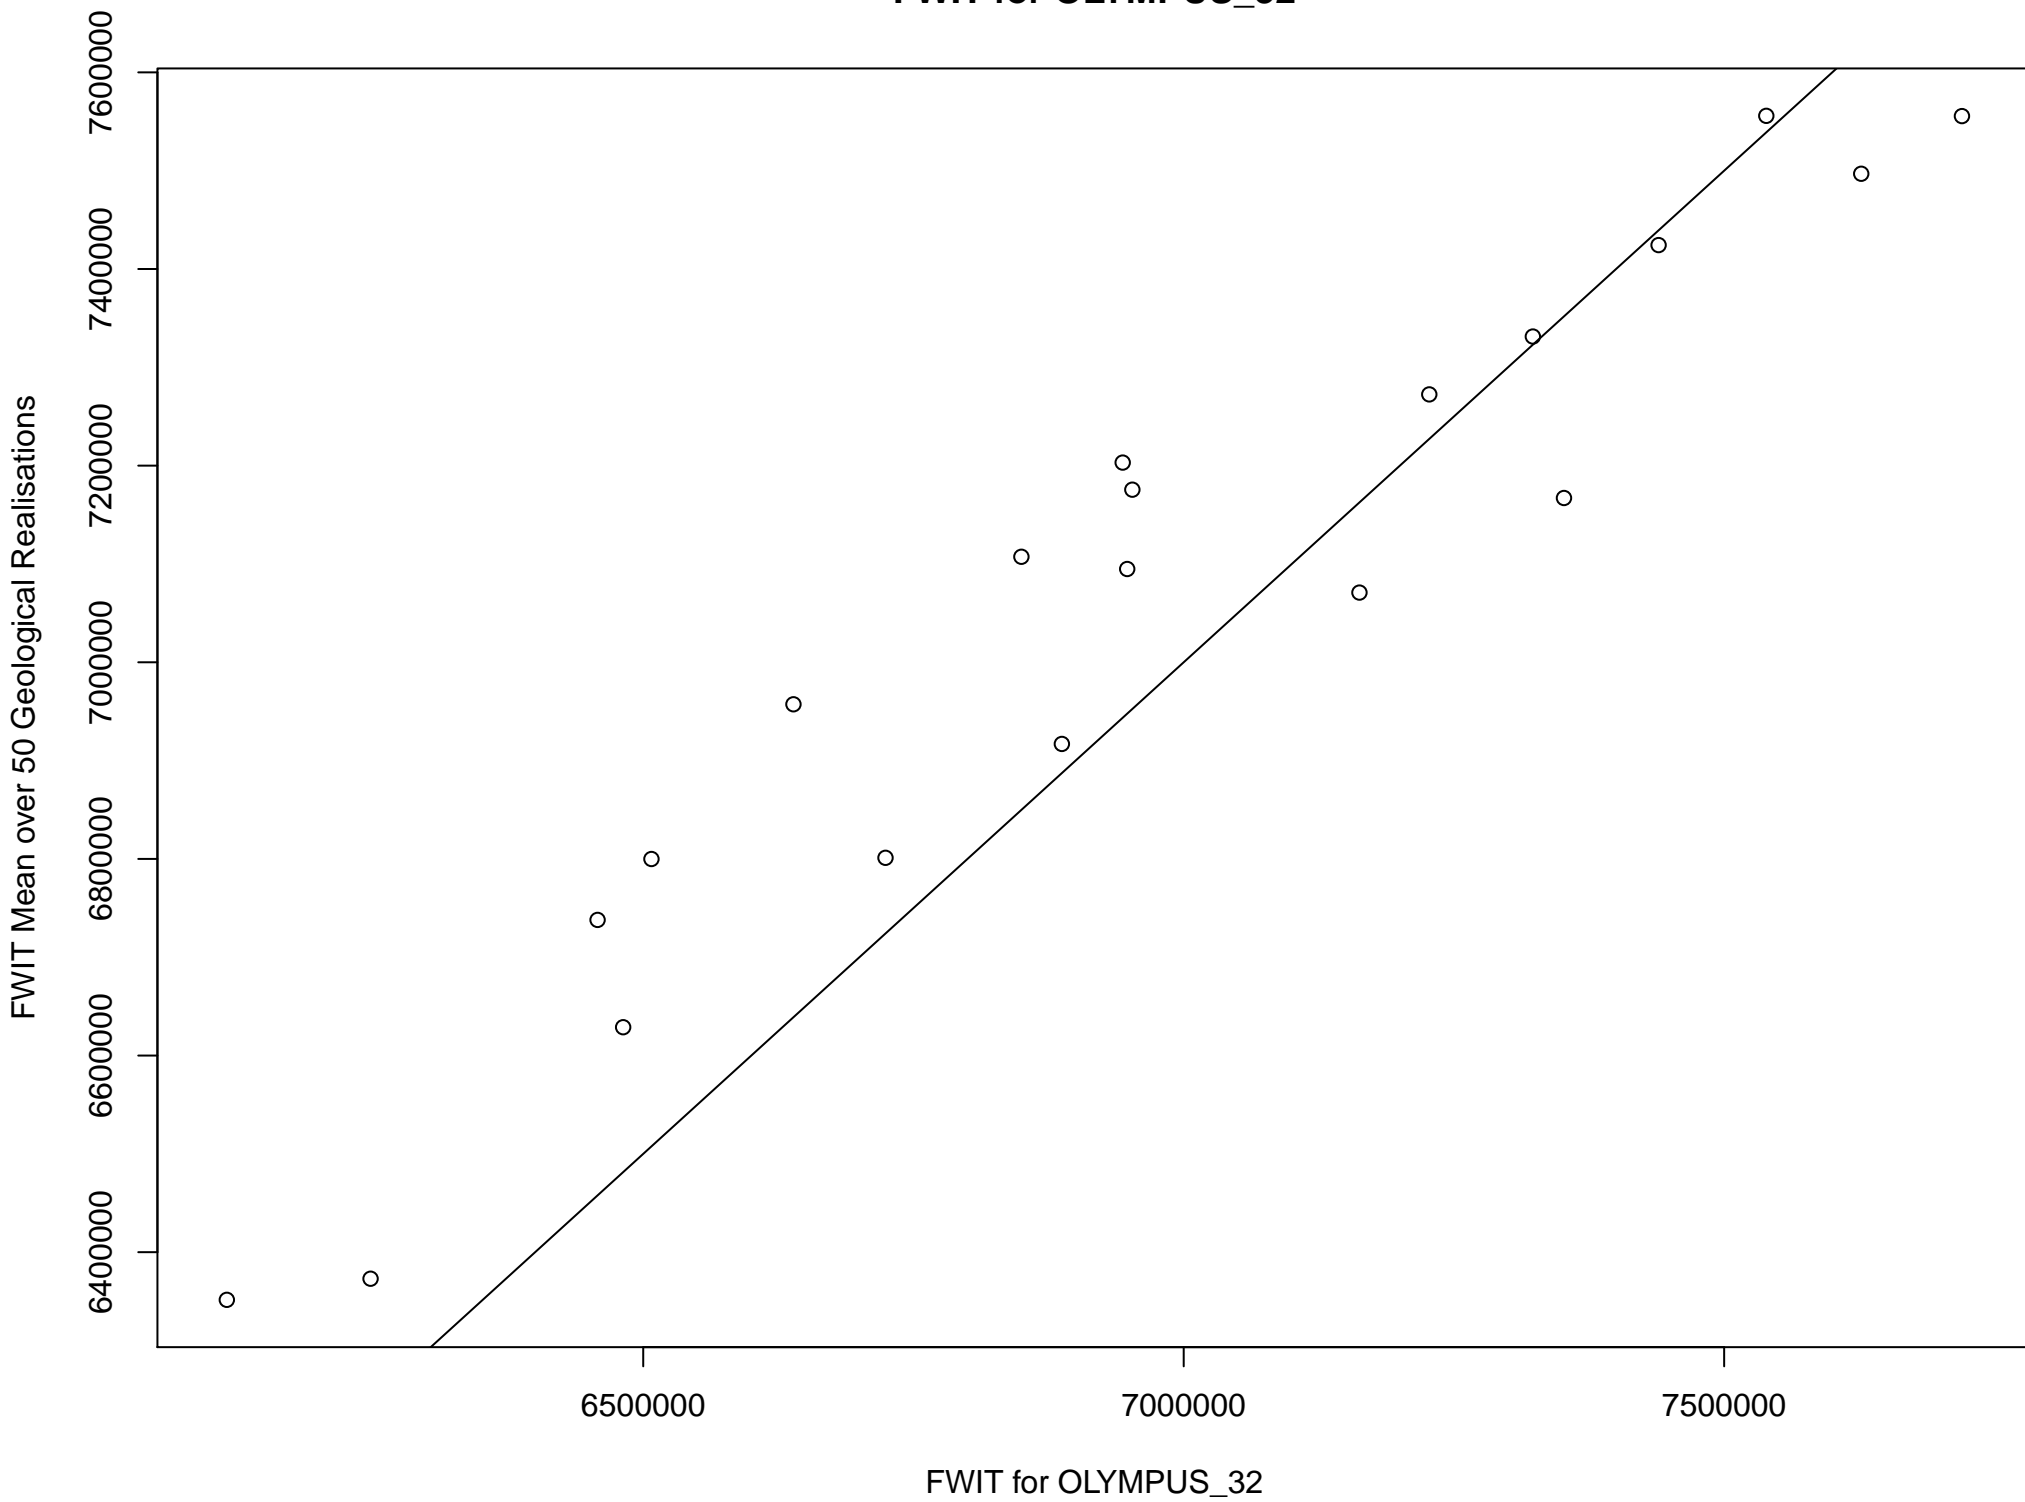



FWIT for OLYMPUS\_33

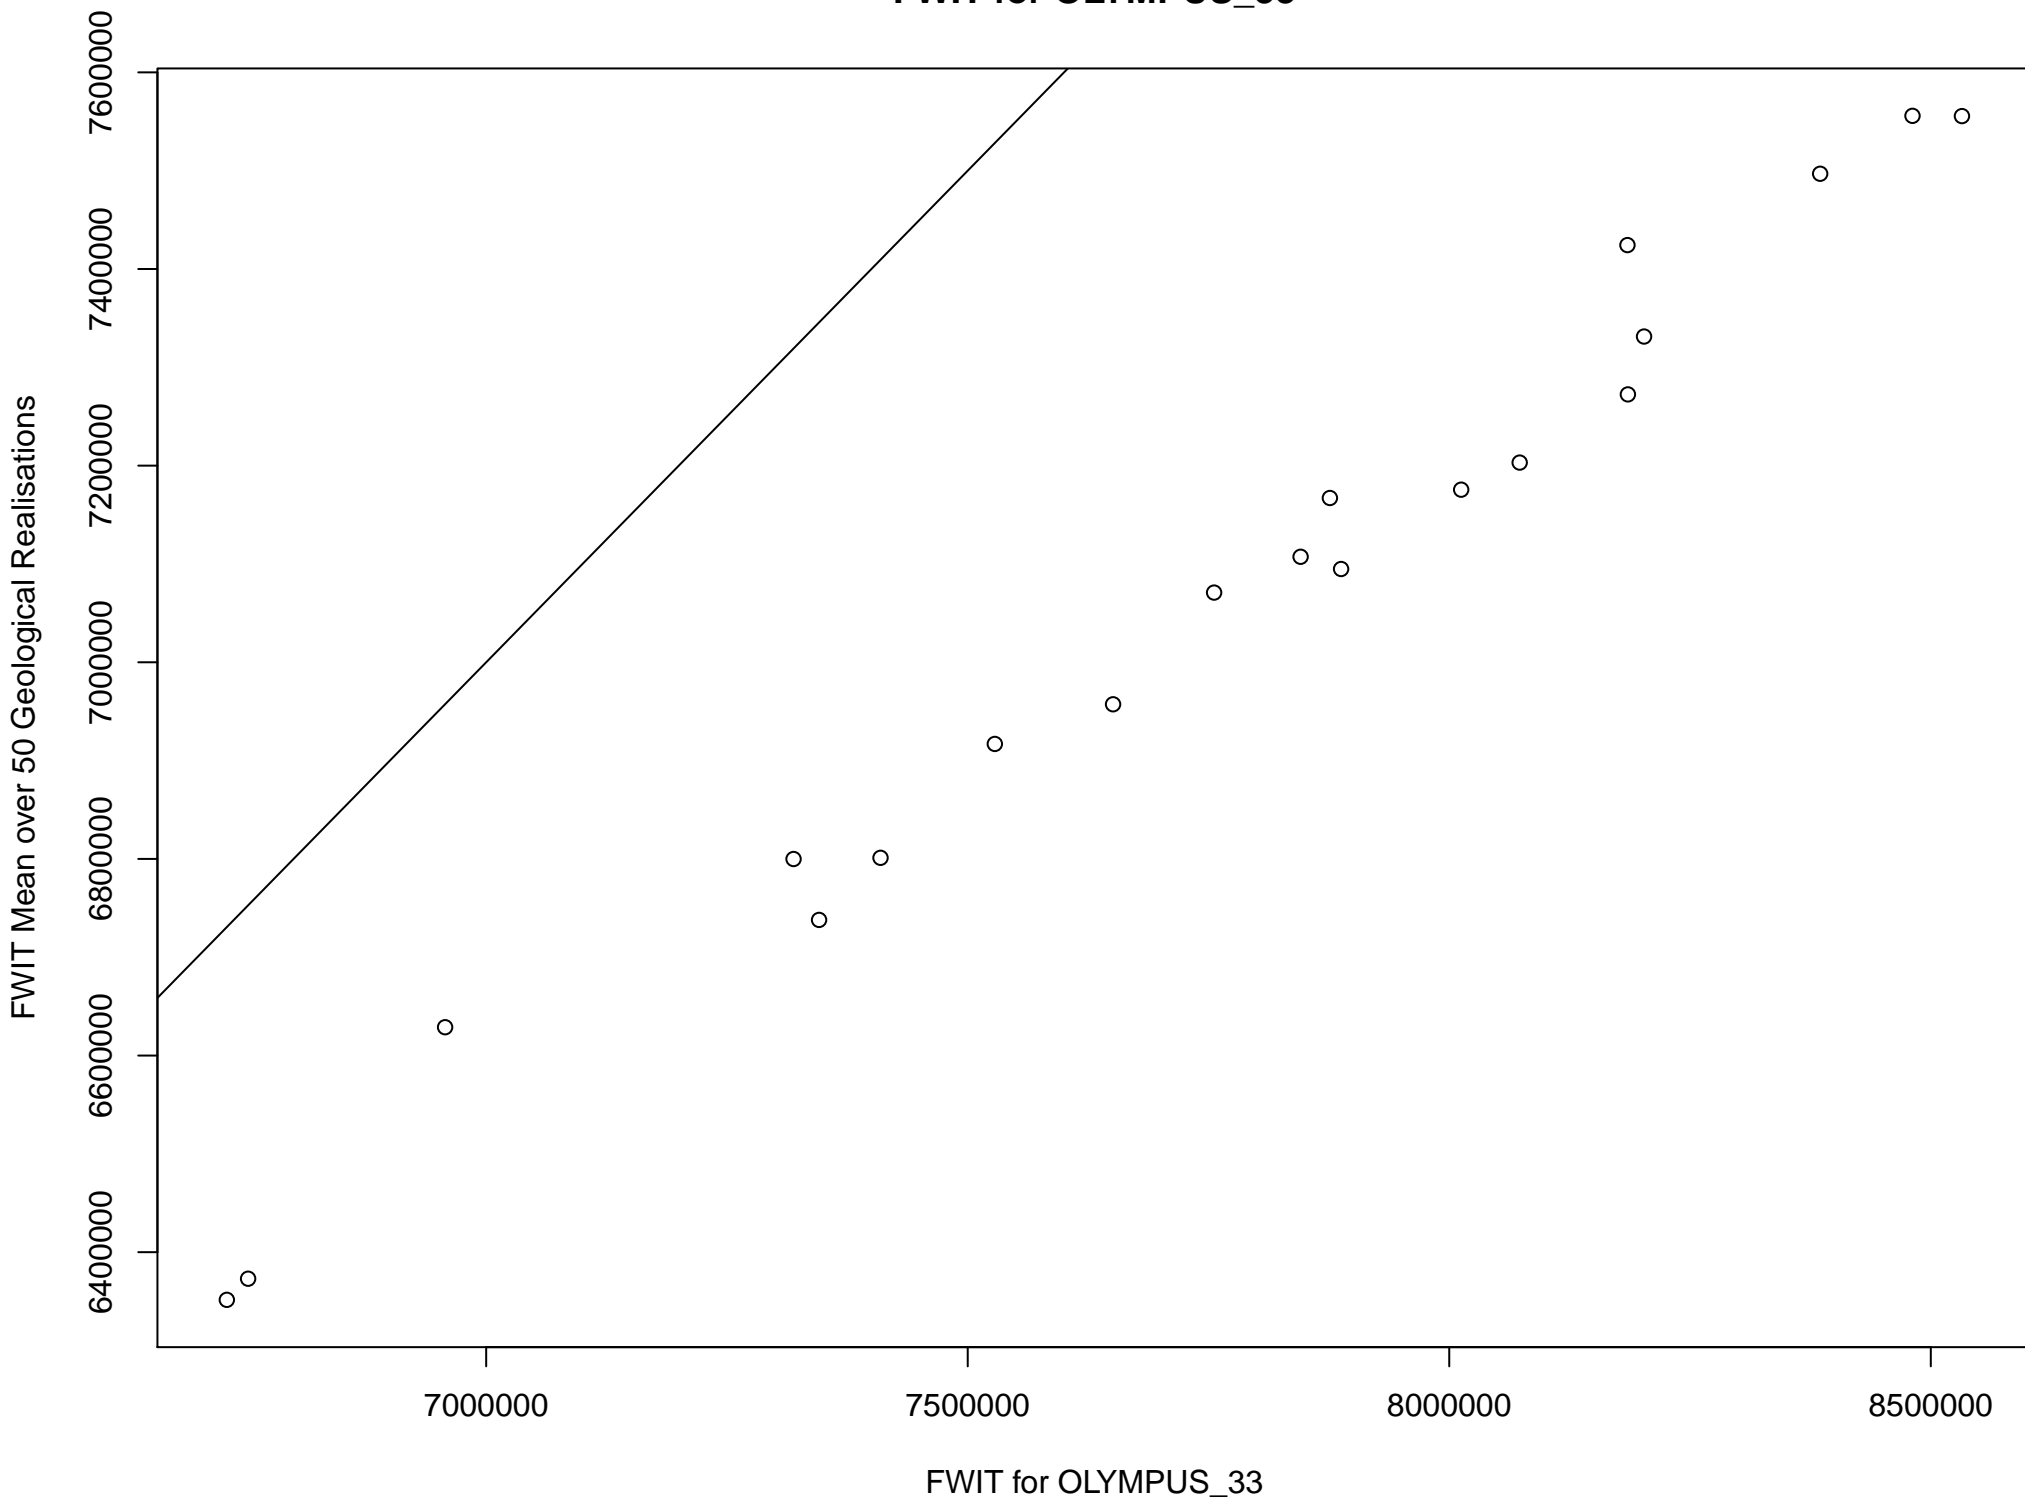

FWIT for OLYMPUS\_34

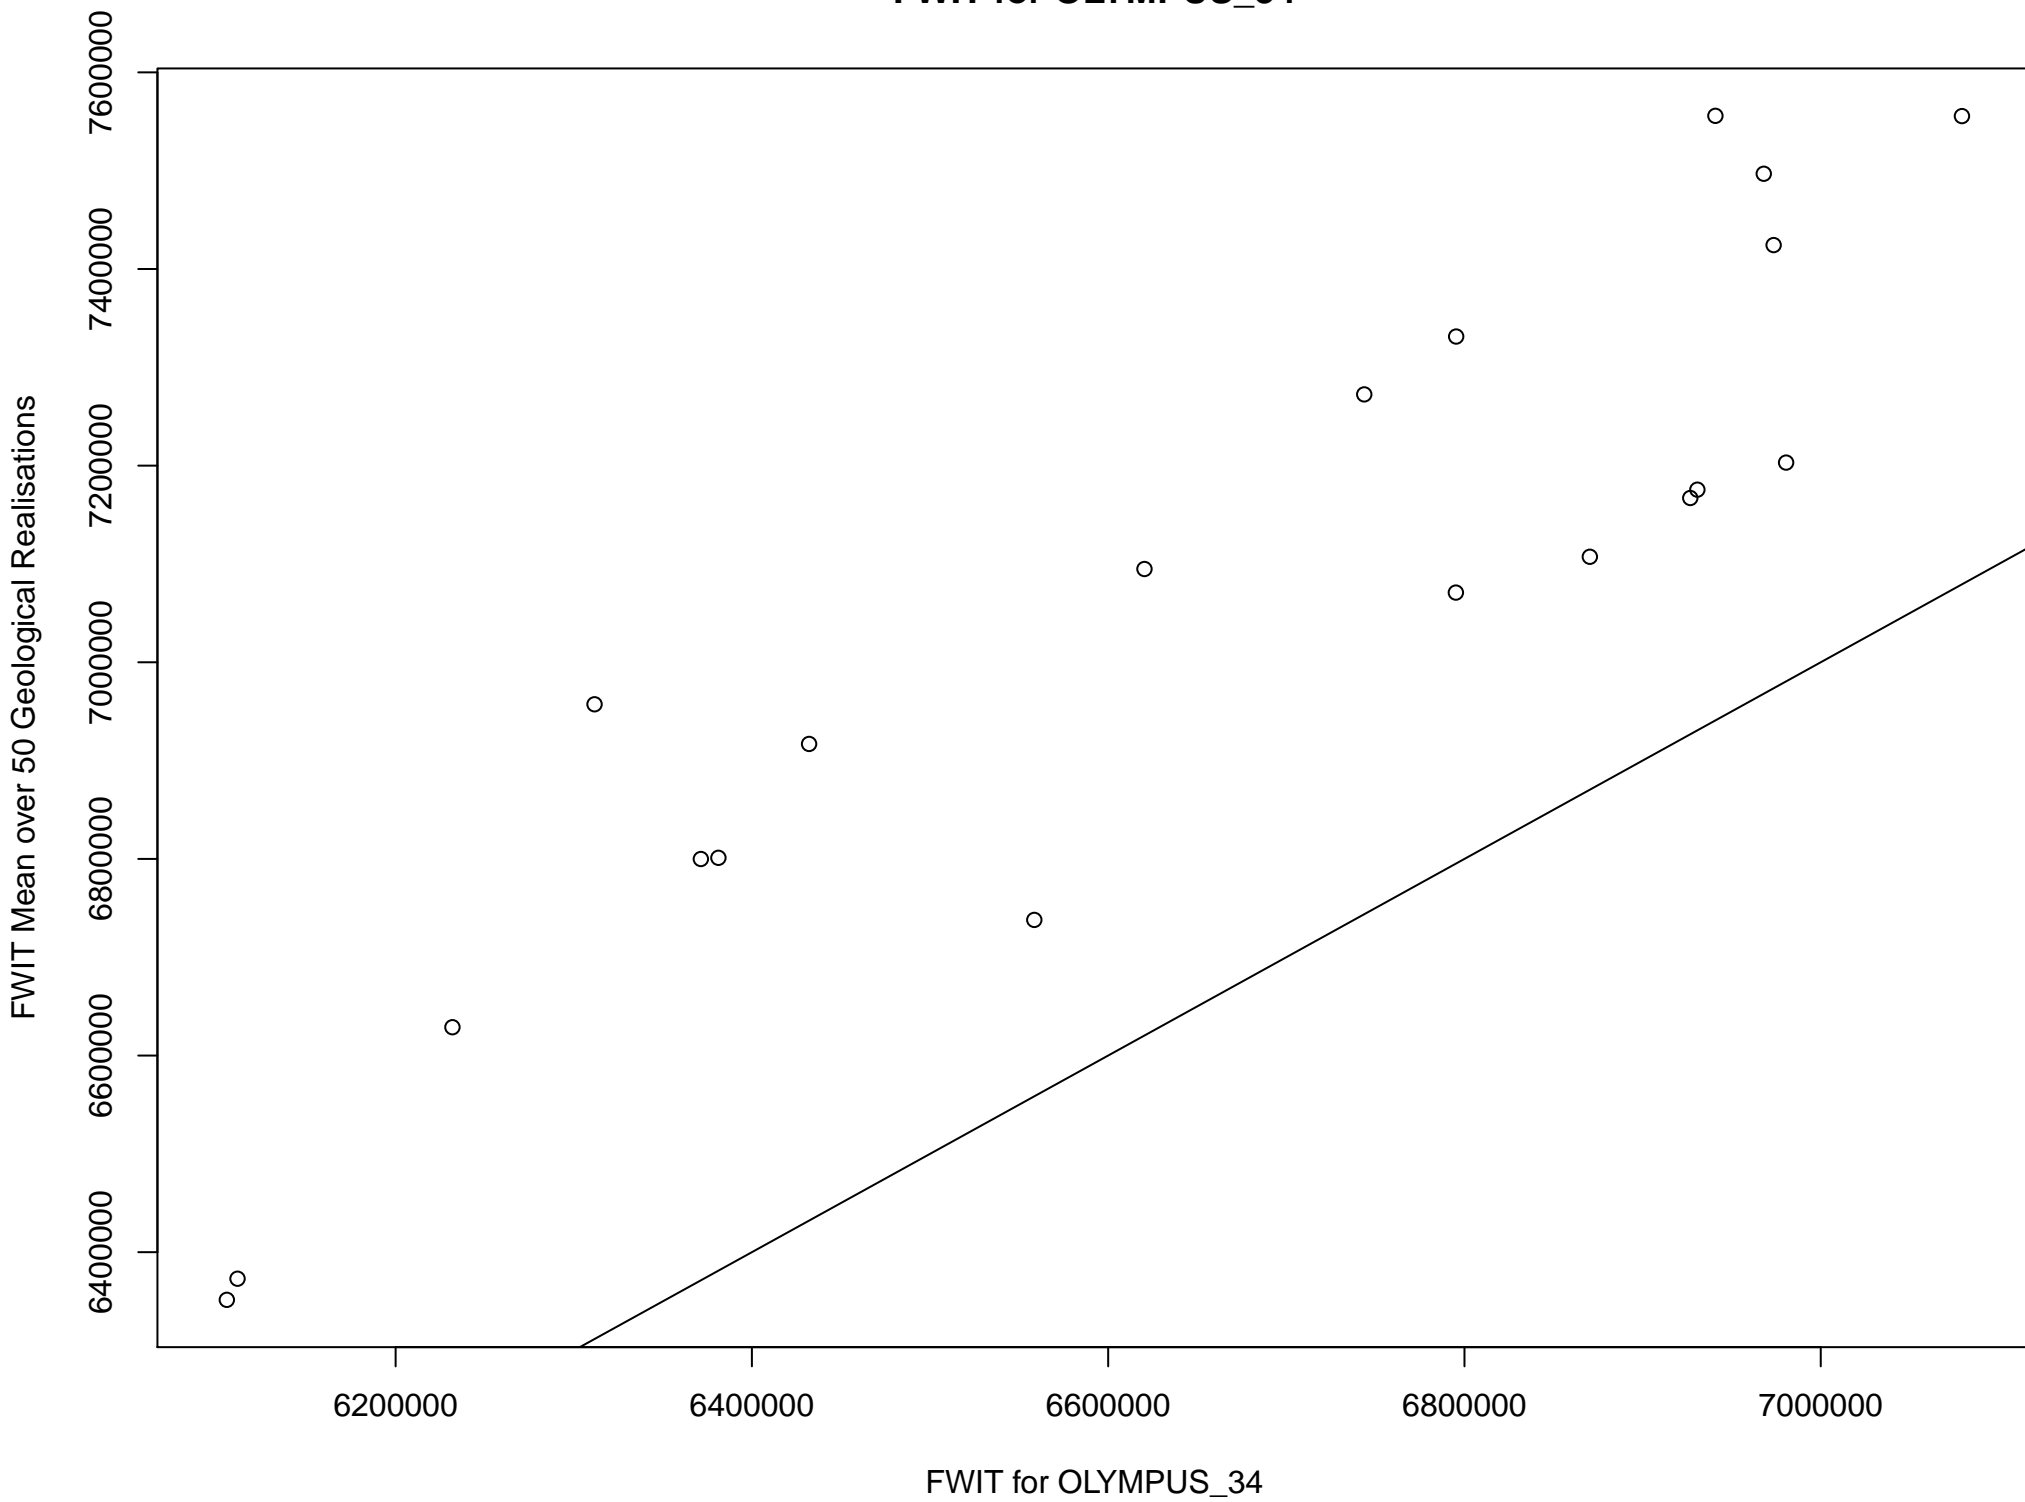

FWIT for OLYMPUS\_35

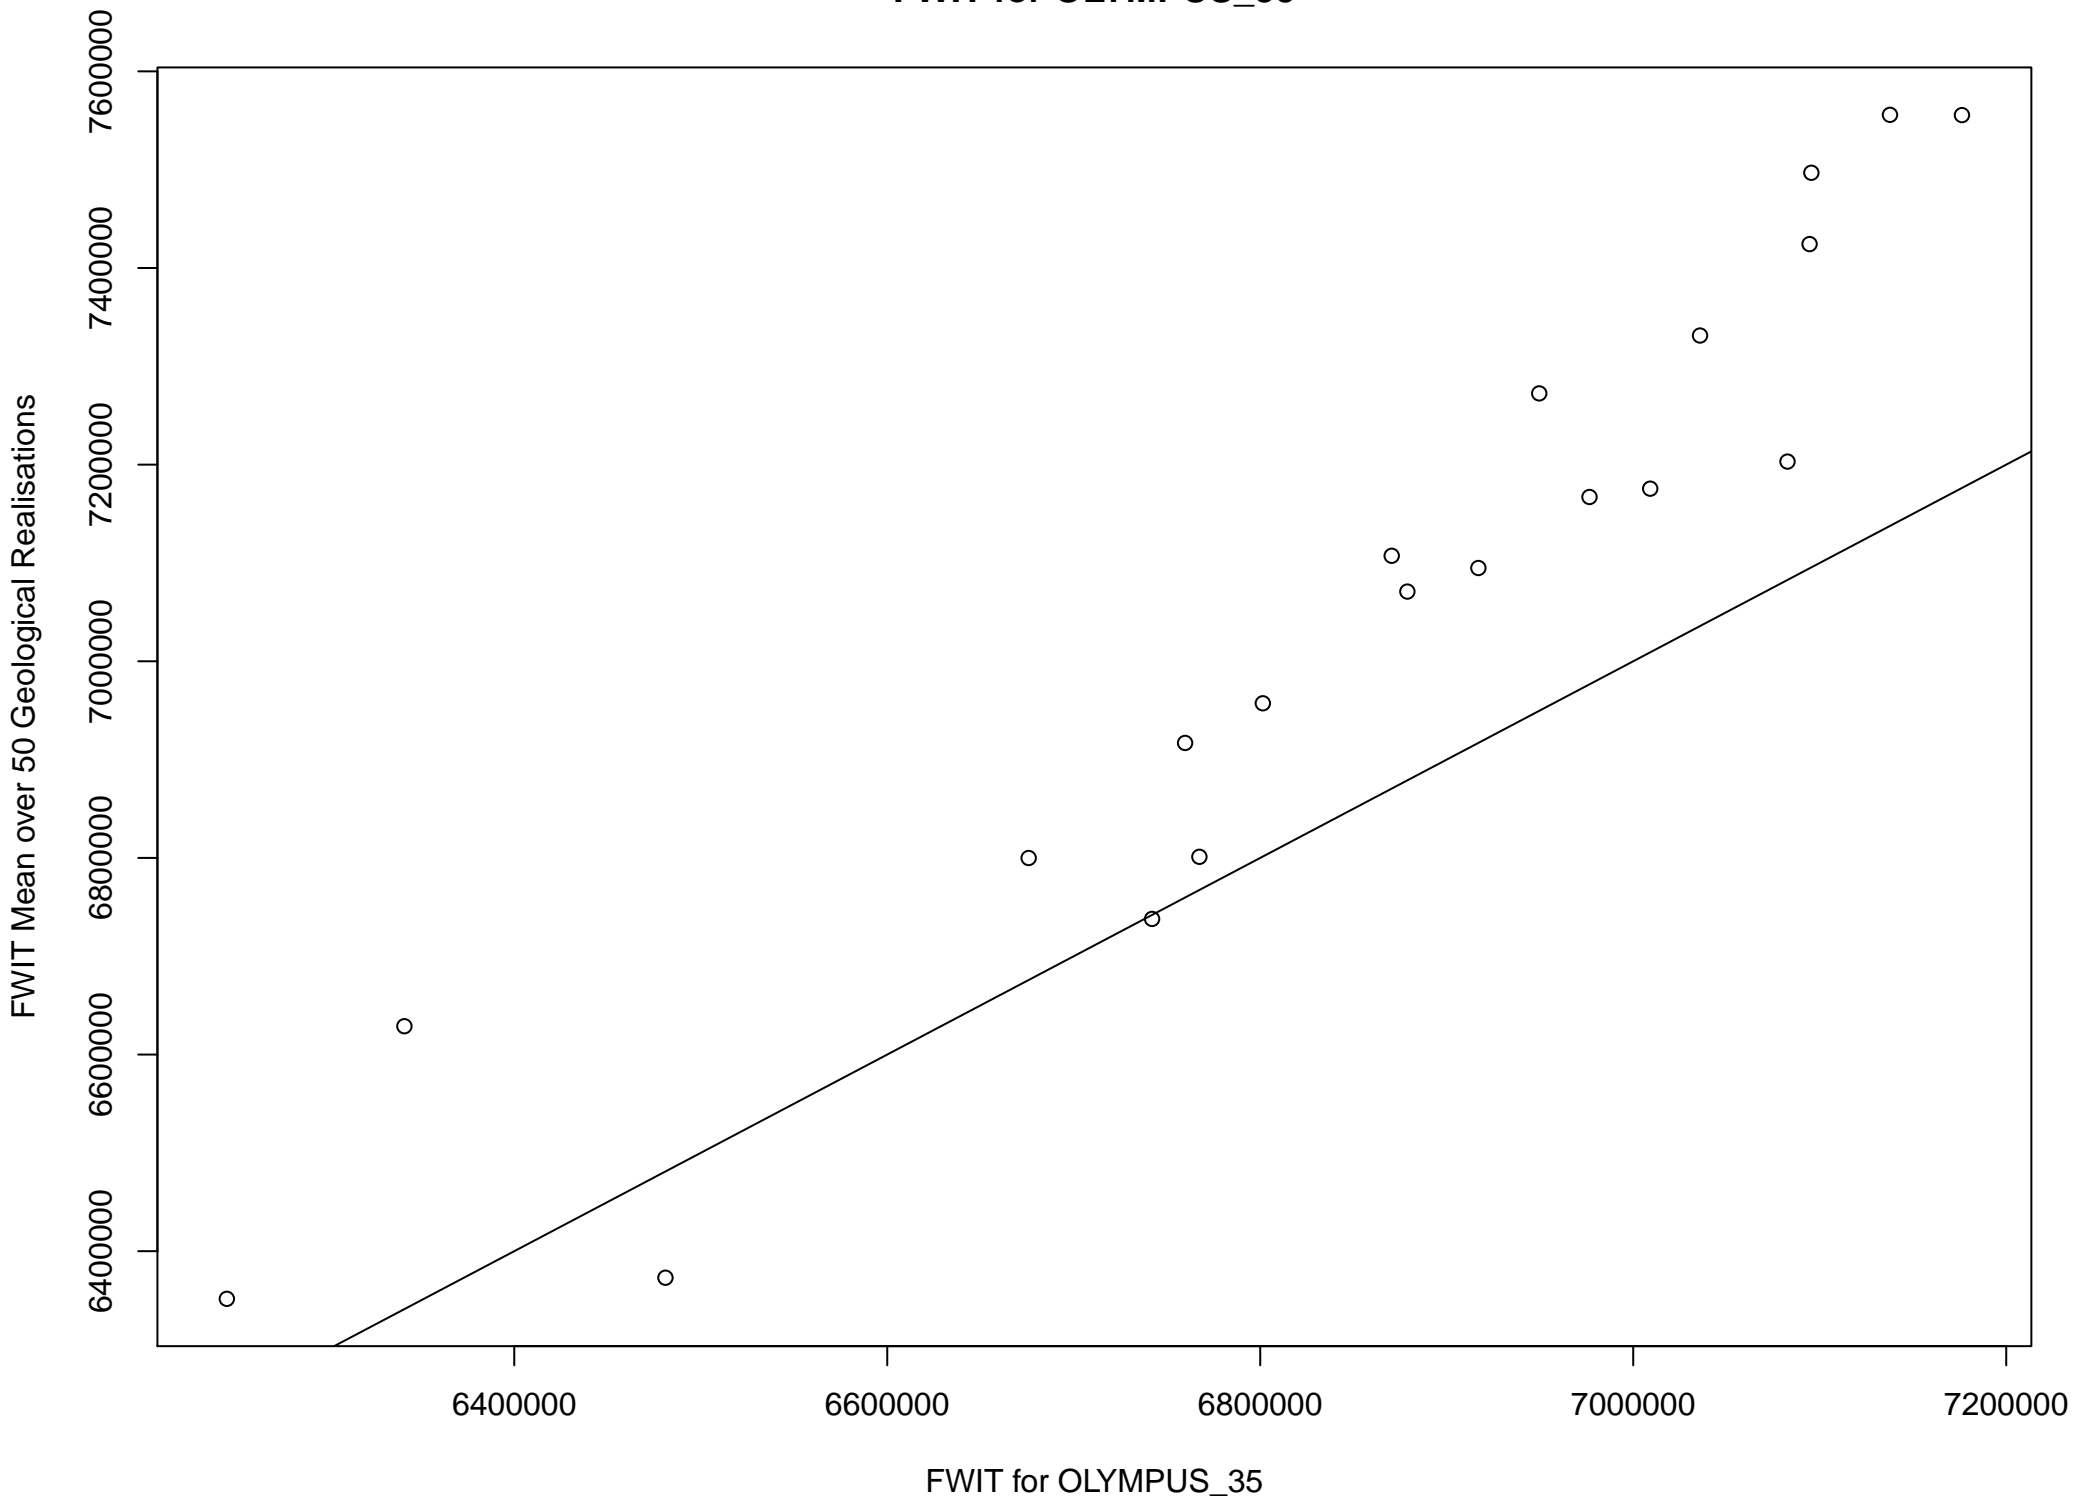

FWIT for OLYMPUS\_36

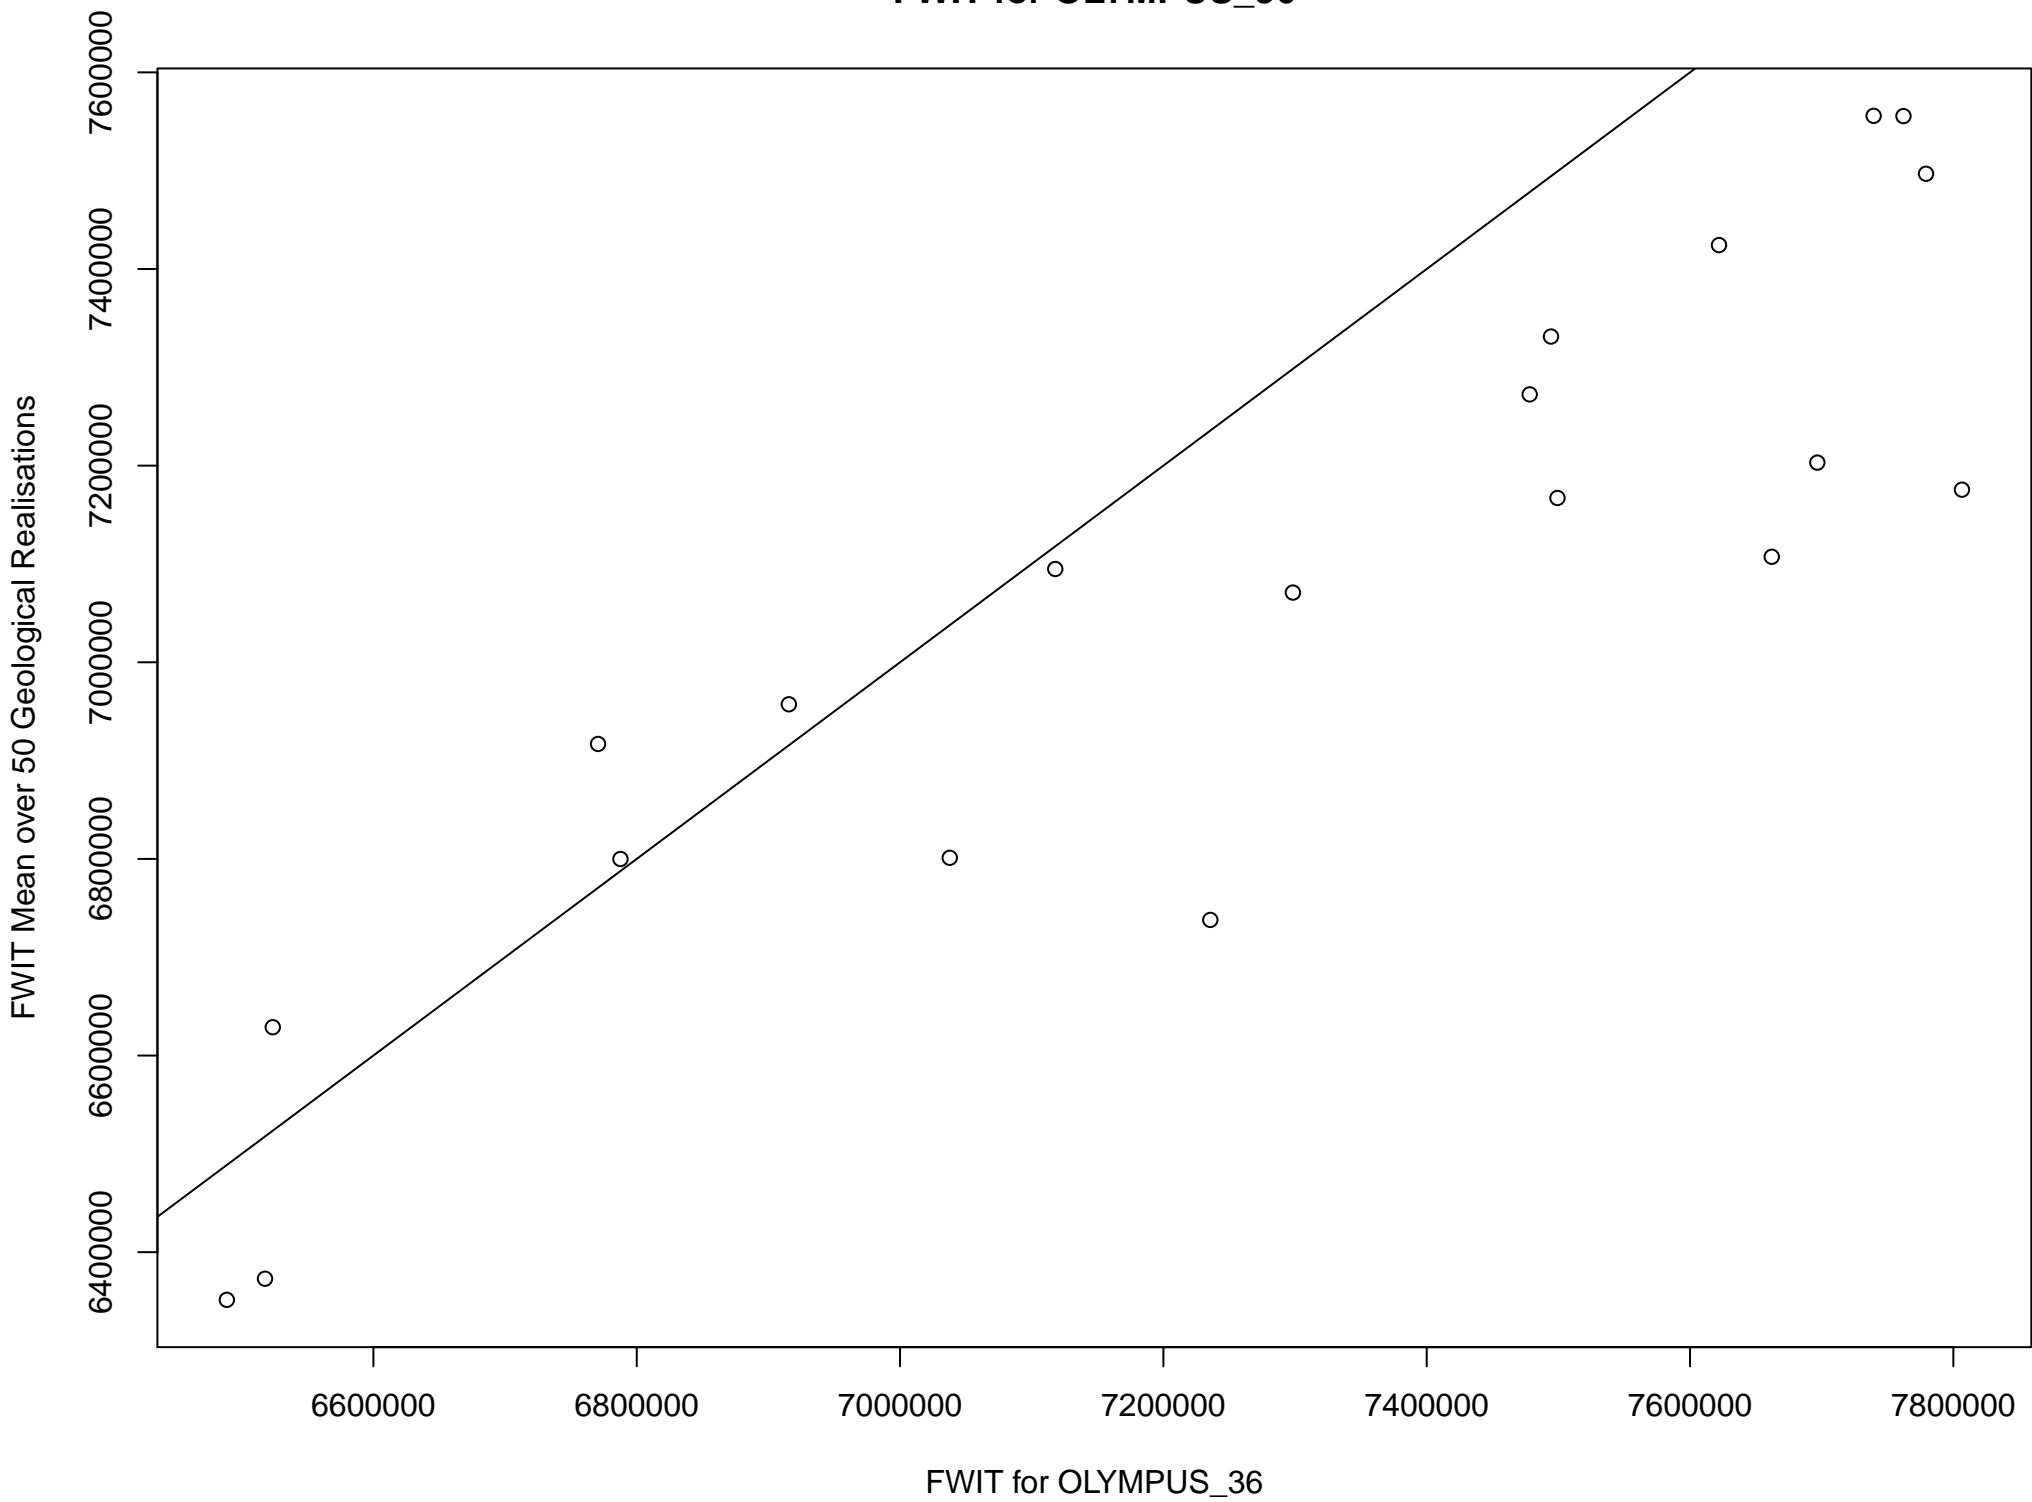

FWIT for OLYMPUS\_37

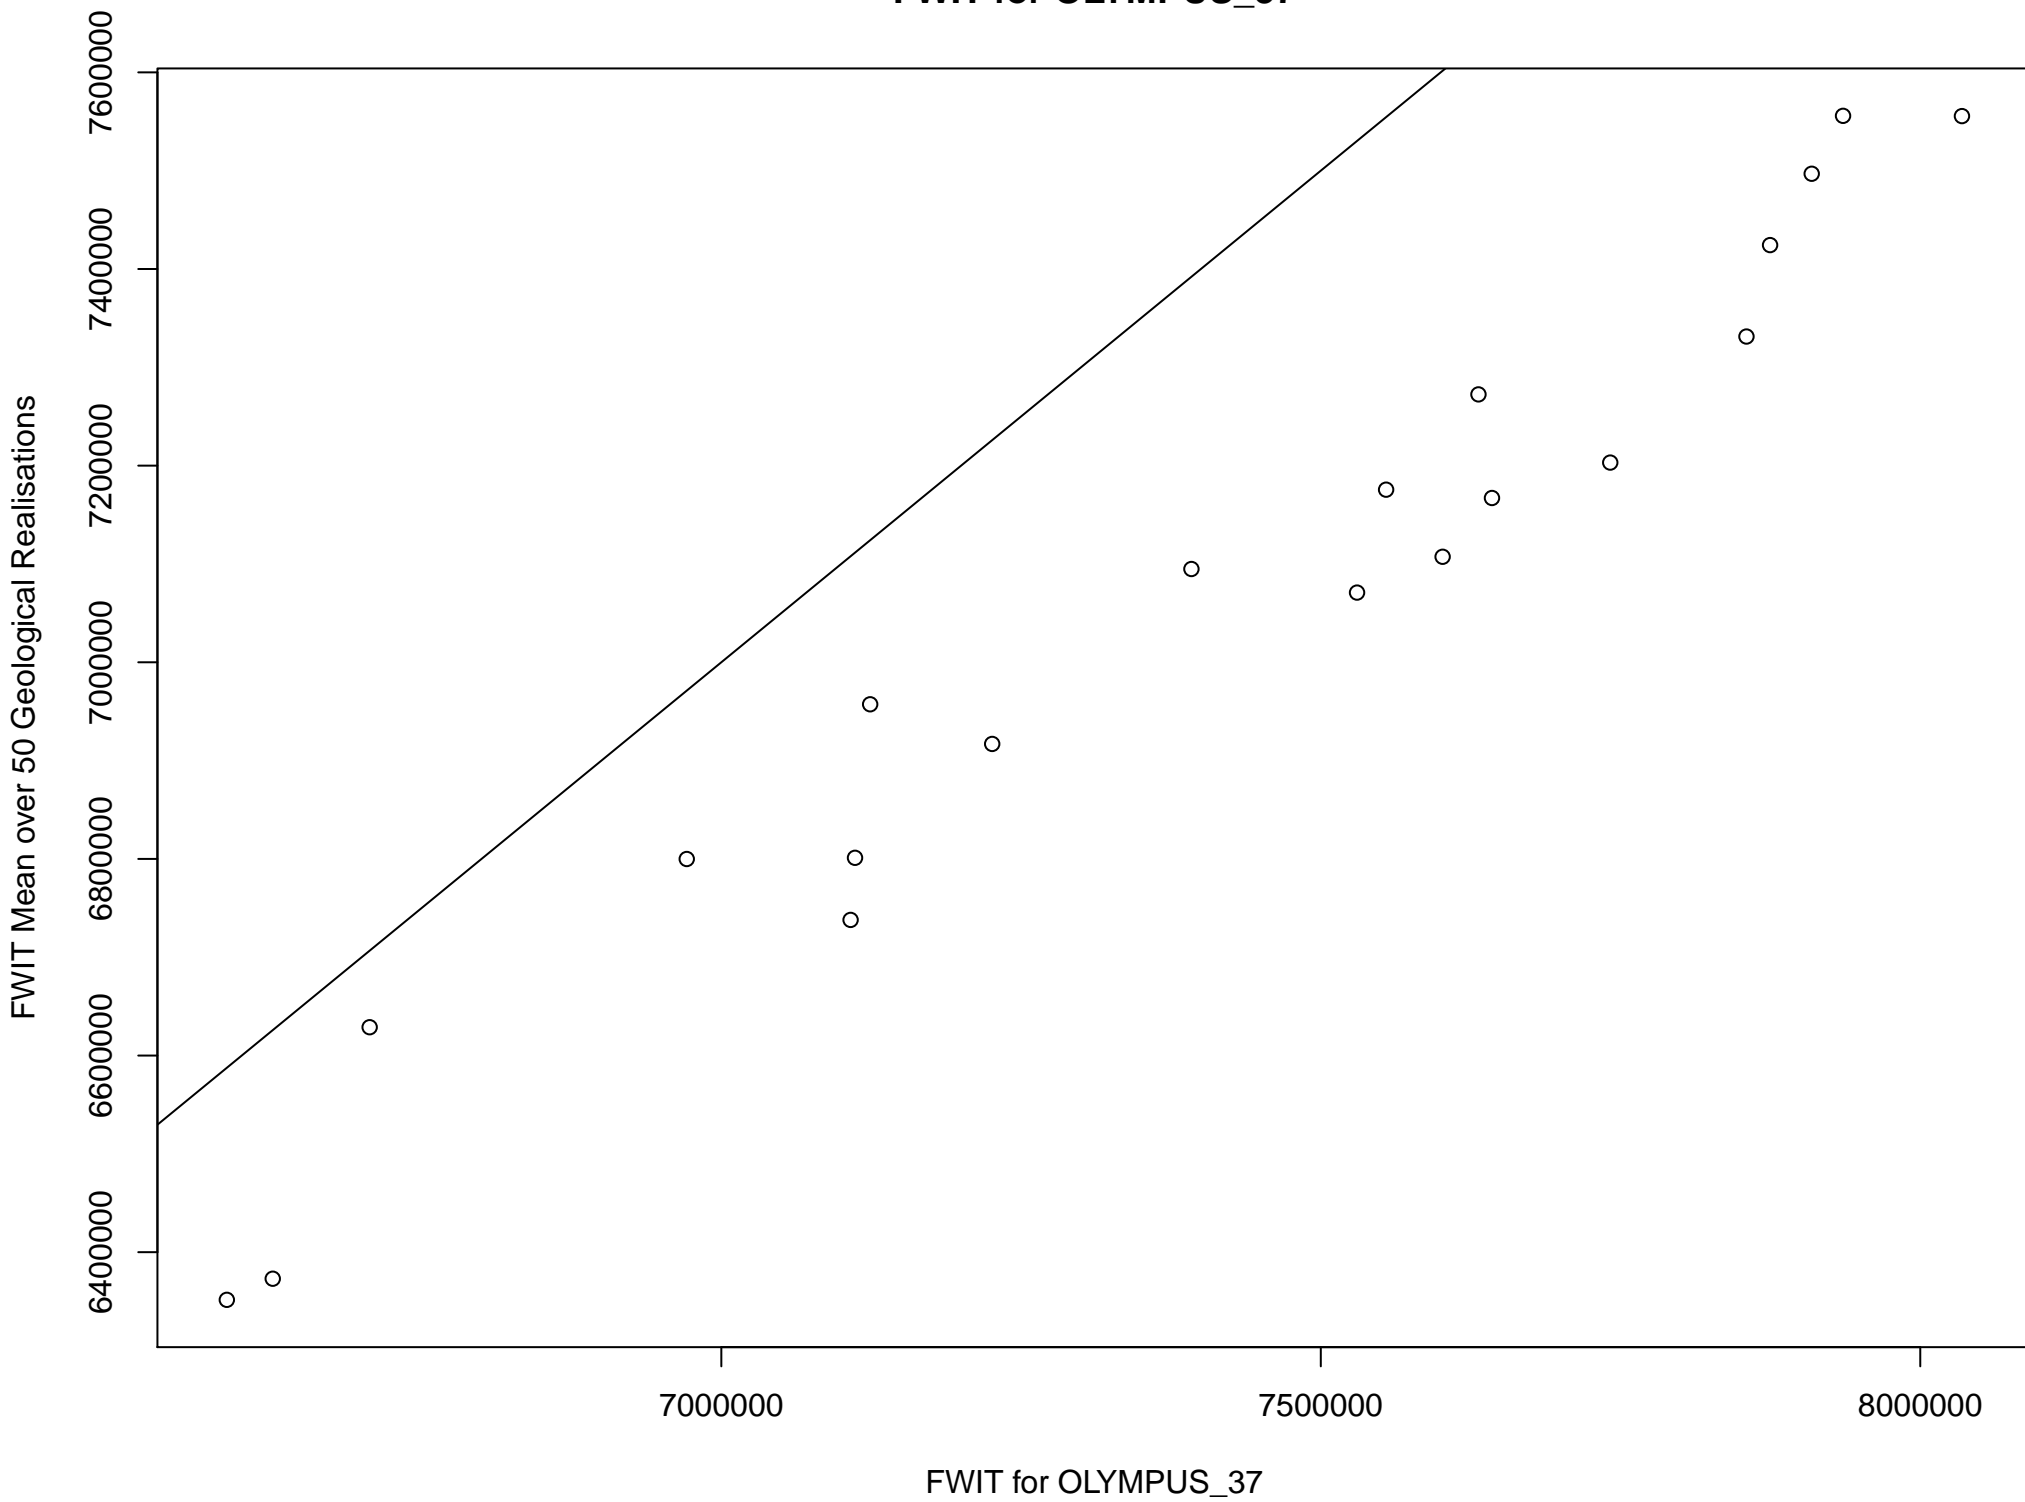

FWIT for OLYMPUS\_38

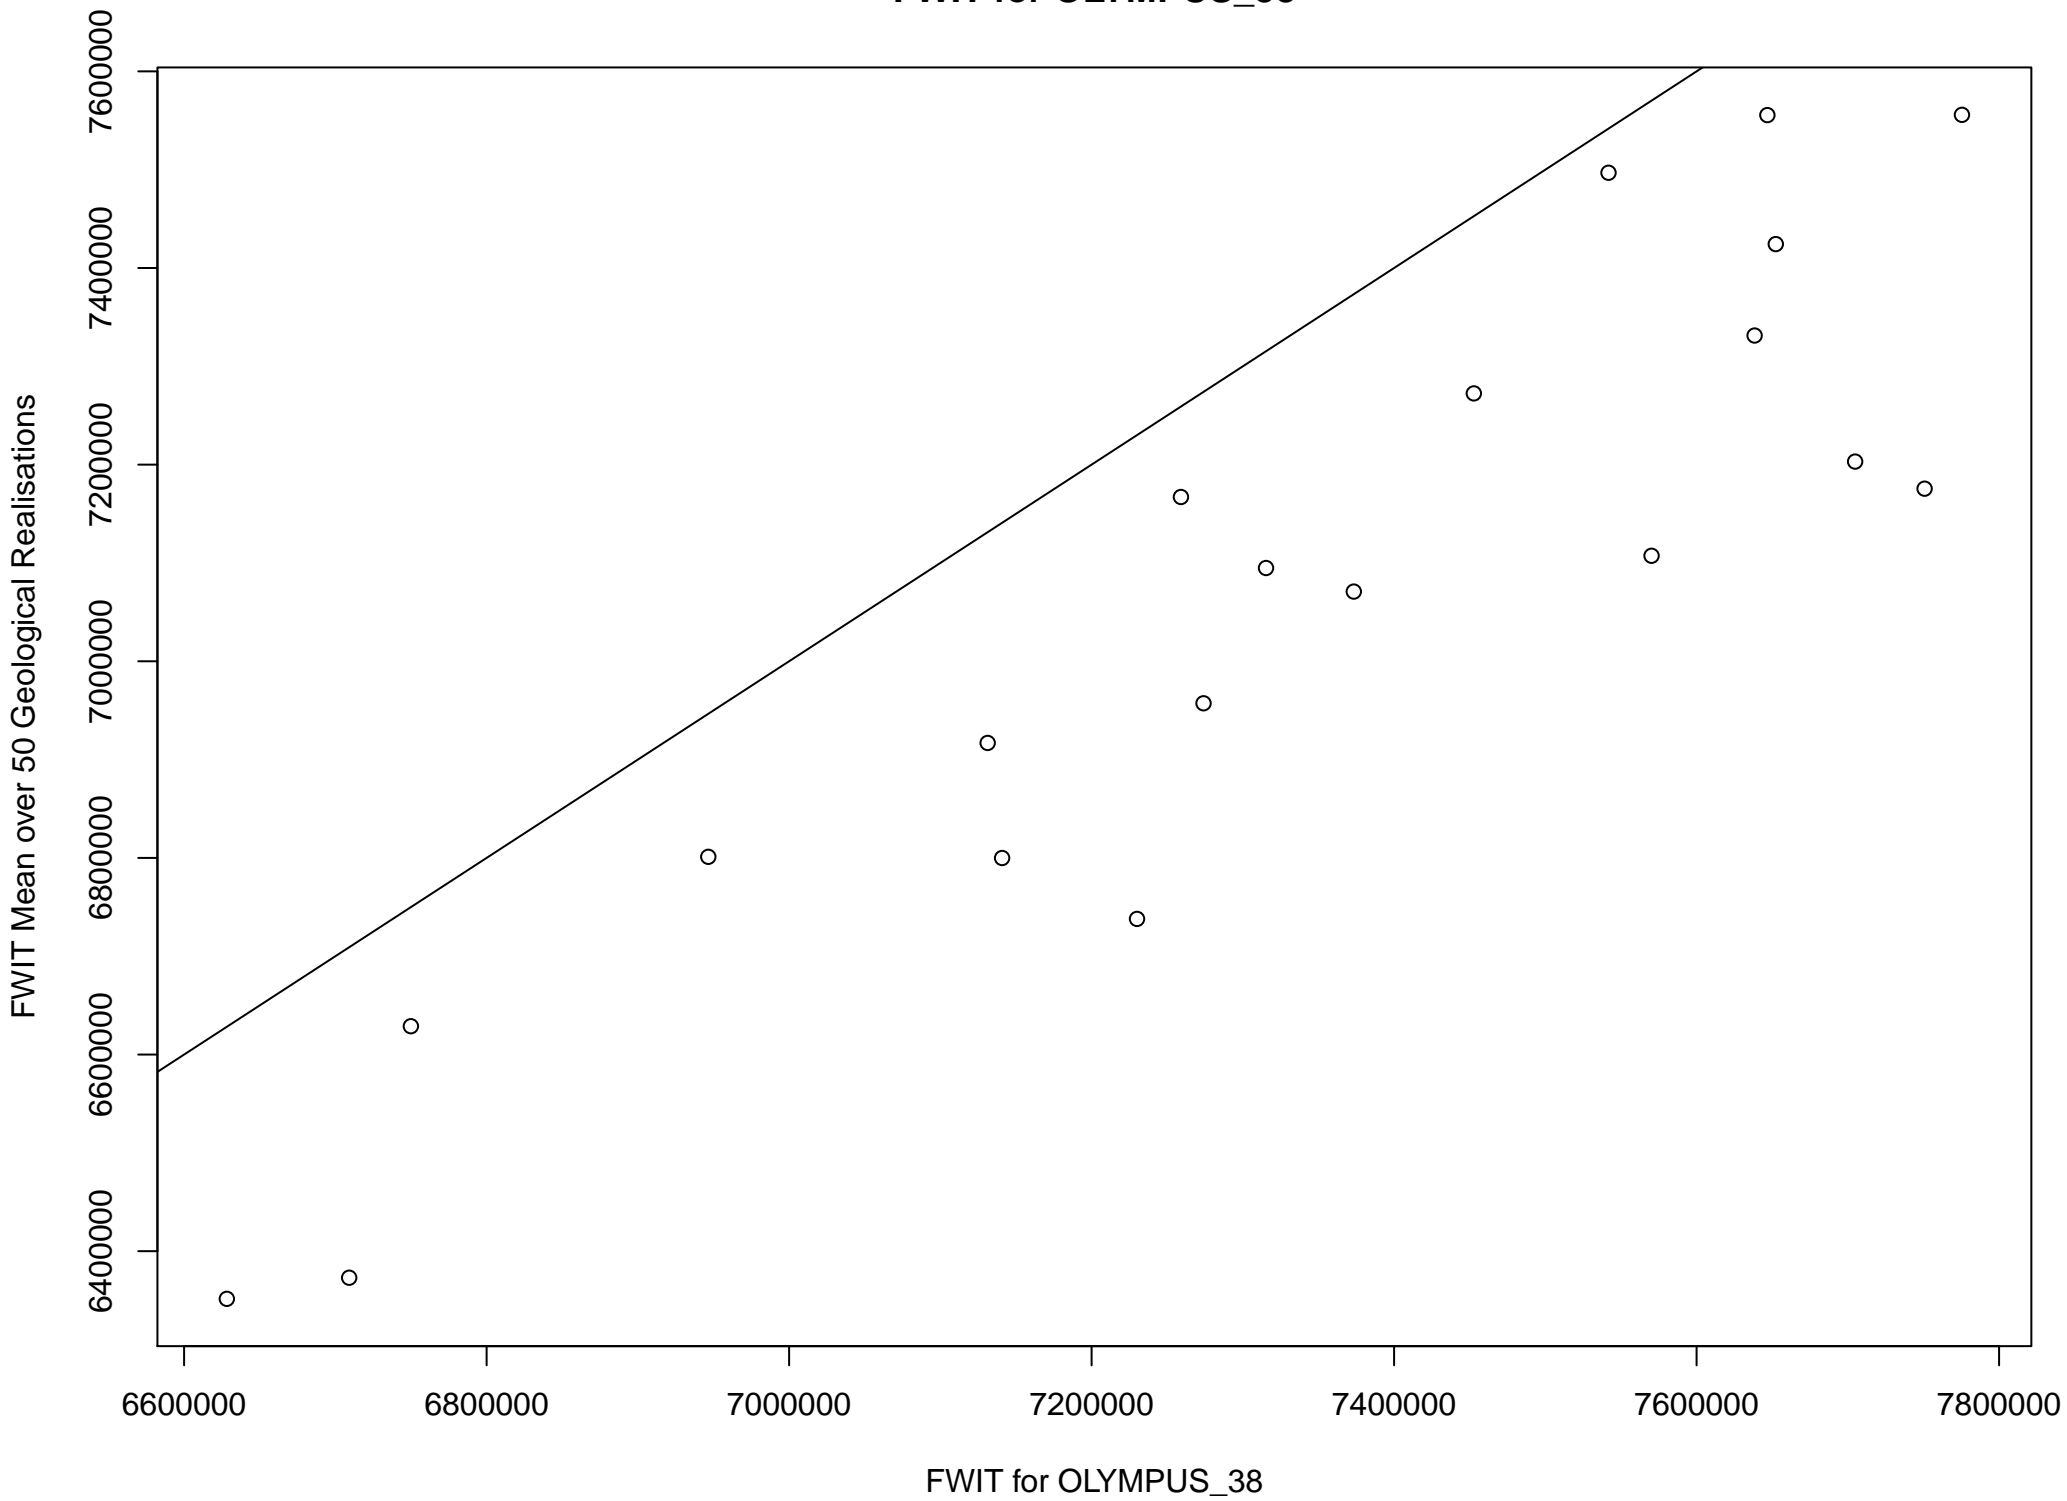

FWIT for OLYMPUS\_39

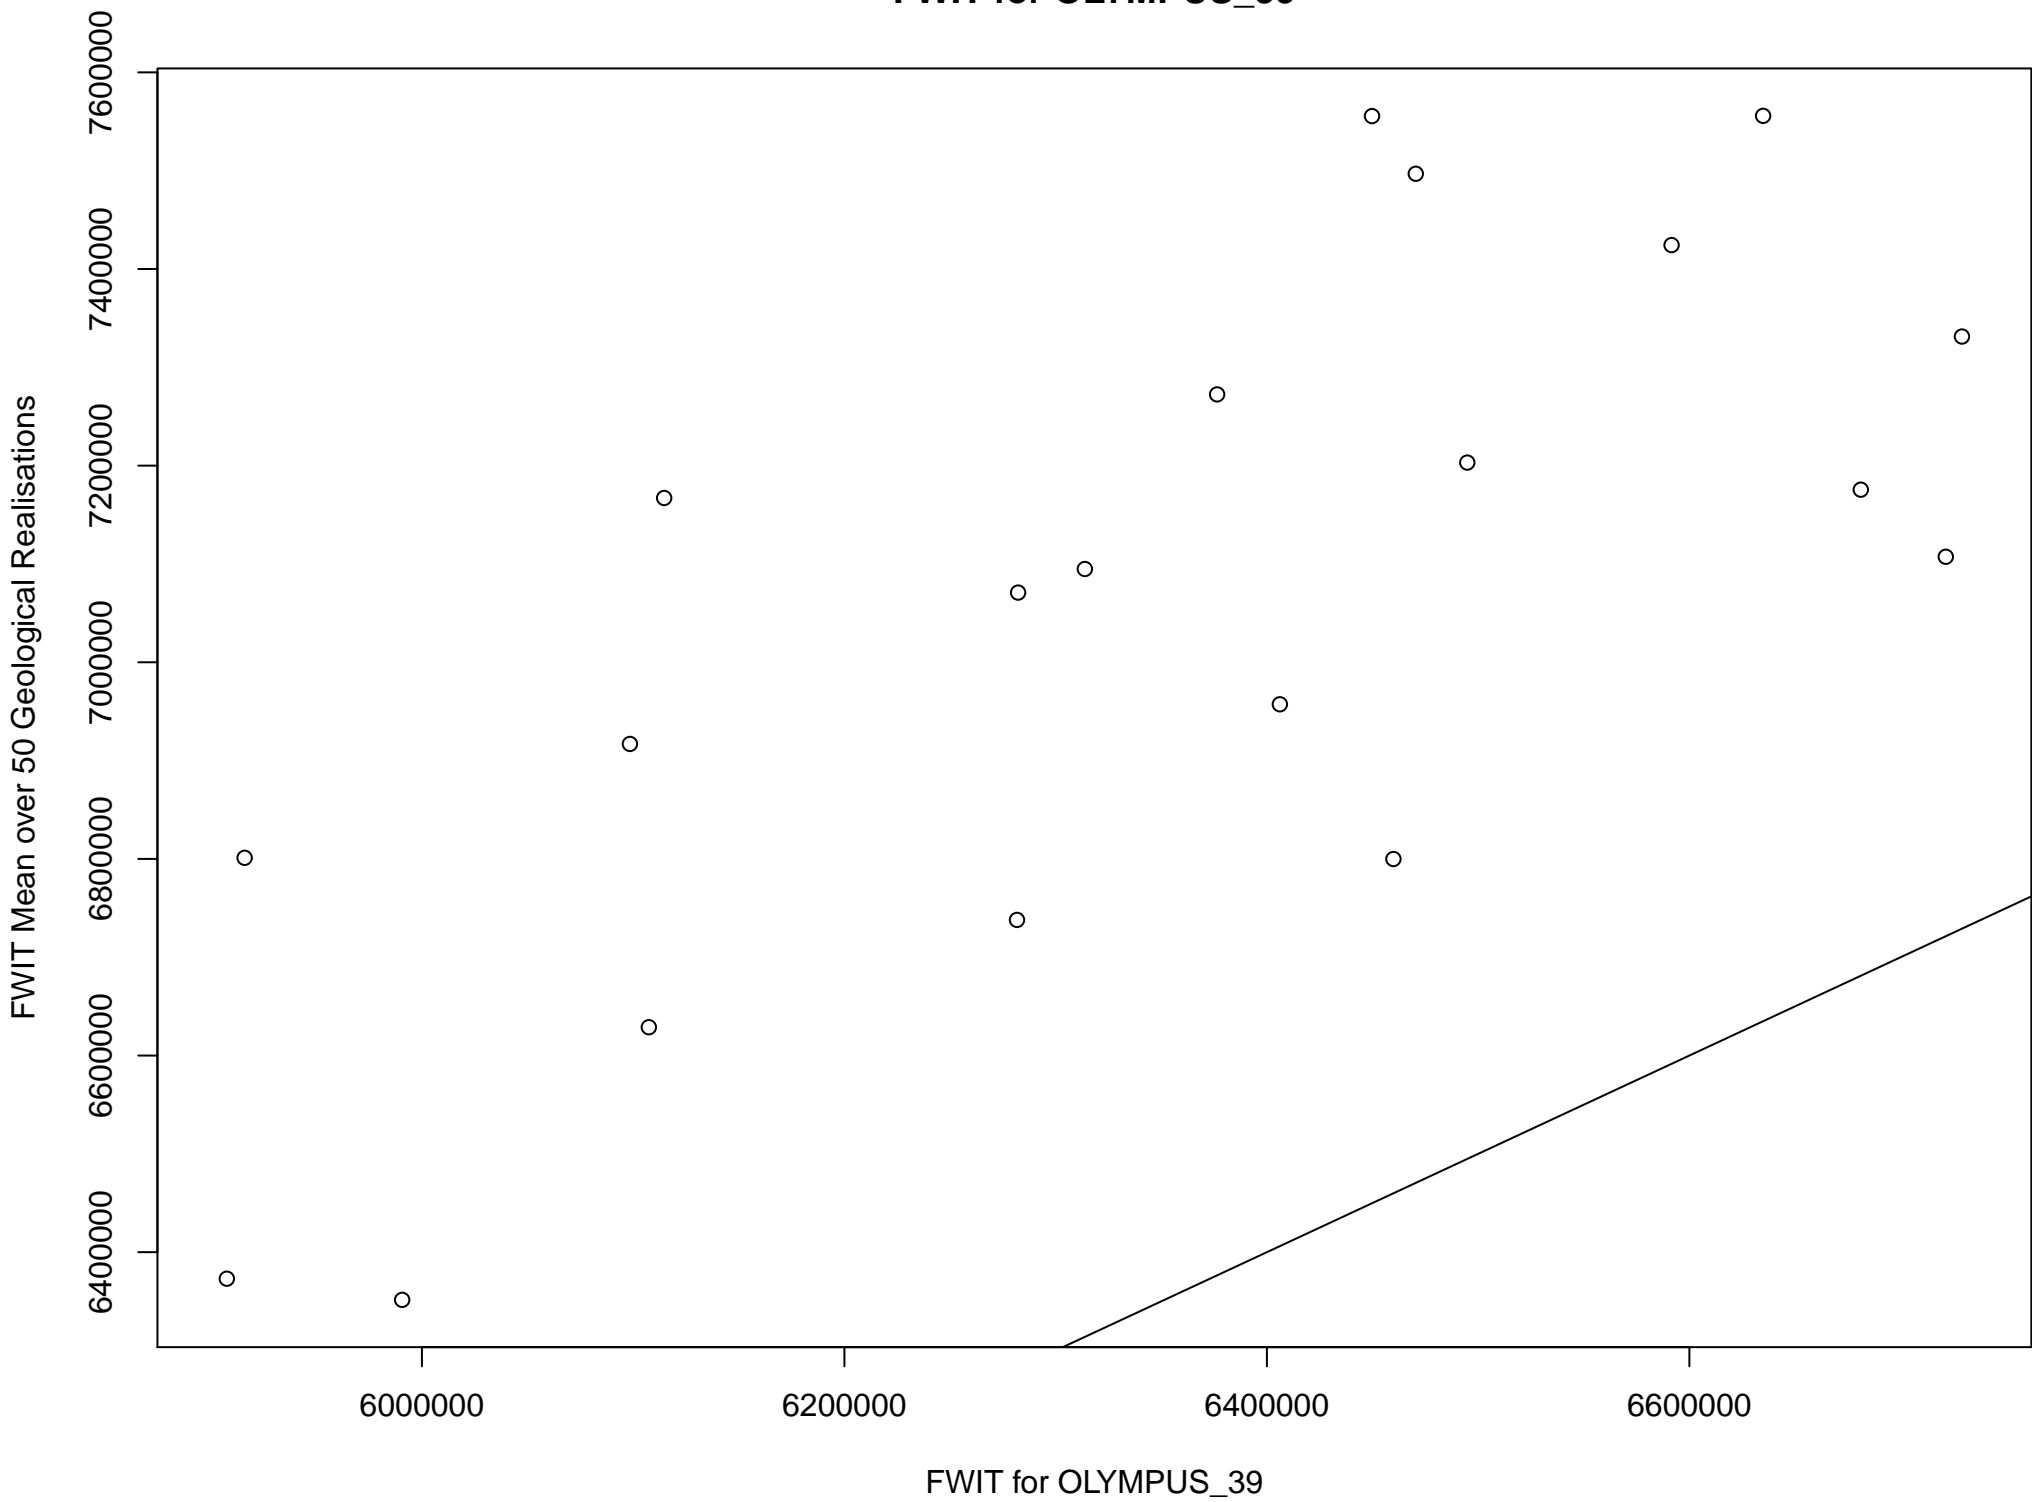

FWIT for OLYMPUS\_40

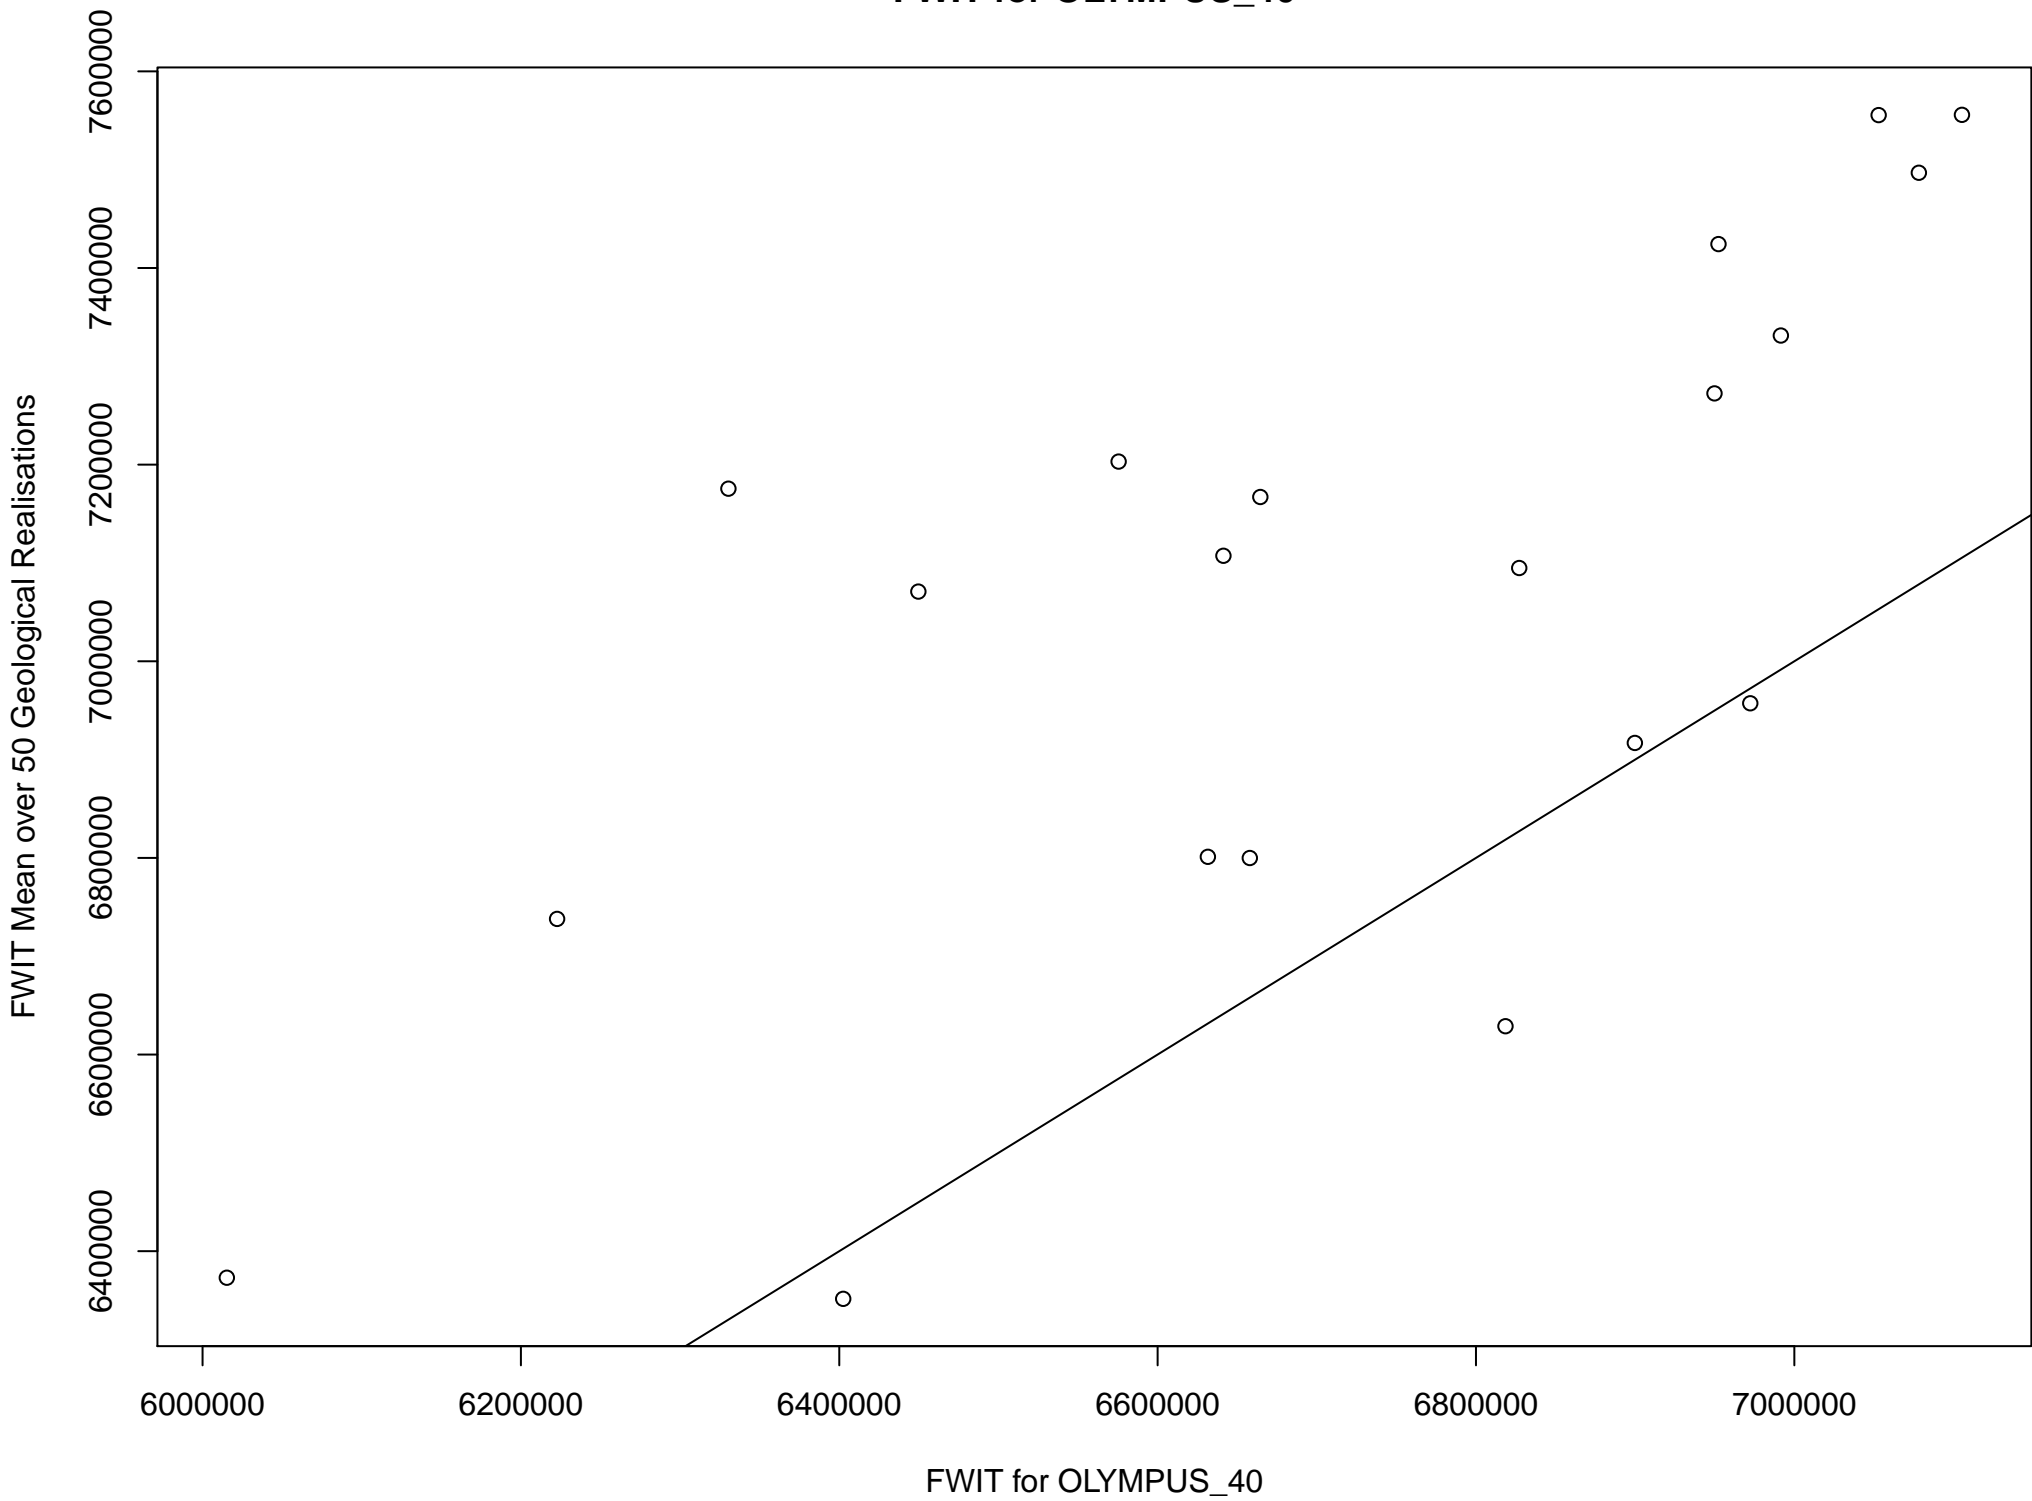



FWIT for OLYMPUS\_41

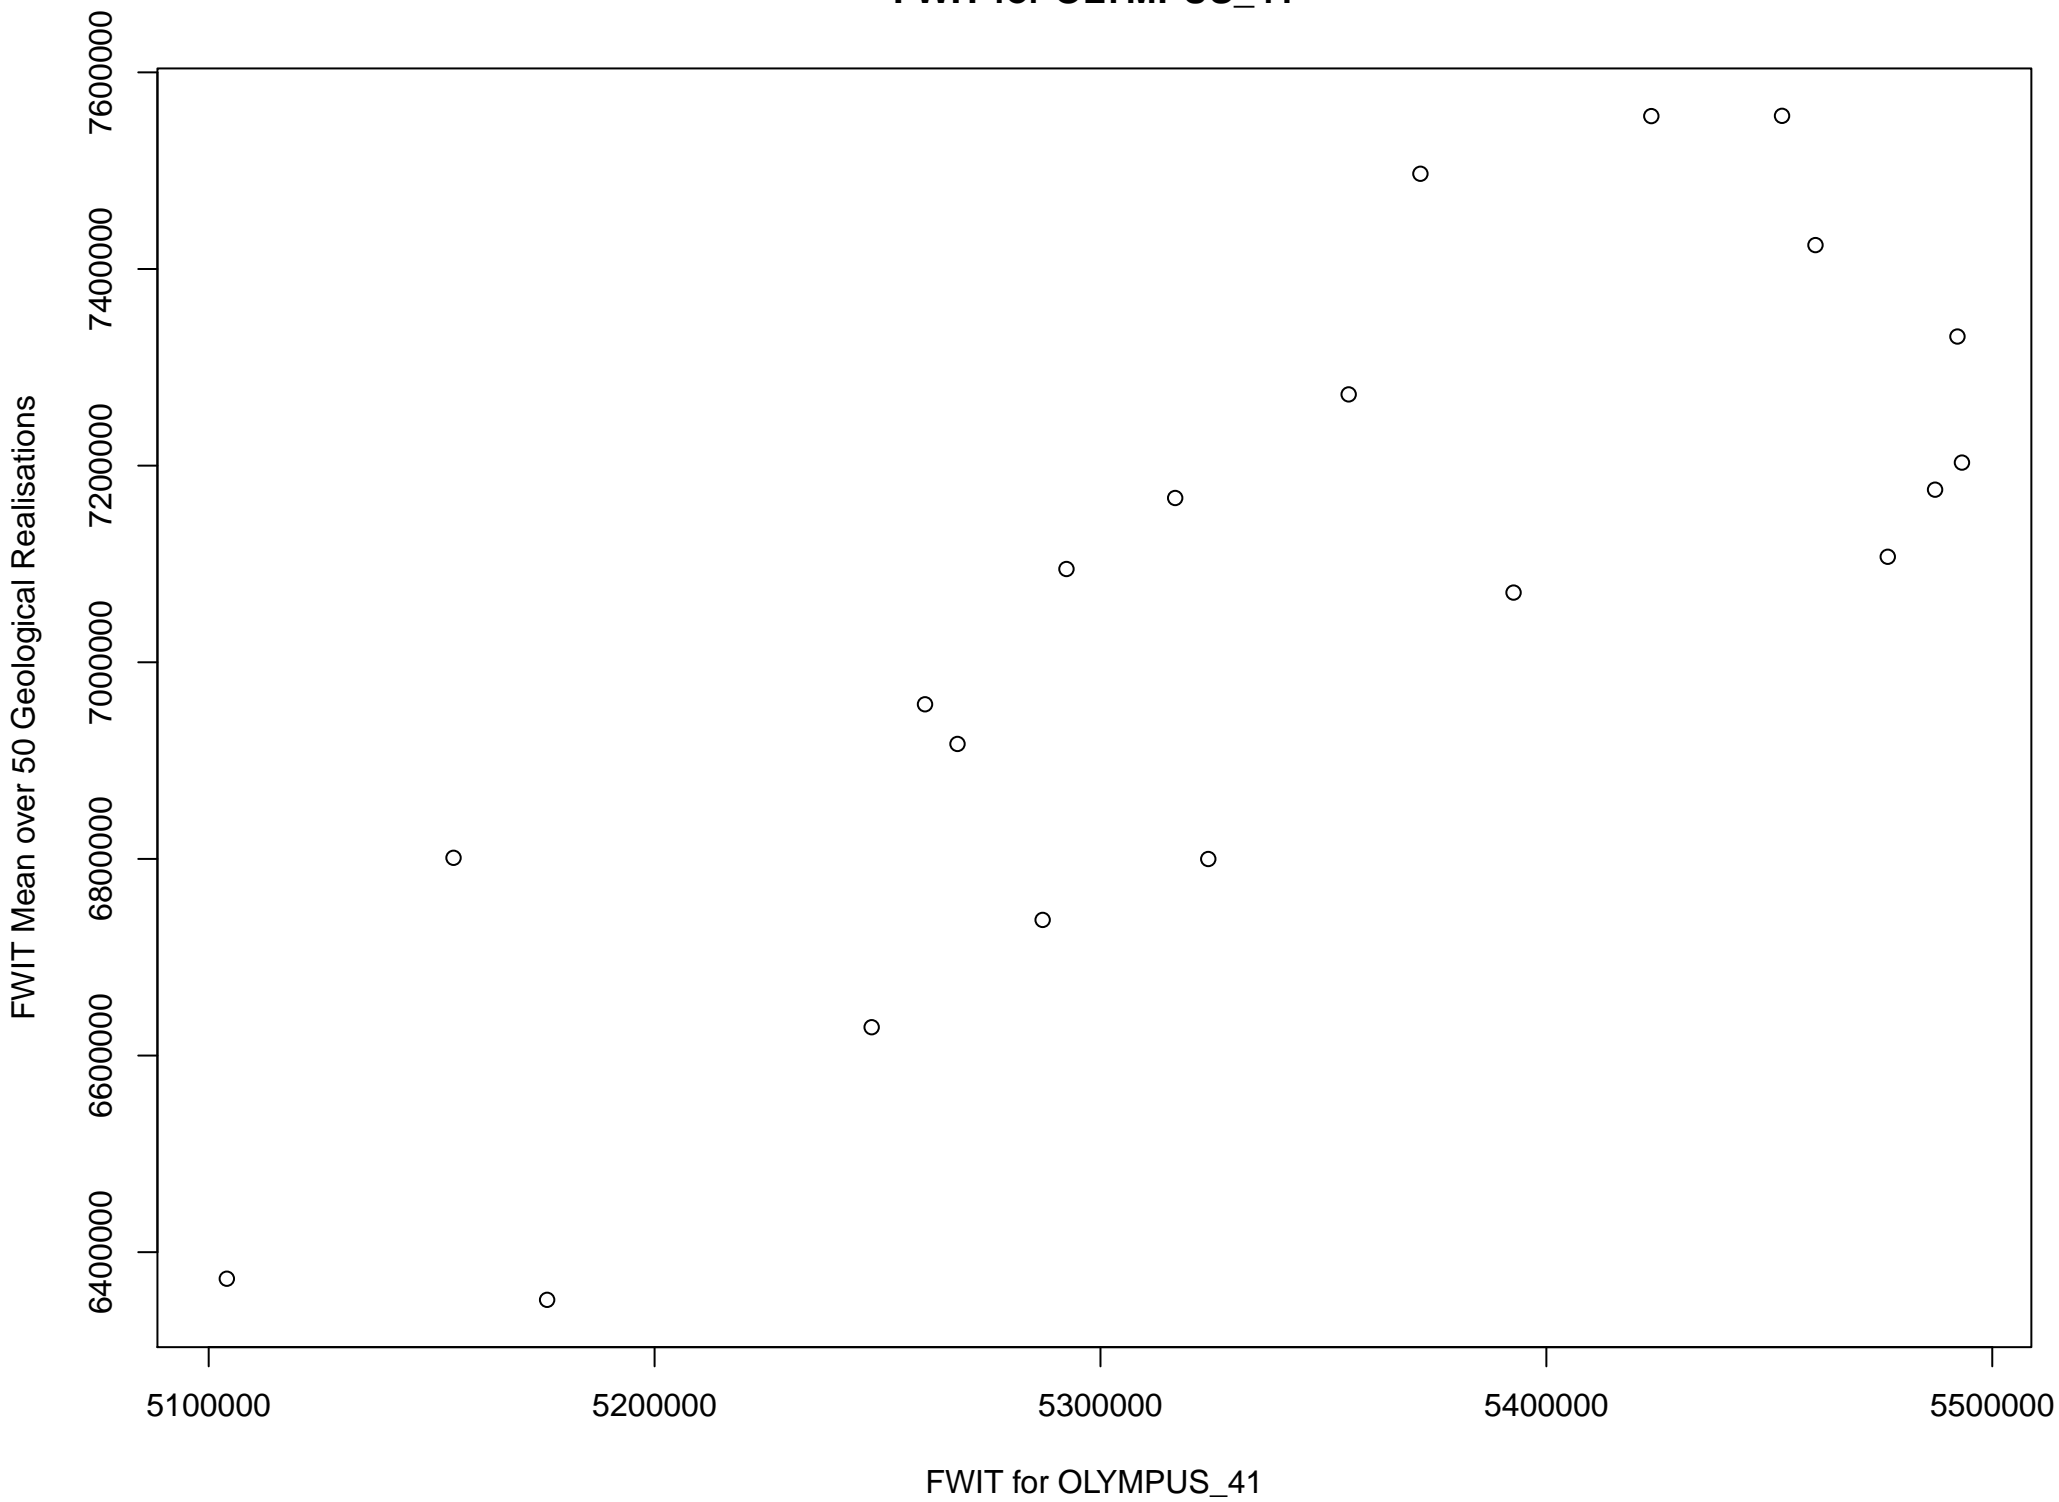

FWIT for OLYMPUS\_42

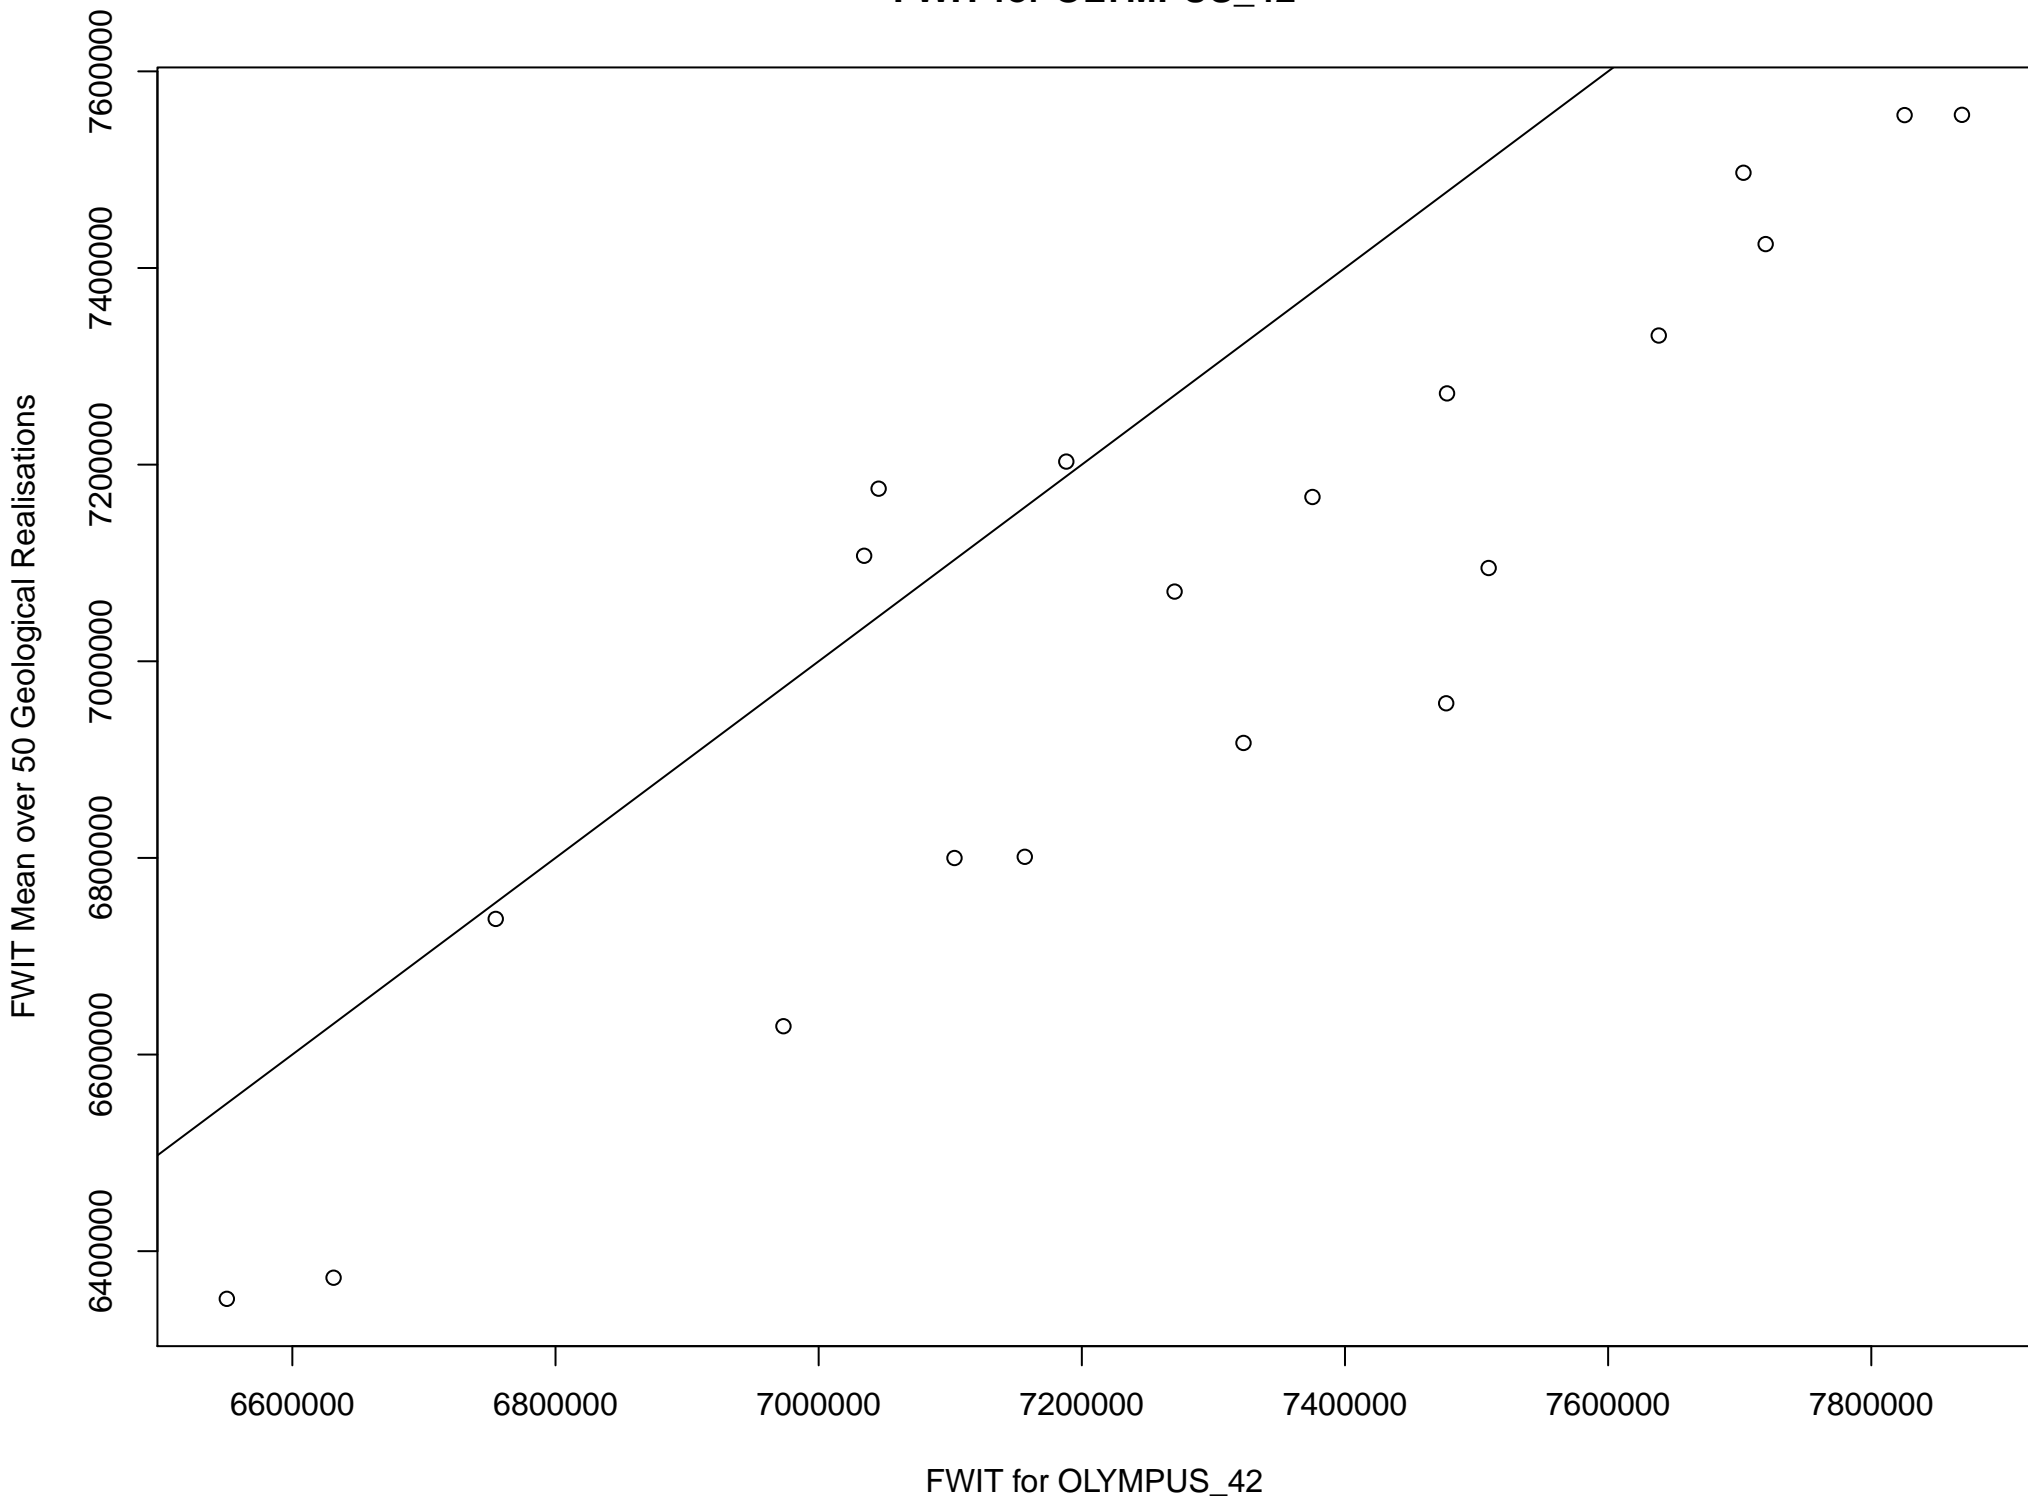

FWIT for OLYMPUS\_43

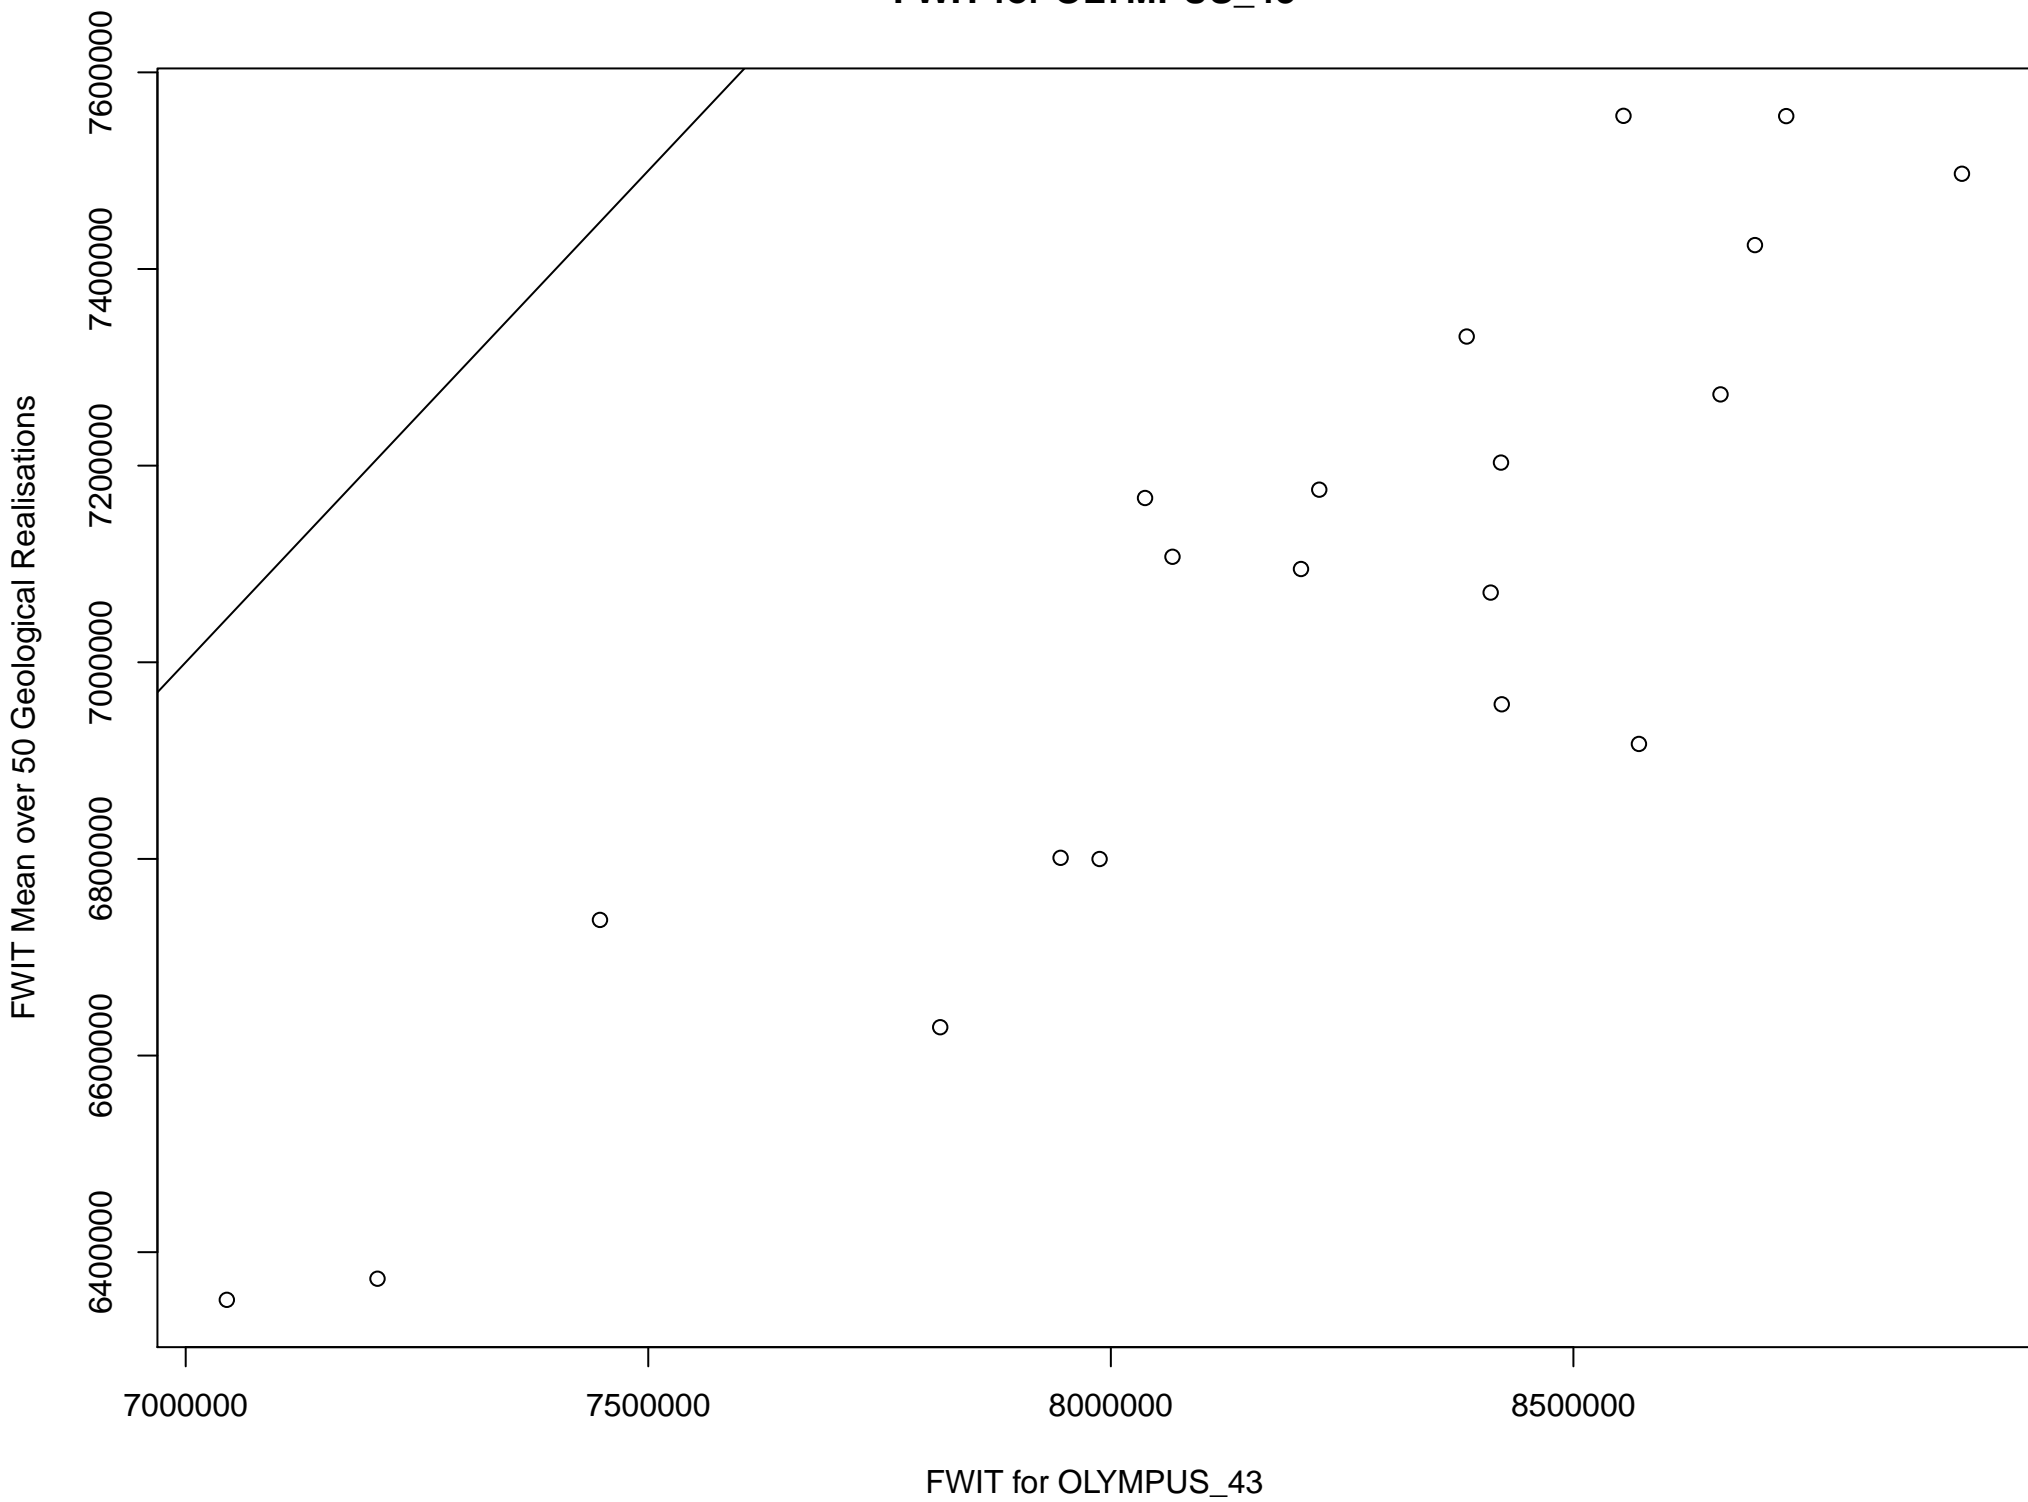

FWIT for OLYMPUS\_44

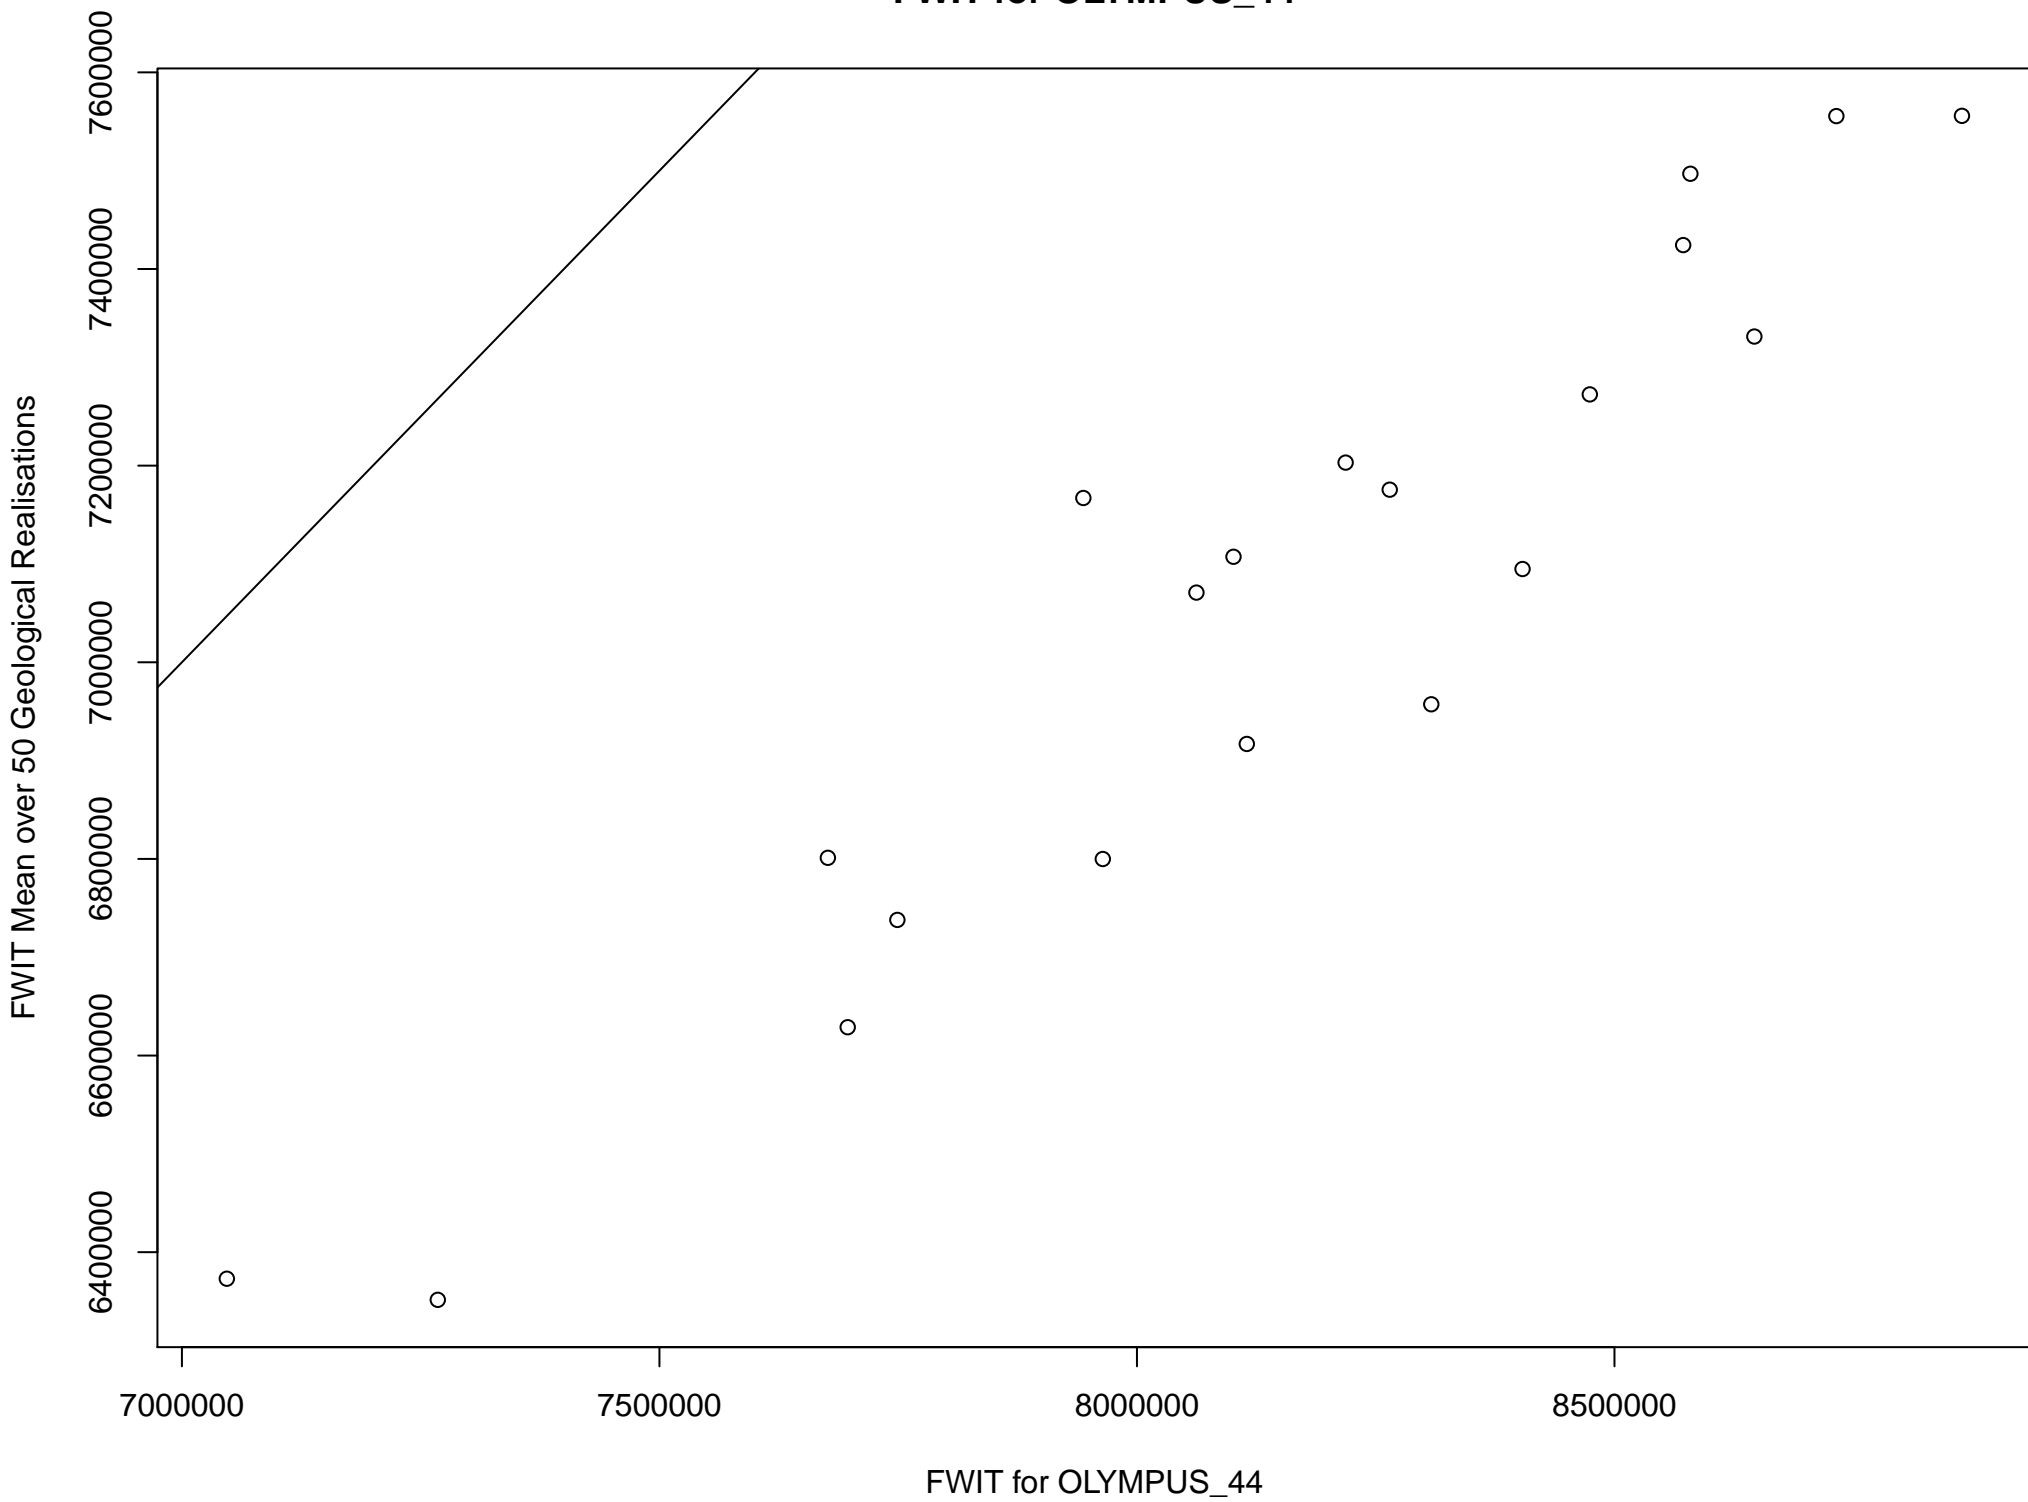

FWIT for OLYMPUS\_45

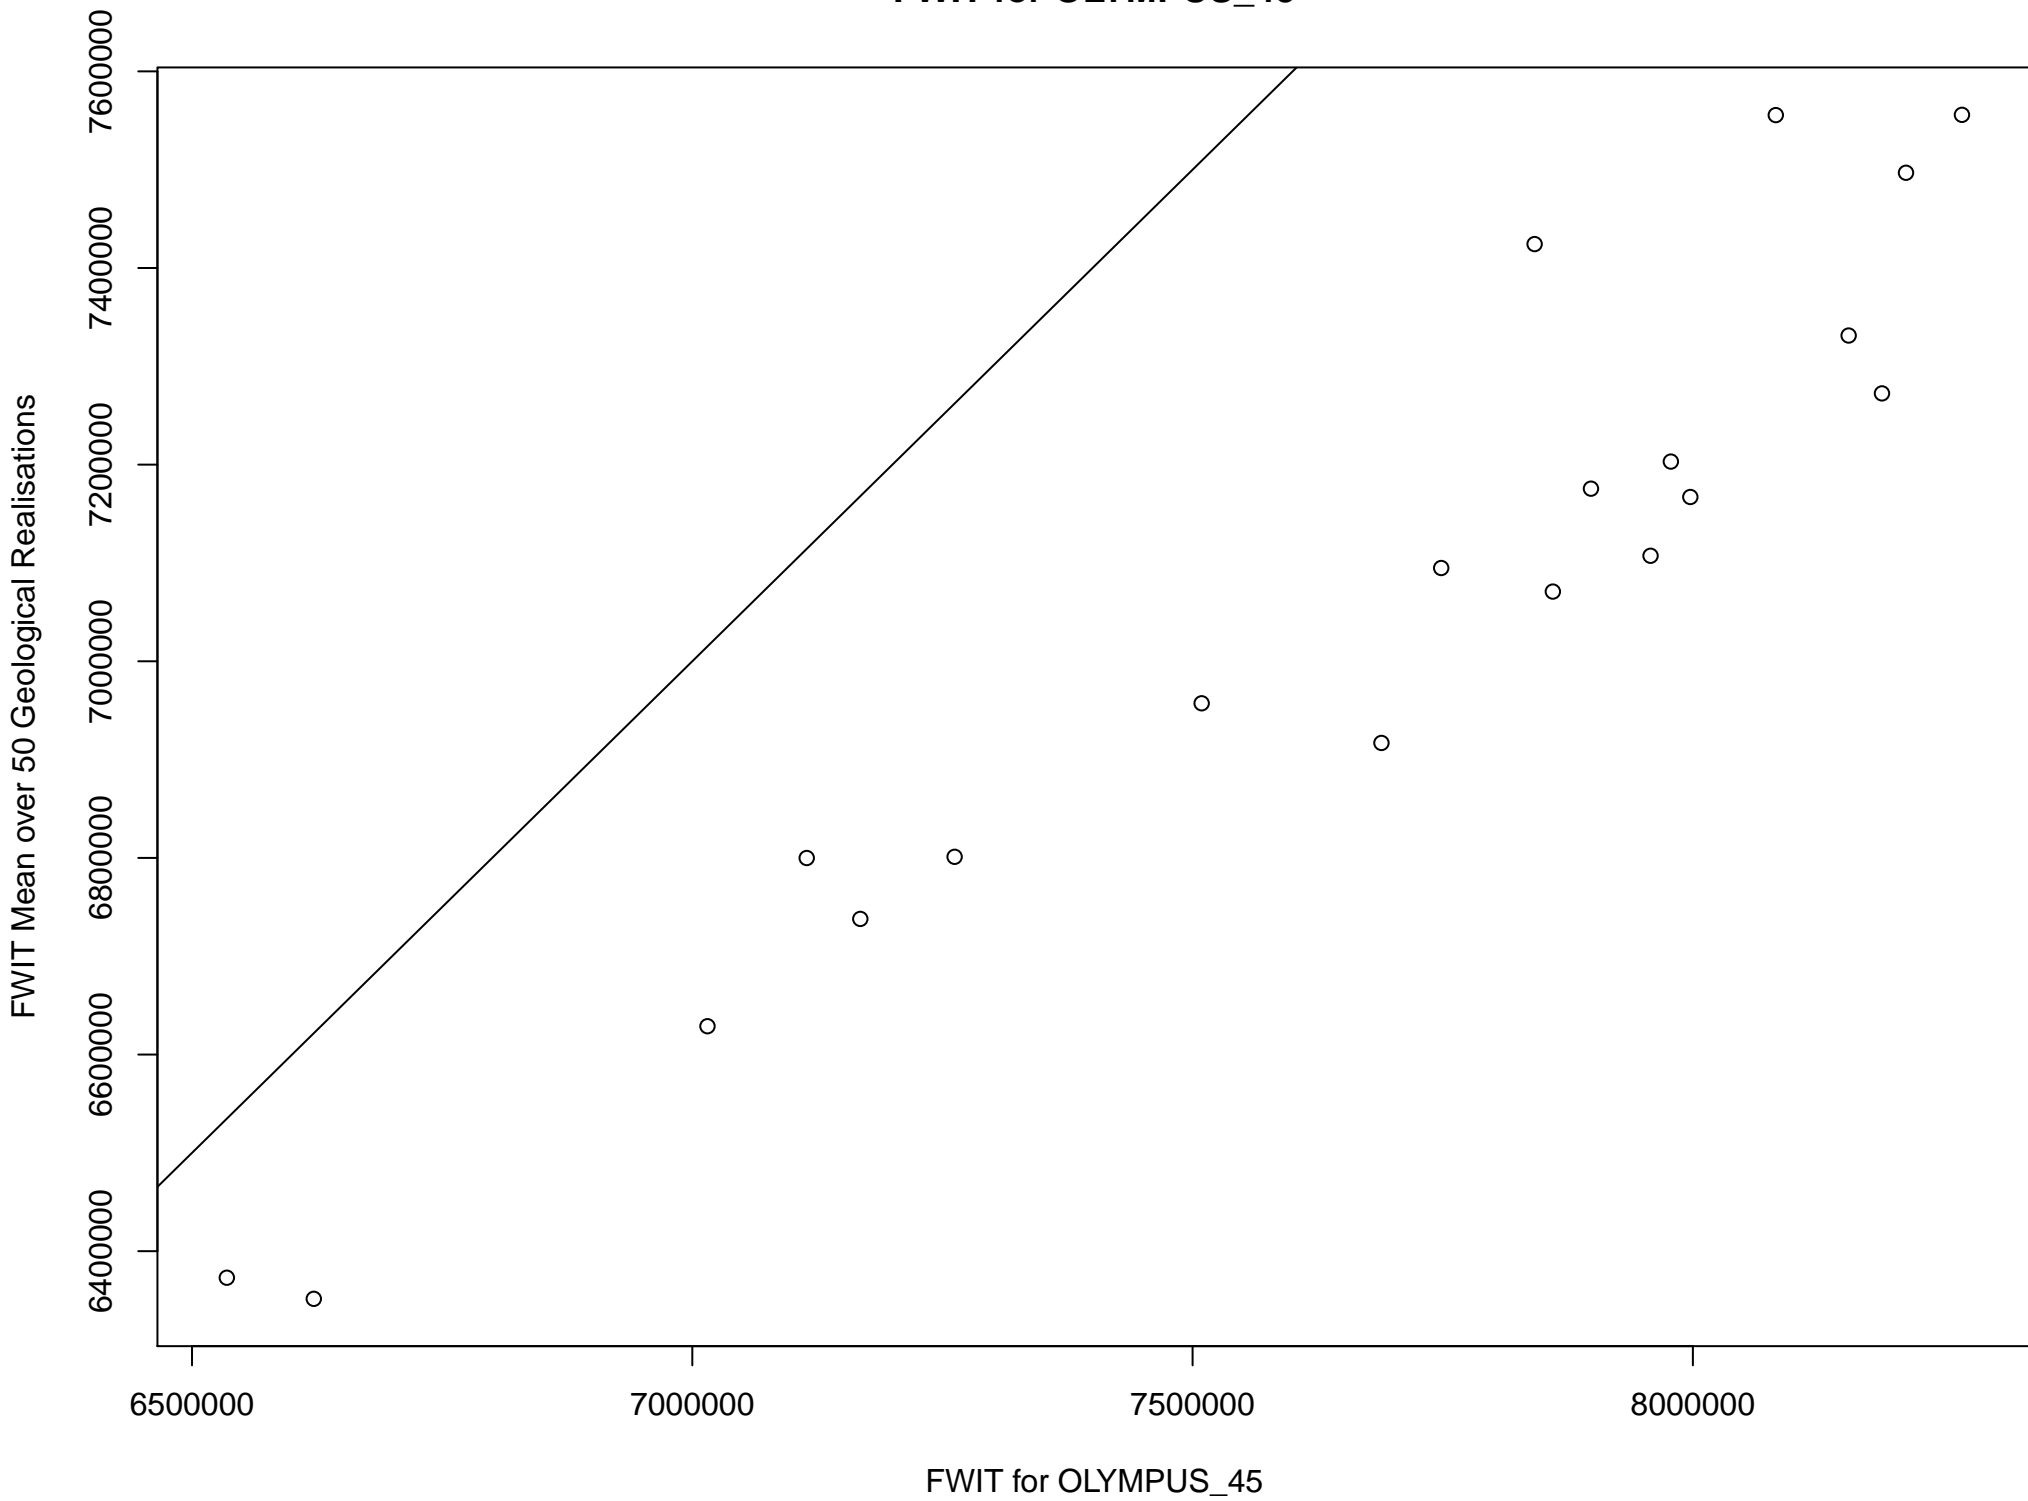

FWIT for OLYMPUS\_46

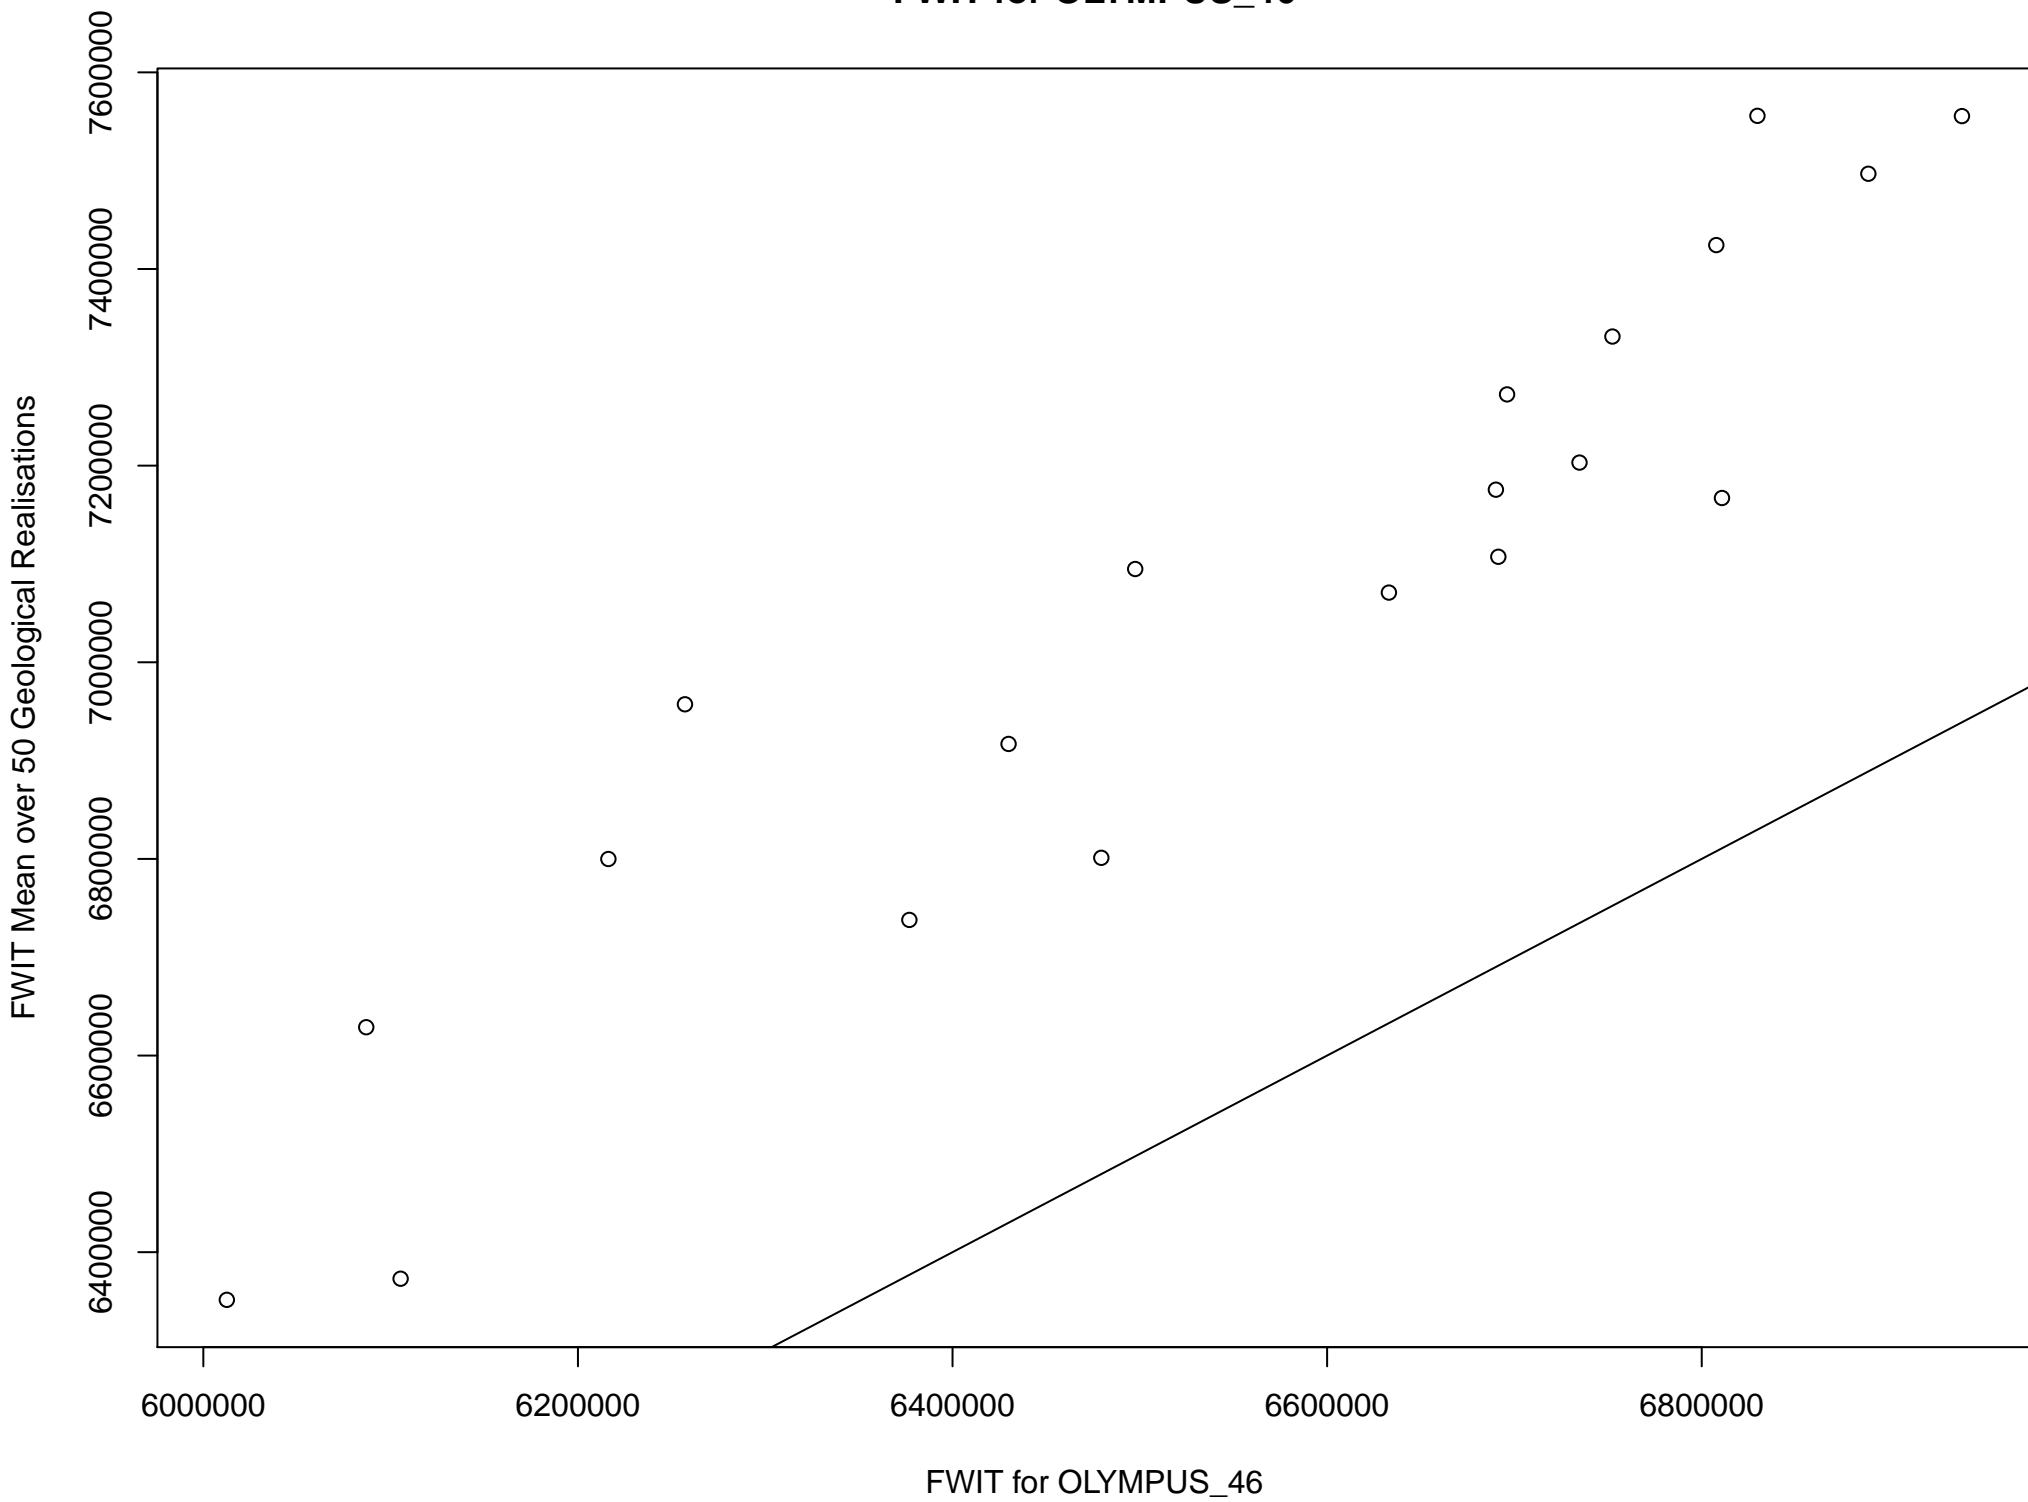

FWIT for OLYMPUS\_47

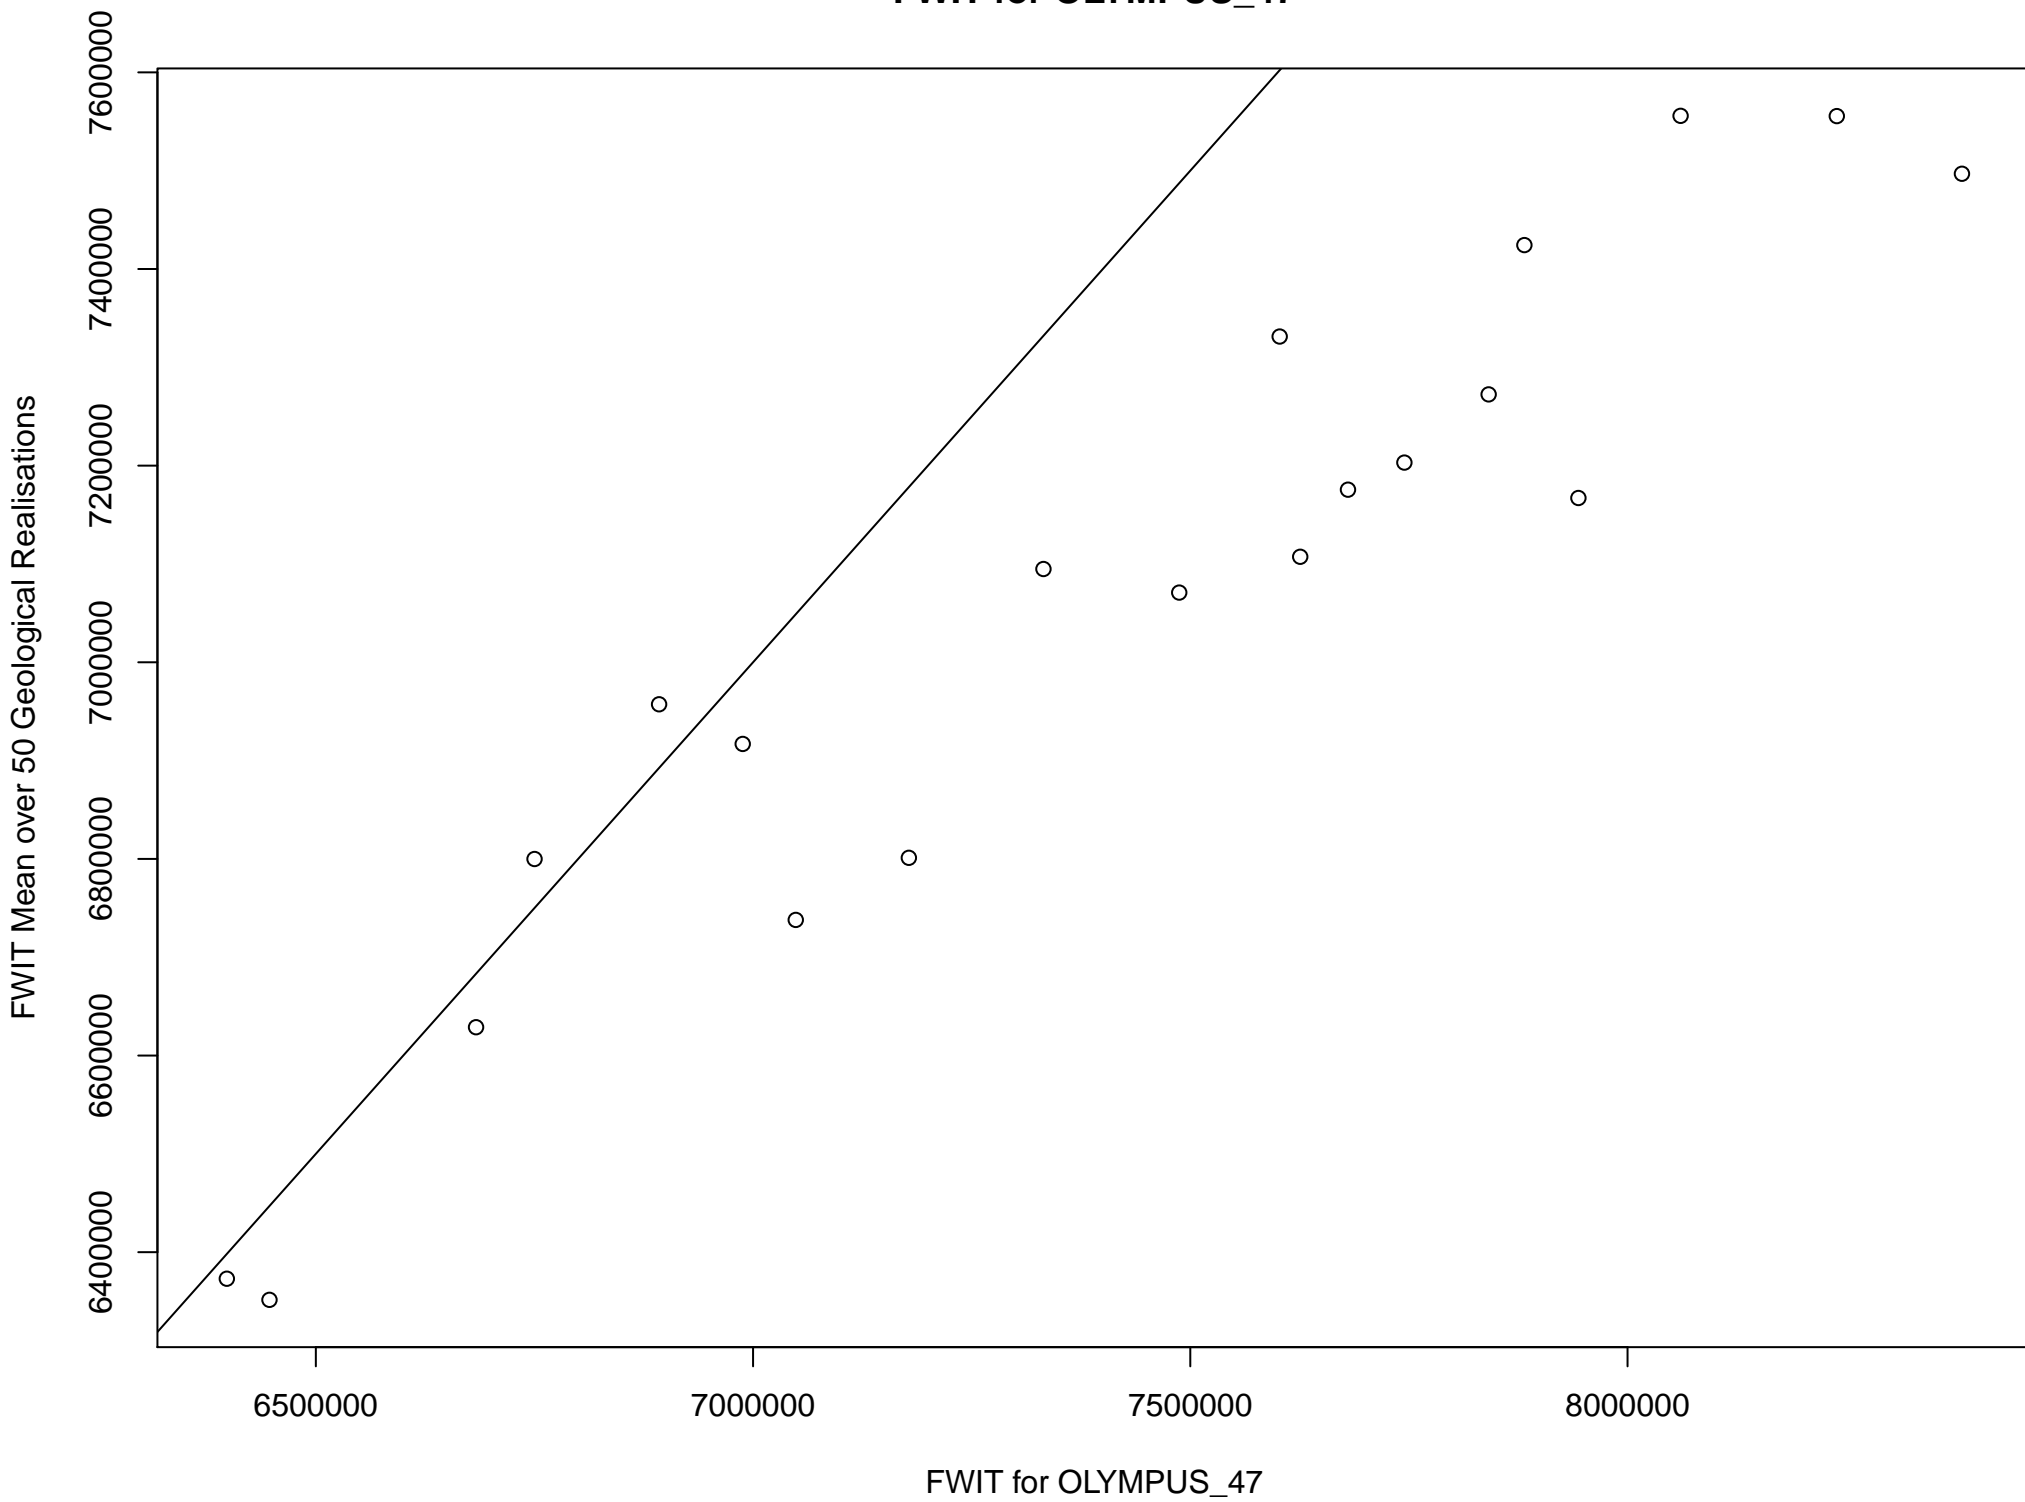

FWIT for OLYMPUS\_48

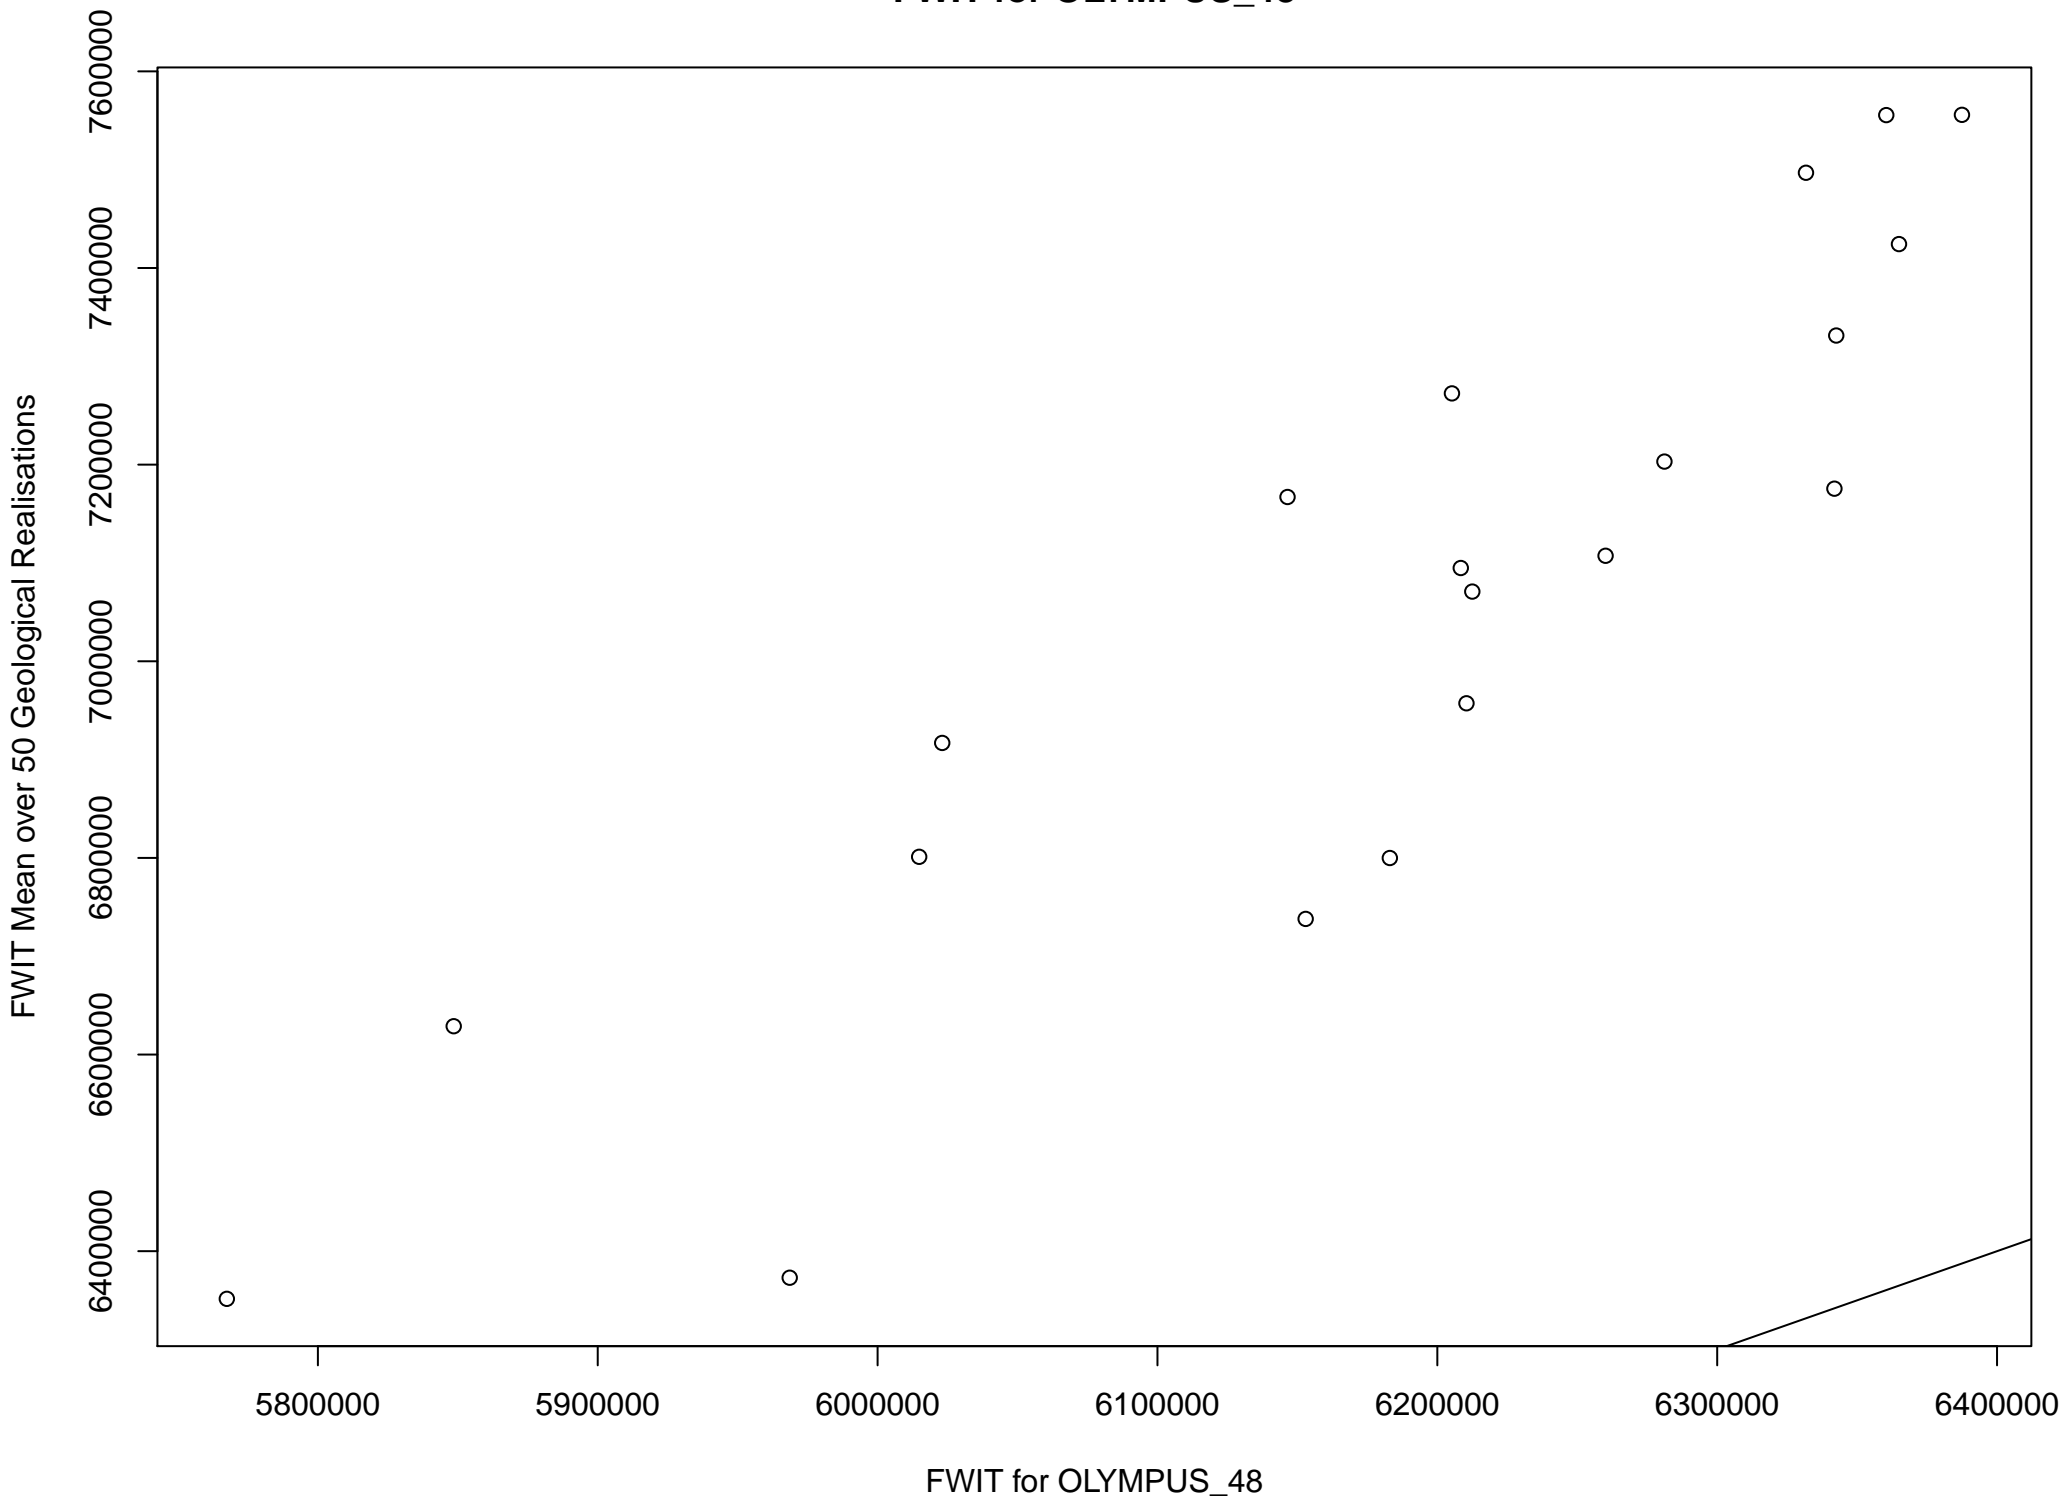



FWIT for OLYMPUS\_49

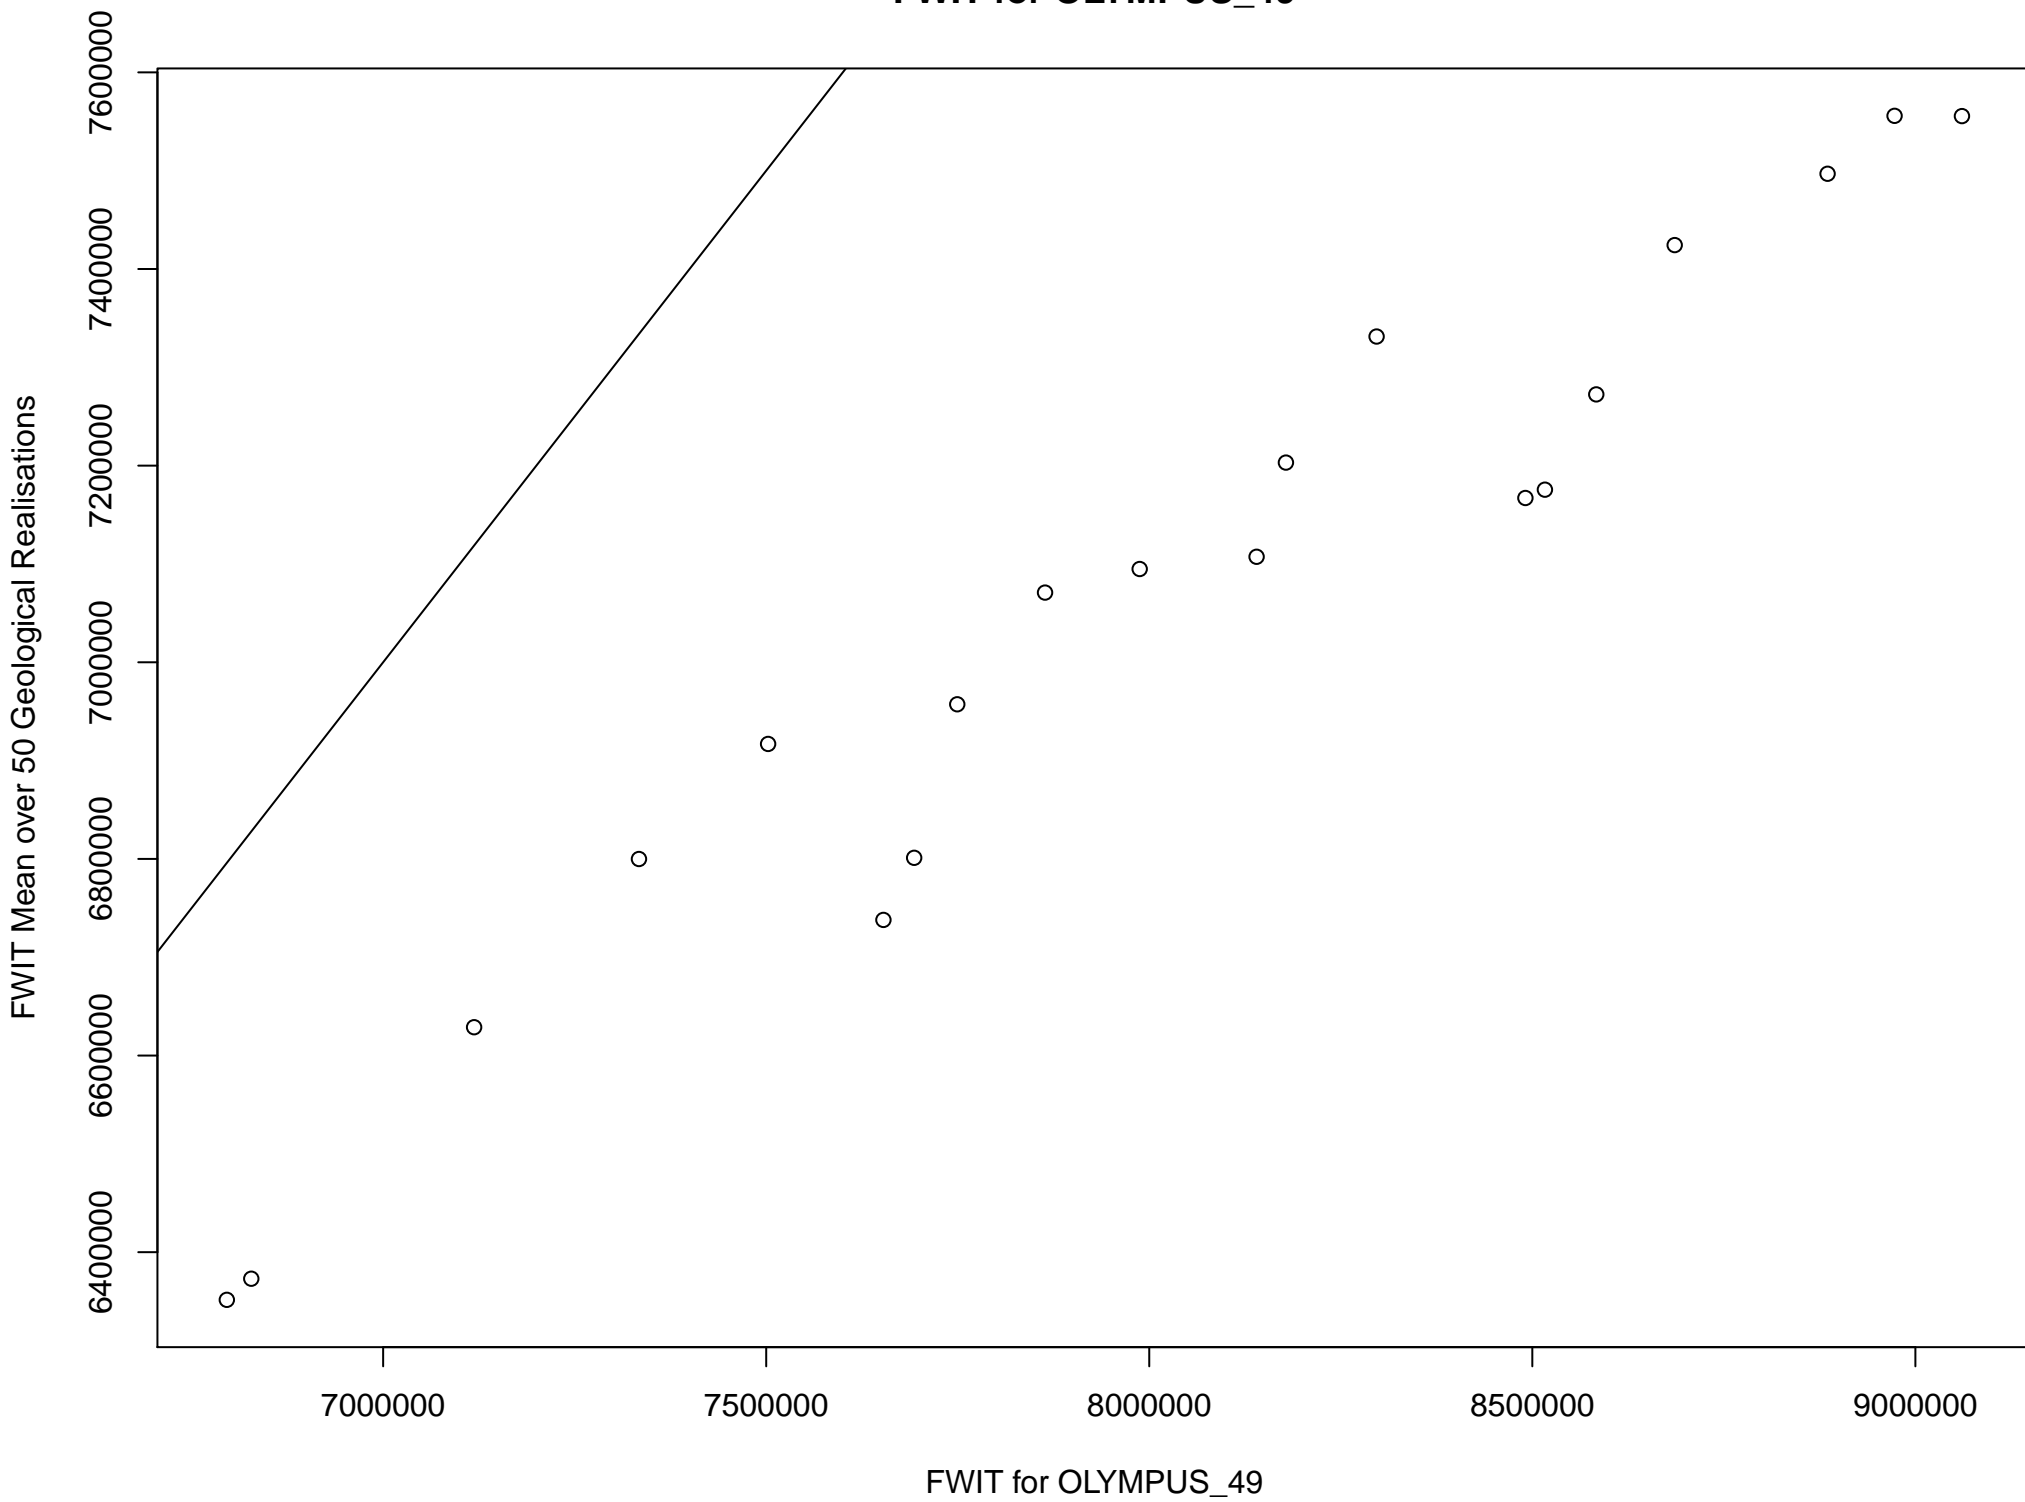

FWIT for OLYMPUS\_50

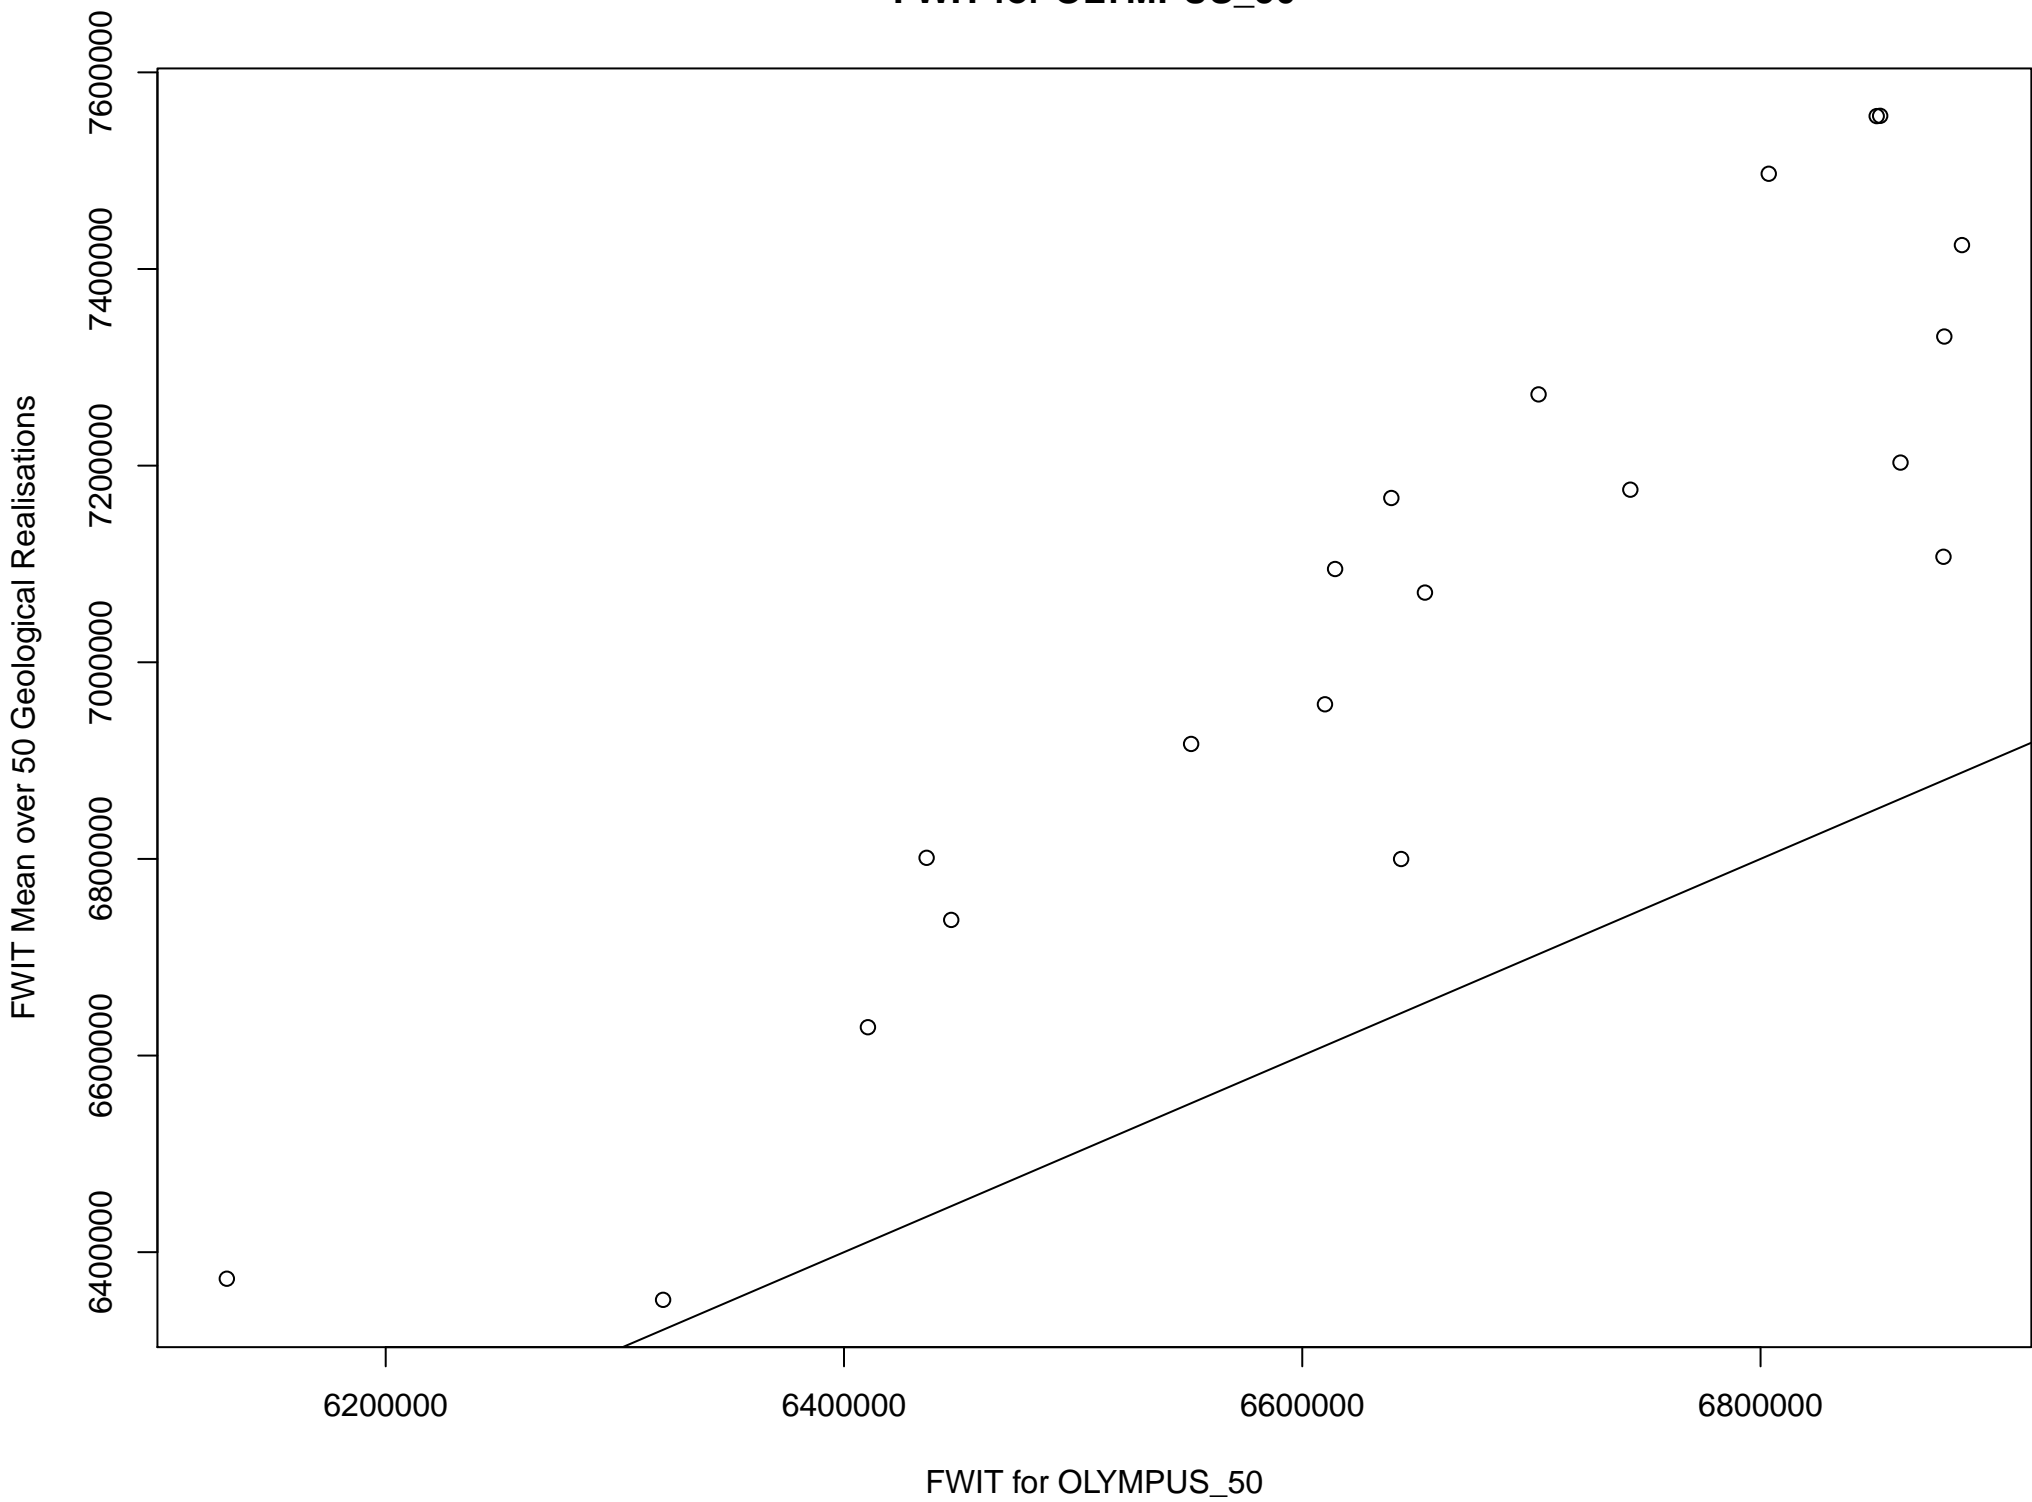

Supplement: Supplementary file 4 [file FWIT-Mean-vs-Model-Output-all-Models.pdf]
