# Supplementary material for: Bayesian Emulation of Grey-Box Multi-Model Ensembles Exploiting Known Interior Structure
Source: arXiv:2406.08367 source file (2025-05-02)

# WOPT.PROD.2 for OLYMPUS\_1

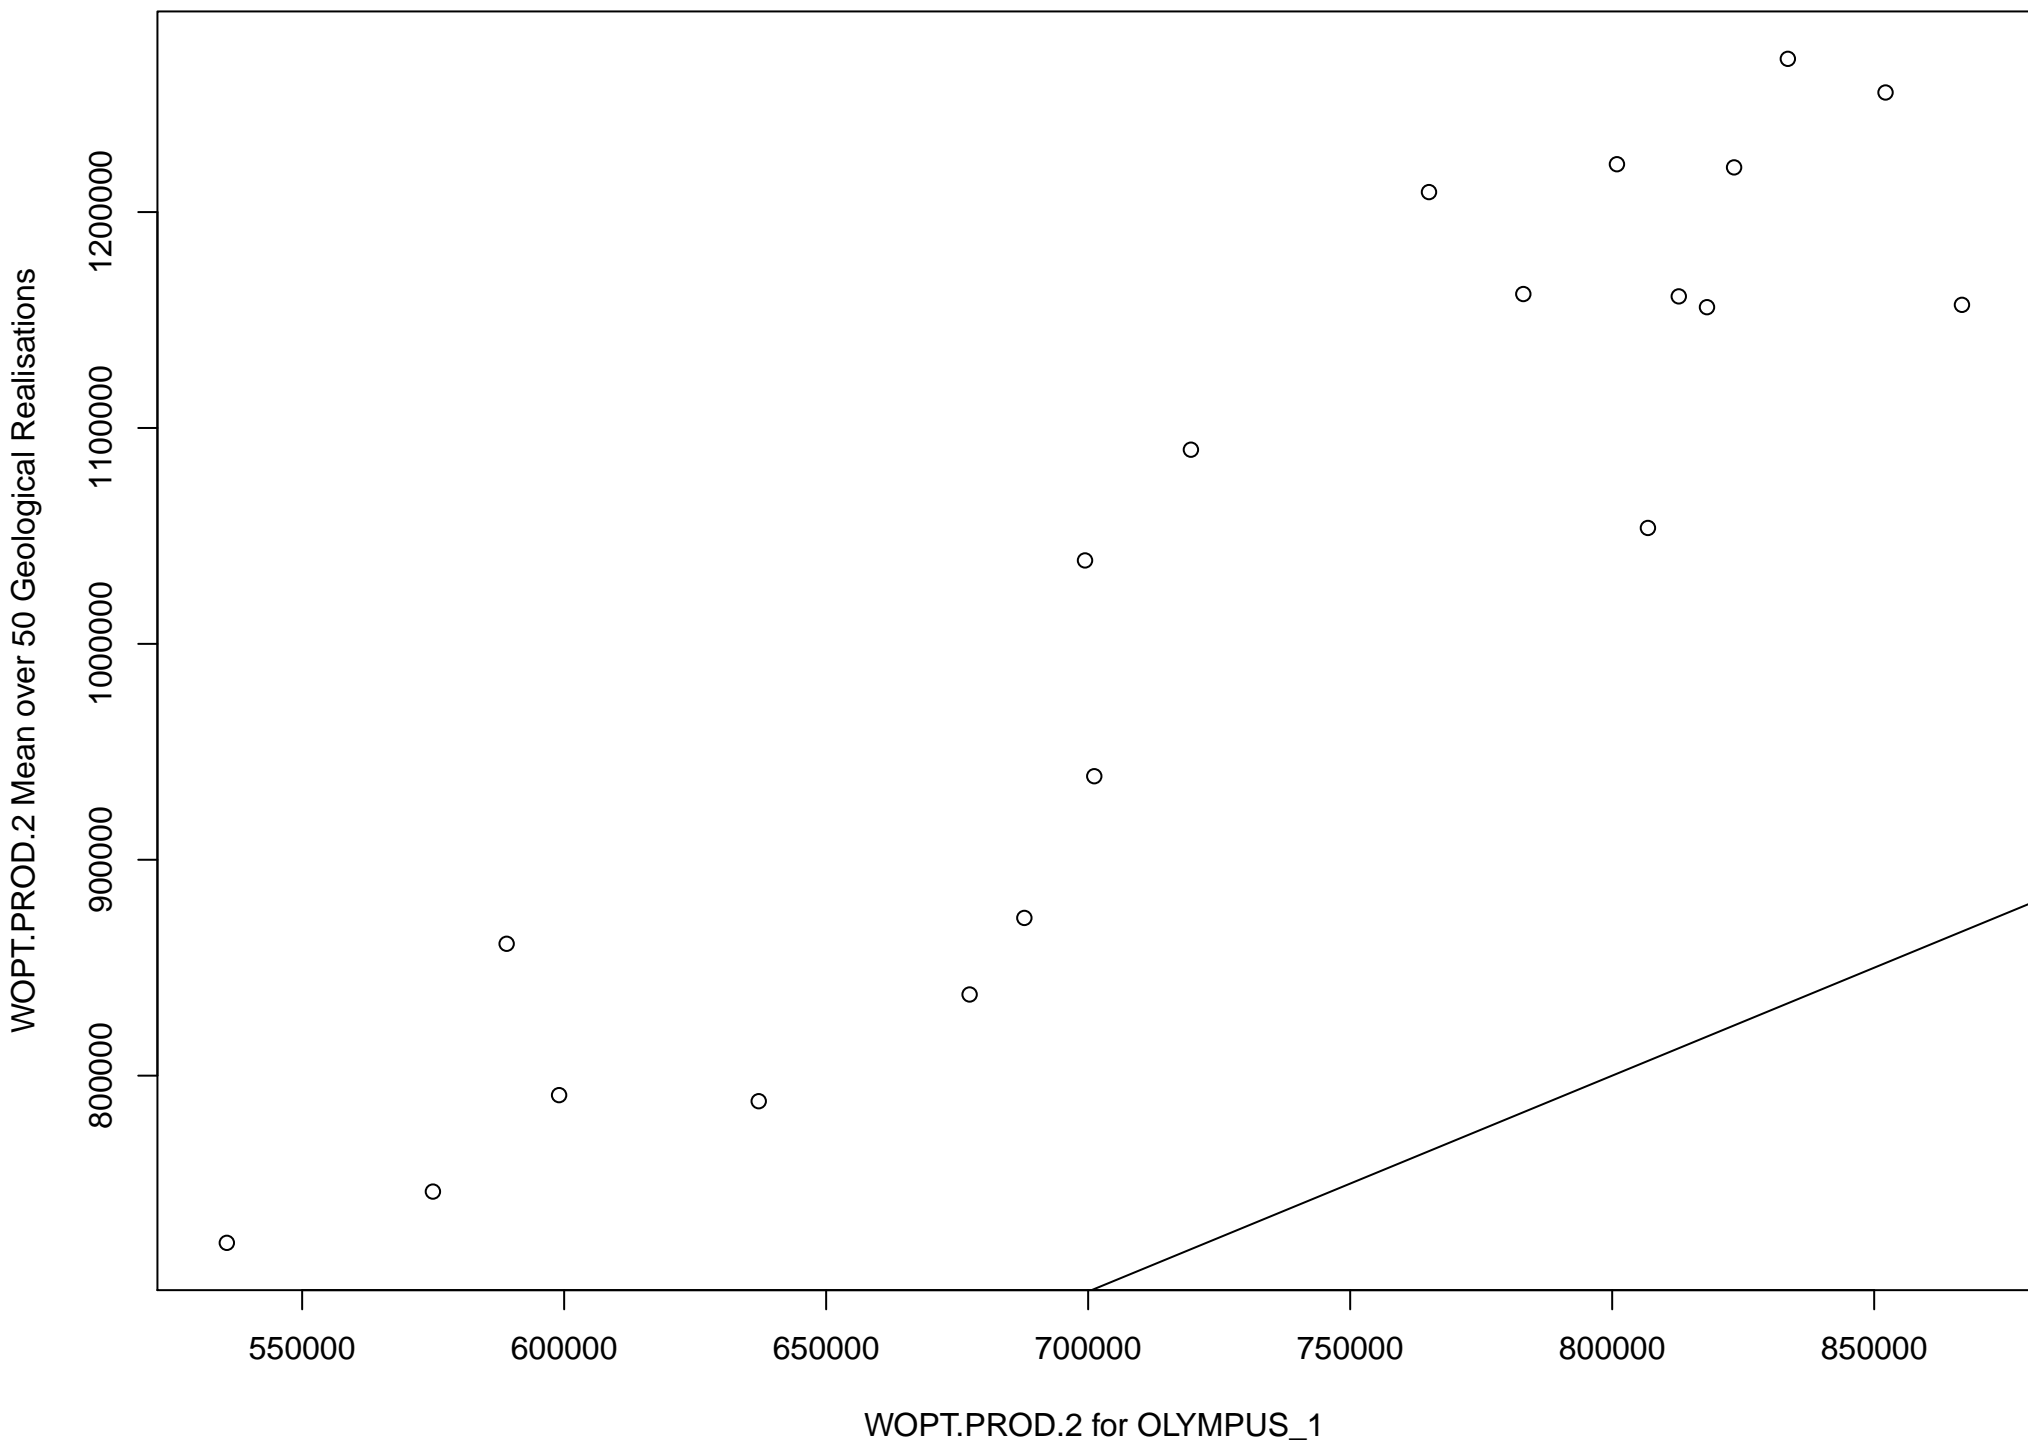

WOPT.PROD.2 for OLYMPUS\_2

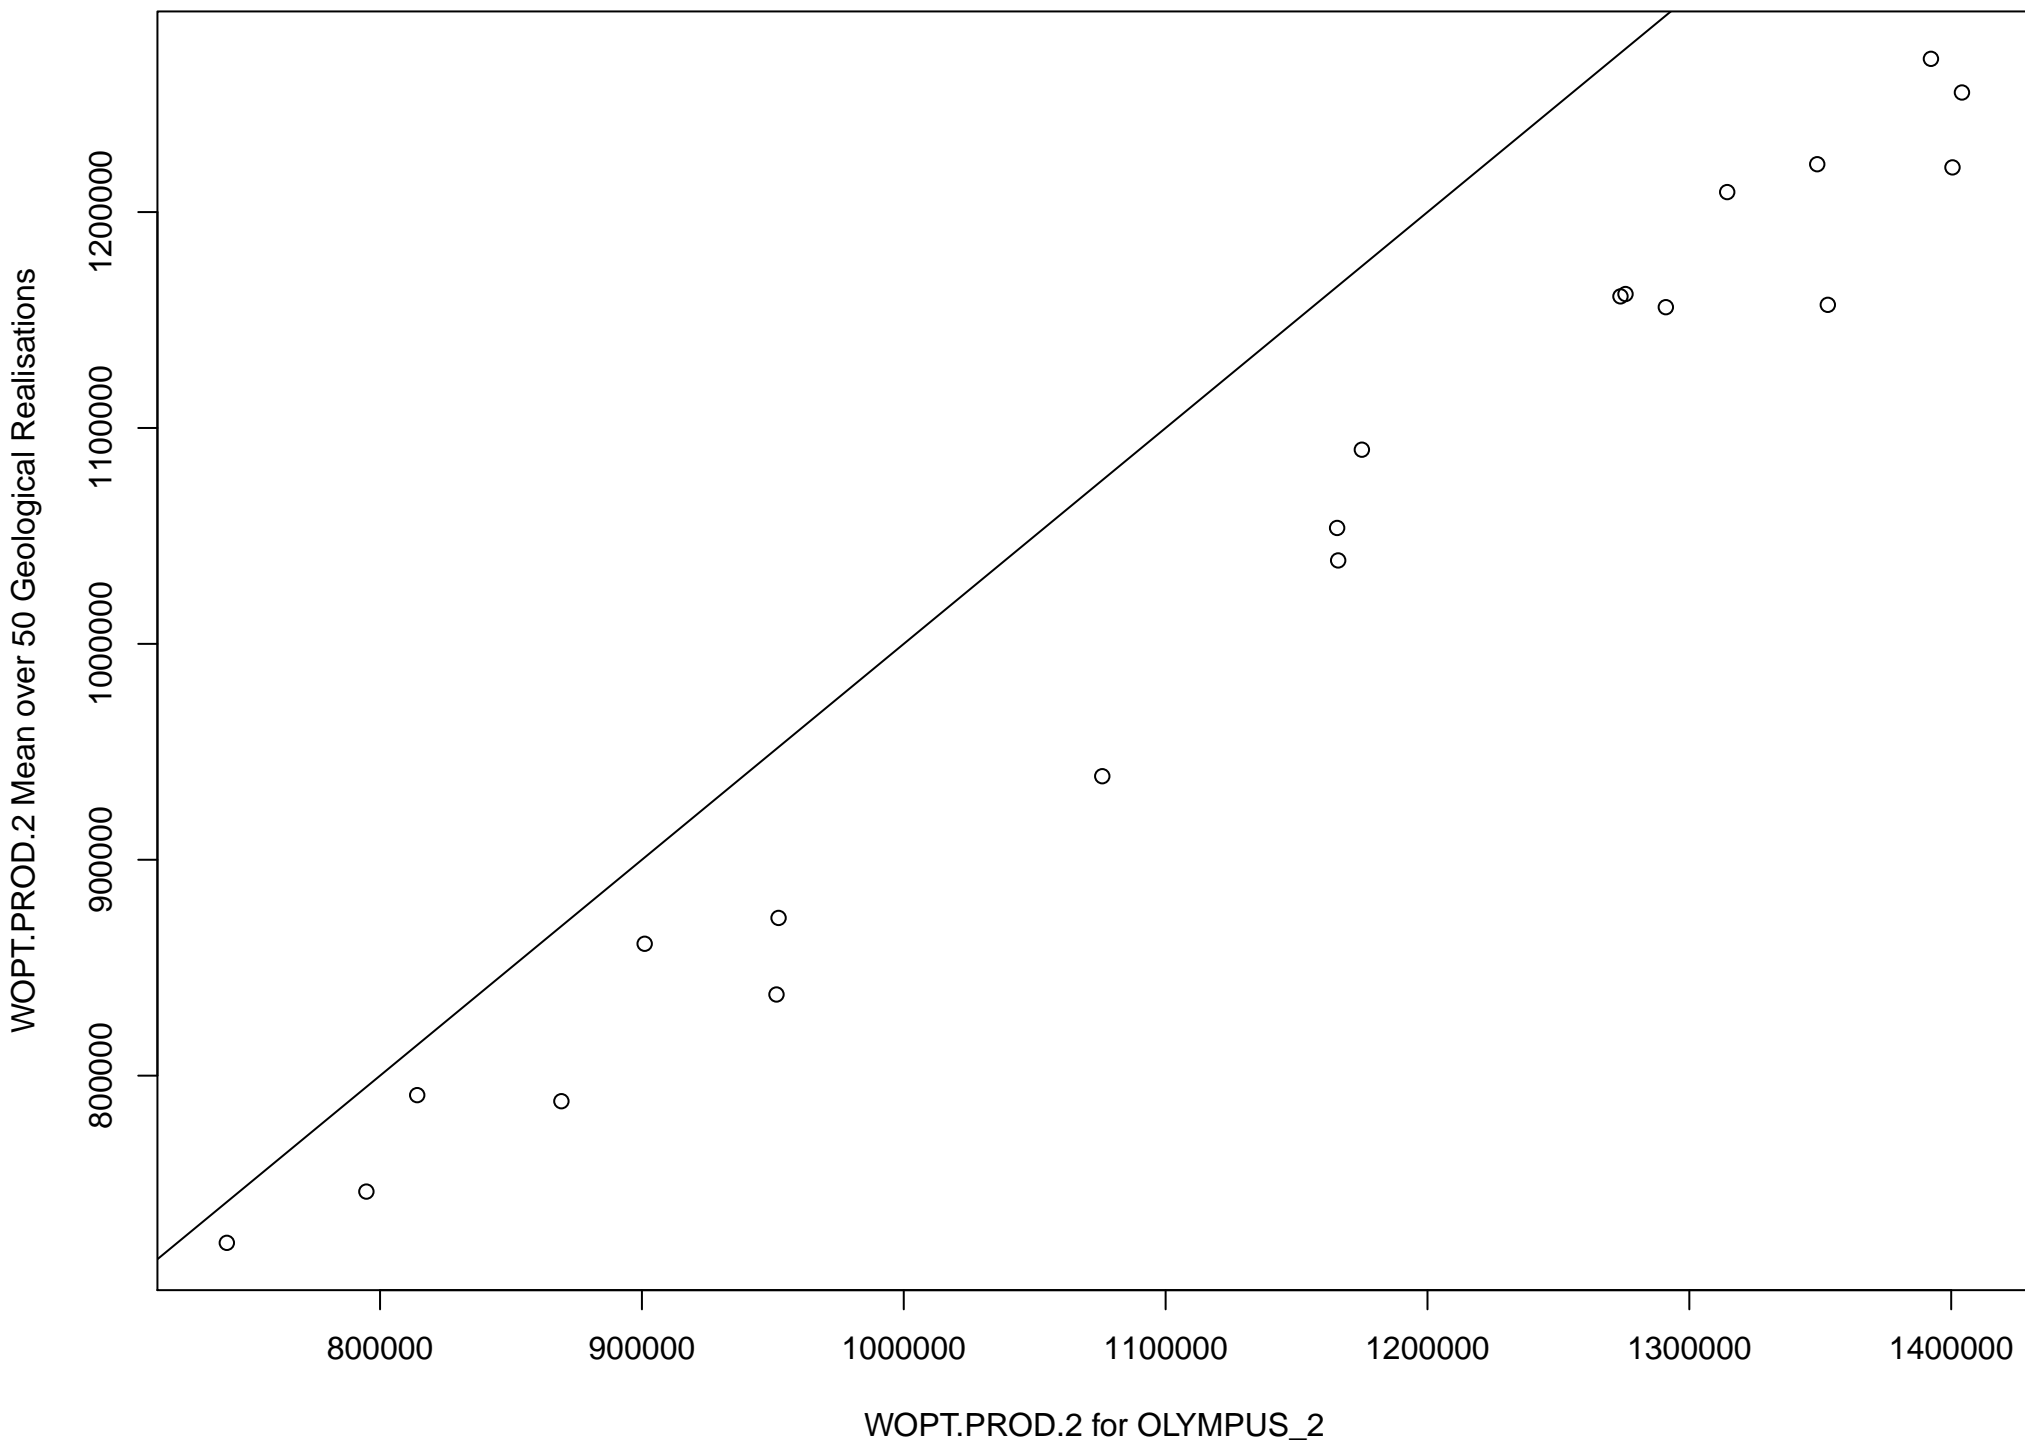

# WOPT.PROD.2 for OLYMPUS\_3

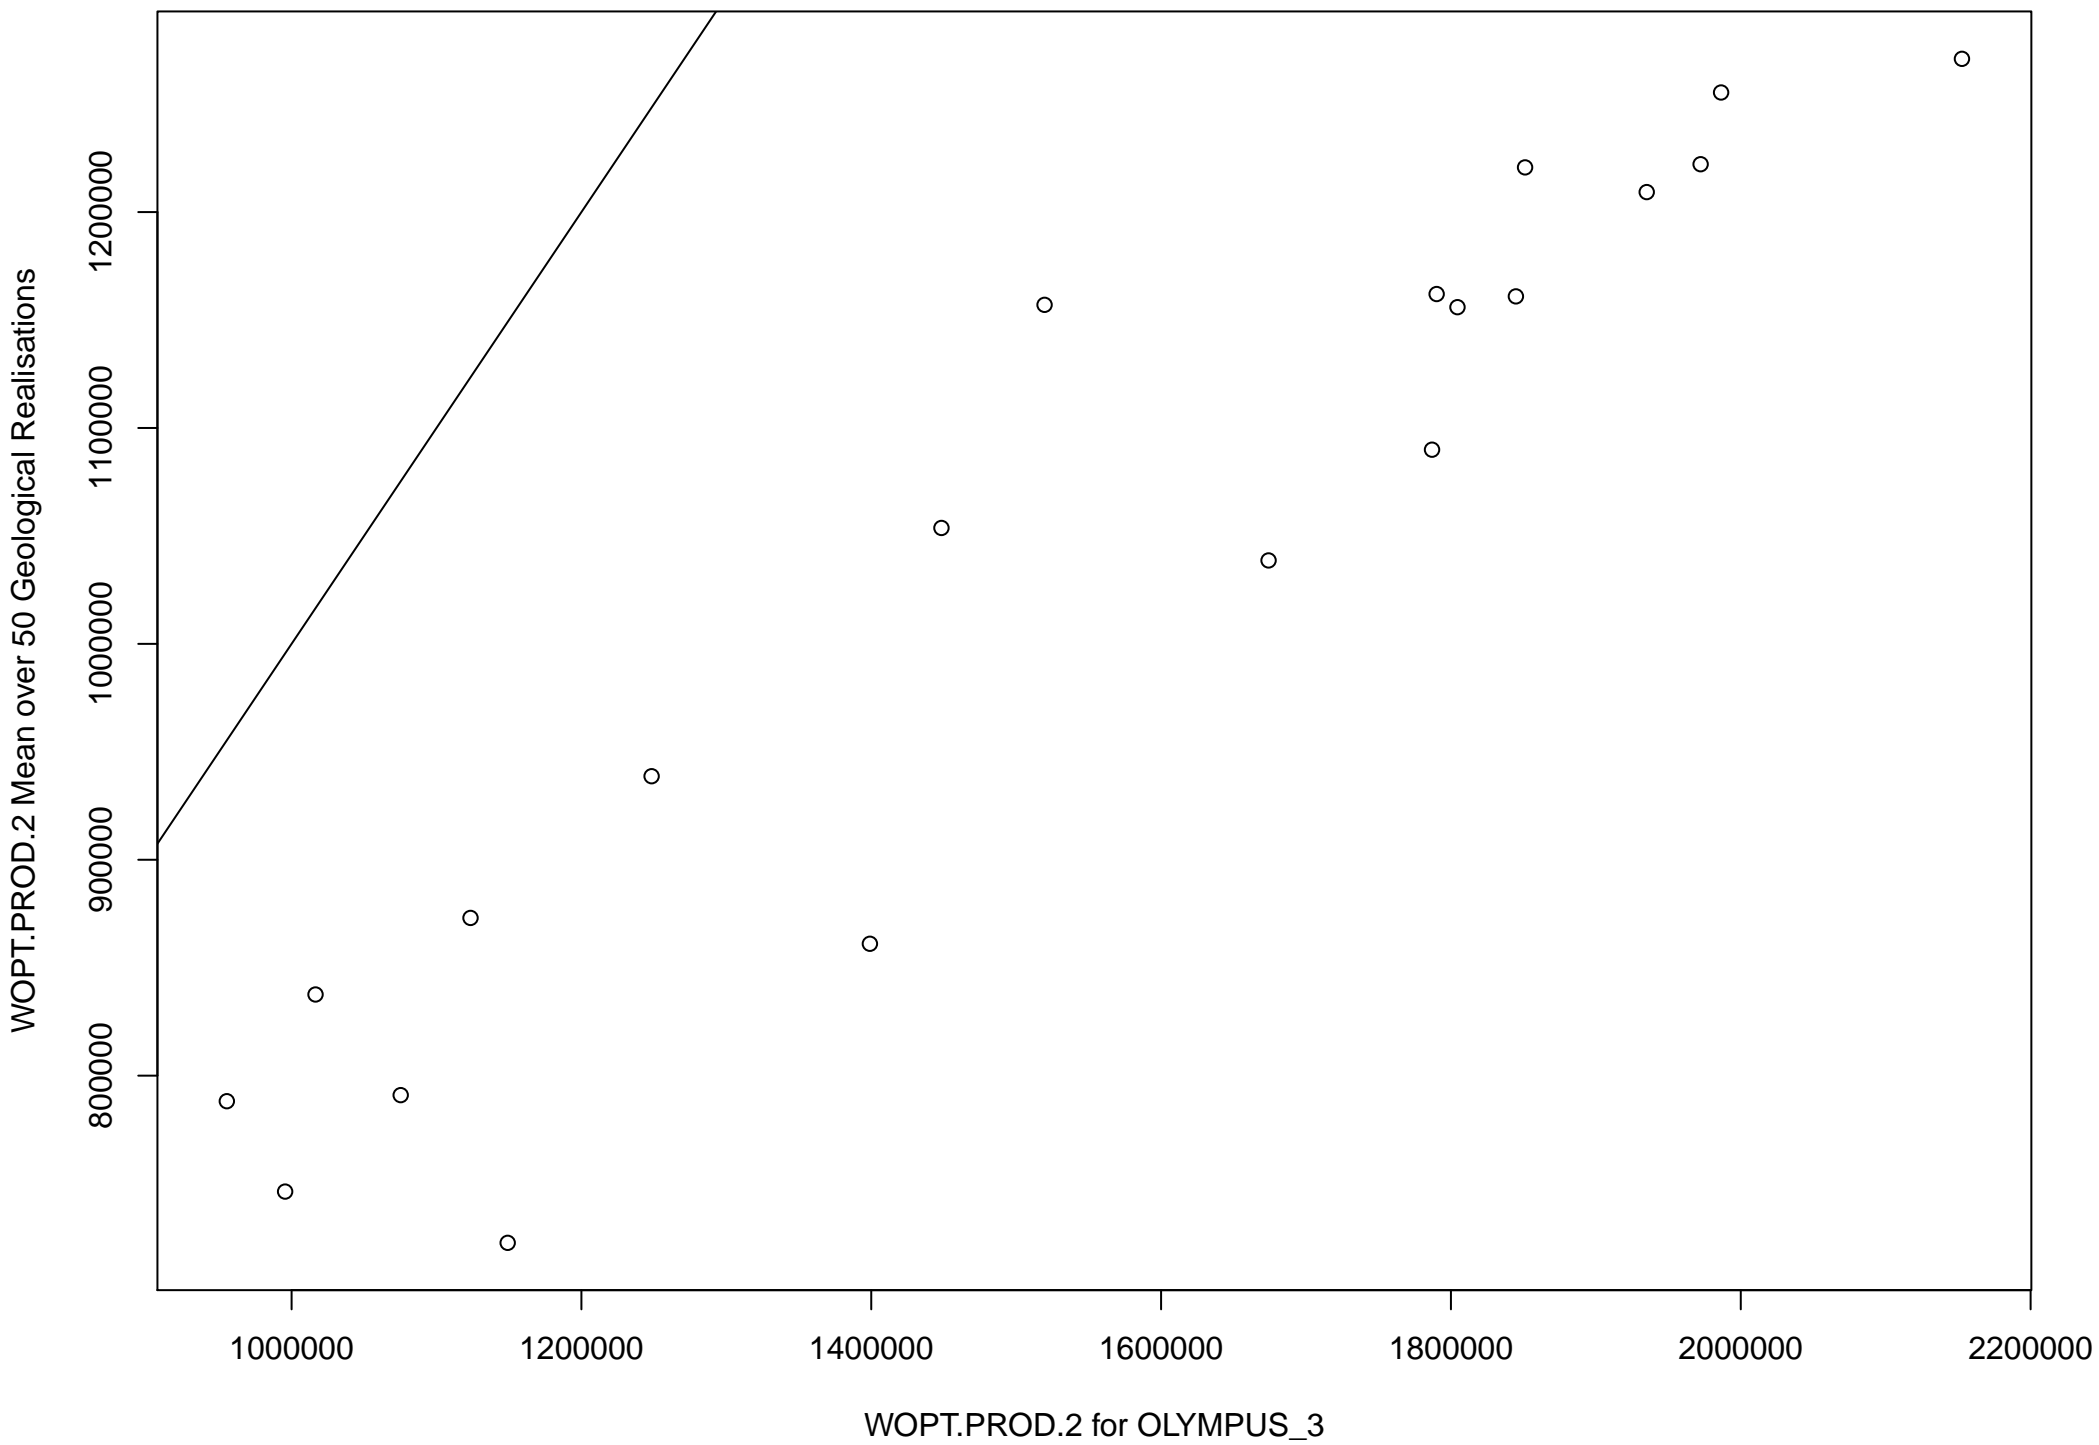

# WOPT.PROD.2 for OLYMPUS\_4

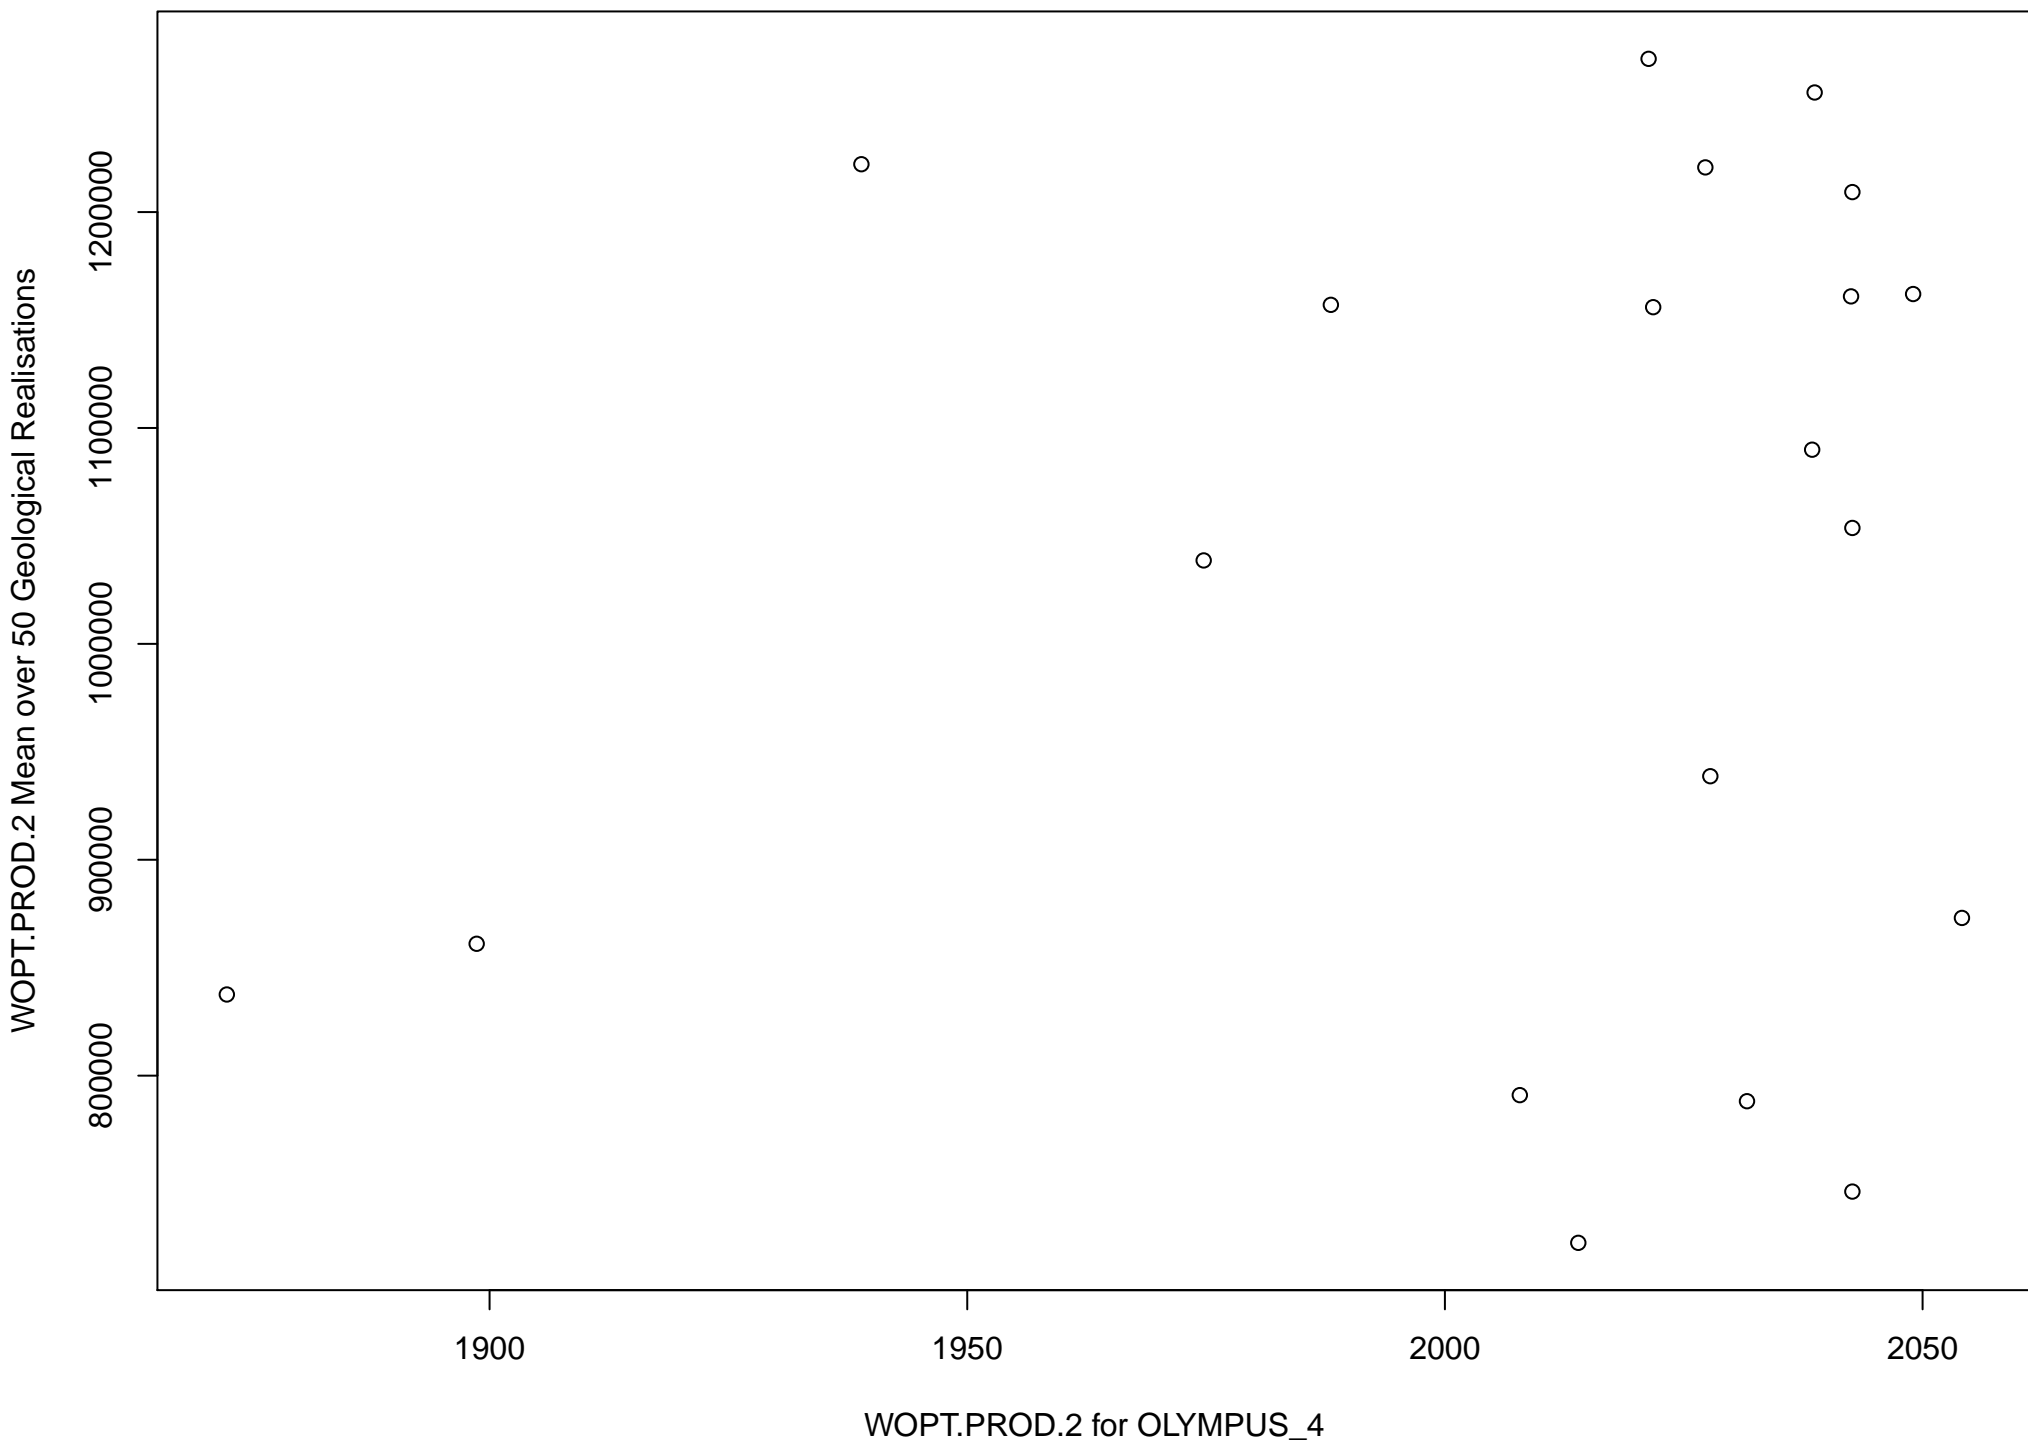

# WOPT.PROD.2 for OLYMPUS\_5

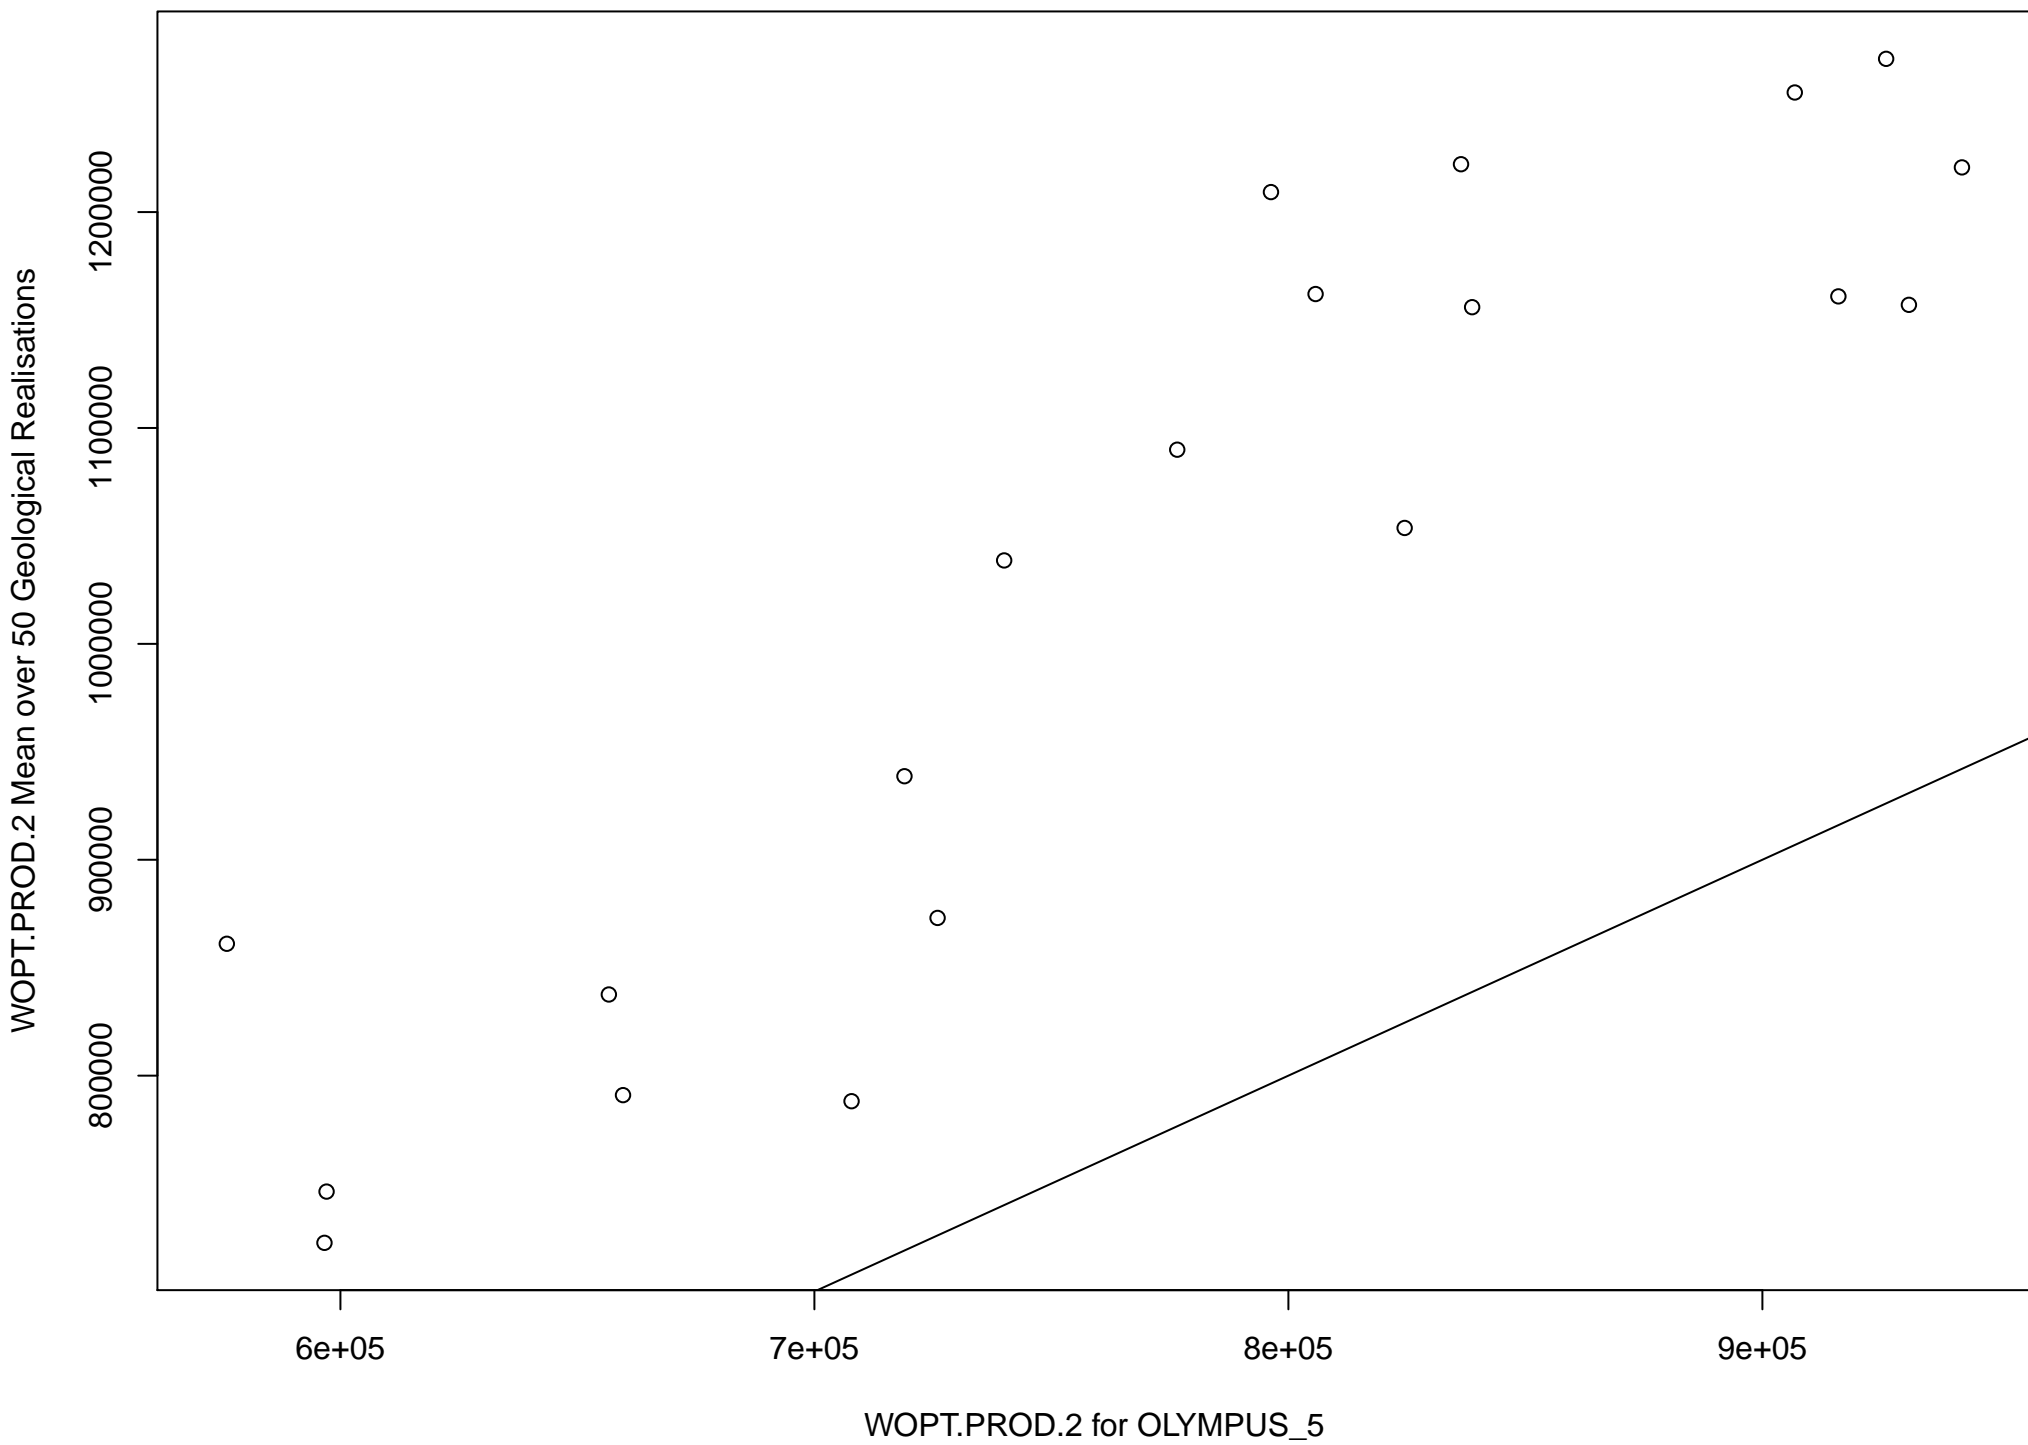

# WOPT.PROD.2 for OLYMPUS\_6

WOPT.PROD.2 Mean over 50 Geological Realisations

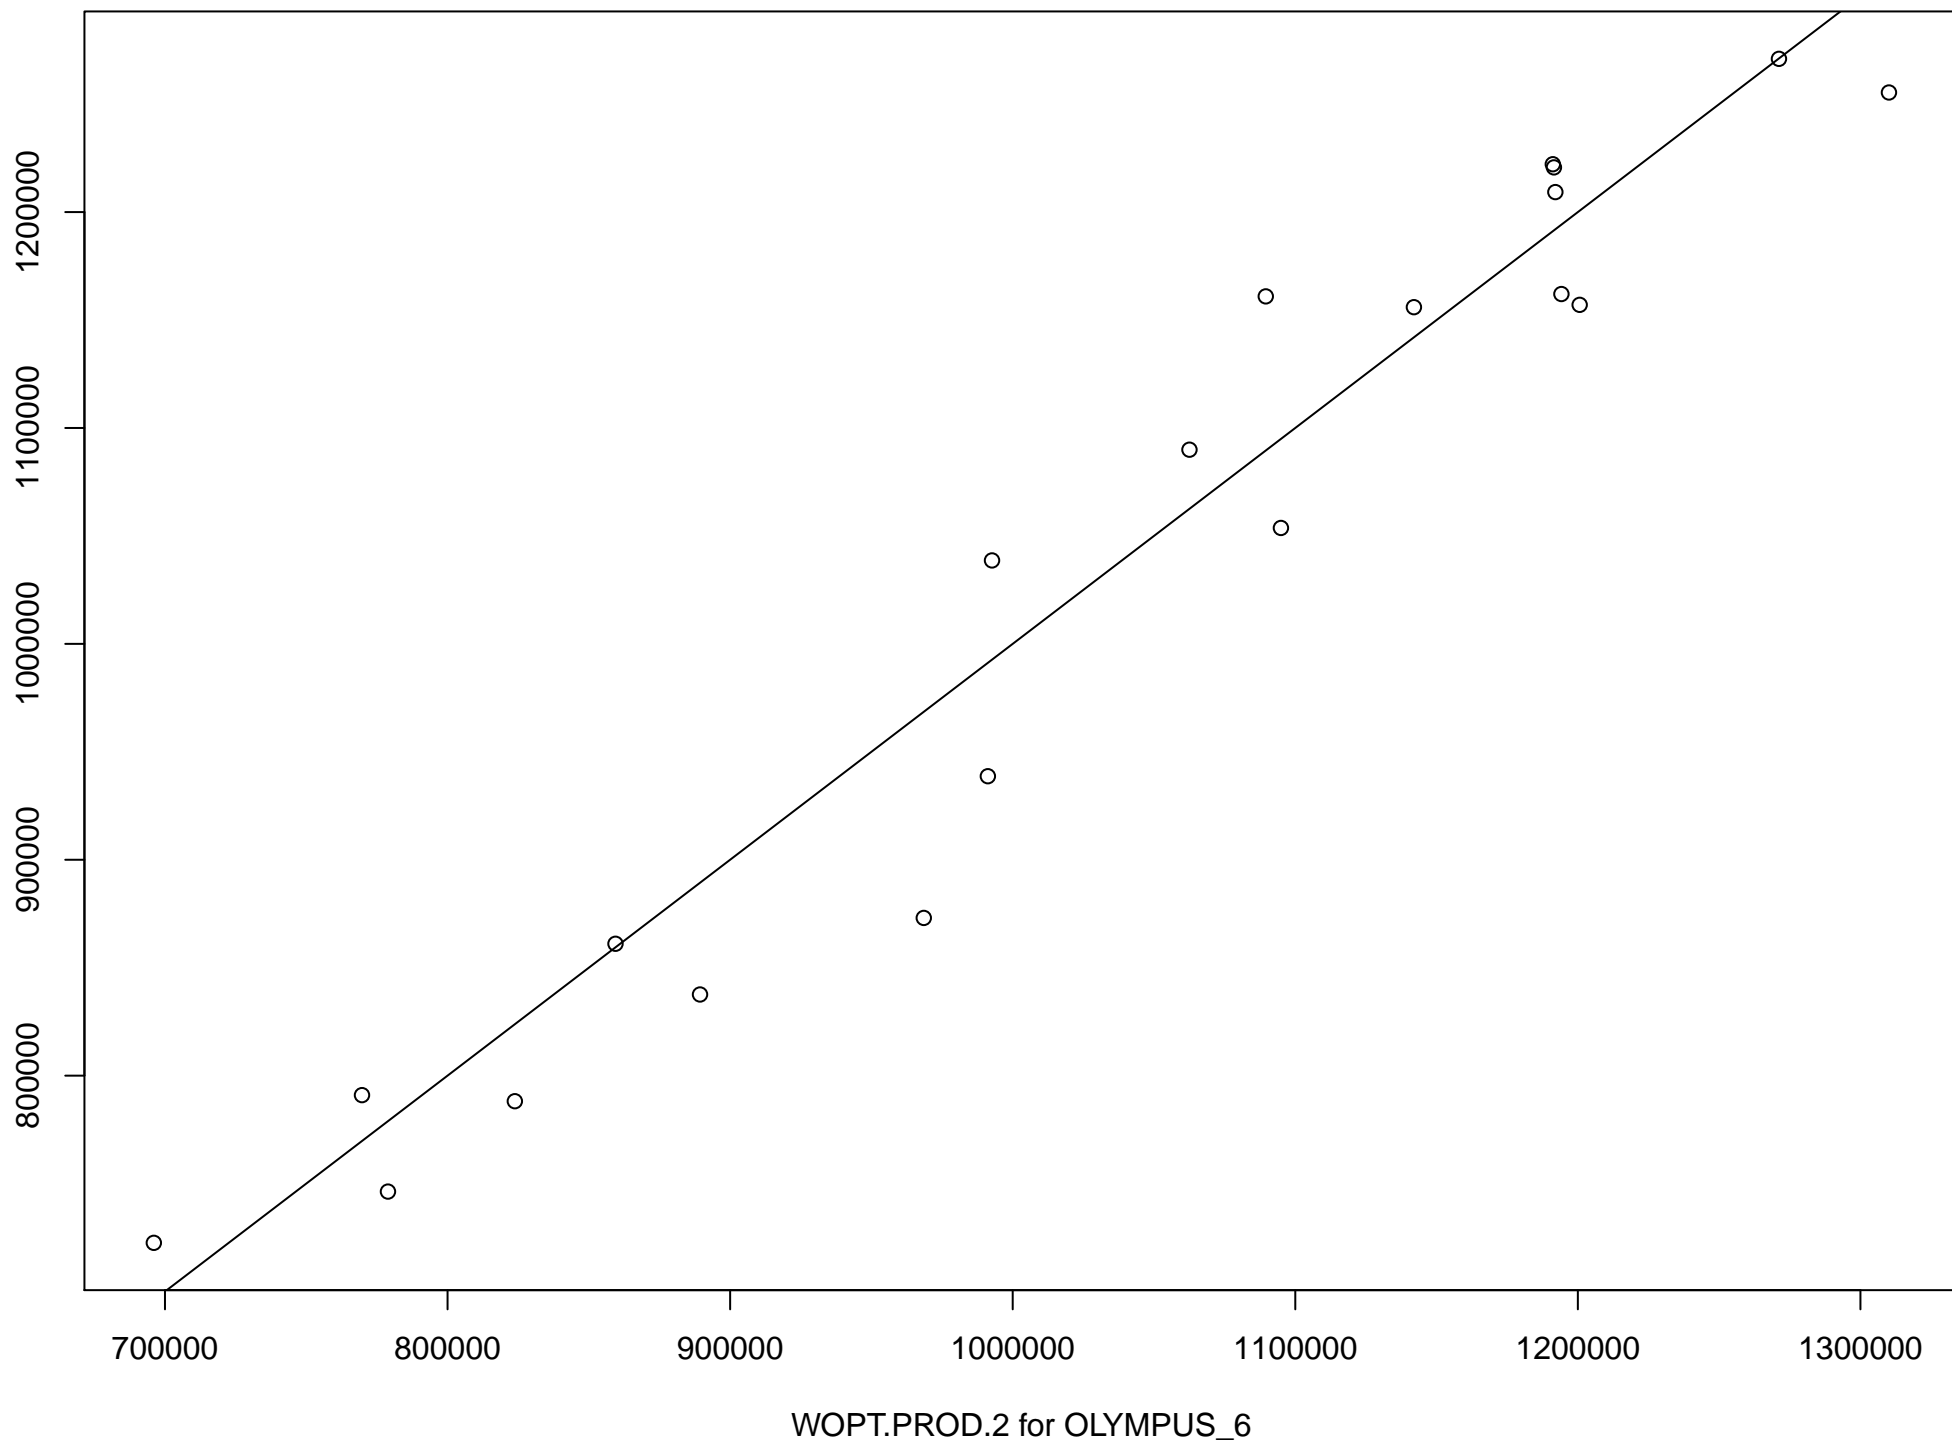

WOPT.PROD.2 for OLYMPUS\_7

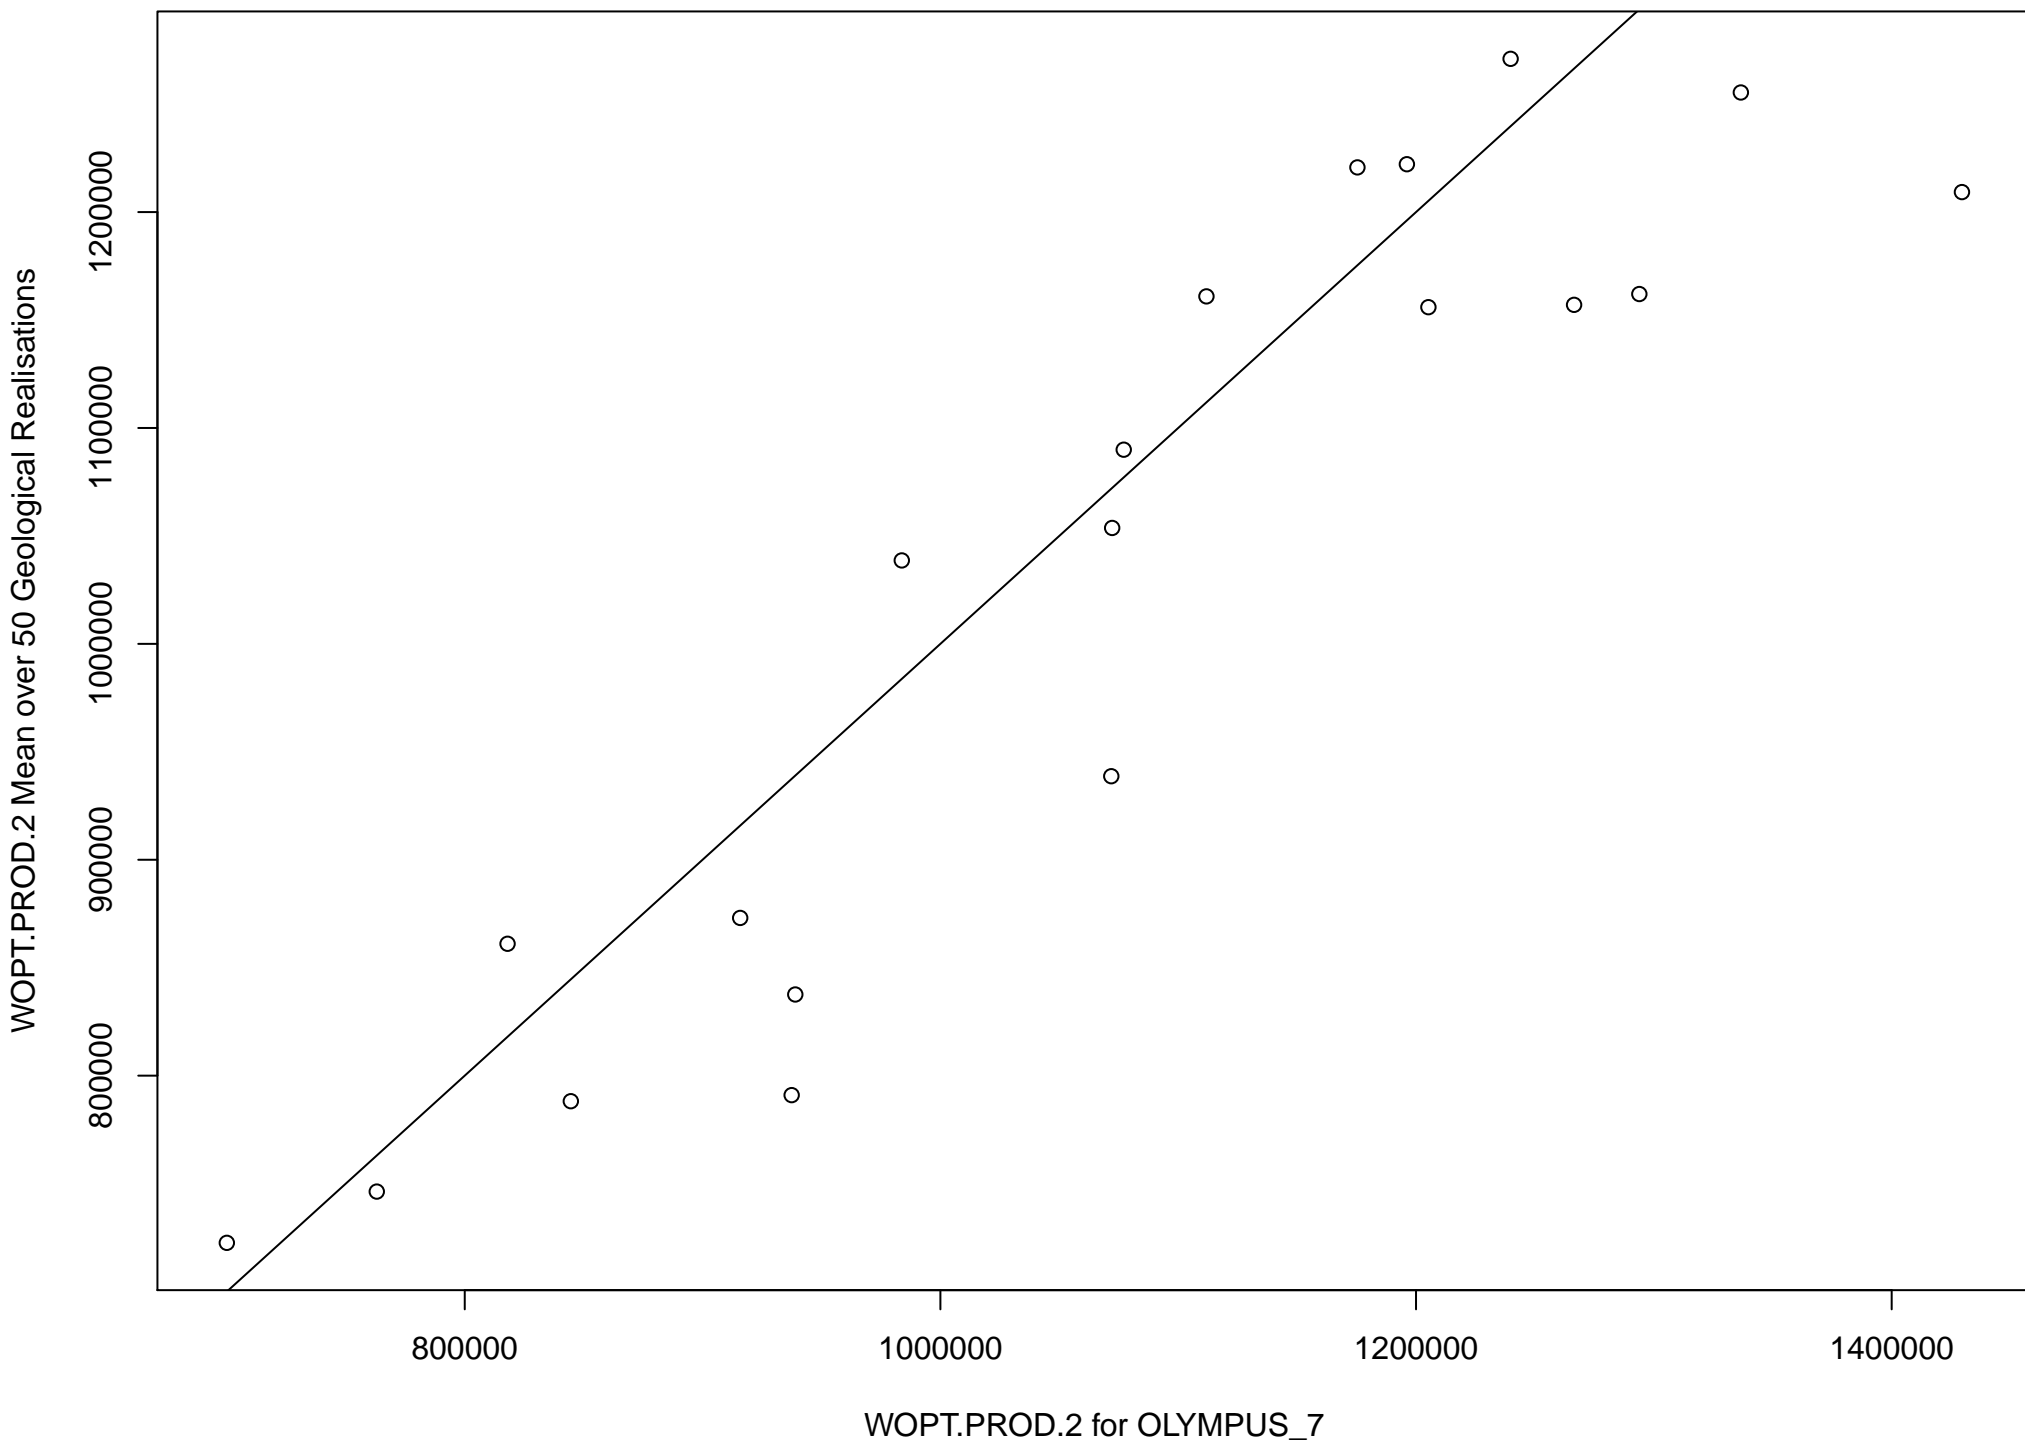

WOPT.PROD.2 for OLYMPUS\_8

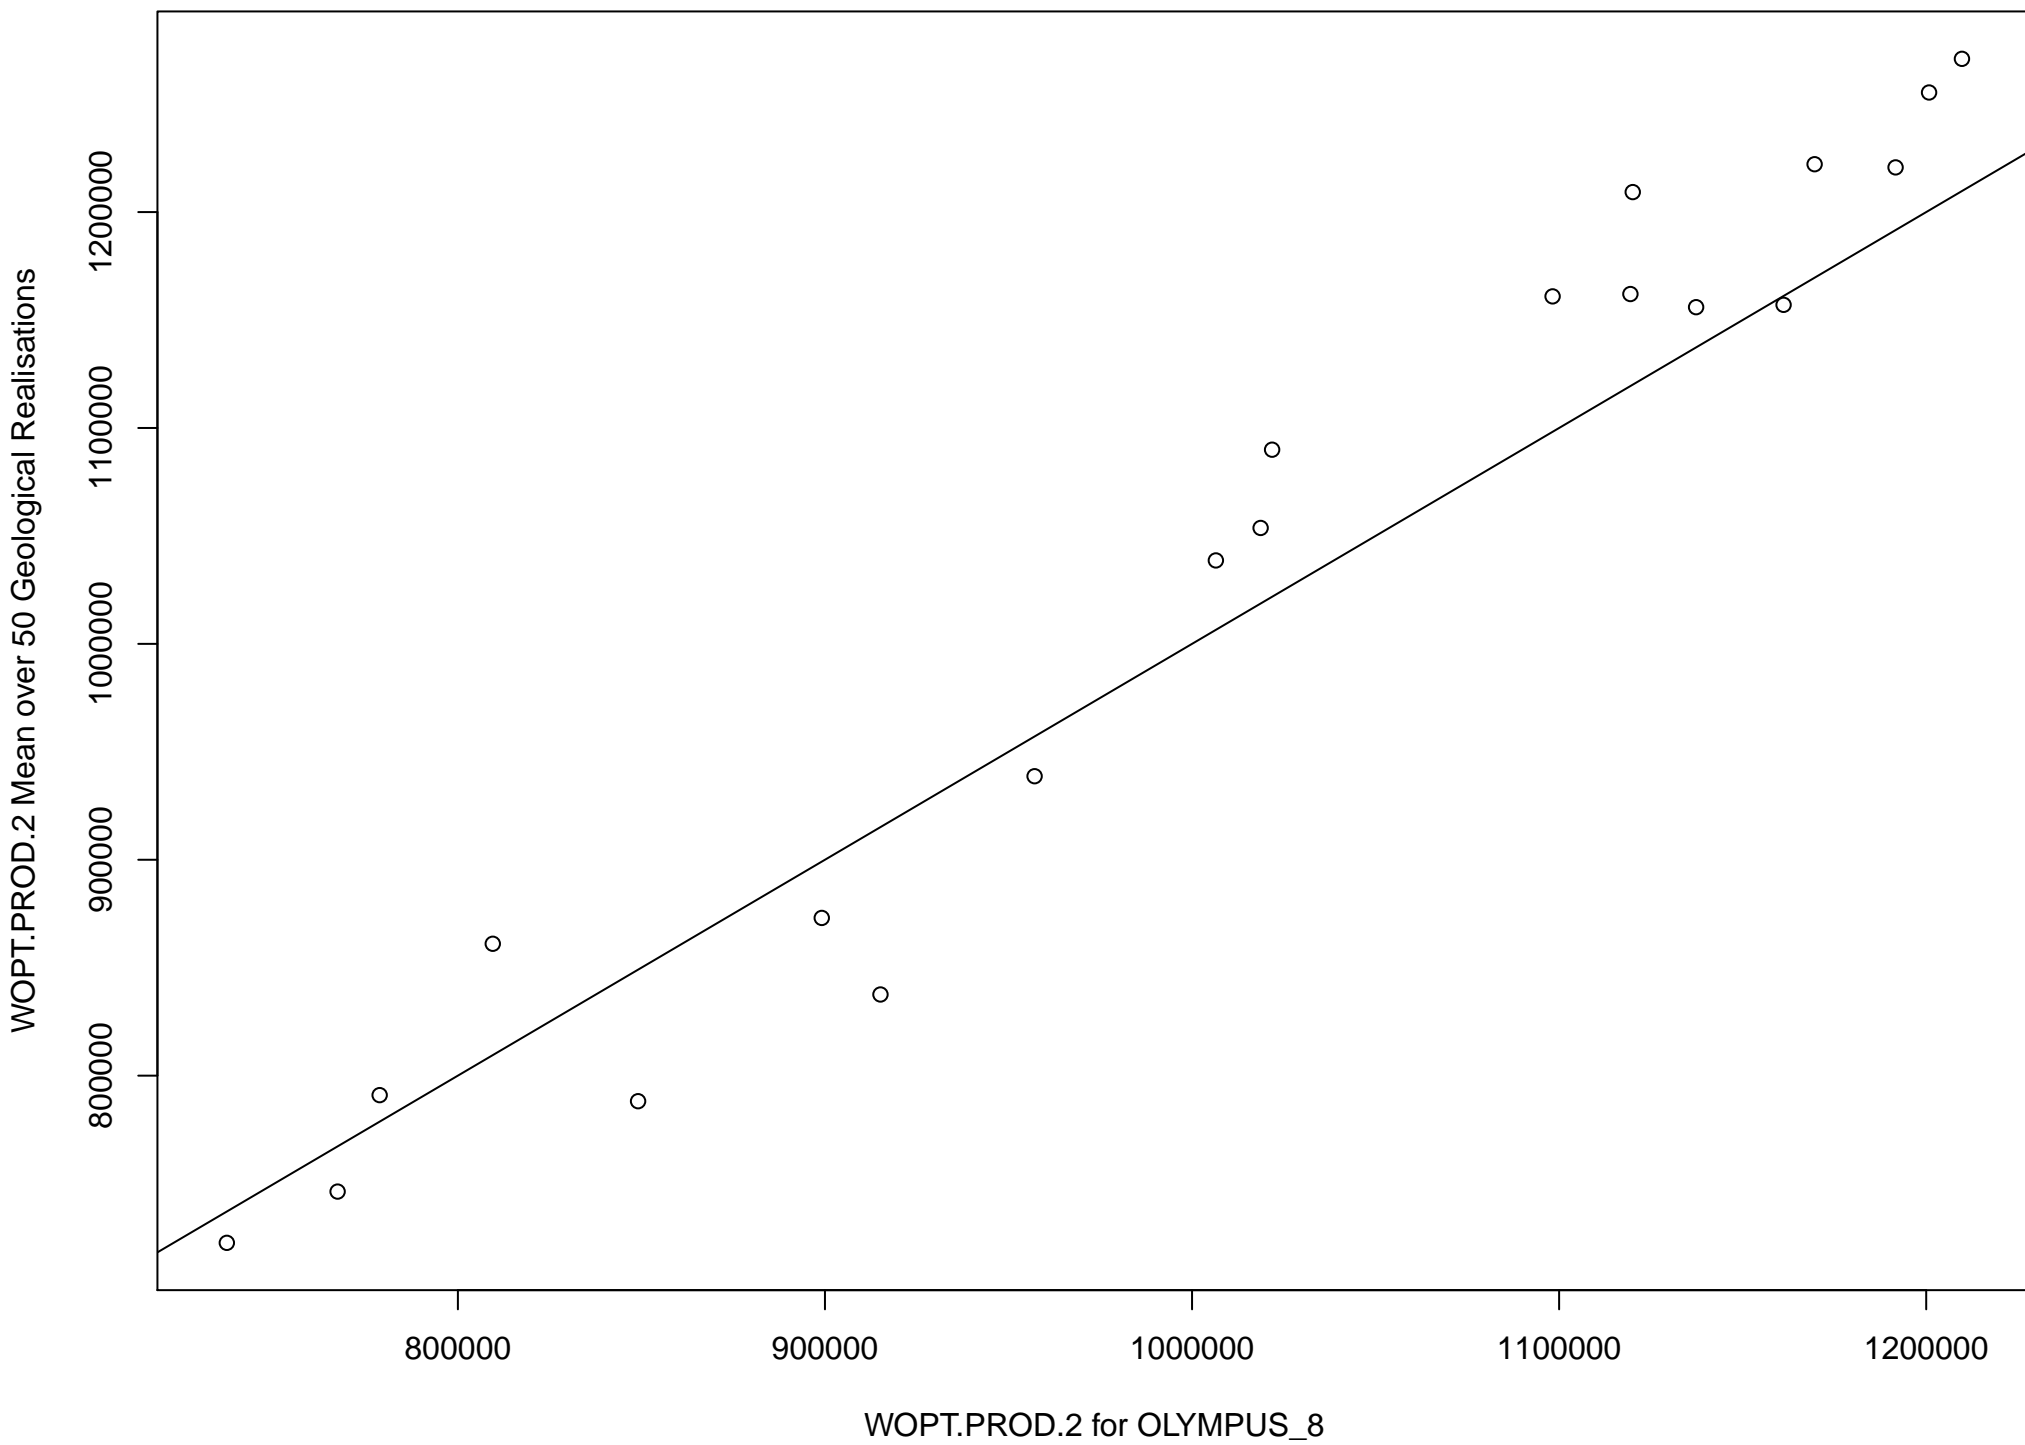



# WOPT.PROD.2 for OLYMPUS\_9

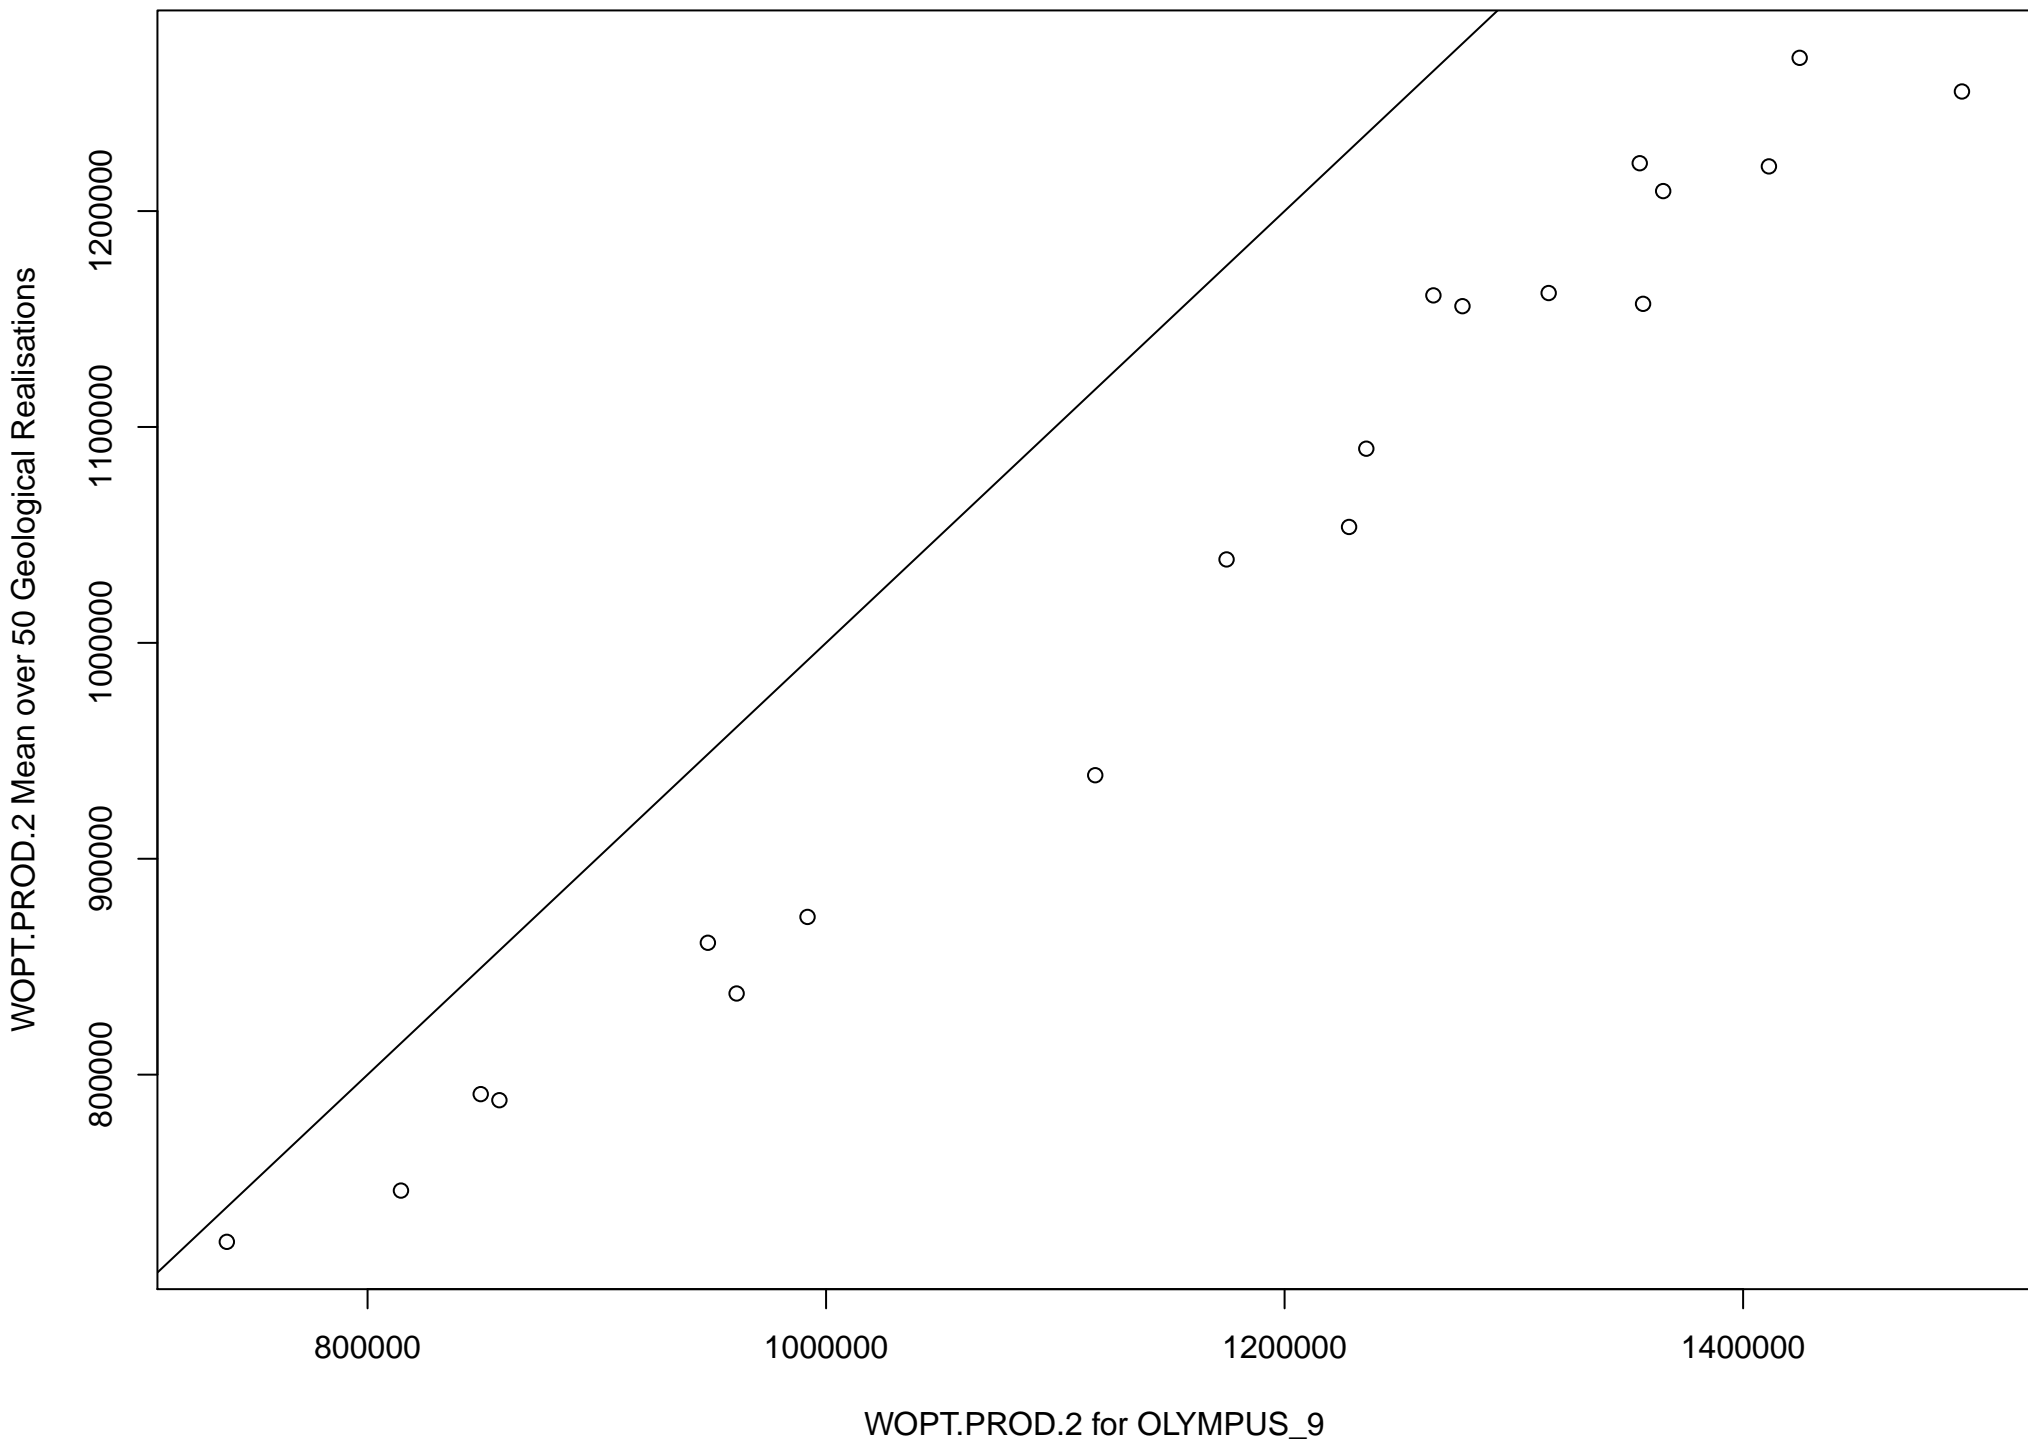

WOPT.PROD.2 for OLYMPUS\_10

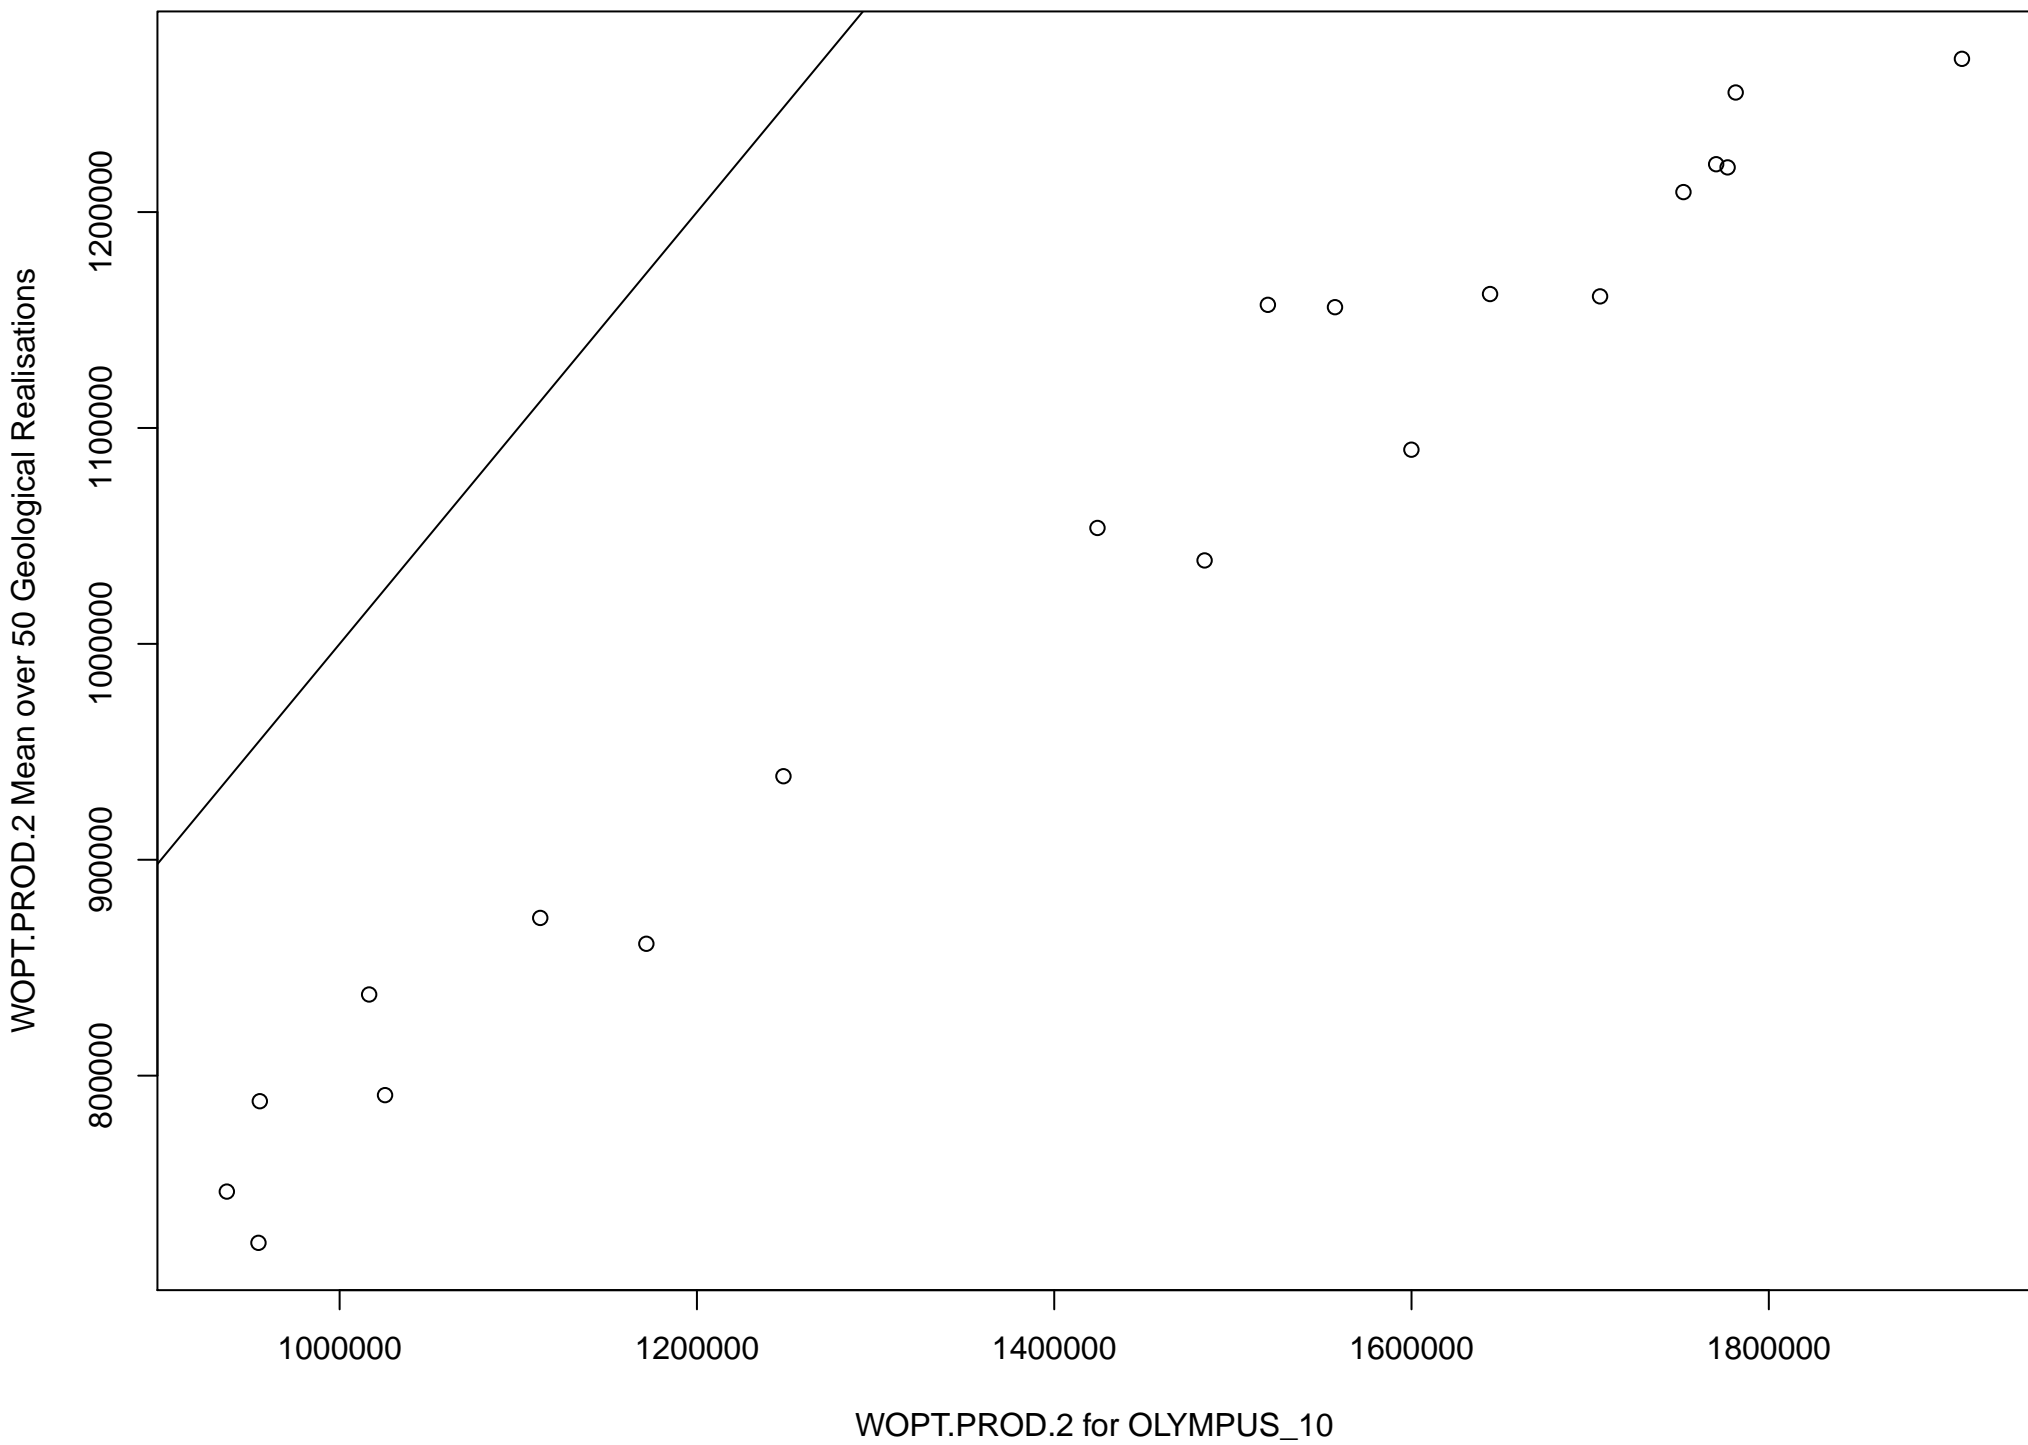

# WOPT.PROD.2 for OLYMPUS\_11

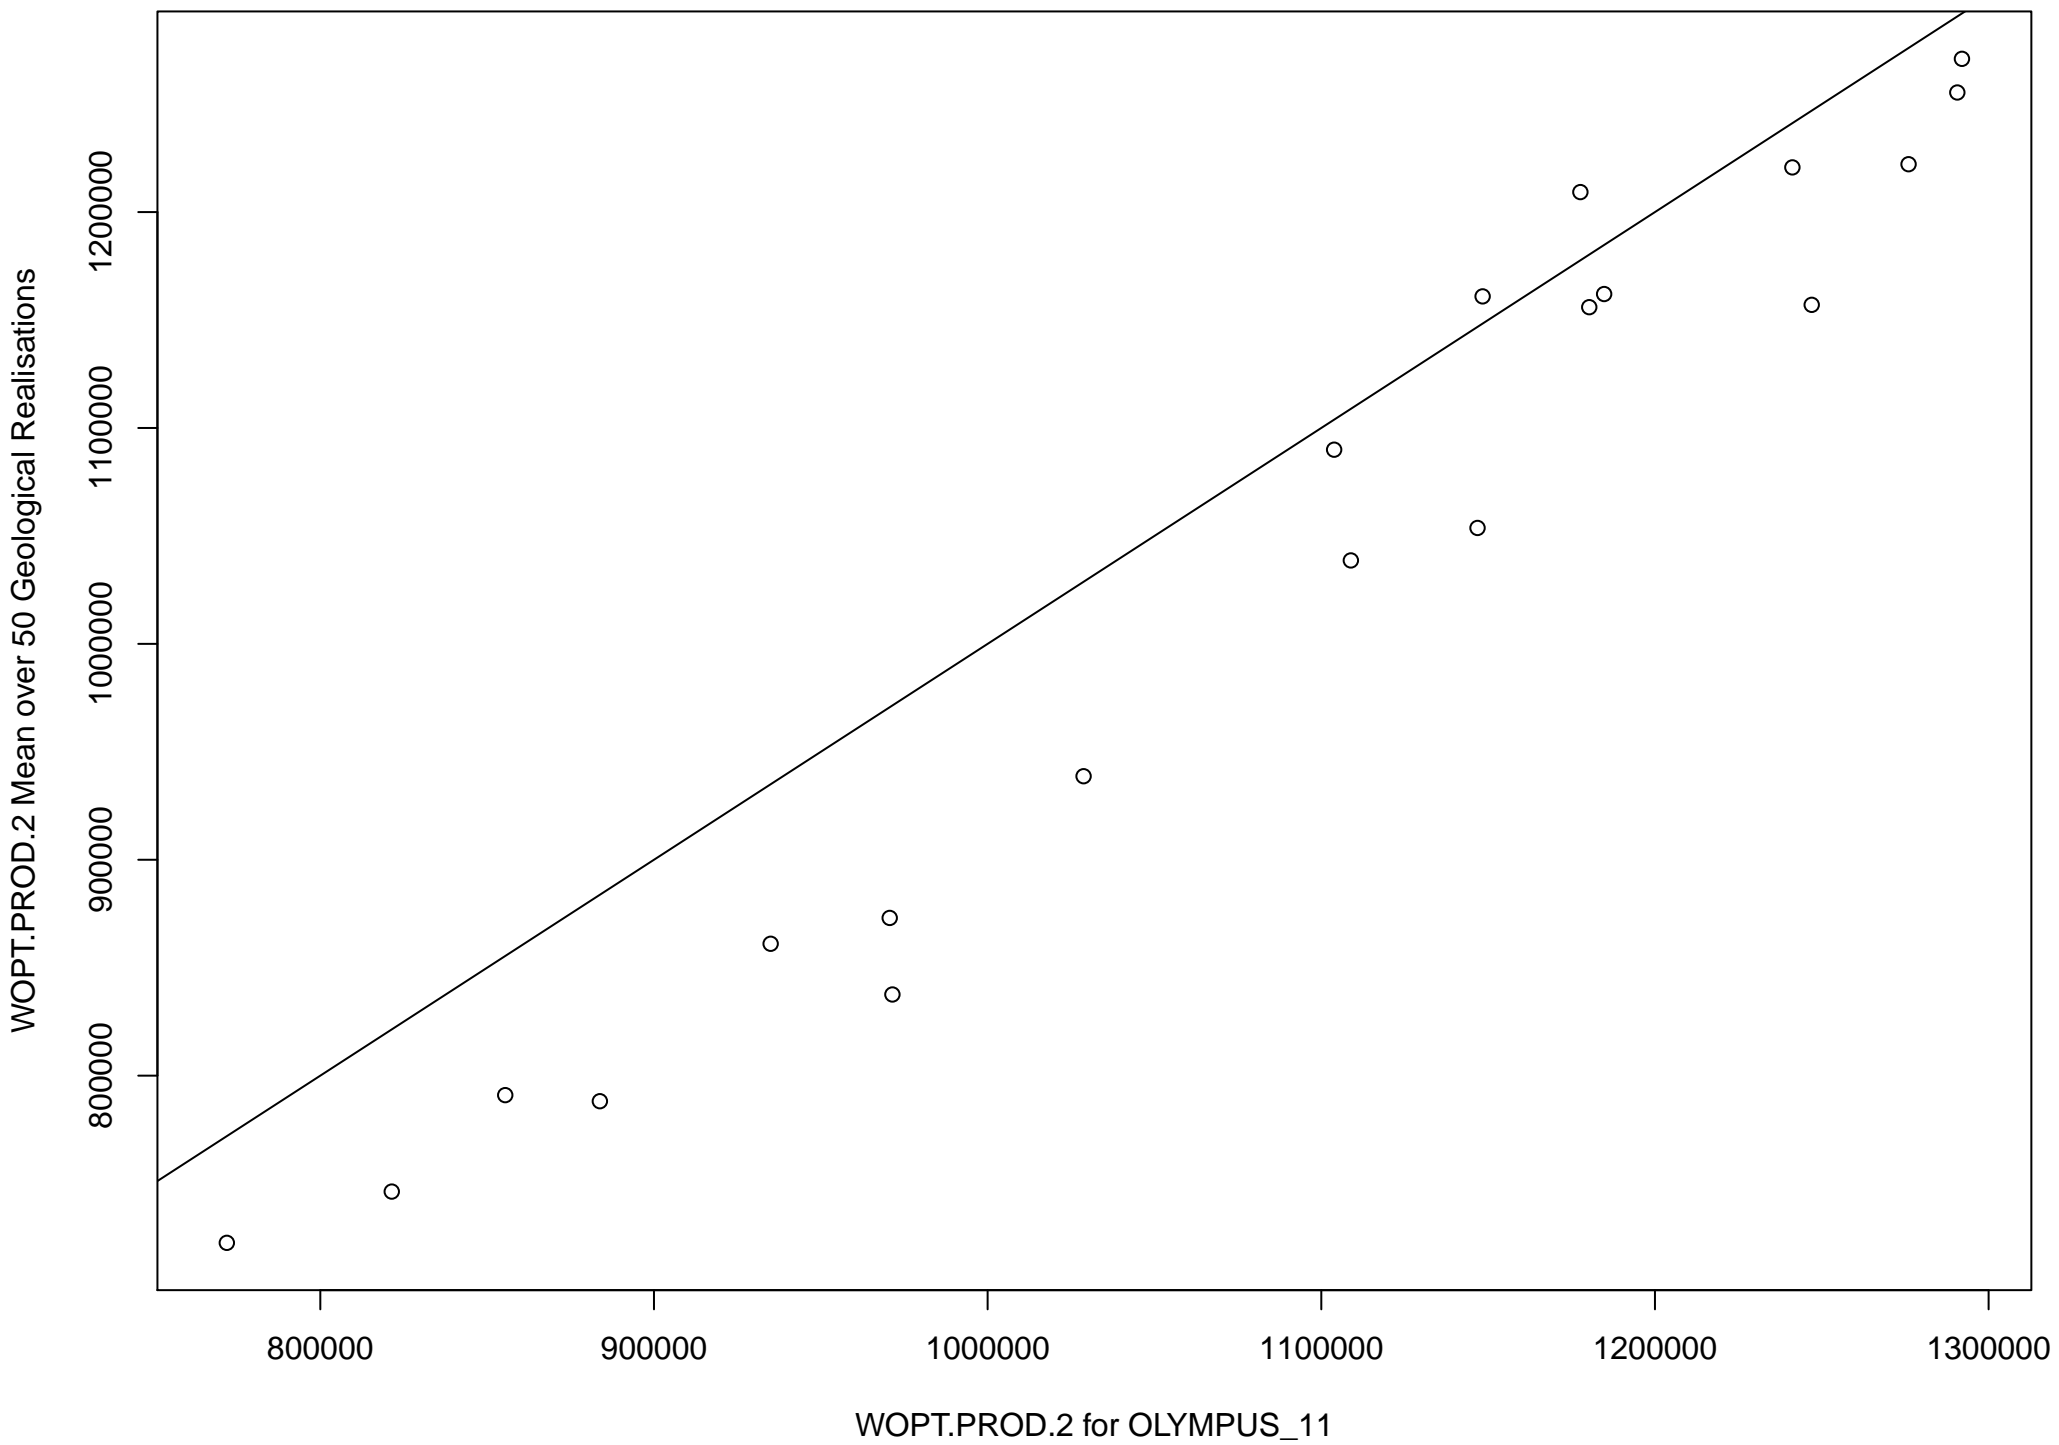

# WOPT.PROD.2 for OLYMPUS\_12

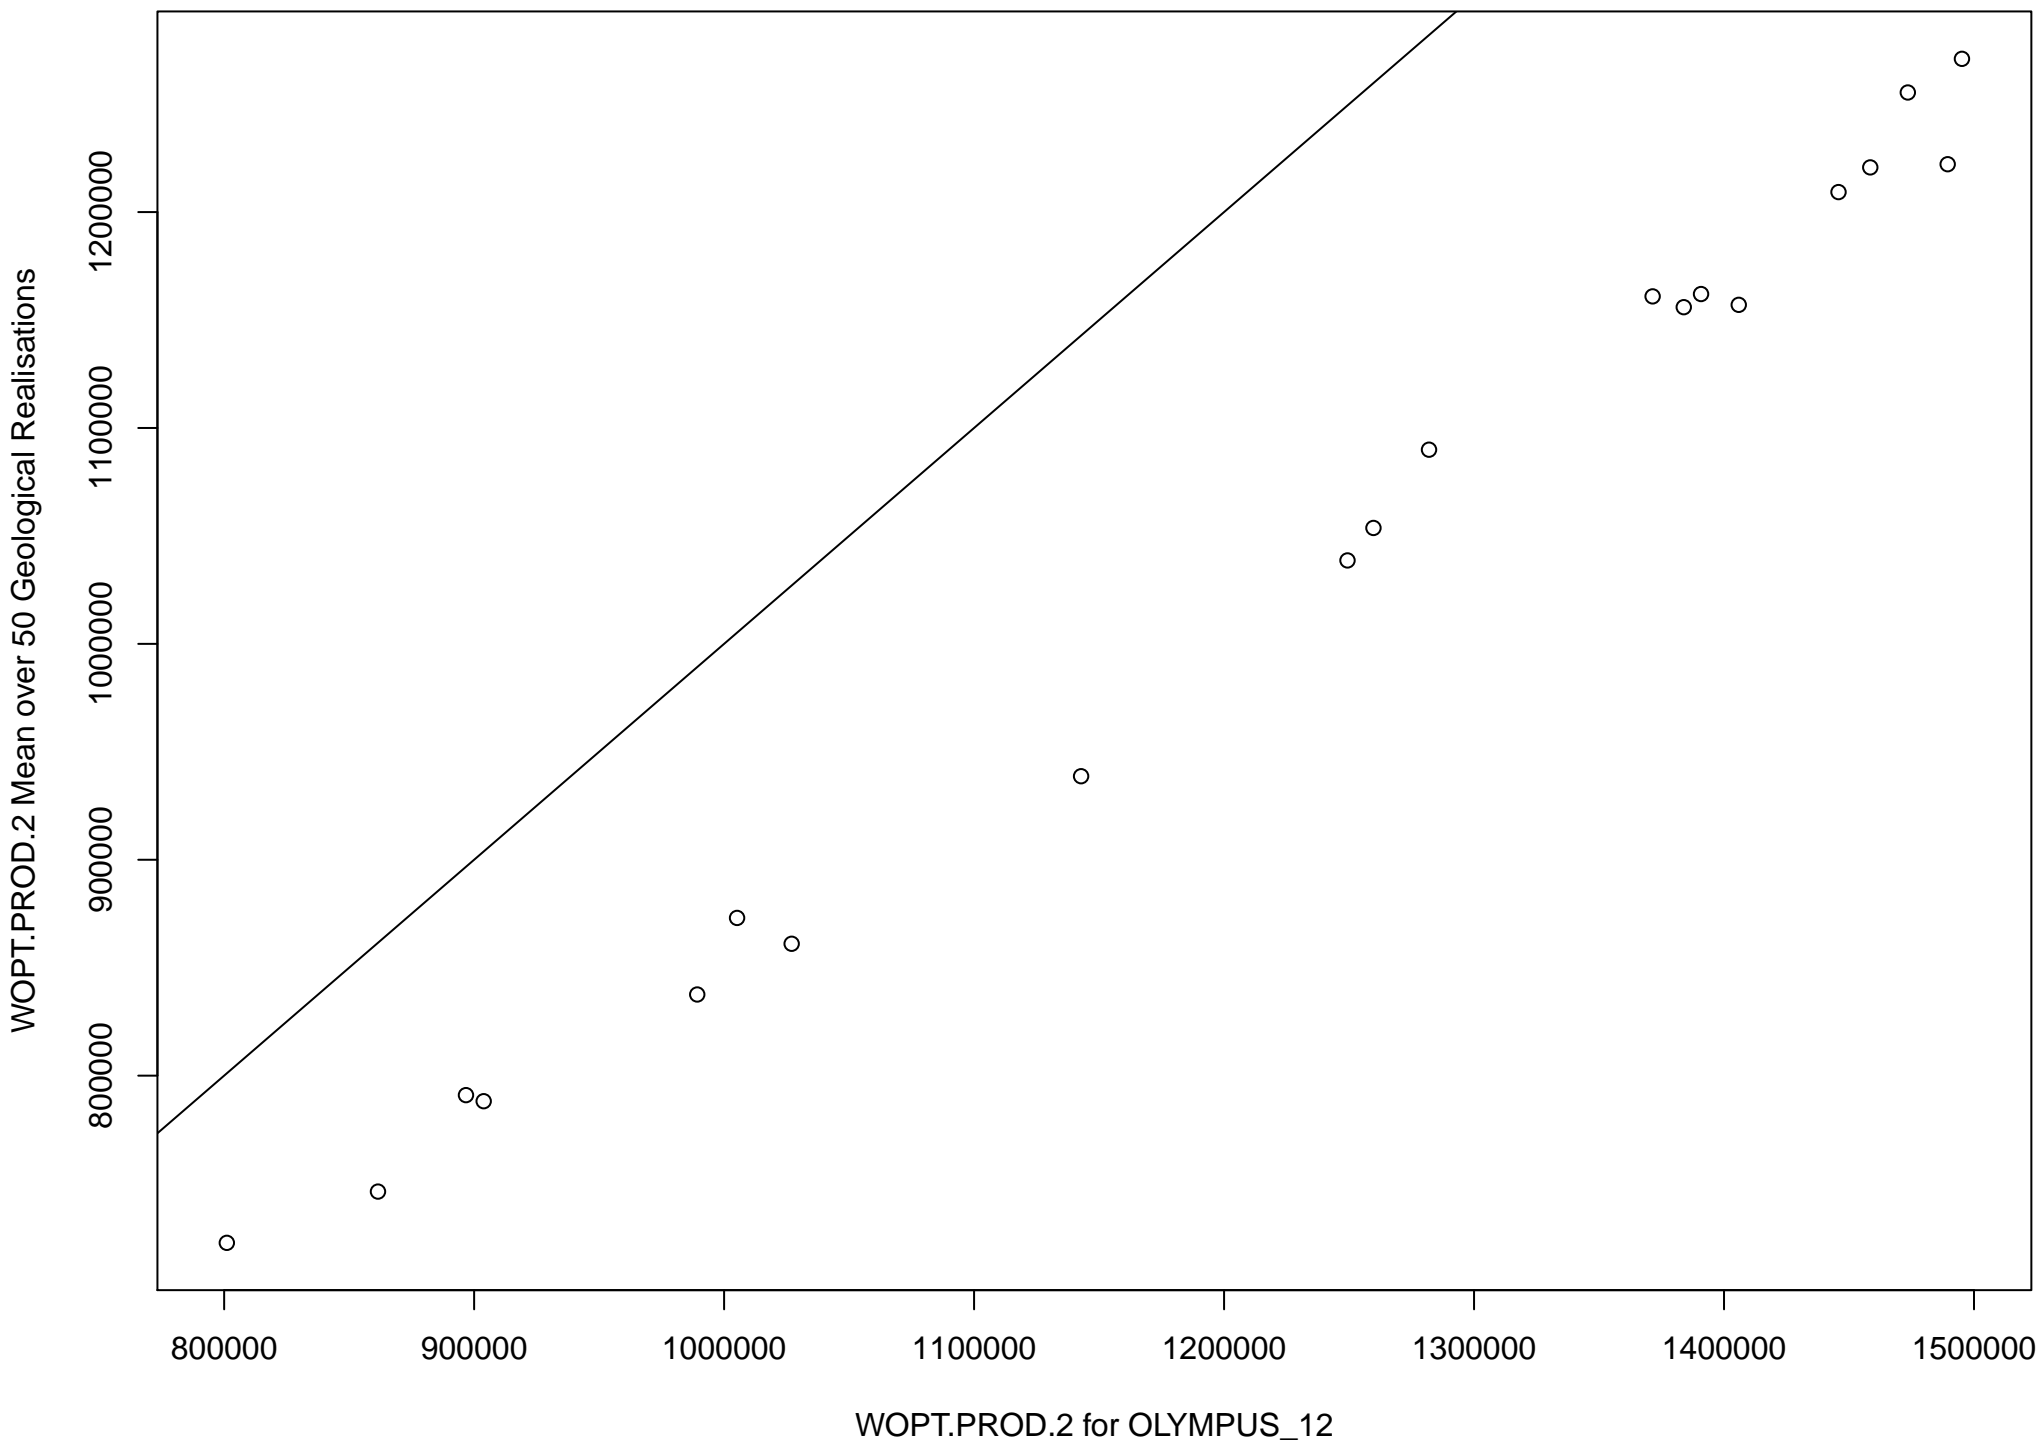

WOPT.PROD.2 for OLYMPUS\_13

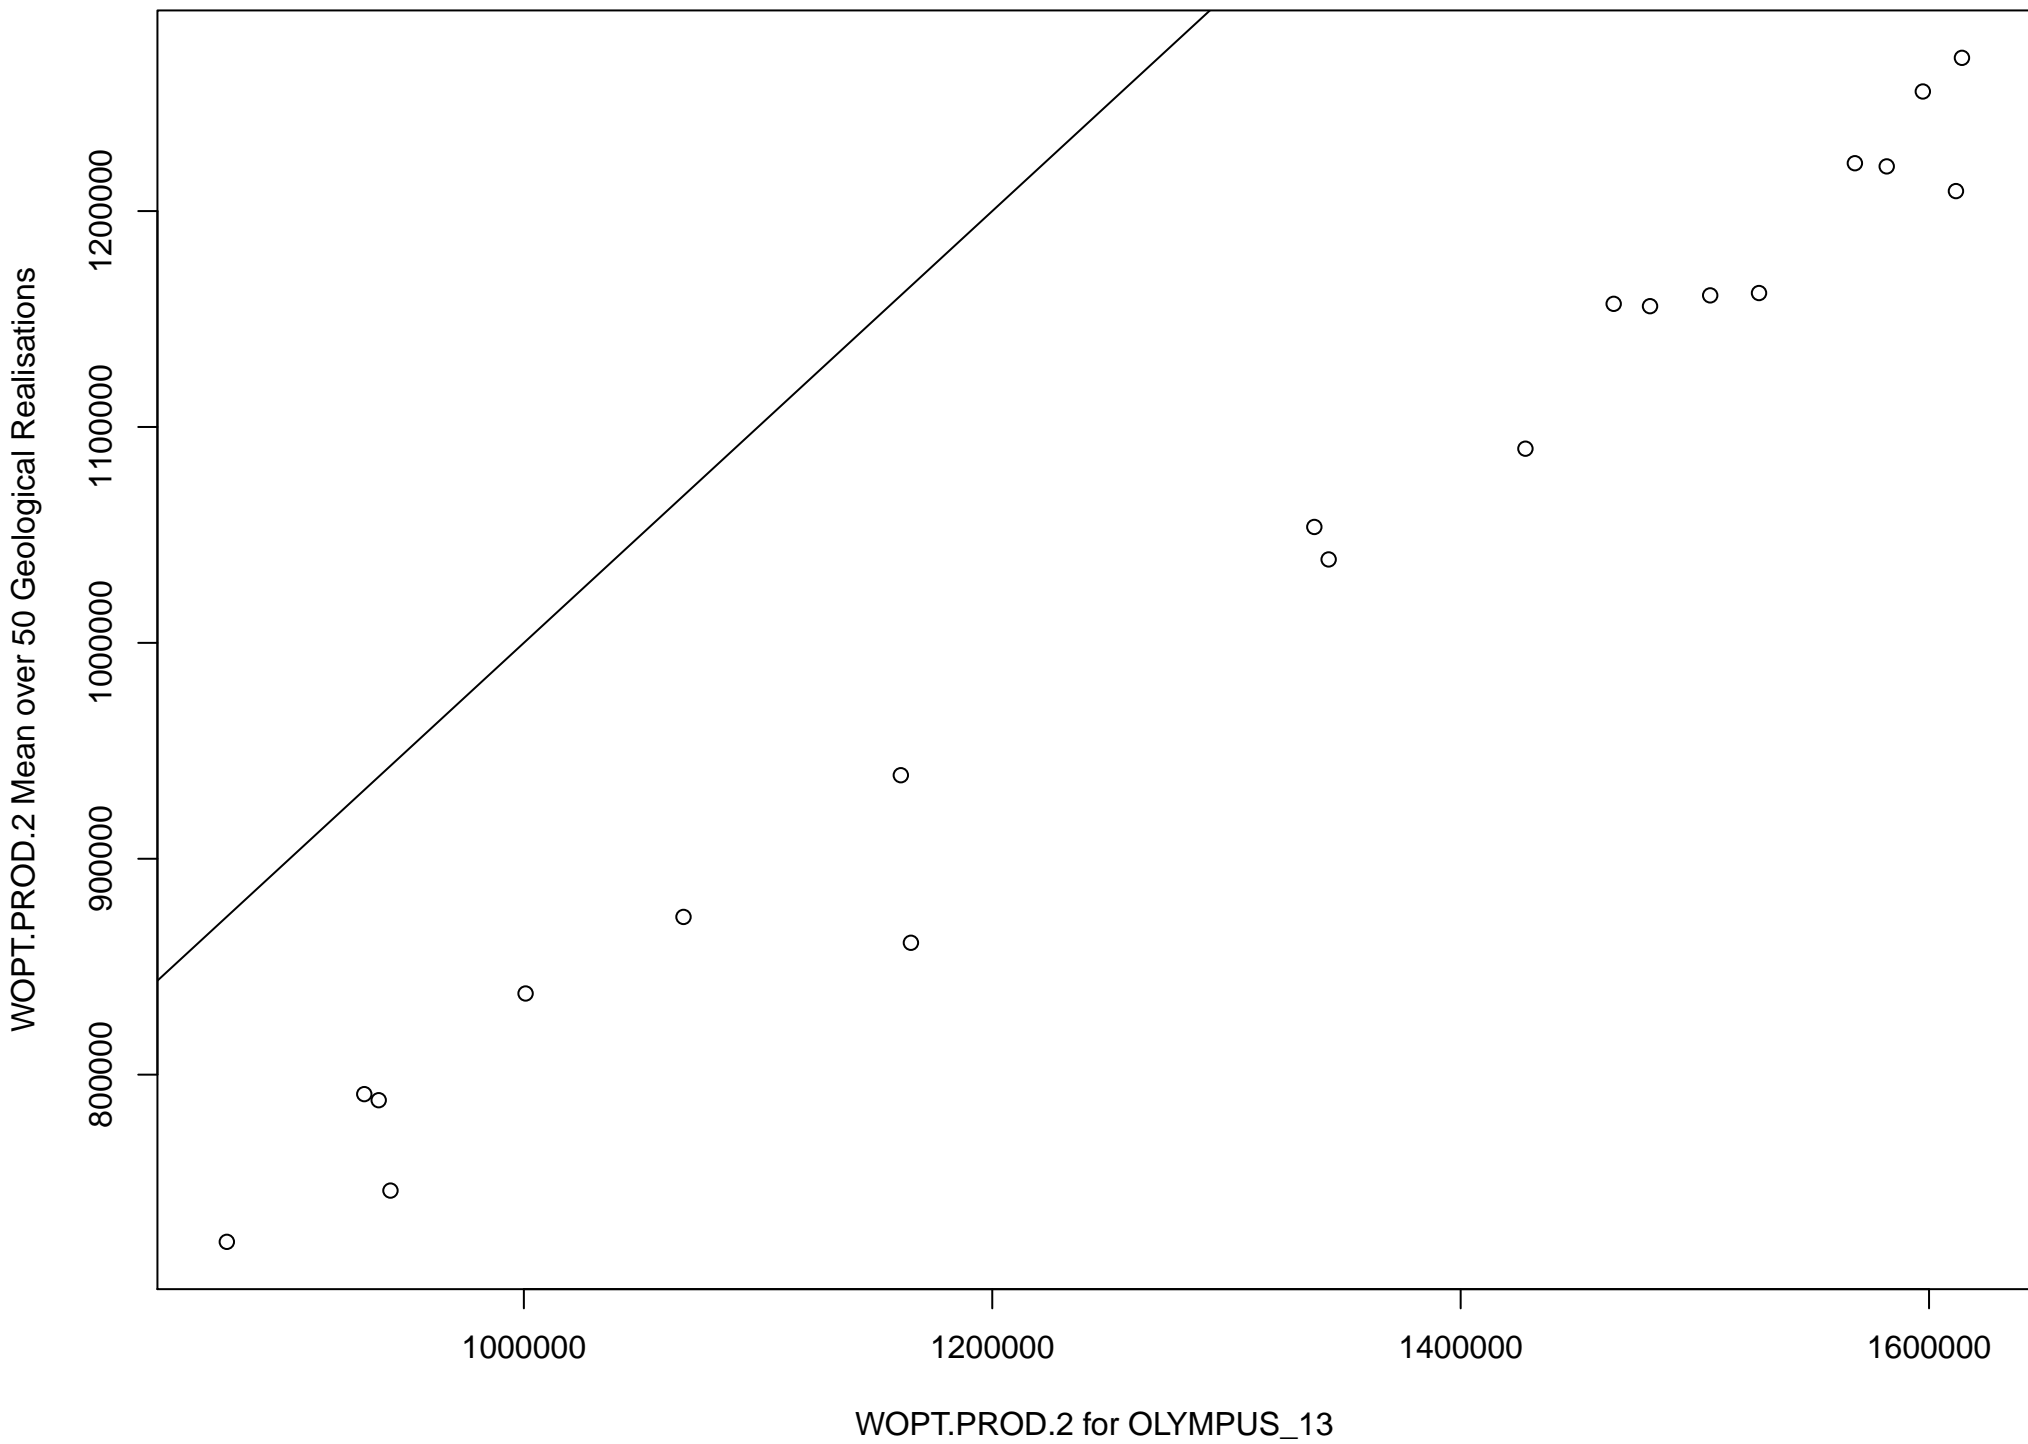

# WOPT.PROD.2 for OLYMPUS\_14

WOPT.PROD.2 Mean over 50 Geological Realisations

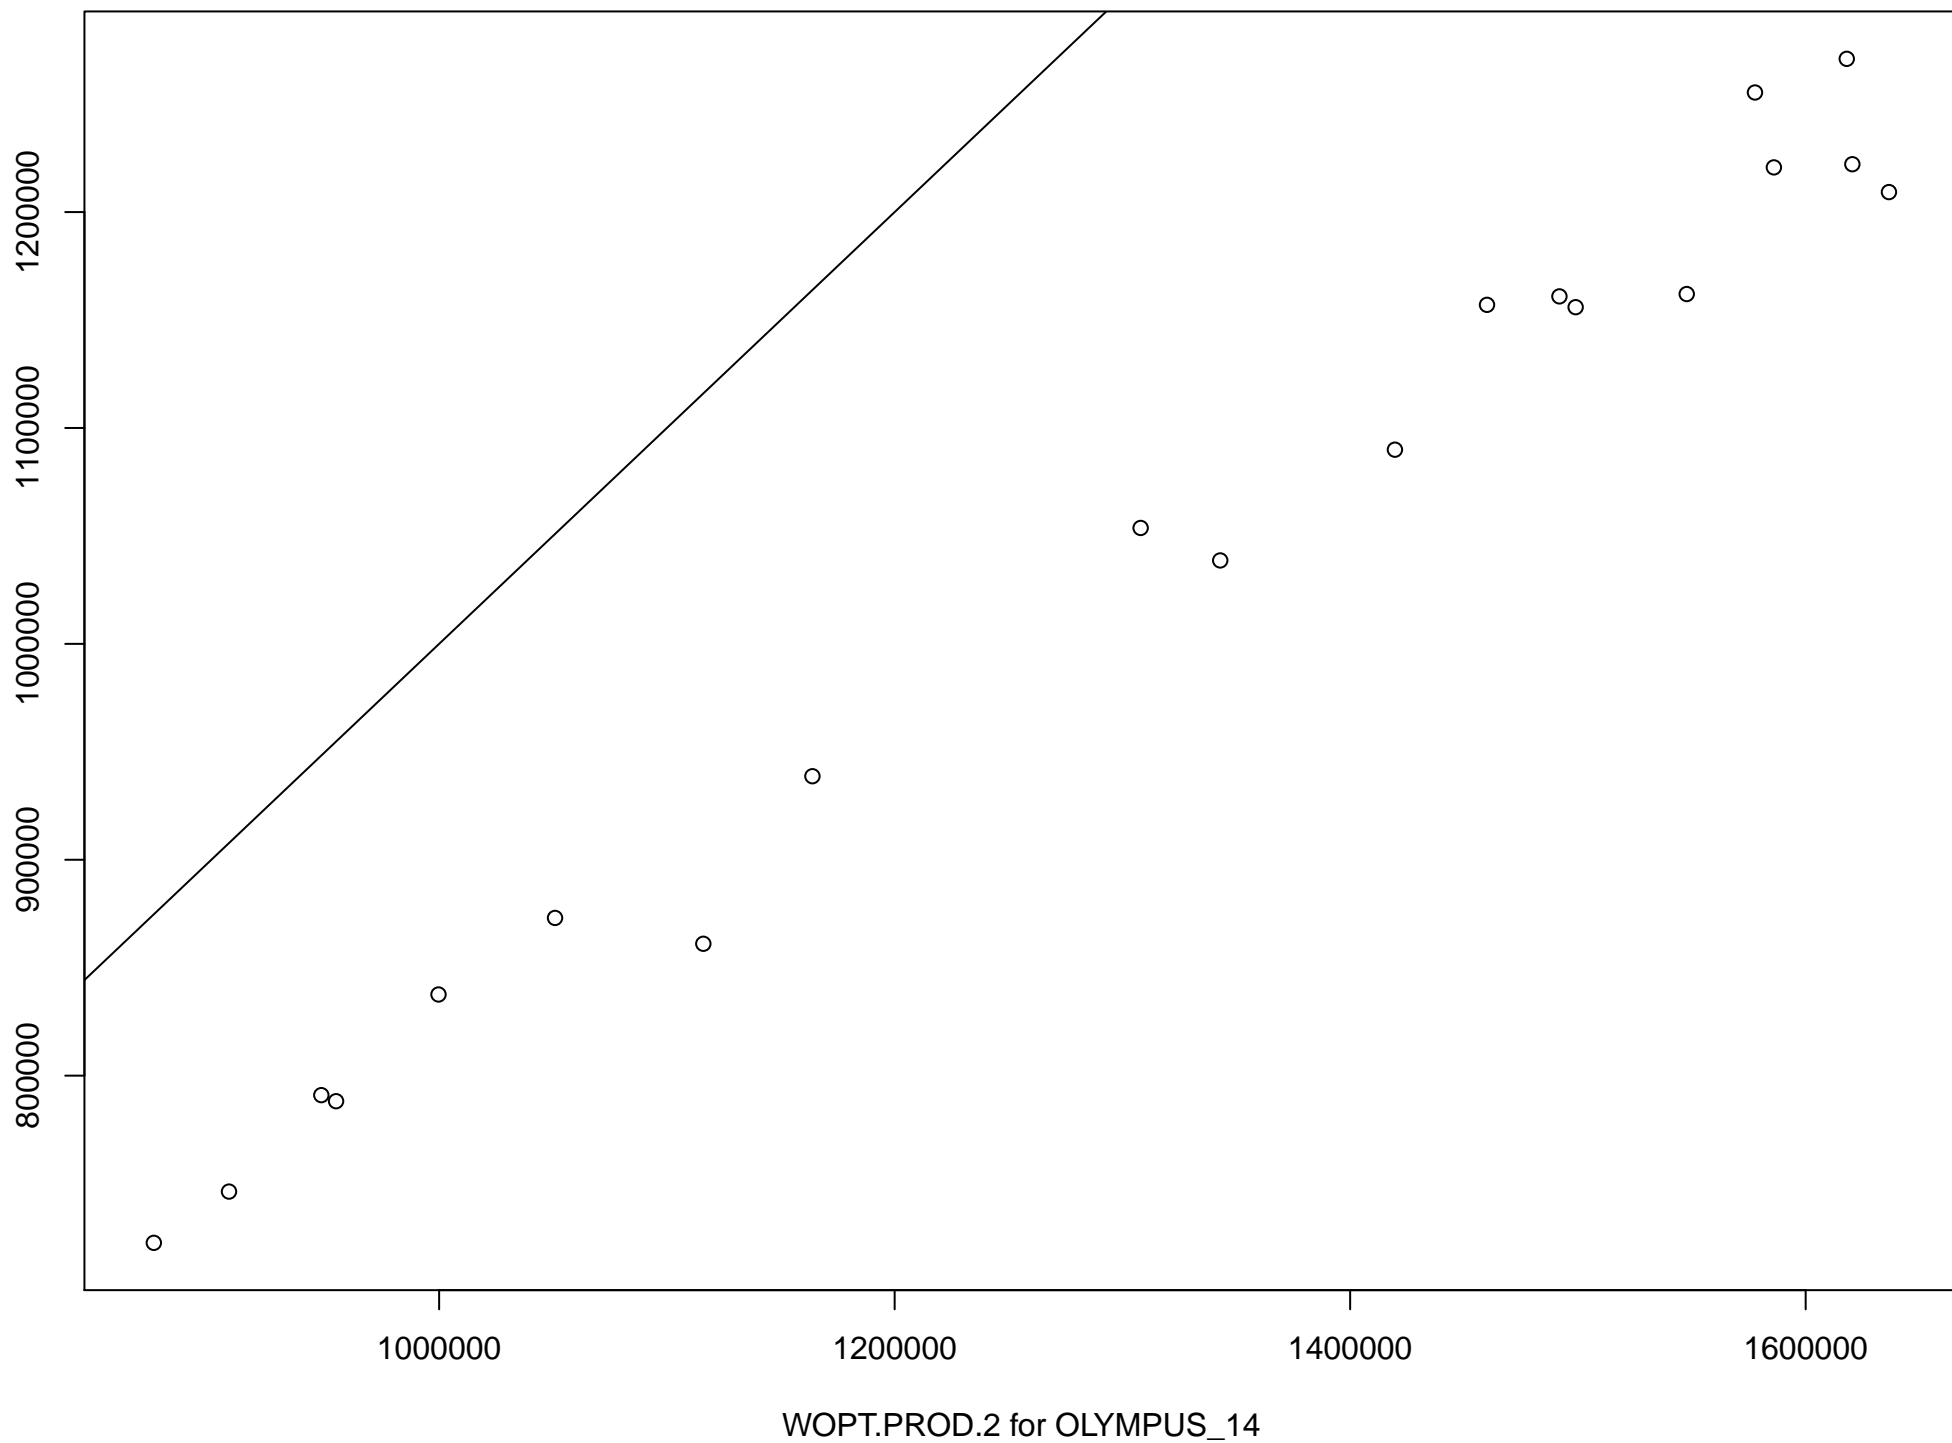

WOPT.PROD.2 for OLYMPUS\_15

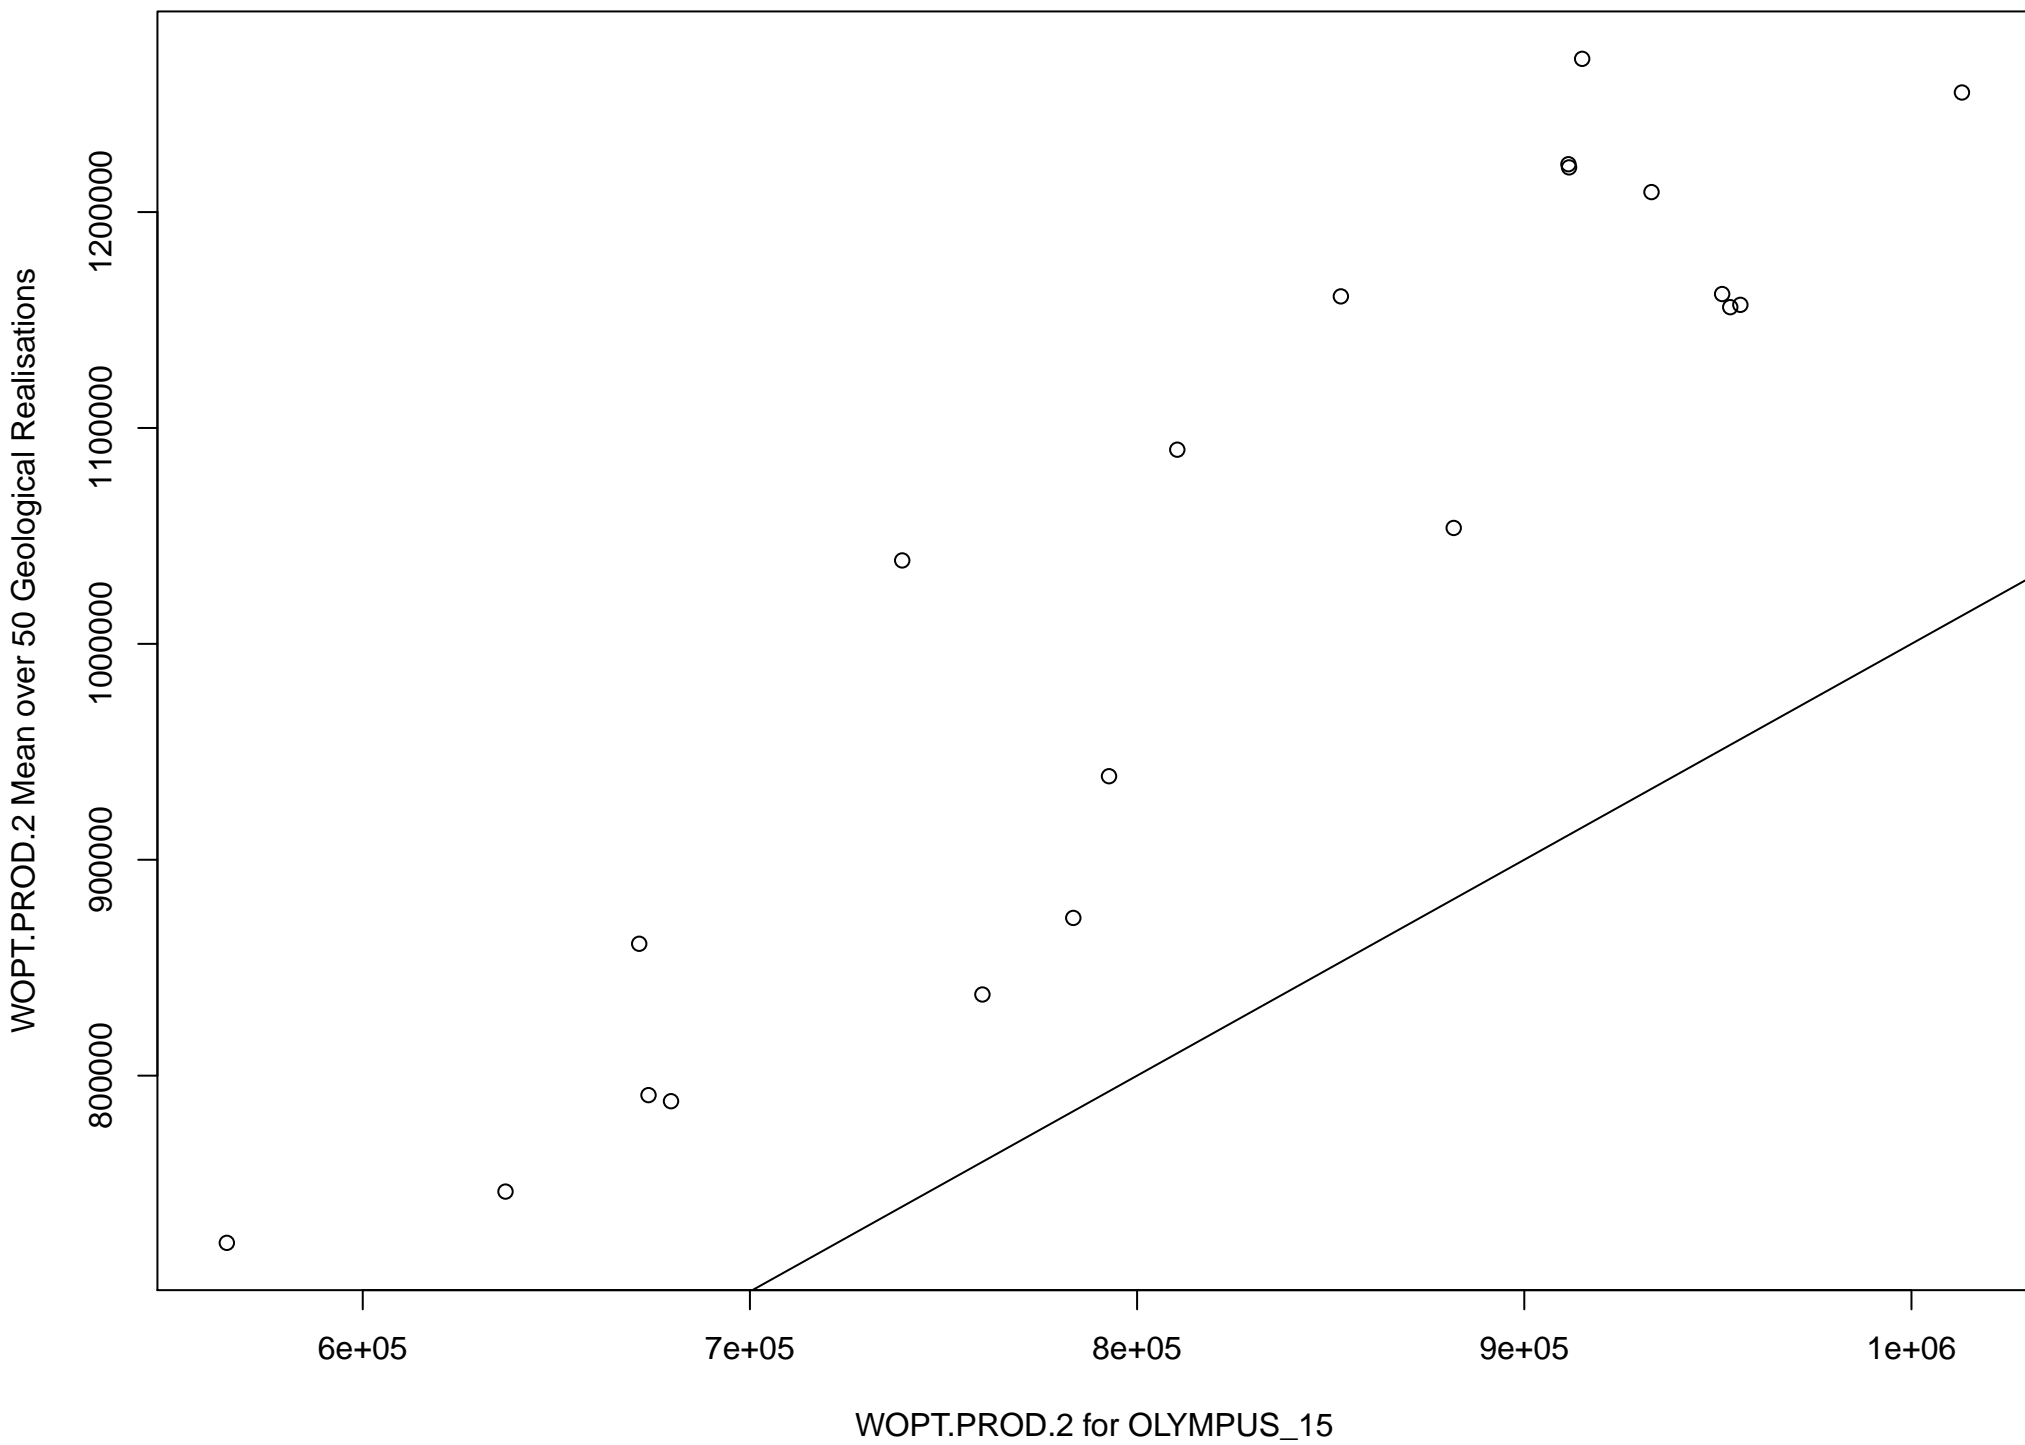

WOPT.PROD.2 for OLYMPUS\_16

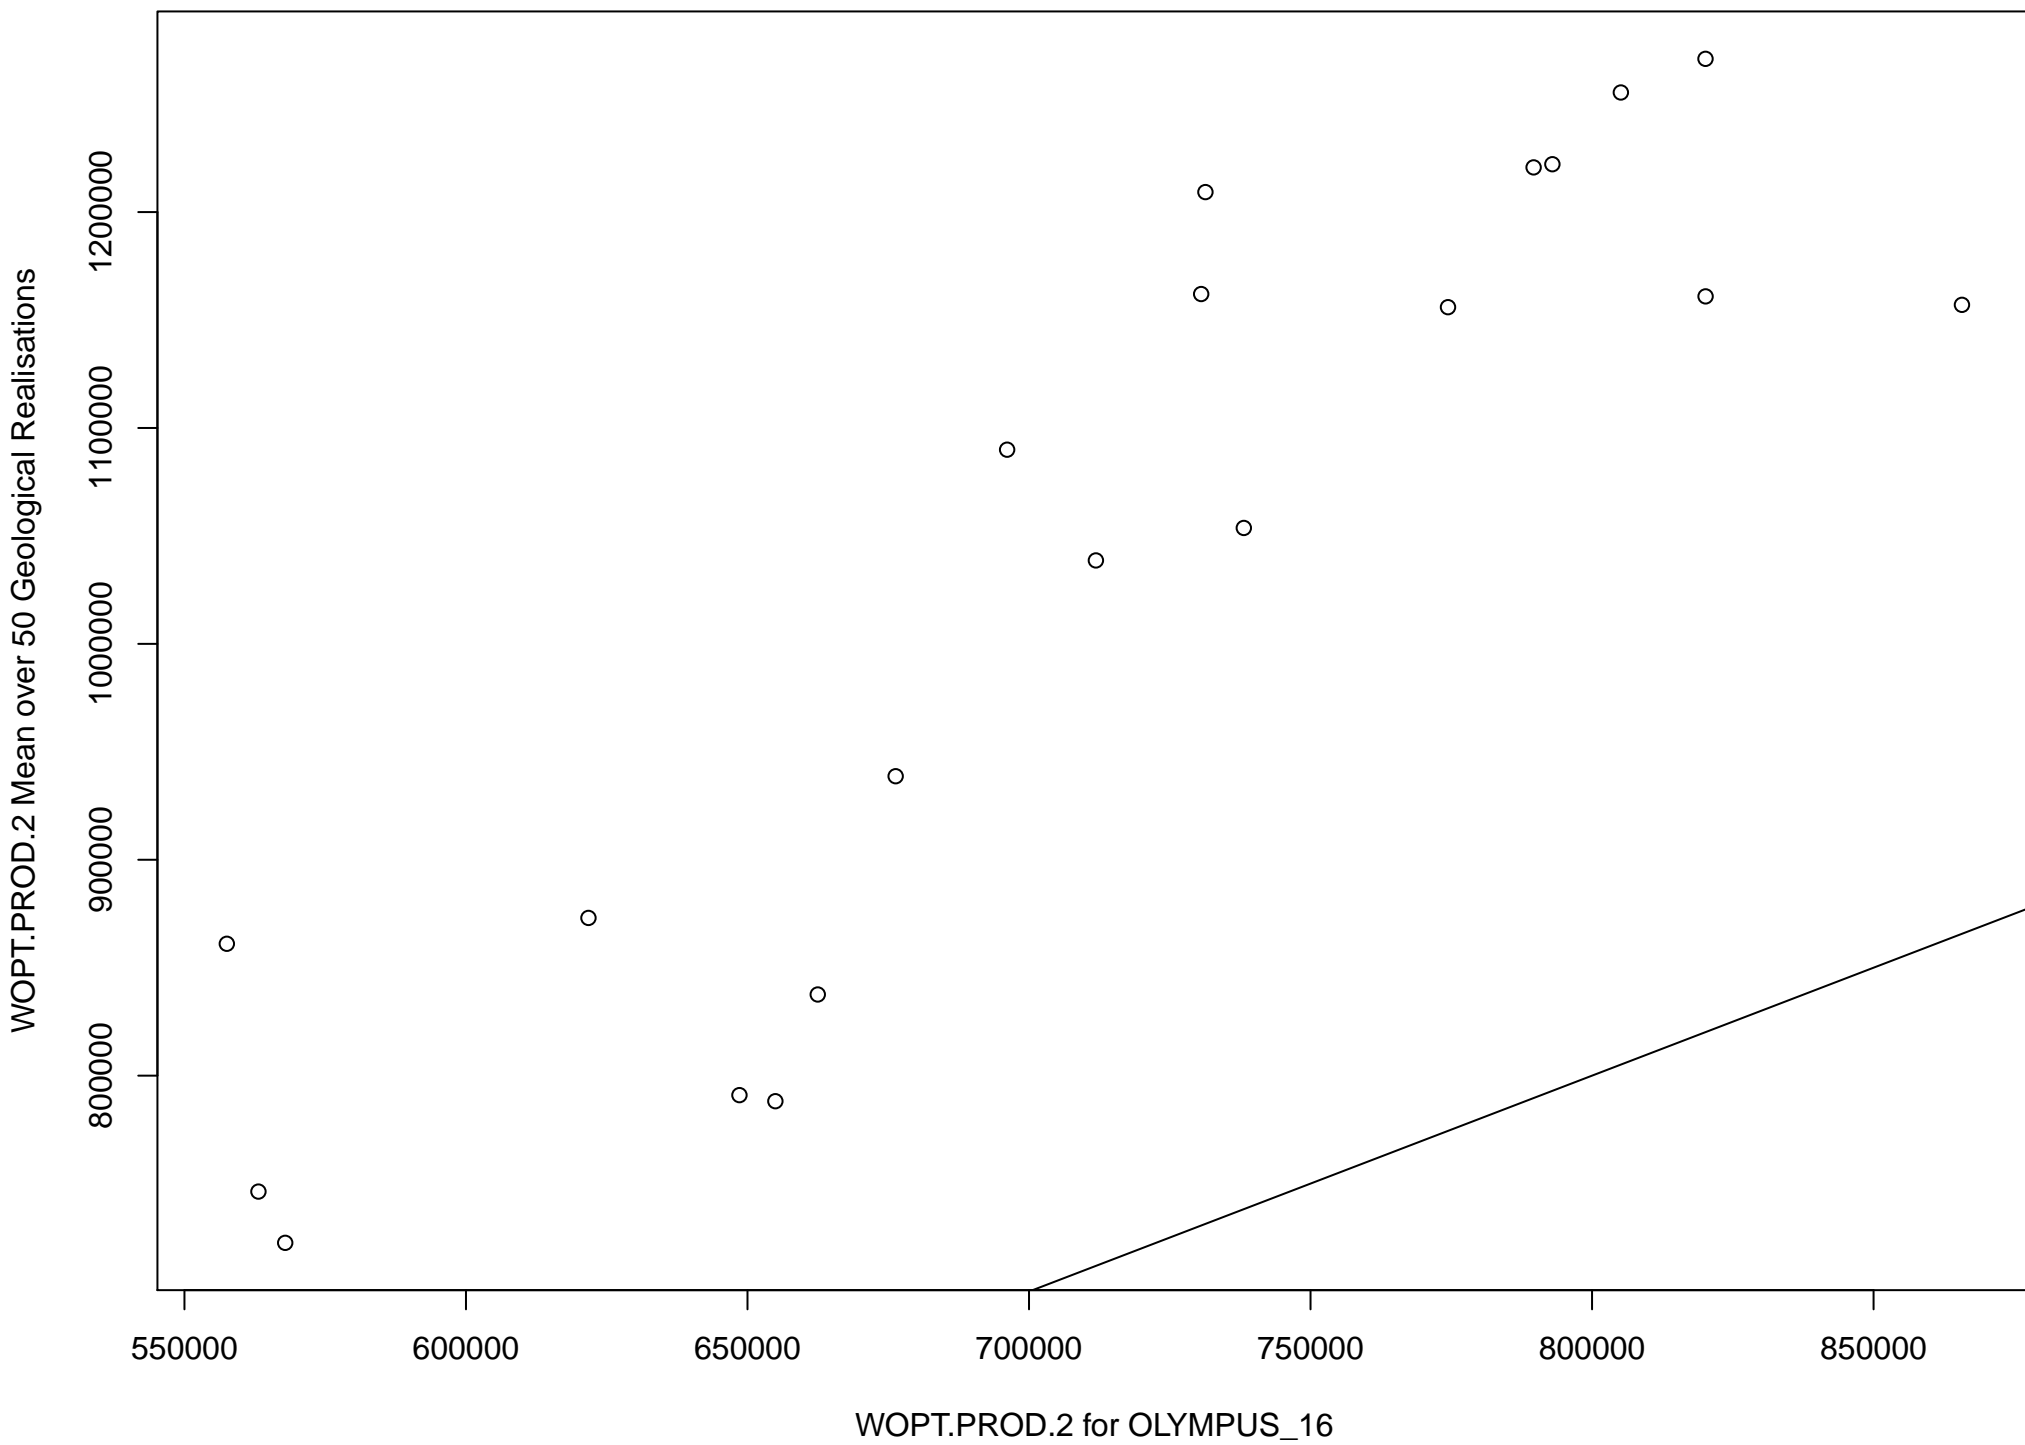



WOPT.PROD.2 for OLYMPUS\_17

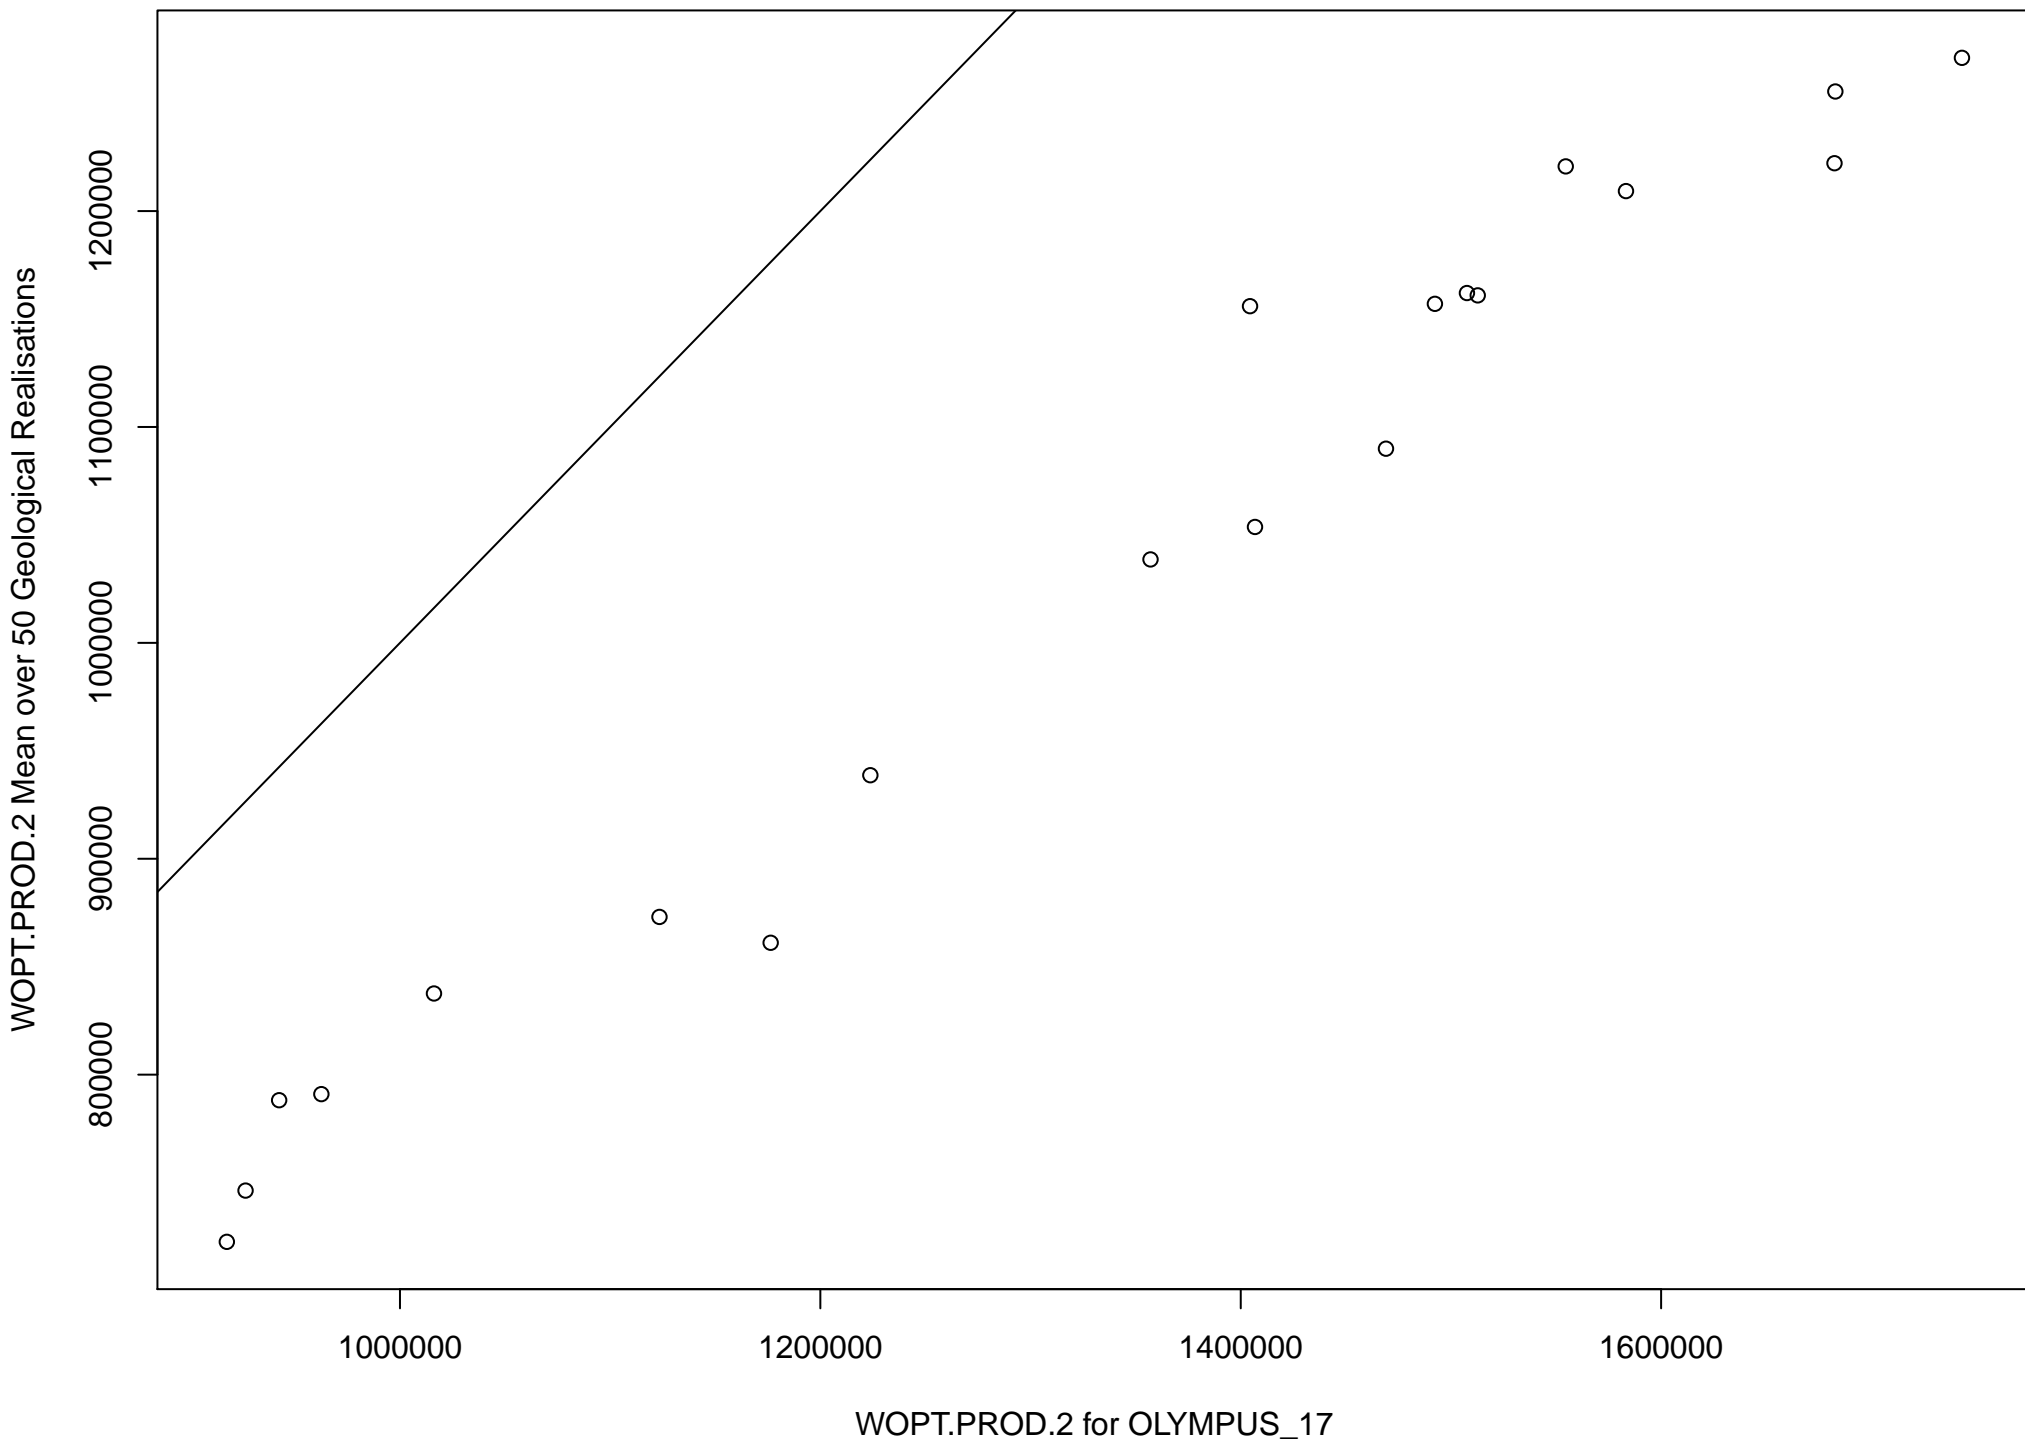

WOPT.PROD.2 for OLYMPUS\_18

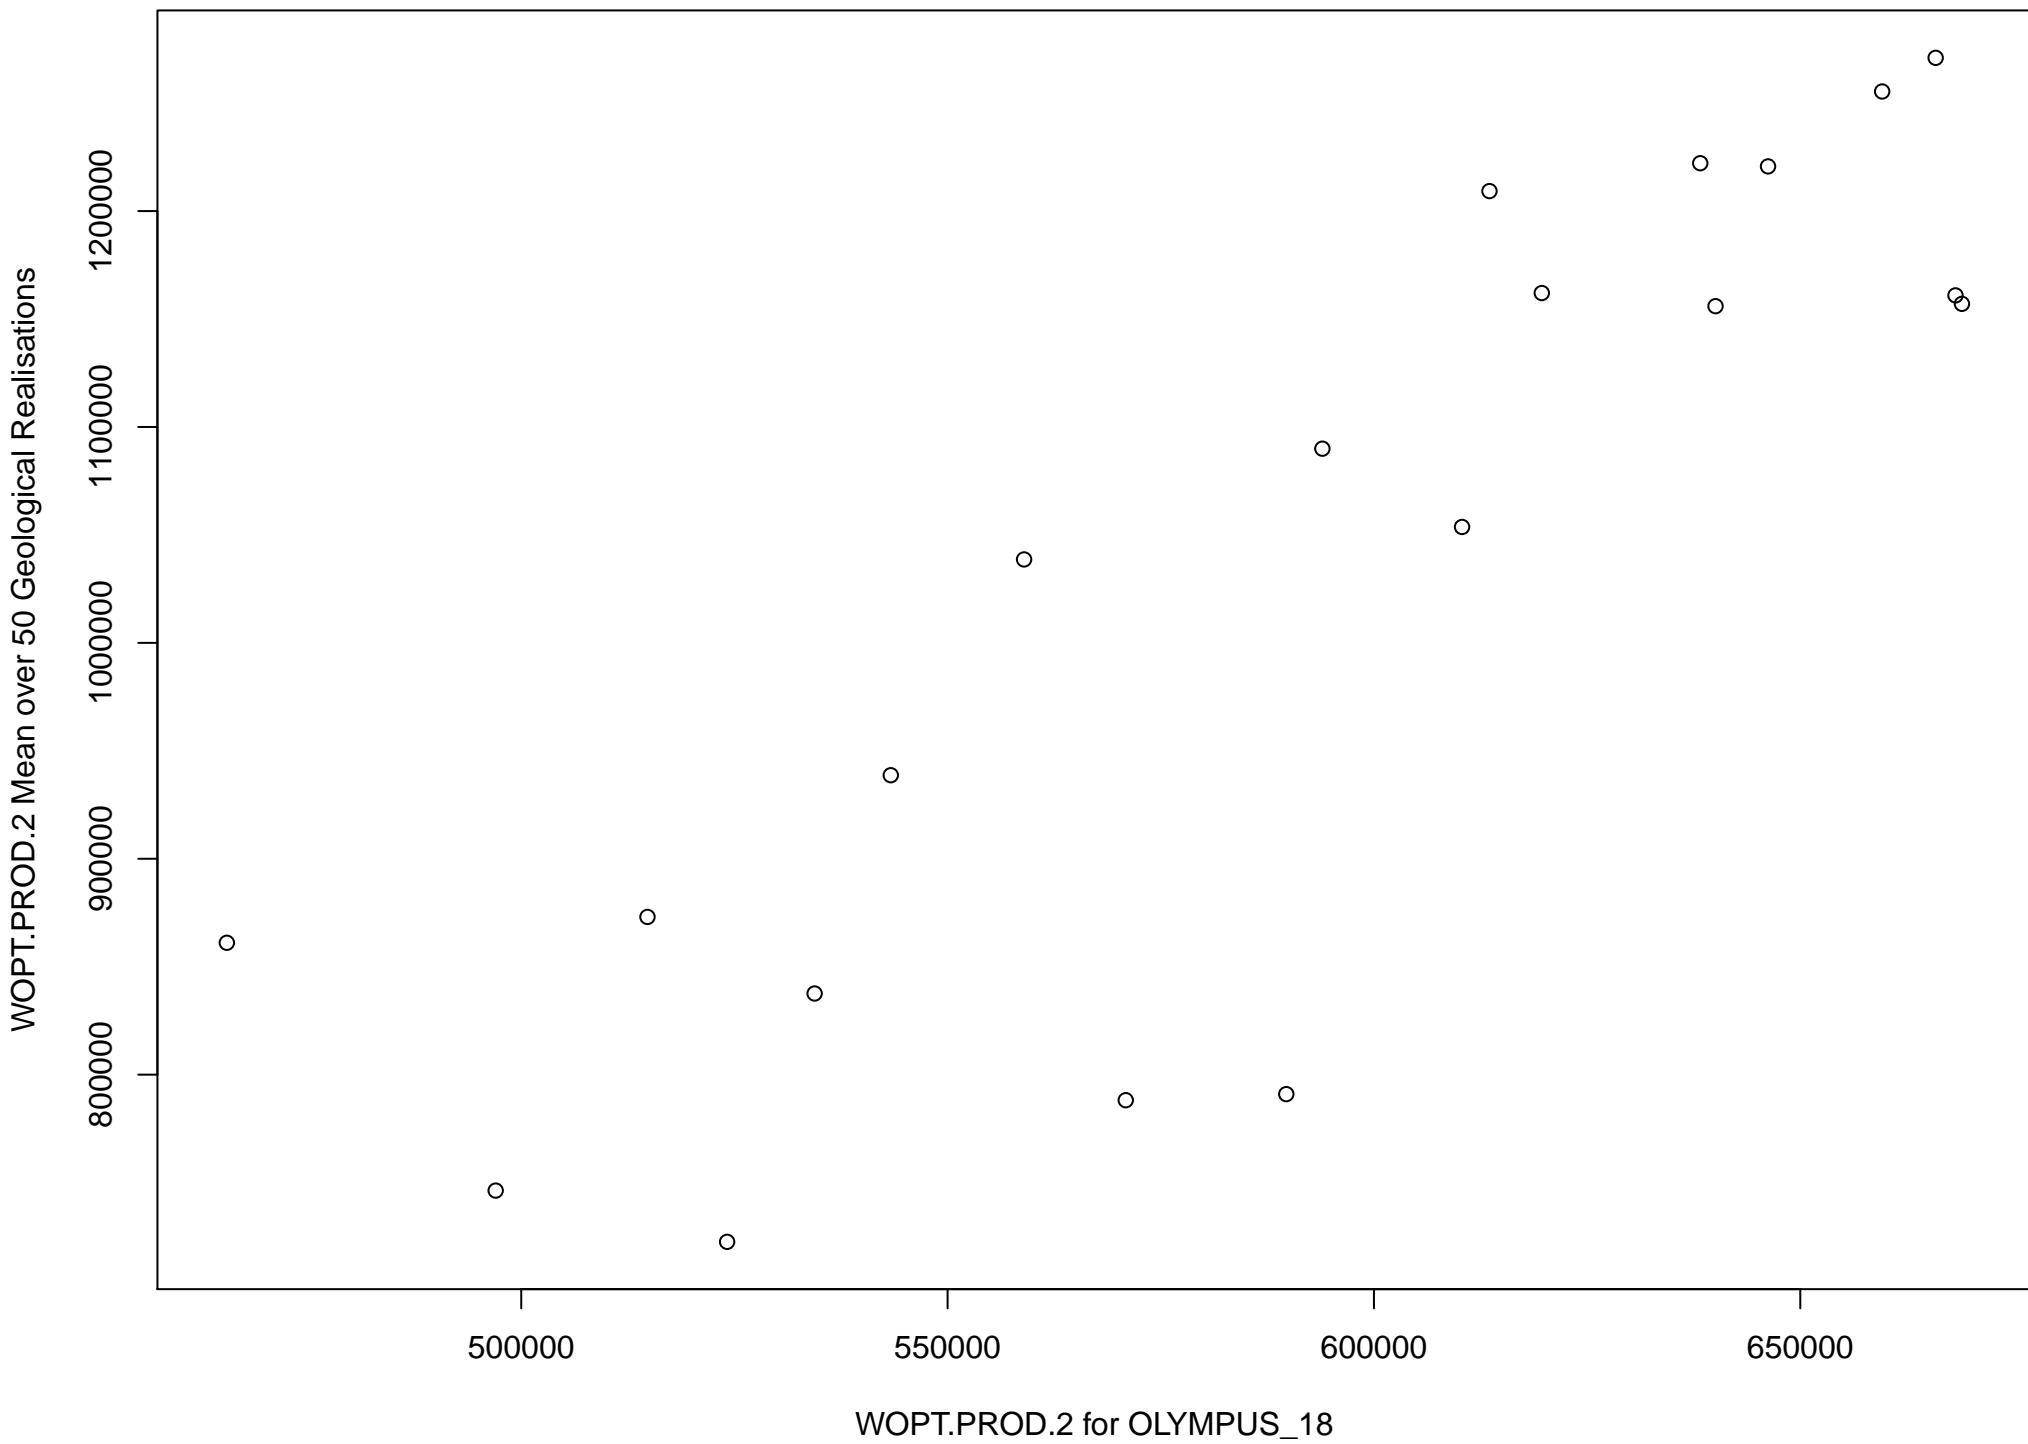

WOPT.PROD.2 for OLYMPUS\_19

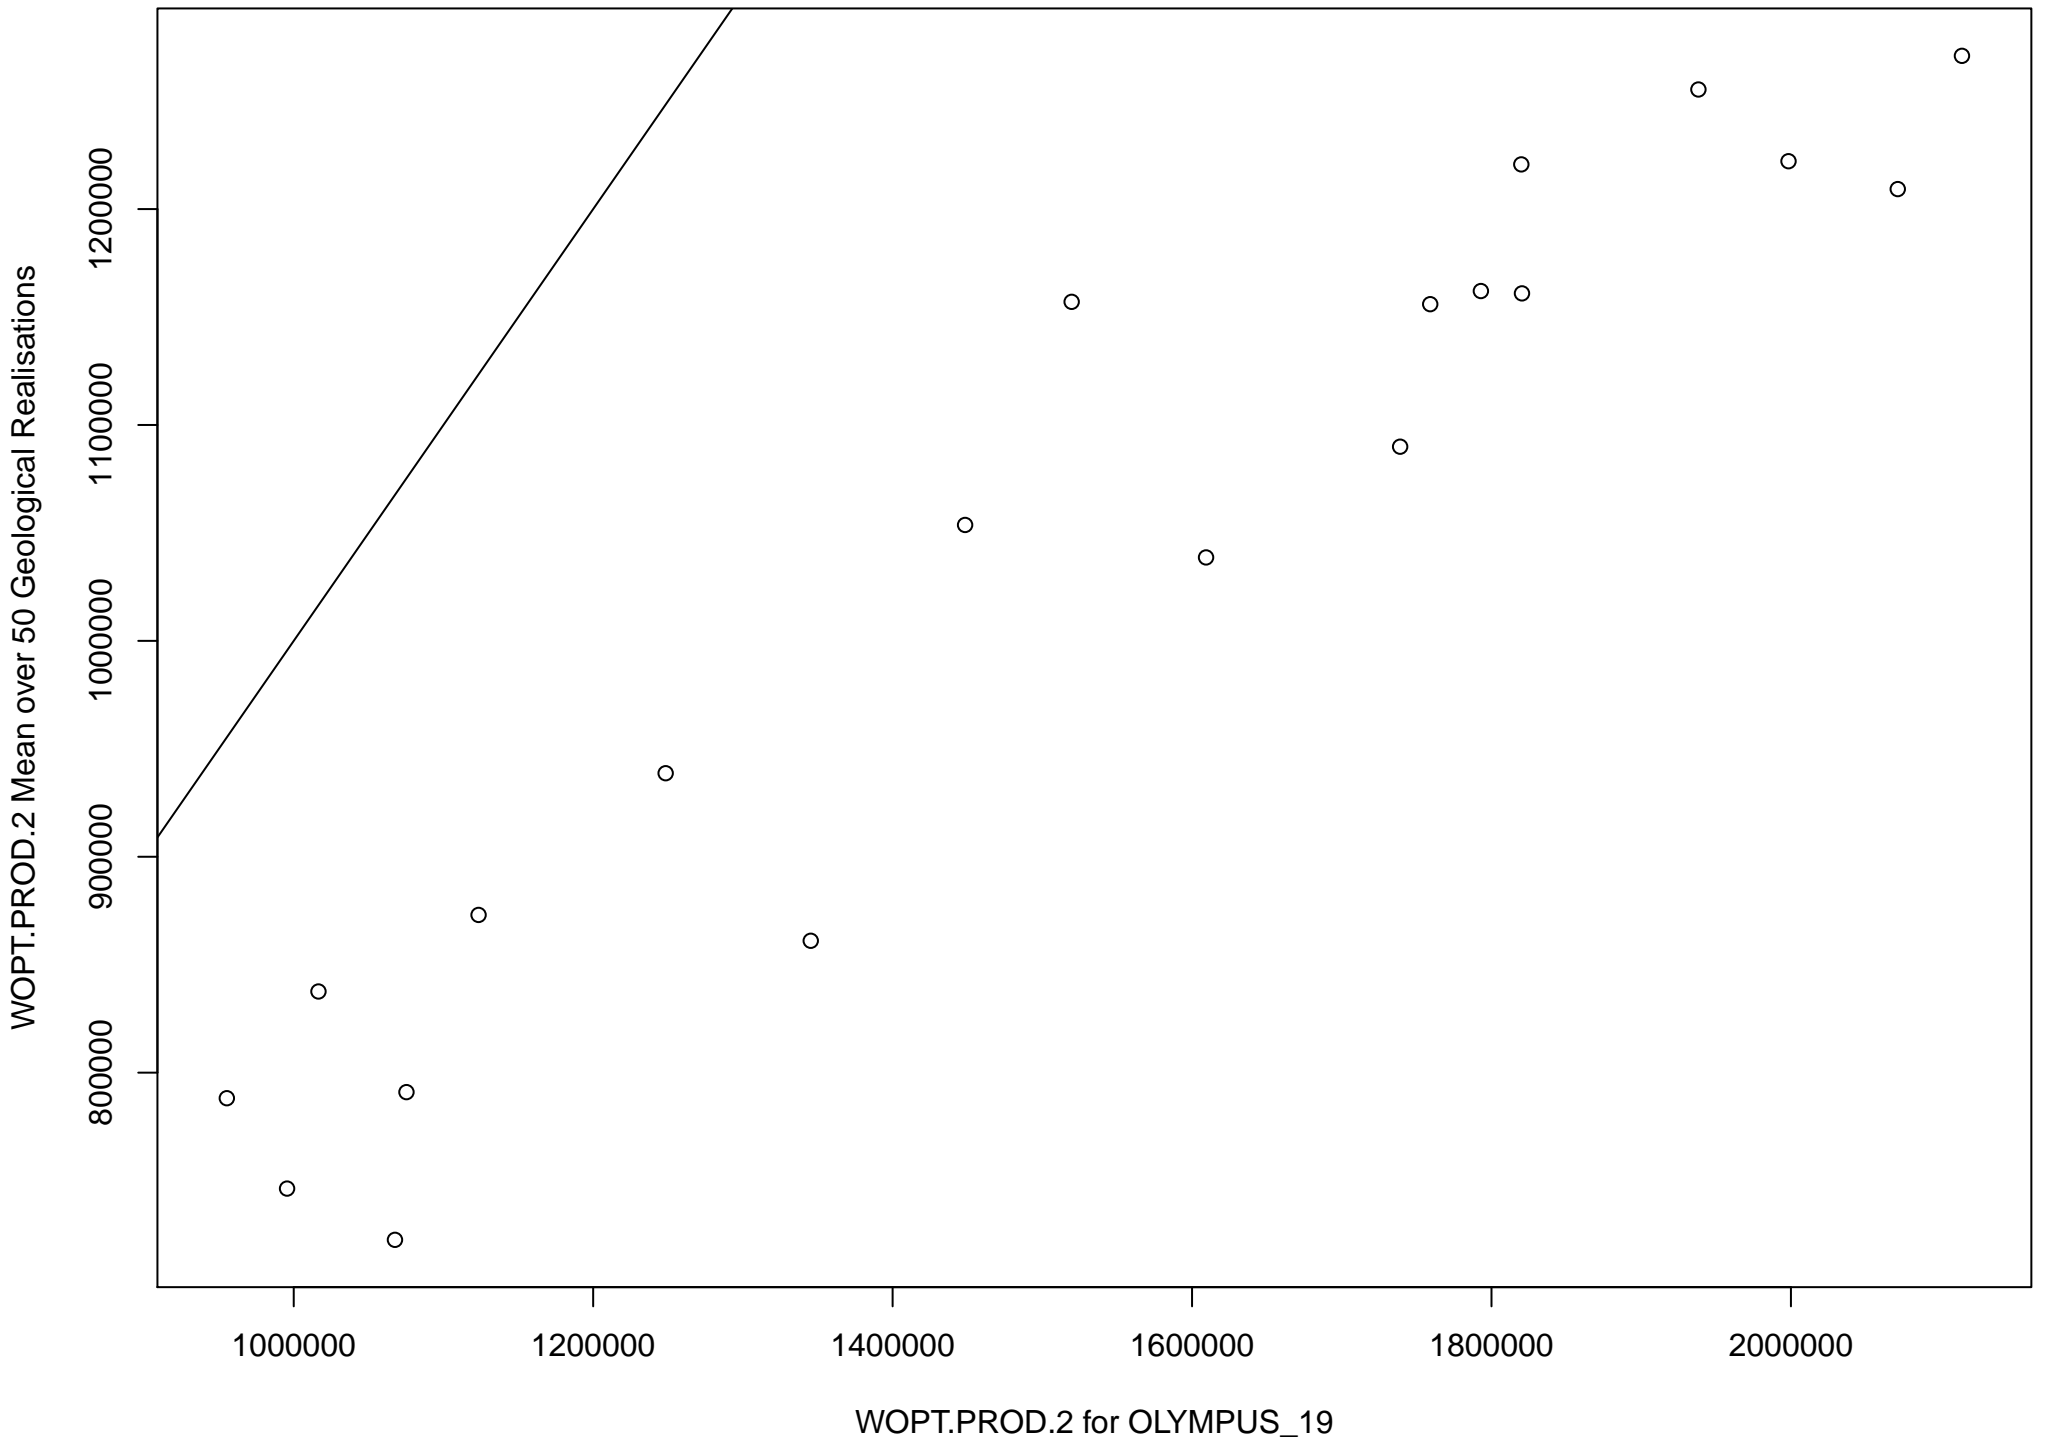

# WOPT.PROD.2 for OLYMPUS\_20

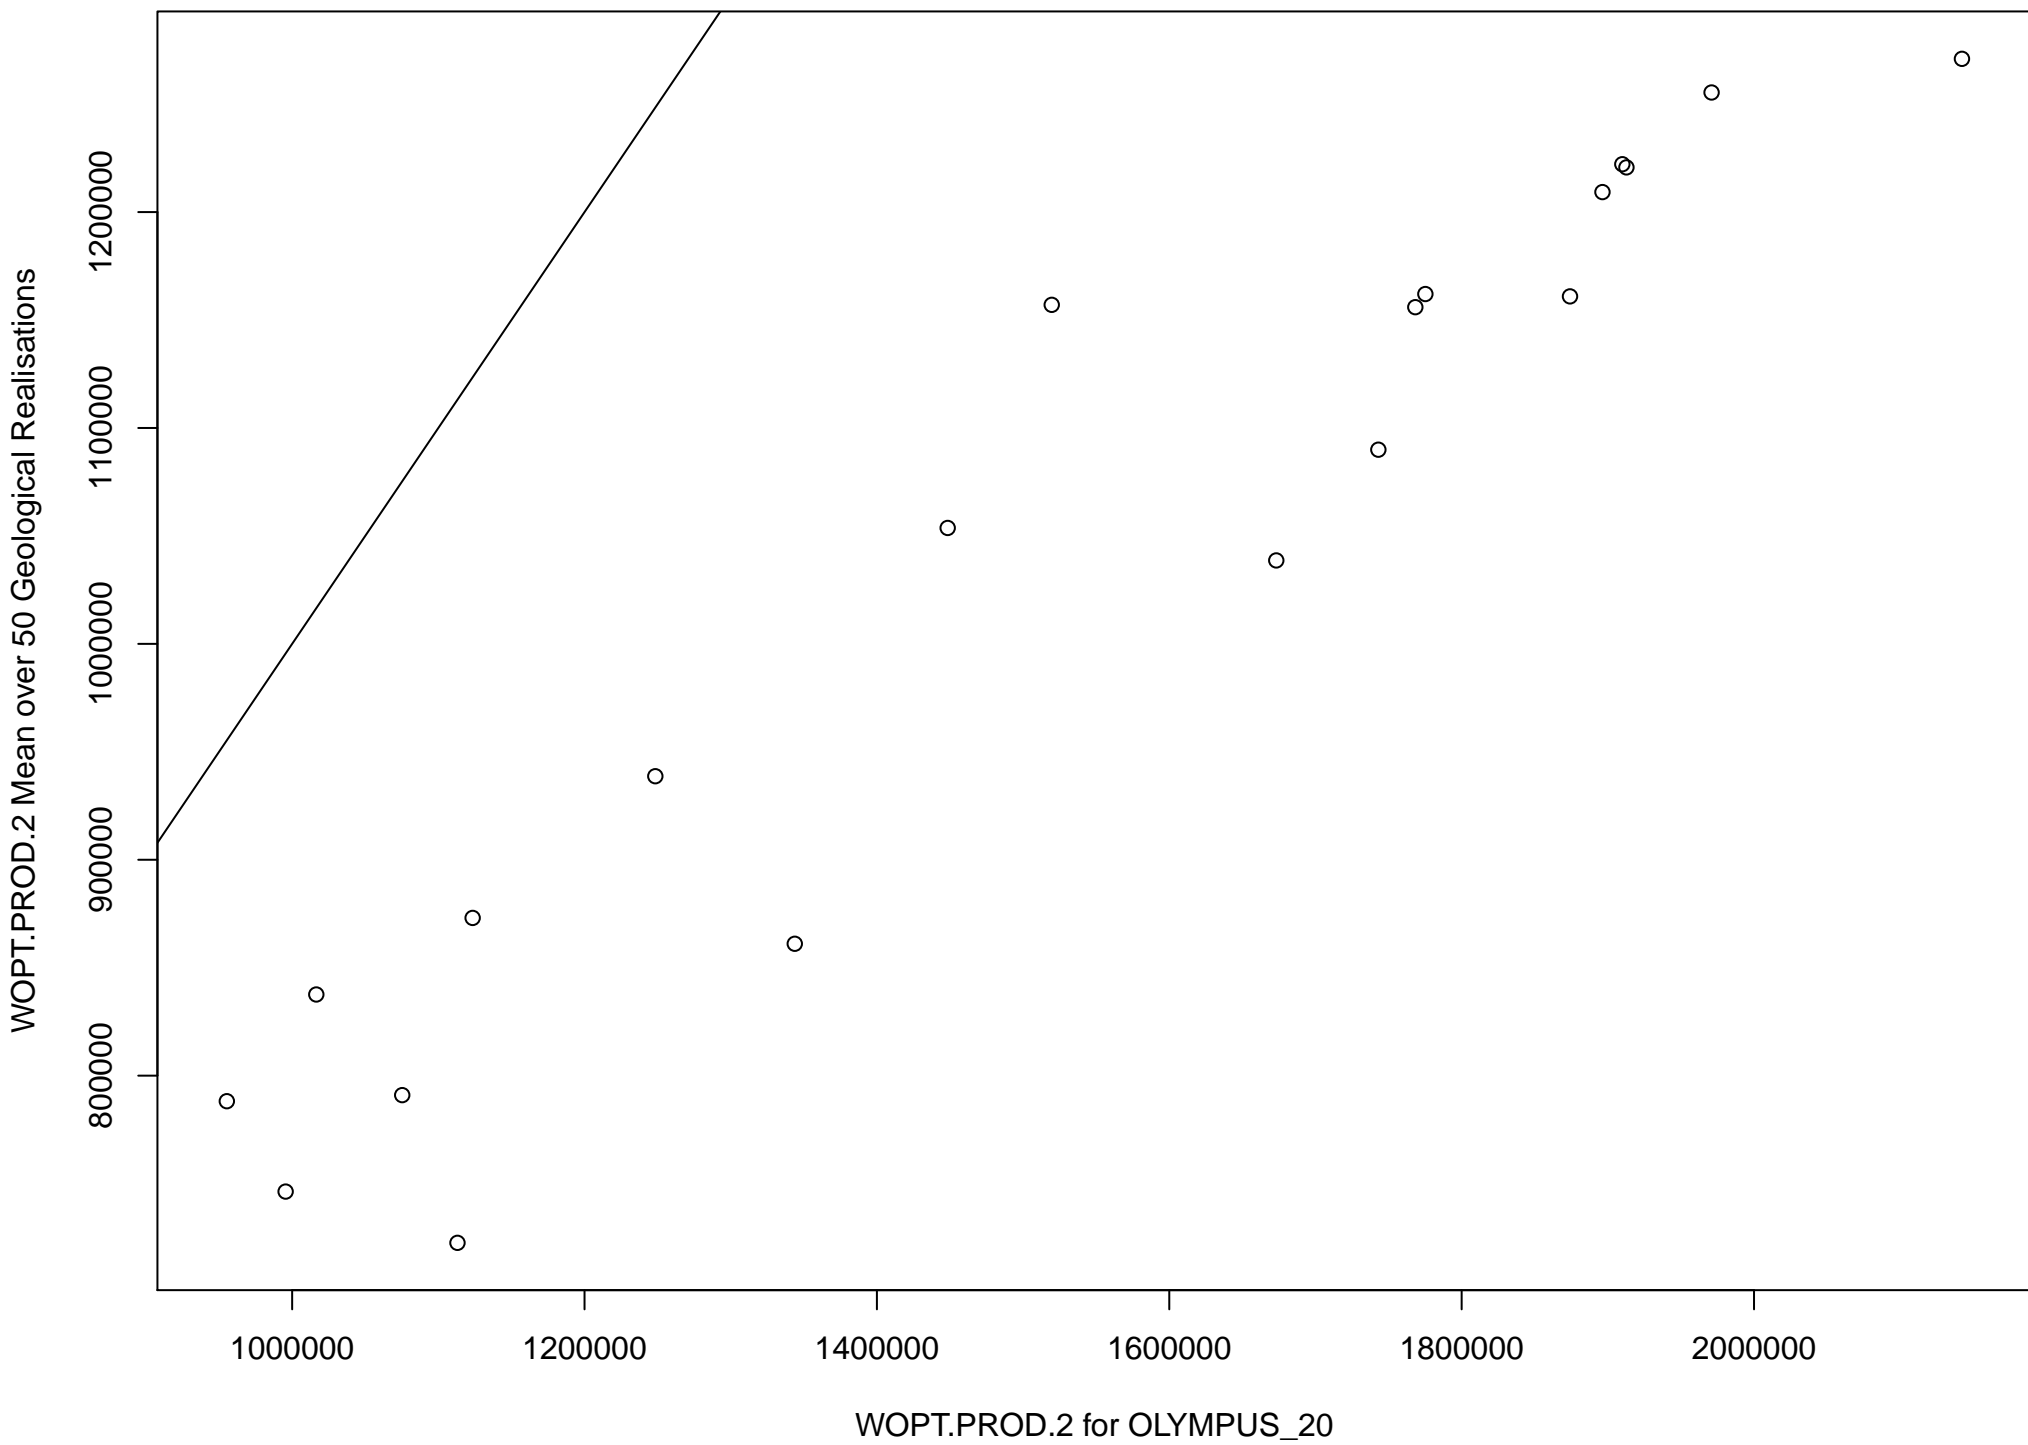

# WOPT.PROD.2 for OLYMPUS\_21

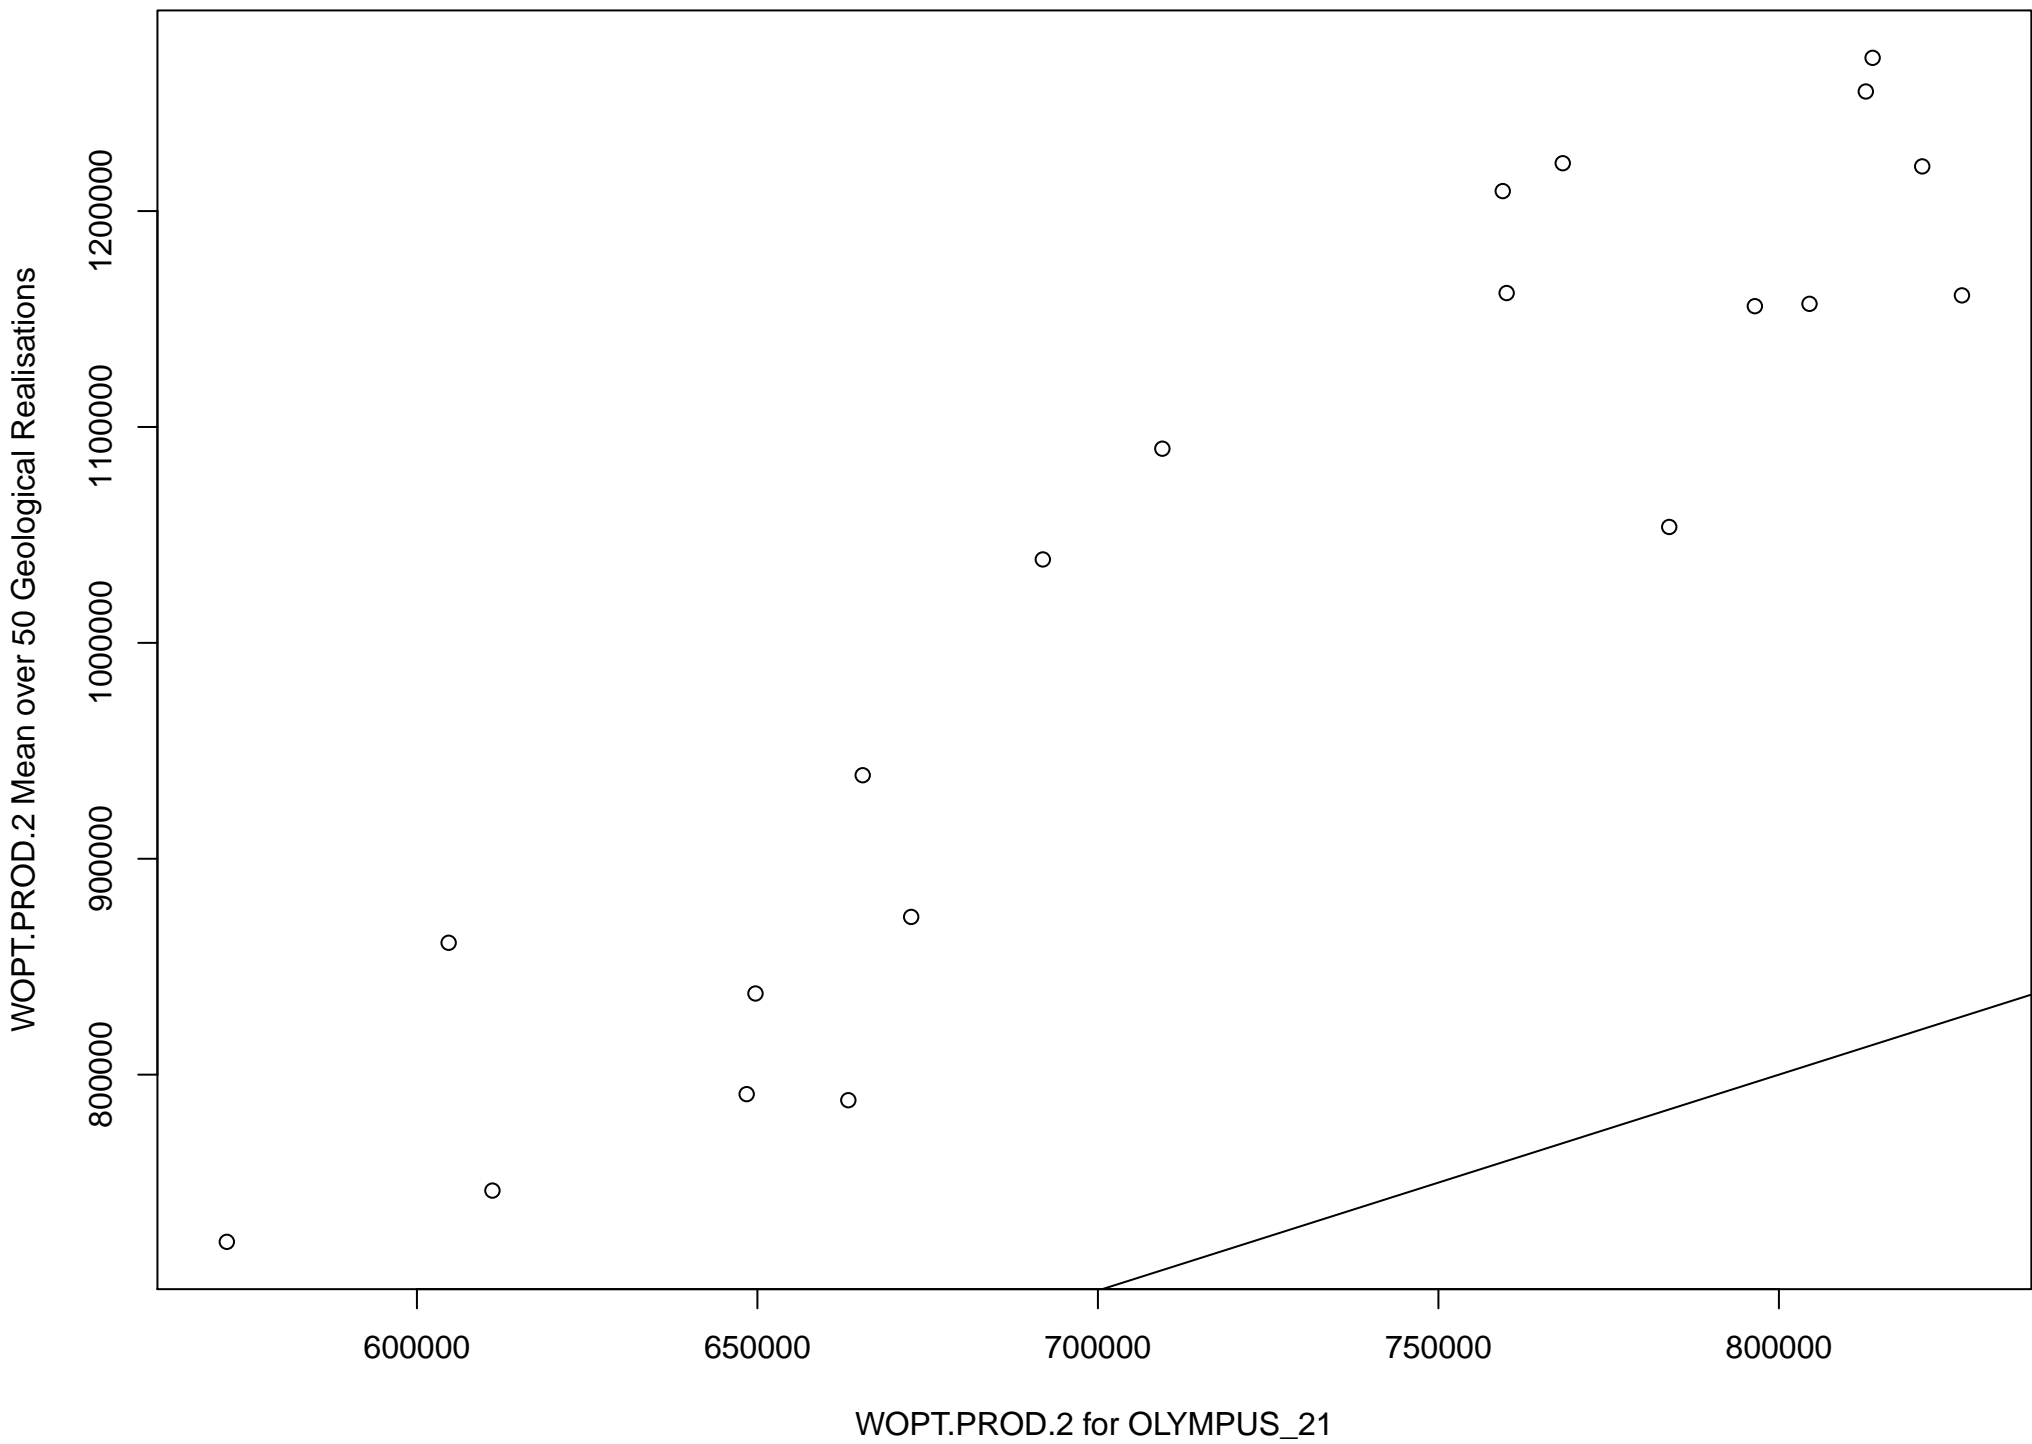

# WOPT.PROD.2 for OLYMPUS\_22

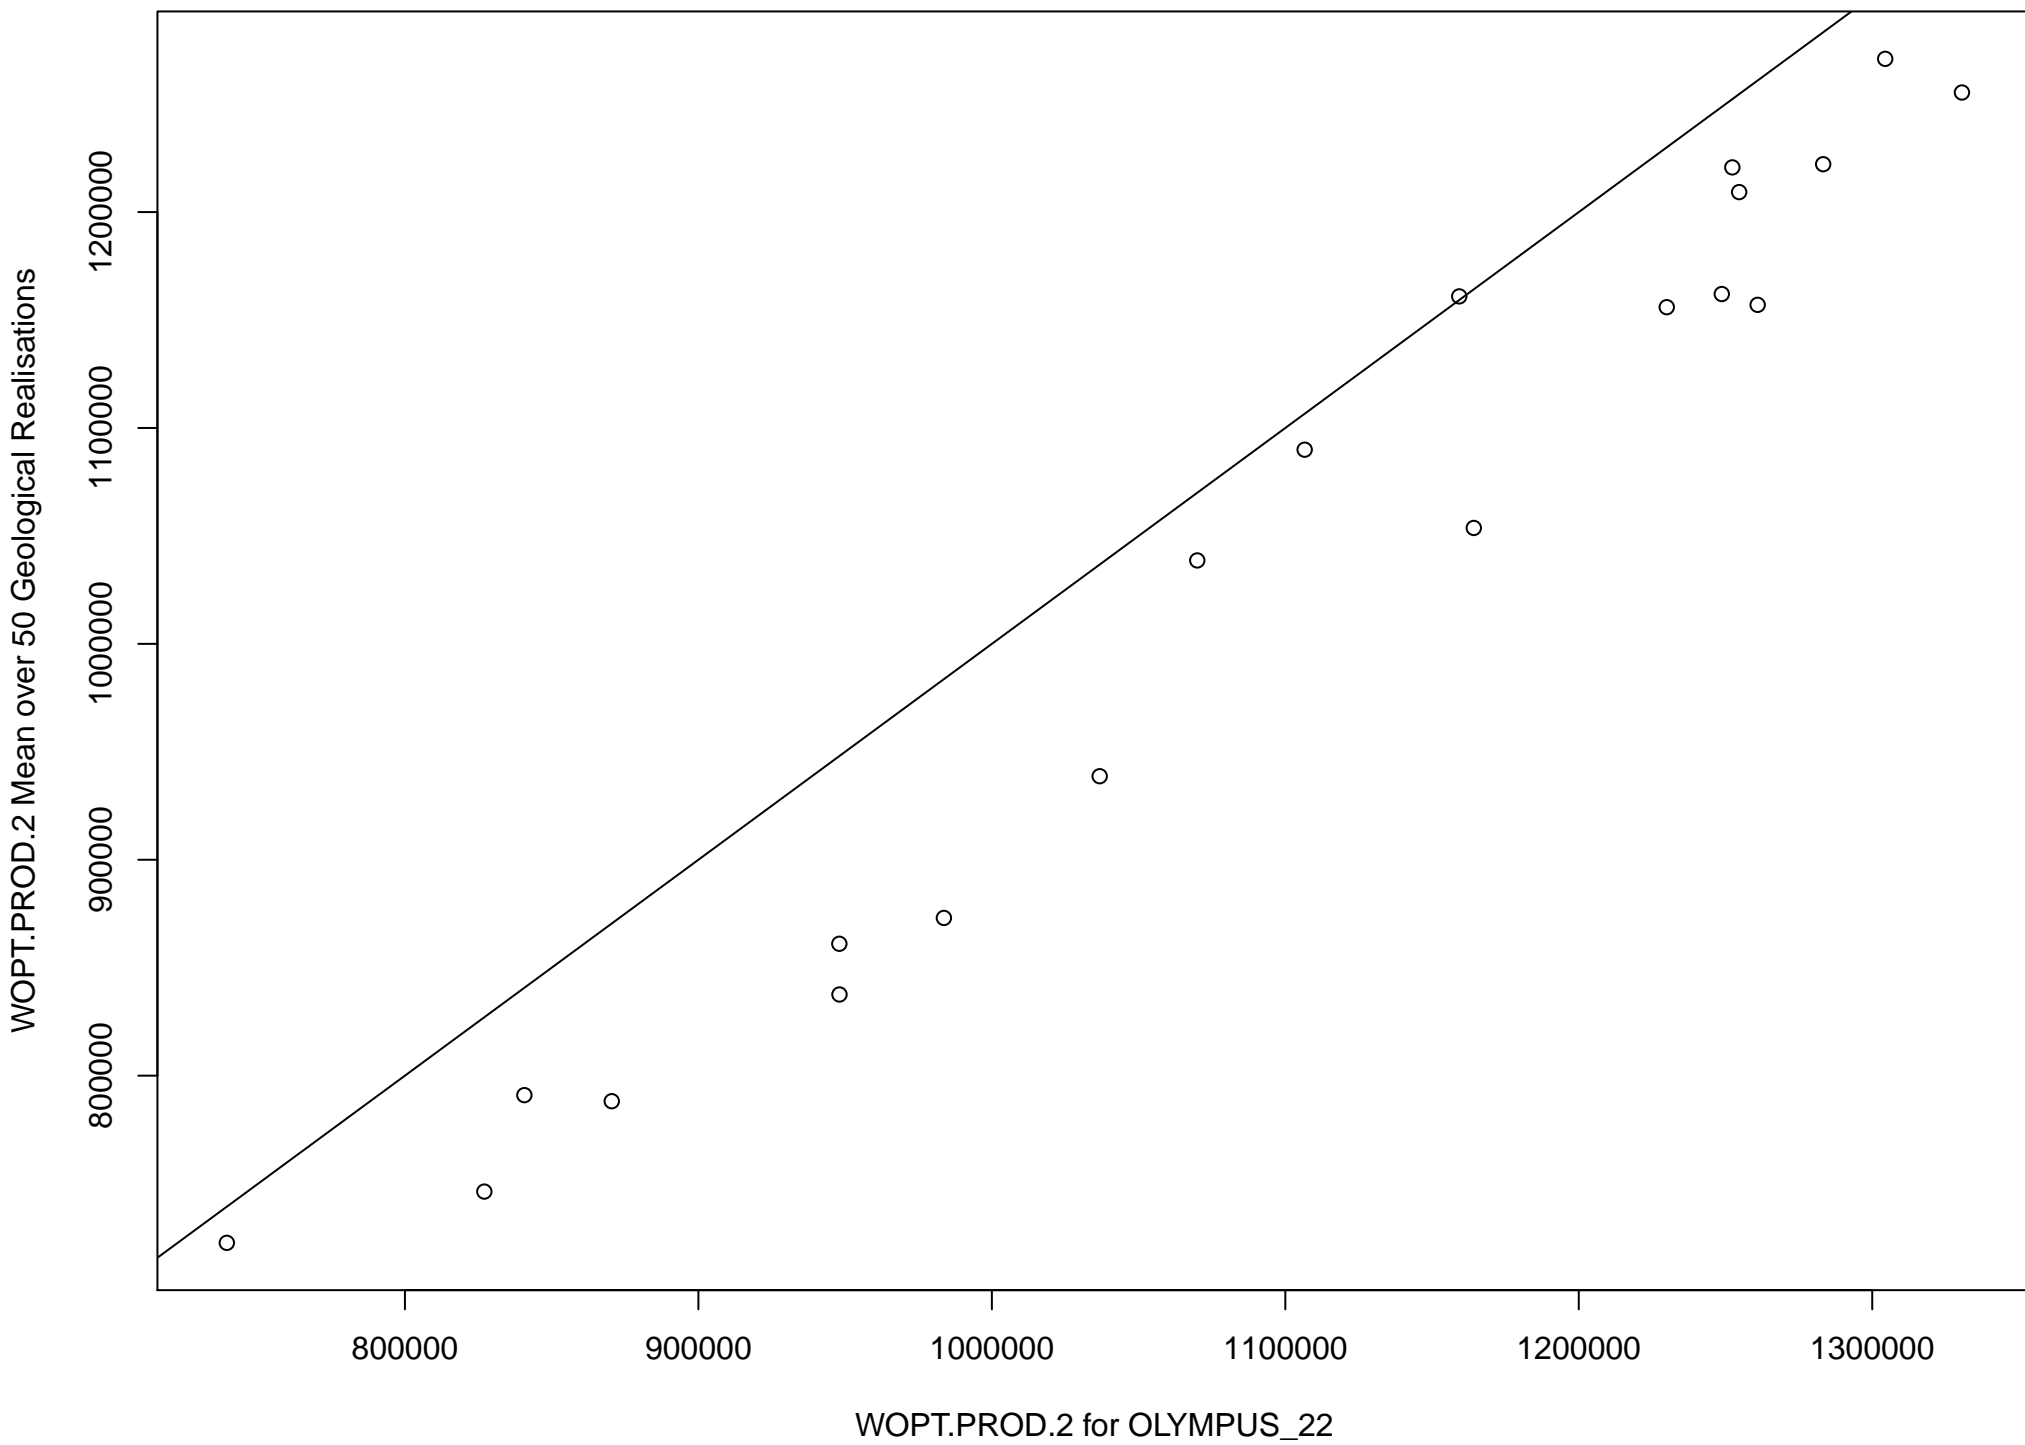

WOPT.PROD.2 for OLYMPUS\_23

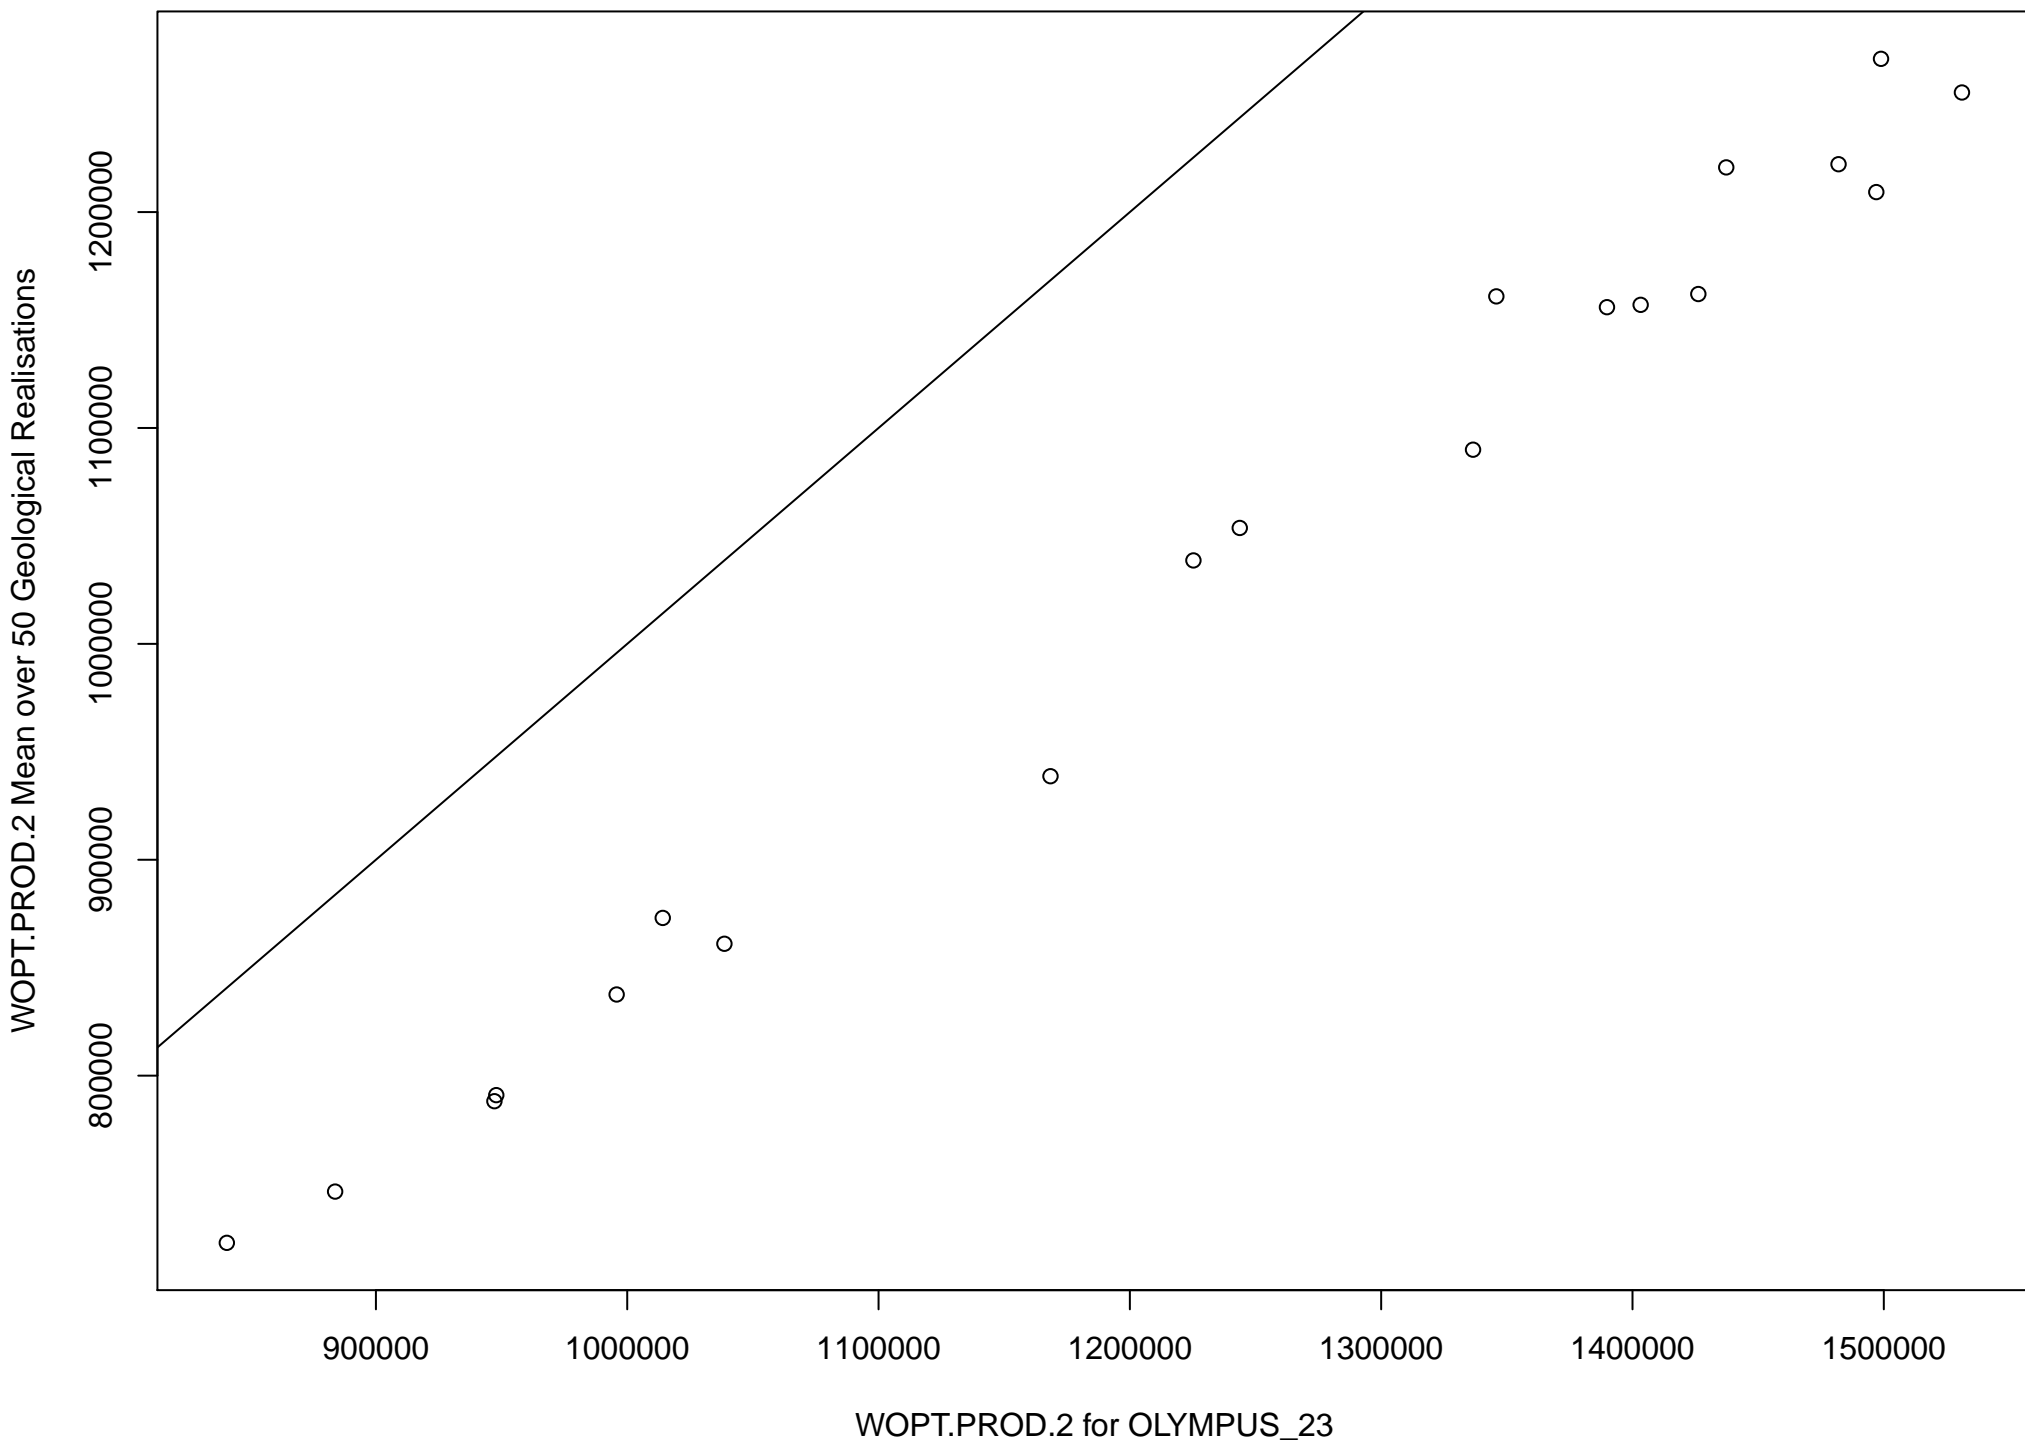

# WOPT.PROD.2 for OLYMPUS\_24

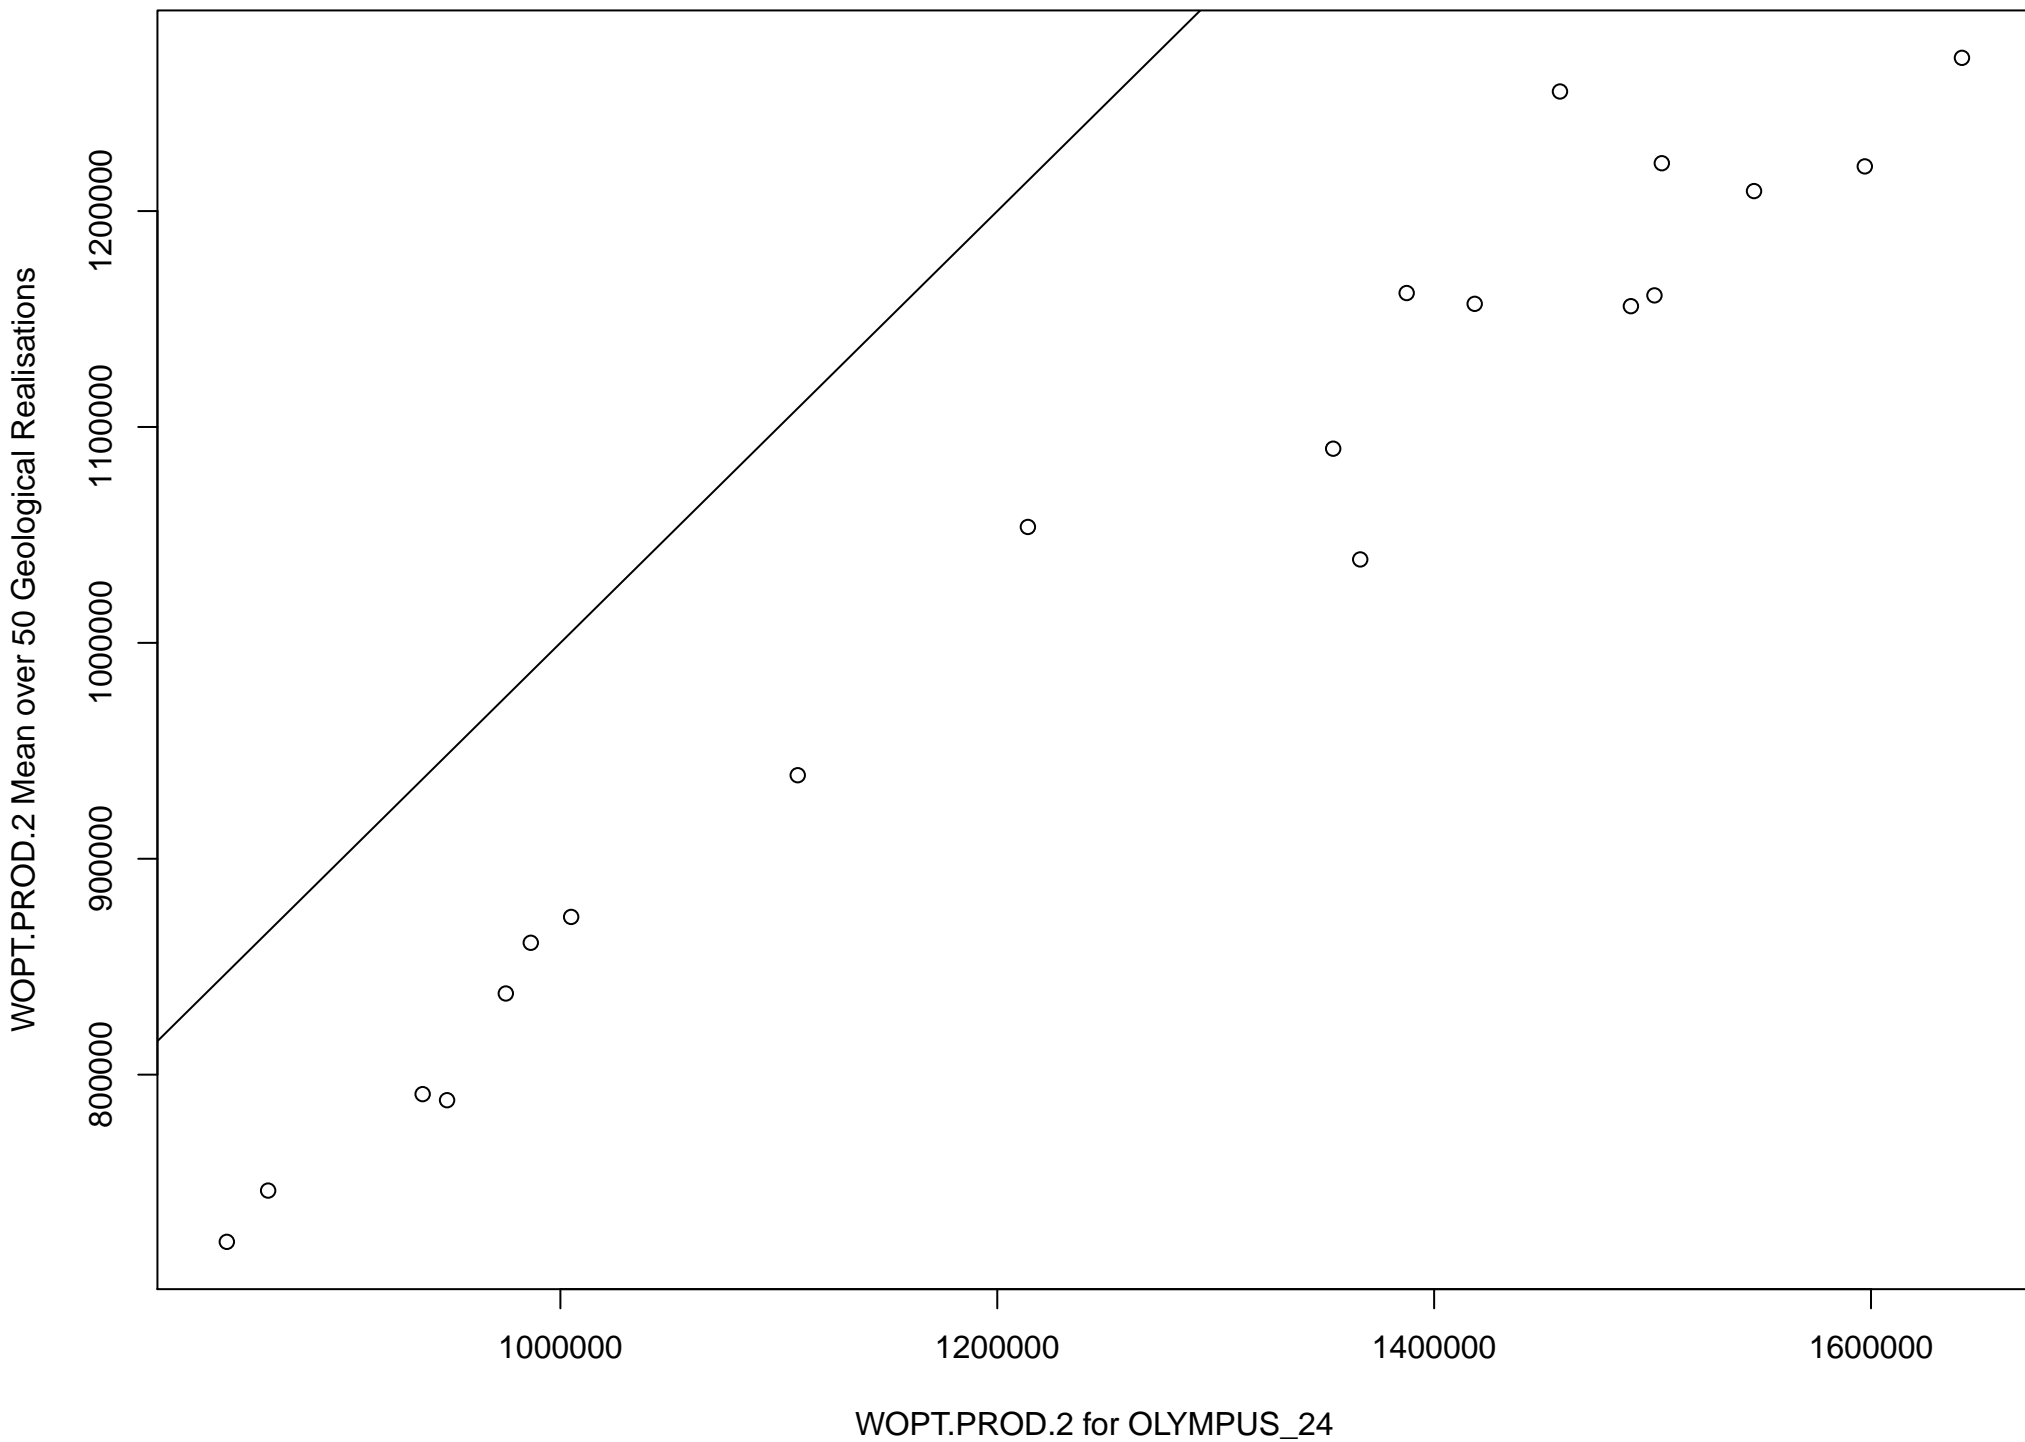



WOPT.PROD.2 for OLYMPUS\_25

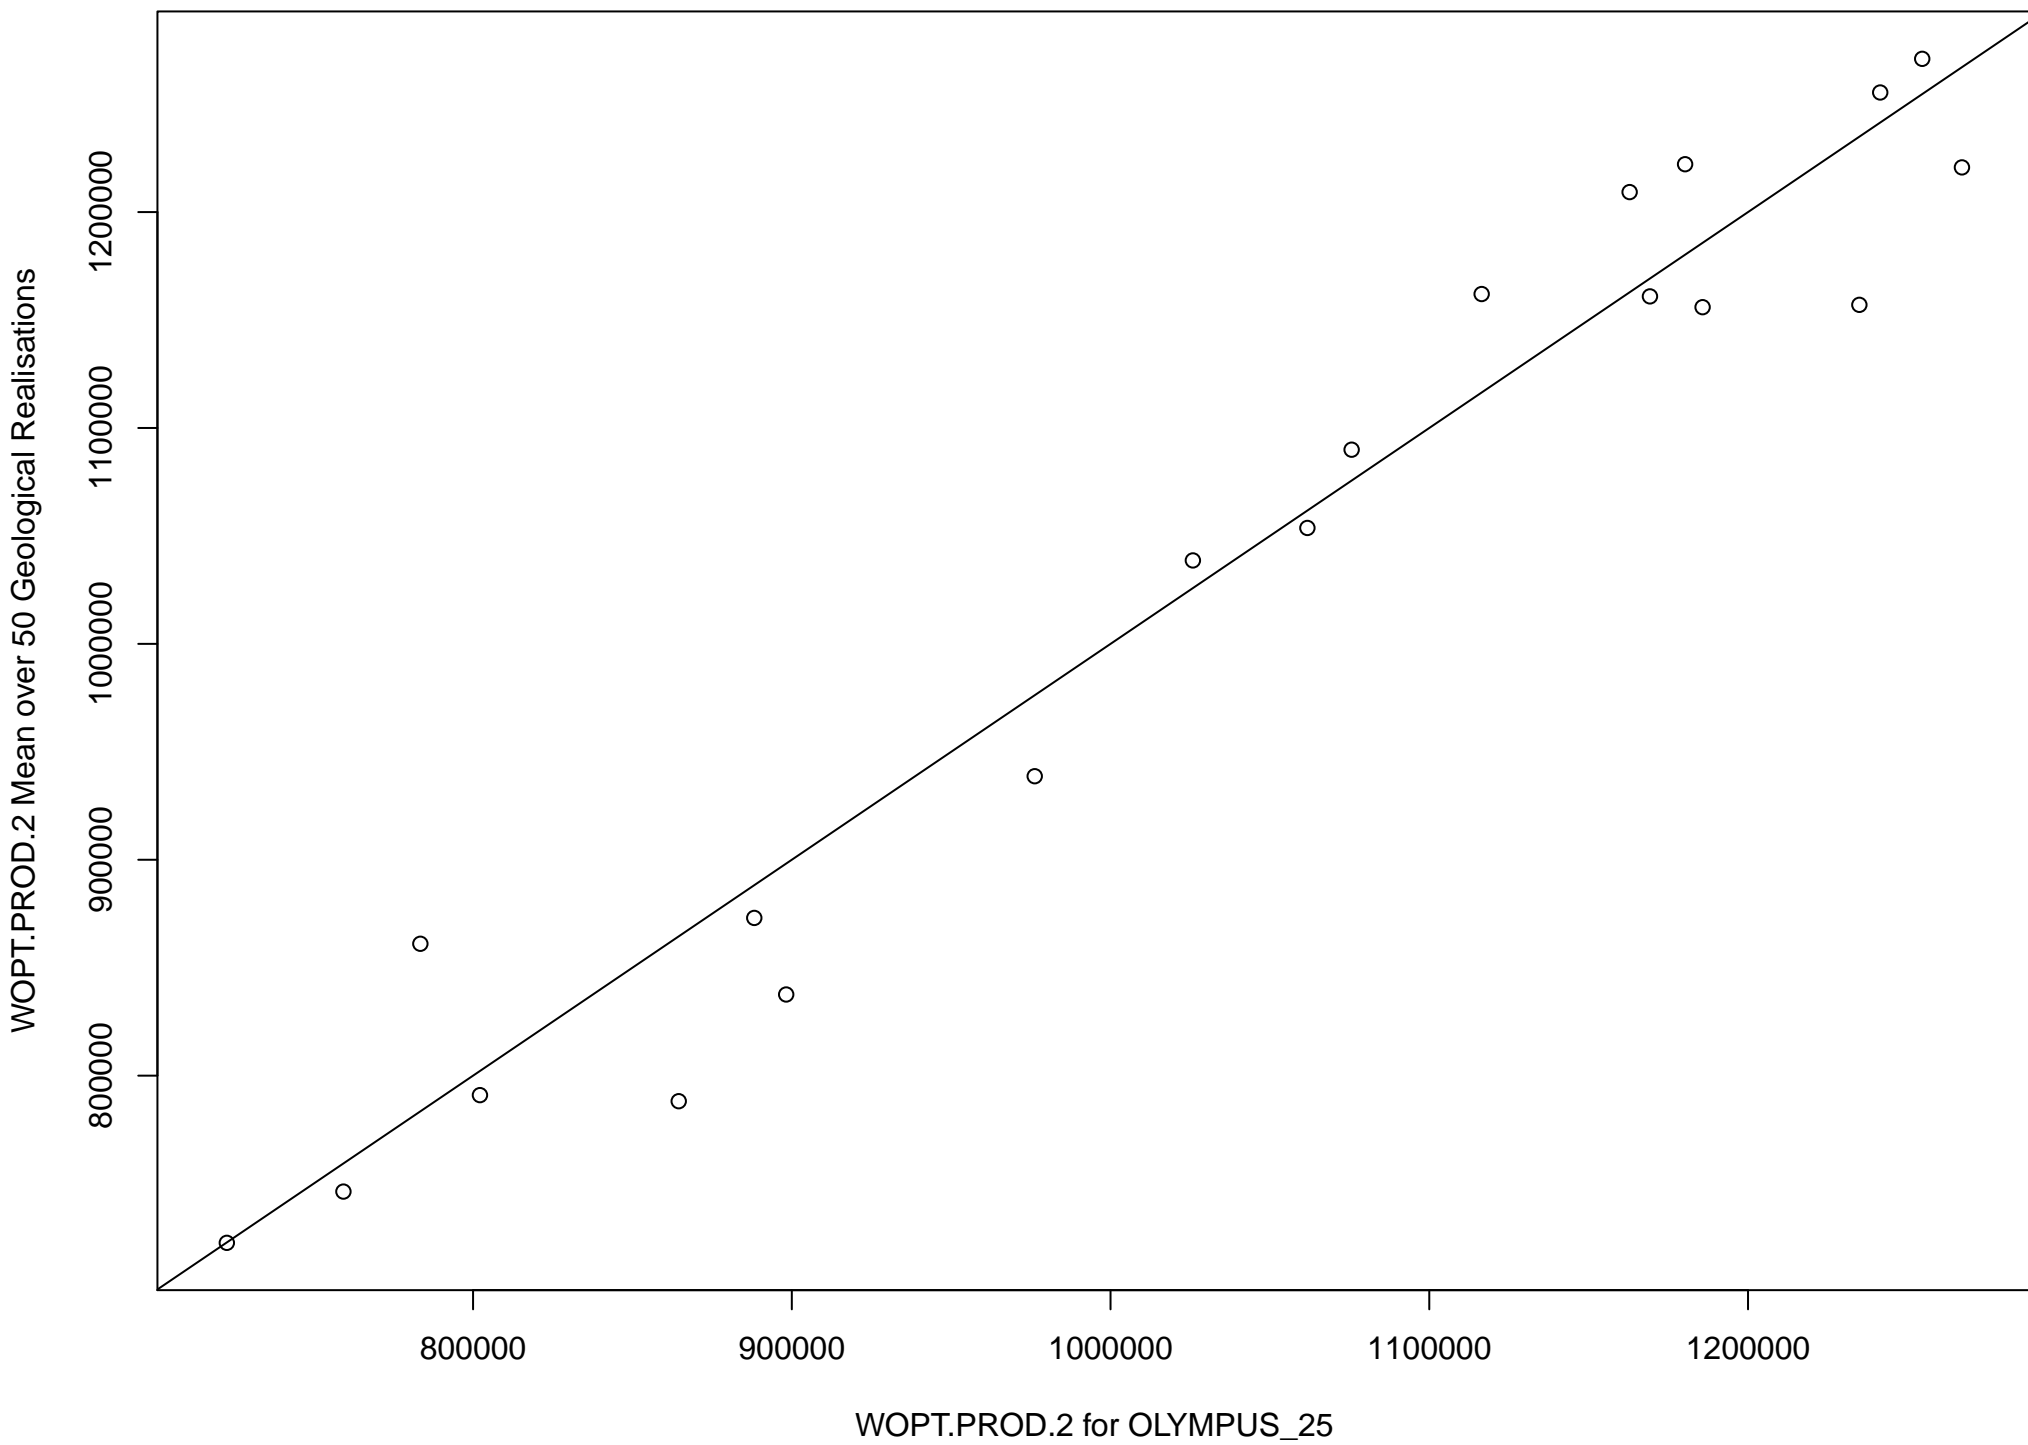

# WOPT.PROD.2 for OLYMPUS\_26

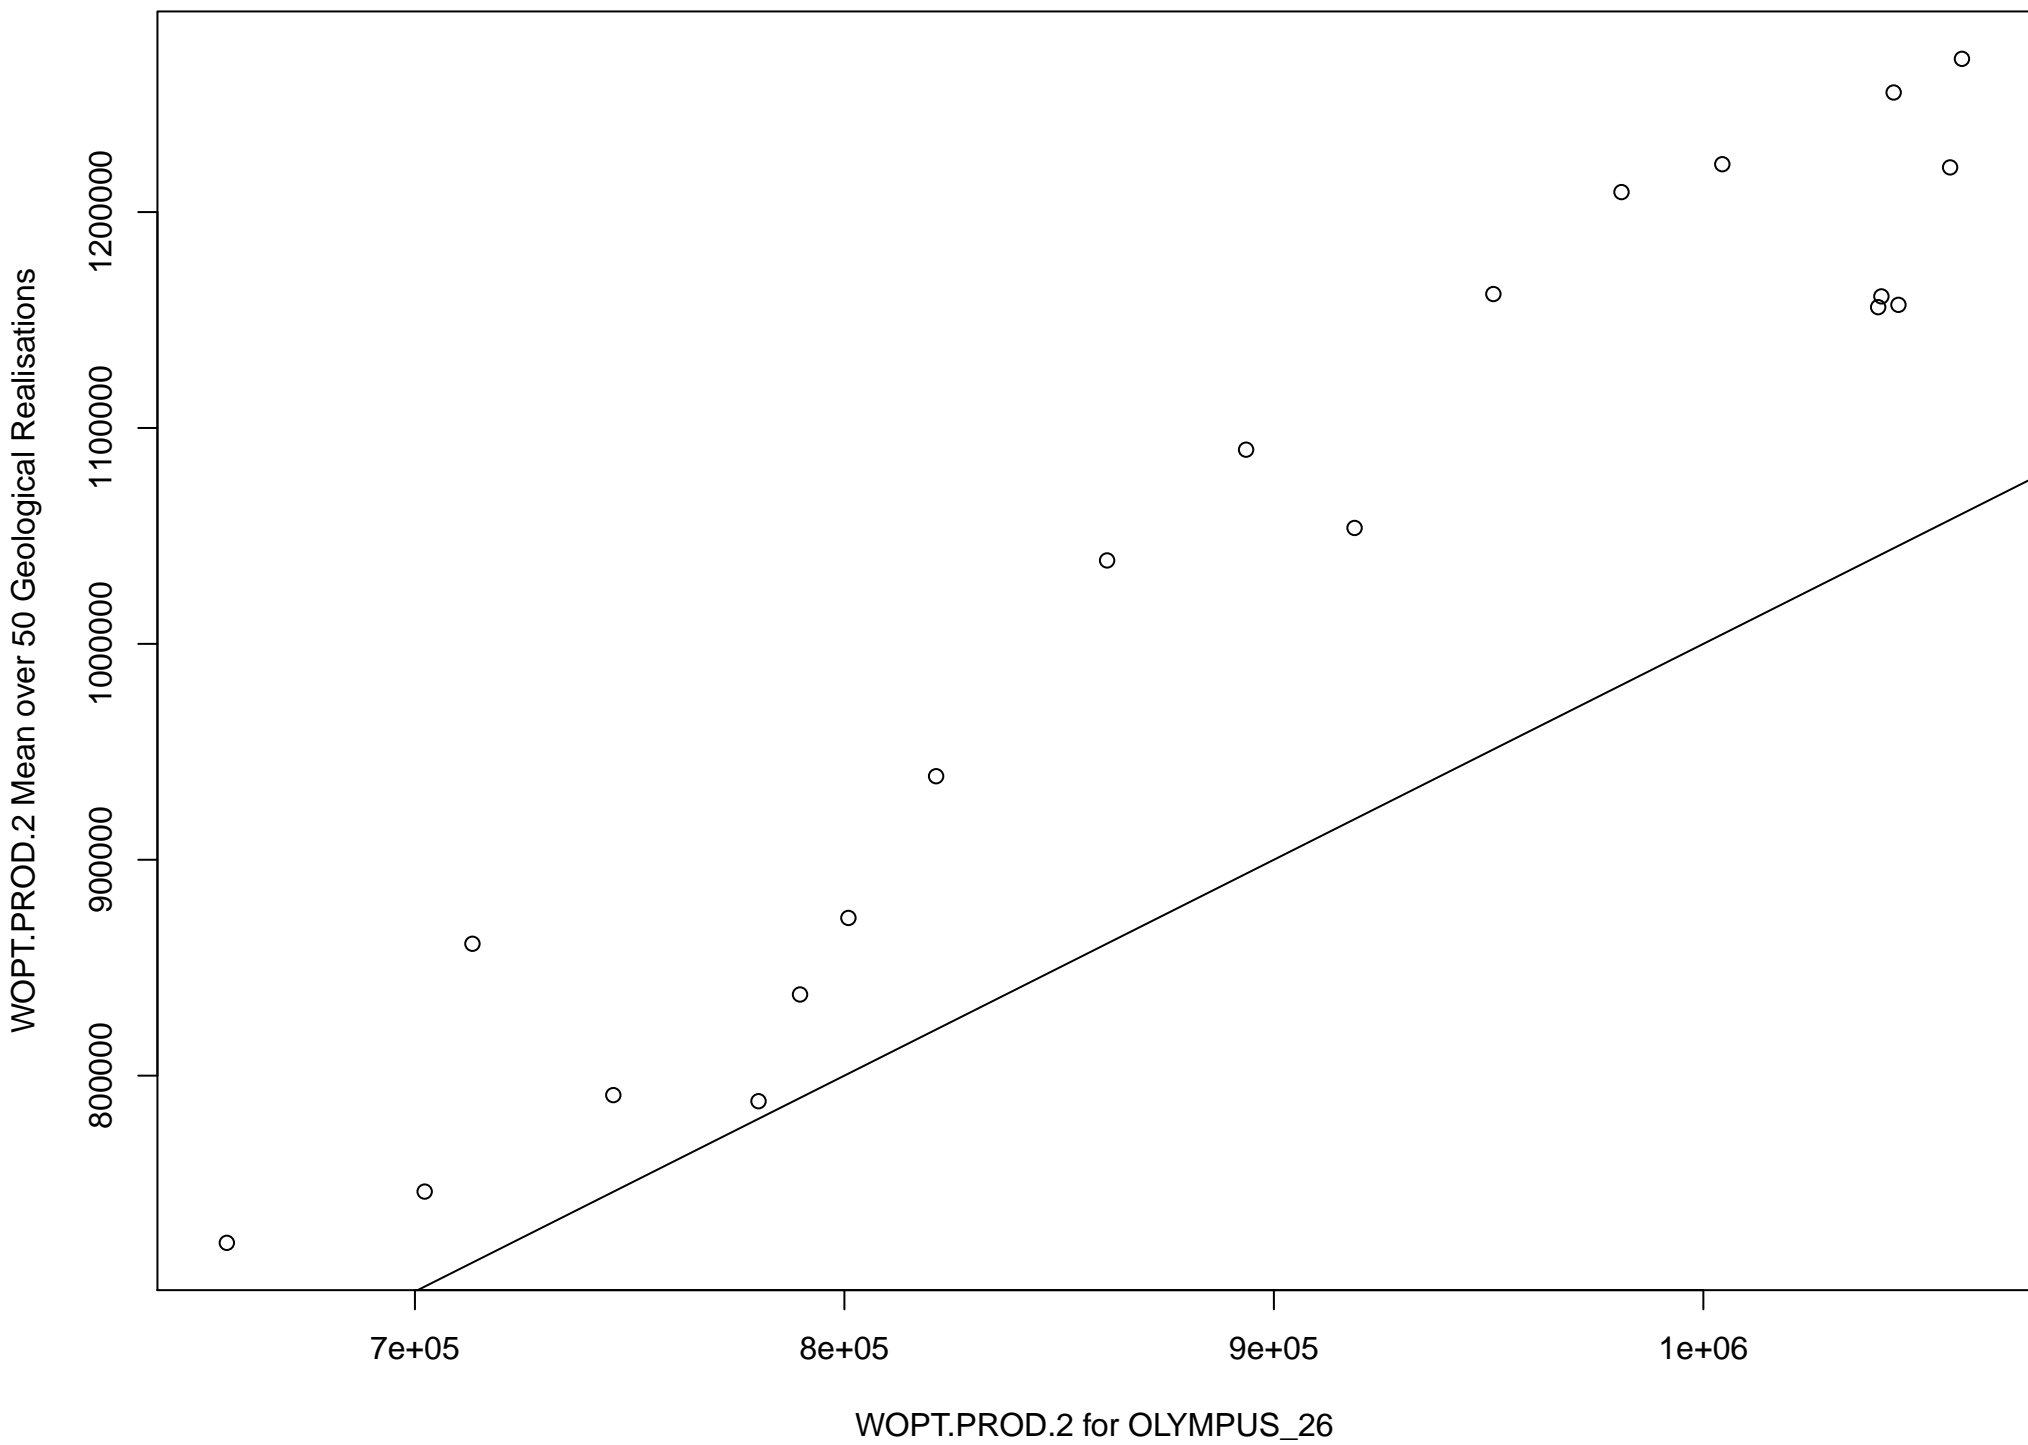

WOPT.PROD.2 for OLYMPUS\_27

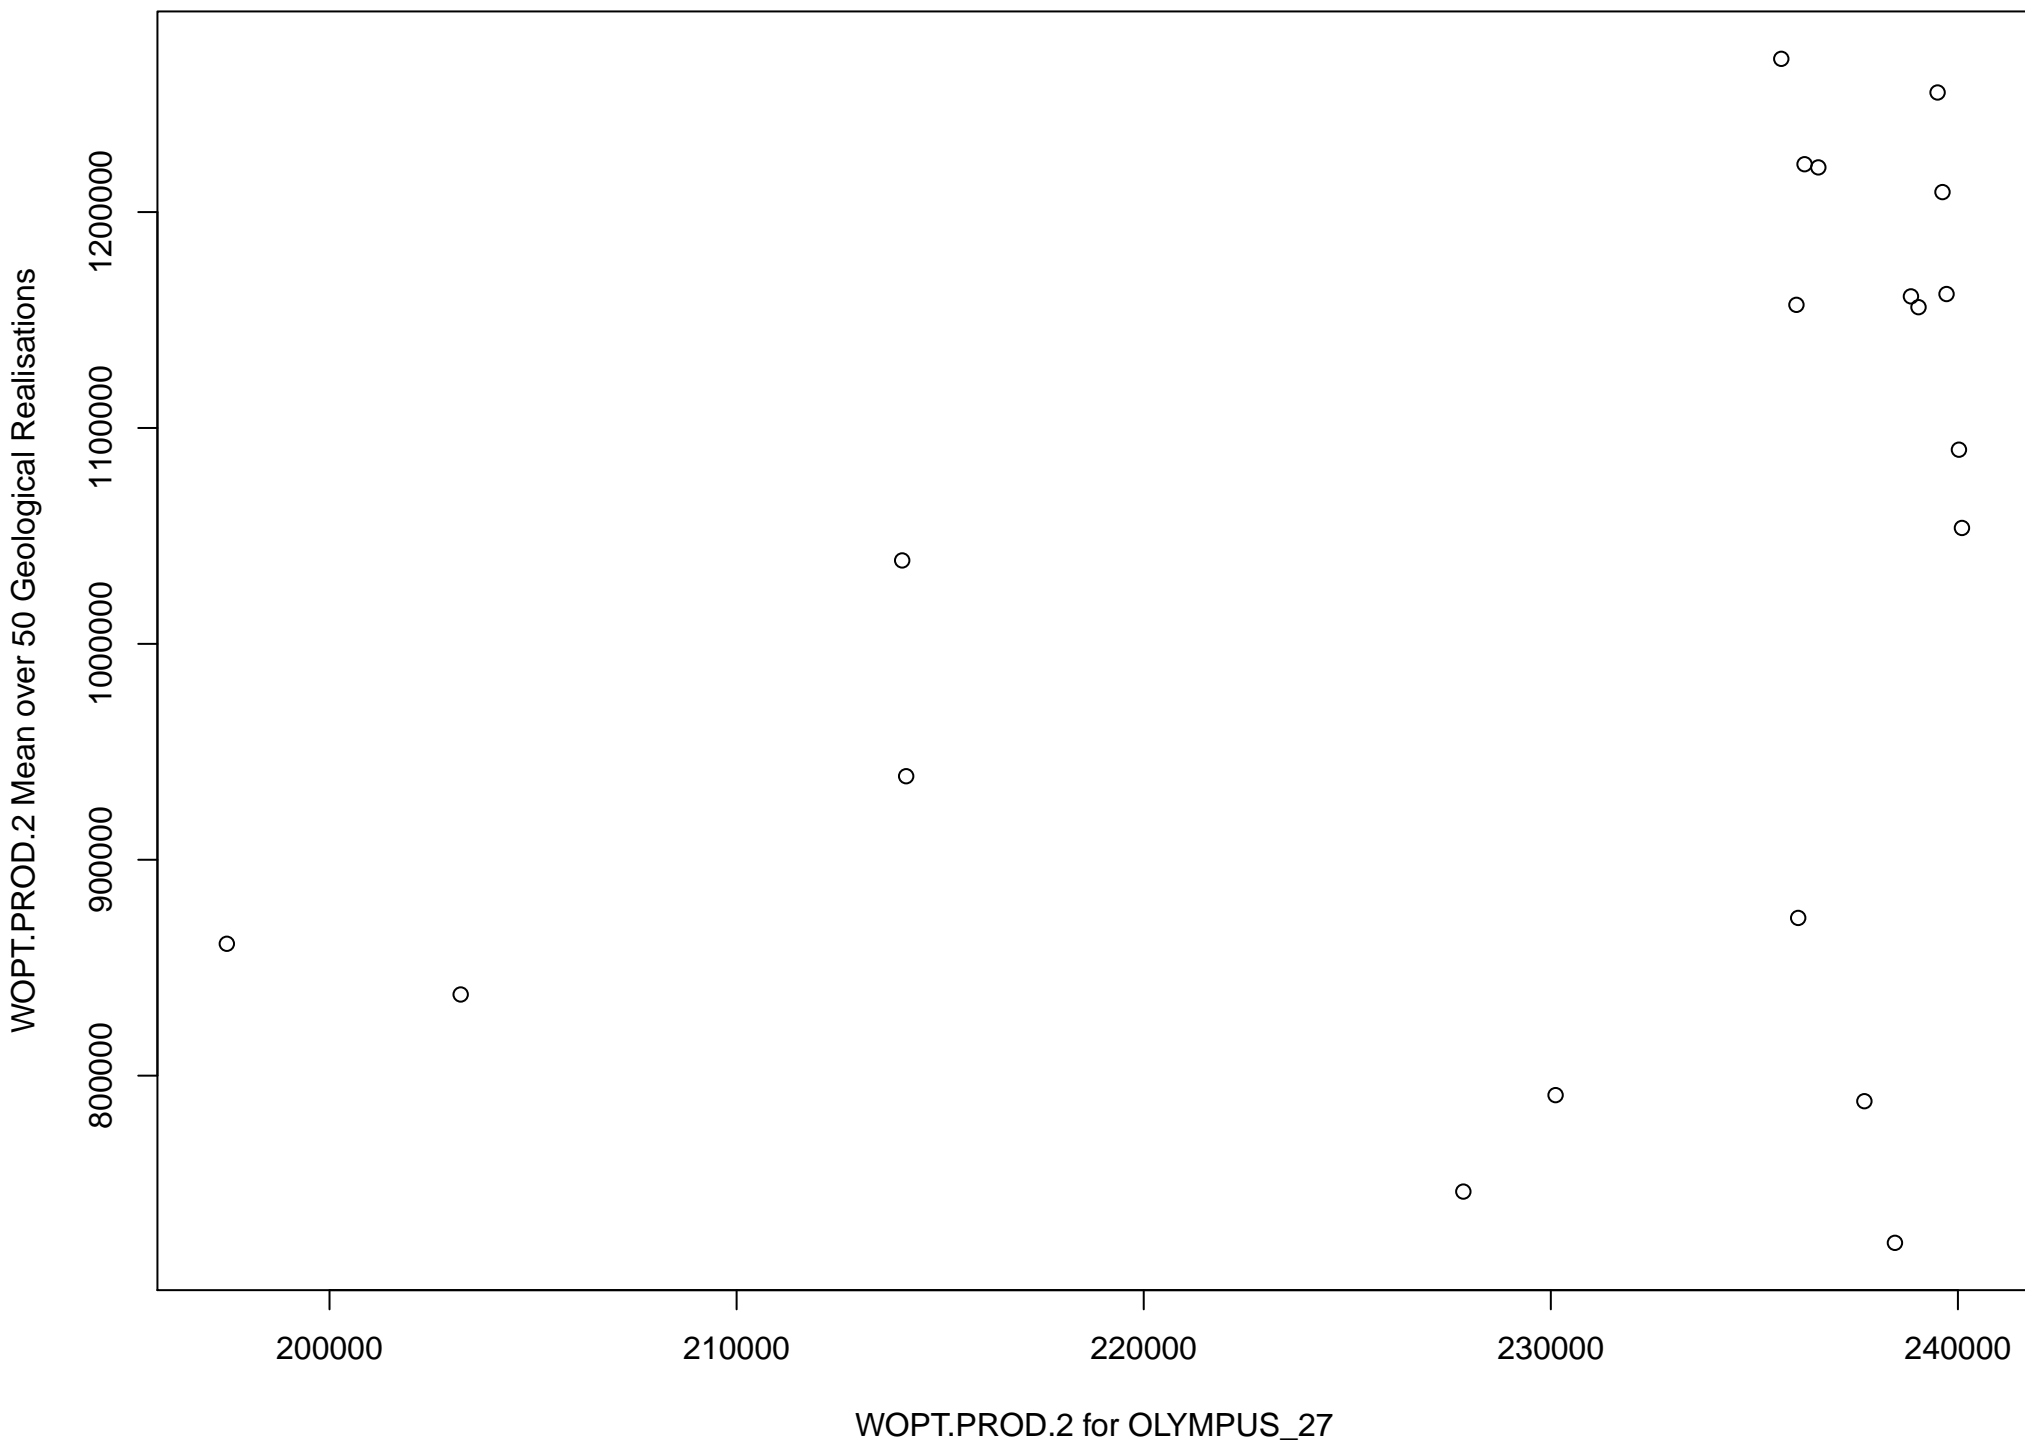

WOPT.PROD.2 for OLYMPUS\_28

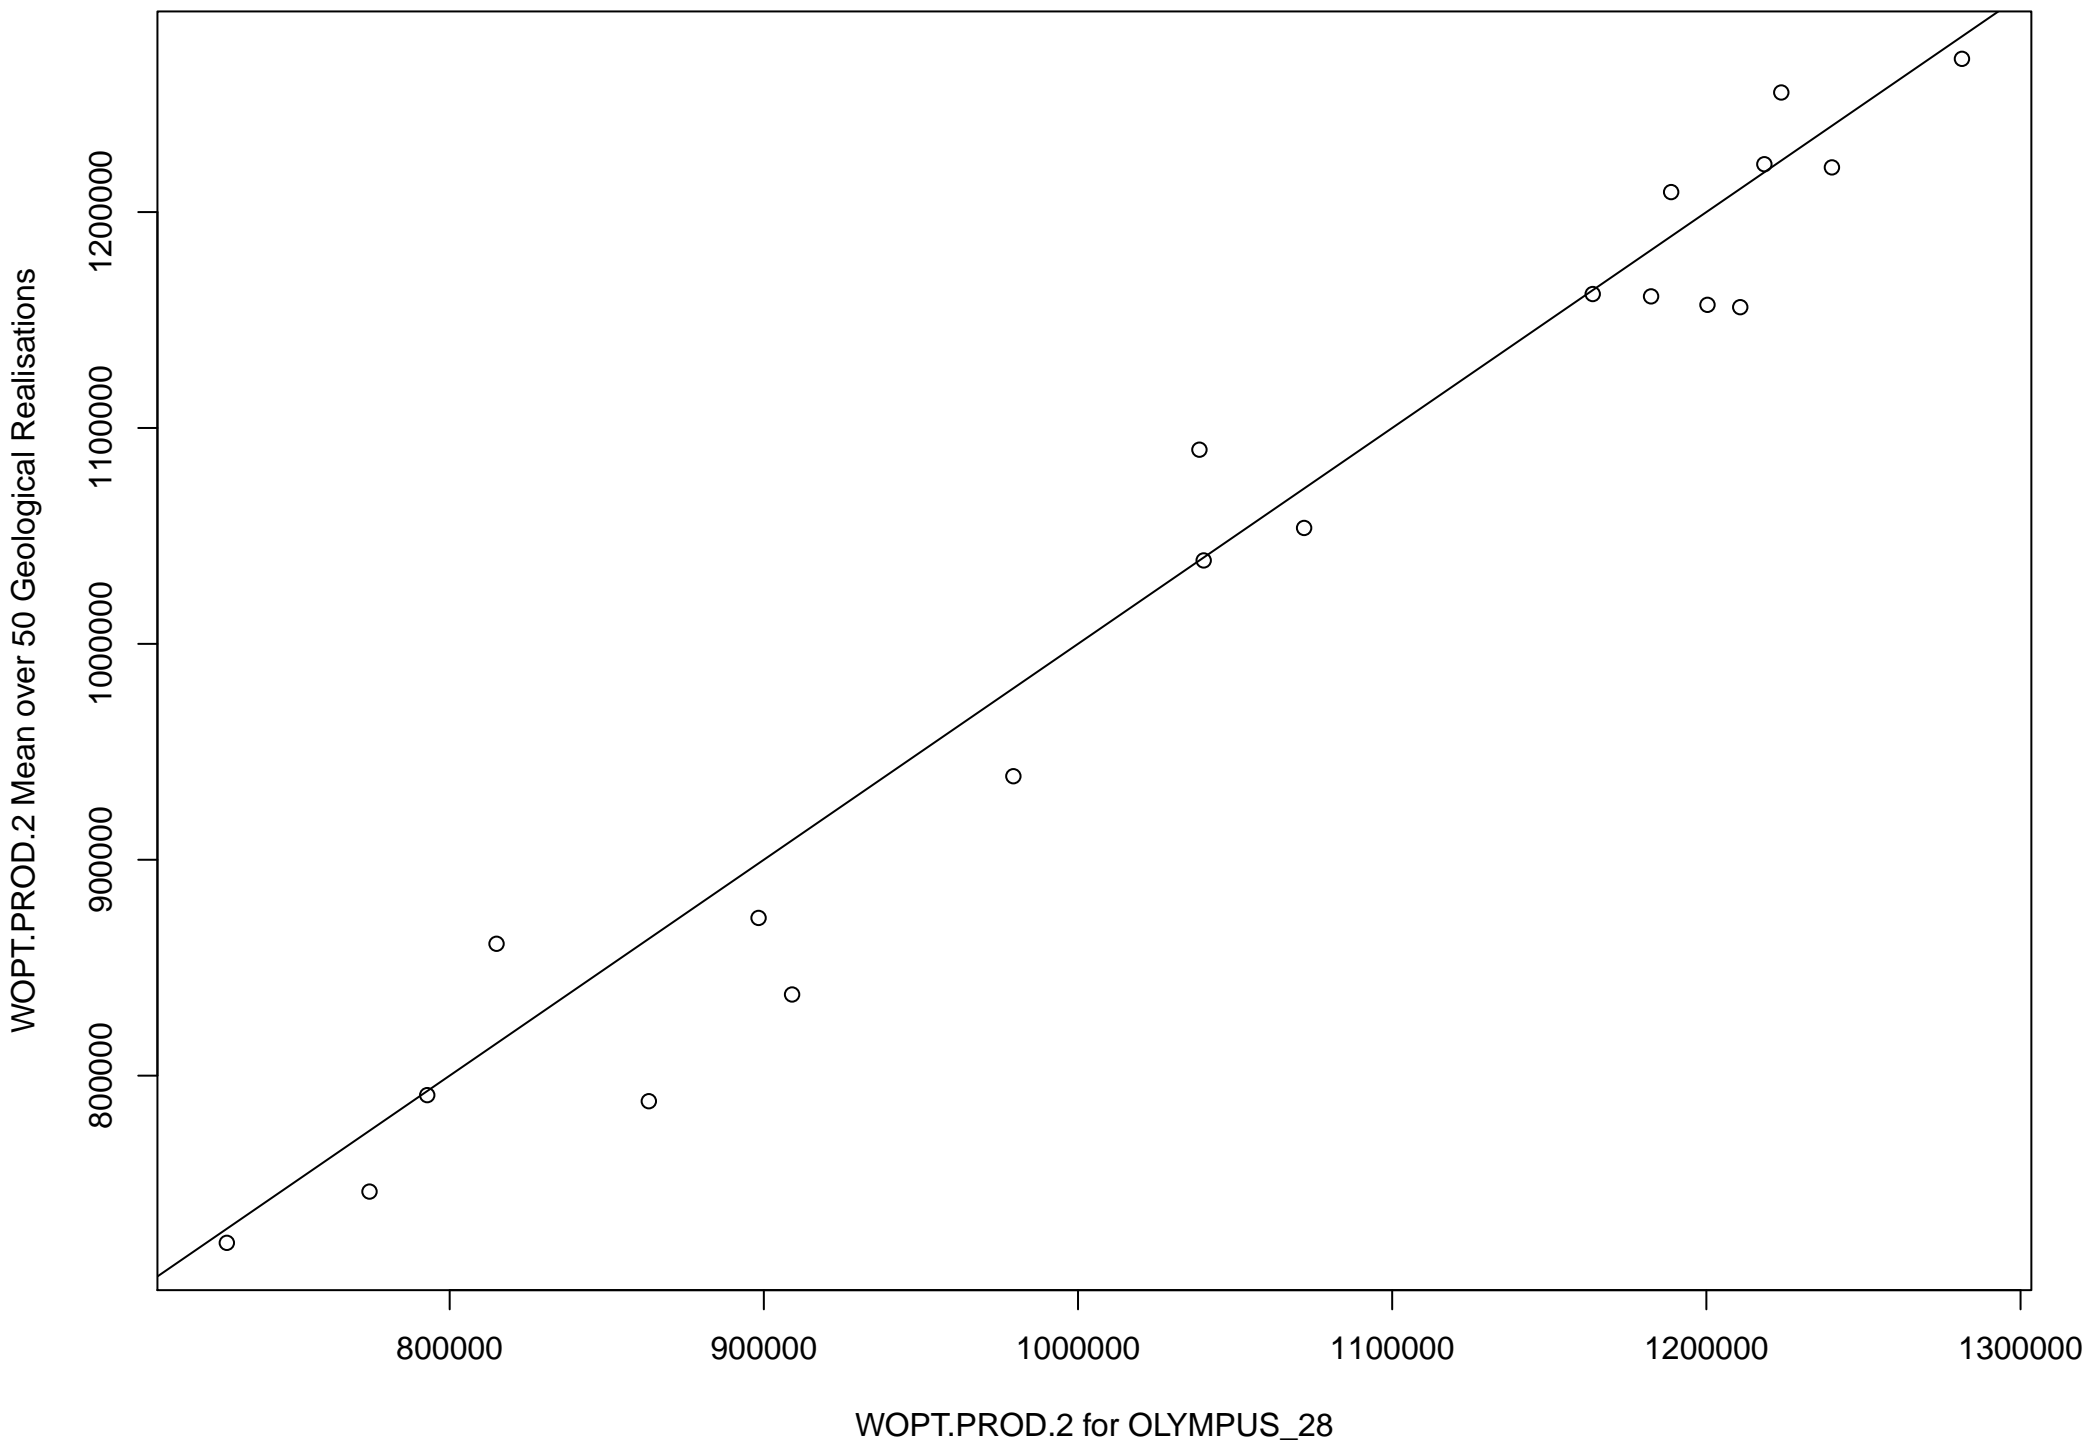

# WOPT.PROD.2 for OLYMPUS\_29

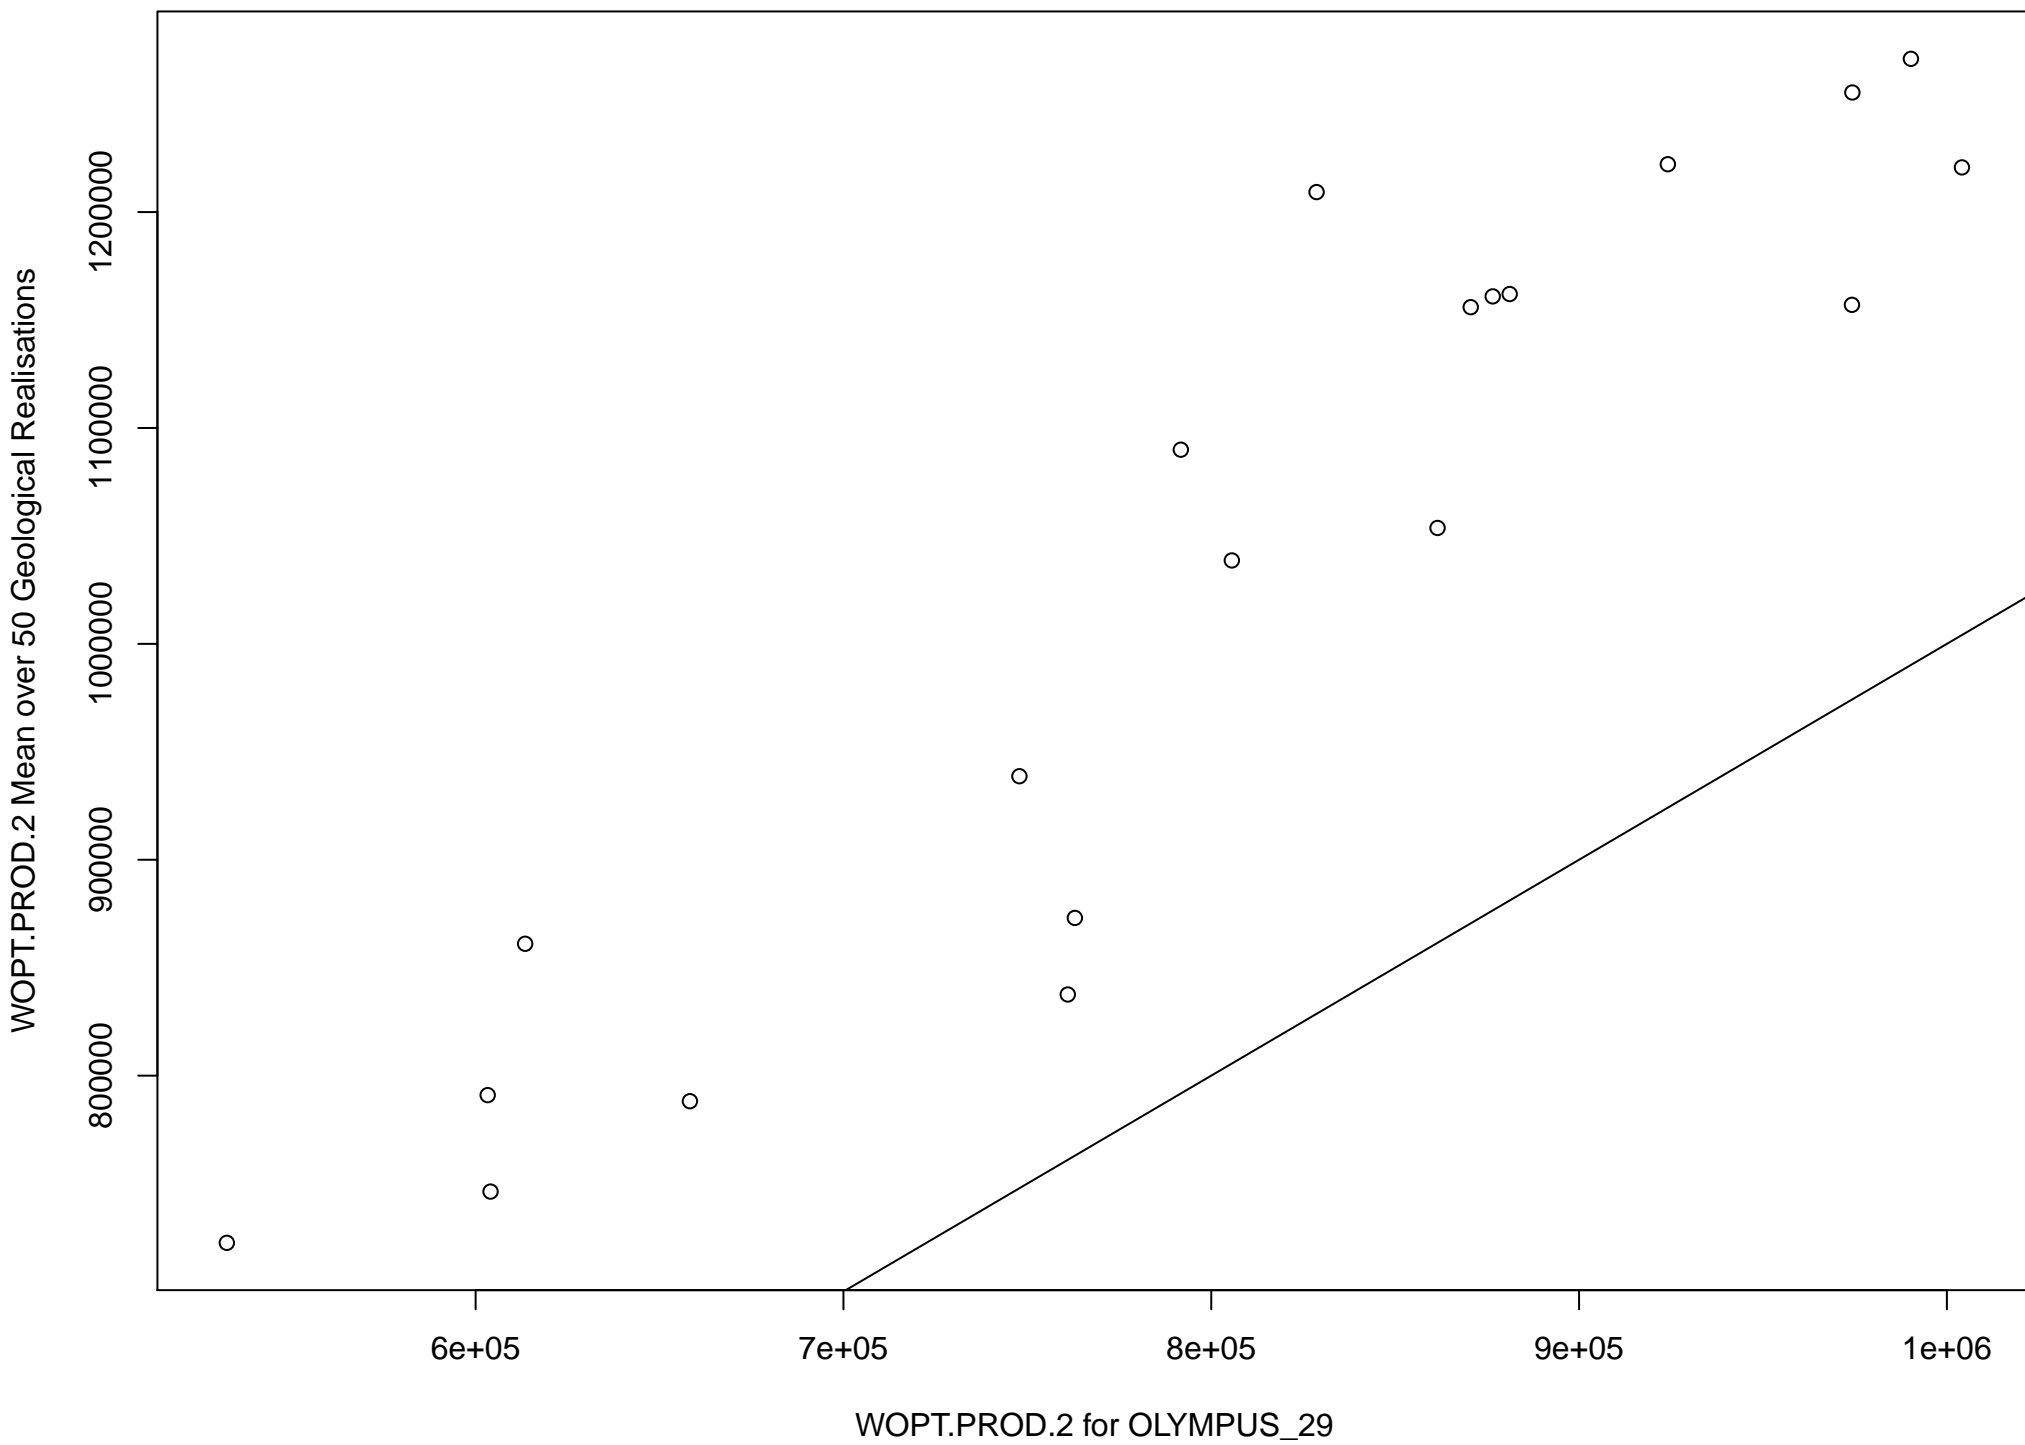

WOPT.PROD.2 for OLYMPUS\_30

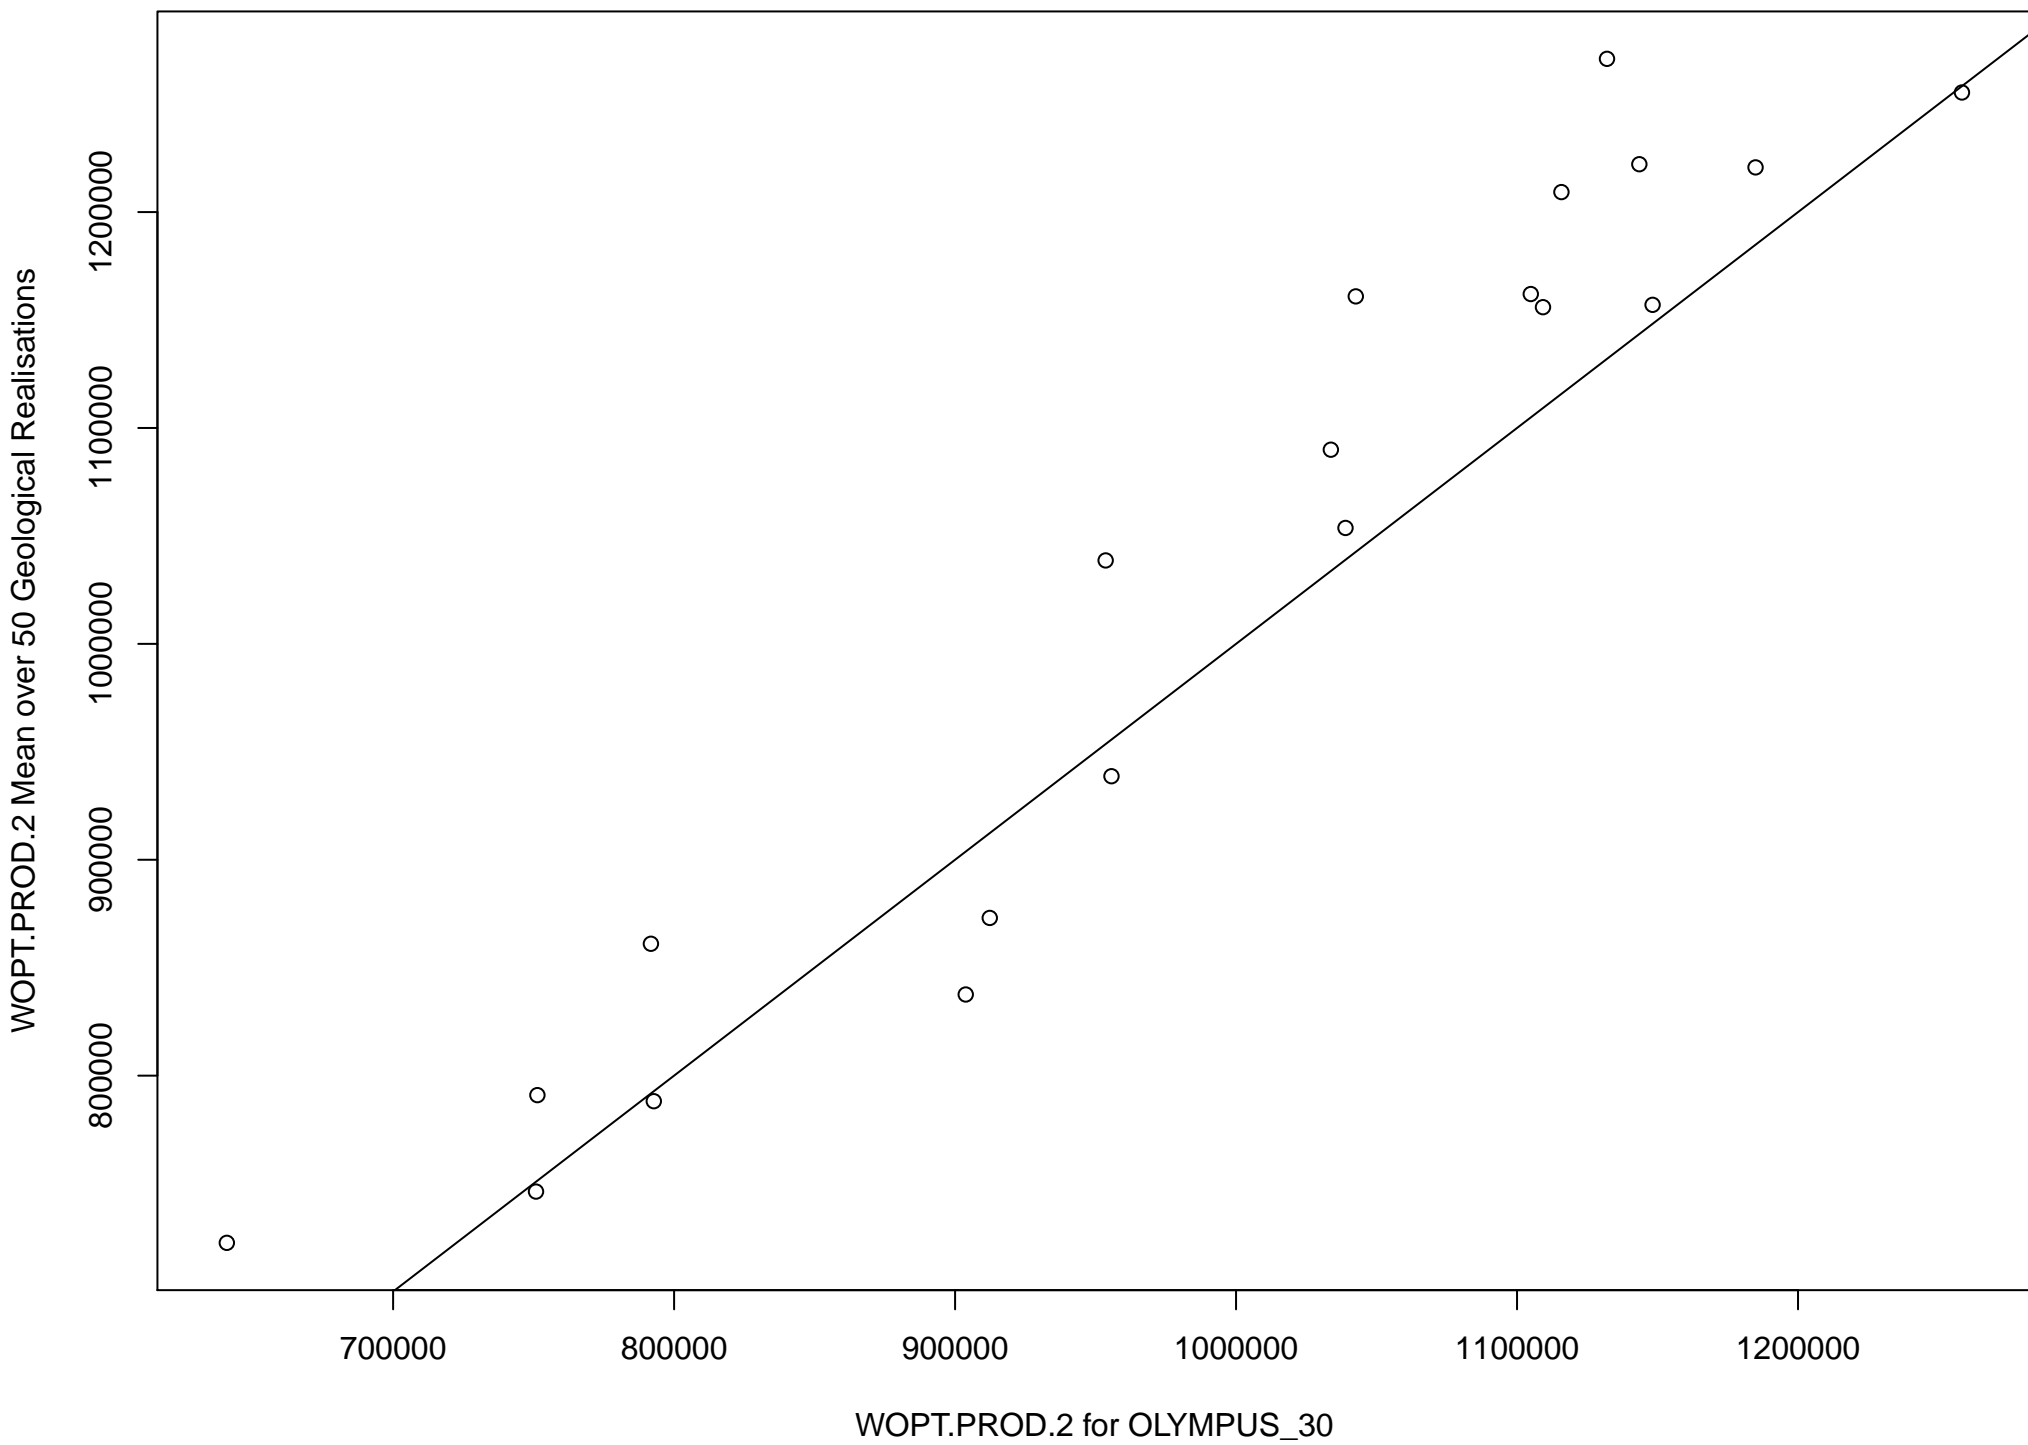

WOPT.PROD.2 for OLYMPUS\_31

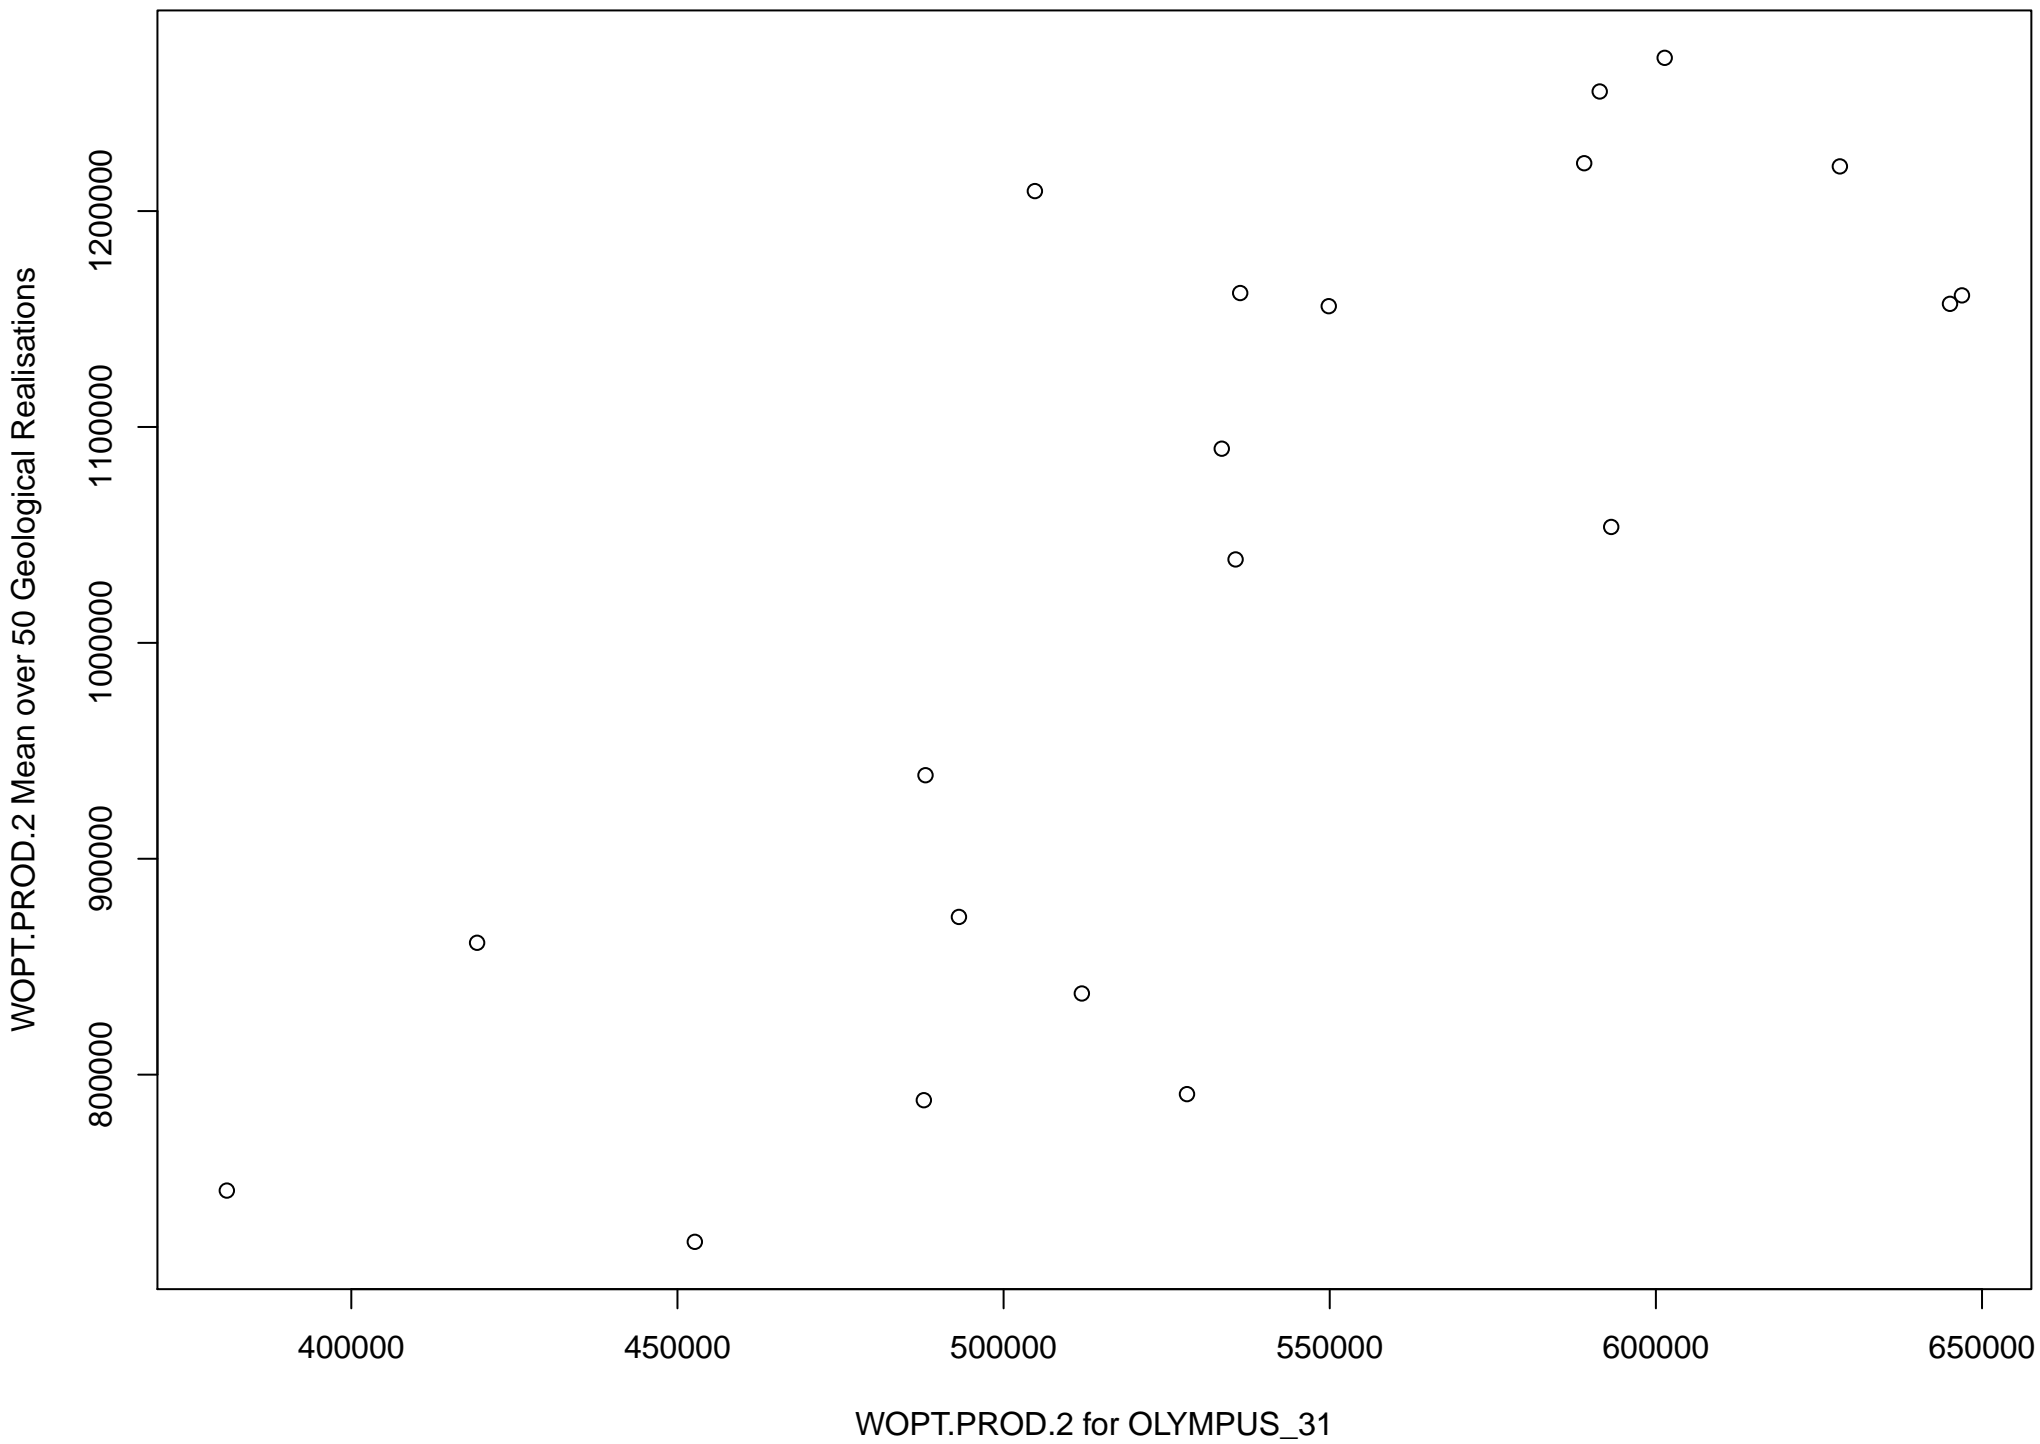

WOPT.PROD.2 for OLYMPUS\_32

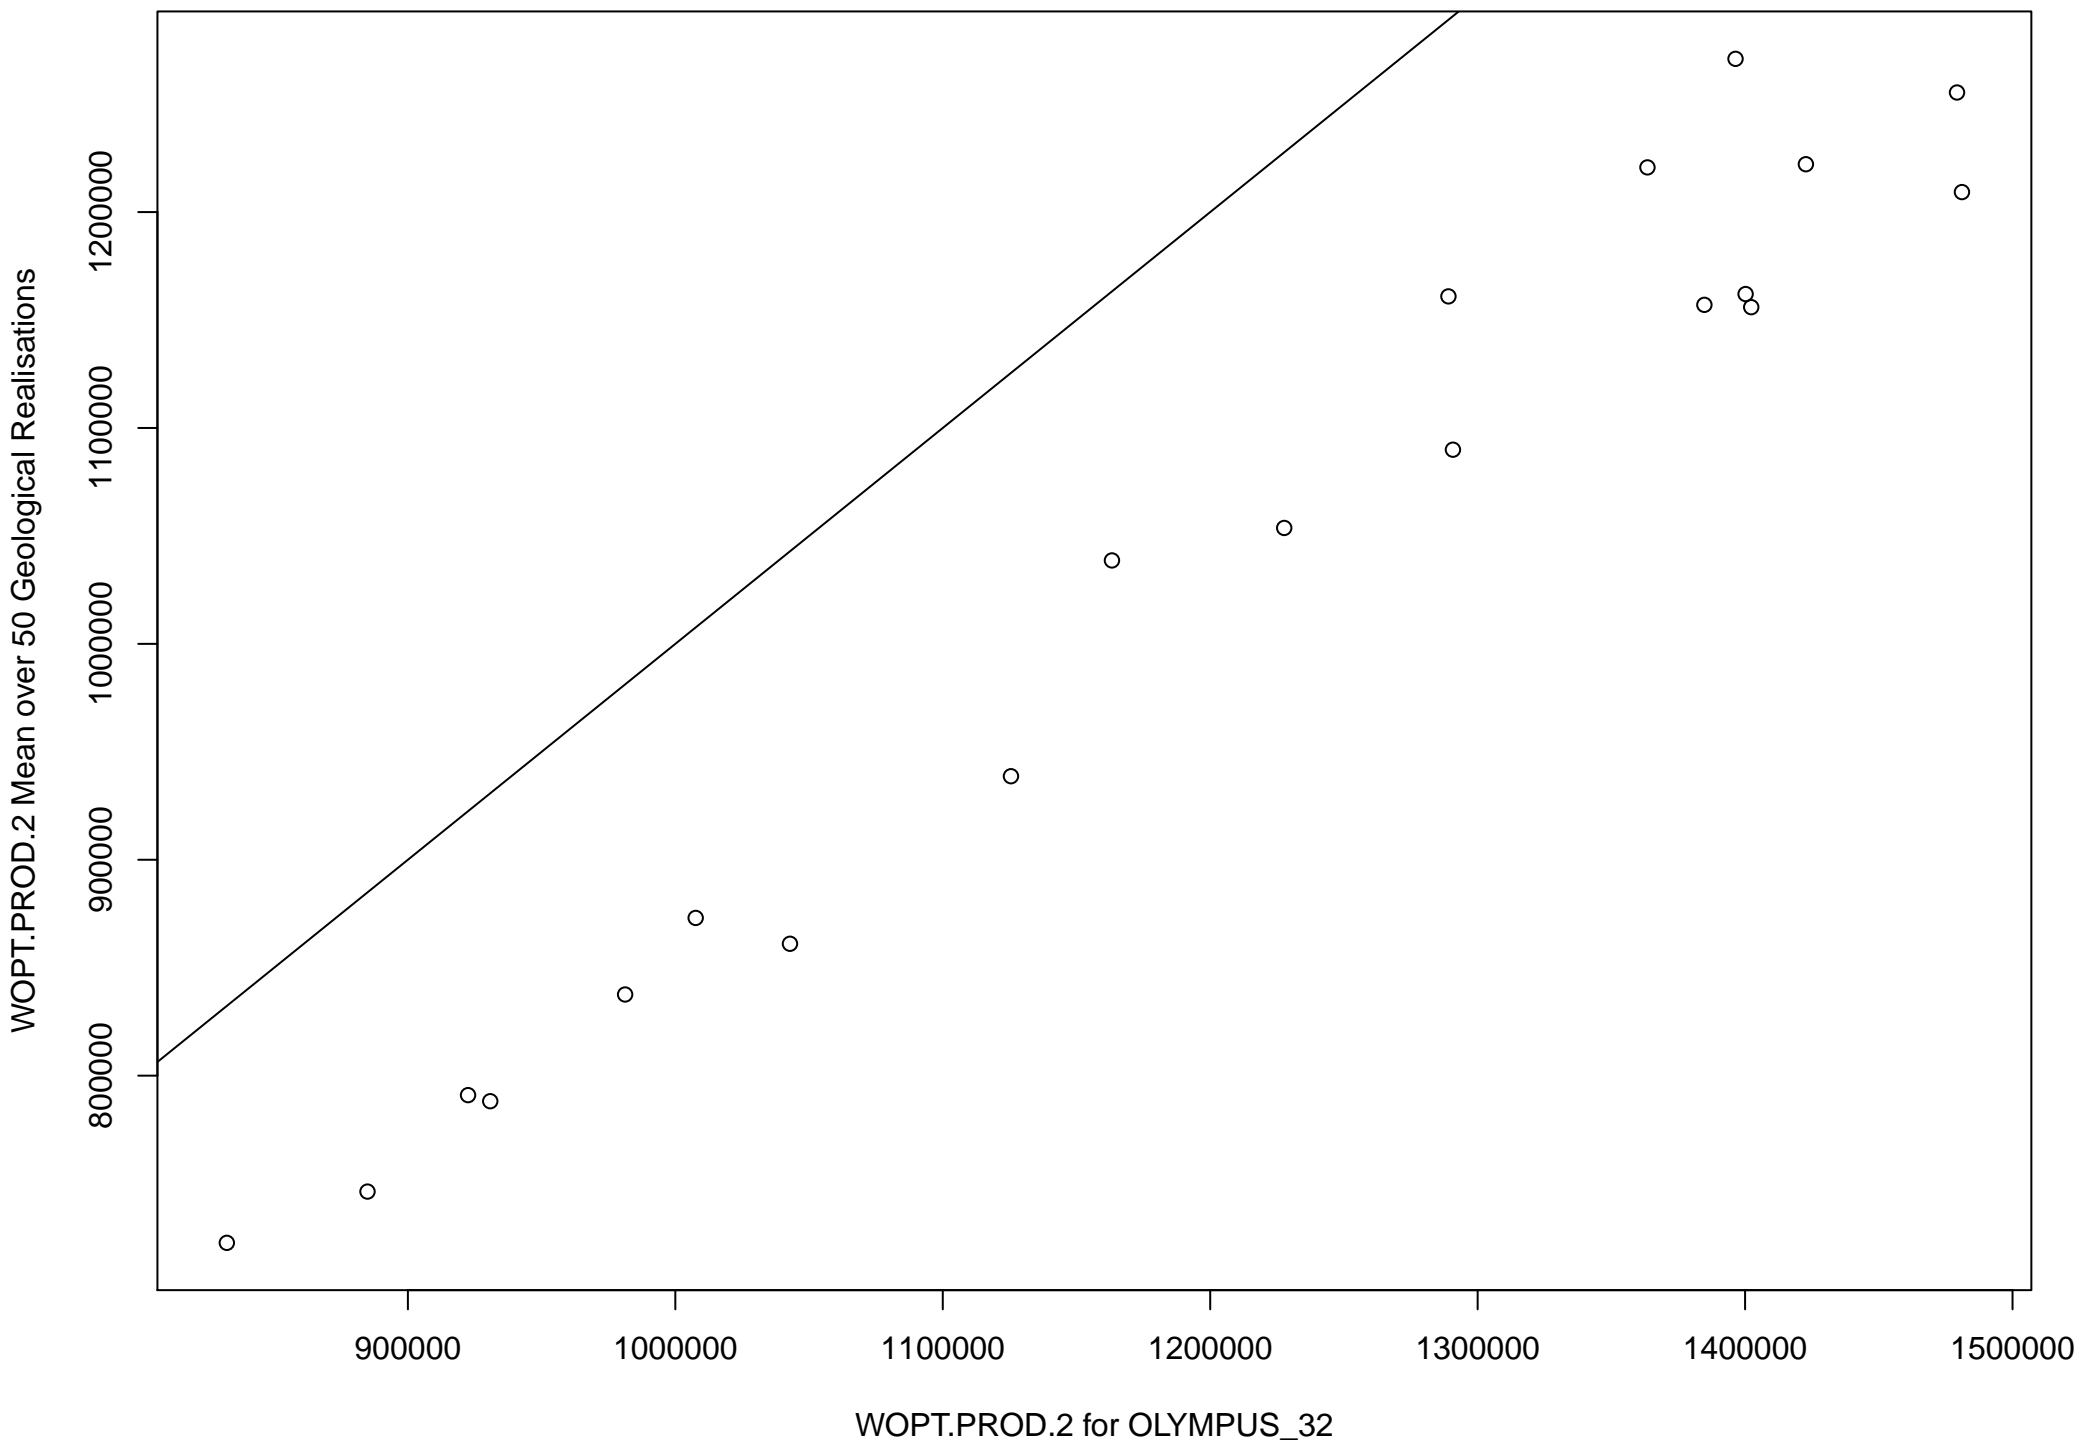



WOPT.PROD.2 for OLYMPUS\_33

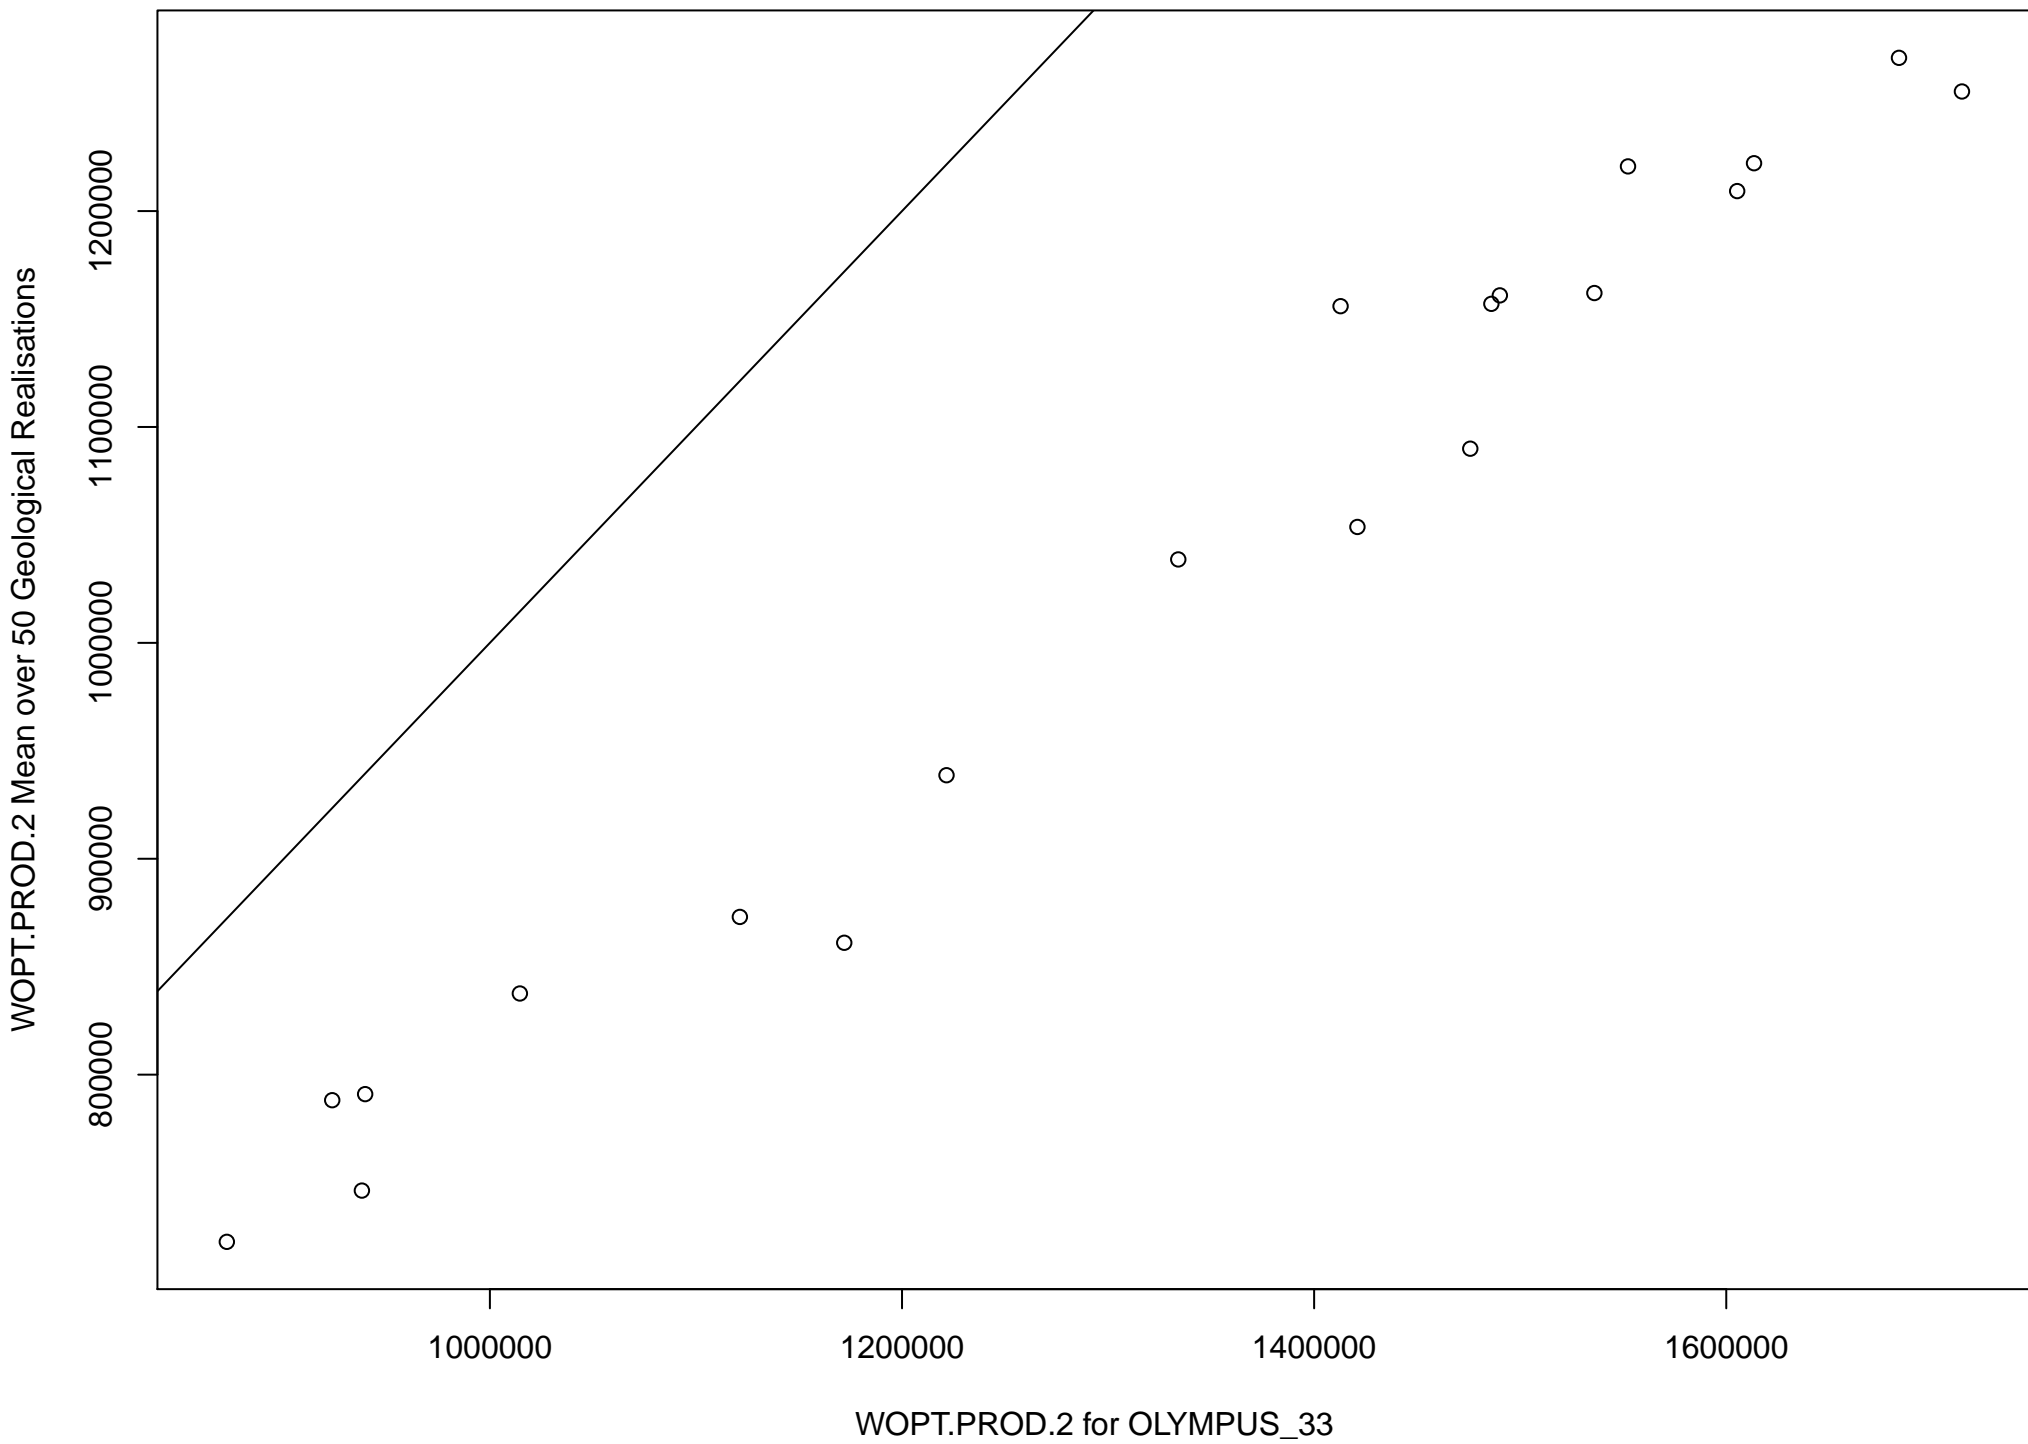

WOPT.PROD.2 for OLYMPUS\_34

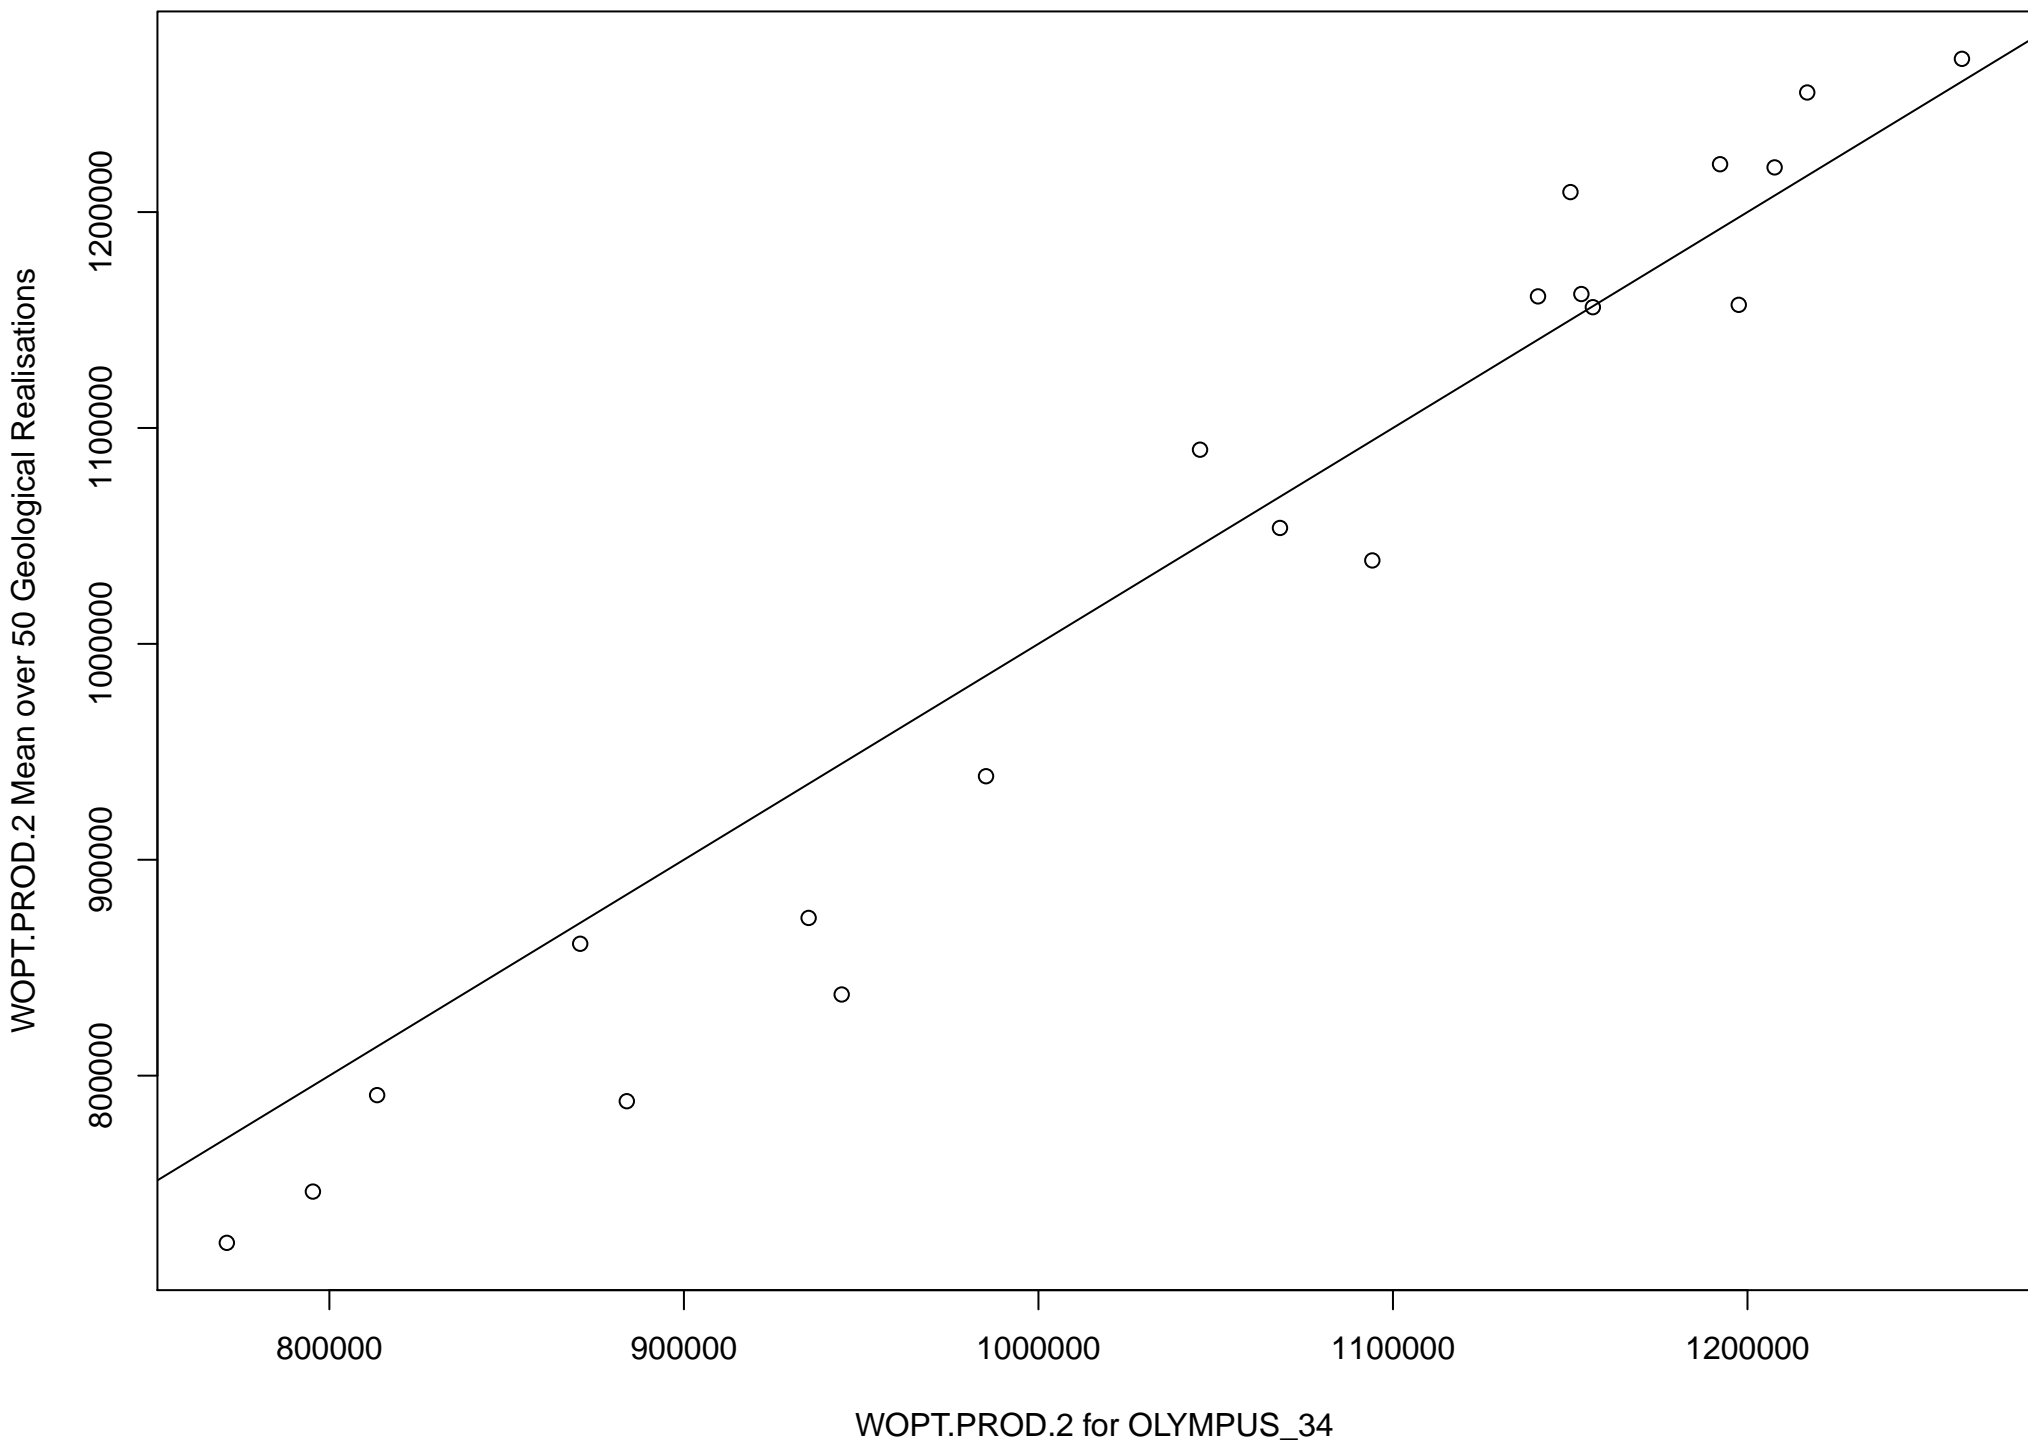

WOPT.PROD.2 for OLYMPUS\_35

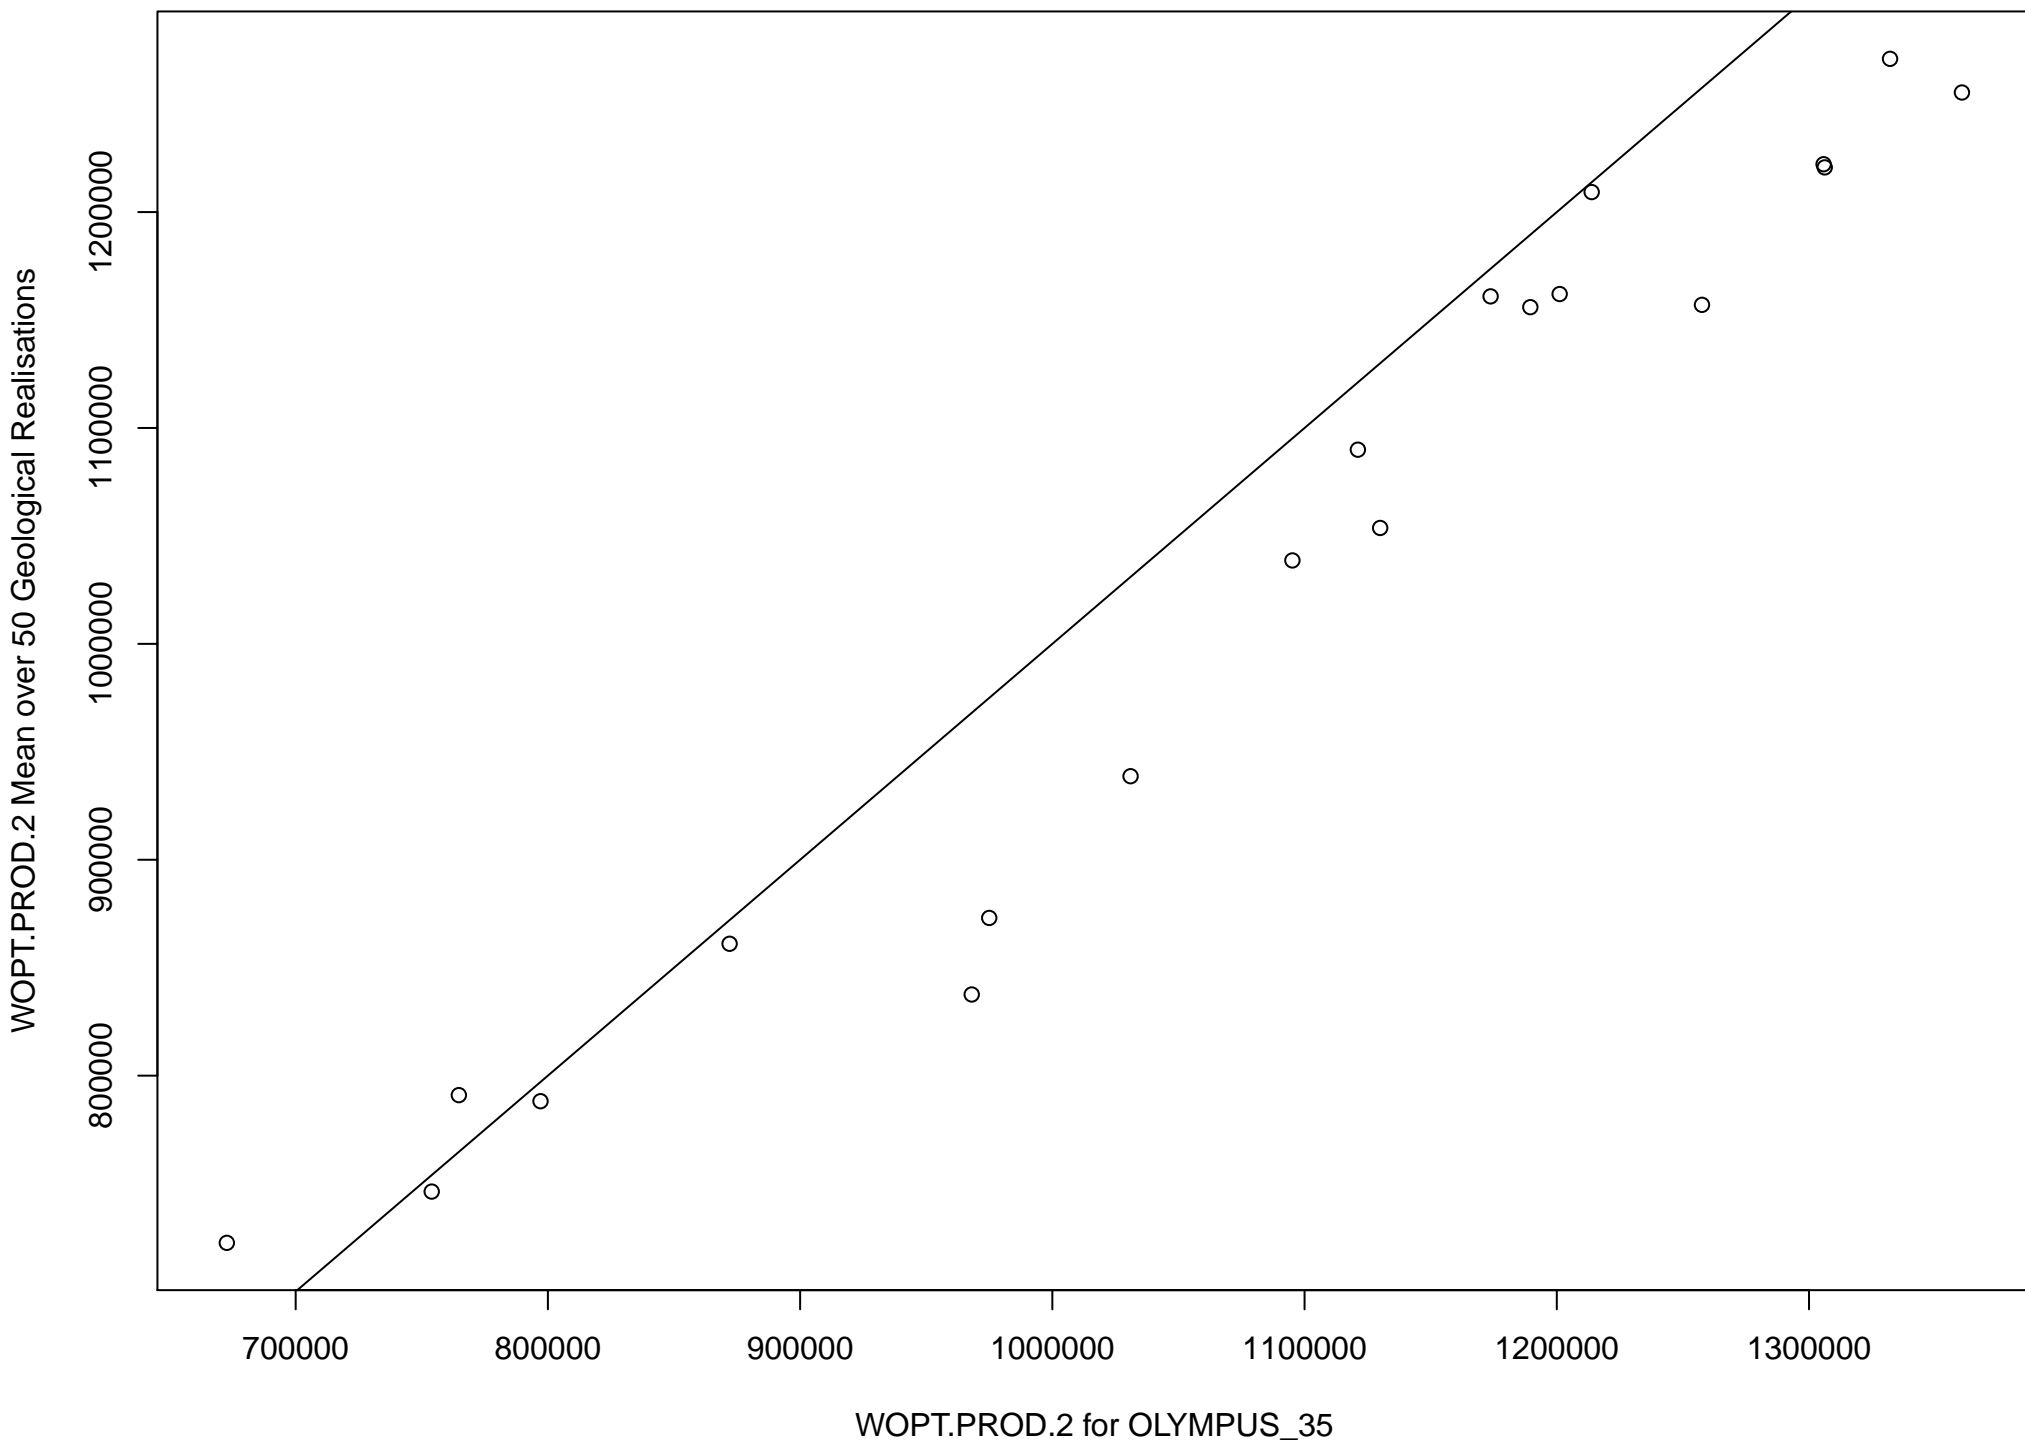

WOPT.PROD.2 for OLYMPUS\_36

WOPT.PROD.2 Mean over 50 Geological Realisations

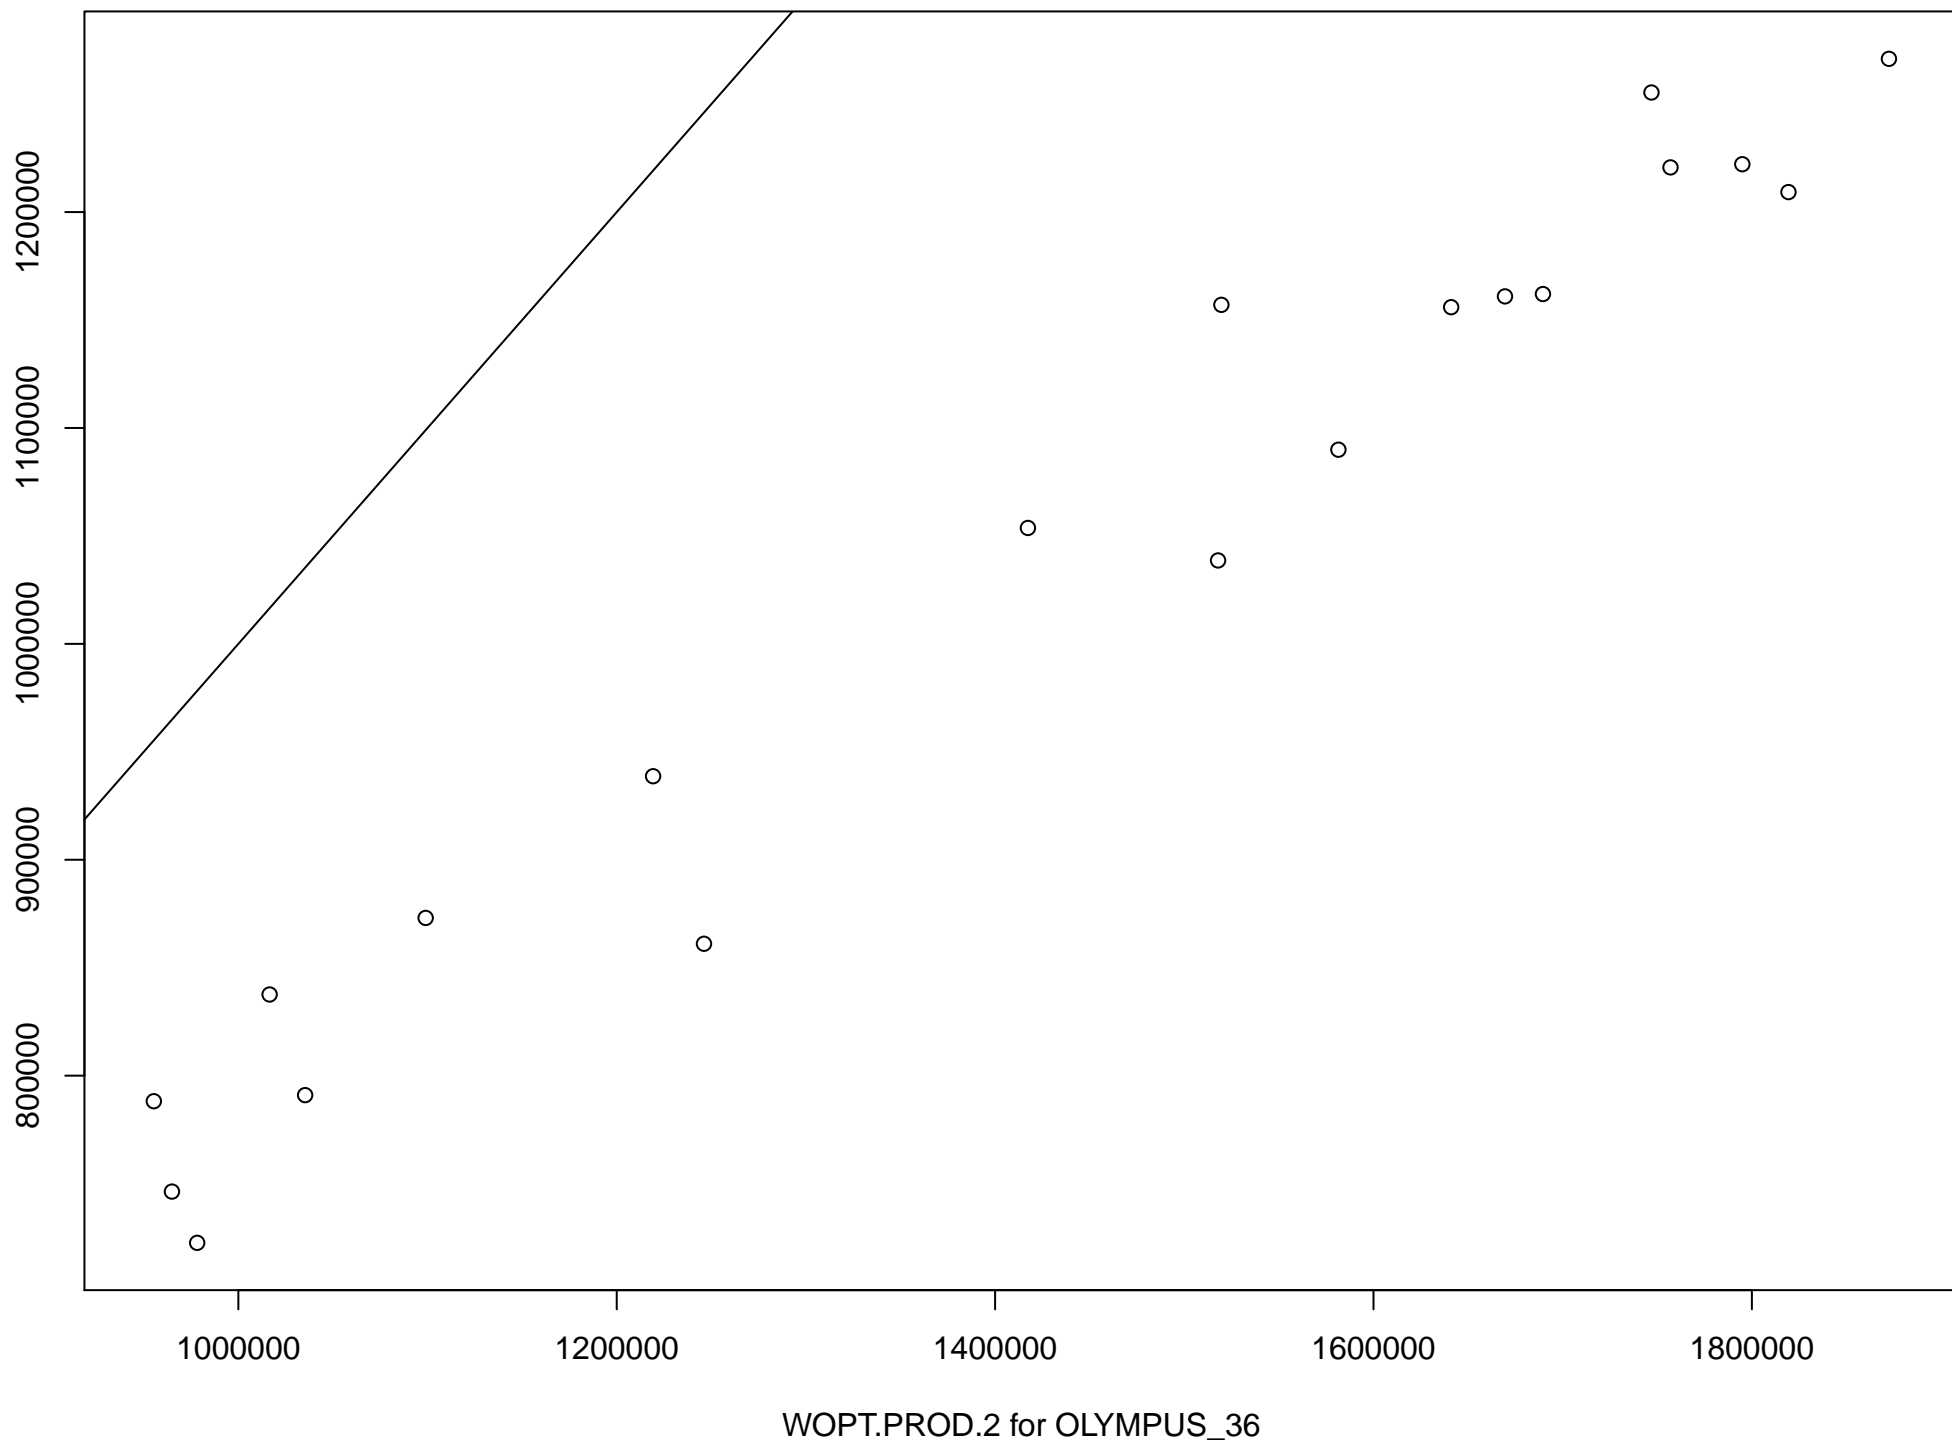

WOPT.PROD.2 for OLYMPUS\_37

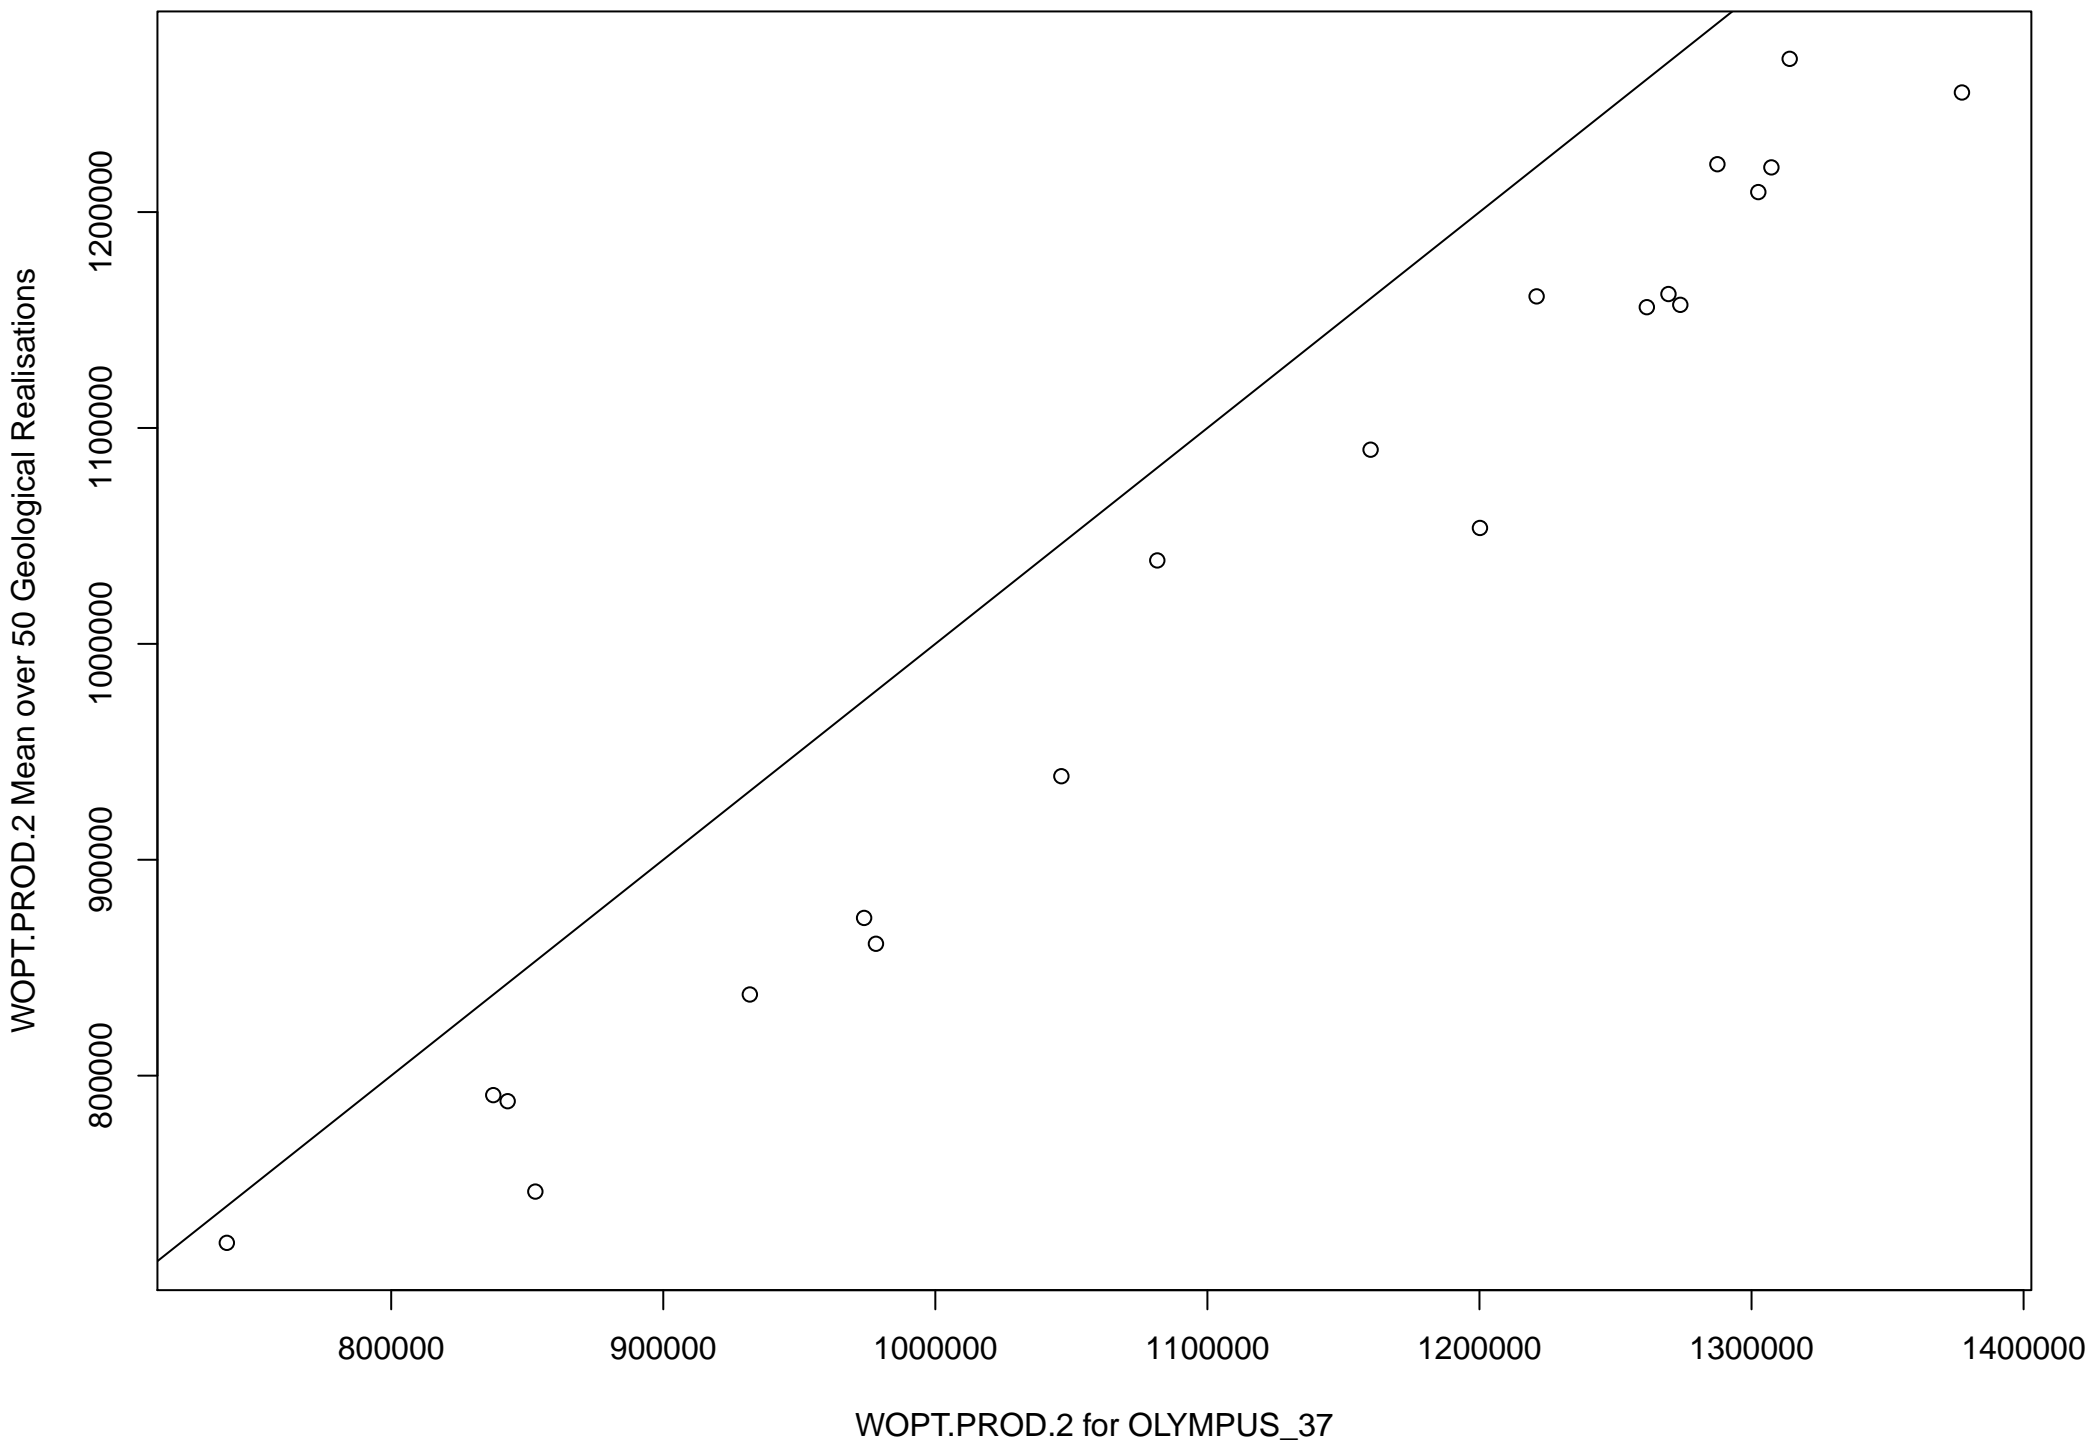

WOPT.PROD.2 for OLYMPUS\_38

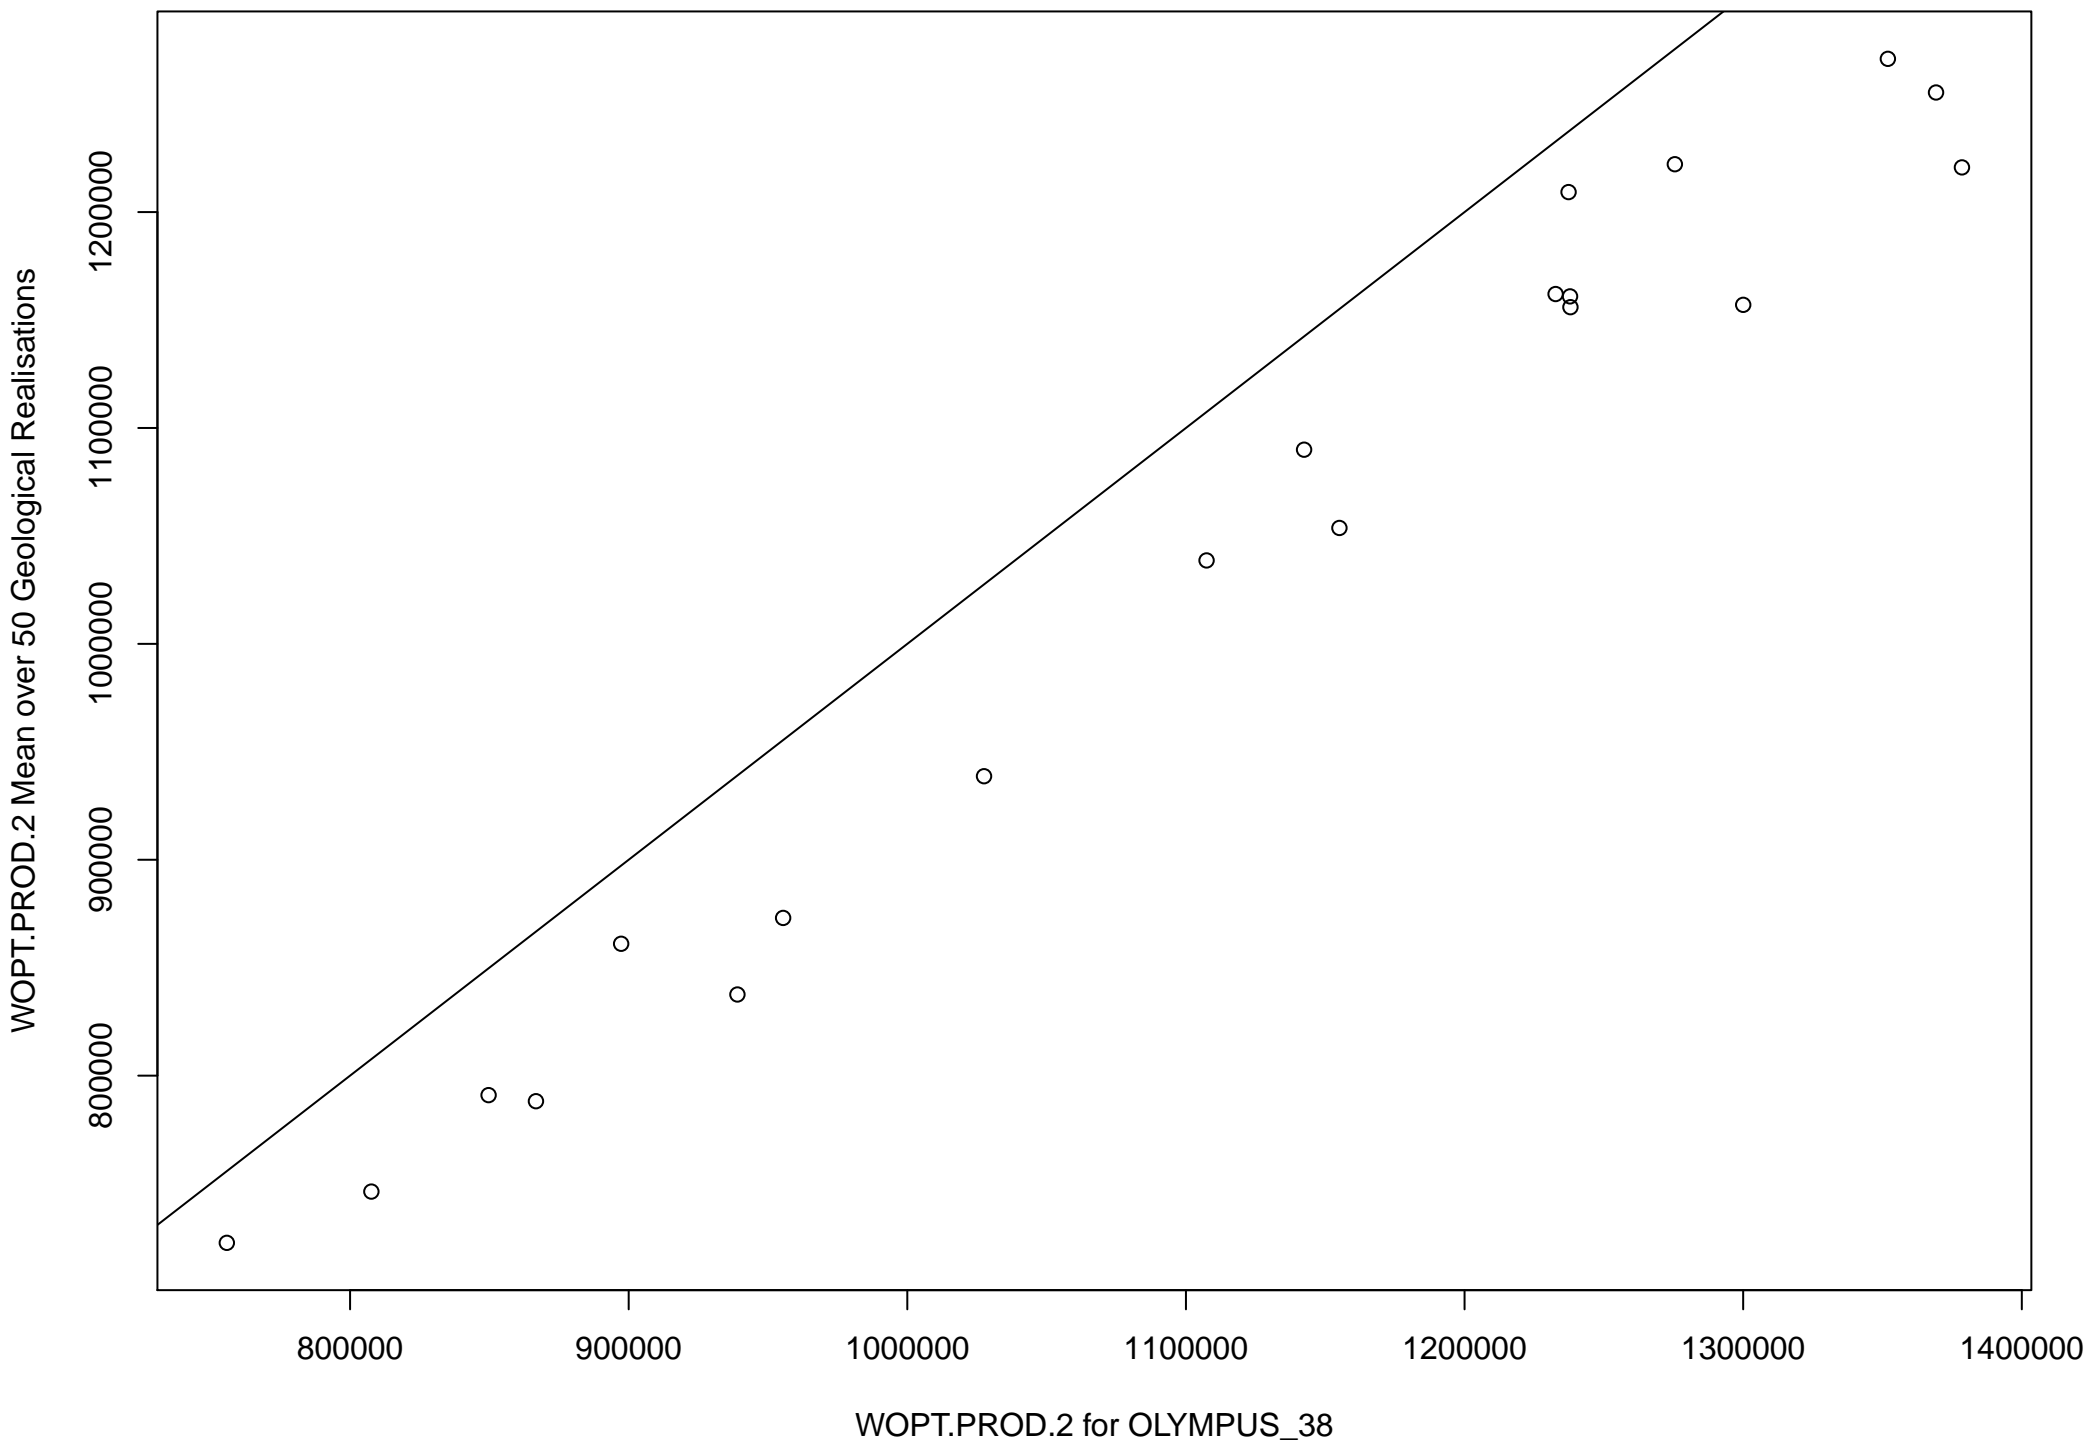

WOPT.PROD.2 for OLYMPUS\_39

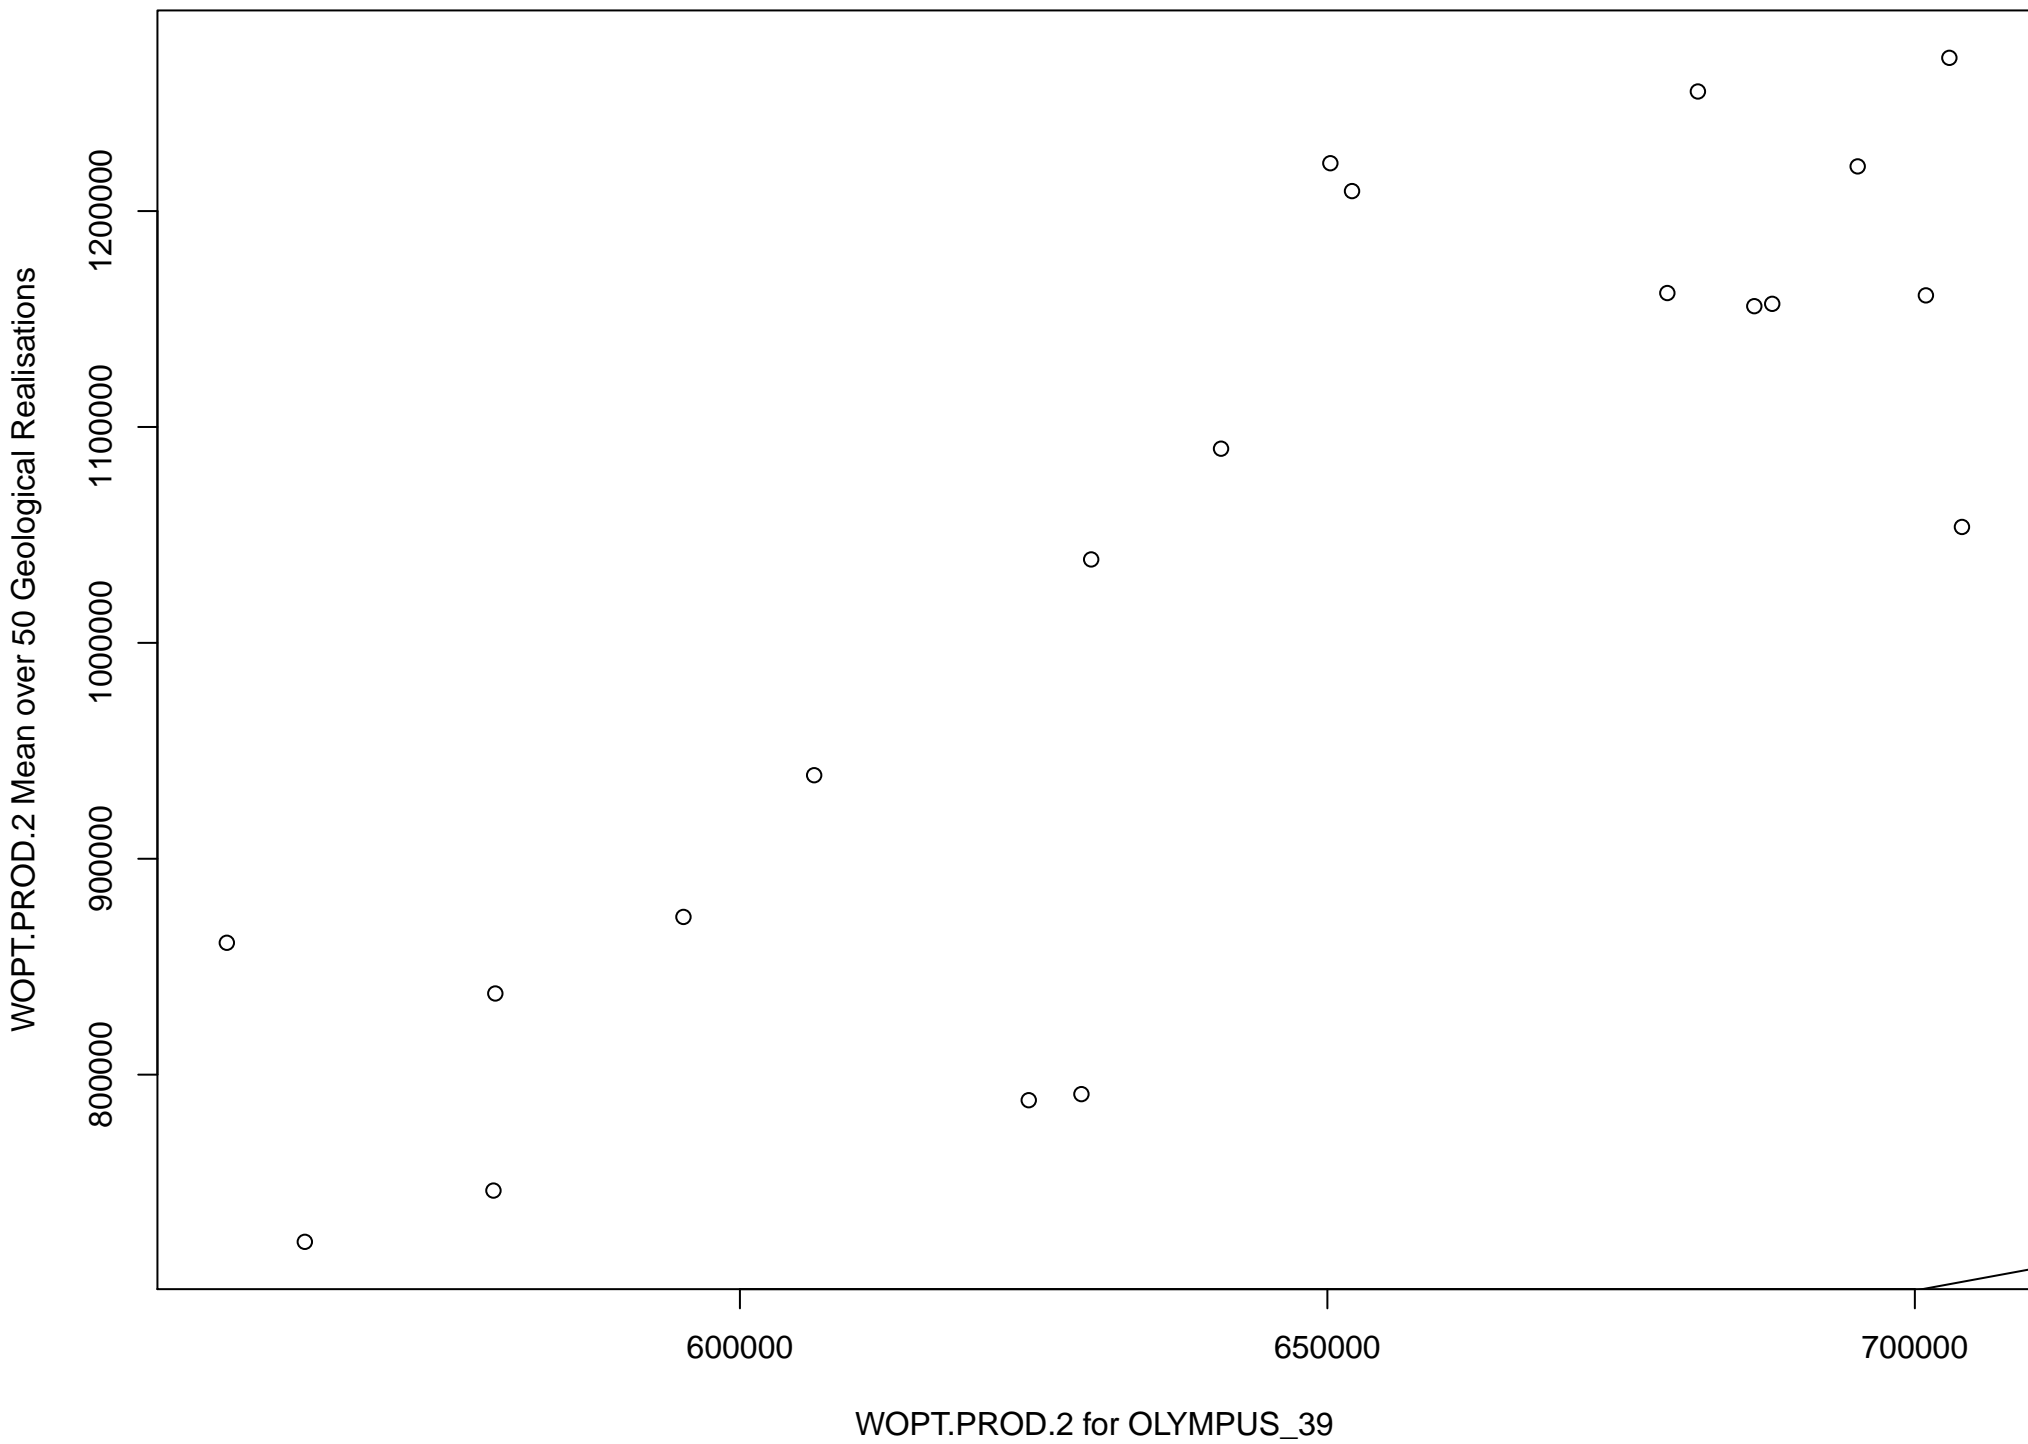

WOPT.PROD.2 for OLYMPUS\_40

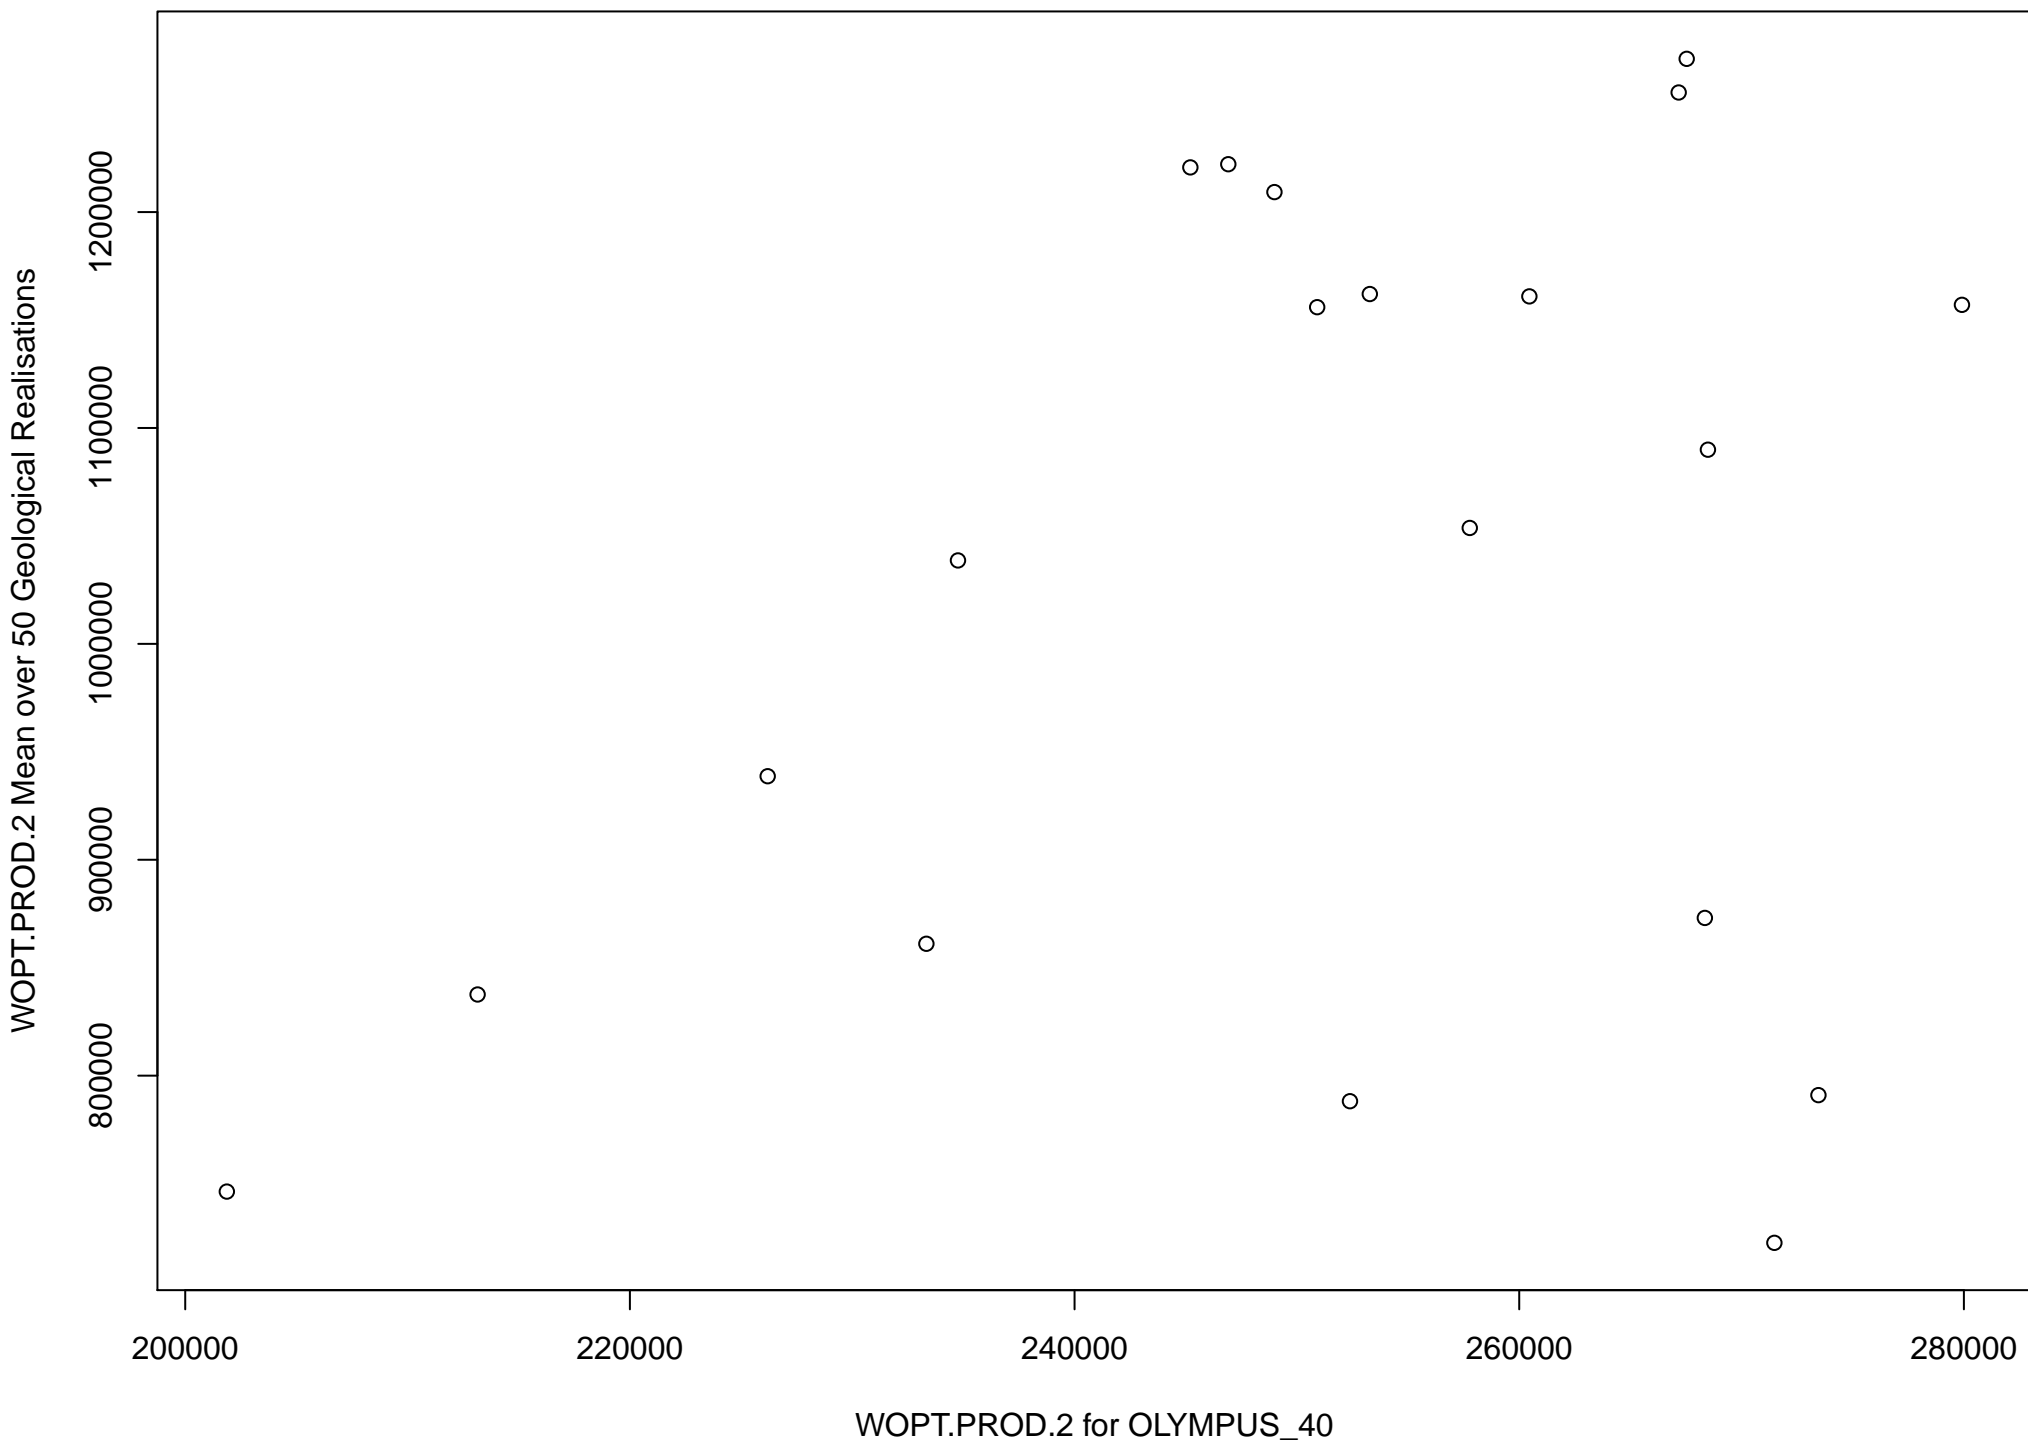



WOPT.PROD.2 for OLYMPUS\_41

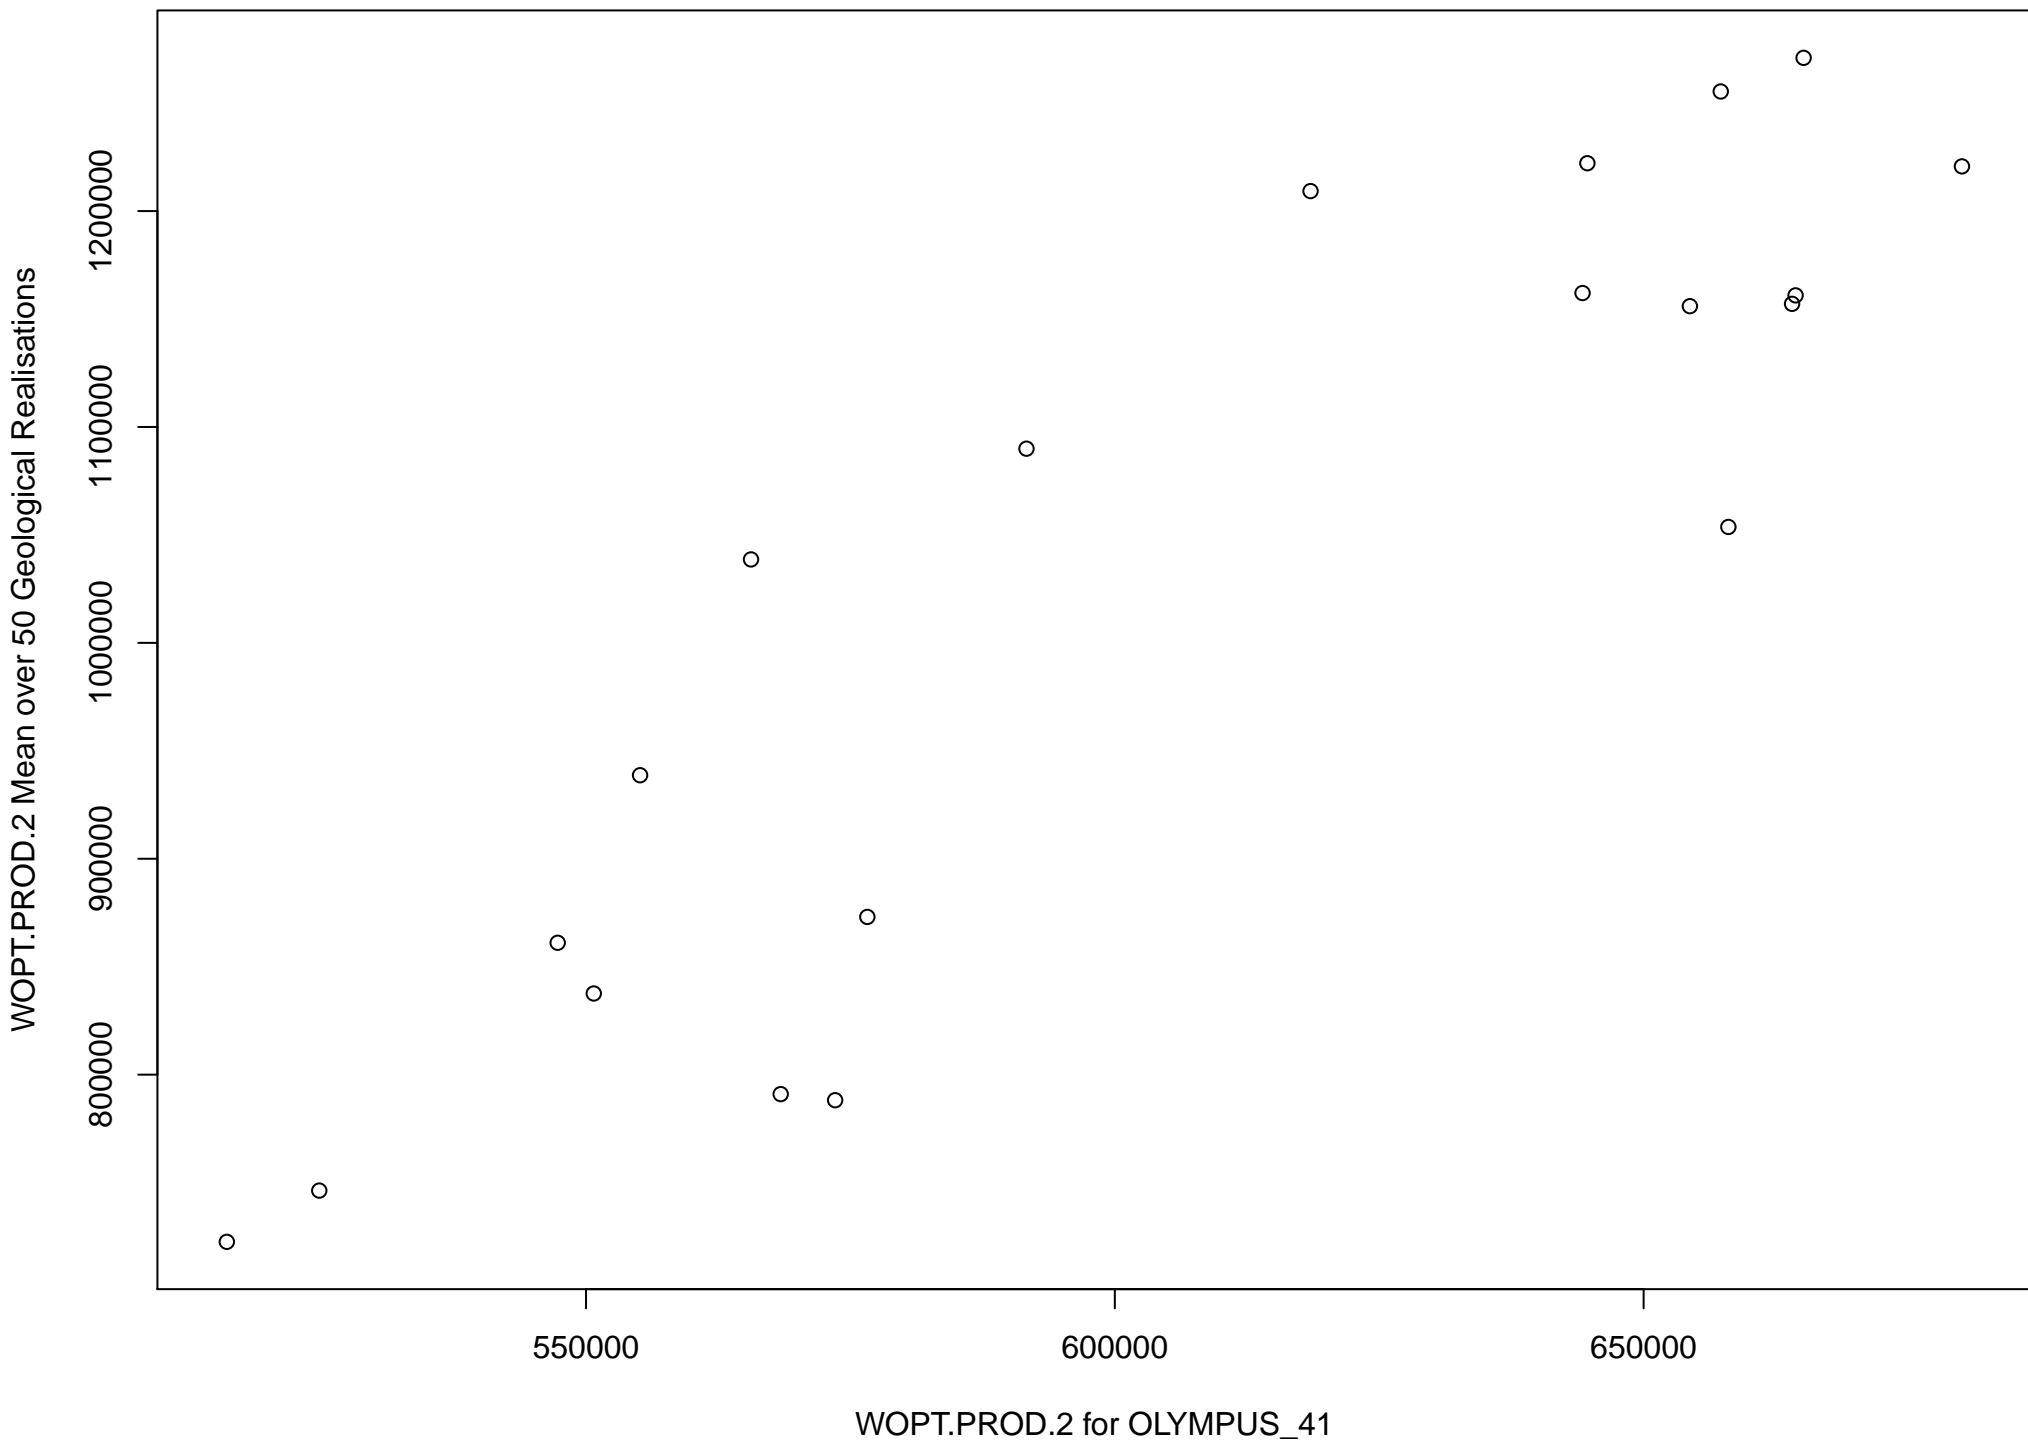

# WOPT.PROD.2 for OLYMPUS\_42

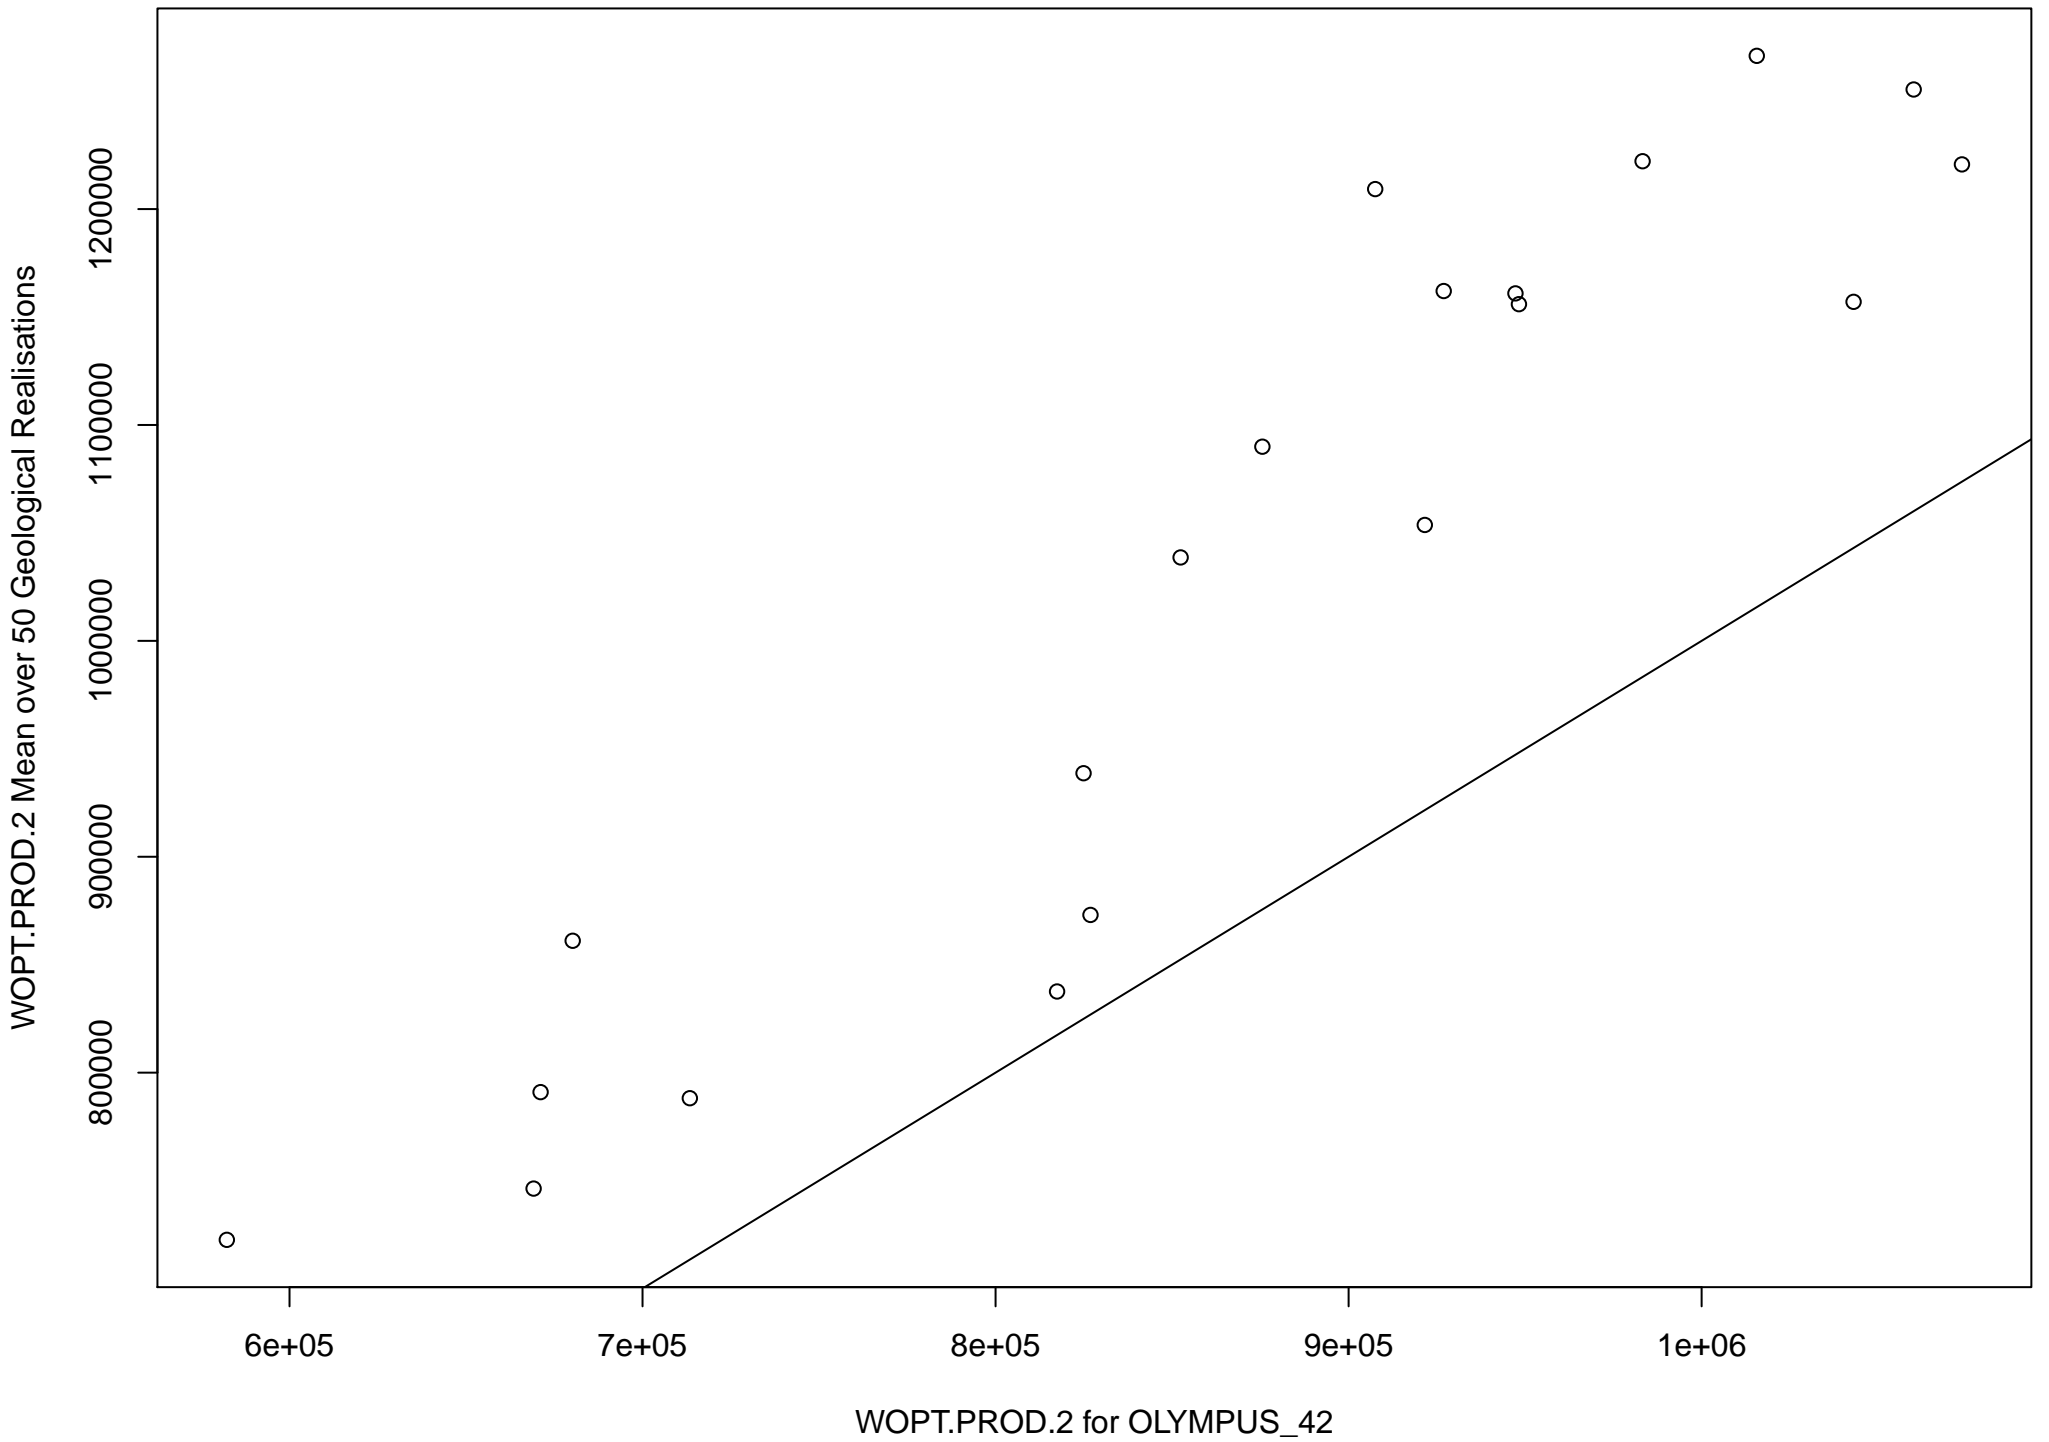

WOPT.PROD.2 for OLYMPUS\_43

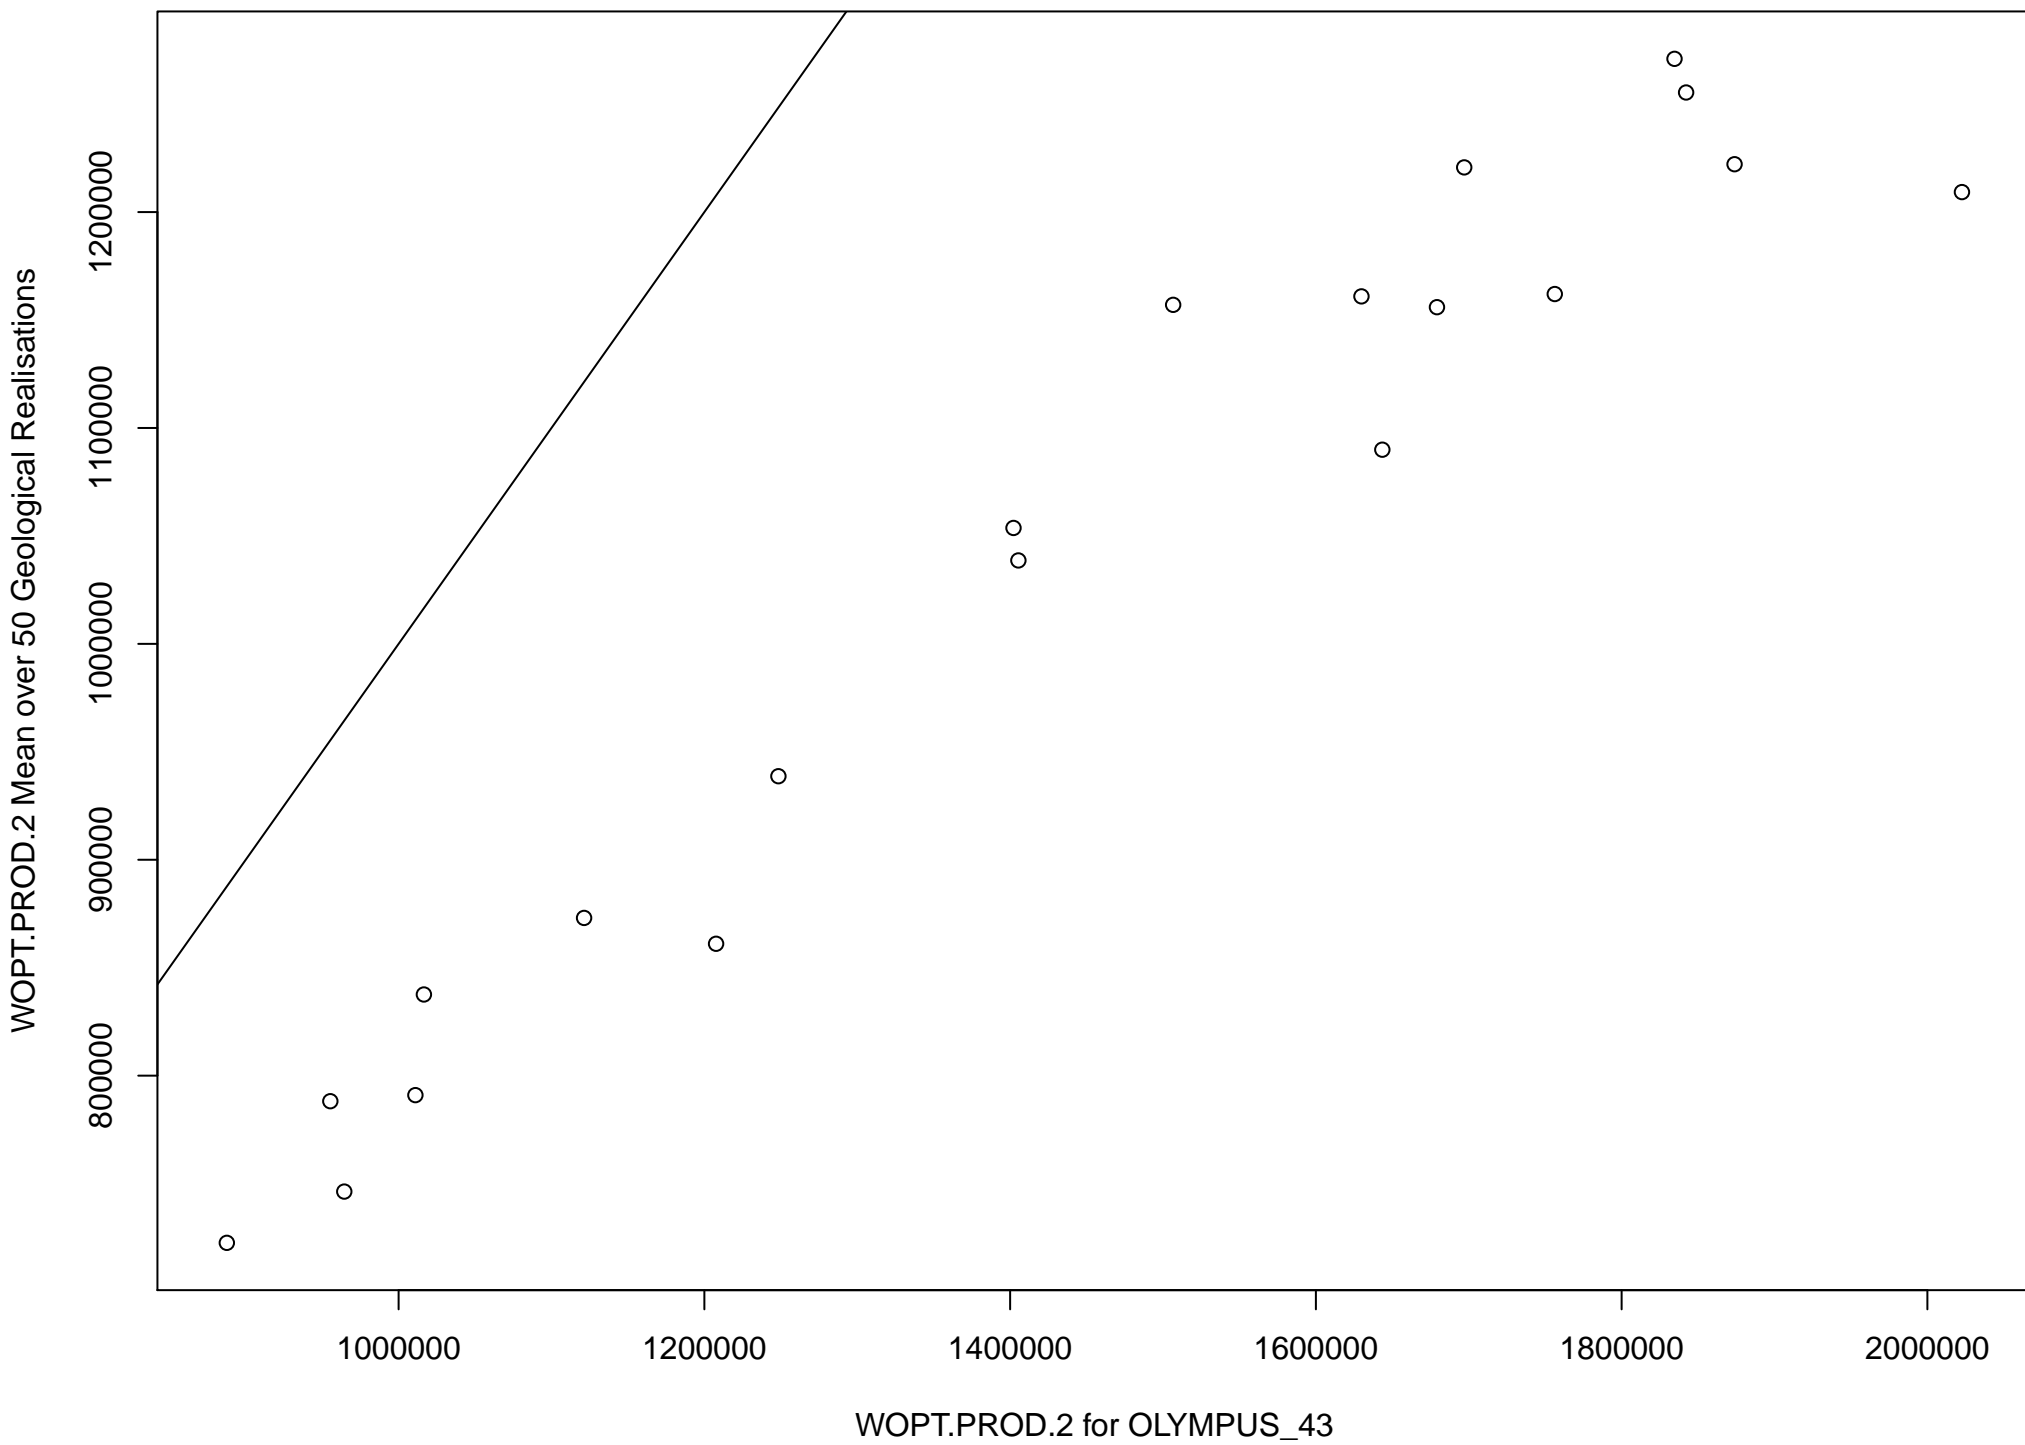

# WOPT.PROD.2 for OLYMPUS\_44

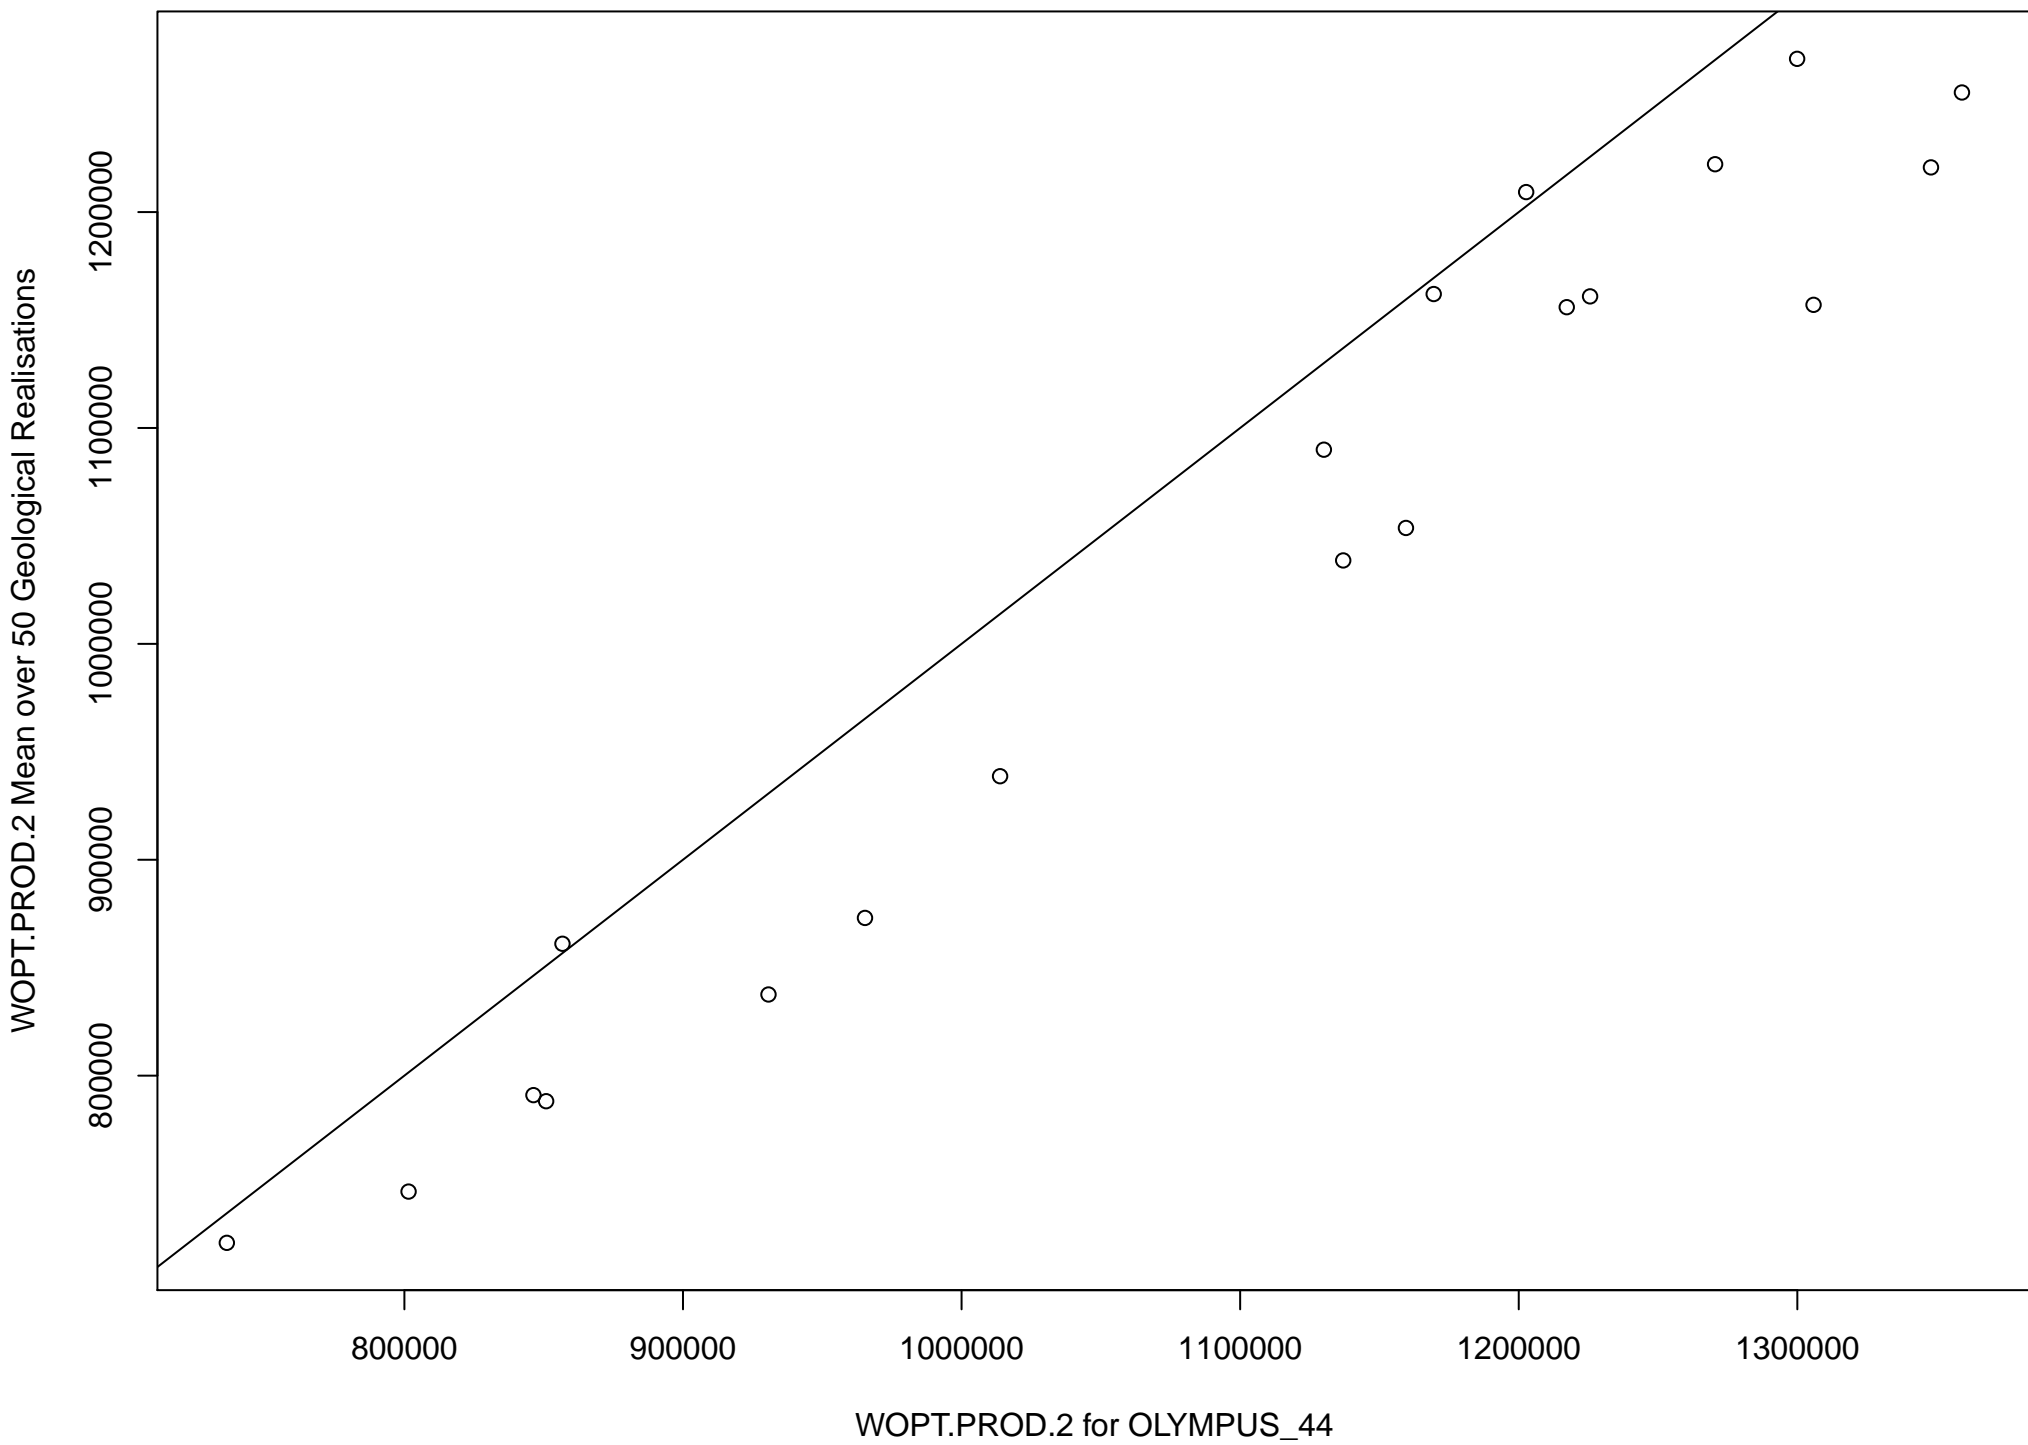

WOPT.PROD.2 for OLYMPUS\_45

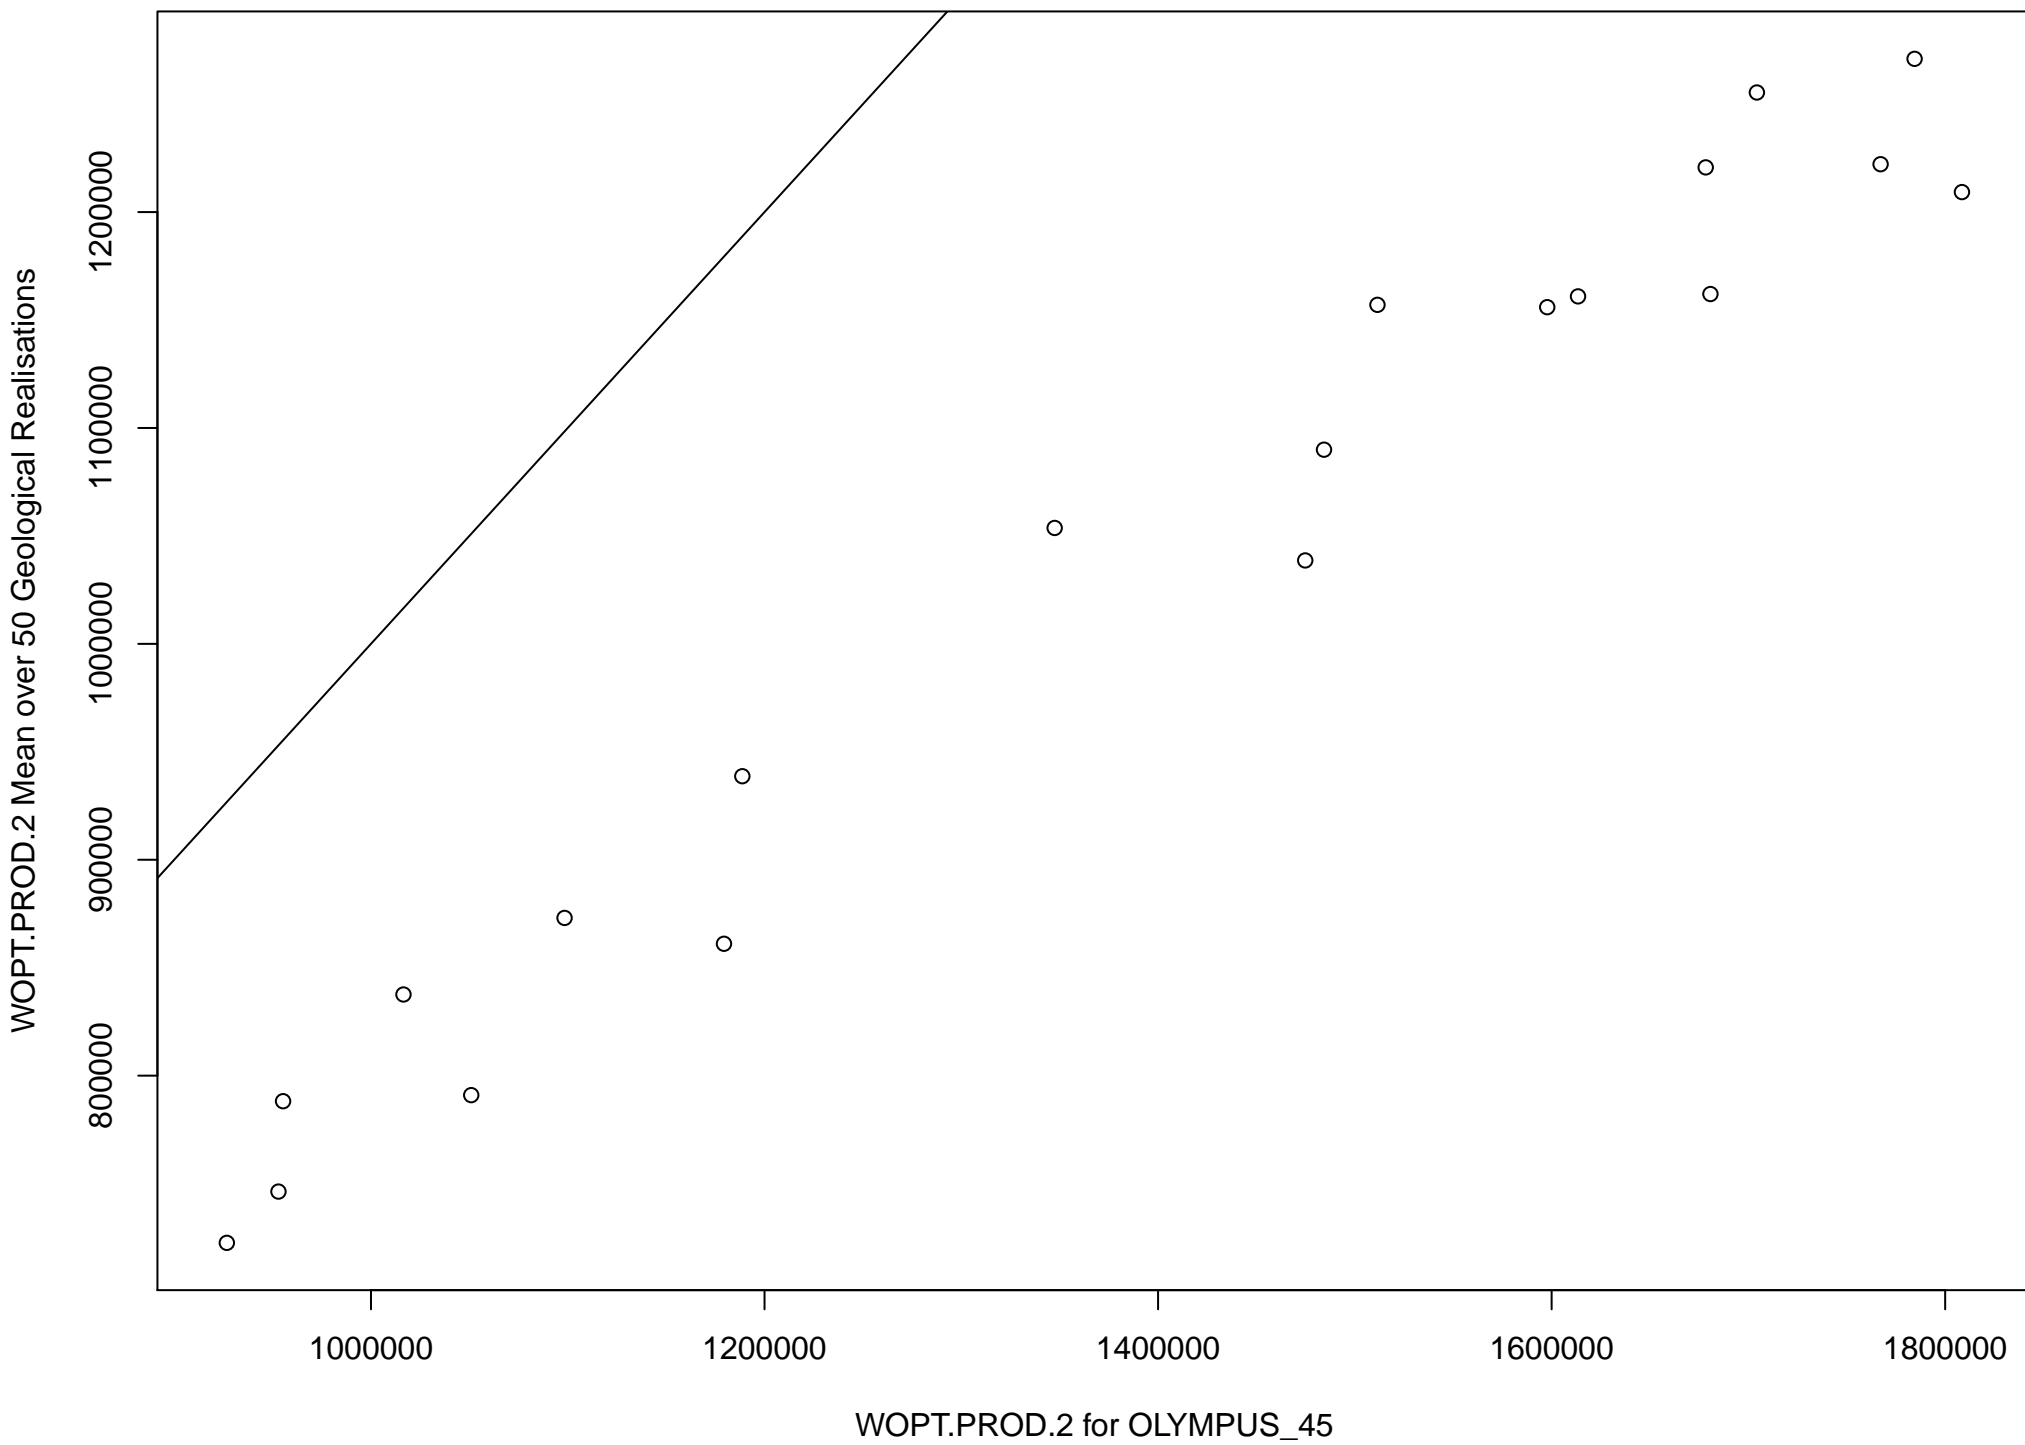

# WOPT.PROD.2 for OLYMPUS\_46

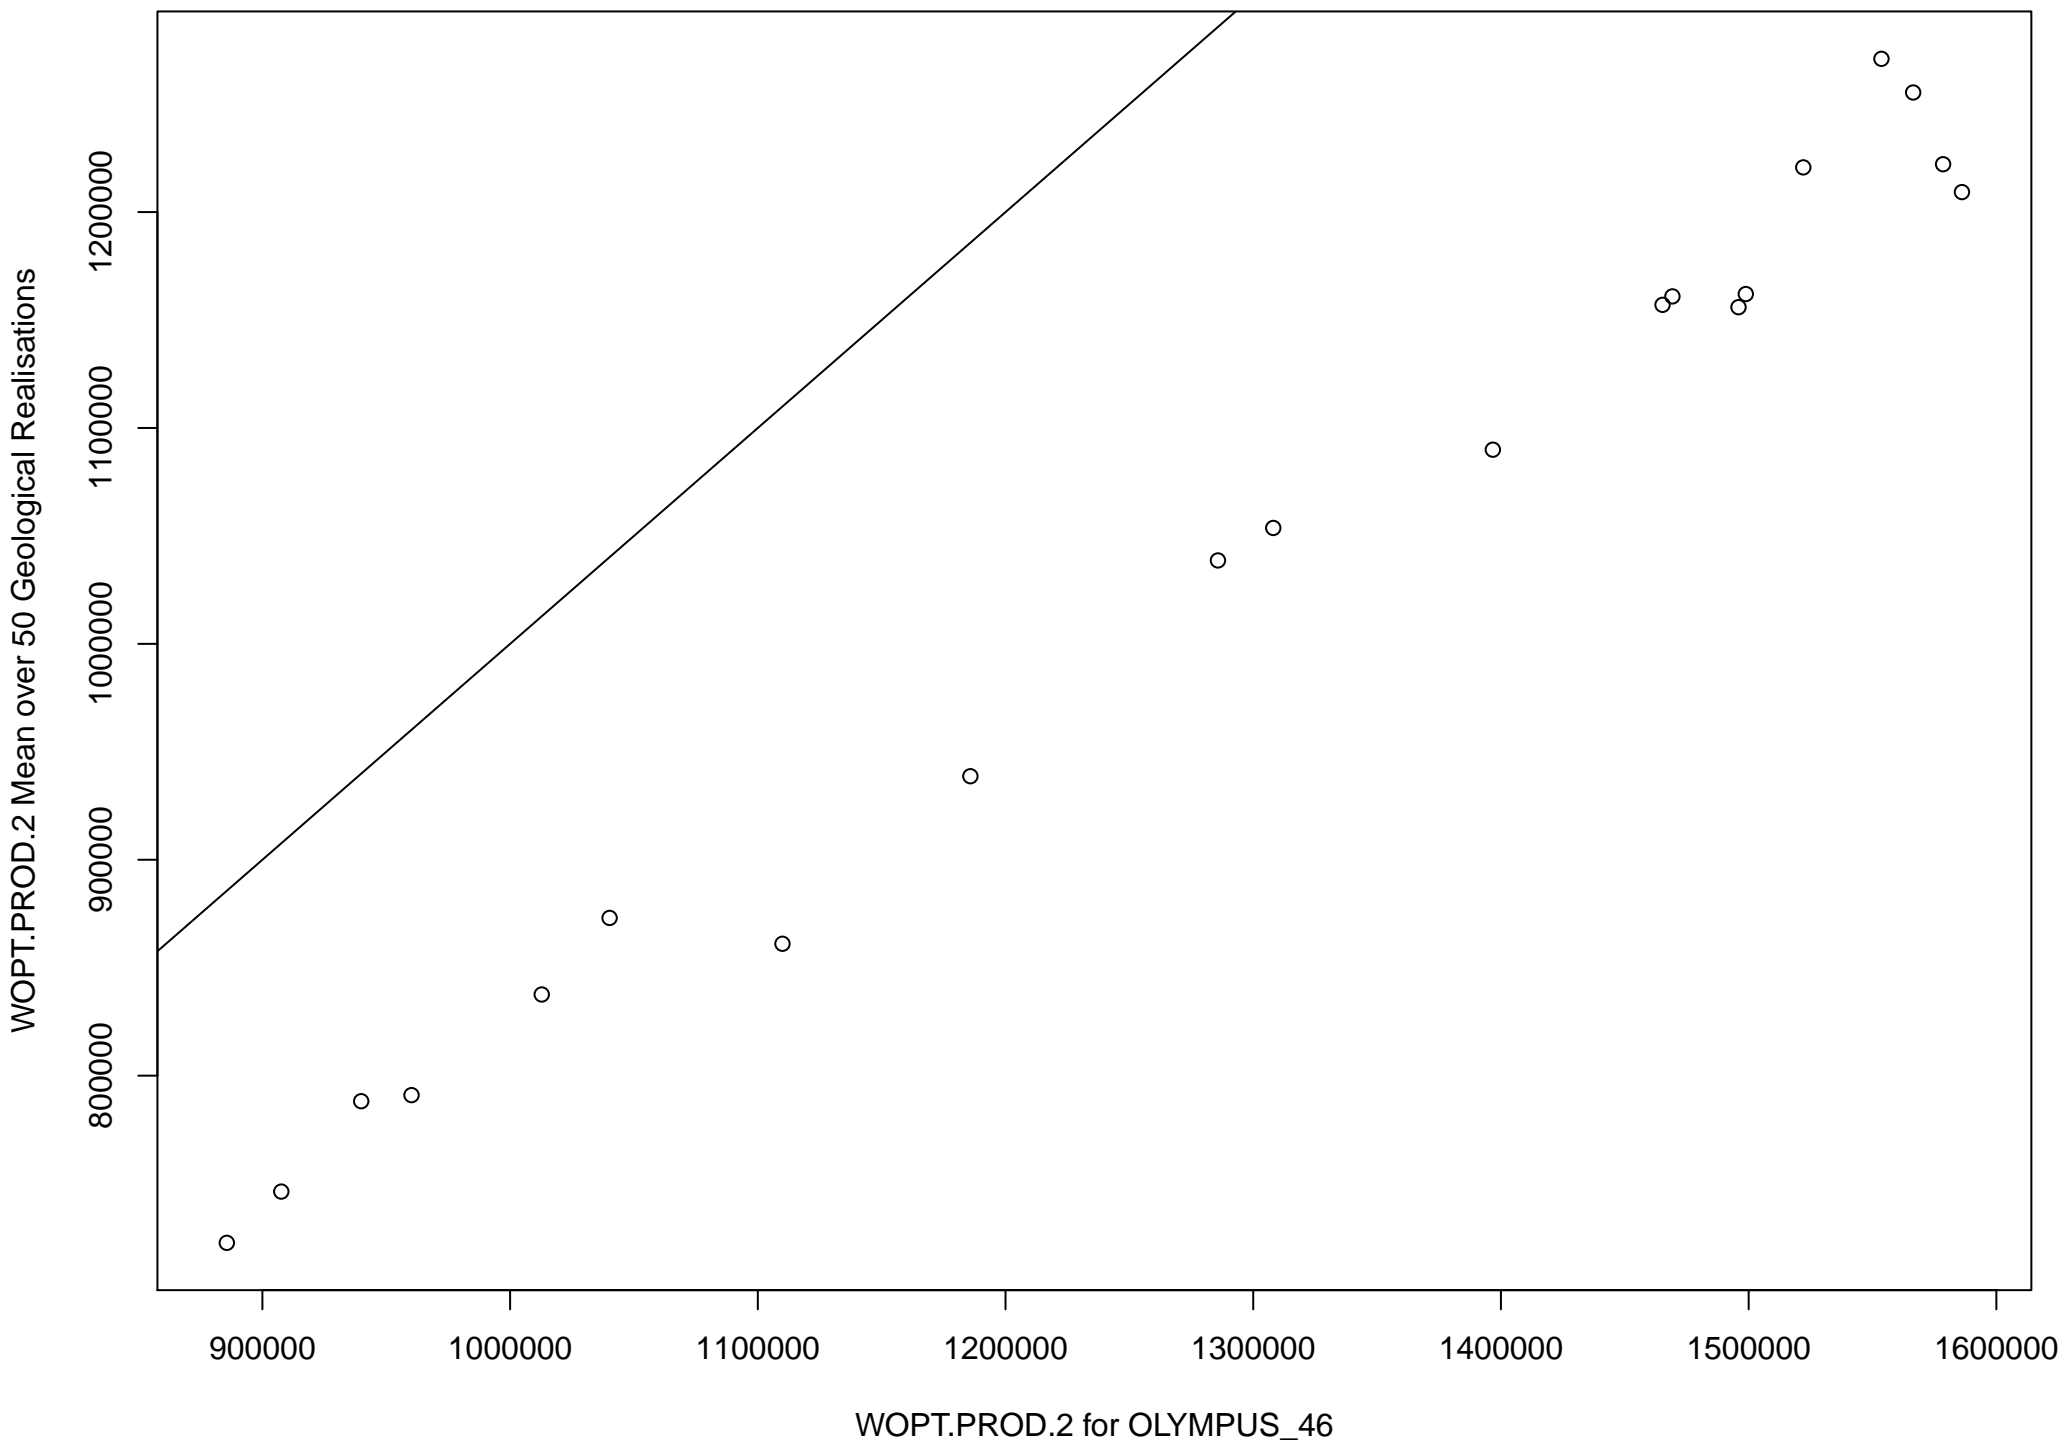

WOPT.PROD.2 for OLYMPUS\_47

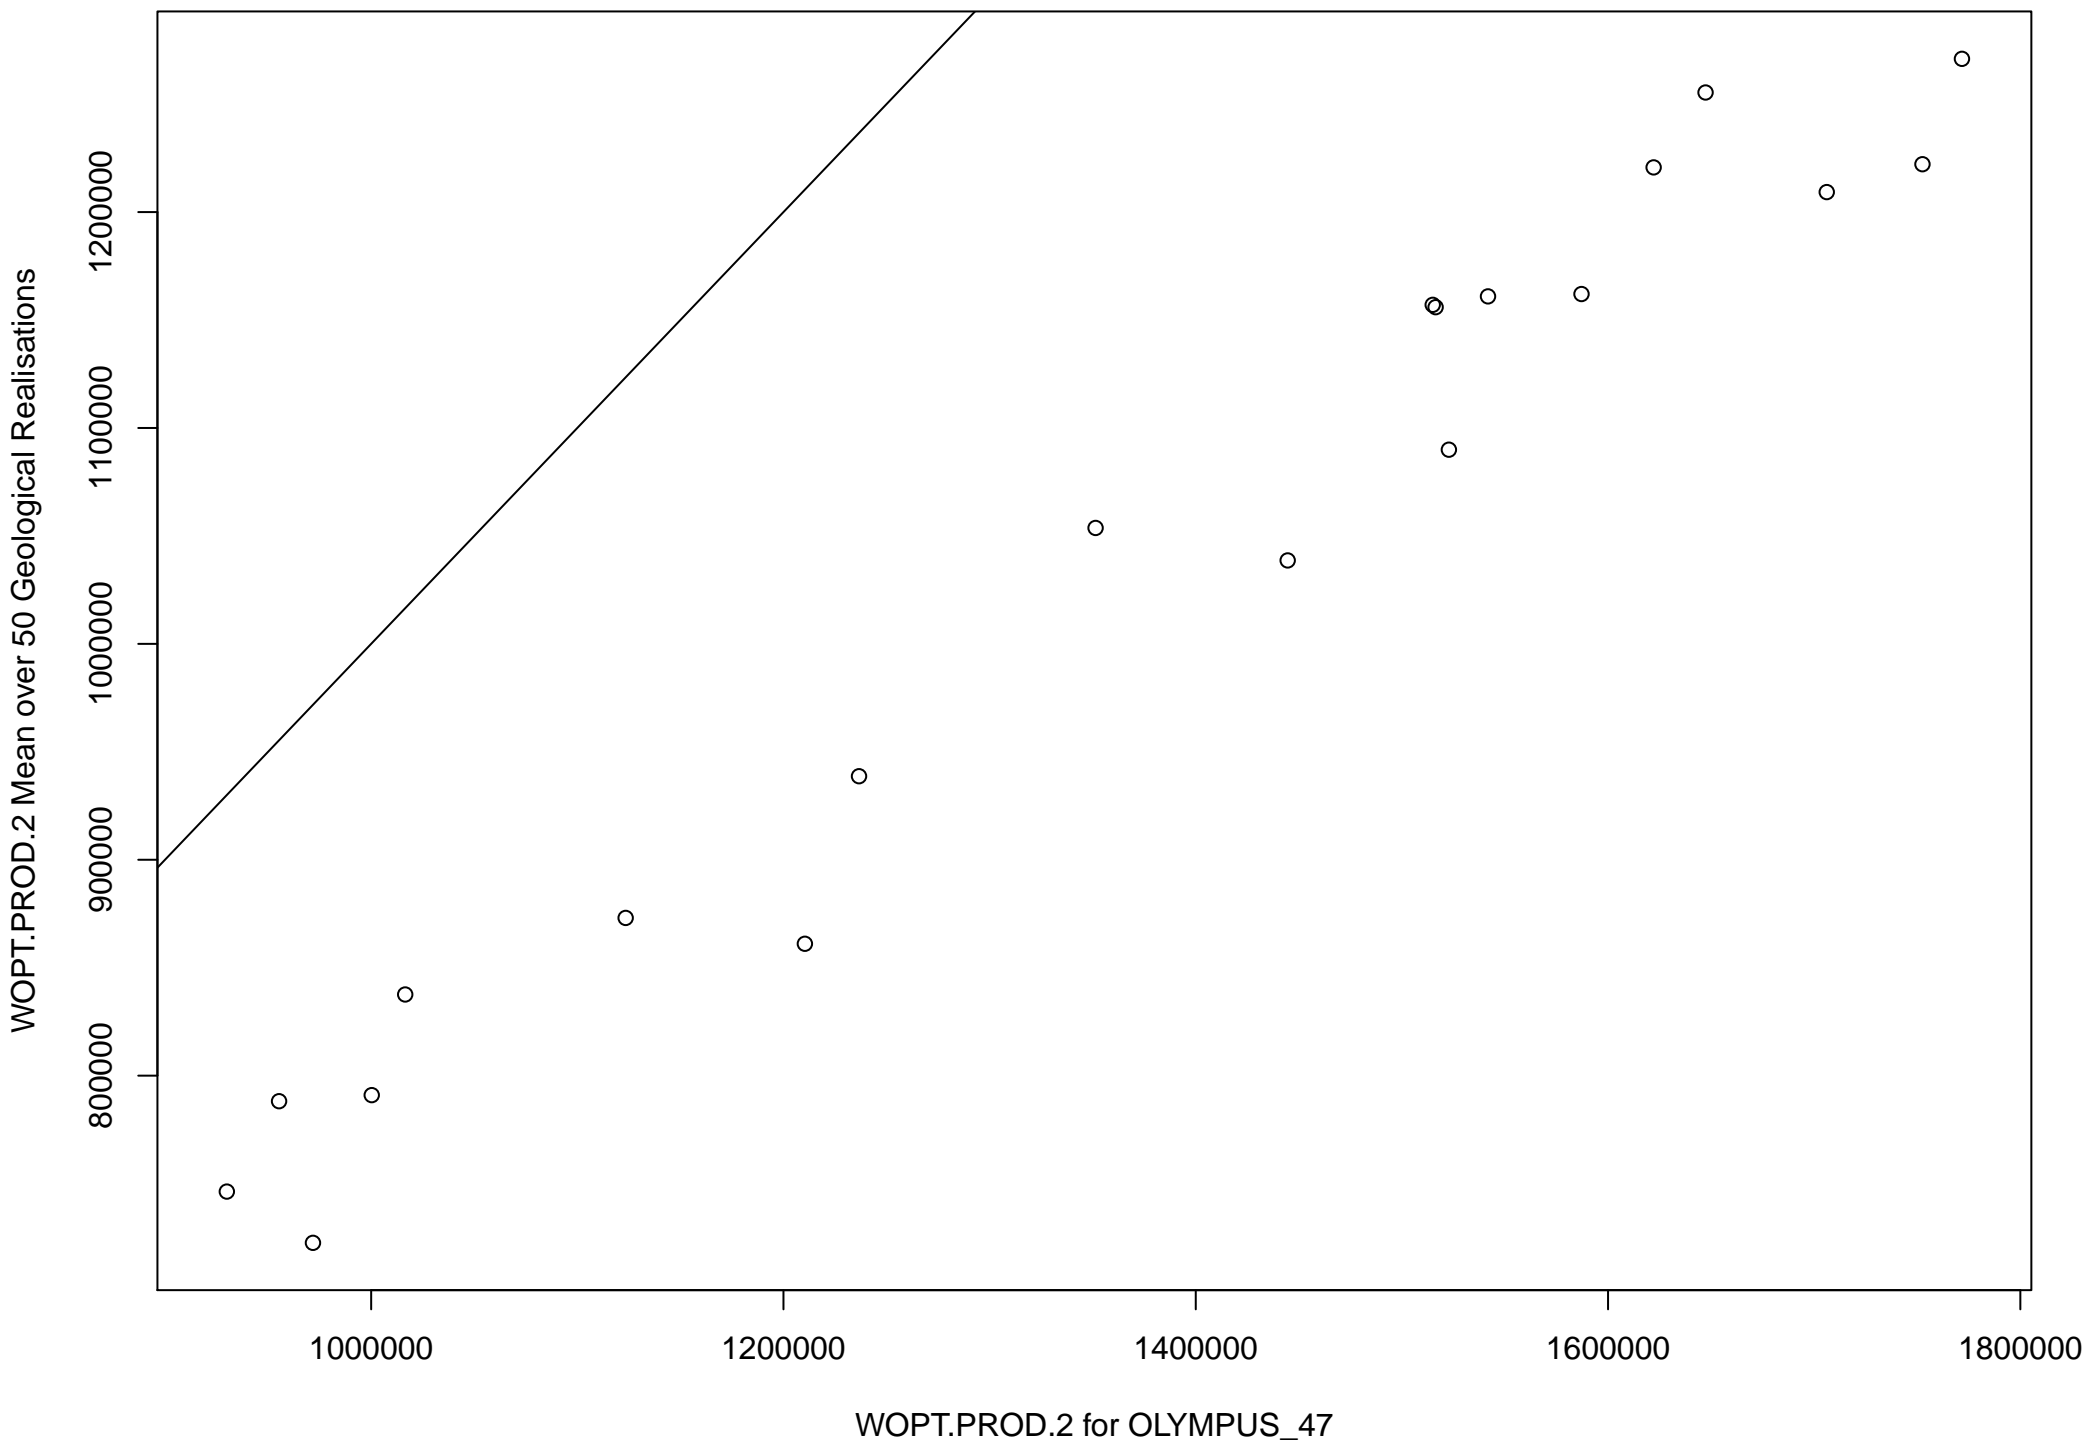

# WOPT.PROD.2 for OLYMPUS\_48

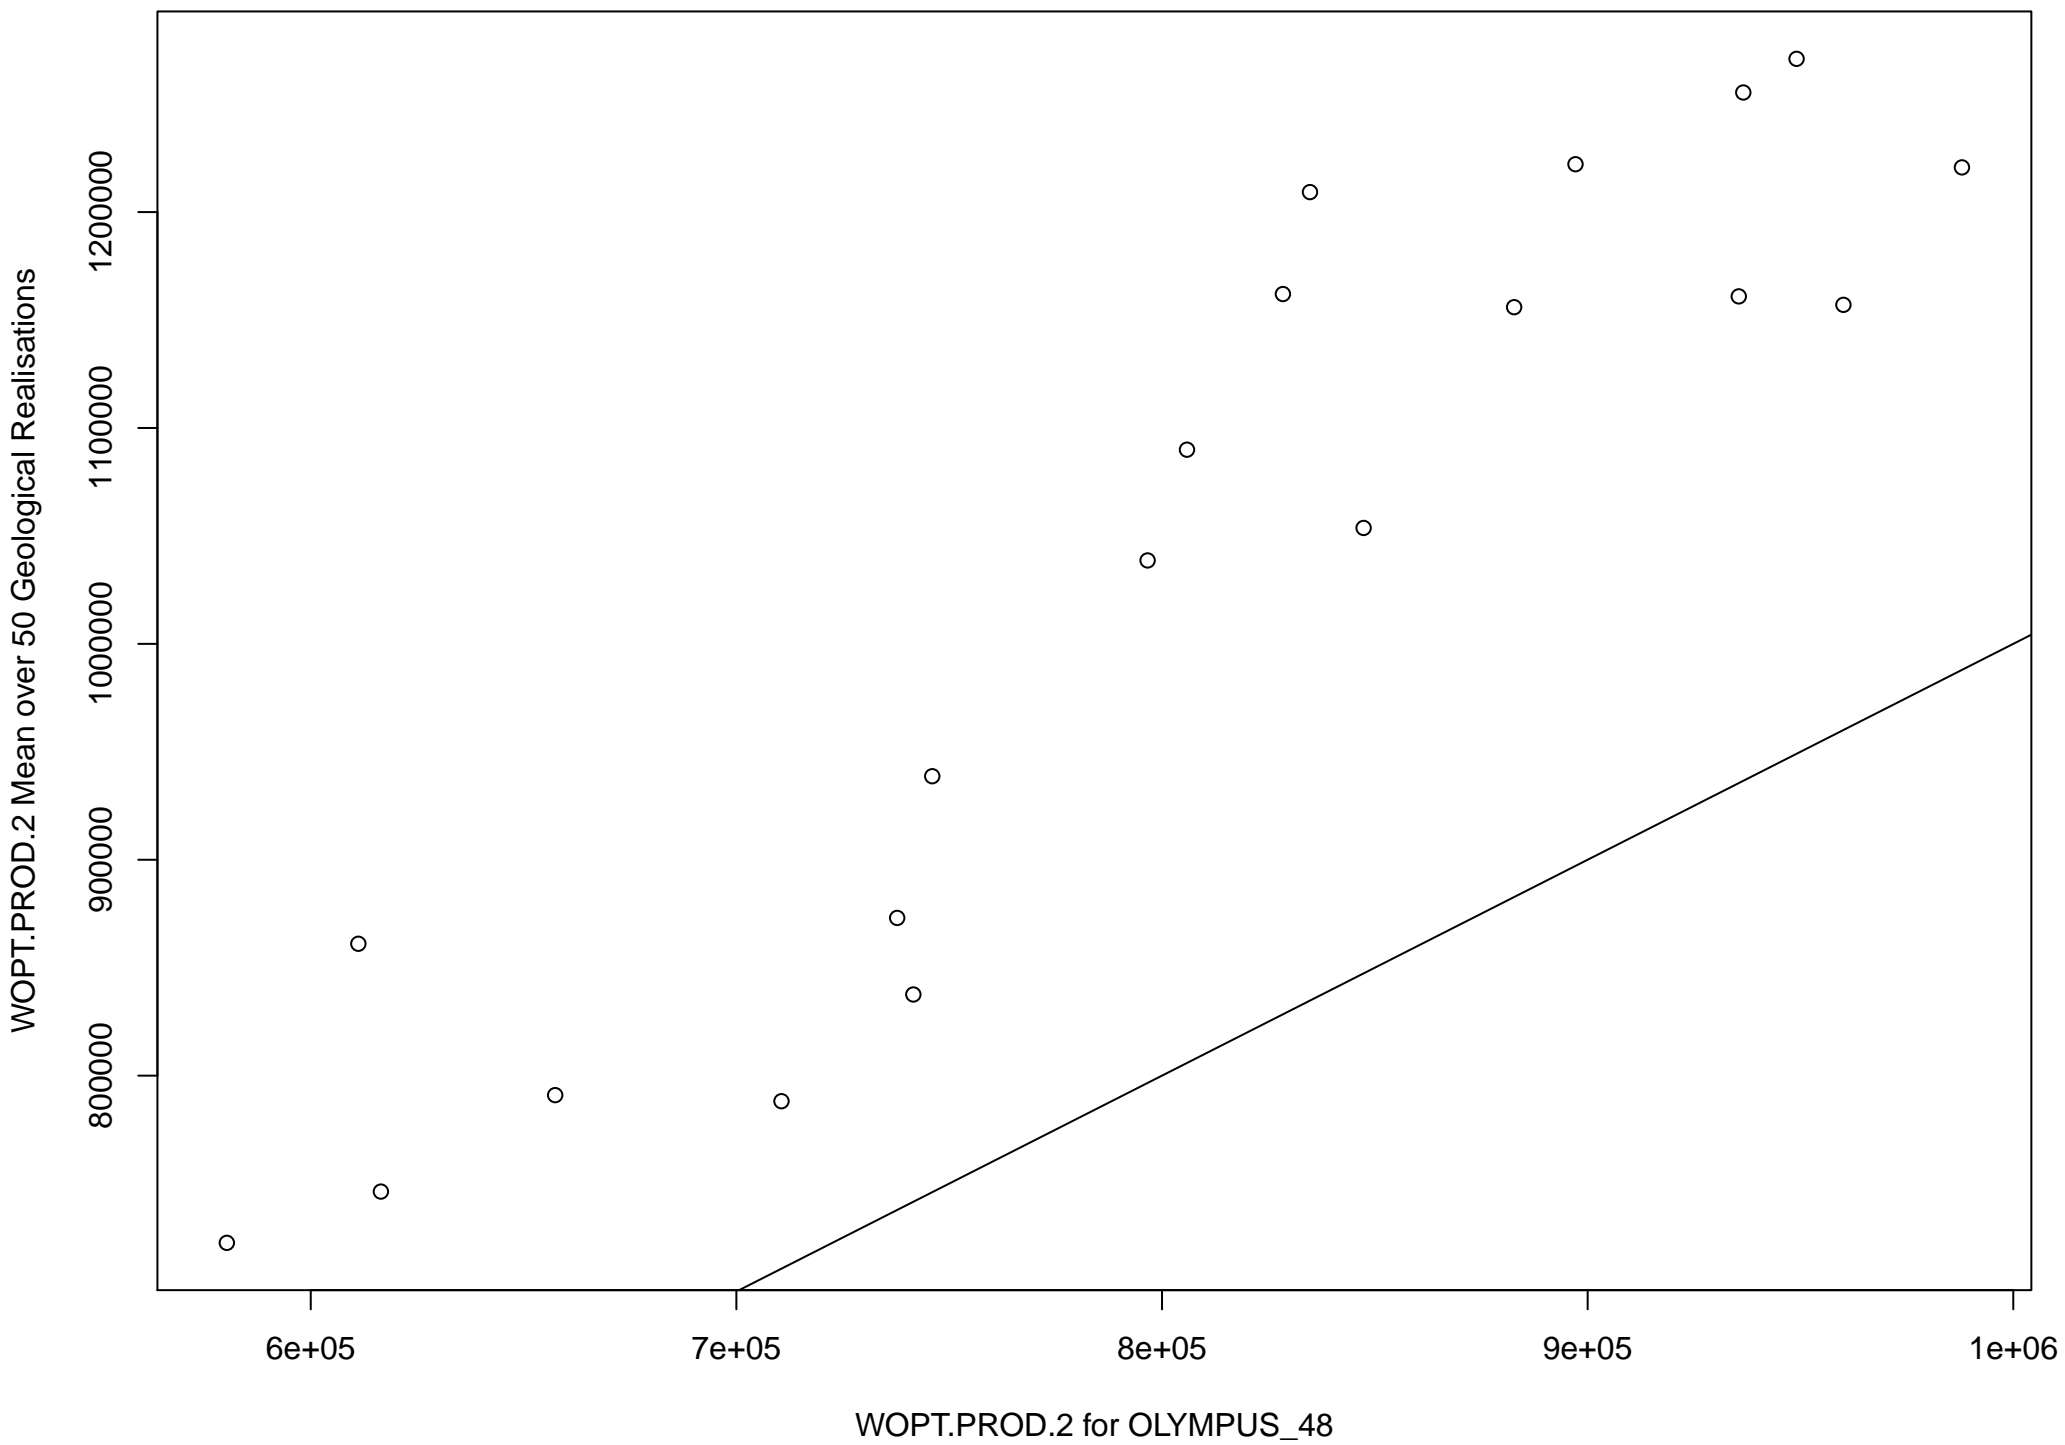



WOPT.PROD.2 for OLYMPUS\_49

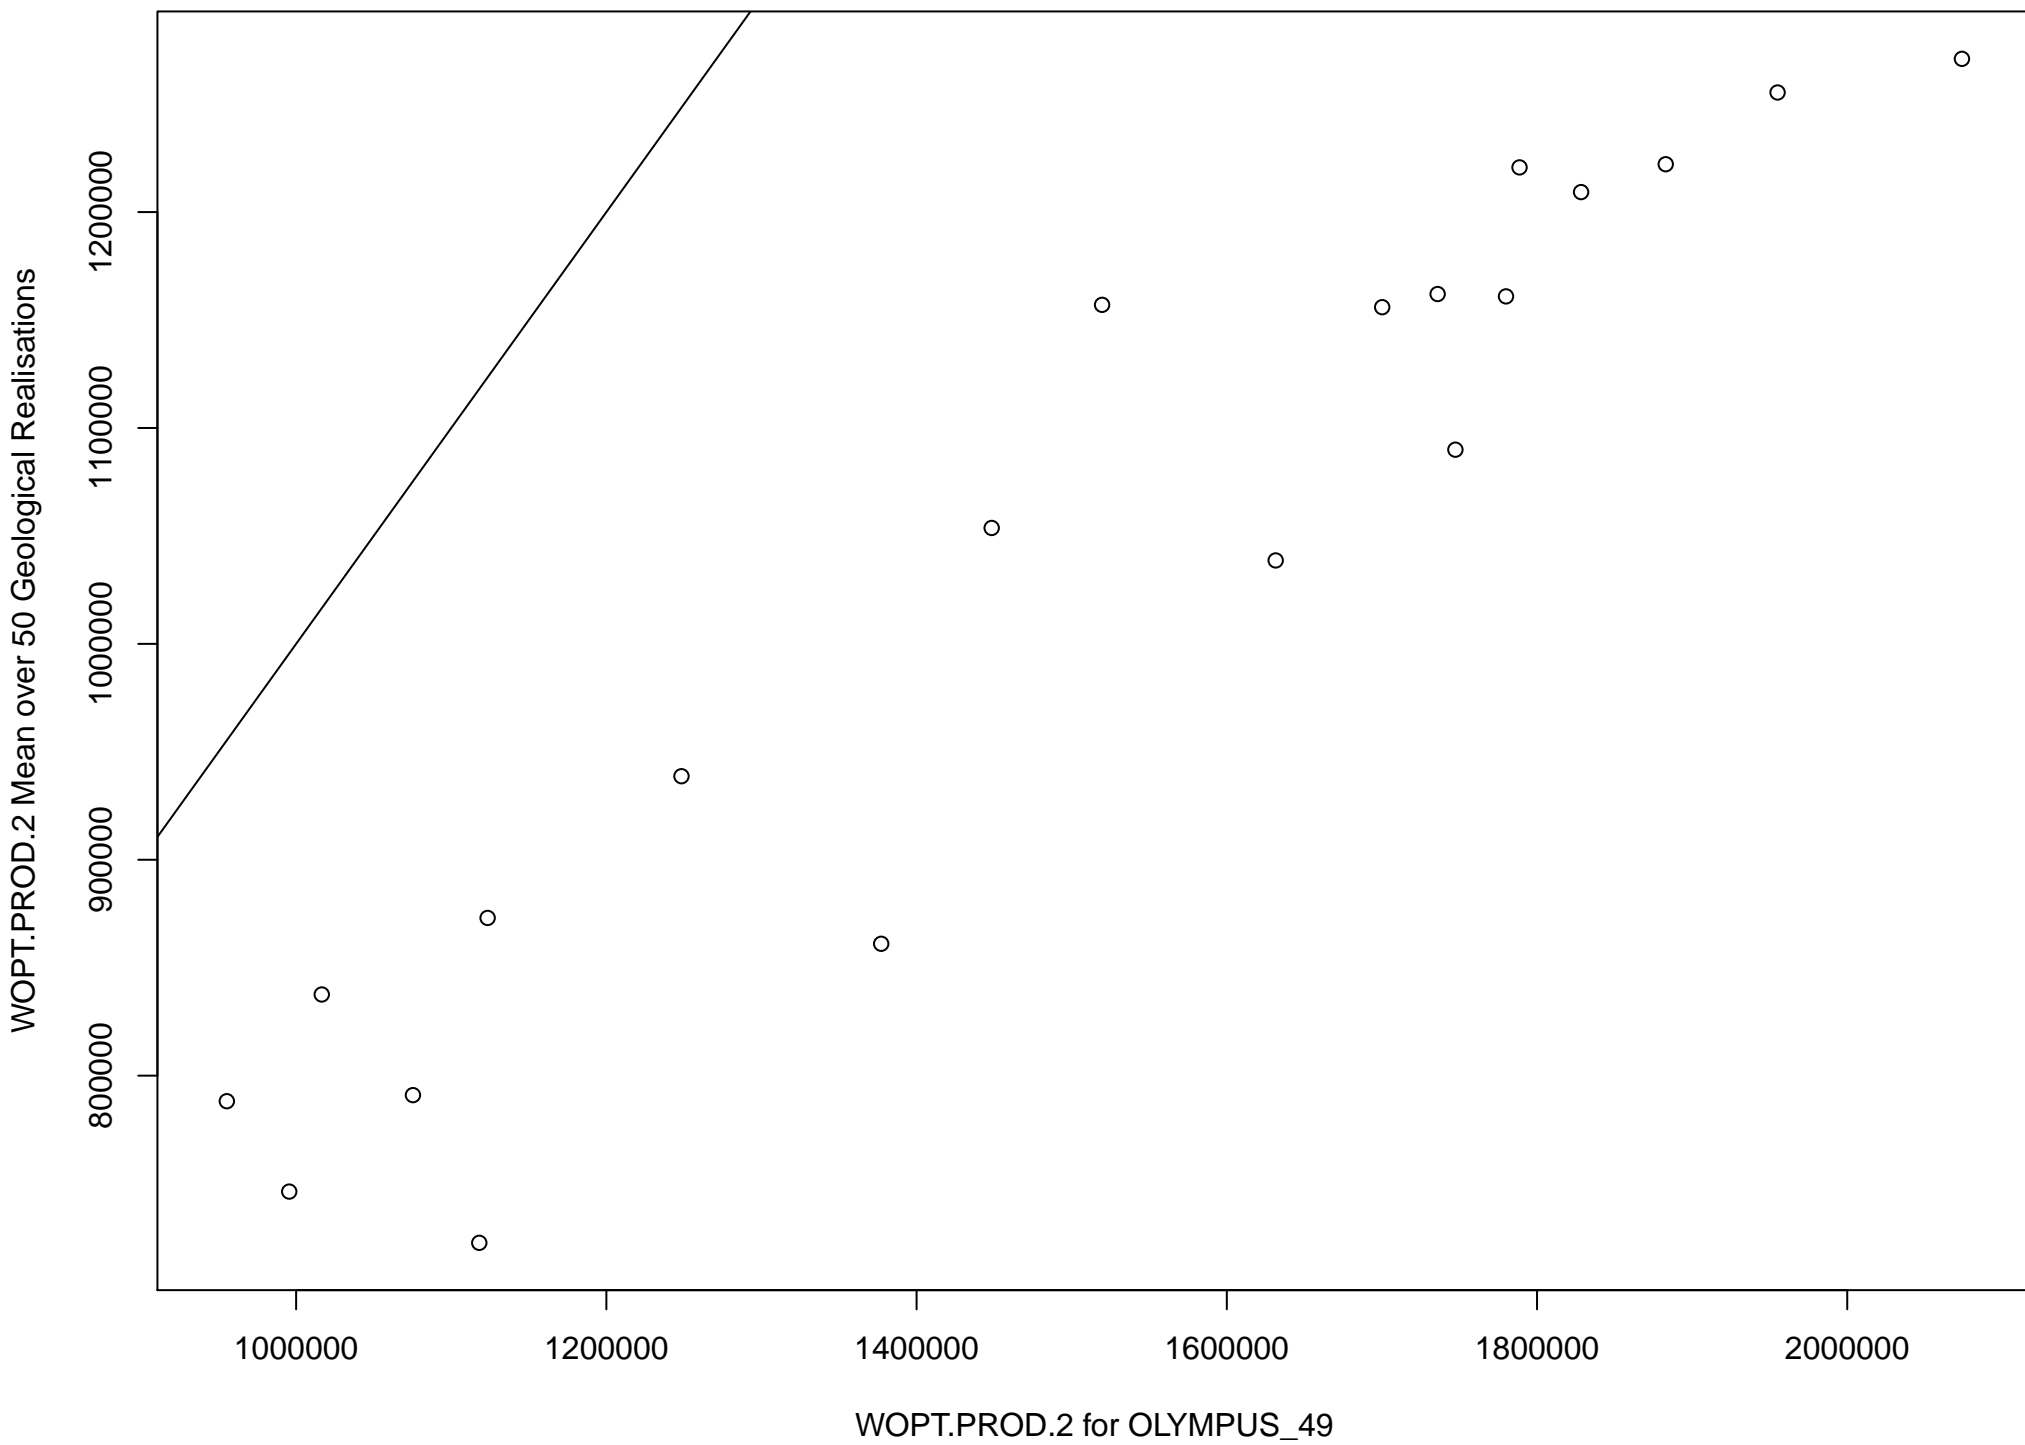

# WOPT.PROD.2 for OLYMPUS\_50

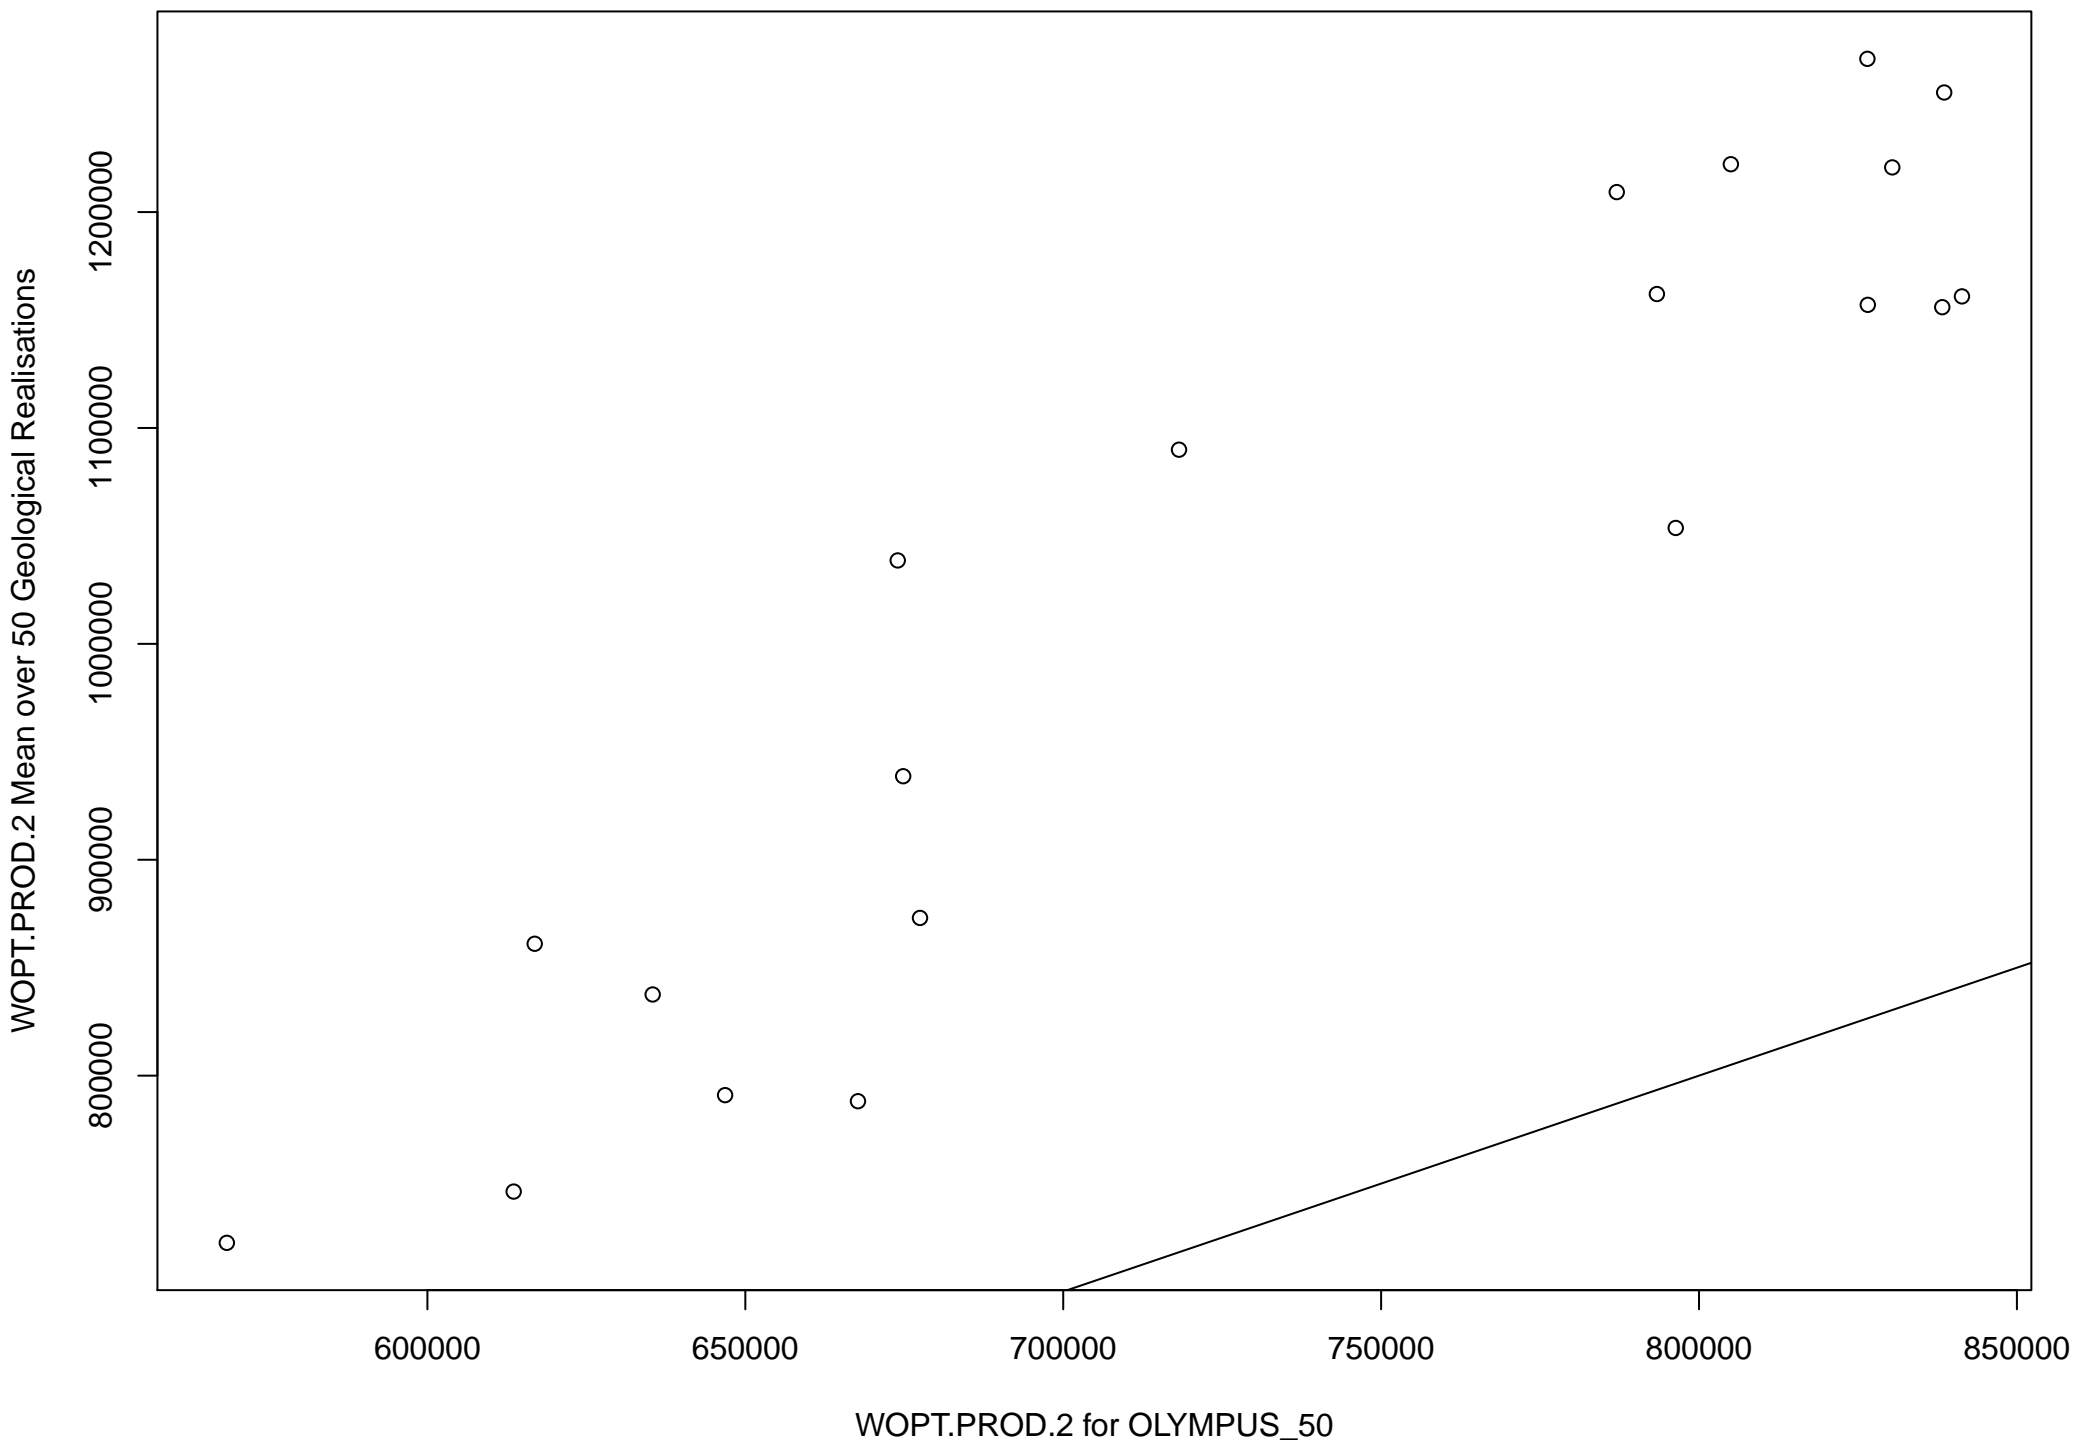

Supplement: Supplementary file 6 [file WOPTPROD2-Mean-vs-Model-Output-all-Models.pdf]
